# Supplementary material for: Distinguishing Legendrian knots with trivial orientation-preserving symmetry group
Source: arXiv:1810.06460 ancillary file (2021-09-14)

# Relations

$$x_{32,28,0,0} = x_{0,0,3,13}$$

(1)

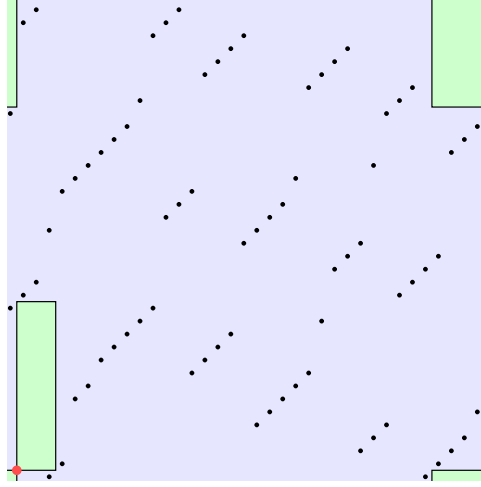

$$x_{33,28,0,1} = x_{0,1,4,13}$$

(2)

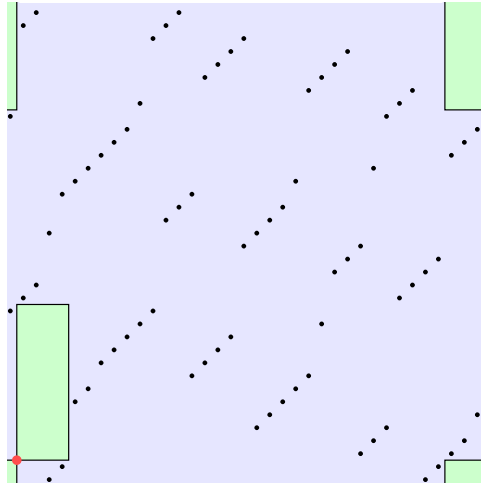

$$x_{34,28,0,2} = 0$$

(3)

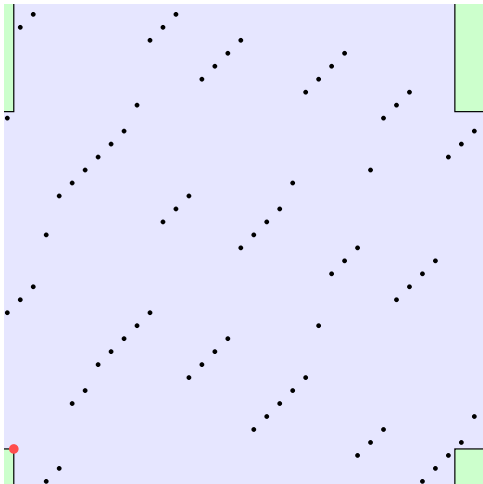

$$x_{35,28,0,4} = 0$$

(4)

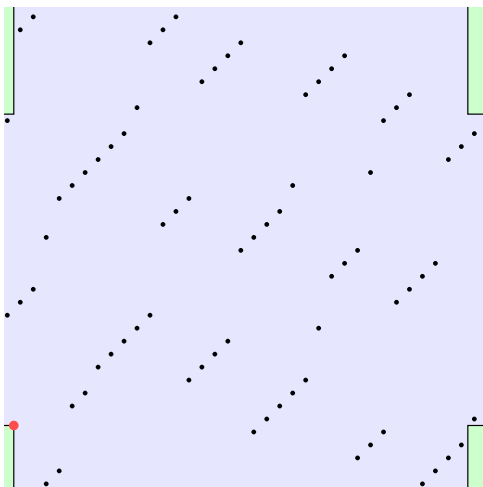

$$0 = x_{0,6,5,13}$$

(5)

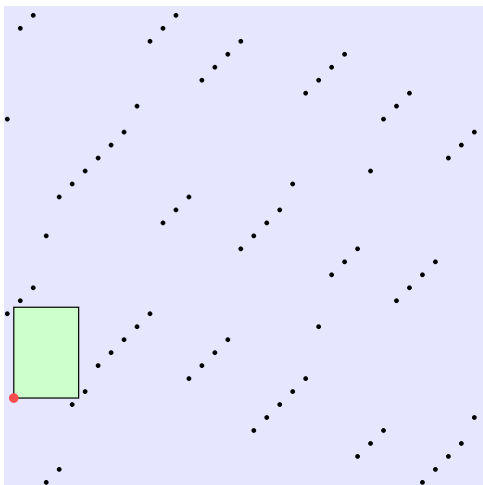

$$0 = x_{0,7,6,13} \tag{6}$$

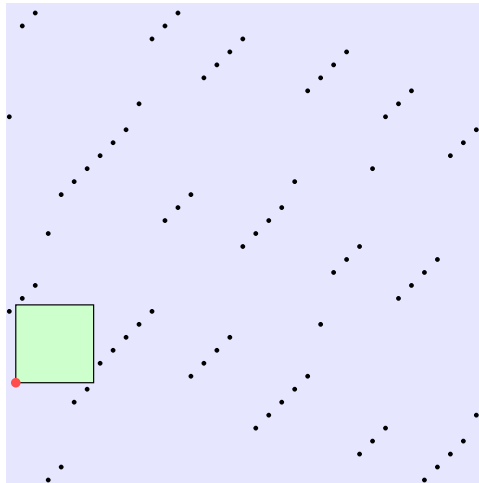

$$0 = x_{0,9,7,13} \tag{7}$$

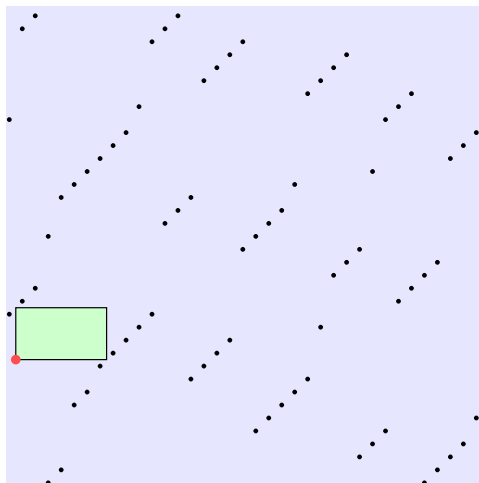

$$0 = x_{0,10,8,13} \tag{8}$$

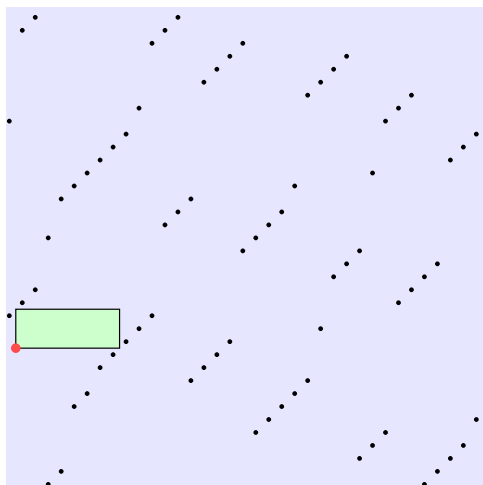

$$0 = x_{0,11,9,13}$$

(9)

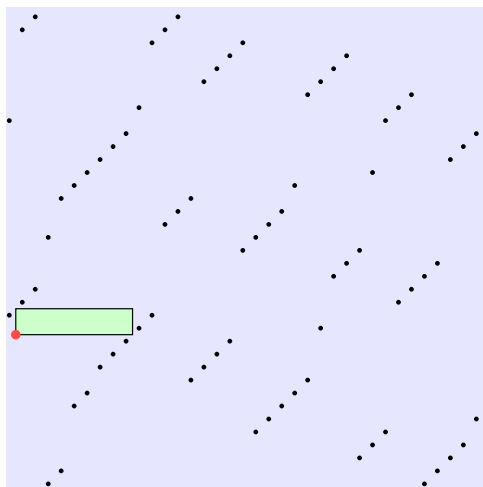

$$x_{36,28,0,12} = x_{0,12,10,13}$$

(10)

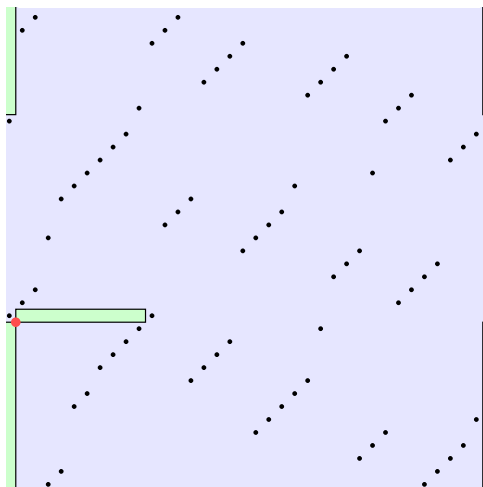

$$\begin{aligned}
& x_{30,13,0,14} + x_{31,13,0,15} + x_{32,13,0,16} + x_{33,13,0,24} + x_{34,13,0,25} + x_{35,13,0,26} + x_{36,13,0,27} = \\
& = x_{0,0,3,13} + x_{0,1,4,13} + x_{0,6,5,13} + x_{0,7,6,13} + x_{0,9,7,13} + x_{0,10,8,13} + x_{0,11,9,13} + x_{0,12,10,13} + x_{0,35,1,13} + x_{0,36,2,13} \quad (11)
\end{aligned}$$

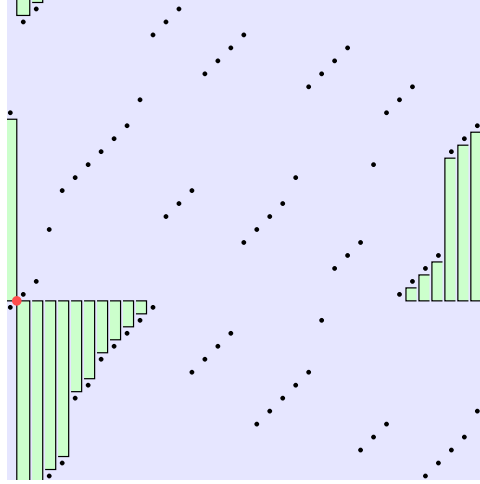

$$x_{30,13,0,14} = x_{0,14,1,34} \quad (12)$$

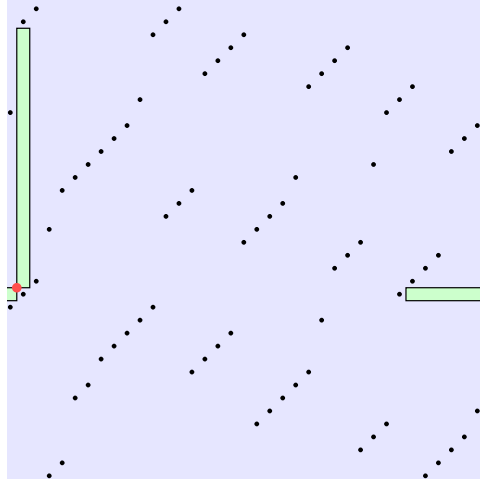

$$x_{31,13,0,15} = x_{0,15,2,34} \quad (13)$$

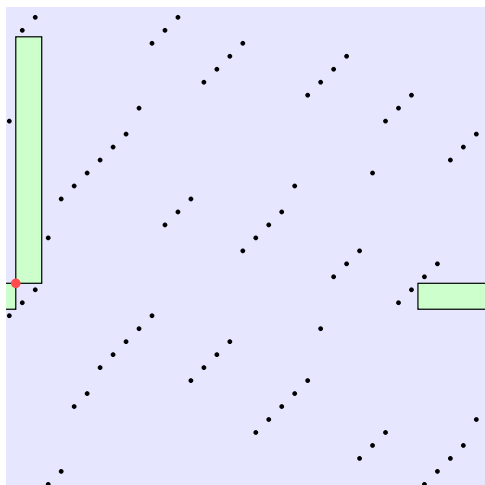

$$x_{32,13,0,16} = 0$$

(14)

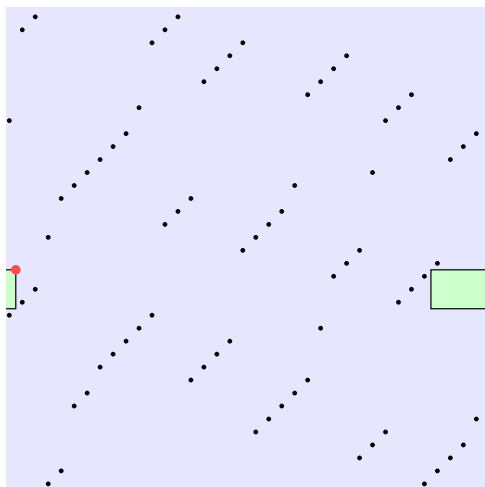

$$0 = x_{0,19,3,34}$$

(15)

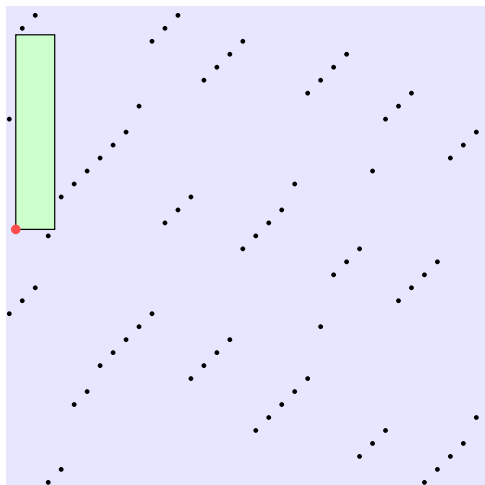

$$0 = x_{0,22,4,34}$$

(16)

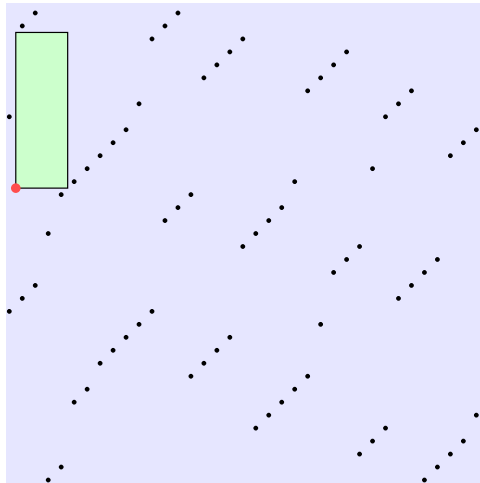

$$0 = x_{0,23,5,34}$$

(17)

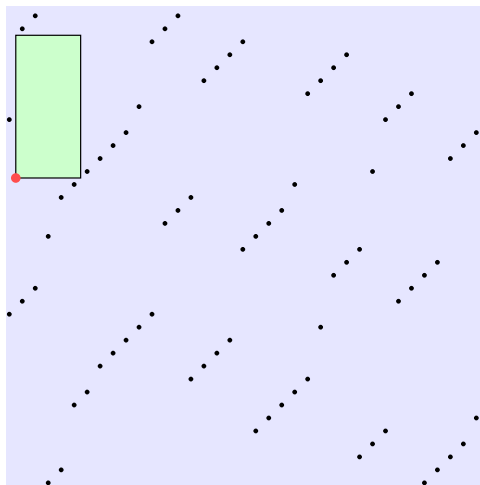

$$x_{33,13,0,24} = x_{0,24,6,34}$$

(18)

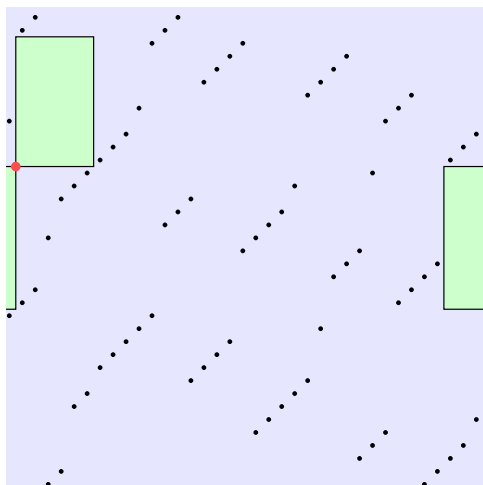

$$x_{34,13,0,25} = x_{0,25,7,34}$$

(19)

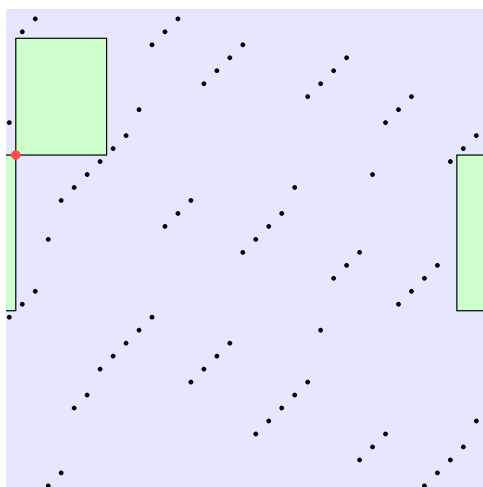

$$x_{35,13,0,26} = x_{0,26,8,34}$$

(20)

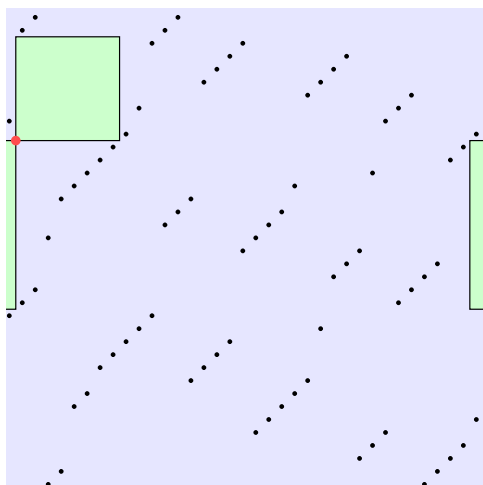



$$x_{36,13,0,27} = x_{0,27,9,34} + x_{0,27,28,28} \quad (21)$$

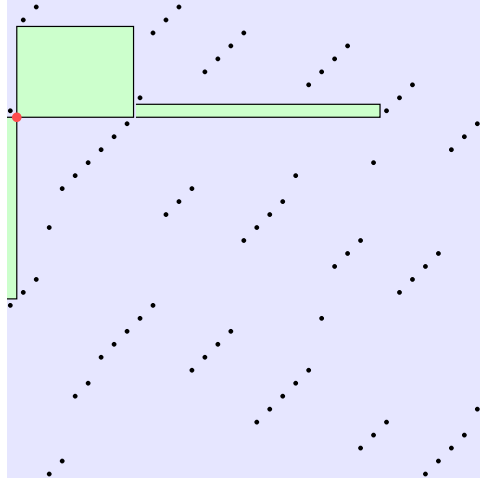

$$x_{31,28,0,36} + x_{32,28,0,0} + x_{33,28,0,1} + x_{34,28,0,2} + x_{35,28,0,4} + x_{36,28,0,12} = x_{0,27,28,28} \quad (22)$$

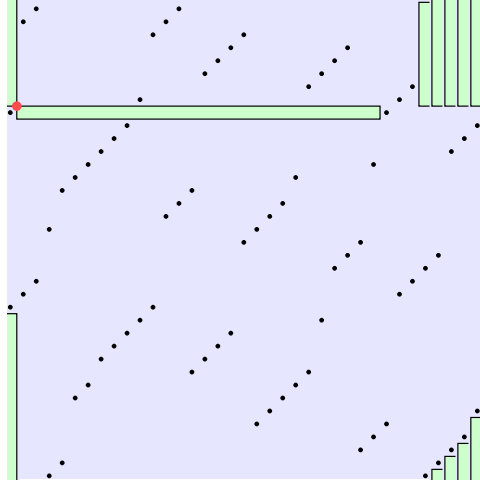

$$x_{26,30,0,36} = 0 \quad (23)$$

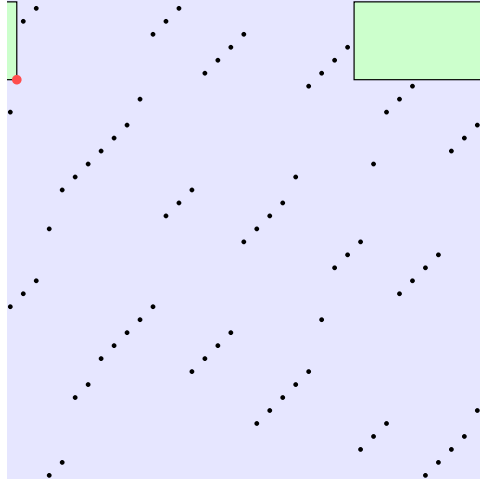

$$x_{18,33,0,36} = 0$$

(24)

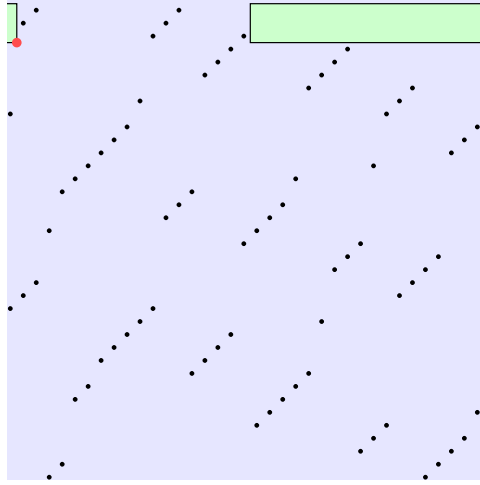

$$x_{12,34,0,35} + x_{13,34,0,36} =$$

$$= x_{0,14,1,34} + x_{0,15,2,34} + x_{0,19,3,34} + x_{0,22,4,34} + x_{0,23,5,34} + x_{0,24,6,34} + x_{0,25,7,34} + x_{0,26,8,34} + x_{0,27,9,34} \quad (25)$$

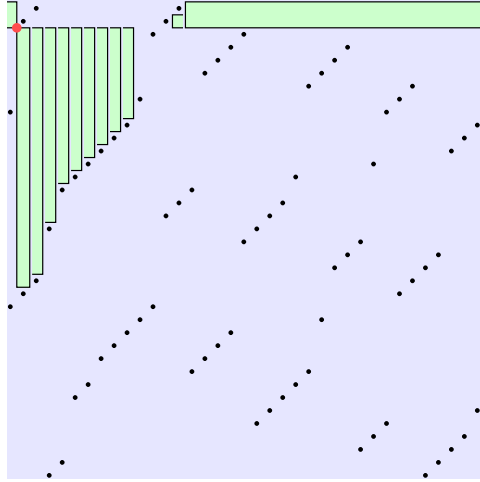

$$x_{12,34,0,35} = x_{0,35,1,13}$$

(26)

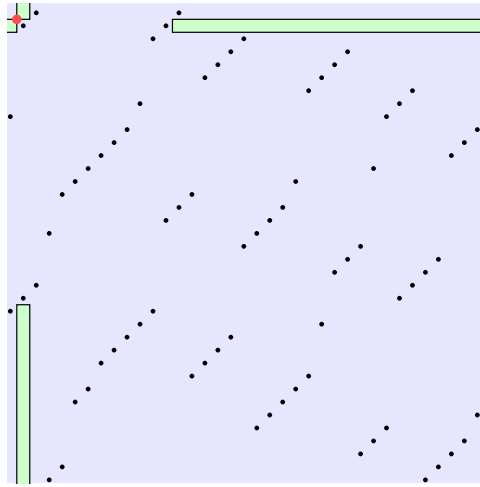

$$x_{13,34,0,36} + x_{18,33,0,36} + x_{26,30,0,36} + x_{31,28,0,36} = x_{0,36,2,13}$$

(27)

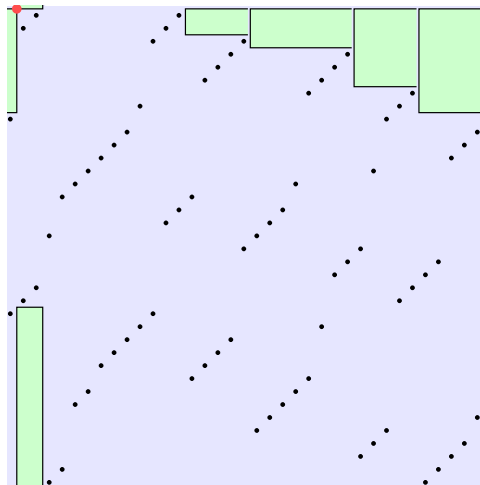

$$x_{32,35,1,0} = x_{1,0,3,14}$$

(28)

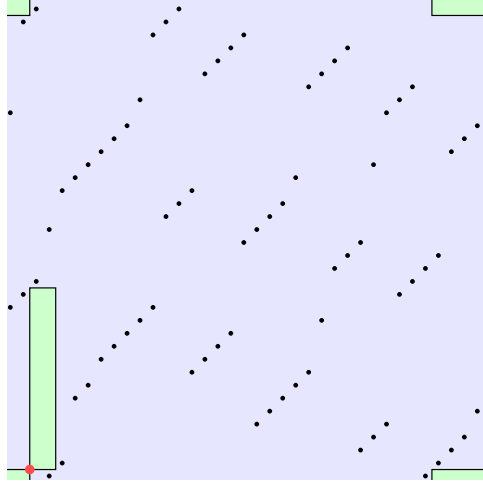

$$x_{33,35,1,1} = x_{1,1,4,14}$$

(29)

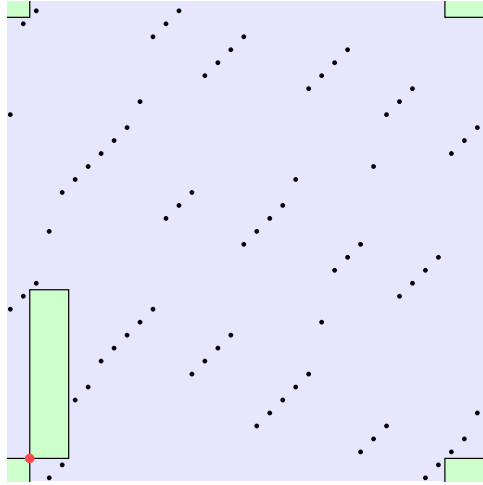

$$x_{34,35,1,2} = 0$$

(30)

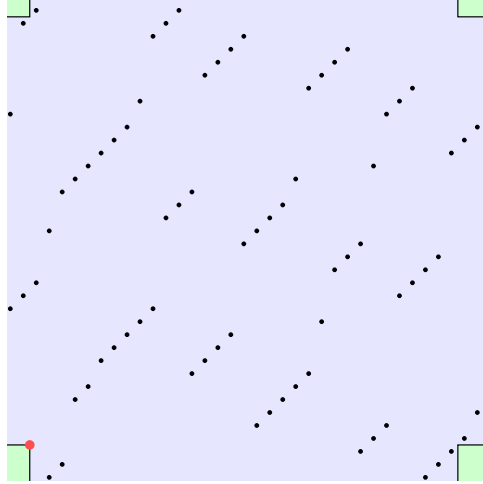

$$x_{35,35,1,4} = 0$$

(31)

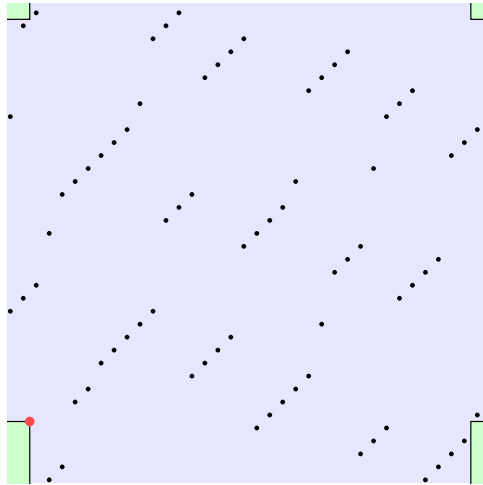

$$0 = x_{1,6,5,14}$$

(32)

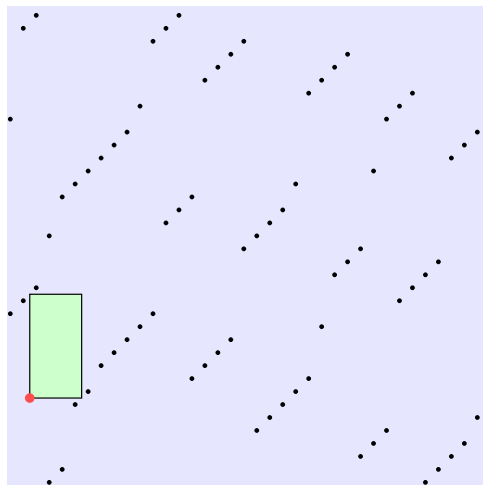

$$0 = x_{1,7,6,14} \tag{33}$$

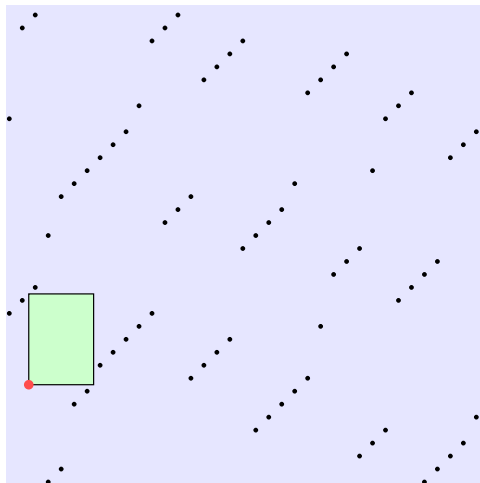

$$0 = x_{1,9,7,14} \tag{34}$$

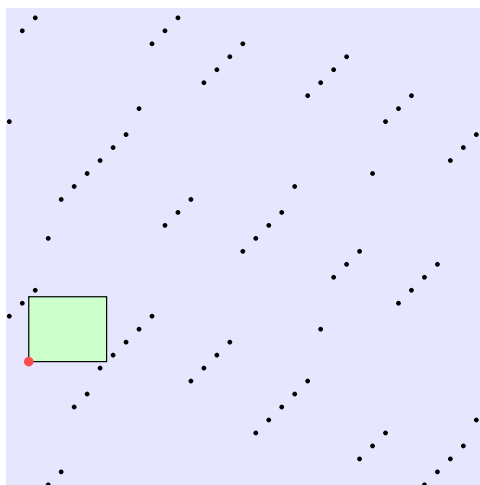

$$0 = x_{1,10,8,14} \tag{35}$$

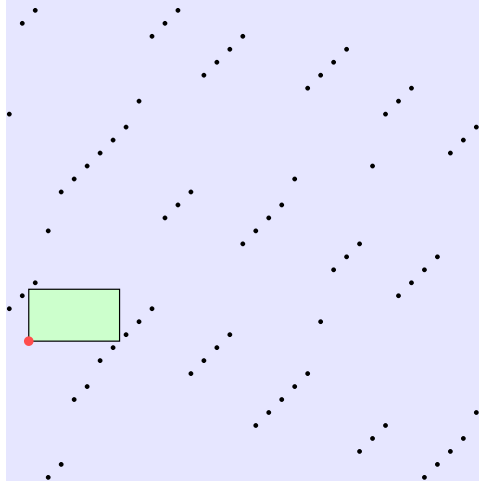

$$0 = x_{1,11,9,14}$$

(36)

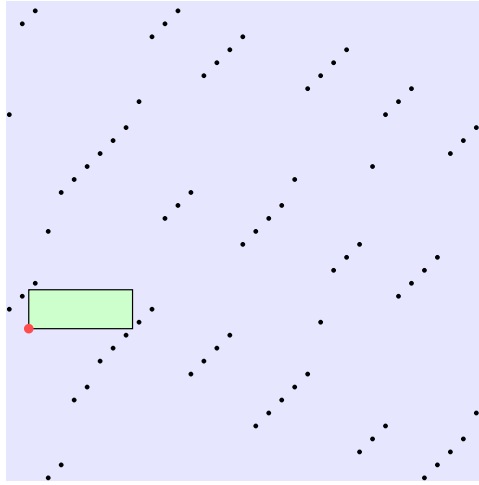

$$x_{36,35,1,12} = x_{1,12,10,14}$$

(37)

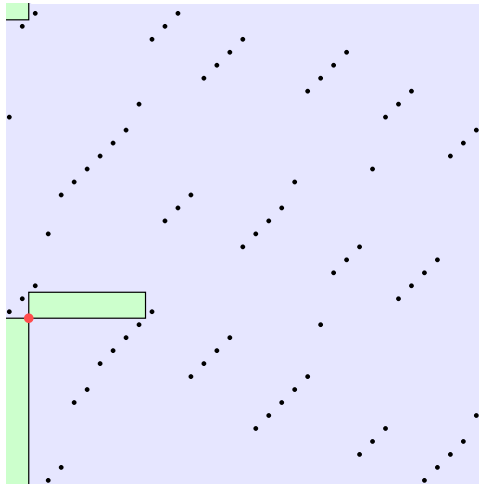

$$x_{0,35,1,13} = x_{1,13,29,14} \quad (38)$$

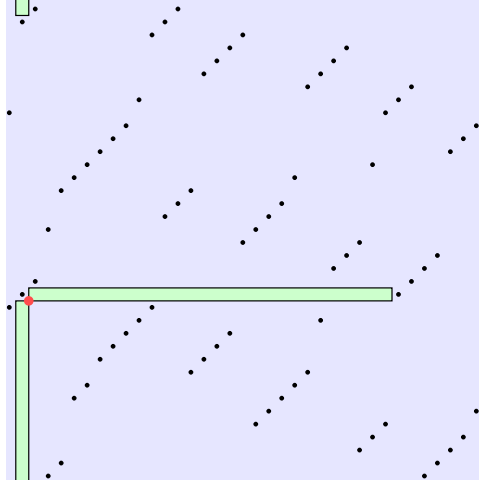

$$\begin{aligned} & x_{0,14,1,34} + x_{31,14,1,15} + x_{32,14,1,16} + x_{33,14,1,24} + x_{34,14,1,25} + x_{35,14,1,26} + x_{36,14,1,27} = \\ & = x_{1,0,3,14} + x_{1,1,4,14} + x_{1,6,5,14} + x_{1,7,6,14} + x_{1,9,7,14} + x_{1,10,8,14} + x_{1,11,9,14} + x_{1,12,10,14} + x_{1,13,29,14} + x_{1,36,2,14} \end{aligned} \quad (39)$$

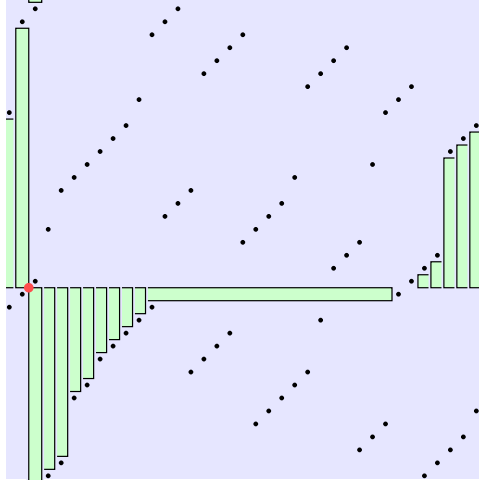

$$x_{31,14,1,15} = x_{1,15,2,35} \quad (40)$$



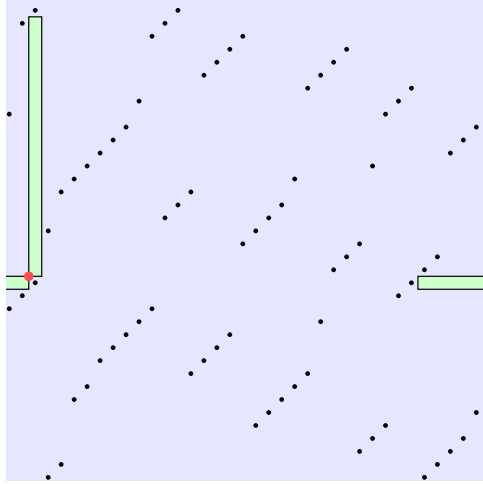

$$x_{32,14,1,16} = 0$$

(41)

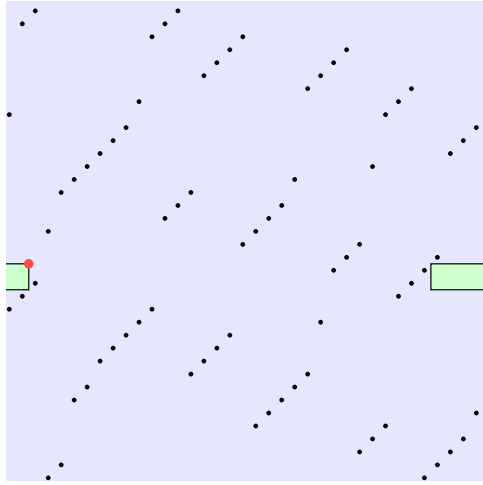

$$0 = x_{1,19,3,35}$$

(42)

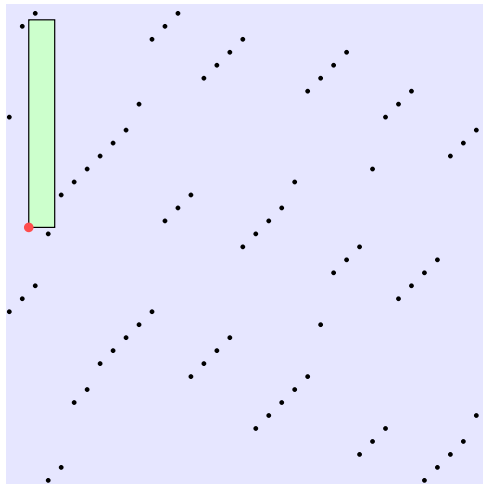

$$0 = x_{1,22,4,35} \quad (43)$$

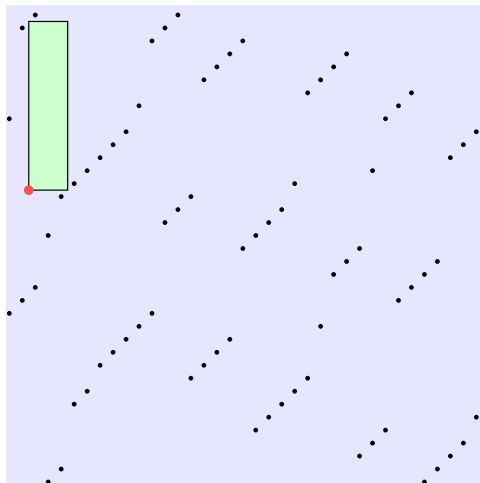

$$0 = x_{1,23,5,35} \quad (44)$$

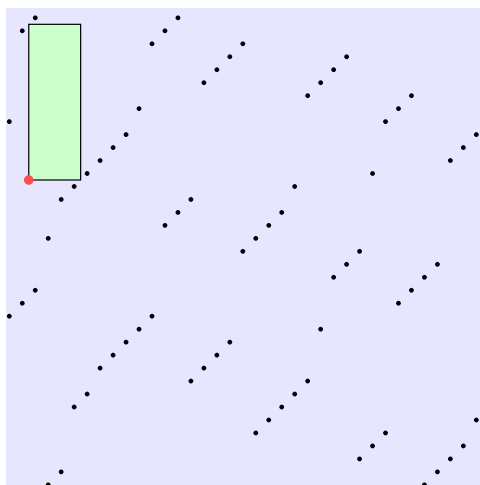

$$x_{33,14,1,24} = x_{1,24,6,35} \quad (45)$$

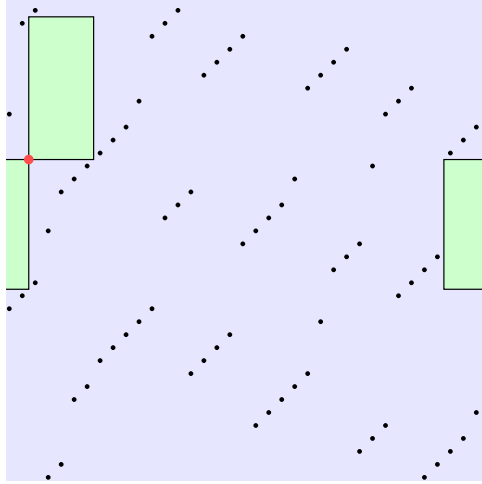

$$x_{34,14,1,25} = x_{1,25,7,35}$$

(46)

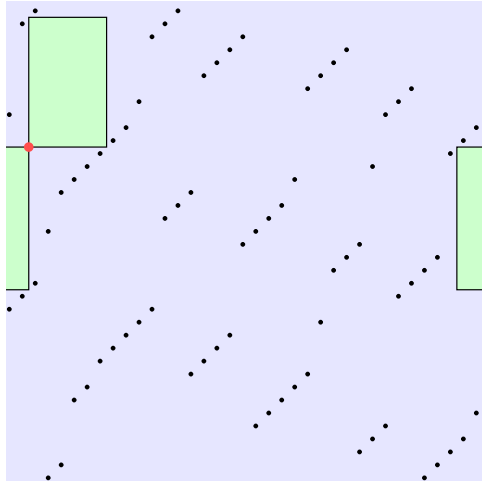

$$x_{35,14,1,26} = x_{1,26,8,35}$$

(47)

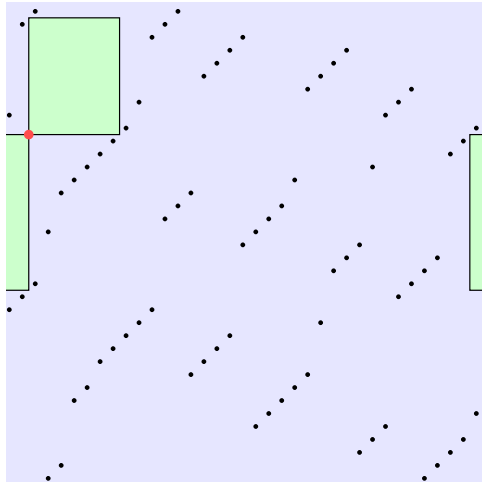

$$x_{36,14,1,27} = x_{1,27,9,35} \quad (48)$$

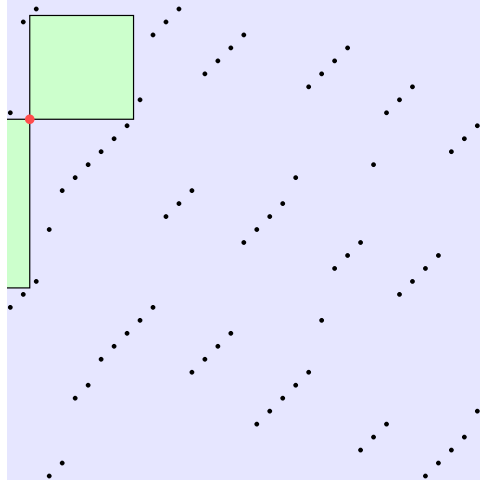

$$0 = x_{1,29,10,35} \quad (49)$$

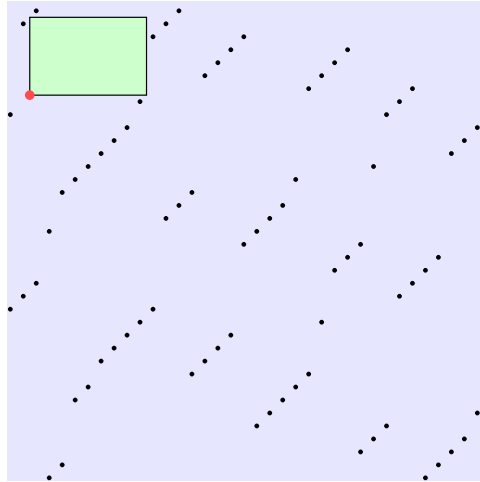

$$x_{0,14,1,34} = x_{1,34,11,35} \quad (50)$$

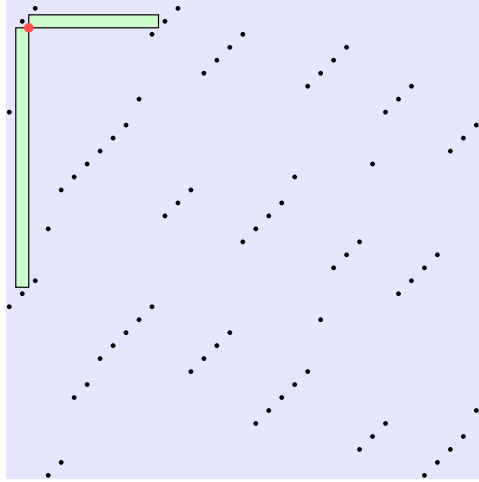

$$\begin{aligned}
 & x_{0,35,1,13} + x_{13,35,1,36} + x_{32,35,1,0} + x_{33,35,1,1} + x_{34,35,1,2} + x_{35,35,1,4} + x_{36,35,1,12} = \\
 & = x_{1,15,2,35} + x_{1,19,3,35} + x_{1,22,4,35} + x_{1,23,5,35} + x_{1,24,6,35} + x_{1,25,7,35} + x_{1,26,8,35} + x_{1,27,9,35} + x_{1,29,10,35} + x_{1,34,11,35} \quad (51)
 \end{aligned}$$

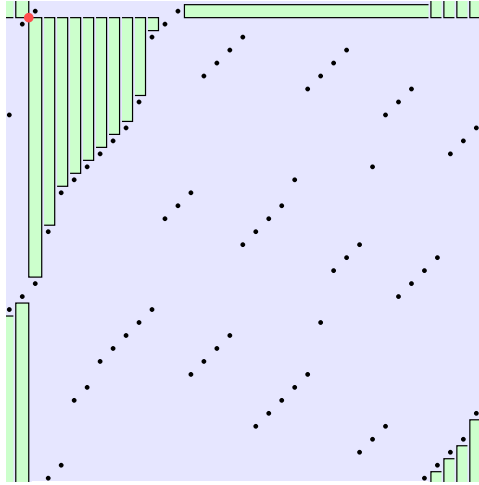

$$x_{13,35,1,36} = x_{1,36,2,14} \quad (52)$$

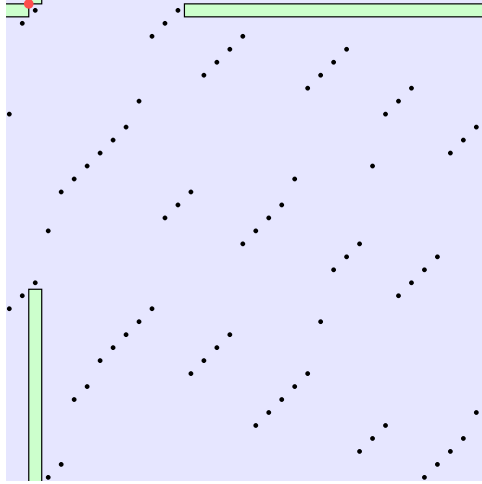

$$x_{32,36,2,0} = x_{2,0,3,18}$$

(53)

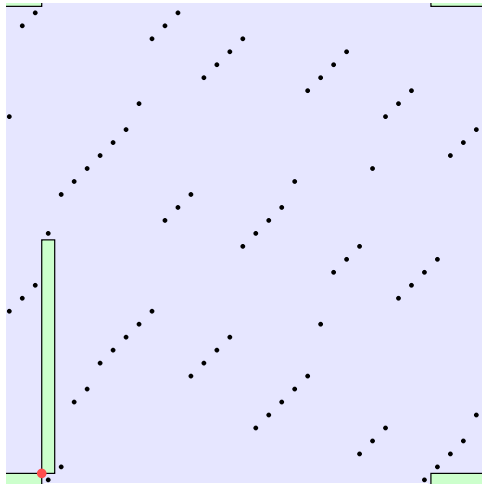

$$x_{33,36,2,1} = x_{2,1,4,18}$$

(54)

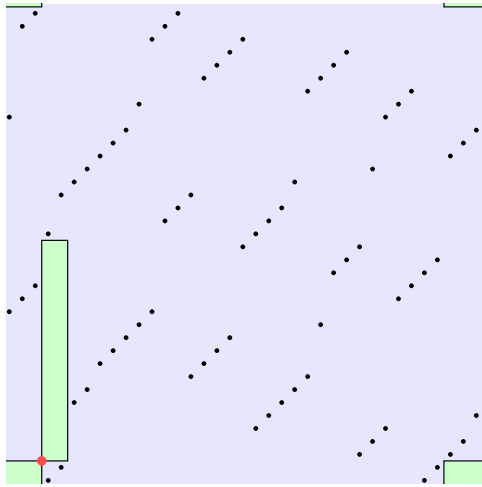

$$x_{34,36,2,2} = 0 \tag{55}$$

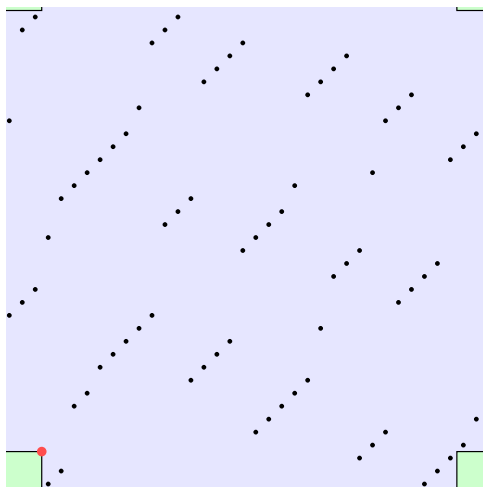

$$x_{35,36,2,4} = 0 \tag{56}$$

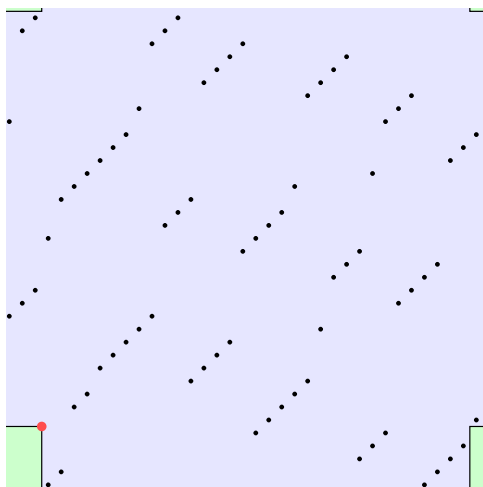

$$0 = x_{2,6,5,18} \tag{57}$$

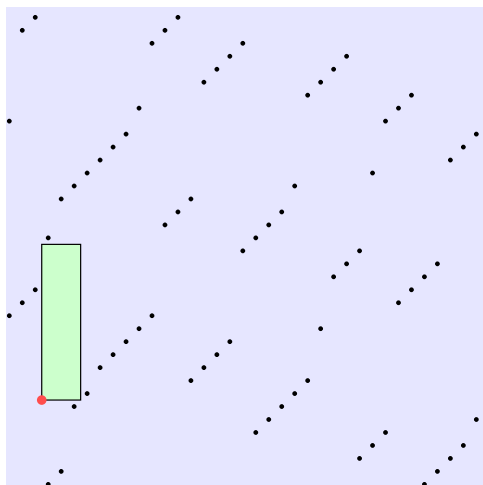

$$0 = x_{2,7,6,18}$$

(58)

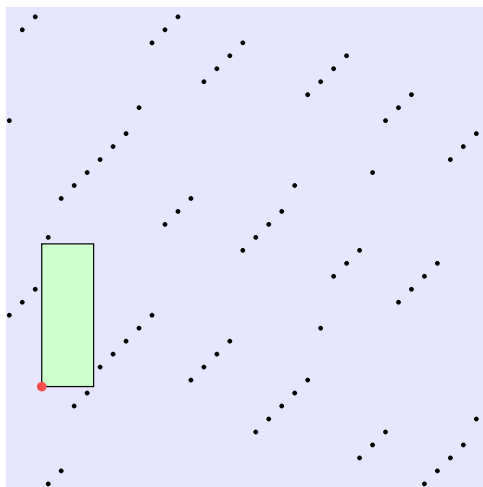

$$0 = x_{2,9,7,18}$$

(59)

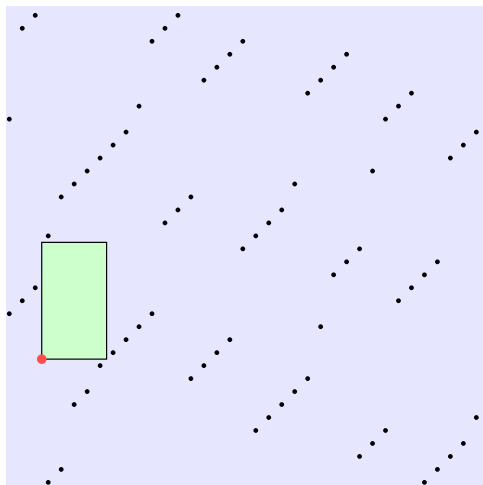



$$0 = x_{2,10,8,18} \tag{60}$$

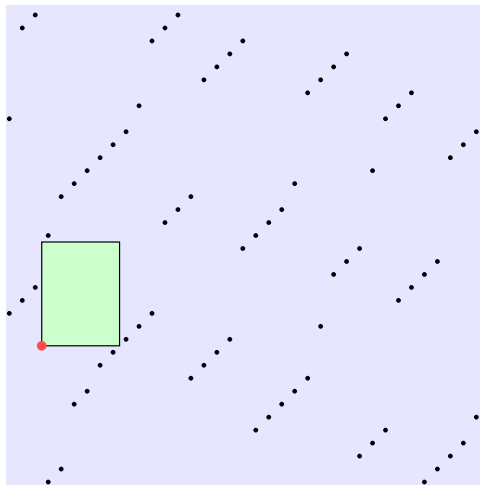

$$0 = x_{2,11,9,18} \tag{61}$$

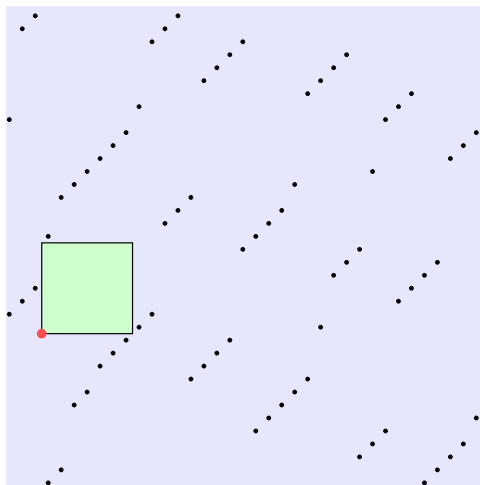

$$x_{36,36,2,12} = x_{2,12,10,18} \tag{62}$$

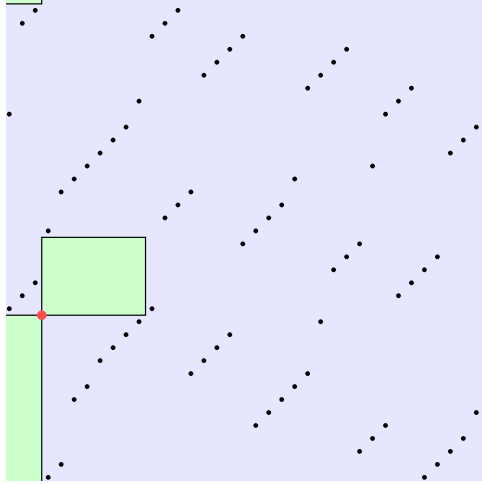

$$x_{0,36,2,13} = x_{2,13,17,18} + x_{2,13,24,17} + x_{2,13,29,15} \quad (63)$$

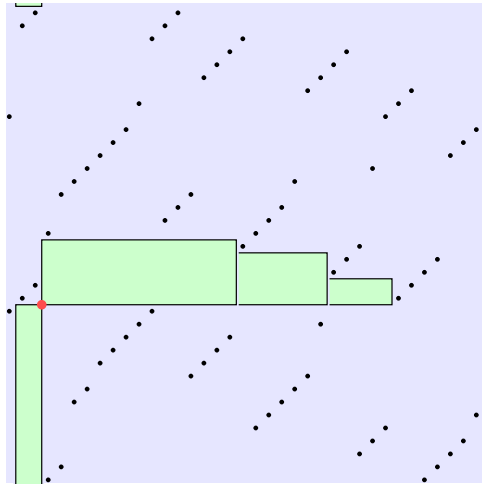

$$x_{1,36,2,14} = x_{2,14,30,15} \quad (64)$$

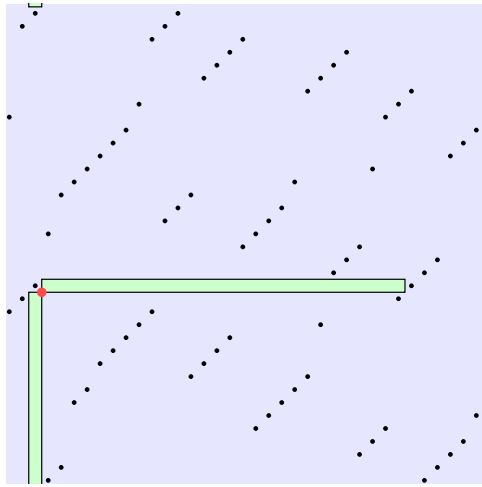

$$x_{0,15,2,34} + x_{1,15,2,35} + x_{33,15,2,24} + x_{34,15,2,25} + x_{35,15,2,26} + x_{36,15,2,27} = x_{2,13,29,15} + x_{2,14,30,15} \quad (65)$$

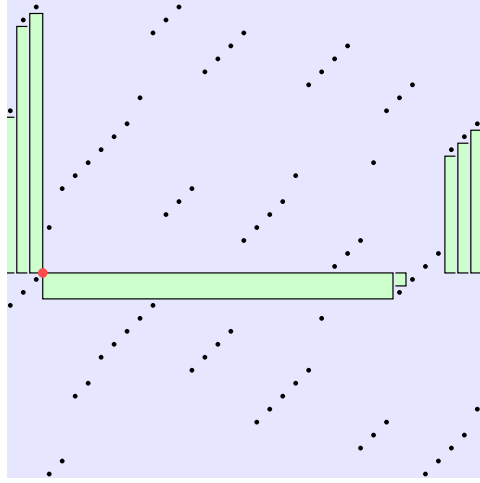

$$x_{27,17,2,23} + x_{28,17,2,24} = x_{2,13,24,17} \quad (66)$$

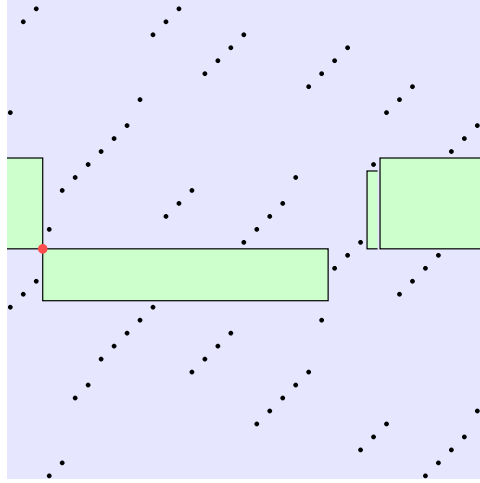

$$\begin{aligned} & x_{19,18,2,19} + x_{20,18,2,20} + x_{21,18,2,22} + x_{22,18,2,23} = \\ & = x_{2,0,3,18} + x_{2,1,4,18} + x_{2,6,5,18} + x_{2,7,6,18} + x_{2,9,7,18} + x_{2,10,8,18} + x_{2,11,9,18} + x_{2,12,10,18} + x_{2,13,17,18} \end{aligned} \quad (67)$$

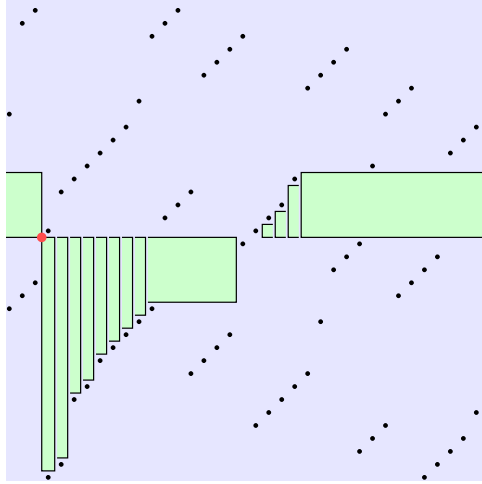

$$x_{19,18,2,19} = x_{2,19,3,36}$$

(68)

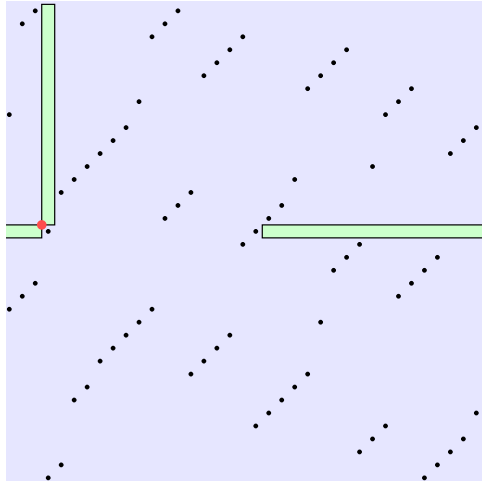

$$x_{20,18,2,20} = 0$$

(69)

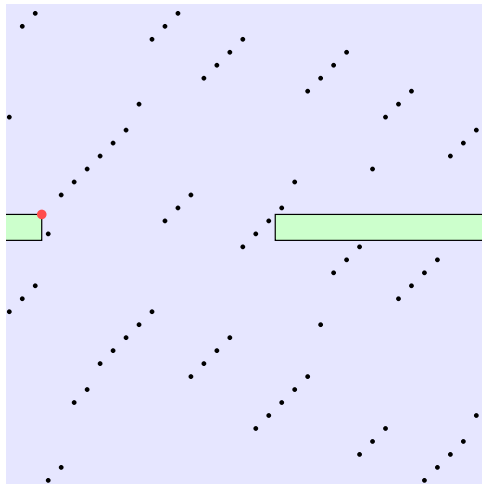

$$x_{21,18,2,22} = x_{2,22,4,36} \quad (70)$$

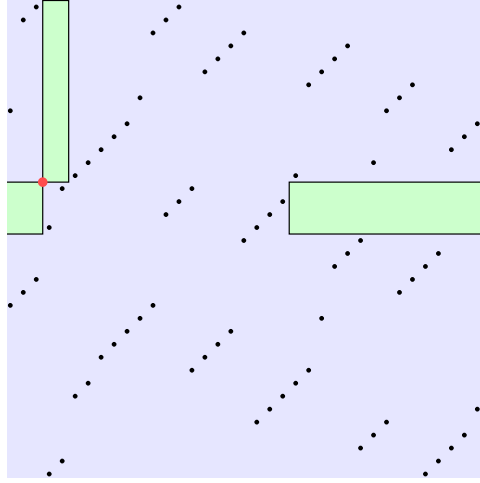

$$x_{22,18,2,23} + x_{27,17,2,23} = x_{2,23,5,36} \quad (71)$$

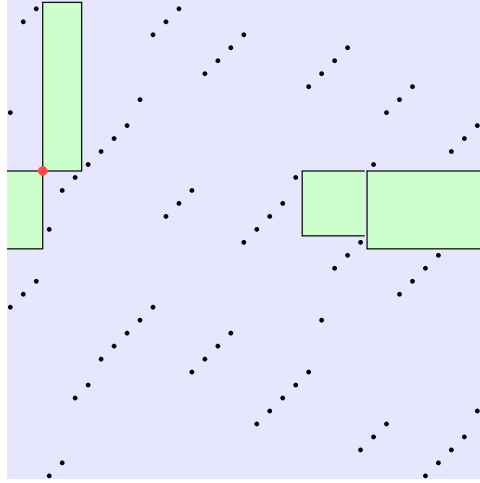

$$x_{28,17,2,24} + x_{33,15,2,24} = x_{2,24,6,36} \quad (72)$$

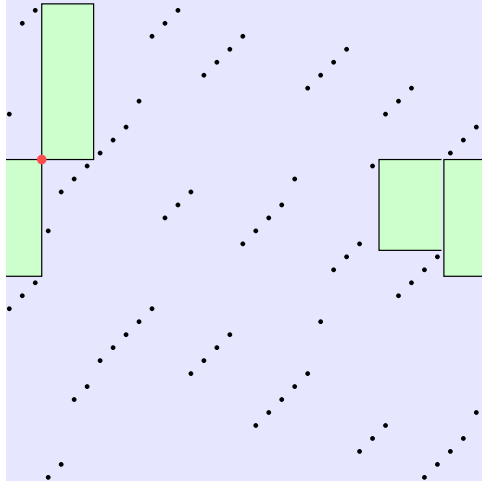

$$x_{34,15,2,25} = x_{2,25,7,36}$$

(73)

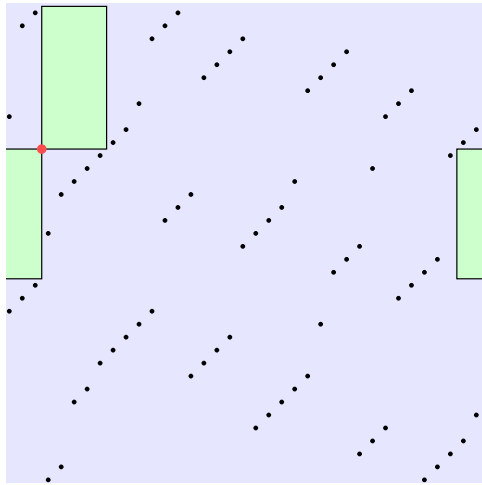

$$x_{35,15,2,26} = x_{2,26,8,36}$$

(74)

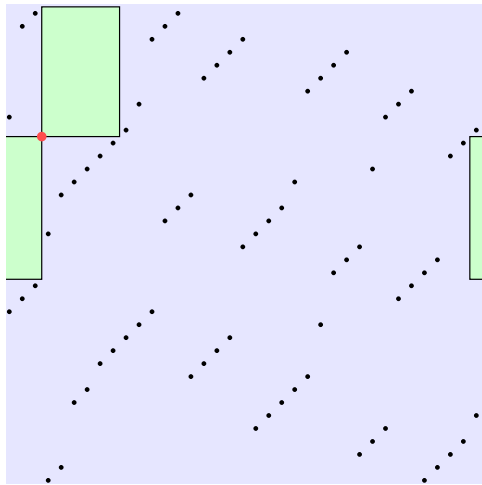

$$x_{36,15,2,27} = x_{2,27,9,36} \quad (75)$$

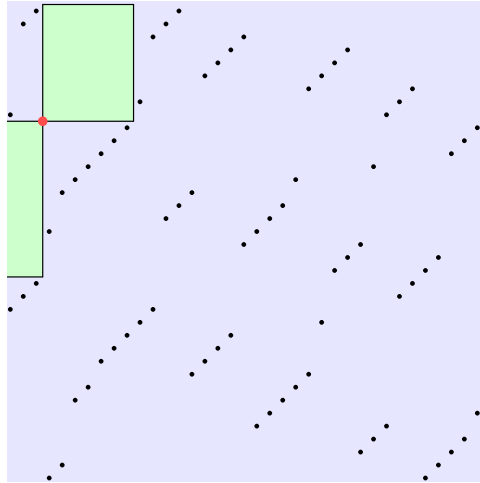

$$0 = x_{2,29,10,36} \quad (76)$$

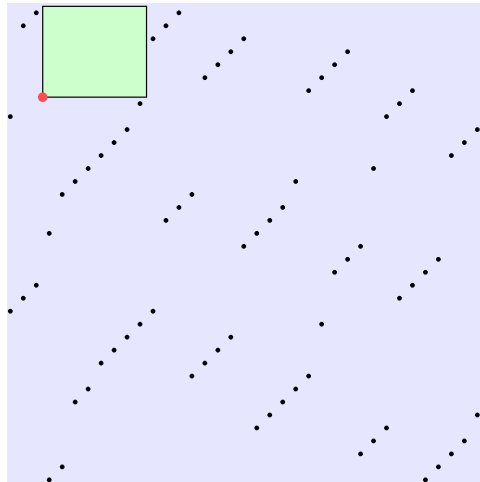

$$x_{0,15,2,34} = x_{2,34,11,36} \quad (77)$$

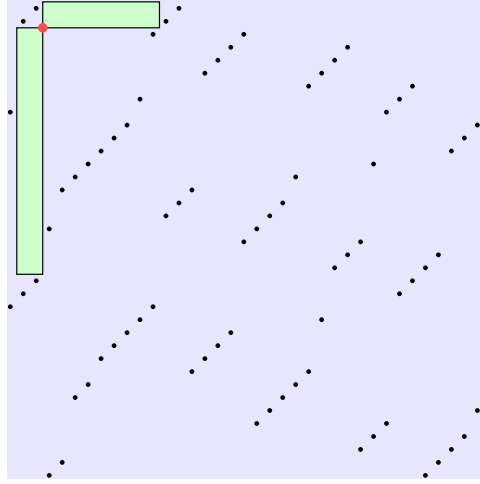

$$x_{1,15,2,35} = x_{2,35,12,36}$$

(78)

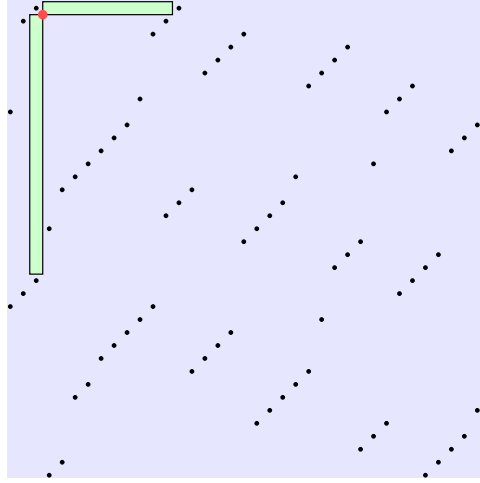

$$\begin{aligned} & x_{0,36,2,13} + x_{1,36,2,14} + x_{32,36,2,0} + x_{33,36,2,1} + x_{34,36,2,2} + x_{35,36,2,4} + x_{36,36,2,12} = \\ & = x_{2,19,3,36} + x_{2,22,4,36} + x_{2,23,5,36} + x_{2,24,6,36} + x_{2,25,7,36} + x_{2,26,8,36} + x_{2,27,9,36} + x_{2,29,10,36} + x_{2,34,11,36} + x_{2,35,12,36} \end{aligned} \quad (79)$$



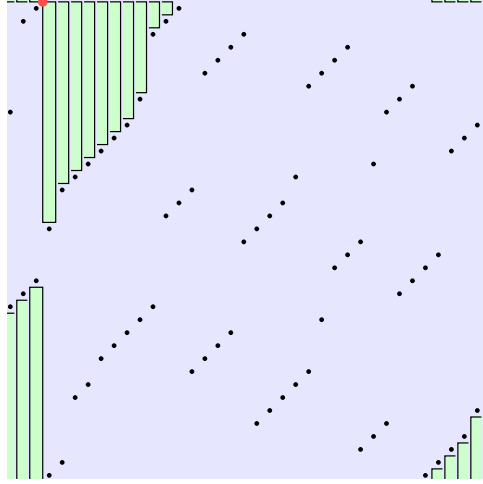

$$\begin{aligned}
 & x_{0,0,3,13} + x_{1,0,3,14} + x_{2,0,3,18} + x_{33,0,3,1} + x_{34,0,3,2} + x_{35,0,3,4} + x_{36,0,3,12} = \\
 & = x_{3,22,4,0} + x_{3,23,5,0} + x_{3,24,6,0} + x_{3,25,7,0} + x_{3,26,8,0} + x_{3,27,9,0} + x_{3,29,10,0} + x_{3,34,11,0} + x_{3,35,12,0} + x_{3,36,31,0} \quad (80)
 \end{aligned}$$

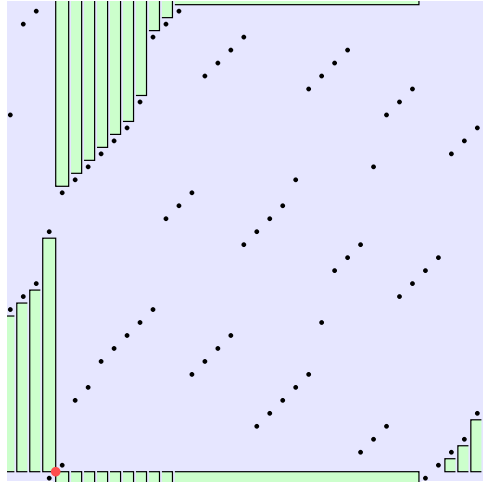

$$x_{33,0,3,1} = x_{3,1,4,21} \quad (81)$$

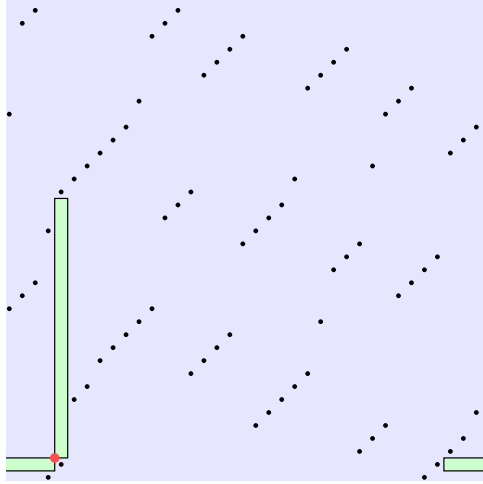

$$x_{34,0,3,2} = 0$$

(82)

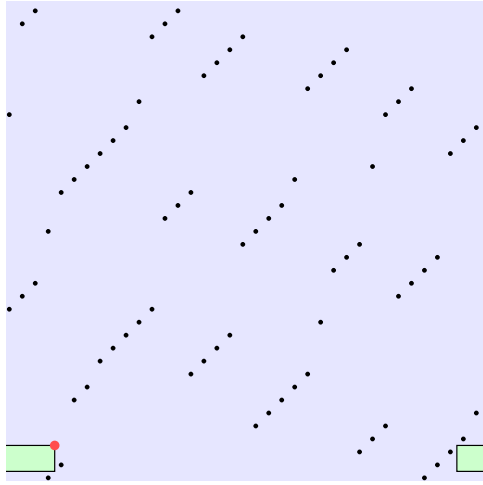

$$x_{35,0,3,4} = 0$$

(83)

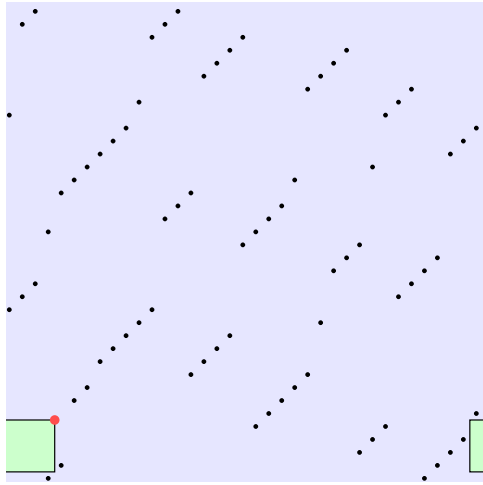

$$0 = x_{3,6,5,21} \tag{84}$$

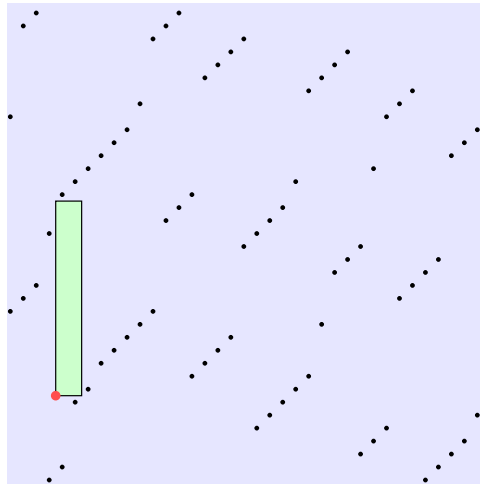

$$0 = x_{3,7,6,21} \tag{85}$$

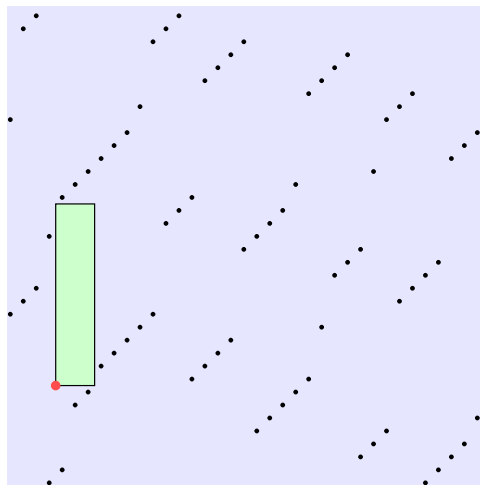

$$0 = x_{3,9,7,21} \tag{86}$$

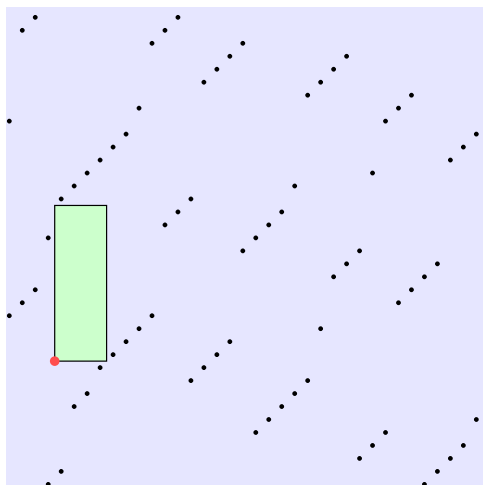

$$0 = x_{3,10,8,21}$$

(87)

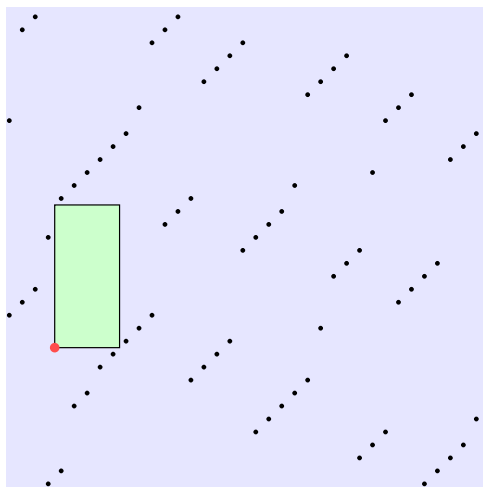

$$0 = x_{3,11,9,21}$$

(88)

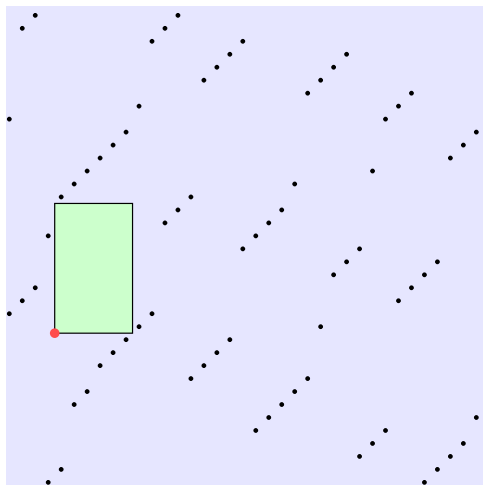

$$x_{36,0,3,12} = x_{3,12,10,21} \tag{89}$$

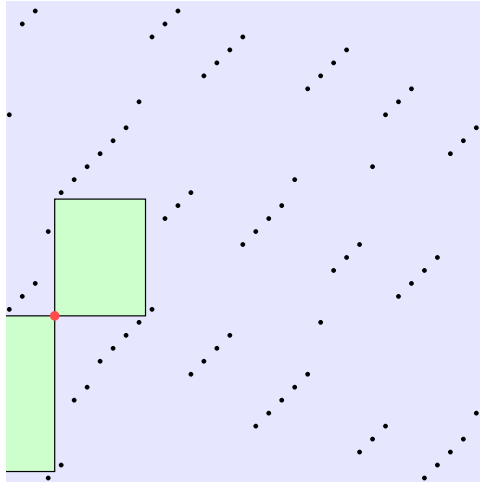

$$x_{0,0,3,13} = x_{3,13,11,21} + x_{3,13,17,19} \tag{90}$$

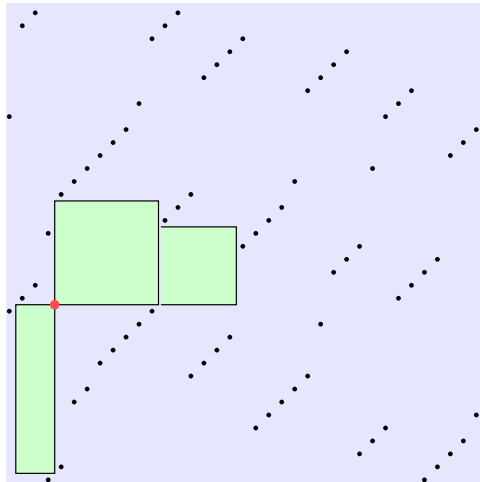

$$x_{1,0,3,14} = 0 \tag{91}$$

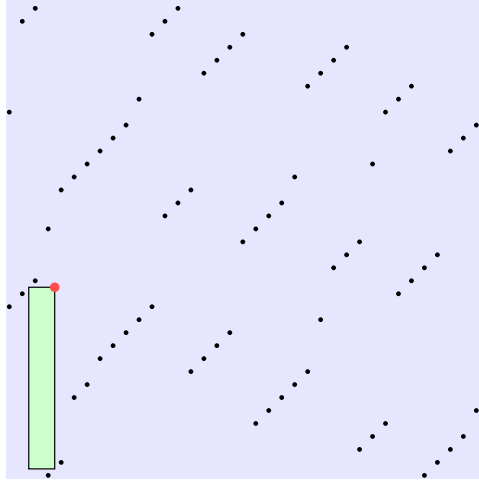

$$x_{2,0,3,18} = x_{3,18,18,19}$$

(92)

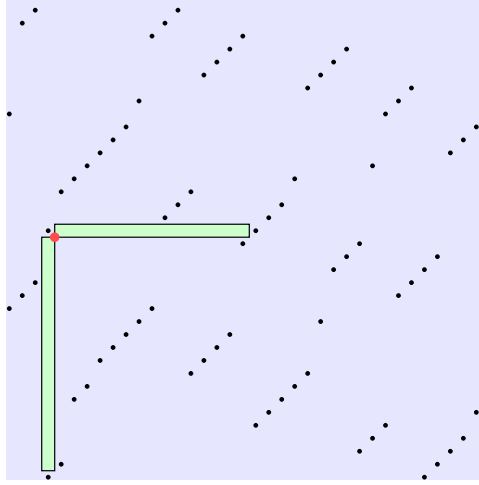

$$\begin{aligned} x_{0,19,3,34} + x_{1,19,3,35} + x_{2,19,3,36} + x_{21,19,3,22} + x_{22,19,3,23} + x_{28,19,3,24} + x_{34,19,3,25} + x_{35,19,3,26} + x_{36,19,3,27} = \\ = x_{3,13,17,19} + x_{3,18,18,19} \end{aligned} \quad (93)$$

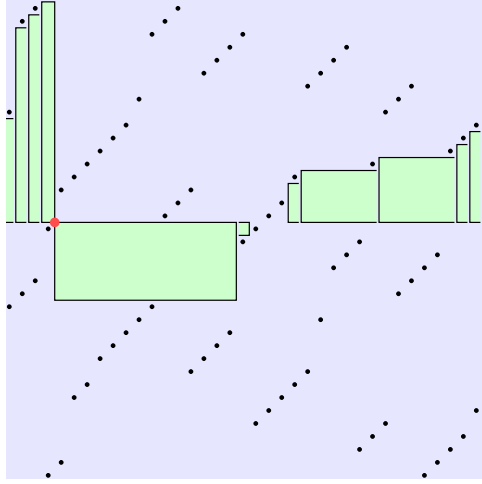

$$x_{14,21,3,22} = x_{3,1,4,21} + x_{3,6,5,21} + x_{3,7,6,21} + x_{3,9,7,21} + x_{3,10,8,21} + x_{3,11,9,21} + x_{3,12,10,21} + x_{3,13,11,21} \quad (94)$$

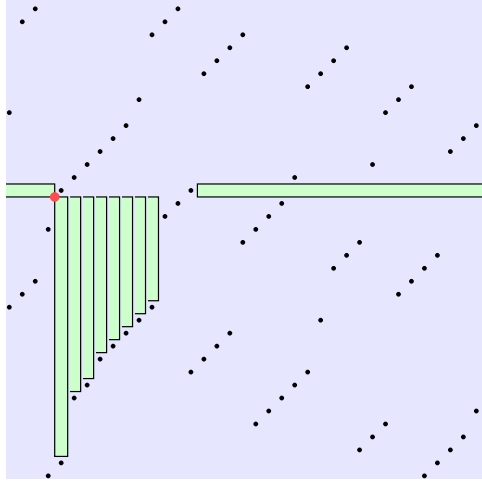

$$x_{14,21,3,22} + x_{21,19,3,22} = x_{3,22,4,0} \quad (95)$$

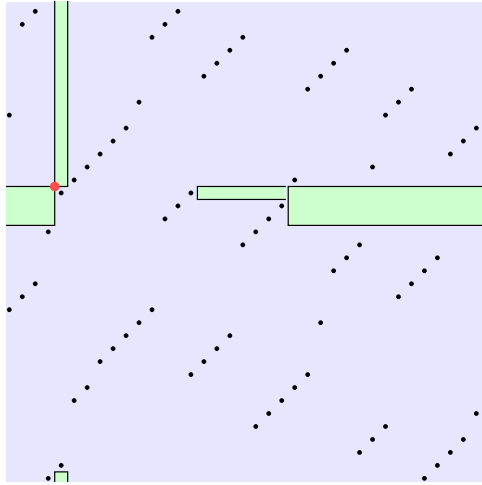

$$x_{22,19,3,23} = x_{3,23,5,0} \quad (96)$$

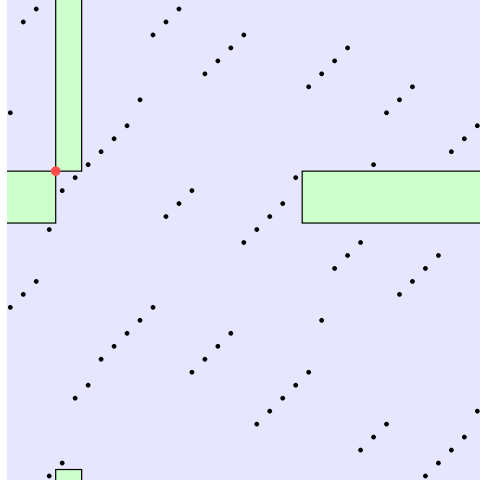

$$x_{28,19,3,24} = x_{3,24,6,0} \quad (97)$$

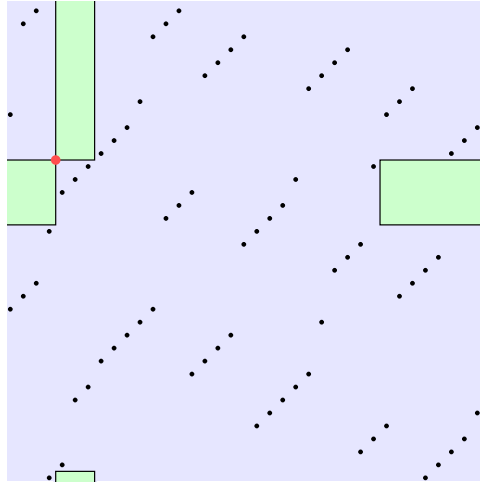

$$x_{34,19,3,25} = x_{3,25,7,0} \quad (98)$$



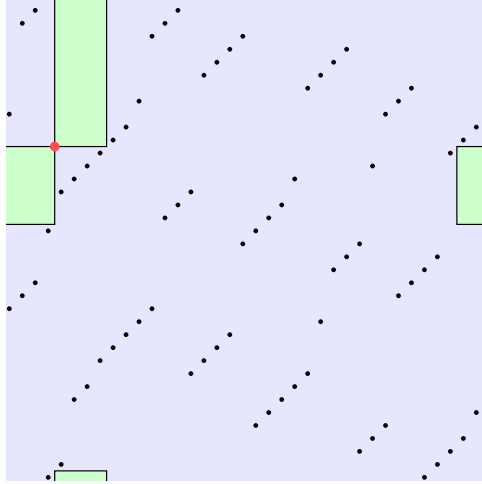

$$x_{35,19,3,26} = x_{3,26,8,0}$$

(99)

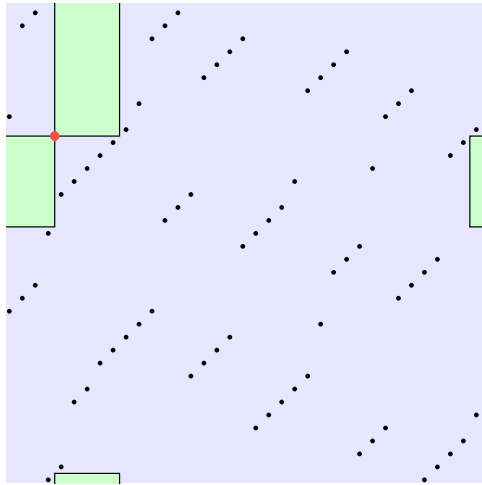

$$x_{36,19,3,27} = x_{3,27,9,0}$$

(100)

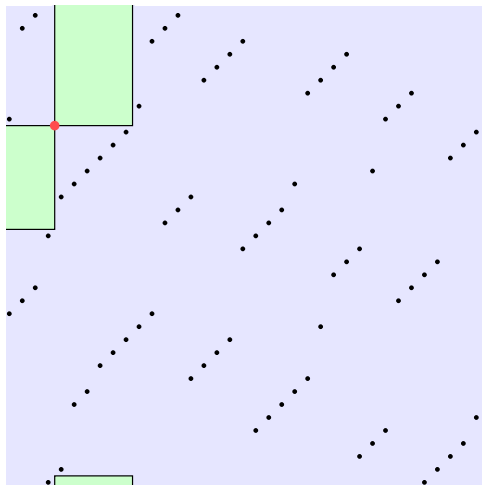

$$0 = x_{3,29,10,0} \tag{101}$$

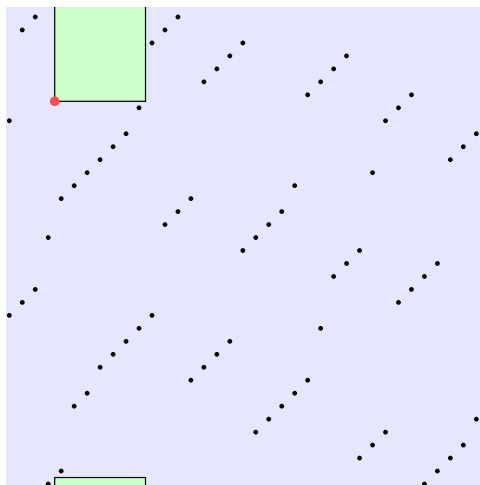

$$x_{0,19,3,34} = x_{3,34,11,0} \tag{102}$$

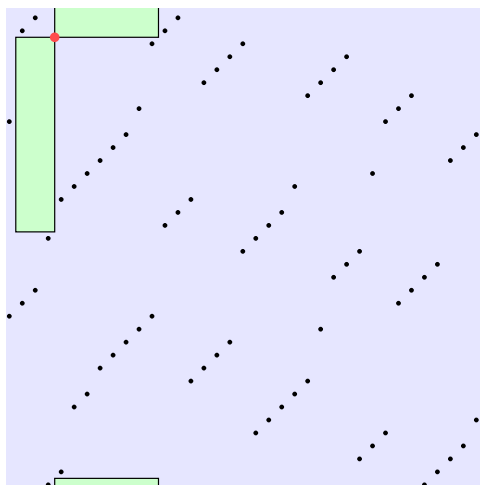

$$x_{1,19,3,35} = x_{3,35,12,0} \tag{103}$$

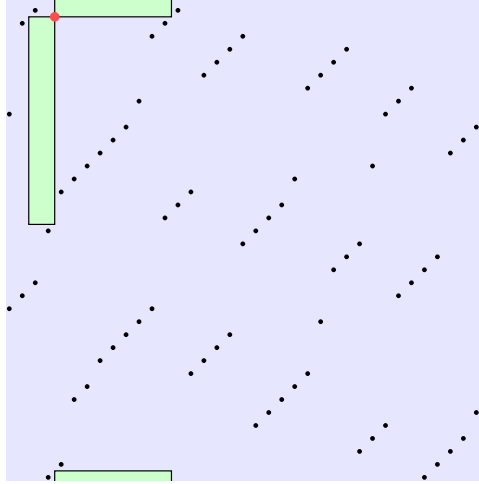

$$x_{2,19,3,36} = x_{3,36,31,0}$$

(104)

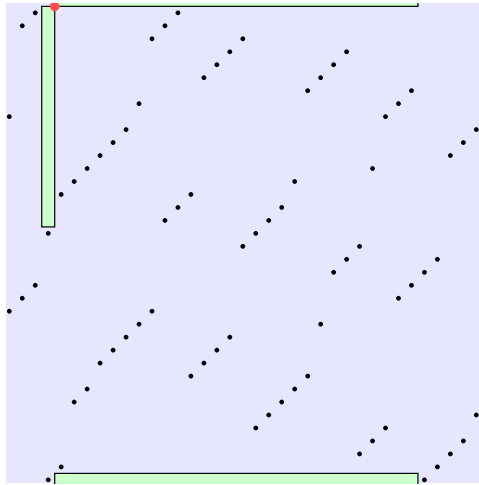

$$x_{3,22,4,0} = x_{4,0,32,1}$$

(105)

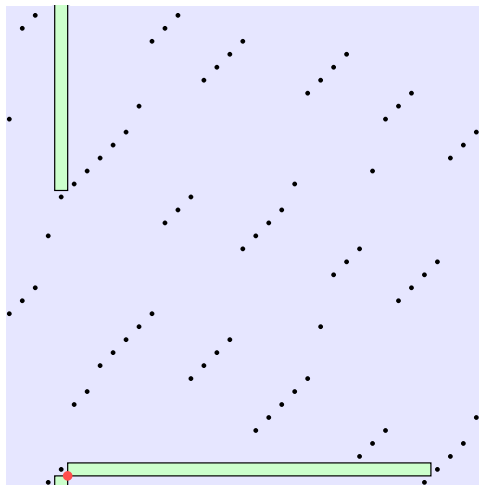

$$x_{0,1,4,13} + x_{1,1,4,14} + x_{2,1,4,18} + x_{3,1,4,21} + x_{36,1,4,12} = x_{4,0,32,1} + x_{4,36,31,1} \quad (106)$$

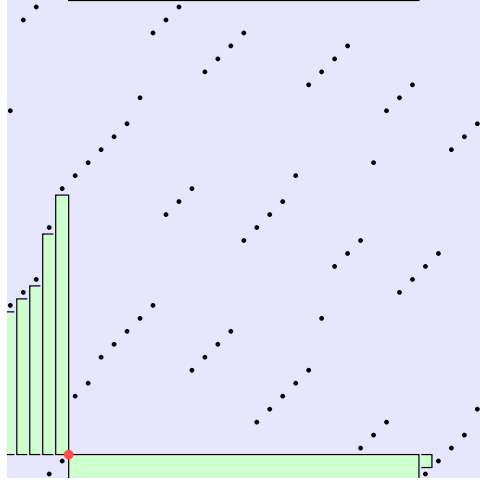

$$0 = x_{4,36,26,3} \quad (107)$$

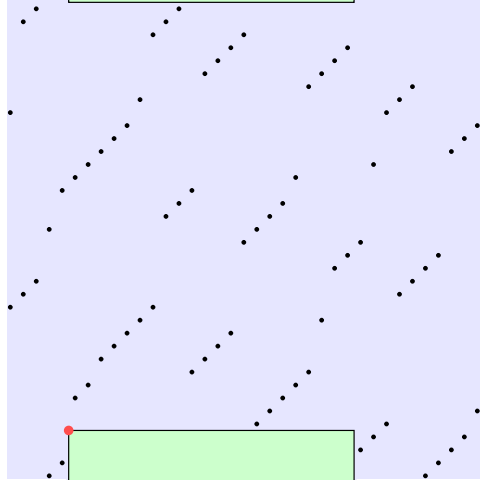

$$\begin{aligned} & x_{21,5,4,6} + x_{22,5,4,7} + x_{23,5,4,11} + x_{24,5,4,12} = \\ & = x_{4,23,5,5} + x_{4,24,6,5} + x_{4,25,7,5} + x_{4,26,8,5} + x_{4,27,9,5} + x_{4,29,10,5} + x_{4,34,11,5} + x_{4,35,12,5} + x_{4,36,18,5} \end{aligned} \quad (108)$$

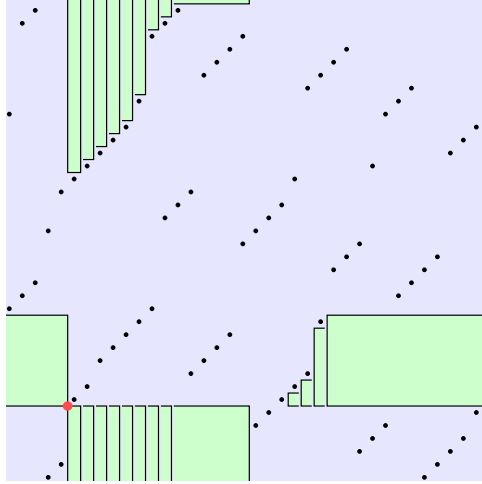

$$x_{21,5,4,6} = x_{4,6,5,22}$$

(109)

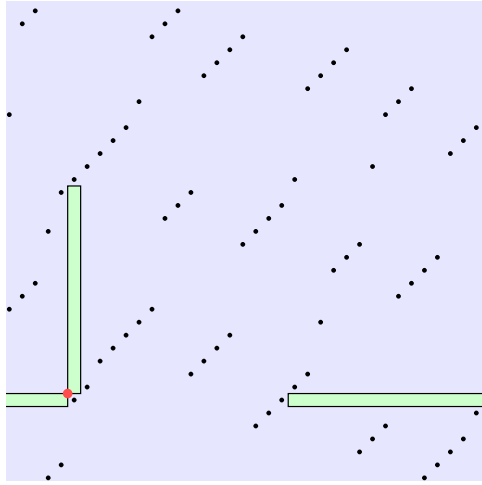

$$x_{22,5,4,7} = x_{4,7,6,22}$$

(110)

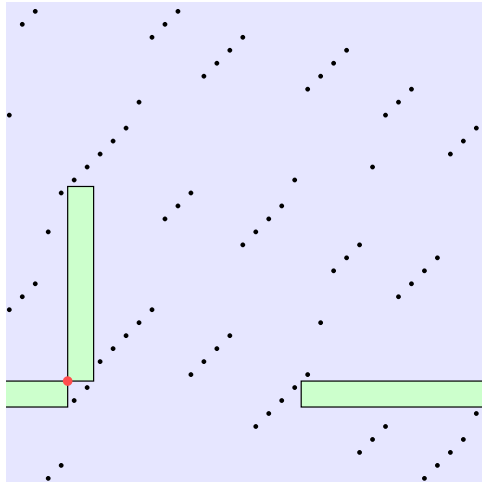

$$0 = x_{4,9,7,22} \tag{111}$$

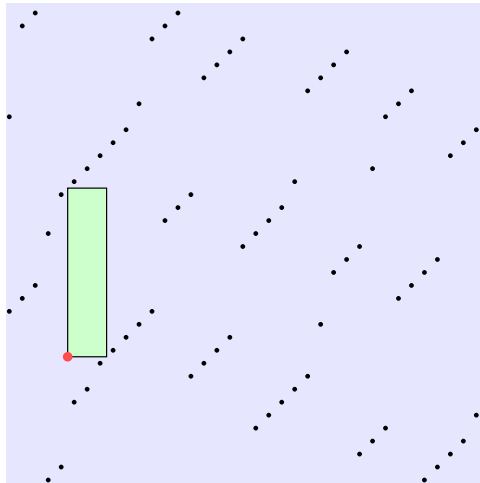

$$0 = x_{4,10,8,22} \tag{112}$$

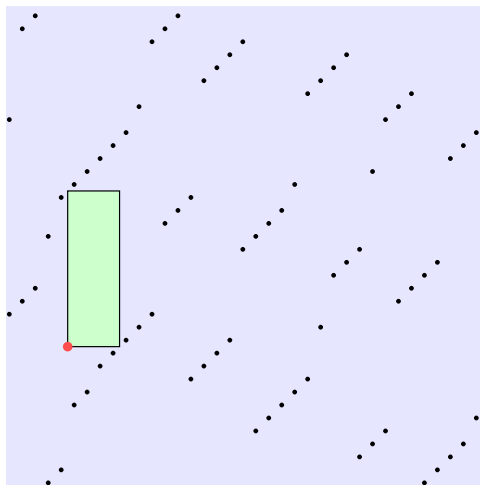

$$x_{23,5,4,11} = x_{4,11,9,22} \tag{113}$$

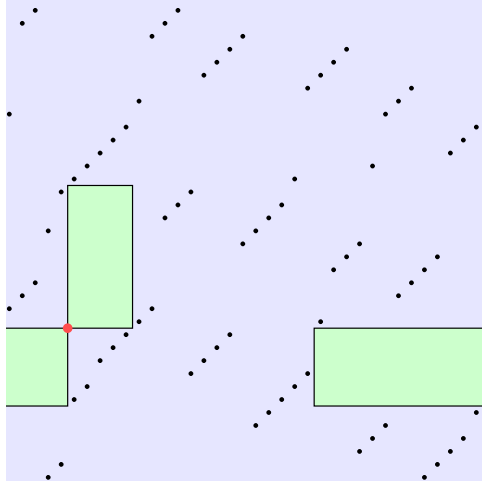

$$x_{24,5,4,12} + x_{36,1,4,12} = x_{4,12,10,22}$$

(114)

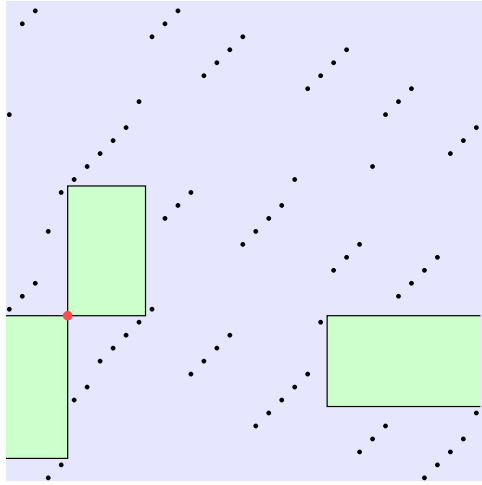

$$x_{0,1,4,13} = x_{4,13,11,22}$$

(115)

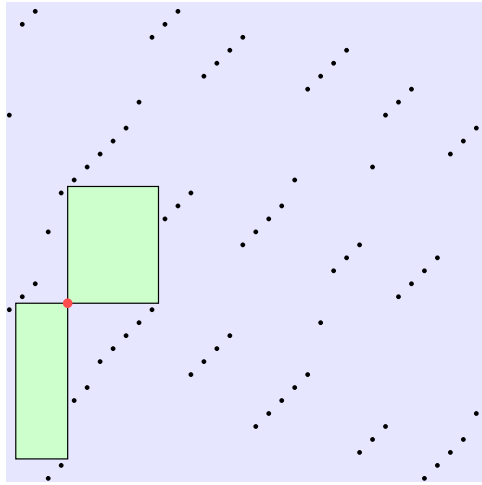

$$x_{1,1,4,14} = 0 \tag{116}$$

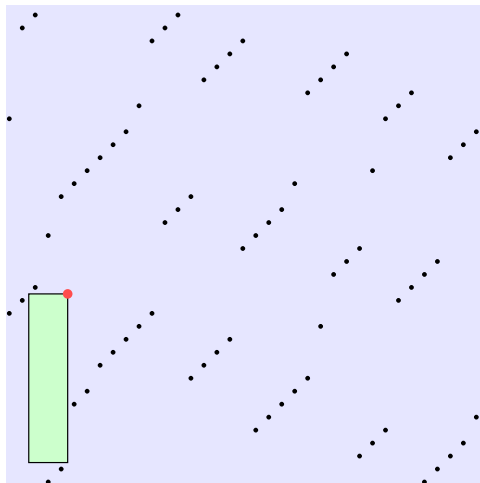

$$x_{2,1,4,18} = 0 \tag{117}$$

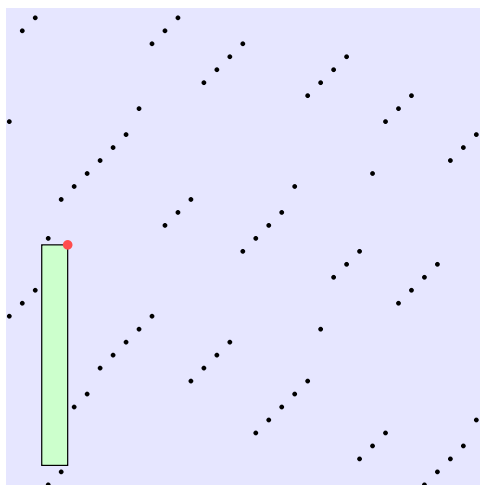

$$0 = x_{4,20,12,22} \tag{118}$$



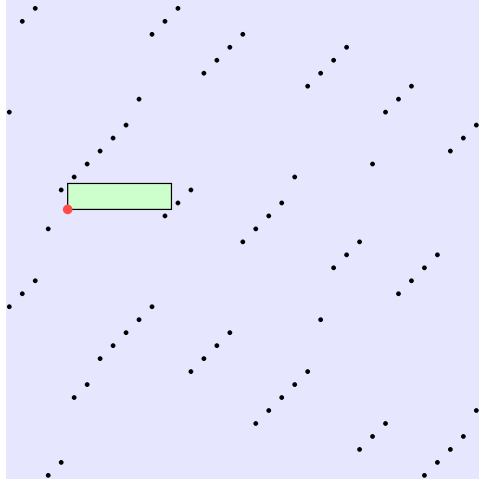

$$x_{3,1,4,21} = x_{4,21,13,22}$$

(119)

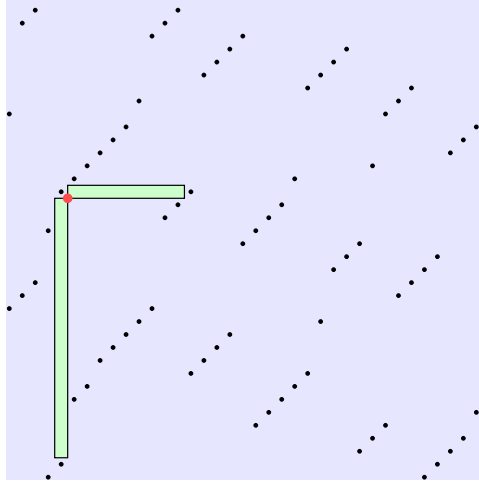

$$\begin{aligned} & x_{0,22,4,34} + x_{1,22,4,35} + x_{2,22,4,36} + x_{3,22,4,0} + x_{22,22,4,23} + x_{28,22,4,24} + x_{34,22,4,25} + x_{35,22,4,26} + x_{36,22,4,27} = \\ & = x_{4,6,5,22} + x_{4,7,6,22} + x_{4,9,7,22} + x_{4,10,8,22} + x_{4,11,9,22} + x_{4,12,10,22} + x_{4,13,11,22} + x_{4,20,12,22} + x_{4,21,13,22} \end{aligned} \quad (120)$$

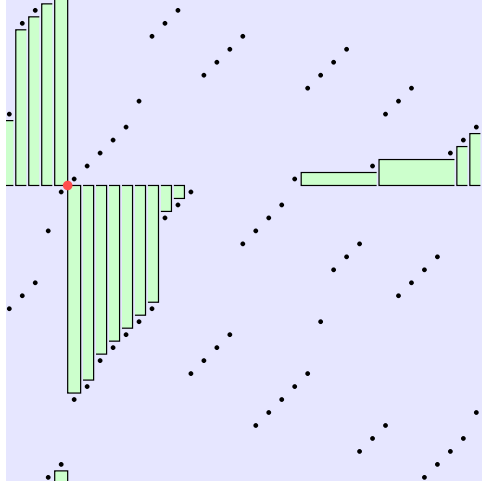

$$x_{22,22,4,23} = x_{4,23,5,5}$$

(121)

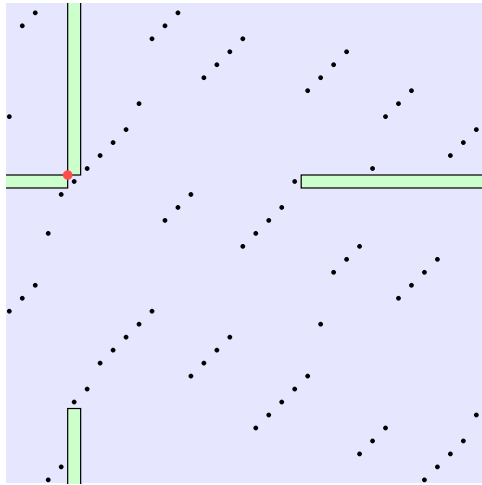

$$x_{28,22,4,24} = x_{4,24,6,5}$$

(122)

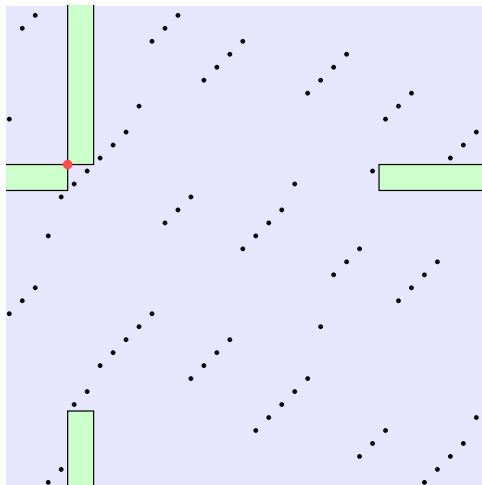

$$x_{34,22,4,25} = x_{4,25,7,5}$$

(123)

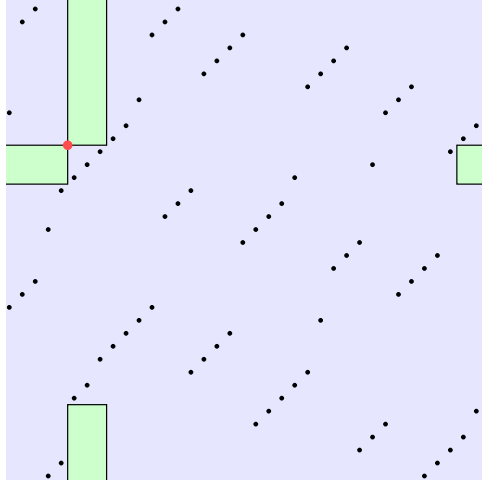

$$x_{35,22,4,26} = x_{4,26,8,5}$$

(124)

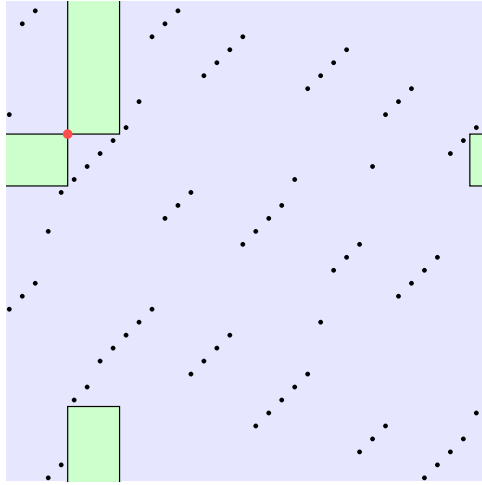

$$x_{36,22,4,27} = x_{4,27,9,5}$$

(125)

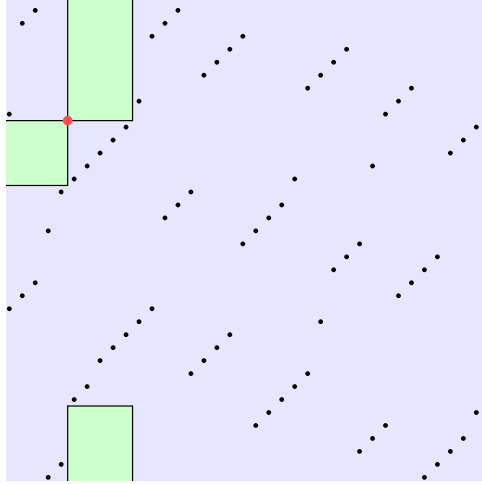

$$0 = x_{4,29,10,5}$$

(126)

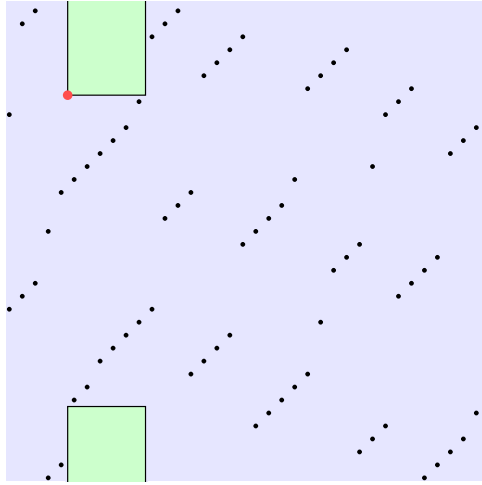

$$x_{0,22,4,34} = x_{4,34,11,5}$$

(127)

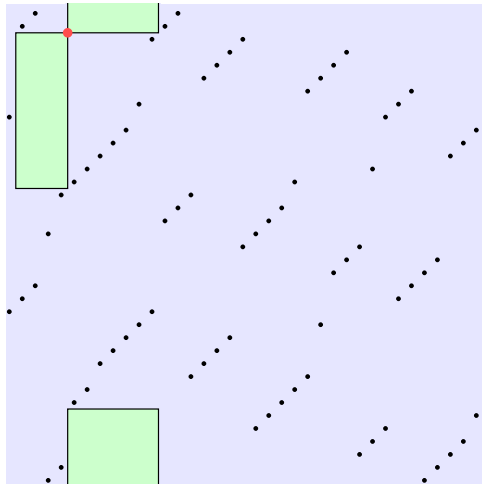

$$x_{1,22,4,35} = x_{4,35,12,5}$$

(128)

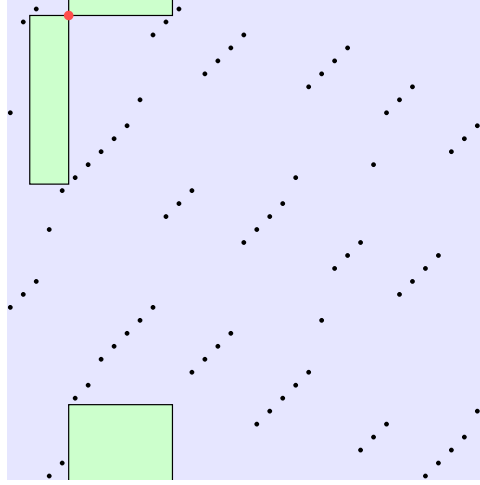

$$x_{2,22,4,36} = x_{4,36,18,5} + x_{4,36,26,3} + x_{4,36,31,1}$$

(129)

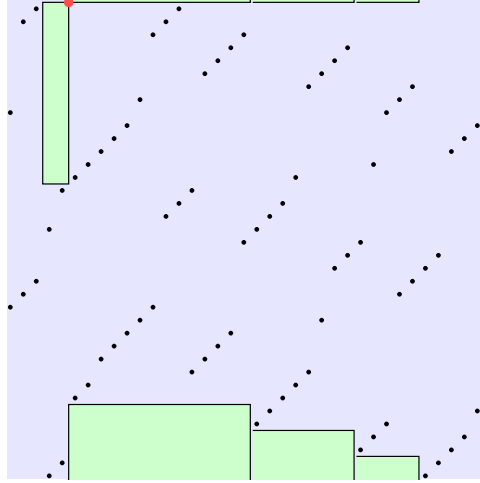

$$x_{3,23,5,0} = 0$$

(130)

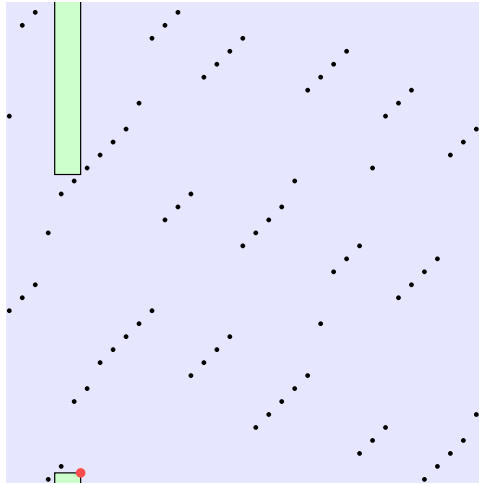

$$0 = x_{5,4,19,6}$$

(131)

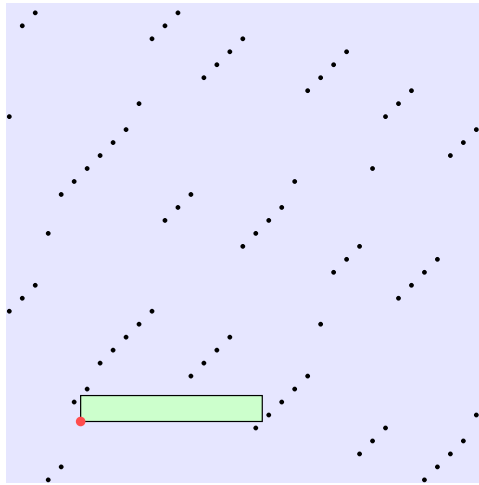

$$x_{4,23,5,5} = x_{5,5,20,6}$$

(132)

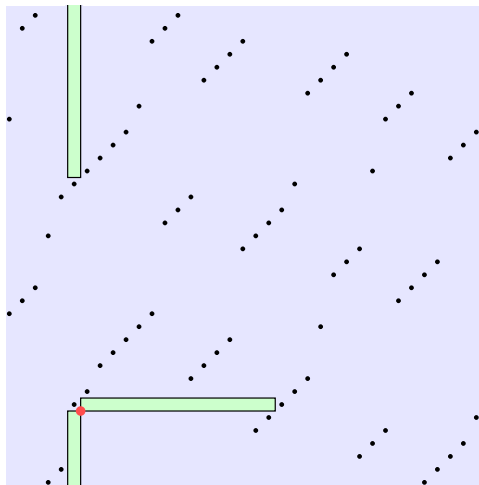

$$\begin{aligned}
& x_{0,6,5,13} + x_{1,6,5,14} + x_{2,6,5,18} + x_{3,6,5,21} + x_{4,6,5,22} + x_{22,6,5,7} + x_{23,6,5,11} + x_{24,6,5,12} = \\
& = x_{5,4,19,6} + x_{5,5,20,6} + x_{5,24,6,6} + x_{5,25,7,6} + x_{5,26,8,6} + x_{5,27,9,6} + x_{5,29,10,6} + x_{5,34,11,6} + x_{5,35,12,6} + x_{5,36,18,6} \quad (133)
\end{aligned}$$

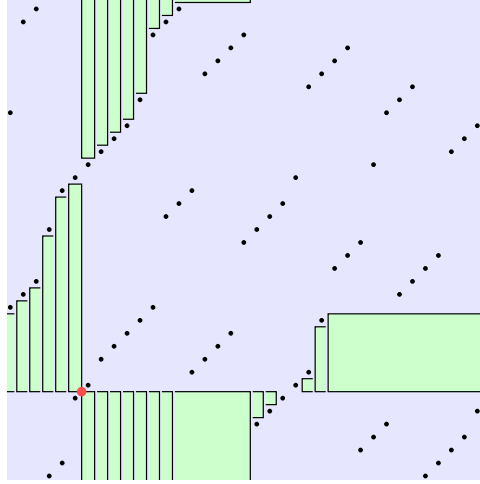

$$x_{22,6,5,7} = x_{5,7,6,23} \quad (134)$$

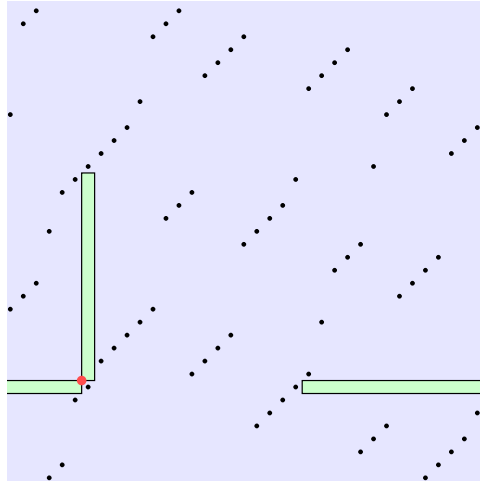

$$0 = x_{5,9,7,23} \quad (135)$$

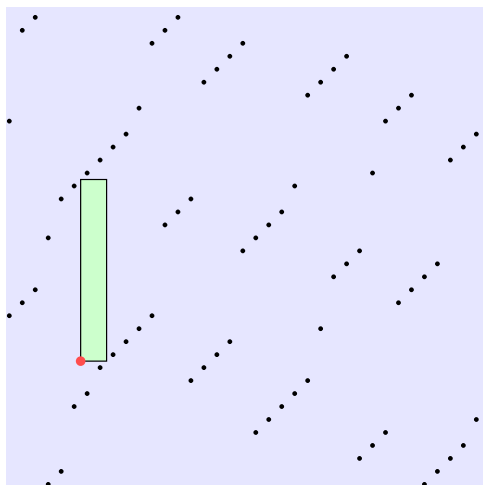

$$0 = x_{5,10,8,23}$$

(136)

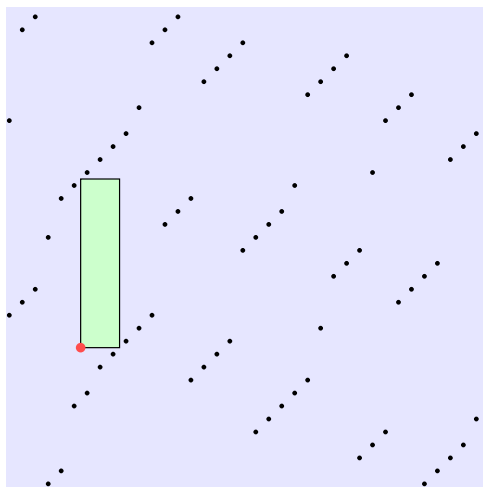

$$x_{23,6,5,11} = x_{5,11,9,23}$$

(137)

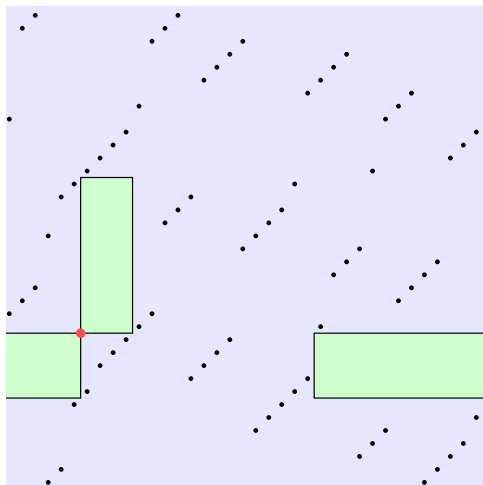



$$x_{24,6,5,12} = x_{5,12,10,23} \tag{138}$$

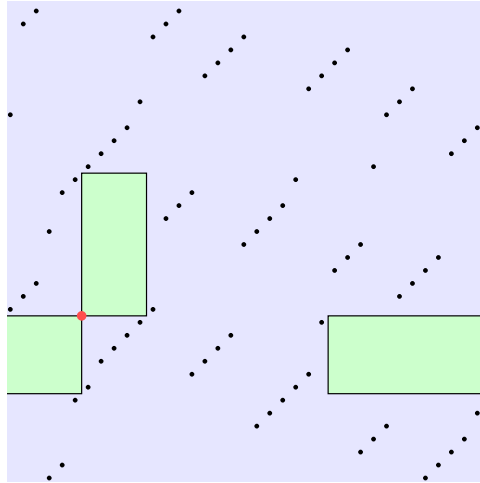

$$x_{0,6,5,13} = x_{5,13,11,23} \tag{139}$$

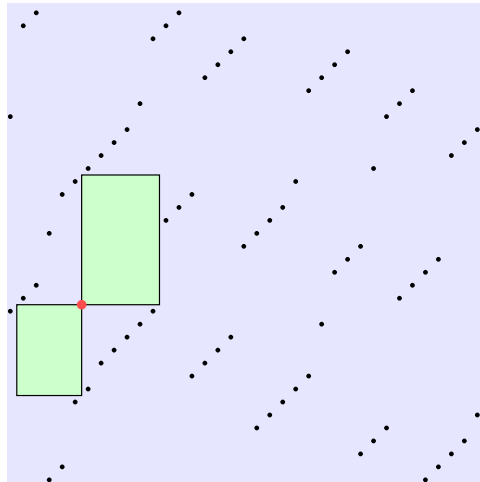

$$x_{1,6,5,14} = 0 \tag{140}$$

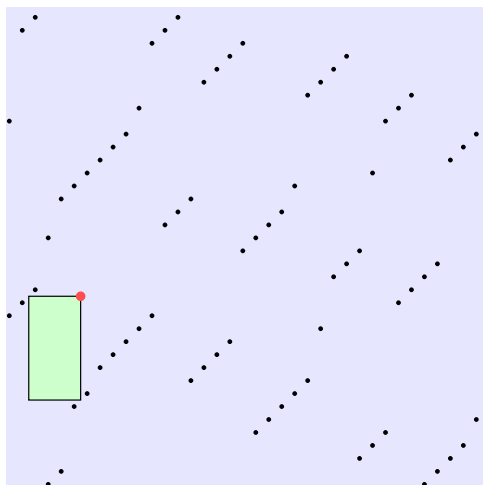

$$x_{2,6,5,18} = 0$$

(141)

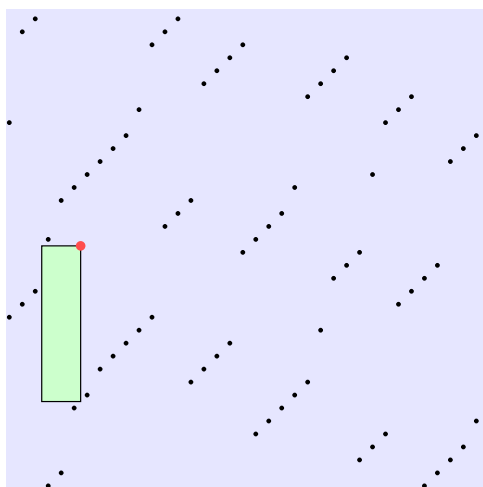

$$0 = x_{5,20,12,23}$$

(142)

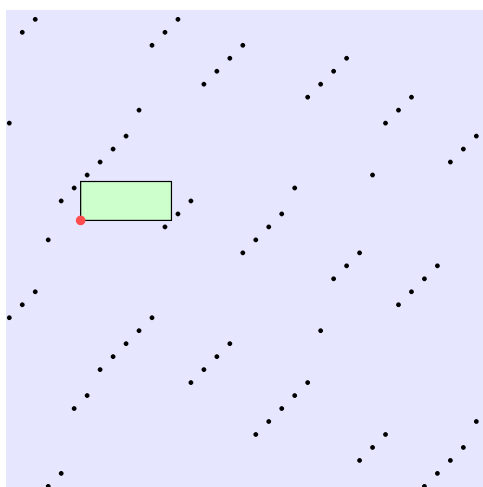

$$x_{3,6,5,21} = x_{5,21,13,23}$$

(143)

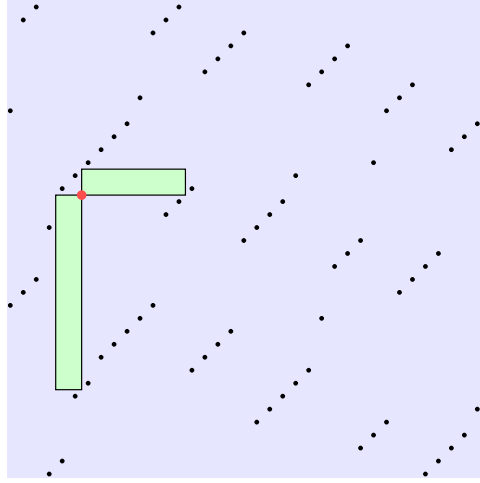

$$x_{4,6,5,22} = x_{5,22,21,23}$$

(144)

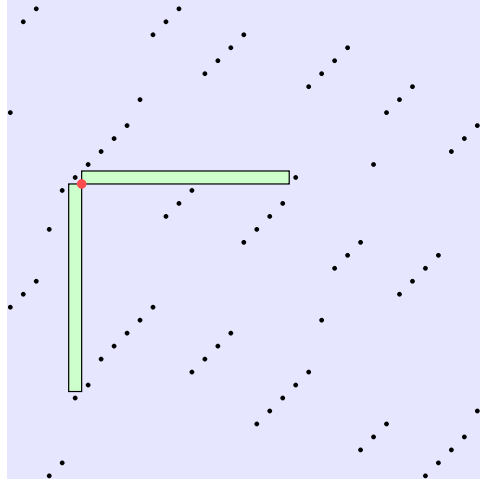

$$\begin{aligned} & x_{0,23,5,34} + x_{1,23,5,35} + x_{2,23,5,36} + x_{3,23,5,0} + x_{4,23,5,5} + x_{28,23,5,24} + x_{34,23,5,25} + x_{35,23,5,26} + x_{36,23,5,27} = \\ & = x_{5,7,6,23} + x_{5,9,7,23} + x_{5,10,8,23} + x_{5,11,9,23} + x_{5,12,10,23} + x_{5,13,11,23} + x_{5,20,12,23} + x_{5,21,13,23} + x_{5,22,21,23} \end{aligned} \quad (145)$$

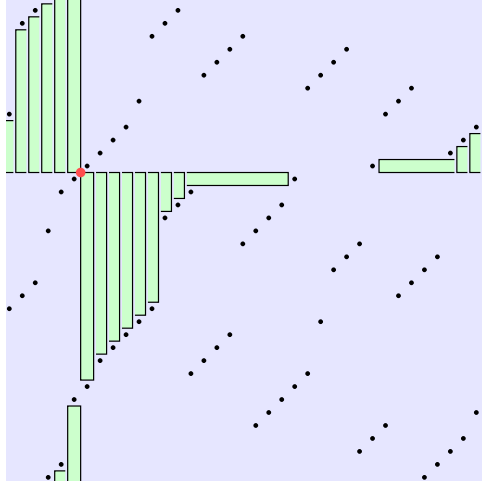

$$x_{28,23,5,24} = x_{5,24,6,6}$$

(146)

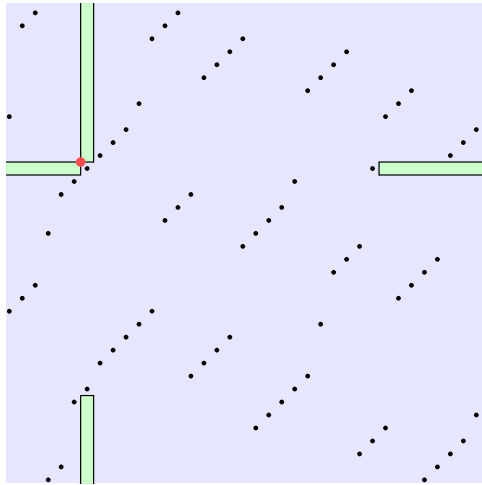

$$x_{34,23,5,25} = x_{5,25,7,6}$$

(147)

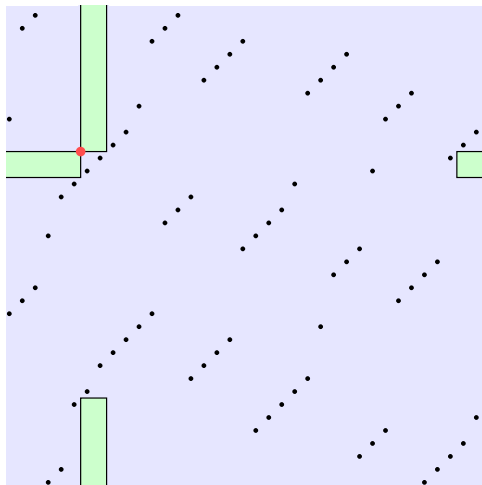

$$x_{35,23,5,26} = x_{5,26,8,6} \quad (148)$$

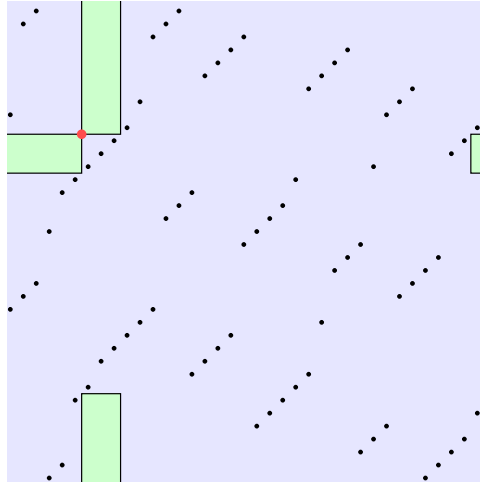

$$x_{36,23,5,27} = x_{5,27,9,6} \quad (149)$$

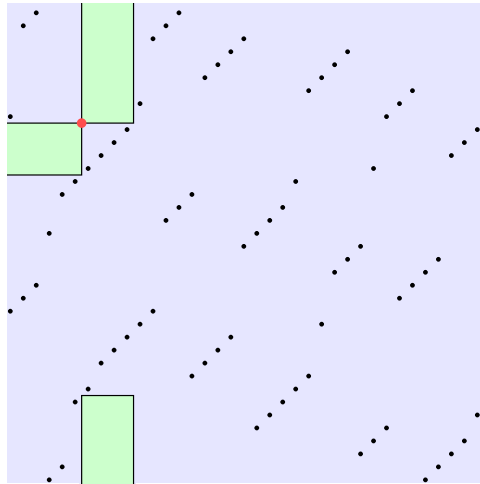

$$0 = x_{5,29,10,6} \quad (150)$$

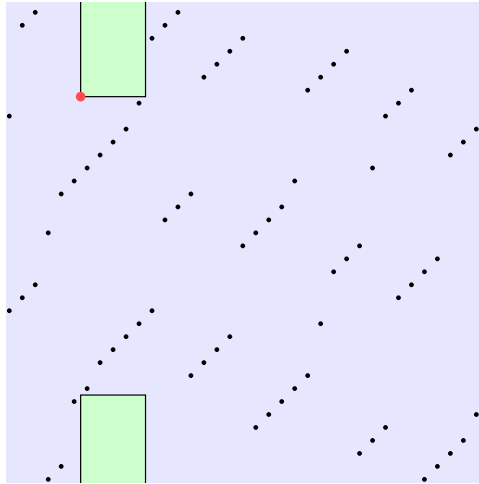

$$x_{0,23,5,34} = x_{5,34,11,6}$$

(151)

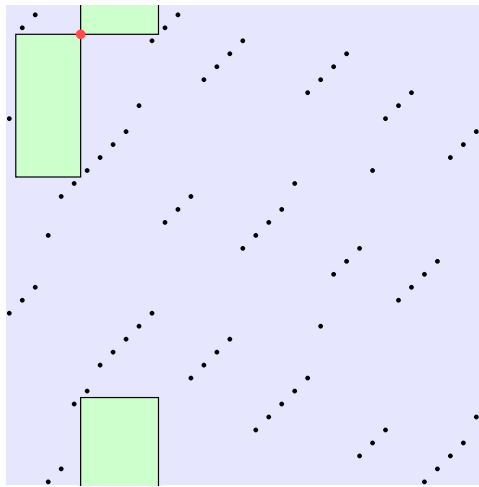

$$x_{1,23,5,35} = x_{5,35,12,6}$$

(152)

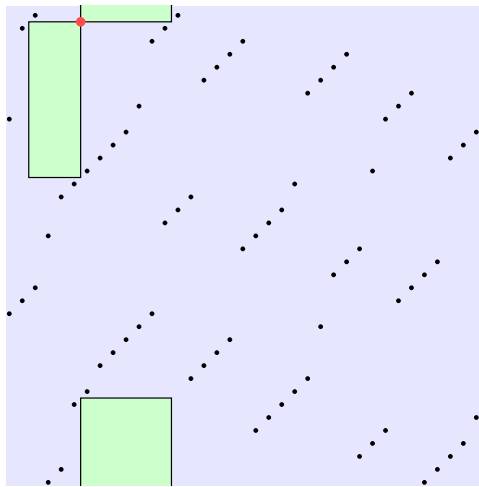

$$x_{2,23,5,36} = x_{5,36,18,6}$$

(153)

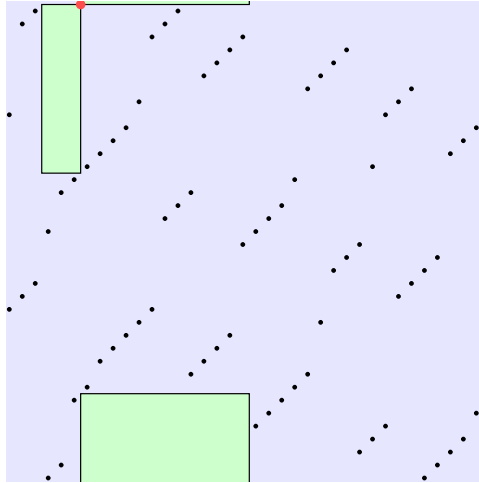

$$x_{3,24,6,0} = 0$$

(154)

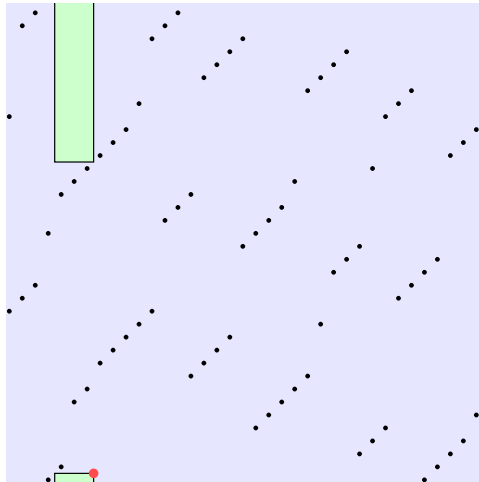

$$0 = x_{6,4,19,7}$$

(155)

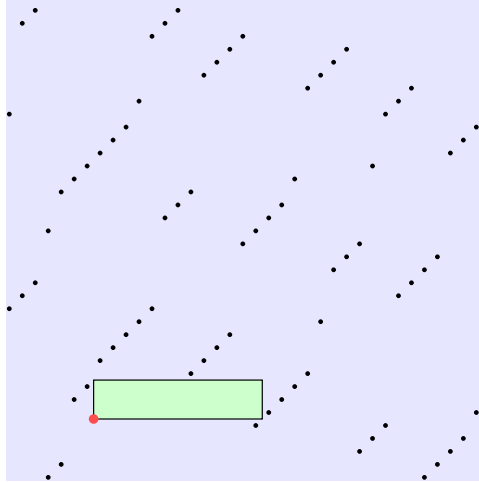

$$x_{4,24,6,5} = x_{6,5,20,7}$$

(156)

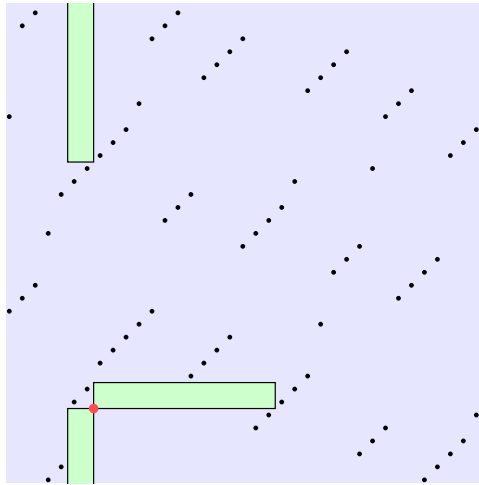

$$x_{5,24,6,6} = x_{6,6,21,7}$$

(157)

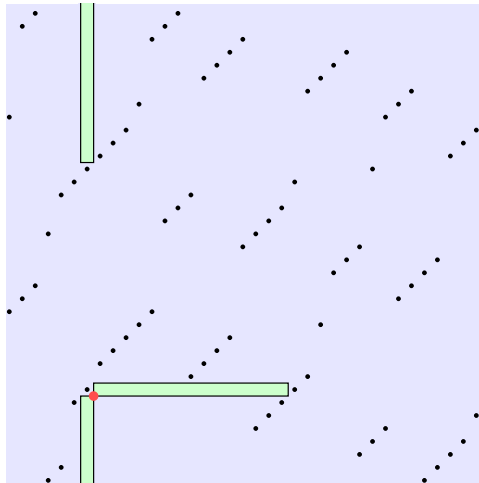



$$\begin{aligned}
x_{0,7,6,13} + x_{1,7,6,14} + x_{2,7,6,18} + x_{3,7,6,21} + x_{4,7,6,22} + x_{5,7,6,23} + x_{23,7,6,11} + x_{24,7,6,12} = \\
= x_{6,4,19,7} + x_{6,5,20,7} + x_{6,6,21,7} + x_{6,36,18,7}
\end{aligned} \tag{158}$$

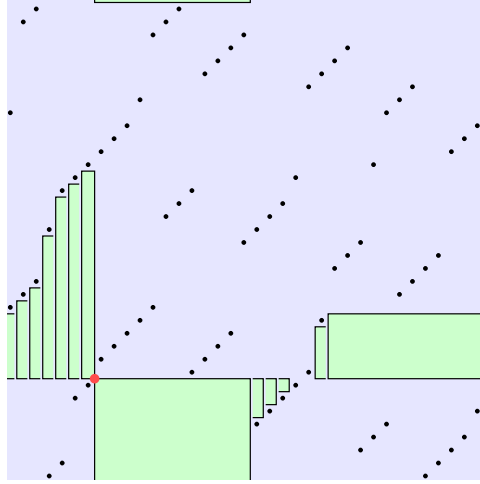

$$x_{15,8,6,9} + x_{16,8,6,10} + x_{17,8,6,11} = x_{6,25,7,8} + x_{6,26,8,8} + x_{6,27,9,8} + x_{6,29,10,8} + x_{6,34,11,8} + x_{6,35,12,8} + x_{6,36,13,8} \tag{159}$$

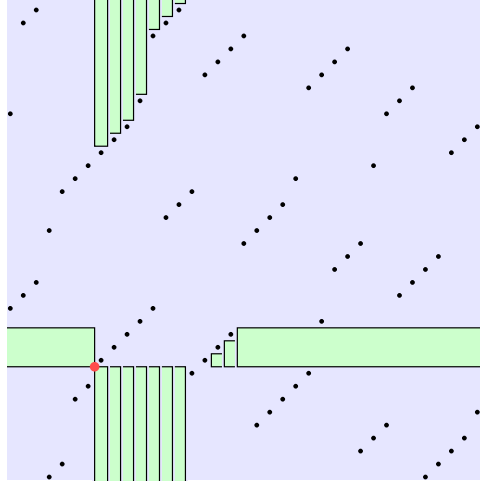

$$x_{15,8,6,9} = x_{6,9,7,24} \tag{160}$$

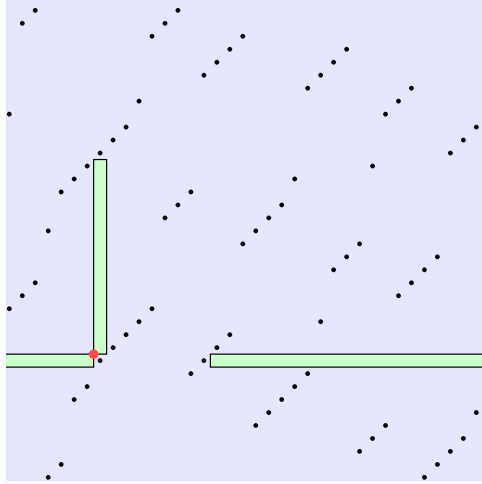

$$x_{16,8,6,10} = x_{6,10,8,24}$$

(161)

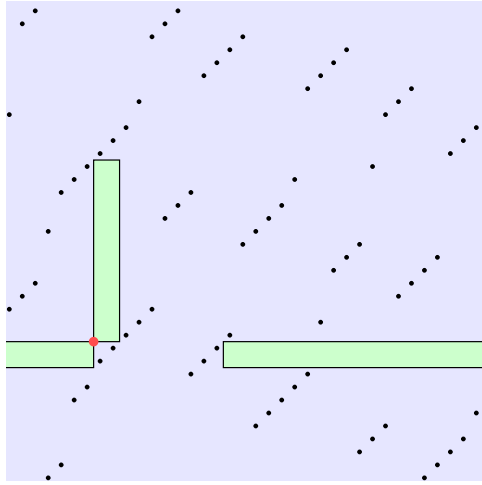

$$x_{17,8,6,11} + x_{23,7,6,11} = x_{6,11,9,24}$$

(162)

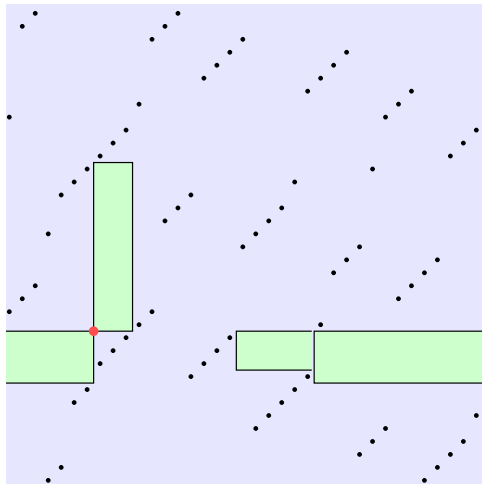

$$x_{24,7,6,12} = x_{6,12,10,24} \tag{163}$$

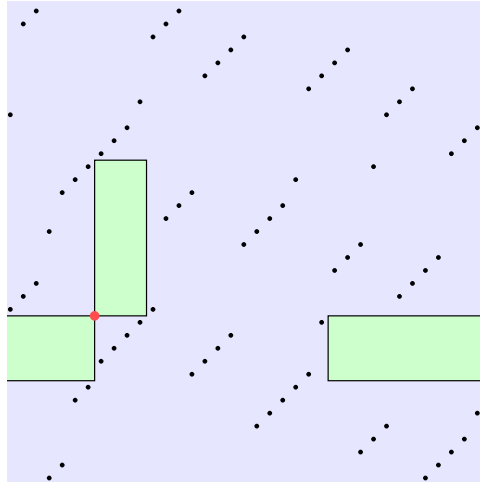

$$x_{0,7,6,13} = x_{6,13,11,24} \tag{164}$$

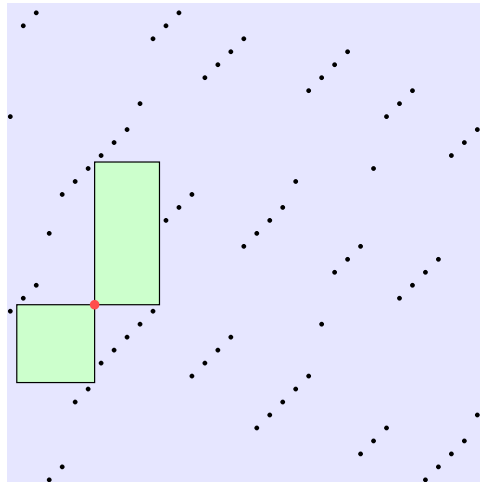

$$x_{1,7,6,14} = 0 \tag{165}$$

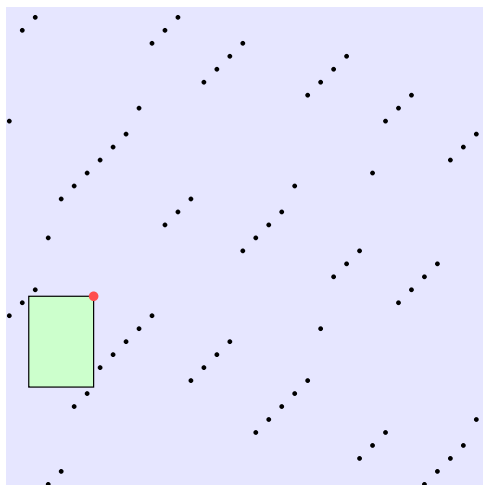

$$x_{2,7,6,18} = 0$$

(166)

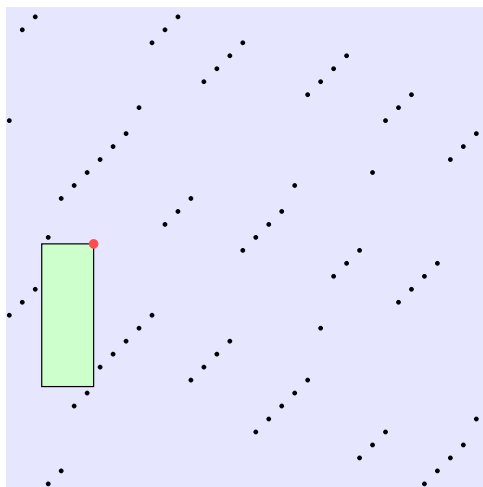

$$0 = x_{6,20,12,24}$$

(167)

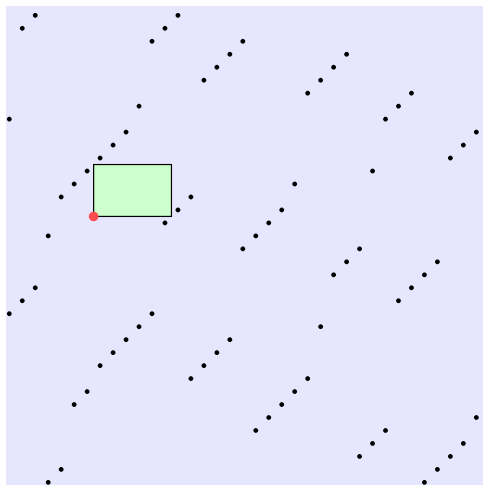

$$x_{3,7,6,21} = x_{6,21,13,24}$$

(168)

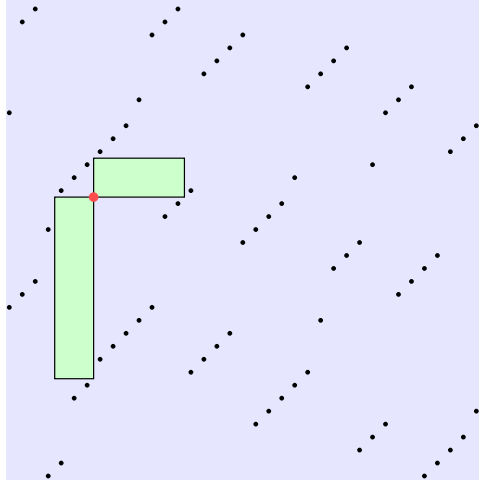

$$x_{4,7,6,22} = x_{6,22,21,24}$$

(169)

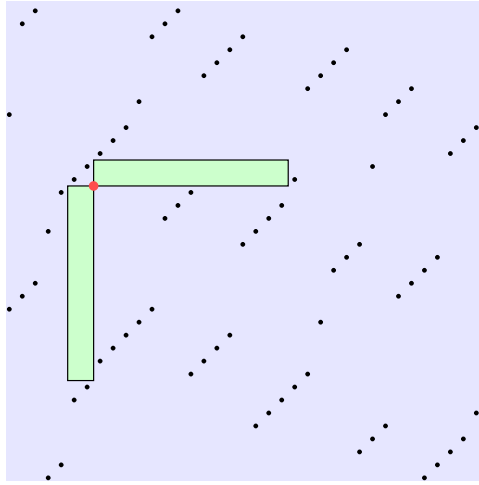

$$x_{5,7,6,23} = x_{6,23,27,24}$$

(170)

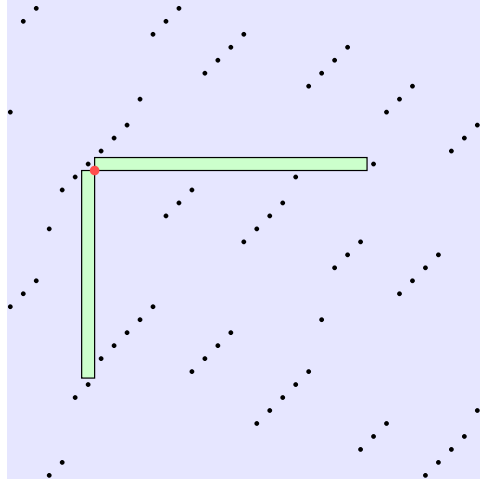

$$\begin{aligned}
 & x_{0,24,6,34} + x_{1,24,6,35} + x_{2,24,6,36} + x_{3,24,6,0} + x_{4,24,6,5} + x_{5,24,6,6} + x_{34,24,6,25} + x_{35,24,6,26} + x_{36,24,6,27} = \\
 & = x_{6,9,7,24} + x_{6,10,8,24} + x_{6,11,9,24} + x_{6,12,10,24} + x_{6,13,11,24} + x_{6,20,12,24} + x_{6,21,13,24} + x_{6,22,21,24} + x_{6,23,27,24} \quad (171)
 \end{aligned}$$

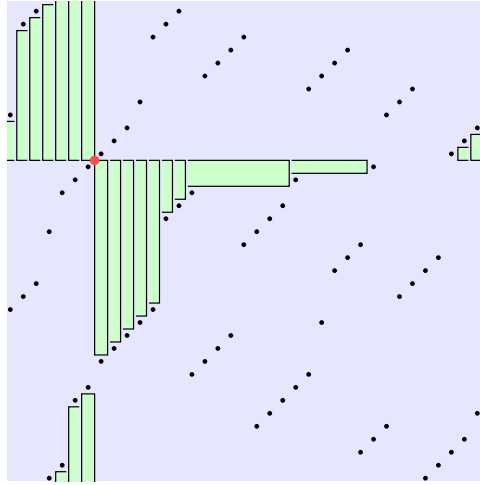

$$x_{34,24,6,25} = x_{6,25,7,8} \quad (172)$$

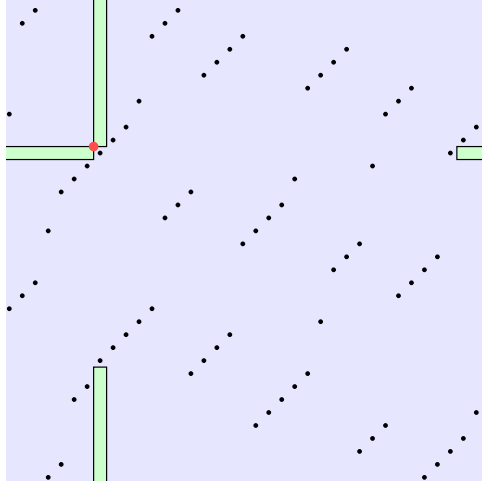

$$x_{35,24,6,26} = x_{6,26,8,8}$$

(173)

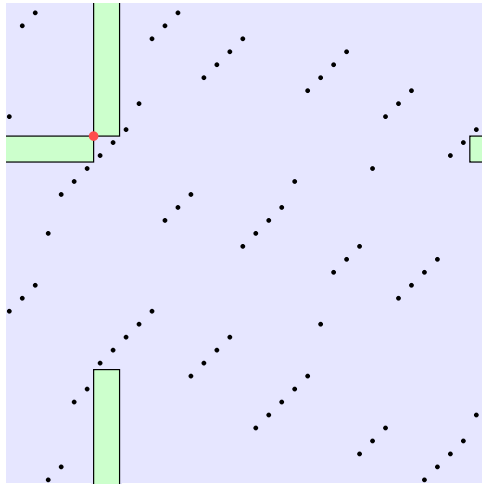

$$x_{36,24,6,27} = x_{6,27,9,8}$$

(174)

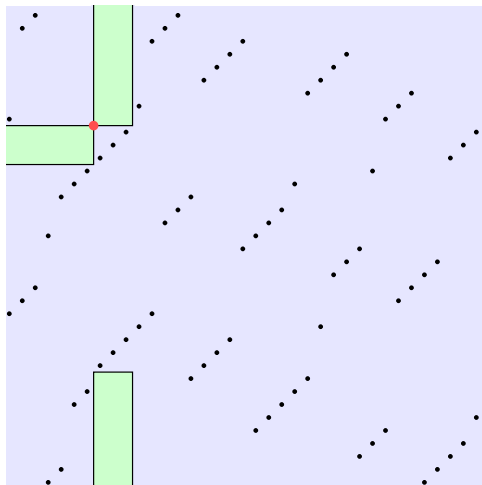

$$0 = x_{6,29,10,8}$$

(175)

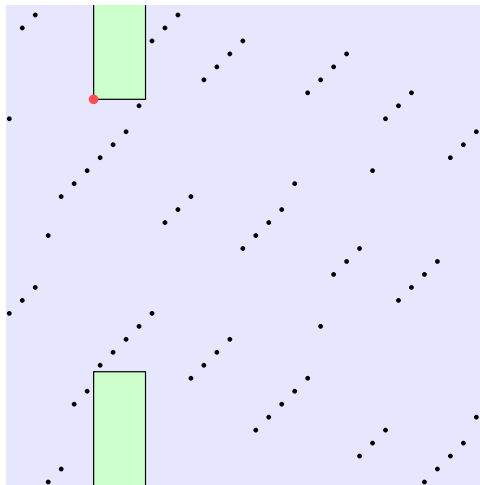

$$x_{0,24,6,34} = x_{6,34,11,8}$$

(176)

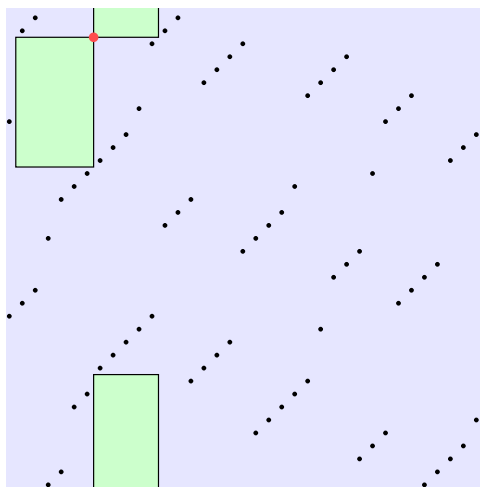

$$x_{1,24,6,35} = x_{6,35,12,8}$$

(177)



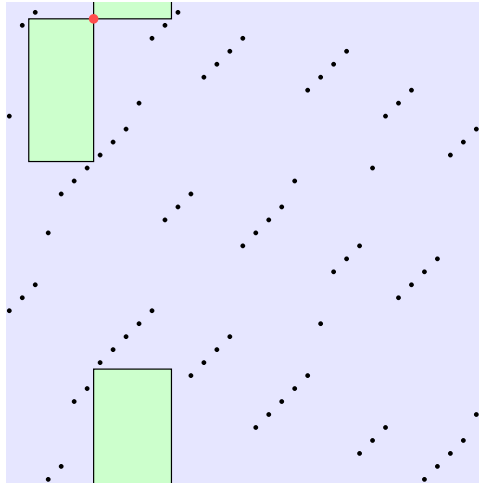

$$x_{2,24,6,36} = x_{6,36,13,8} + x_{6,36,18,7}$$

(178)

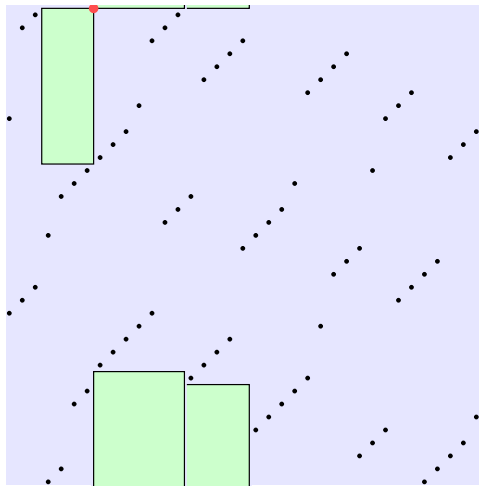

$$x_{3,25,7,0} = 0$$

(179)

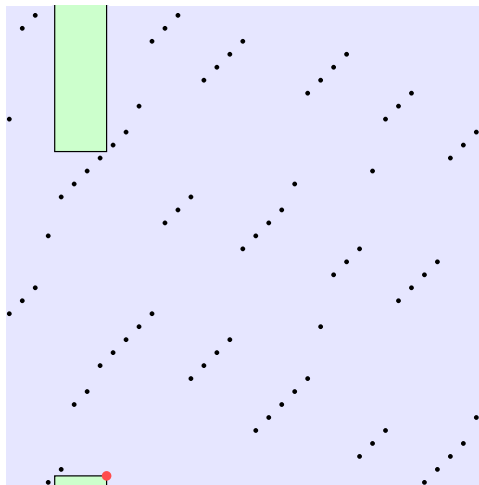

$$x_{4,25,7,5} = 0 \tag{180}$$

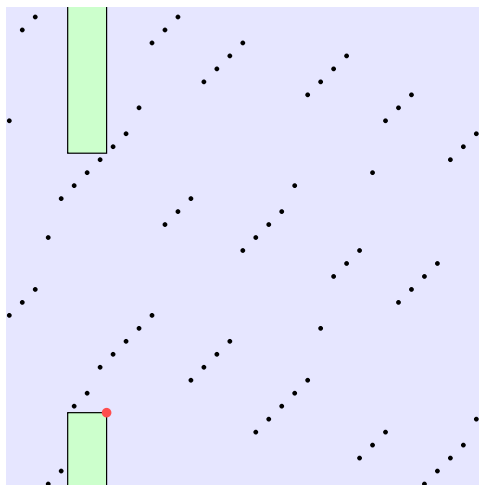

$$x_{5,25,7,6} = 0 \tag{181}$$

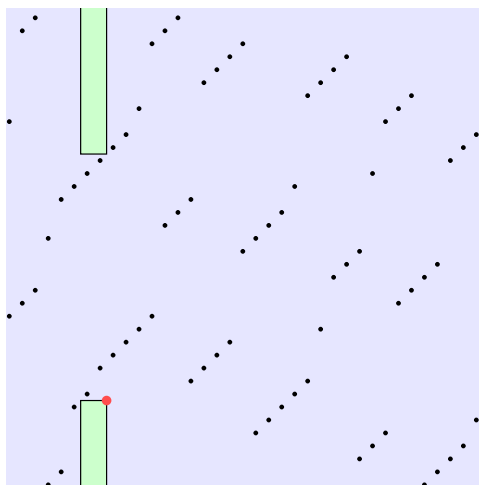

$$x_{6,25,7,8} = x_{7,8,14,9} \tag{182}$$

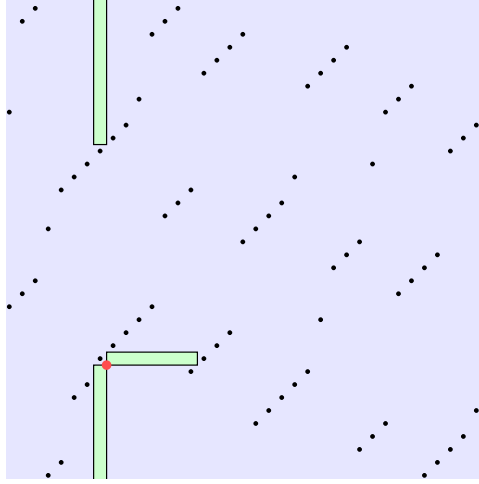

$$\begin{aligned}
 & x_{0,9,7,13} + x_{1,9,7,14} + x_{2,9,7,18} + x_{3,9,7,21} + x_{4,9,7,22} + x_{5,9,7,23} + x_{6,9,7,24} + x_{16,9,7,10} + x_{17,9,7,11} + x_{24,9,7,12} = \\
 & = x_{7,8,14,9} + x_{7,26,8,9} + x_{7,27,9,9} + x_{7,29,10,9} + x_{7,34,11,9} + x_{7,35,12,9} + x_{7,36,13,9} \quad (183)
 \end{aligned}$$

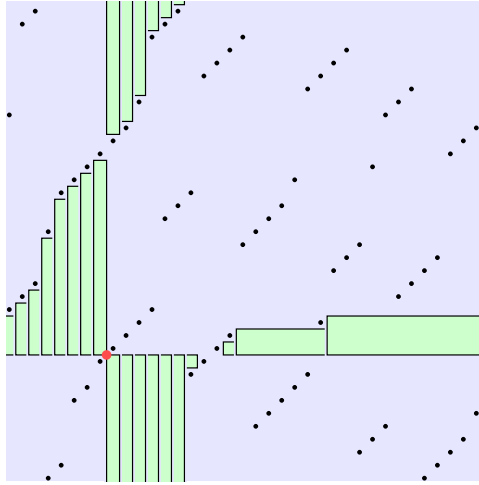

$$x_{16,9,7,10} = x_{7,10,8,25} \quad (184)$$

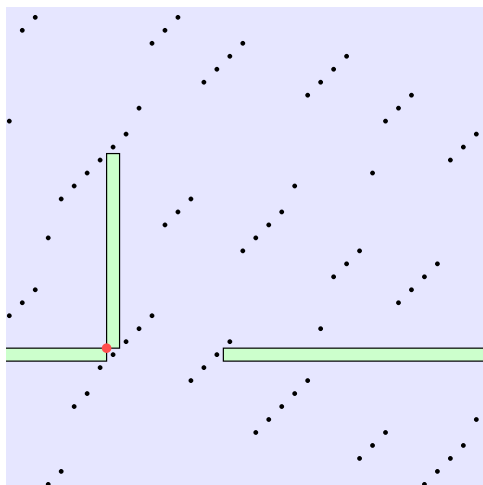

$$x_{17,9,7,11} = x_{7,11,9,25}$$

(185)

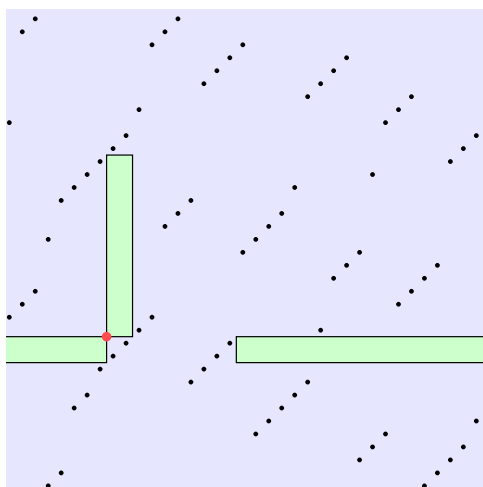

$$x_{24,9,7,12} = x_{7,12,10,25}$$

(186)

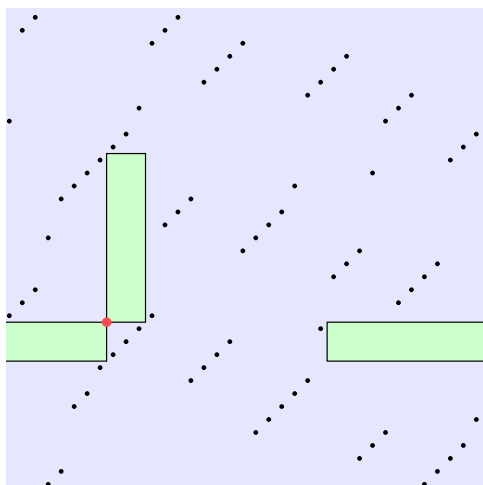

$$x_{0,9,7,13} = x_{7,13,11,25}$$

(187)

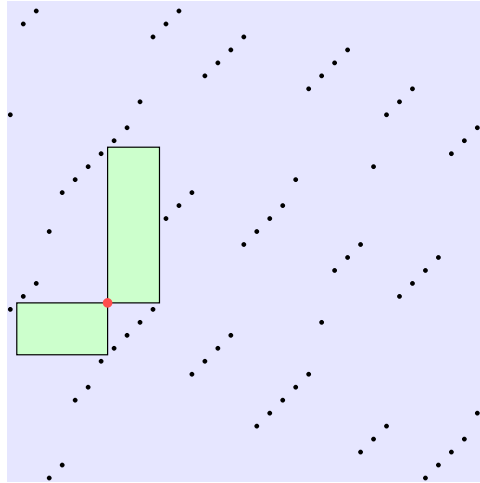

$$x_{1,9,7,14} = 0$$

(188)

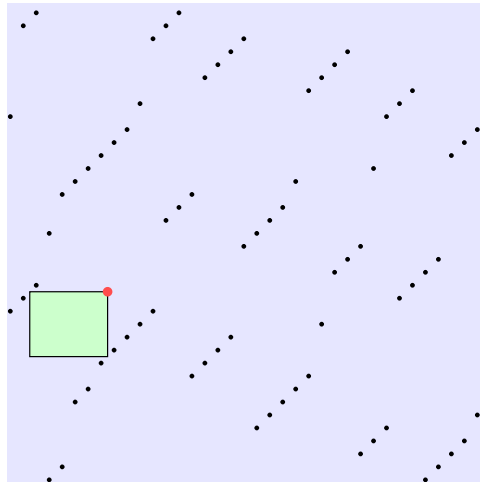

$$x_{2,9,7,18} = 0$$

(189)

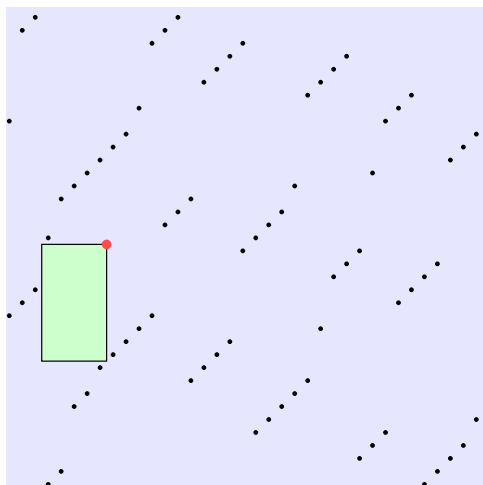

$$0 = x_{7,20,12,25}$$

(190)

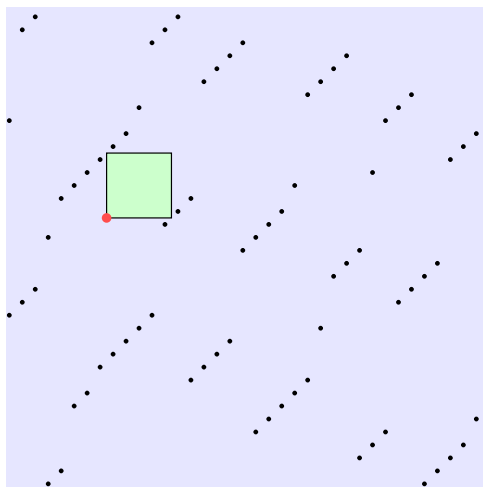

$$x_{3,9,7,21} = x_{7,21,13,25}$$

(191)

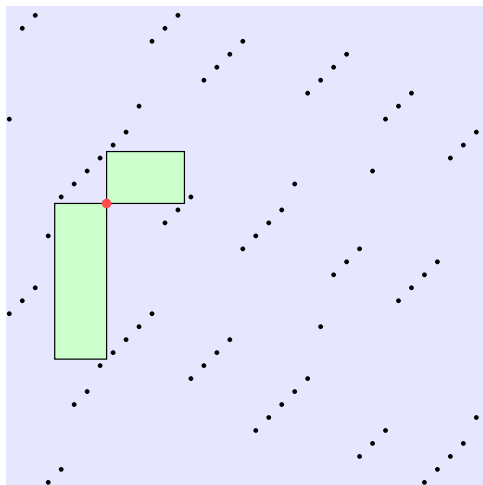

$$x_{4,9,7,22} = x_{7,22,21,25}$$

(192)

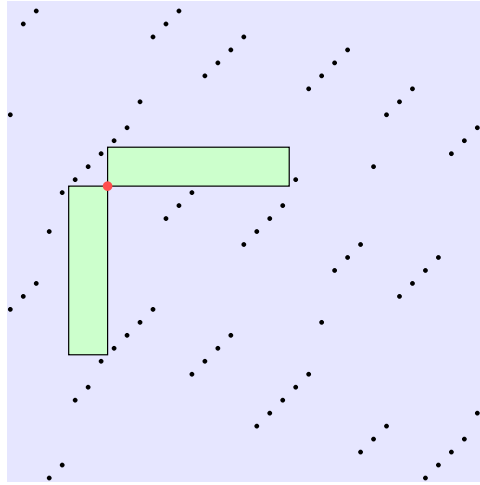

$$x_{5,9,7,23} = x_{7,23,27,25}$$

(193)

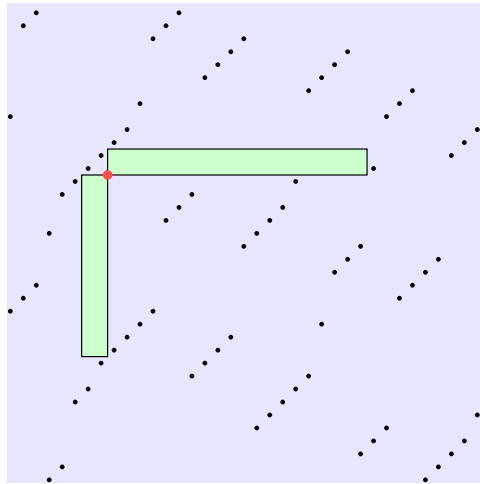

$$x_{6,9,7,24} = x_{7,24,33,25}$$

(194)

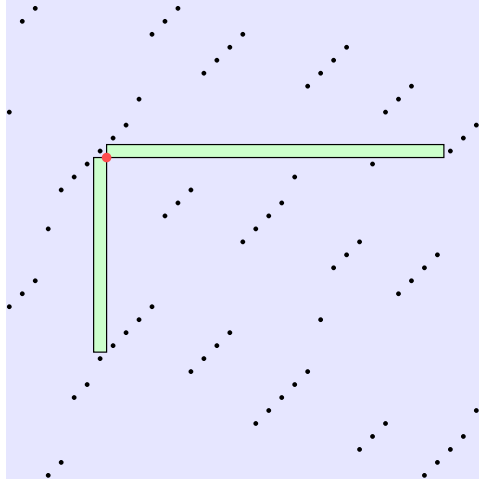

$$\begin{aligned}
 & x_{0,25,7,34} + x_{1,25,7,35} + x_{2,25,7,36} + x_{3,25,7,0} + x_{4,25,7,5} + x_{5,25,7,6} + x_{6,25,7,8} + x_{35,25,7,26} + x_{36,25,7,27} = \\
 & = x_{7,10,8,25} + x_{7,11,9,25} + x_{7,12,10,25} + x_{7,13,11,25} + x_{7,20,12,25} + x_{7,21,13,25} + x_{7,22,21,25} + x_{7,23,27,25} + x_{7,24,33,25} \quad (195)
 \end{aligned}$$

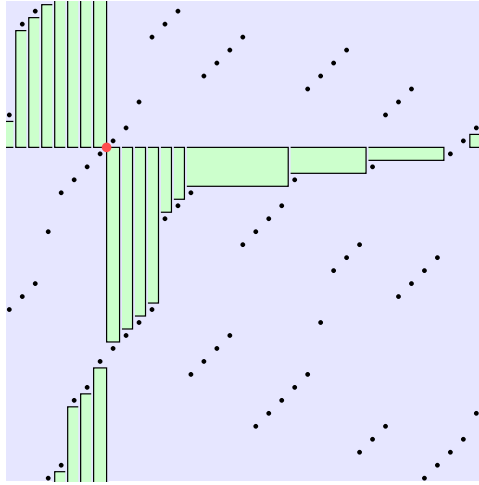

$$x_{35,25,7,26} = x_{7,26,8,9} \quad (196)$$



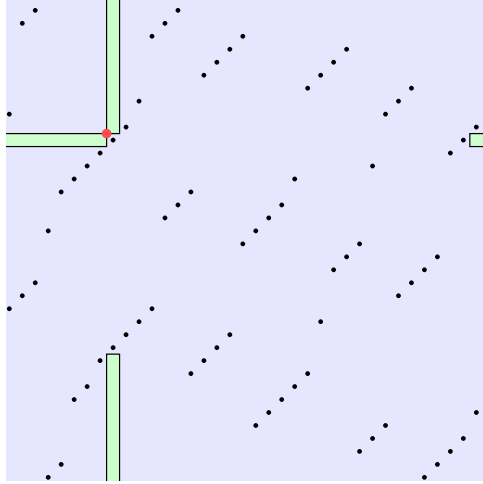

$$x_{36,25,7,27} = x_{7,27,9,9}$$

(197)

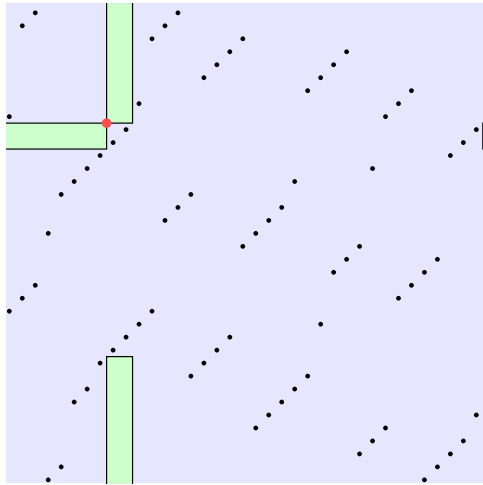

$$0 = x_{7,29,10,9}$$

(198)

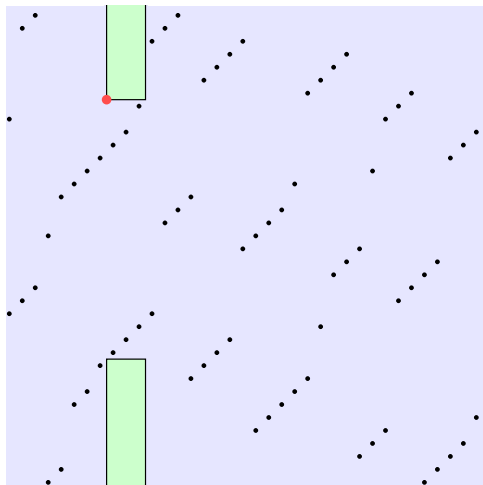

$$x_{0,25,7,34} = x_{7,34,11,9}$$

(199)

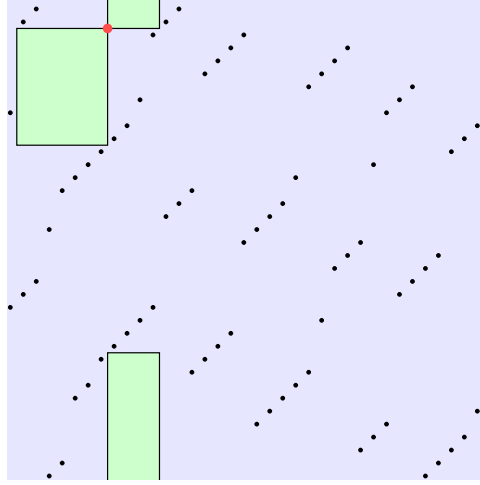

$$x_{1,25,7,35} = x_{7,35,12,9}$$

(200)

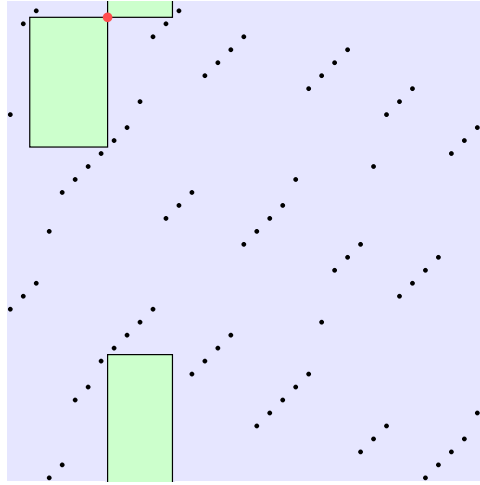

$$x_{2,25,7,36} = x_{7,36,13,9}$$

(201)

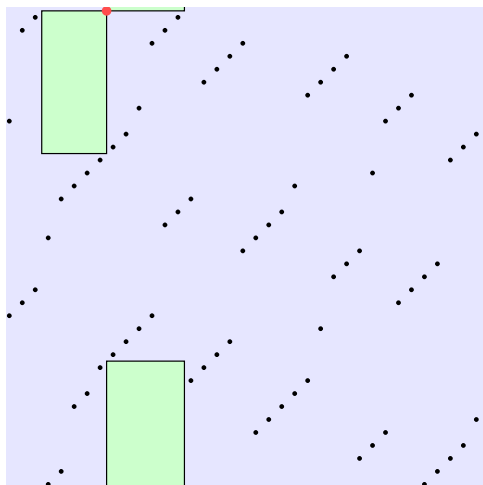

$$x_{3,26,8,0} = 0$$

(202)

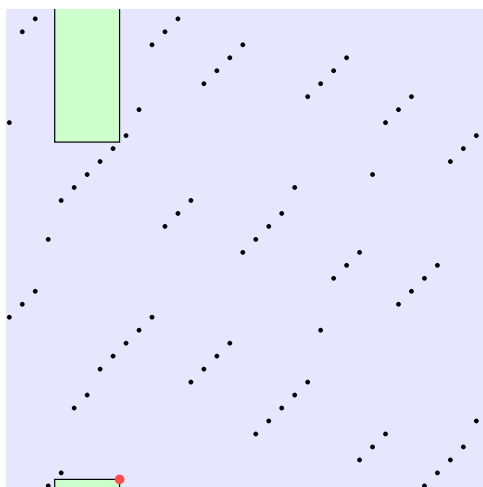

$$x_{4,26,8,5} = 0$$

(203)

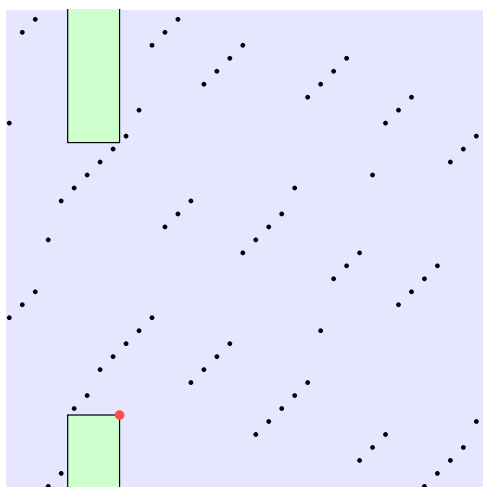

$$x_{5,26,8,6} = 0 \tag{204}$$

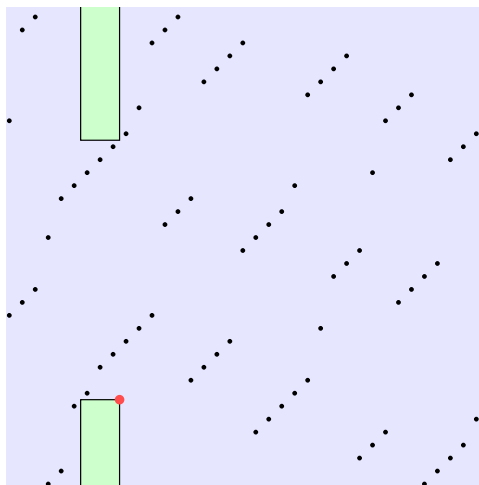

$$x_{6,26,8,8} = x_{8,8,14,10} \tag{205}$$

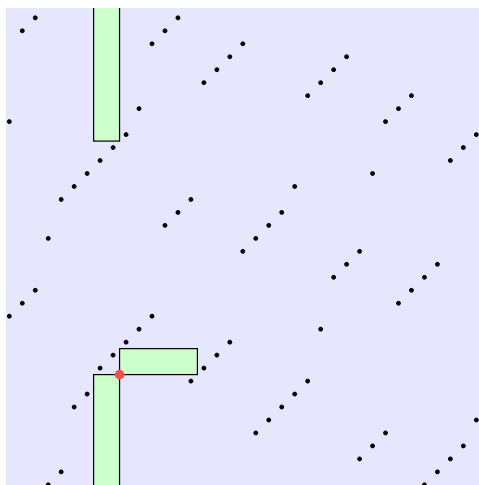

$$x_{7,26,8,9} = x_{8,9,15,10} \tag{206}$$

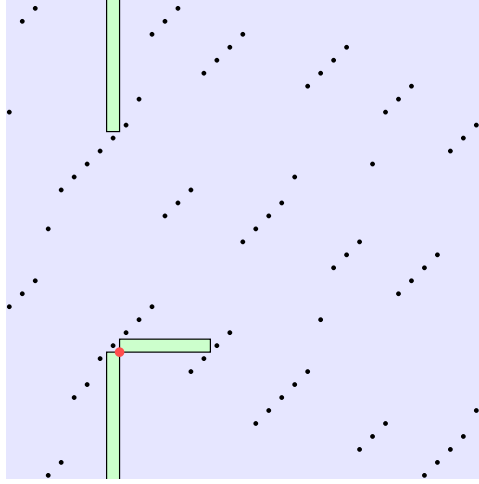

$$\begin{aligned}
 & x_{0,10,8,13} + x_{1,10,8,14} + x_{2,10,8,18} + x_{3,10,8,21} + x_{4,10,8,22} + x_{5,10,8,23} + x_{6,10,8,24} + x_{7,10,8,25} + x_{17,10,8,11} + x_{24,10,8,12} = \\
 & = x_{8,8,14,10} + x_{8,9,15,10} + x_{8,27,9,10} + x_{8,29,10,10} + x_{8,34,11,10} + x_{8,35,12,10} + x_{8,36,13,10} \quad (207)
 \end{aligned}$$

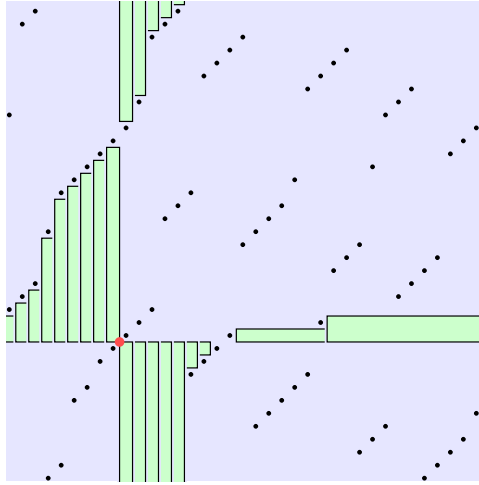

$$x_{17,10,8,11} = x_{8,11,9,26} \quad (208)$$

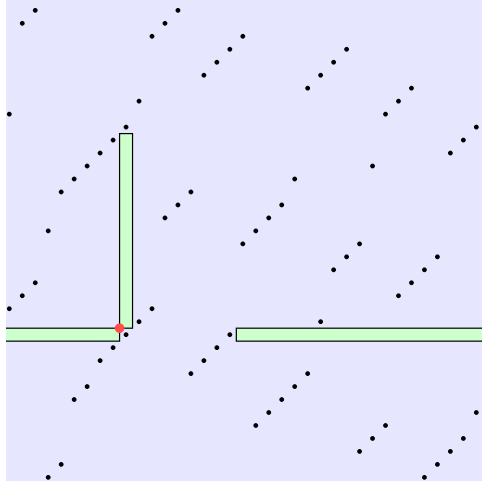

$$x_{24,10,8,12} = x_{8,12,10,26}$$

(209)

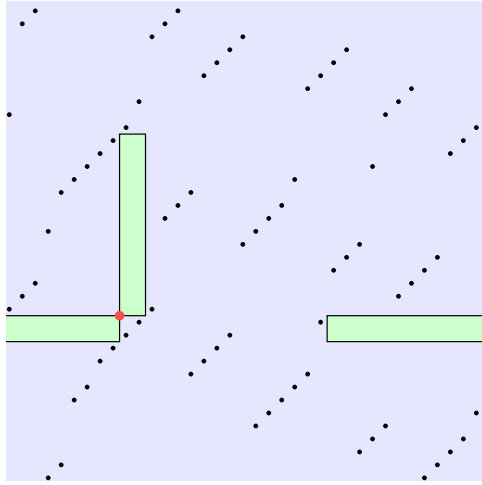

$$x_{0,10,8,13} = x_{8,13,11,26}$$

(210)

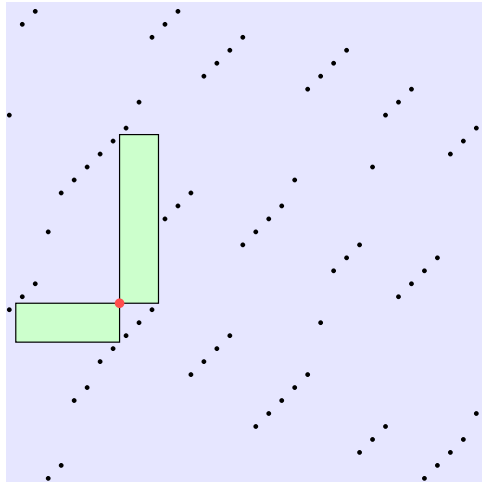

$$x_{1,10,8,14} = 0 \tag{211}$$

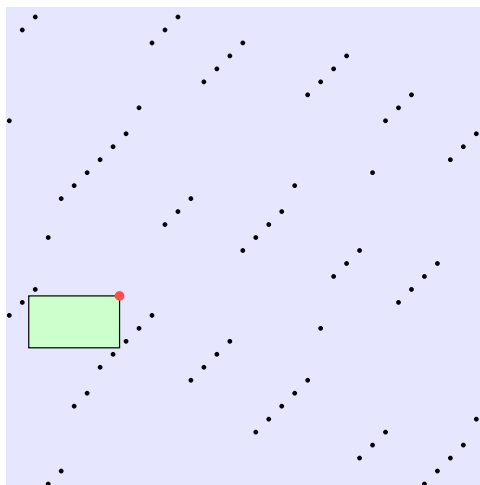

$$x_{2,10,8,18} = 0 \tag{212}$$

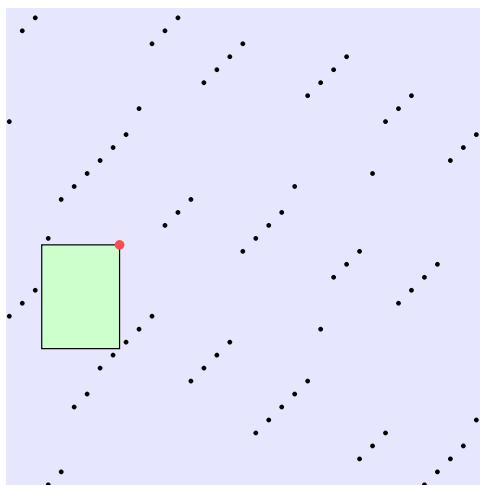

$$0 = x_{8,20,12,26} \tag{213}$$

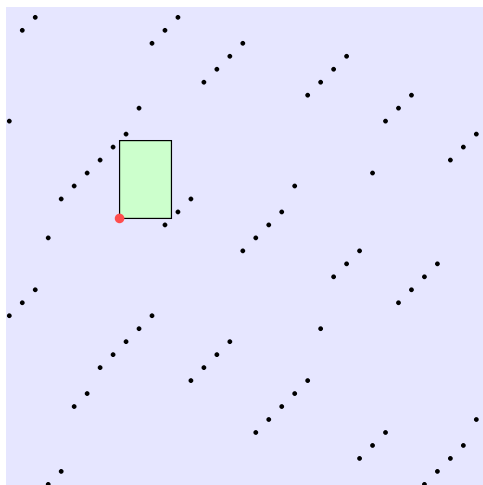

$$x_{3,10,8,21} = x_{8,21,13,26}$$

(214)

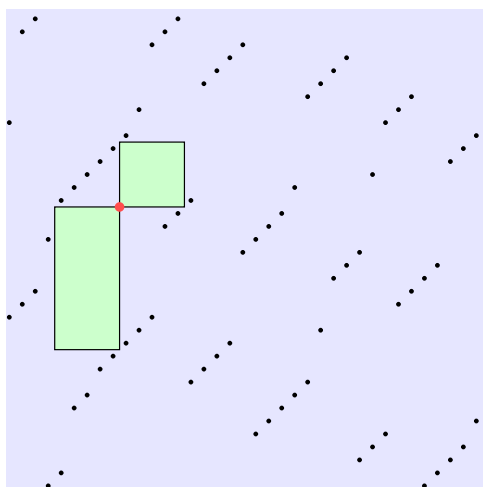

$$x_{4,10,8,22} = x_{8,22,21,26}$$

(215)

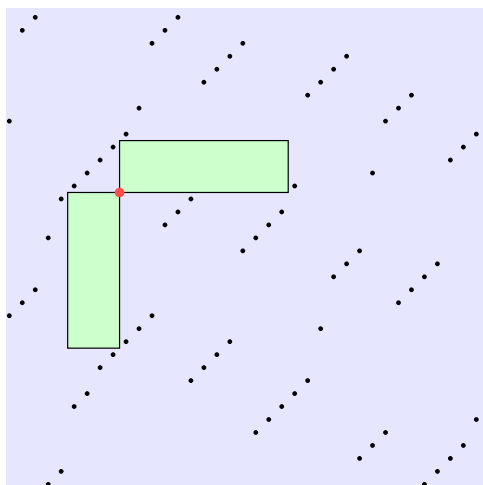



$$x_{5,10,8,23} = x_{8,23,27,26} \quad (216)$$

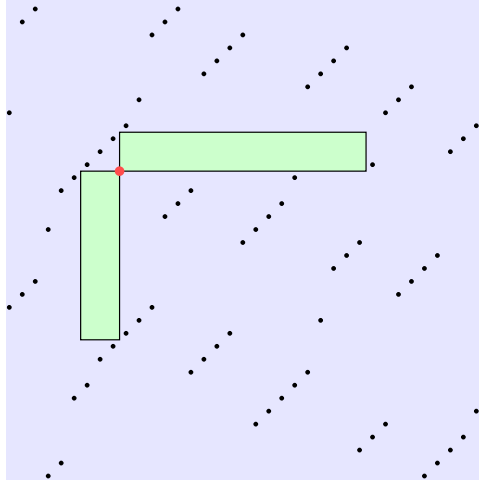

$$x_{6,10,8,24} = x_{8,24,33,26} \quad (217)$$

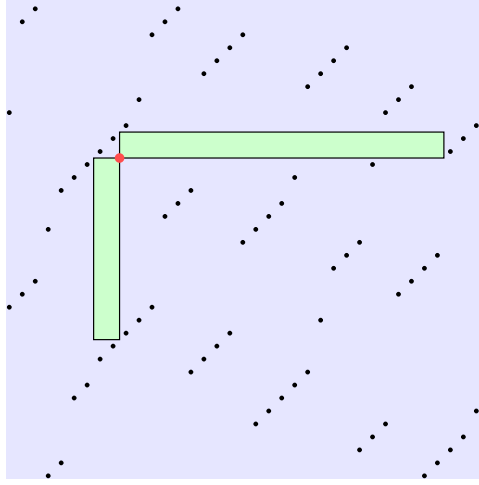

$$x_{7,10,8,25} = x_{8,25,34,26} \quad (218)$$

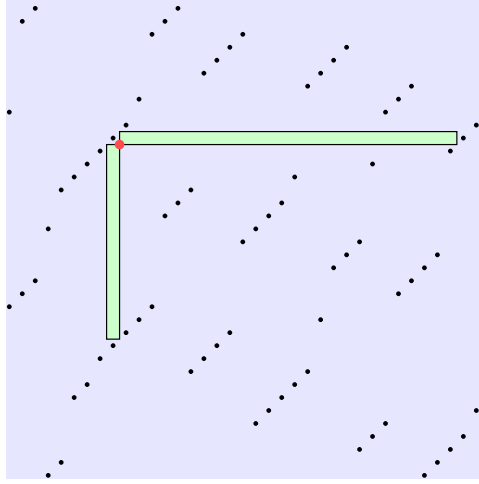

$$\begin{aligned}
 & x_{0,26,8,34} + x_{1,26,8,35} + x_{2,26,8,36} + x_{3,26,8,0} + x_{4,26,8,5} + x_{5,26,8,6} + x_{6,26,8,8} + x_{7,26,8,9} + x_{36,26,8,27} = \\
 & = x_{8,11,9,26} + x_{8,12,10,26} + x_{8,13,11,26} + x_{8,20,12,26} + x_{8,21,13,26} + x_{8,22,21,26} + x_{8,23,27,26} + x_{8,24,33,26} + x_{8,25,34,26} \quad (219)
 \end{aligned}$$

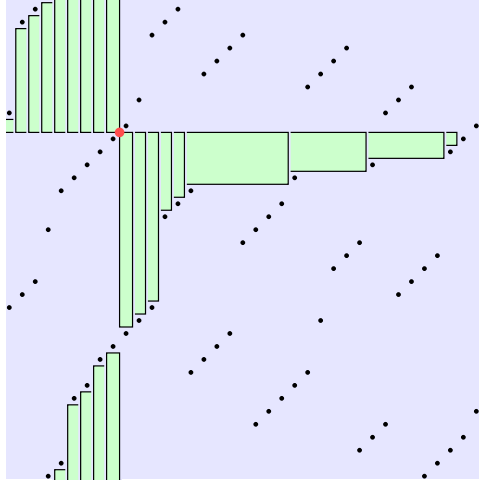

$$x_{36,26,8,27} = x_{8,27,9,10} \quad (220)$$

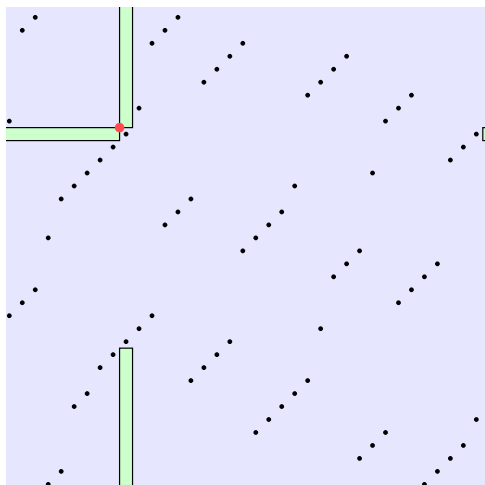

$$0 = x_{8,29,10,10}$$

(221)

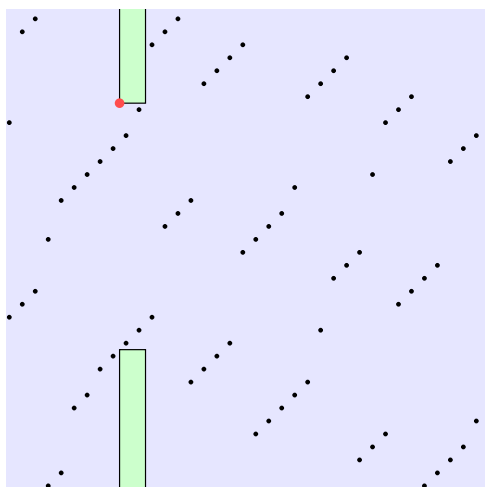

$$x_{0,26,8,34} = x_{8,34,11,10}$$

(222)

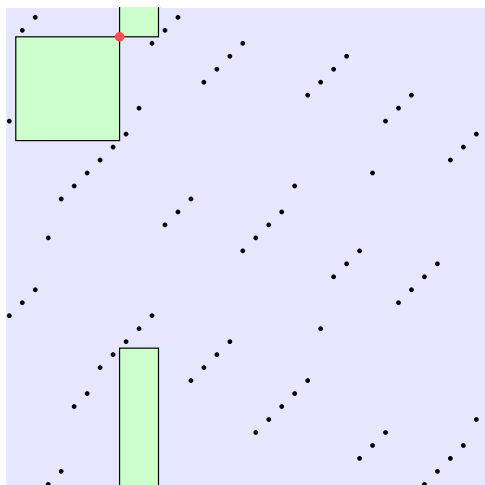

$$x_{1,26,8,35} = x_{8,35,12,10}$$

(223)

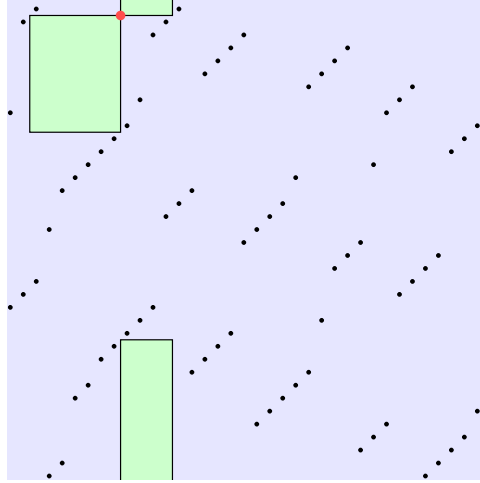

$$x_{2,26,8,36} = x_{8,36,13,10}$$

(224)

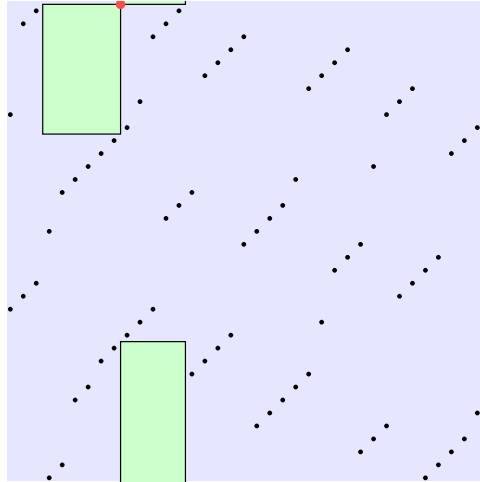

$$x_{3,27,9,0} = 0$$

(225)

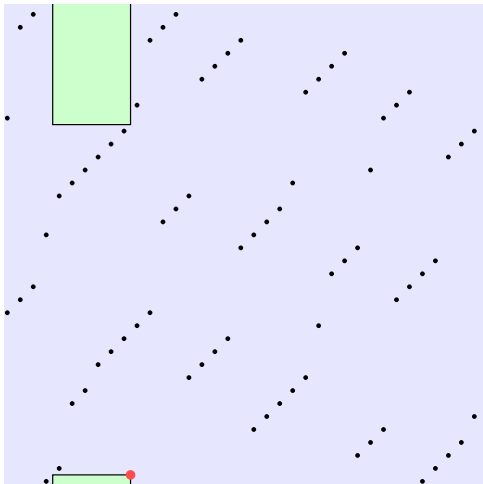

$$x_{4,27,9,5} = 0$$

(226)

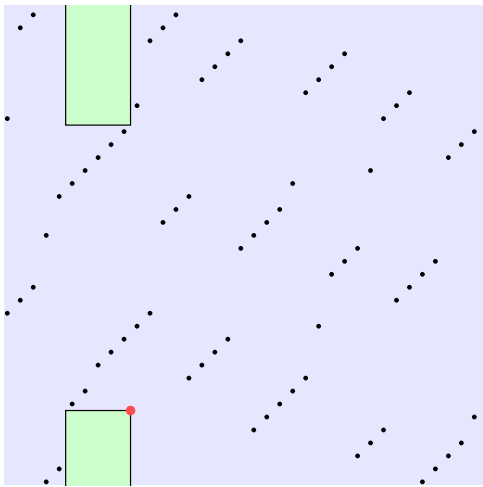

$$x_{5,27,9,6} = 0$$

(227)

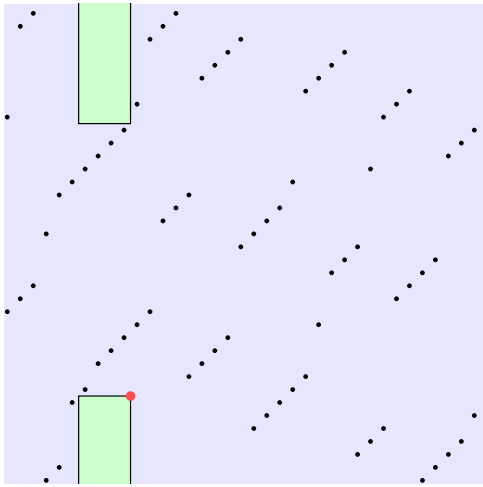

$$x_{6,27,9,8} = x_{9,8,14,11}$$

(228)

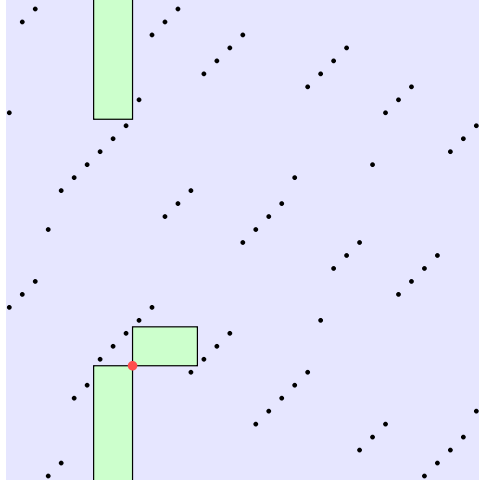

$$x_{7,27,9,9} = x_{9,9,15,11}$$

(229)

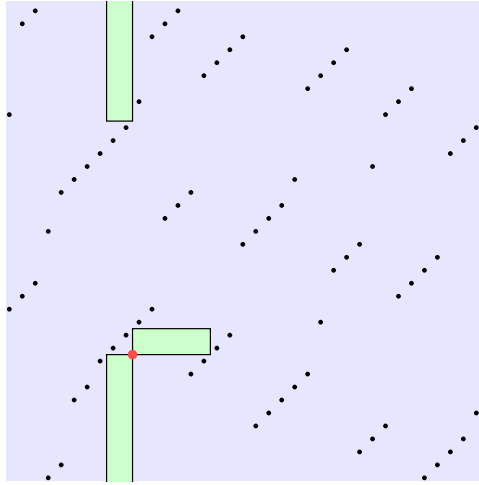

$$x_{8,27,9,10} = x_{9,10,16,11}$$

(230)

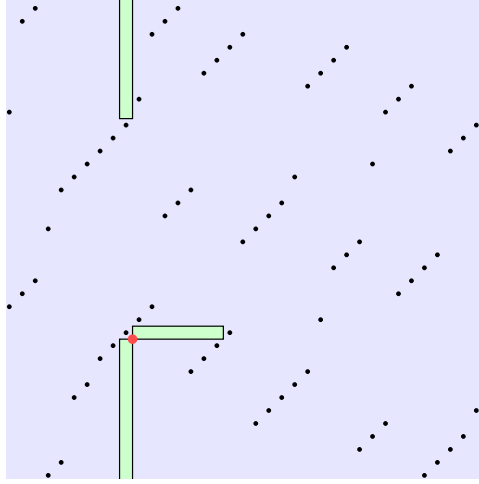

$$\begin{aligned}
 & x_{0,11,9,13} + x_{1,11,9,14} + x_{2,11,9,18} + x_{3,11,9,21} + x_{4,11,9,22} + x_{5,11,9,23} + x_{6,11,9,24} + x_{7,11,9,25} + x_{8,11,9,26} + x_{24,11,9,12} = \\
 & = x_{9,8,14,11} + x_{9,9,15,11} + x_{9,10,16,11} + x_{9,29,10,11} + x_{9,34,11,11} + x_{9,35,12,11} + x_{9,36,13,11} \quad (231)
 \end{aligned}$$

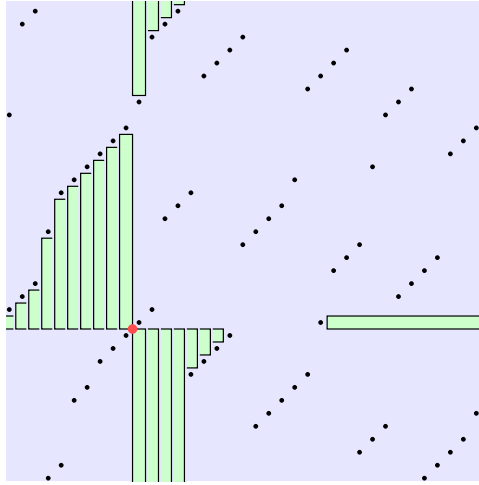

$$x_{24,11,9,12} = x_{9,12,10,28} \quad (232)$$

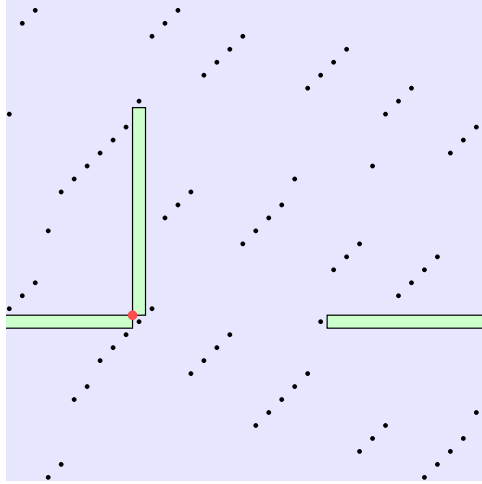

$$x_{0,11,9,13} = x_{9,13,11,28}$$

(233)

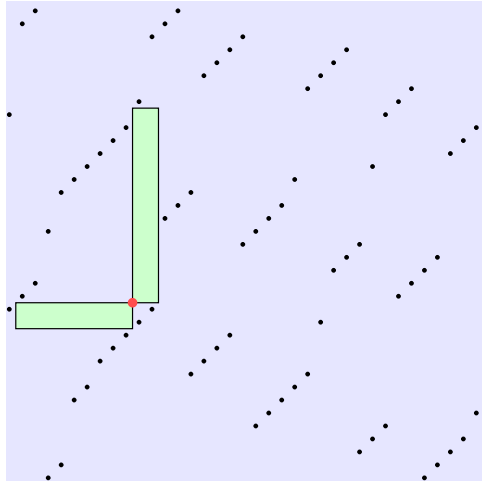

$$x_{1,11,9,14} = 0$$

(234)

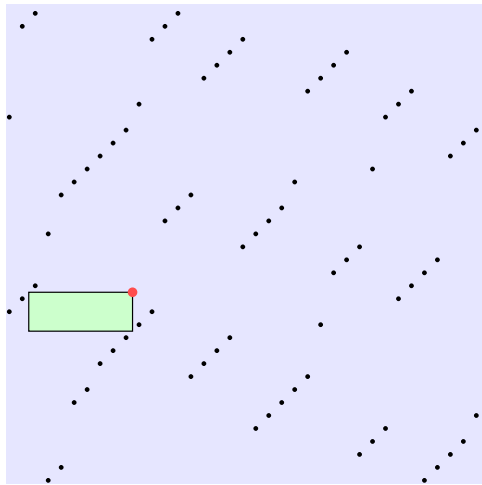



$$x_{2,11,9,18} = 0 \tag{235}$$

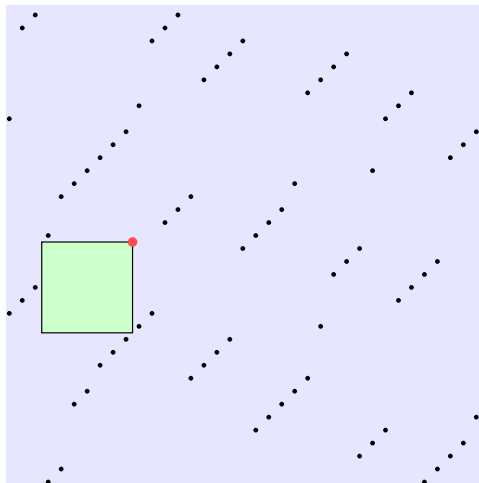

$$0 = x_{9,20,12,28} \tag{236}$$

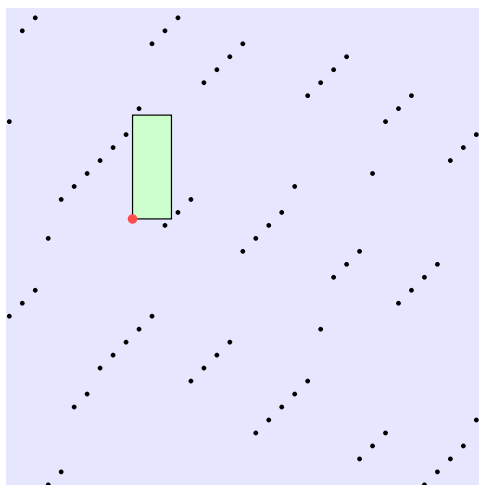

$$x_{3,11,9,21} = x_{9,21,13,28} \tag{237}$$

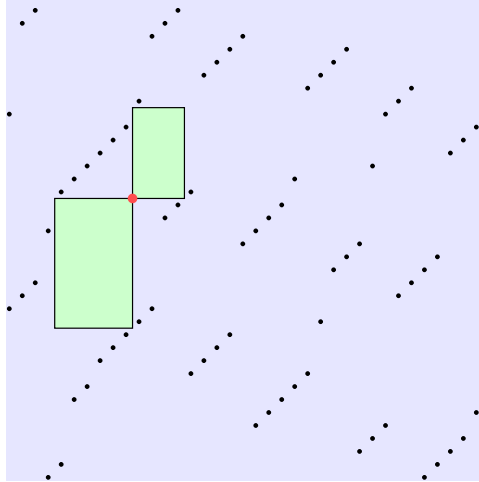

$$x_{4,11,9,22} = x_{9,22,21,28}$$

(238)

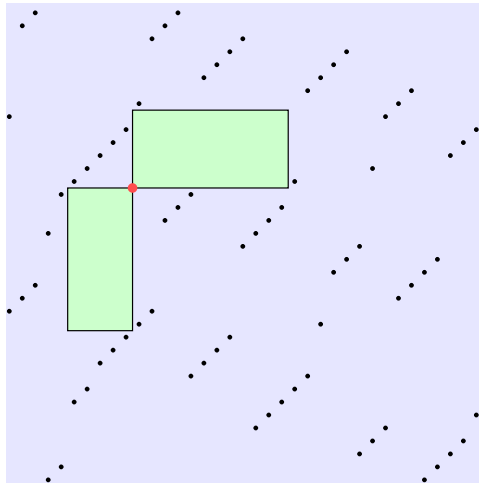

$$x_{5,11,9,23} = x_{9,23,27,28}$$

(239)

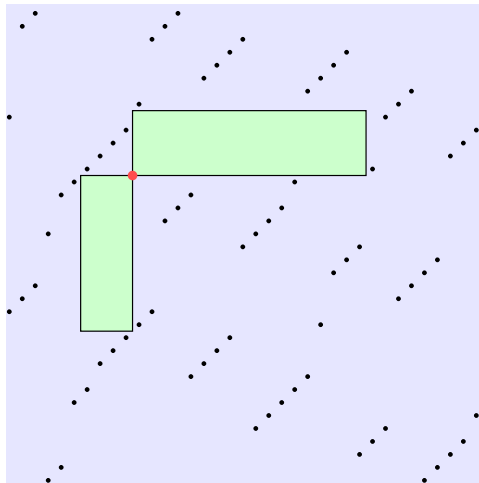

$$x_{6,11,9,24} = x_{9,24,28,28} + x_{9,24,33,27} \quad (240)$$

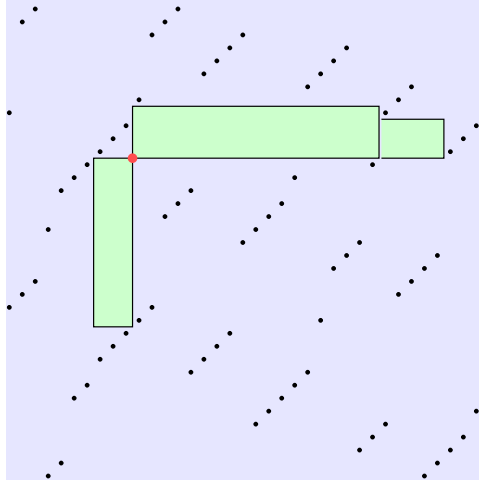

$$x_{7,11,9,25} = x_{9,25,34,27} \quad (241)$$

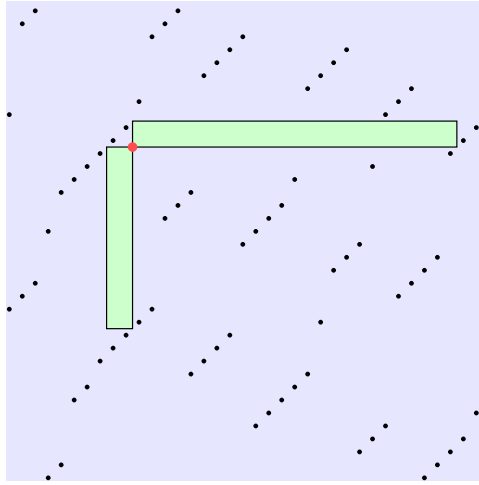

$$x_{8,11,9,26} = x_{9,26,35,27} \quad (242)$$

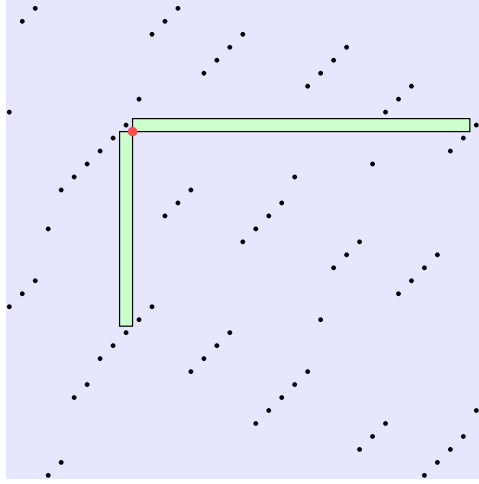

$$\begin{aligned}
 x_{0,27,9,34} + x_{1,27,9,35} + x_{2,27,9,36} + x_{3,27,9,0} + x_{4,27,9,5} + x_{5,27,9,6} + x_{6,27,9,8} + x_{7,27,9,9} + x_{8,27,9,10} = \\
 = x_{9,24,33,27} + x_{9,25,34,27} + x_{9,26,35,27} \quad (243)
 \end{aligned}$$

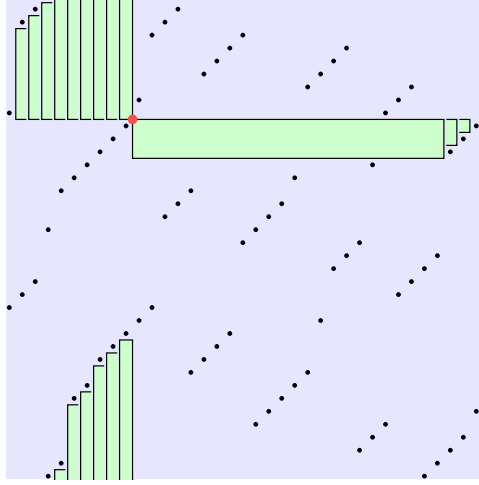

$$x_{30,28,9,29} + x_{31,28,9,34} = x_{9,12,10,28} + x_{9,13,11,28} + x_{9,20,12,28} + x_{9,21,13,28} + x_{9,22,21,28} + x_{9,23,27,28} + x_{9,24,28,28} \quad (244)$$

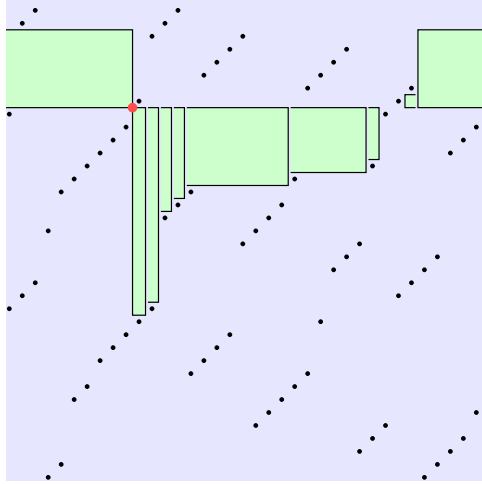

$$x_{30,28,9,29} = x_{9,29,10,11}$$

(245)

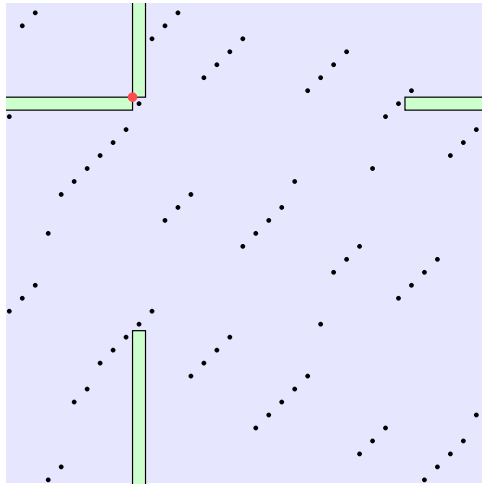

$$x_{0,27,9,34} + x_{31,28,9,34} = x_{9,34,11,11}$$

(246)

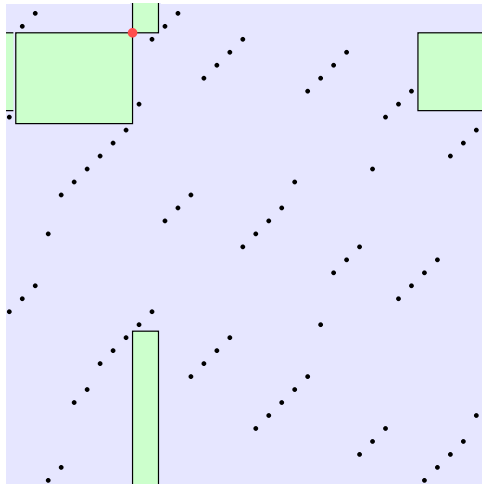

$$x_{1,27,9,35} = x_{9,35,12,11}$$

(247)

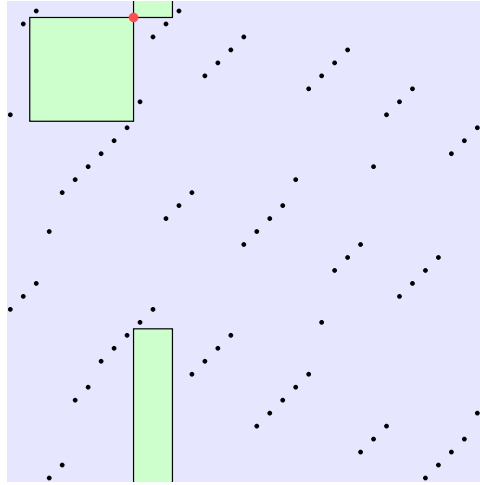

$$x_{2,27,9,36} = x_{9,36,13,11}$$

(248)

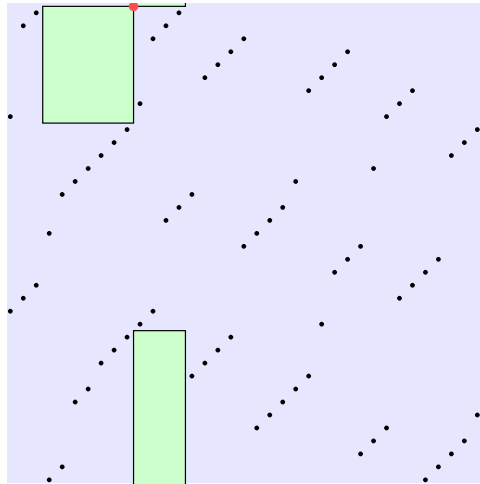

$$x_{3,29,10,0} = 0$$

(249)

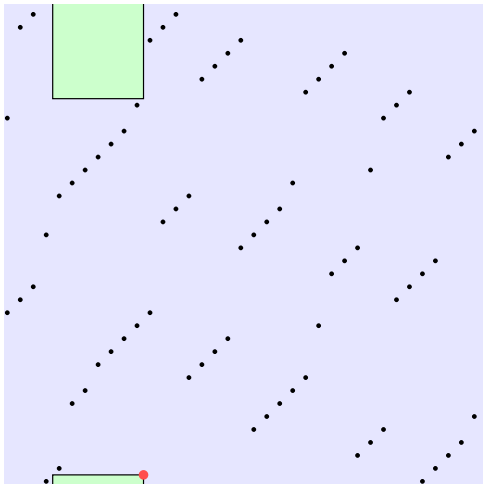

$$x_{4,29,10,5} = 0$$

(250)

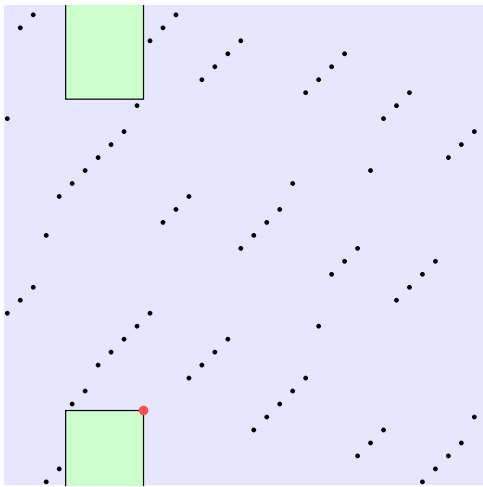

$$x_{5,29,10,6} = 0$$

(251)

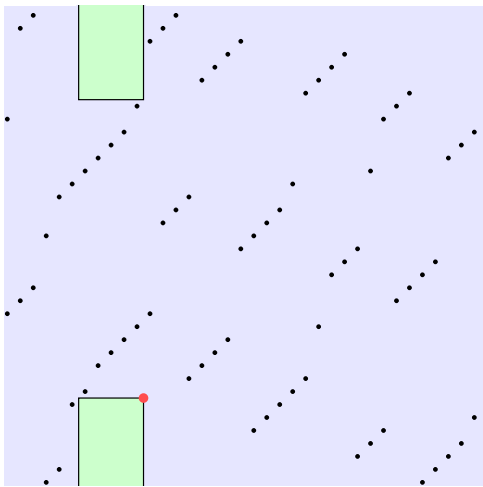

$$x_{6,29,10,8} = x_{10,8,14,12} \quad (252)$$

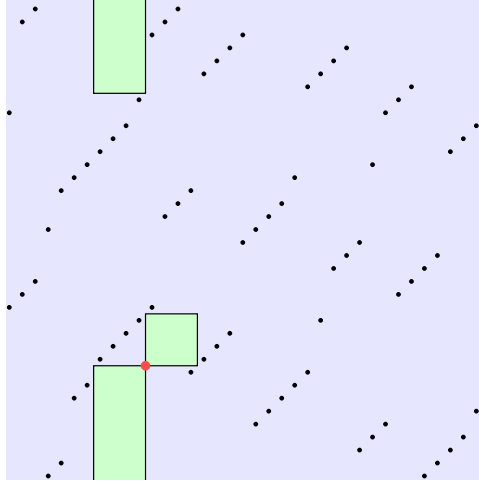

$$x_{7,29,10,9} = x_{10,9,15,12} \quad (253)$$

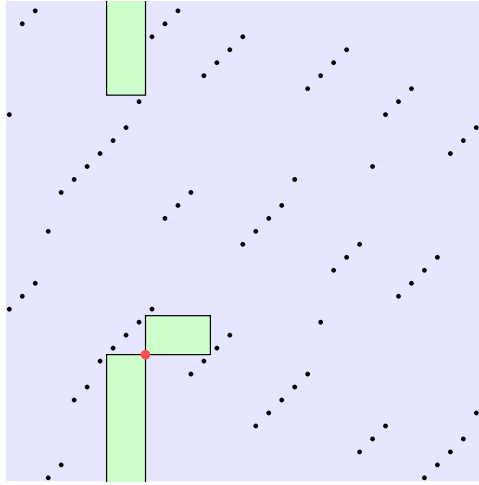

$$x_{8,29,10,10} = x_{10,10,16,12} \quad (254)$$



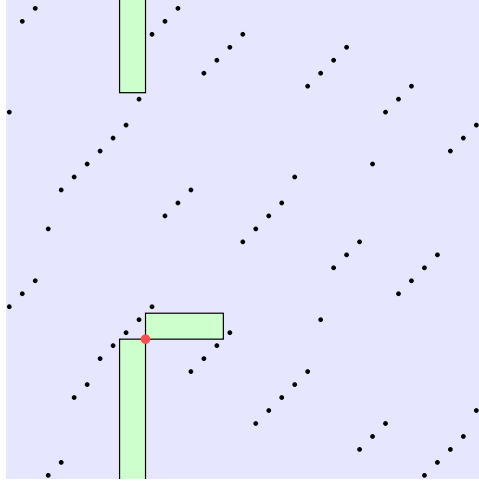

$$x_{9,29,10,11} = x_{10,11,23,12}$$

(255)

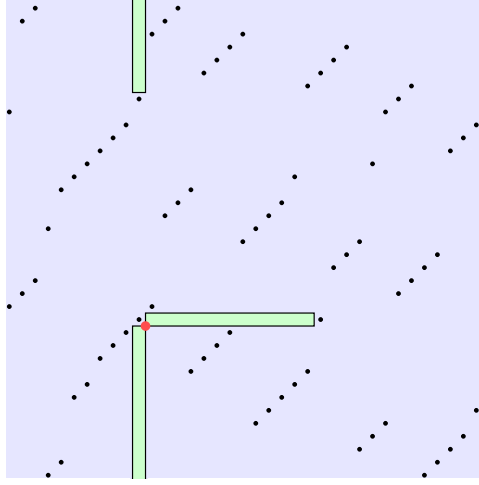

$$\begin{aligned} x_{0,12,10,13} + x_{1,12,10,14} + x_{2,12,10,18} + x_{3,12,10,21} + x_{4,12,10,22} + x_{5,12,10,23} + x_{6,12,10,24} + x_{7,12,10,25} + x_{8,12,10,26} + x_{9,12,10,28} = \\ = x_{10,8,14,12} + x_{10,9,15,12} + x_{10,10,16,12} + x_{10,11,23,12} + x_{10,34,11,12} + x_{10,35,12,12} + x_{10,36,13,12} \end{aligned} \quad (256)$$

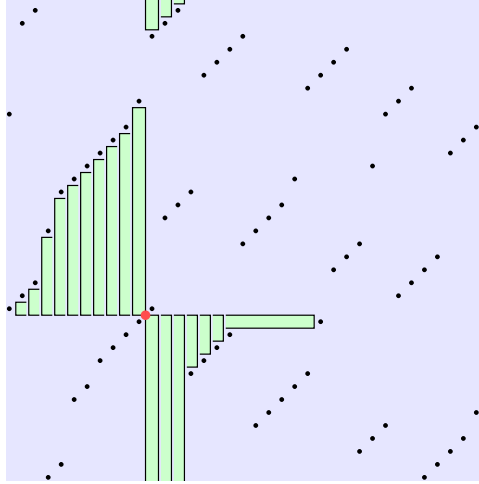

$$x_{0,12,10,13} = x_{10,13,11,33}$$

(257)

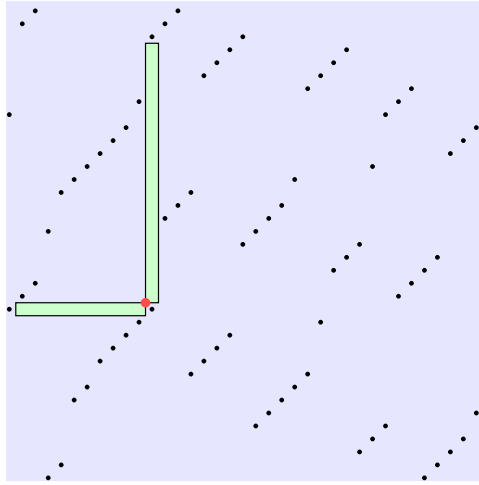

$$x_{1,12,10,14} = 0$$

(258)

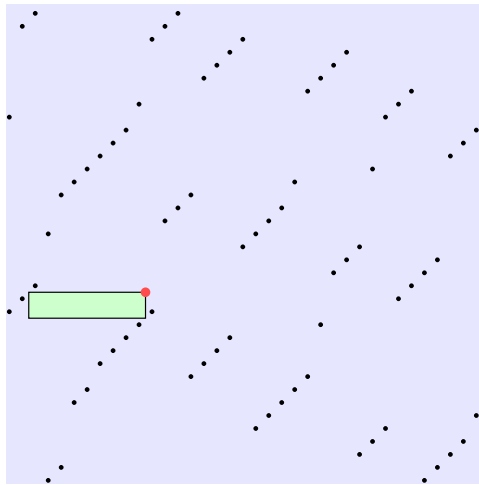

$$x_{2,12,10,18} = 0 \tag{259}$$

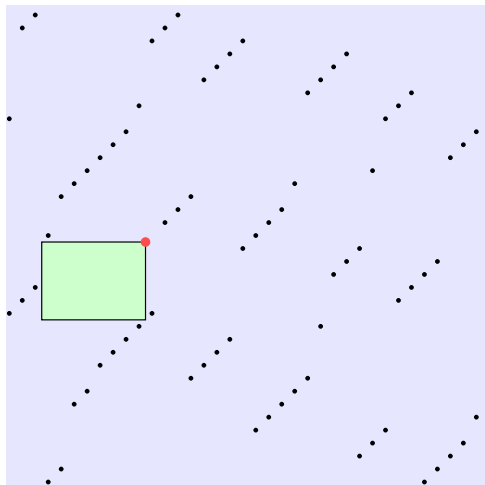

$$0 = x_{10,20,12,33} \tag{260}$$

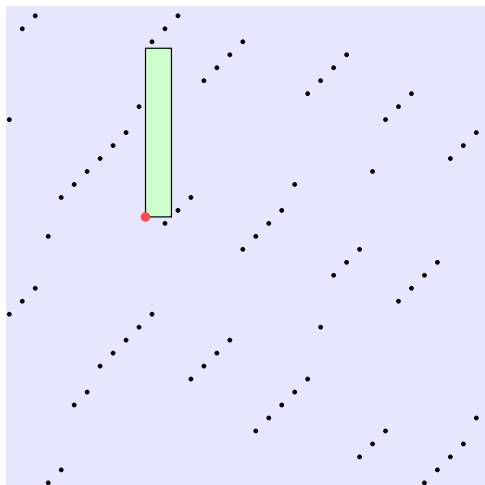

$$x_{3,12,10,21} = x_{10,21,13,33} \tag{261}$$

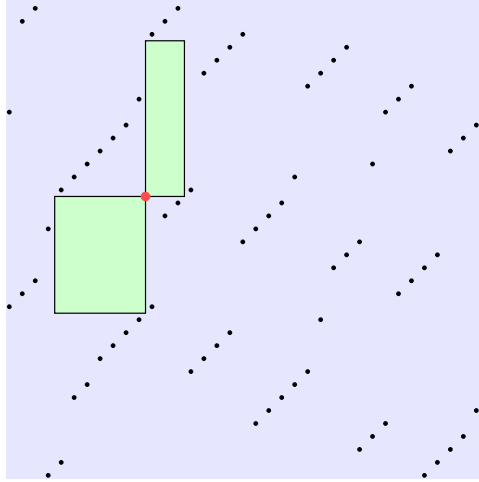

$$x_{4,12,10,22} = x_{10,22,14,33} + x_{10,22,21,30}$$

(262)

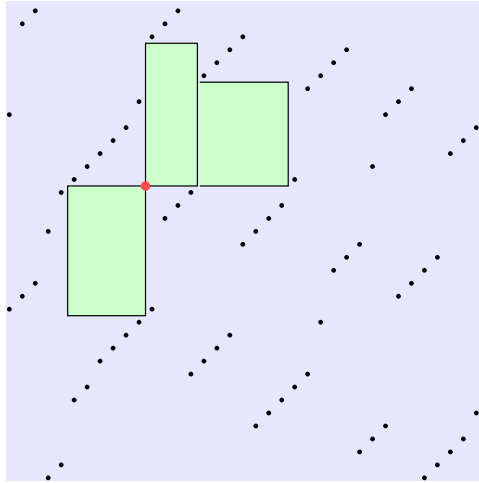

$$x_{5,12,10,23} = x_{10,23,22,30} + x_{10,23,27,29}$$

(263)

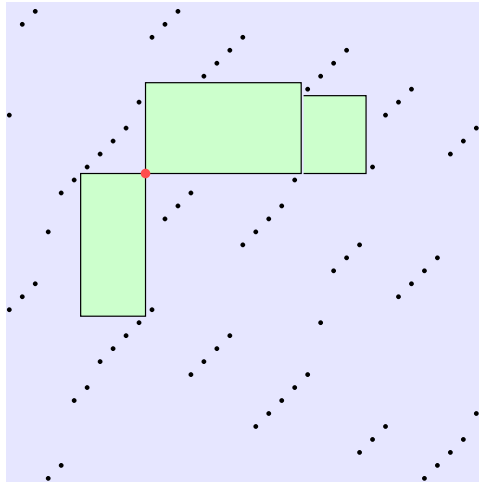

$$x_{6,12,10,24} = x_{10,24,28,29} \tag{264}$$

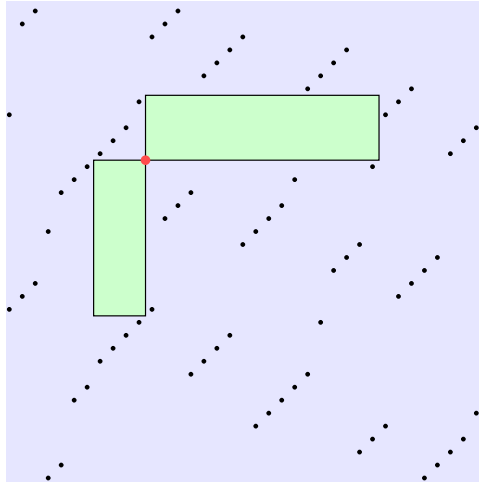

$$x_{7,12,10,25} = 0 \tag{265}$$

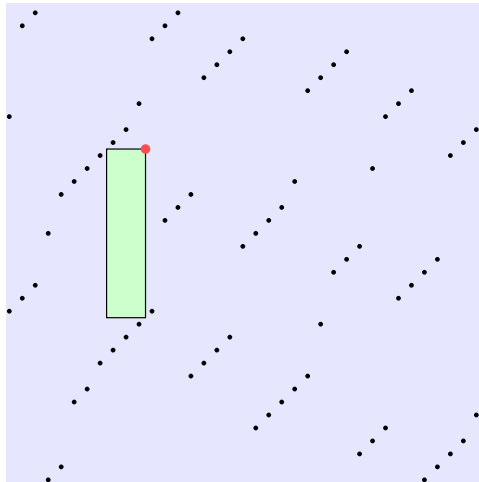

$$x_{8,12,10,26} = 0 \tag{266}$$

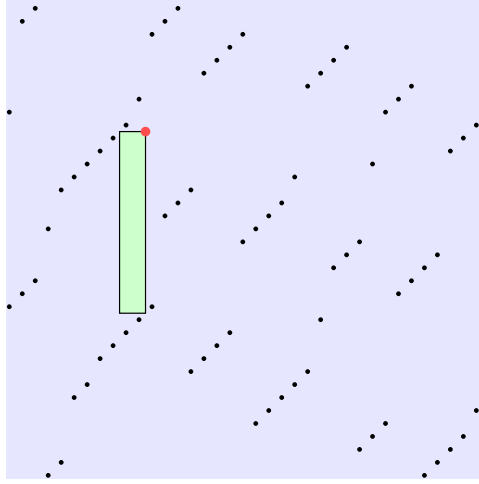

$$x_{9,12,10,28} = x_{10,28,29,29}$$

(267)

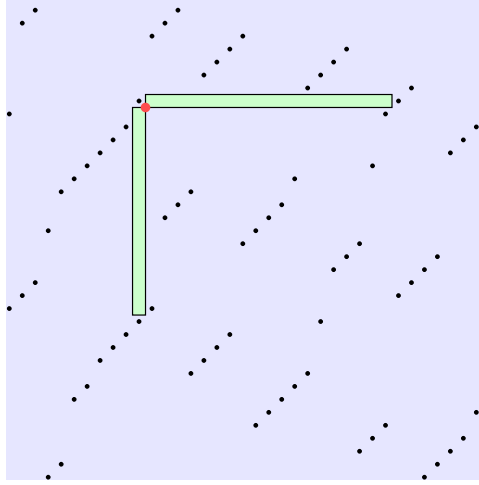

$$\begin{aligned} x_{1,29,10,35} + x_{2,29,10,36} + x_{3,29,10,0} + x_{4,29,10,5} + x_{5,29,10,6} + x_{6,29,10,8} + x_{7,29,10,9} + x_{8,29,10,10} + x_{9,29,10,11} + x_{31,29,10,34} = \\ = x_{10,23,27,29} + x_{10,24,28,29} + x_{10,28,29,29} \end{aligned} \quad (268)$$

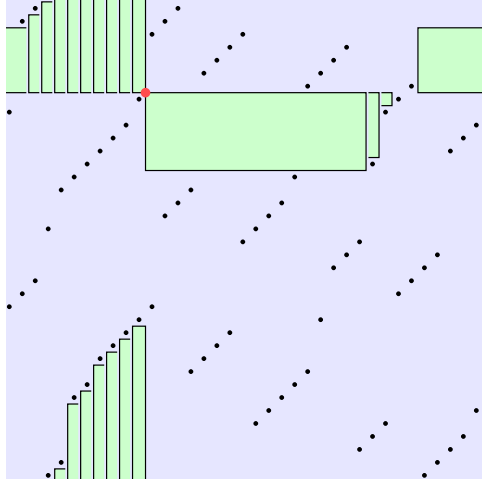

$$x_{26,30,10,34} = x_{10,22,21,30} + x_{10,23,22,30}$$

(269)

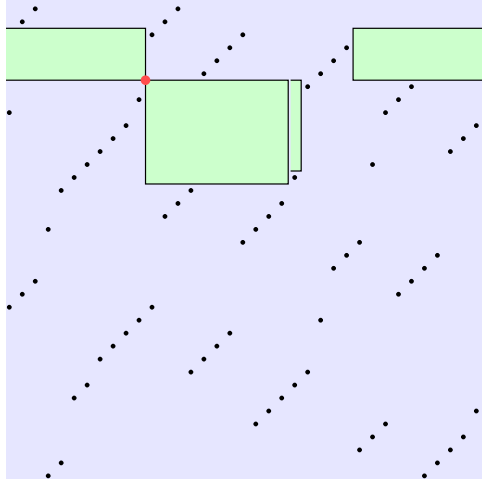

$$x_{18,33,10,34} = x_{10,13,11,33} + x_{10,20,12,33} + x_{10,21,13,33} + x_{10,22,14,33}$$

(270)

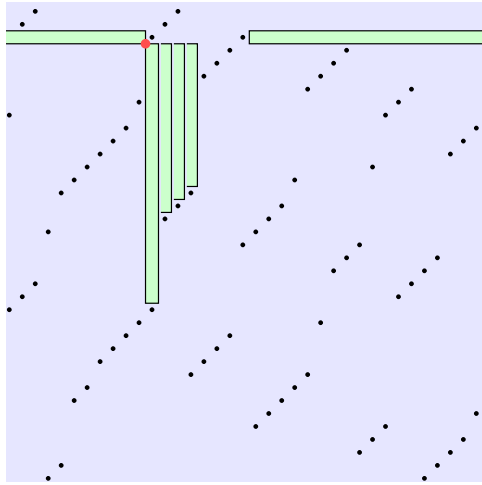

$$x_{18,33,10,34} + x_{26,30,10,34} + x_{31,29,10,34} = x_{10,34,11,12} \quad (271)$$

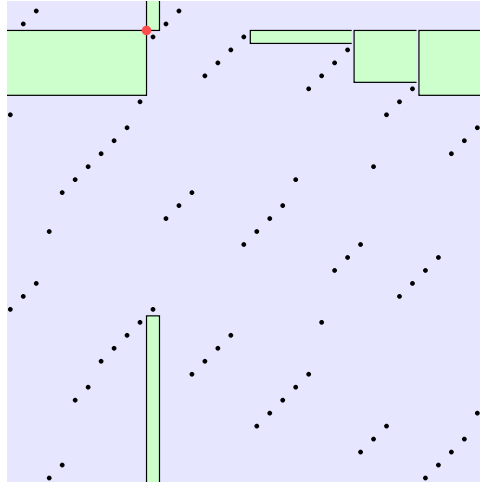

$$x_{1,29,10,35} = x_{10,35,12,12} \quad (272)$$

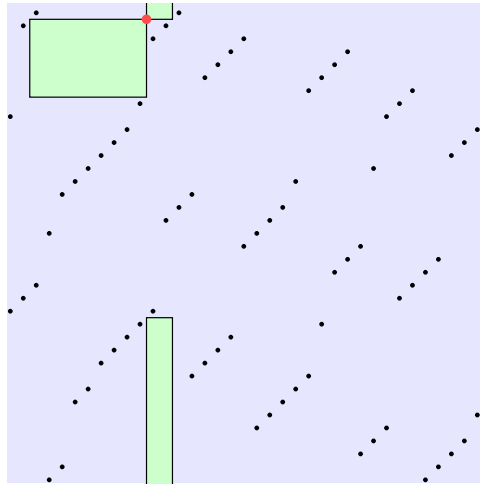

$$x_{2,29,10,36} = x_{10,36,13,12} \quad (273)$$



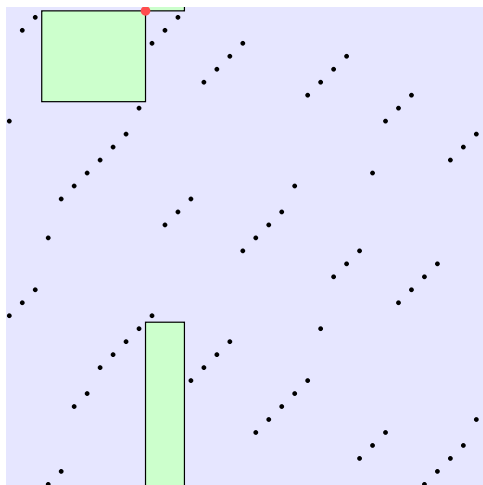

$$x_{3,34,11,0} = 0$$

(274)

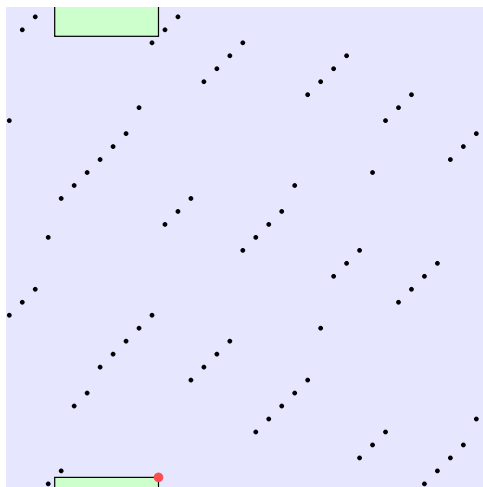

$$x_{4,34,11,5} = 0$$

(275)

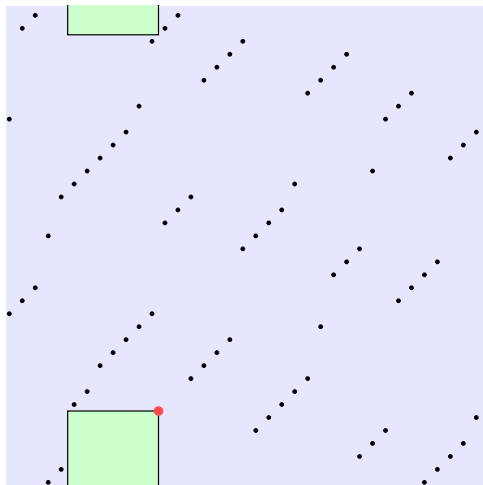

$$x_{5,34,11,6} = 0 \tag{276}$$

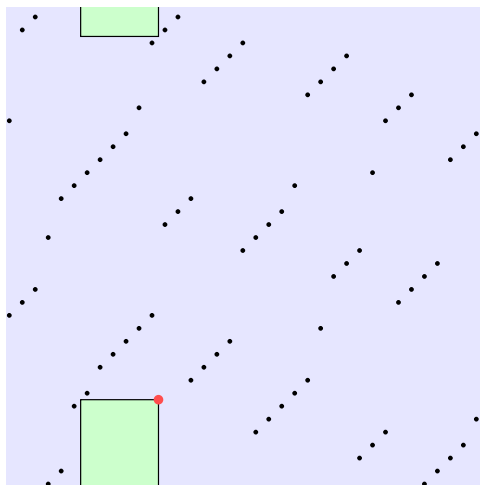

$$x_{6,34,11,8} = x_{11,8,14,19} \tag{277}$$

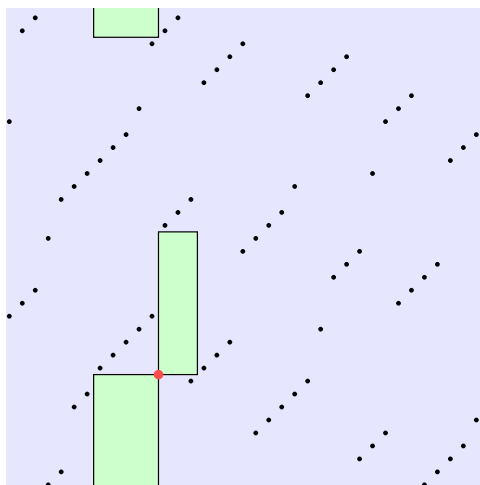

$$x_{7,34,11,9} = x_{11,9,15,19} \tag{278}$$

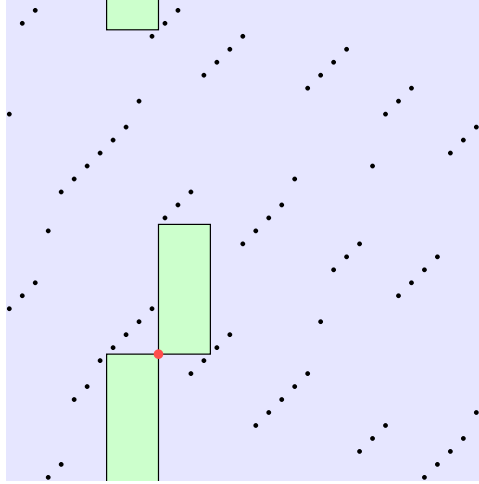

$$x_{8,34,11,10} = x_{11,10,16,19}$$

(279)

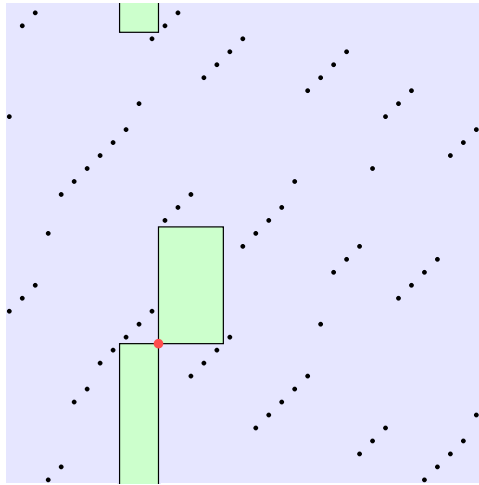

$$x_{9,34,11,11} = x_{11,11,17,19} + x_{11,11,23,17}$$

(280)

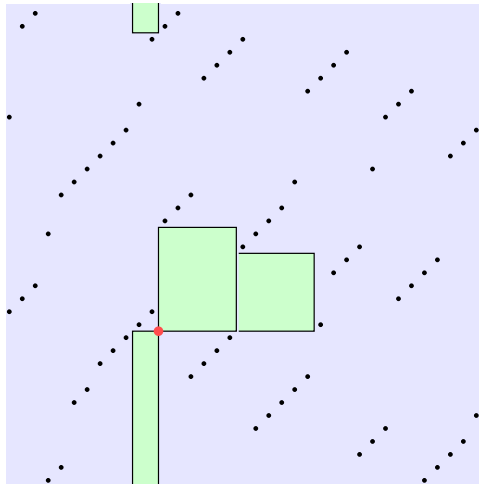

$$x_{10,34,11,12} = x_{11,12,24,17} + x_{11,12,29,15} + x_{11,12,36,13} \quad (281)$$

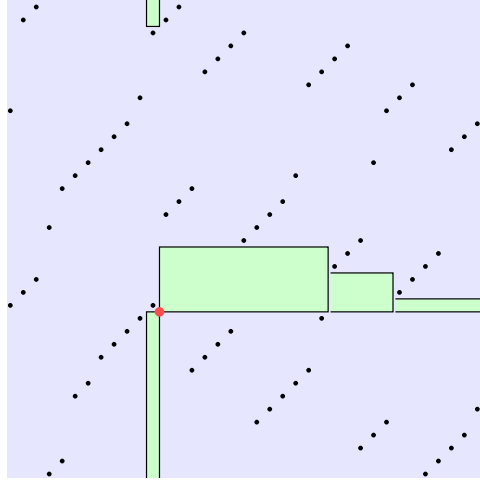

$$x_{3,13,11,21} + x_{4,13,11,22} + x_{5,13,11,23} + x_{6,13,11,24} + x_{7,13,11,25} + x_{8,13,11,26} + x_{9,13,11,28} + x_{10,13,11,33} = x_{11,12,36,13} \quad (282)$$

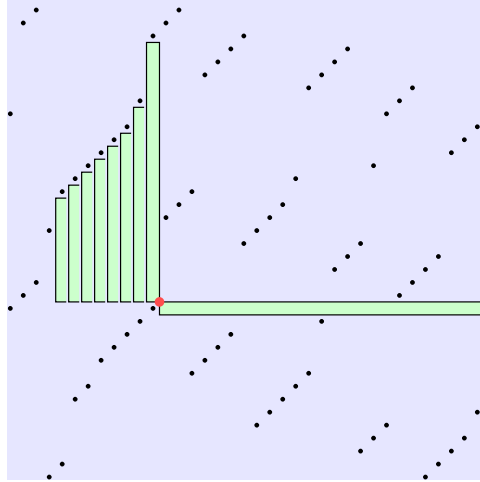

$$0 = x_{11,12,29,15} \quad (283)$$

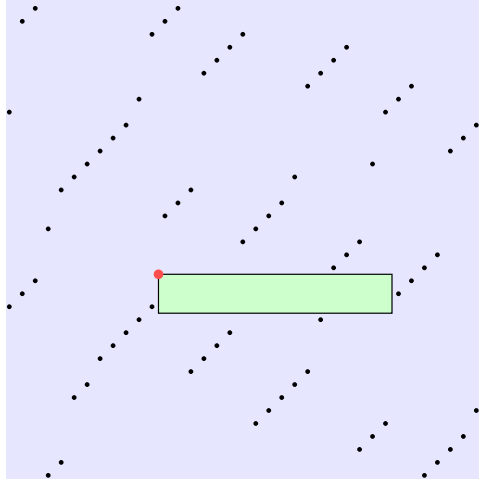

$$0 = x_{11,11,23,17} + x_{11,12,24,17} \quad (284)$$

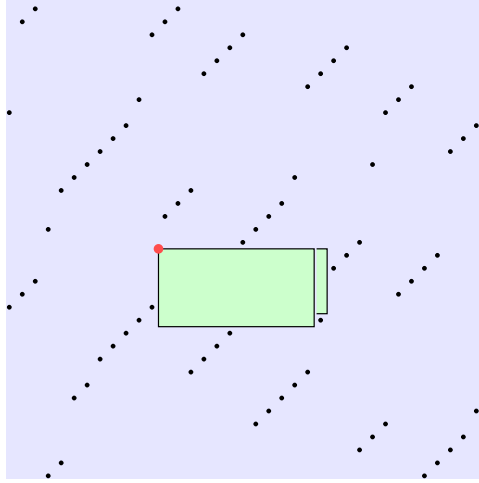

$$x_{20,19,11,20} + x_{21,19,11,21} = x_{11,8,14,19} + x_{11,9,15,19} + x_{11,10,16,19} + x_{11,11,17,19} + x_{11,35,12,19} + x_{11,36,13,19} \quad (285)$$

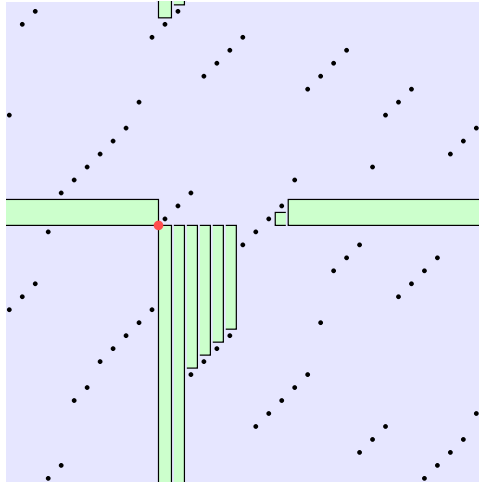

$$x_{20,19,11,20} = x_{11,20,12,34}$$

(286)

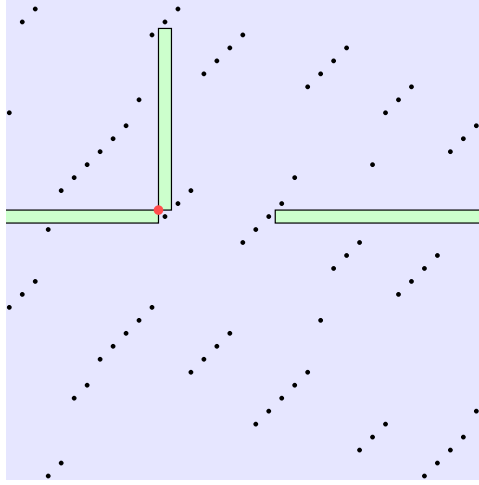

$$x_{3,13,11,21} + x_{21,19,11,21} = x_{11,21,13,34}$$

(287)

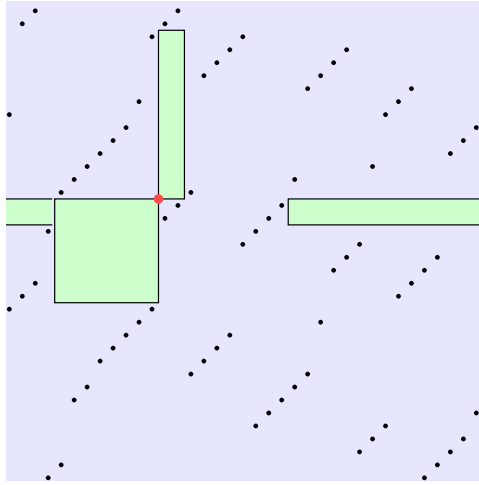

$$x_{4,13,11,22} = x_{11,22,14,34}$$

(288)

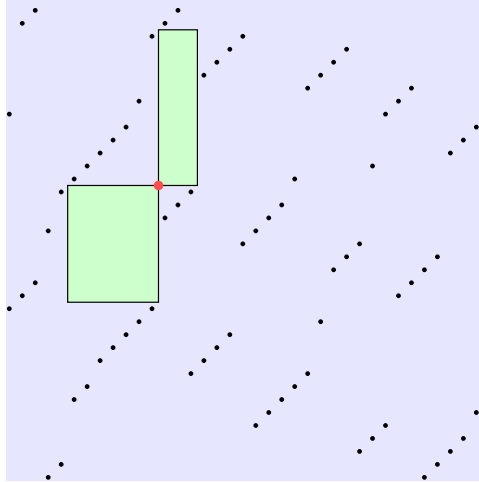

$$x_{5,13,11,23} = 0$$

(289)

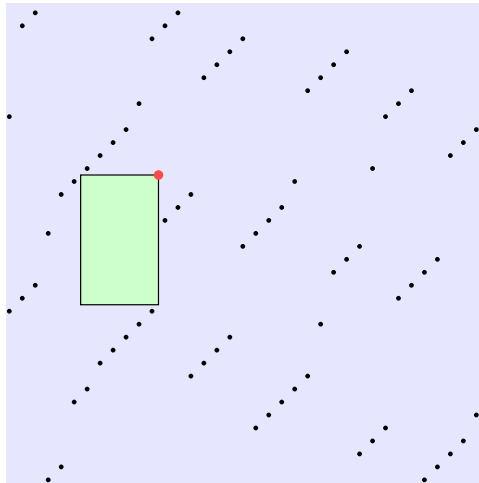

$$x_{6,13,11,24} = 0$$

(290)

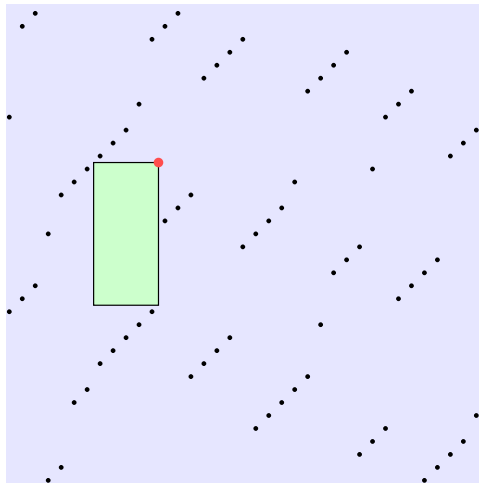

$$x_{7,13,11,25} = 0 \tag{291}$$

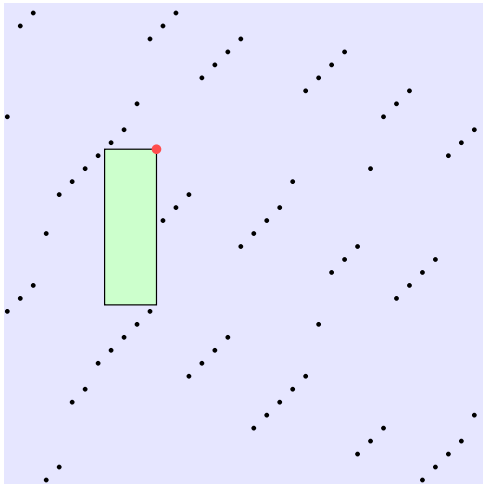

$$x_{8,13,11,26} = 0 \tag{292}$$

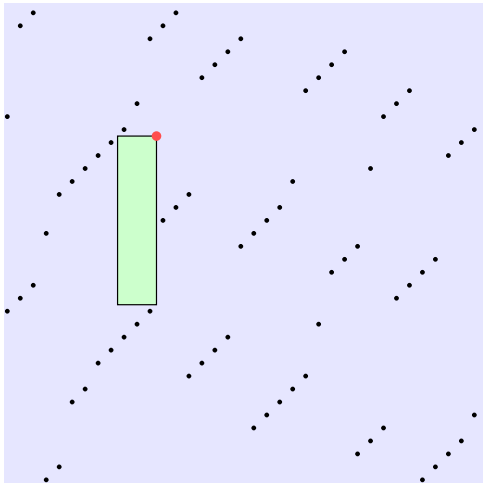

$$x_{9,13,11,28} = 0 \tag{293}$$



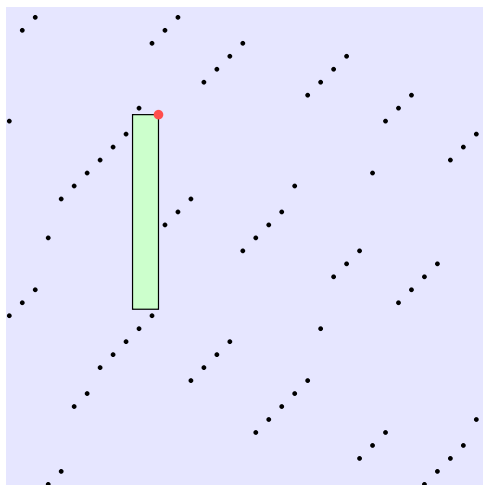

$$0 = x_{11,31,15,34}$$

(294)

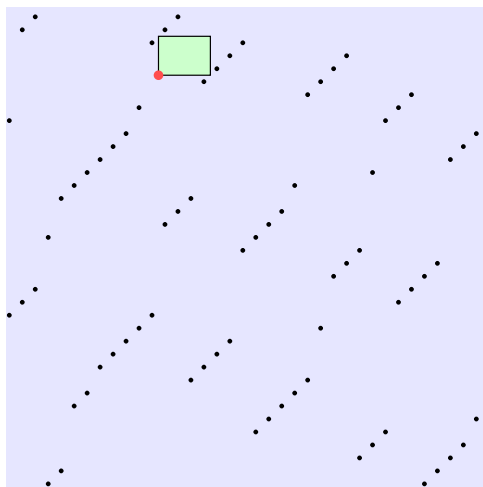

$$0 = x_{11,32,16,34}$$

(295)

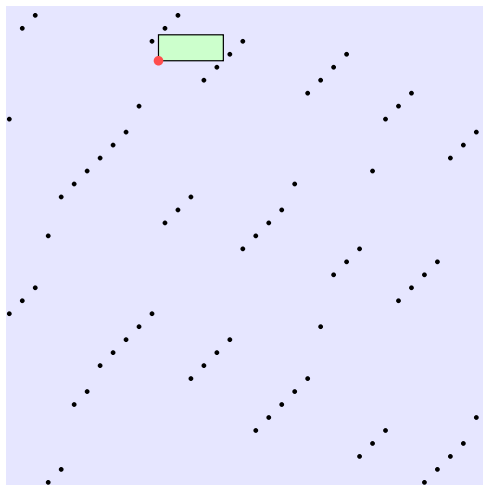

$$x_{10,13,11,33} = x_{11,33,17,34}$$

(296)

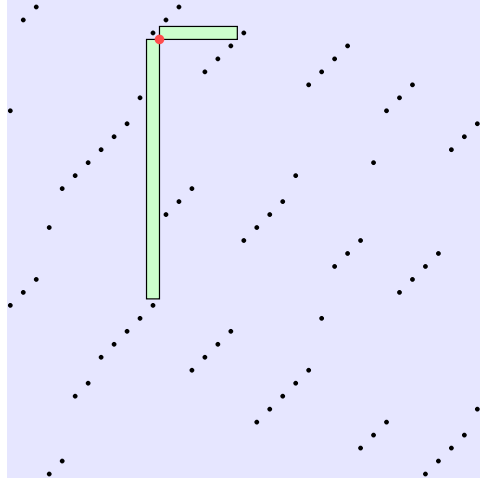

$$\begin{aligned} & x_{1,34,11,35} + x_{2,34,11,36} + x_{3,34,11,0} + x_{4,34,11,5} + x_{5,34,11,6} + x_{6,34,11,8} + x_{7,34,11,9} + x_{8,34,11,10} + x_{9,34,11,11} + x_{10,34,11,12} = \\ & = x_{11,20,12,34} + x_{11,21,13,34} + x_{11,22,14,34} + x_{11,31,15,34} + x_{11,32,16,34} + x_{11,33,17,34} \end{aligned} \quad (297)$$

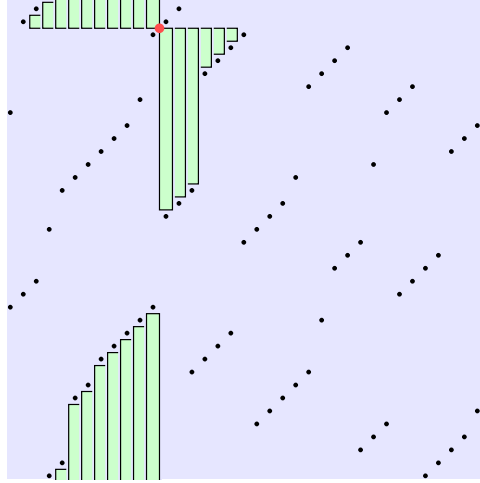

$$x_{1,34,11,35} = x_{11,35,12,19}$$

(298)

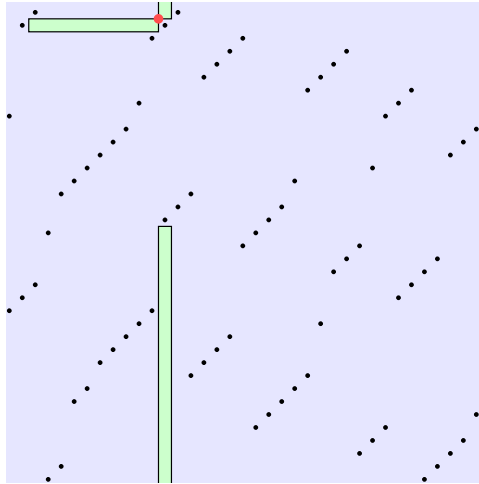

$$x_{2,34,11,36} = x_{11,36,13,19}$$

(299)

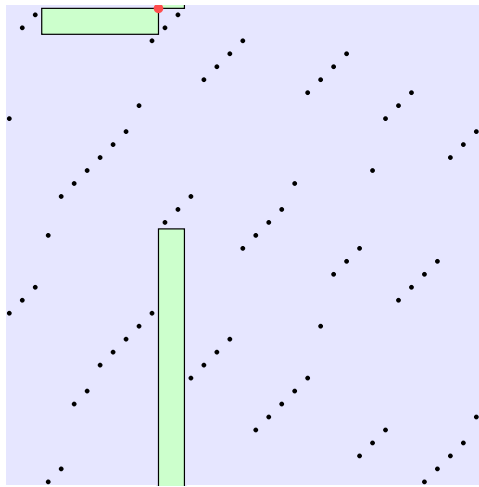

$$x_{3,35,12,0} = 0$$

(300)

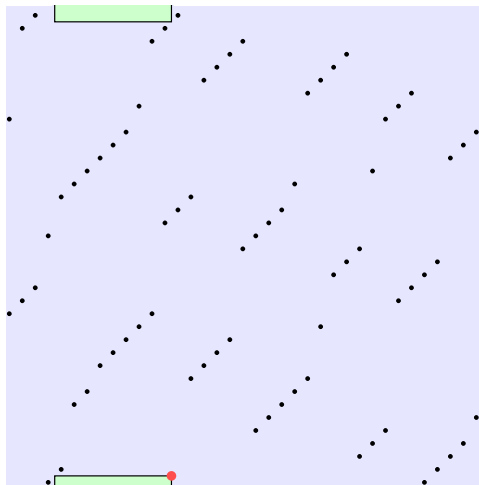

$$x_{4,35,12,5} = 0$$

(301)

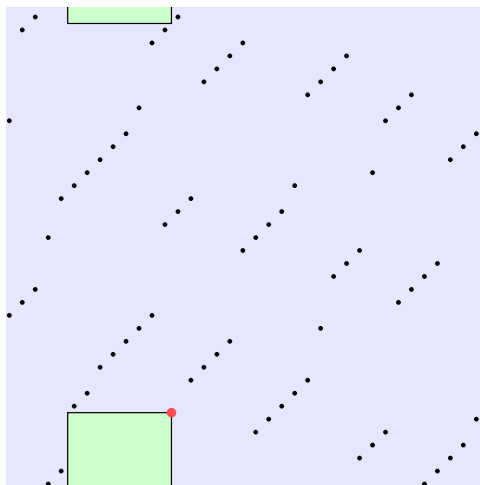

$$x_{5,35,12,6} = 0$$

(302)

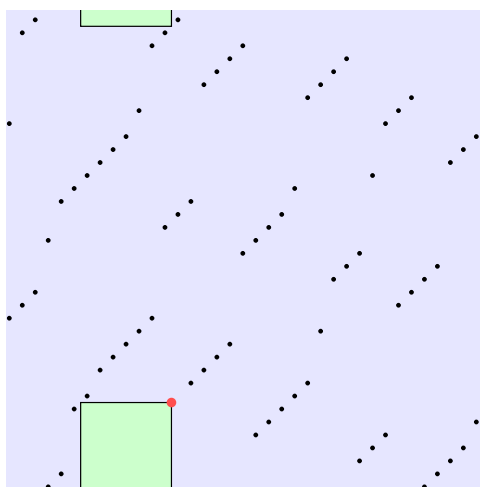

$$x_{6,35,12,8} = x_{12,8,14,20}$$

(303)

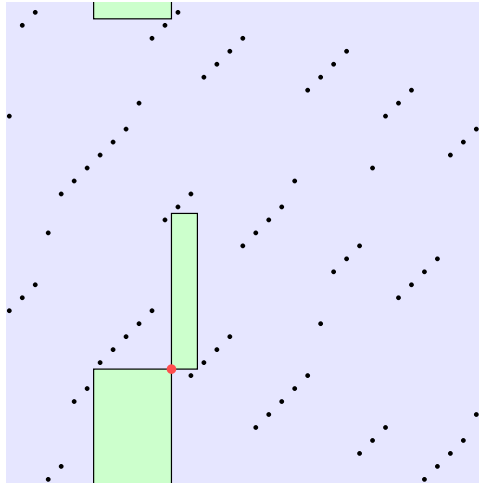

$$x_{7,35,12,9} = x_{12,9,15,20}$$

(304)

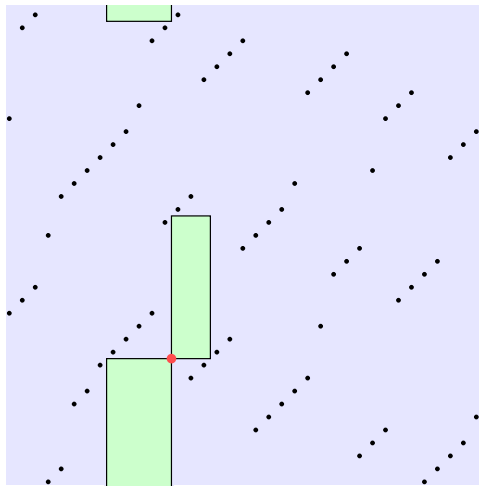

$$x_{8,35,12,10} = x_{12,10,16,20}$$

(305)

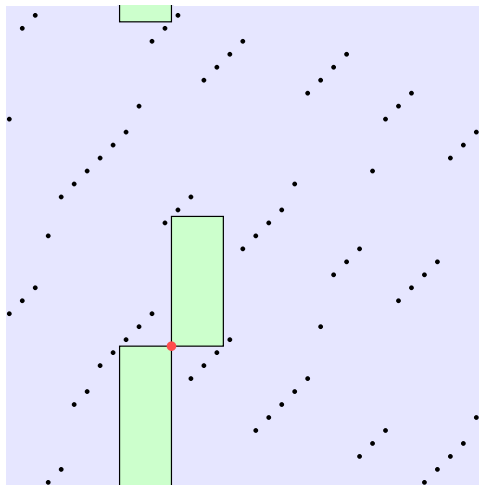

$$x_{9,35,12,11} = x_{12,11,17,20} \tag{306}$$

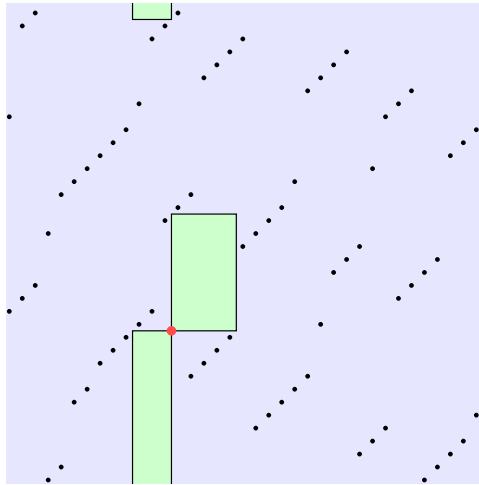

$$x_{10,35,12,12} = 0 \tag{307}$$

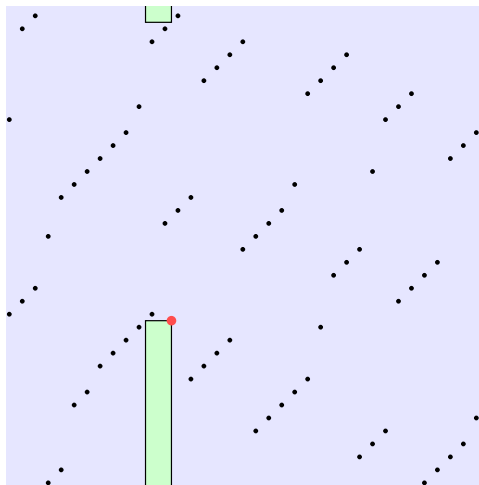

$$0 = x_{12,18,18,20} \tag{308}$$

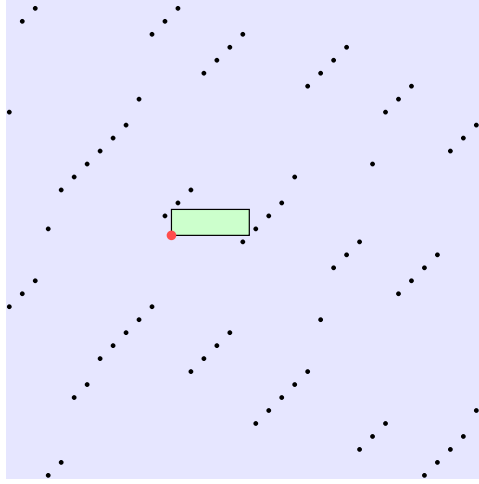

$$x_{11,35,12,19} = x_{12,19,19,20}$$

(309)

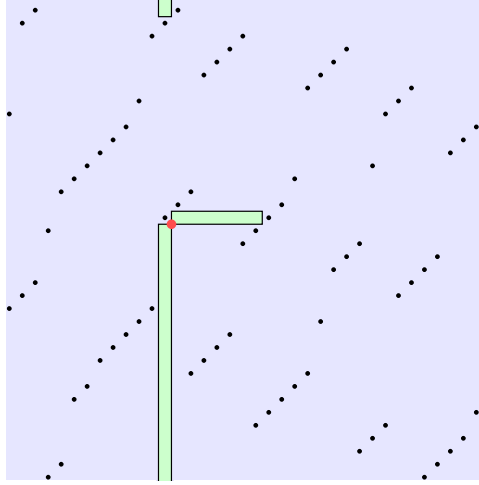

$$\begin{aligned} & x_{4,20,12,22} + x_{5,20,12,23} + x_{6,20,12,24} + x_{7,20,12,25} + x_{8,20,12,26} + x_{9,20,12,28} + x_{10,20,12,33} + x_{11,20,12,34} + x_{21,20,12,21} = \\ & = x_{12,8,14,20} + x_{12,9,15,20} + x_{12,10,16,20} + x_{12,11,17,20} + x_{12,18,18,20} + x_{12,19,19,20} + x_{12,36,13,20} \end{aligned} \quad (310)$$

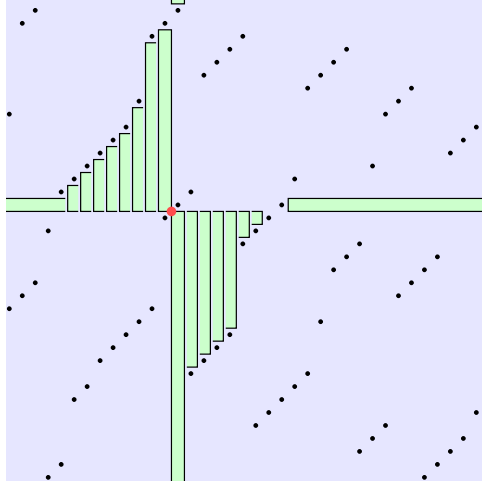

$$x_{21,20,12,21} = x_{12,21,13,35}$$

(311)

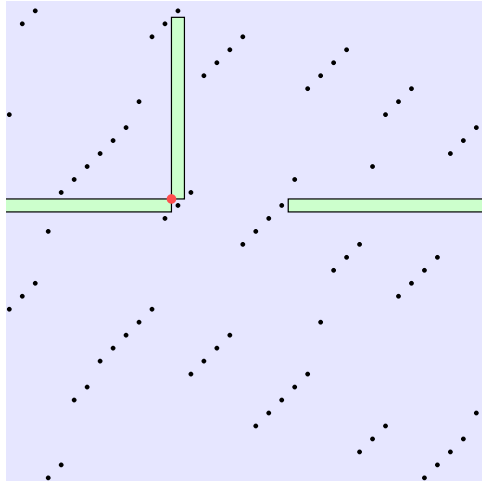

$$x_{4,20,12,22} = x_{12,22,14,35}$$

(312)

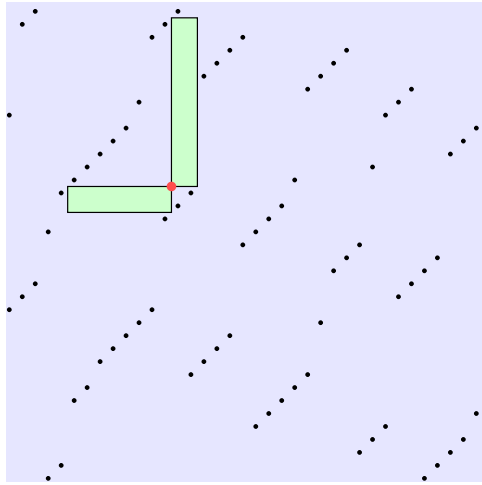



$$x_{5,20,12,23} = 0 \tag{313}$$

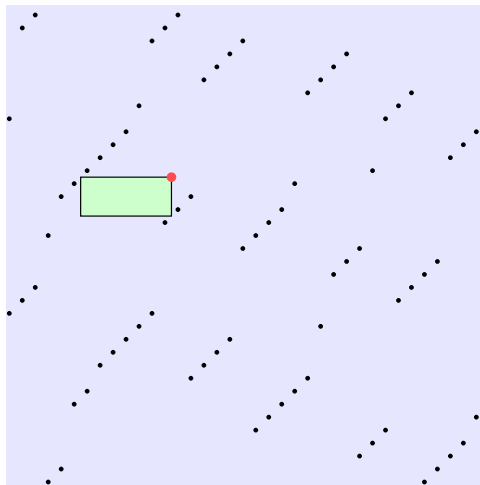

$$x_{6,20,12,24} = 0 \tag{314}$$

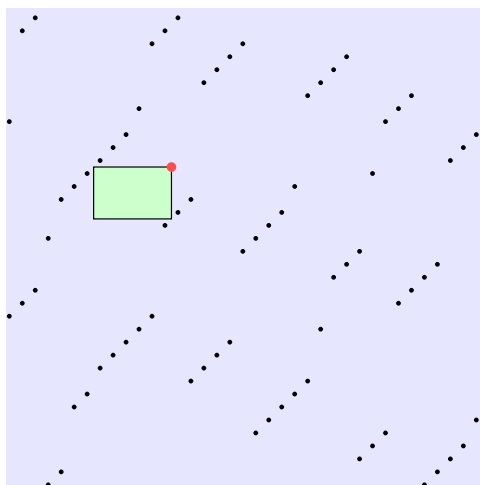

$$x_{7,20,12,25} = 0 \tag{315}$$

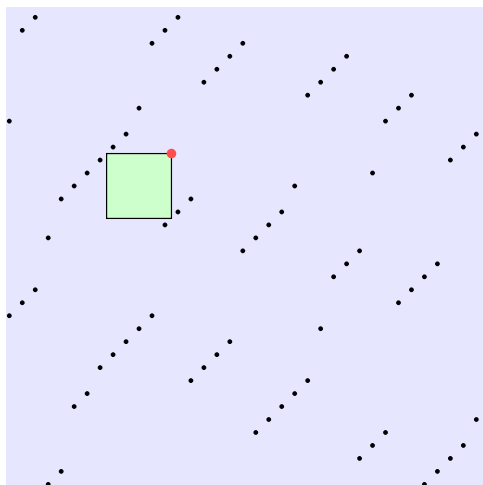

$$x_{8,20,12,26} = 0$$

(316)

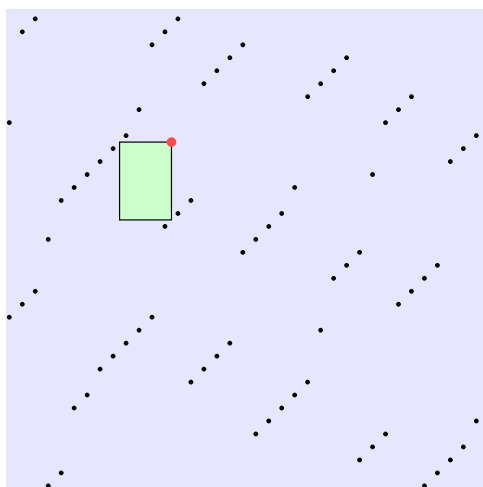

$$x_{9,20,12,28} = 0$$

(317)

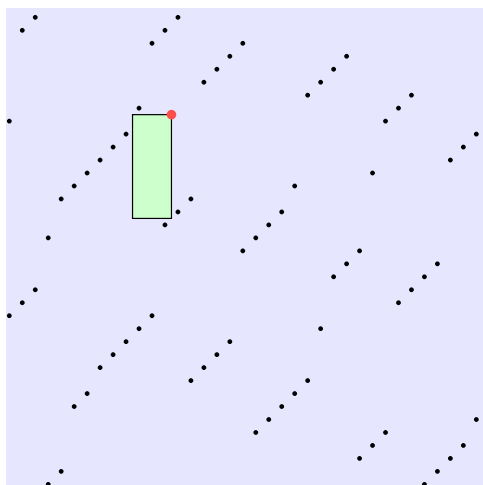

$$0 = x_{12,31,15,35} \tag{318}$$

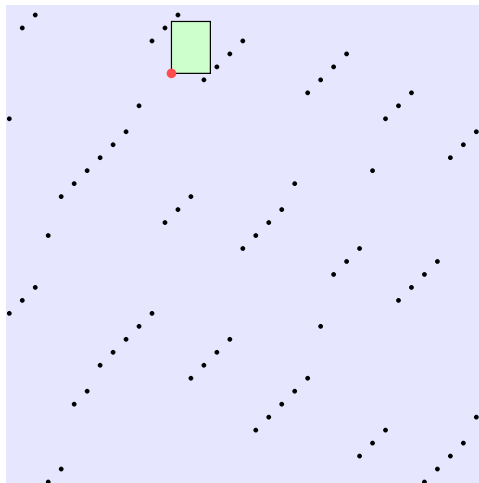

$$0 = x_{12,32,16,35} \tag{319}$$

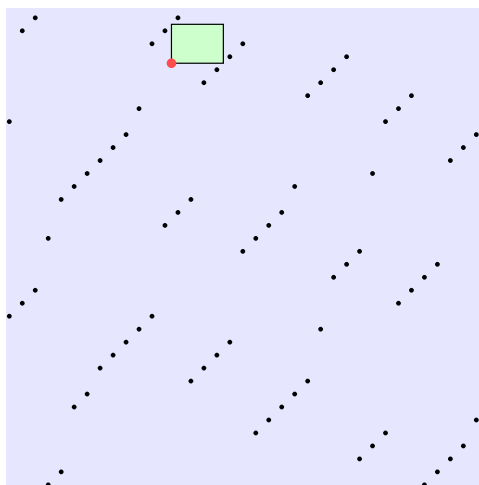

$$x_{10,20,12,33} = x_{12,33,17,35} \tag{320}$$

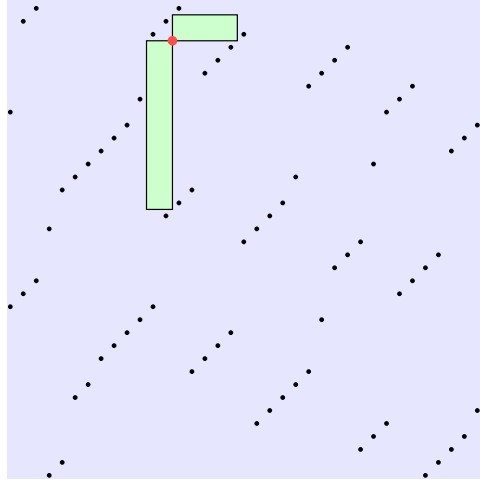

$$x_{11,20,12,34} = x_{12,34,0,35}$$

(321)

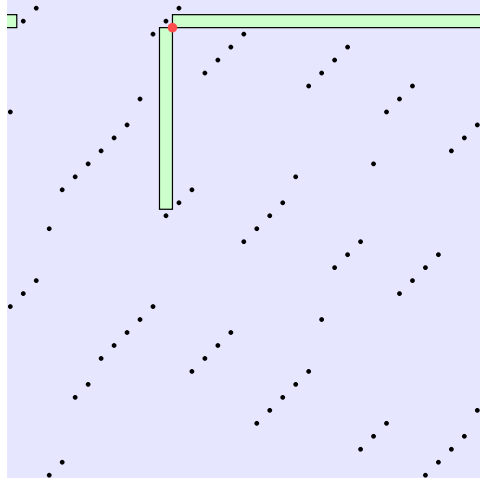

$$\begin{aligned} & x_{2,35,12,36} + x_{3,35,12,0} + x_{4,35,12,5} + x_{5,35,12,6} + x_{6,35,12,8} + x_{7,35,12,9} + x_{8,35,12,10} + x_{9,35,12,11} + x_{10,35,12,12} + x_{11,35,12,19} = \\ & = x_{12,21,13,35} + x_{12,22,14,35} + x_{12,31,15,35} + x_{12,32,16,35} + x_{12,33,17,35} + x_{12,34,0,35} \end{aligned} \quad (322)$$

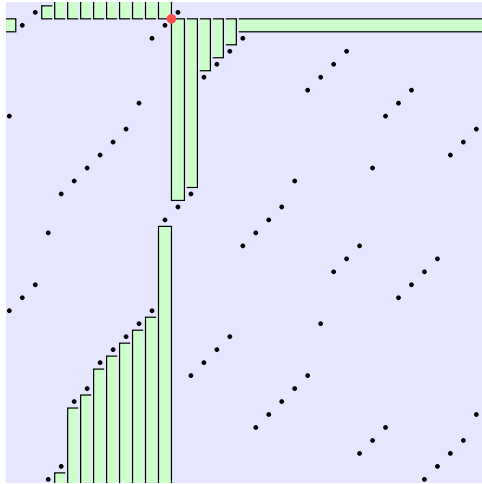

$$x_{2,35,12,36} = x_{12,36,13,20}$$

(323)

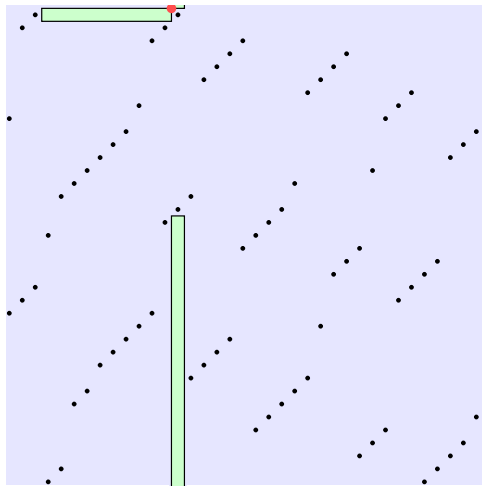

$$0 = x_{13,34,31,1}$$

(324)

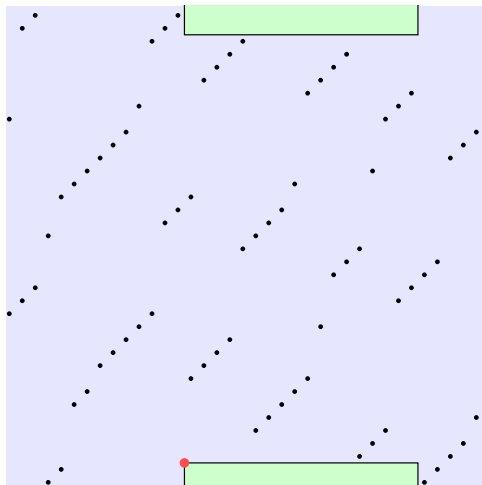

$$0 = x_{13,34,26,3}$$

(325)

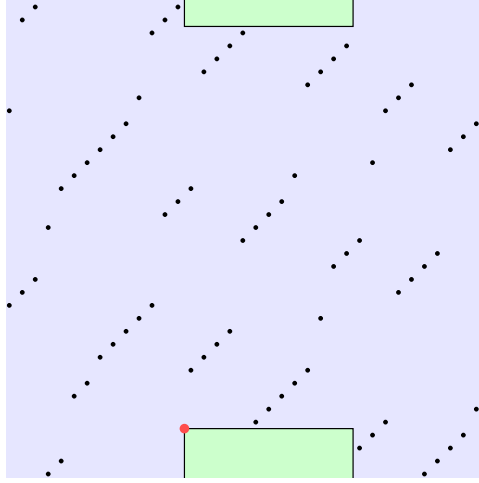

$$x_{23,7,13,8} = x_{13,22,14,7} + x_{13,31,15,7} + x_{13,32,16,7} + x_{13,33,17,7} + x_{13,34,18,7}$$

(326)

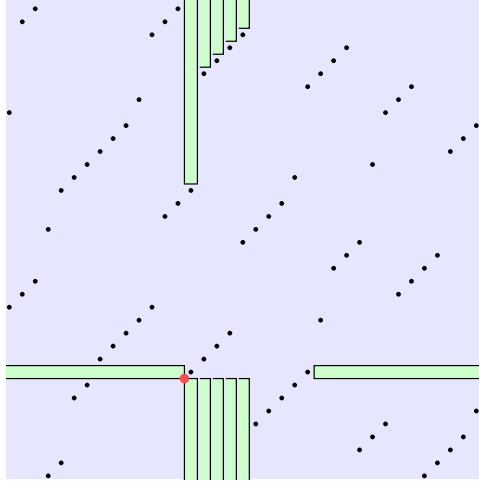

$$x_{6,36,13,8} + x_{23,7,13,8} = x_{13,8,14,21}$$

(327)

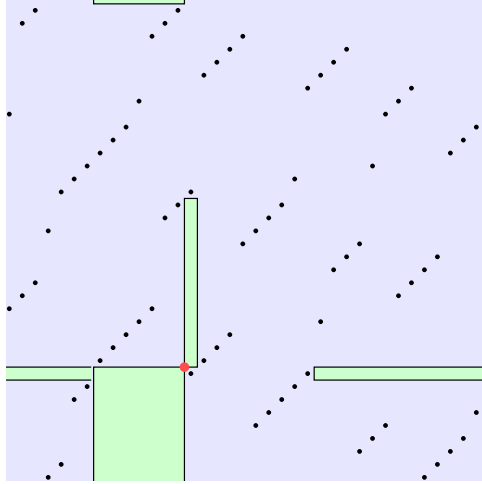

$$x_{7,36,13,9} = x_{13,9,15,21}$$

(328)

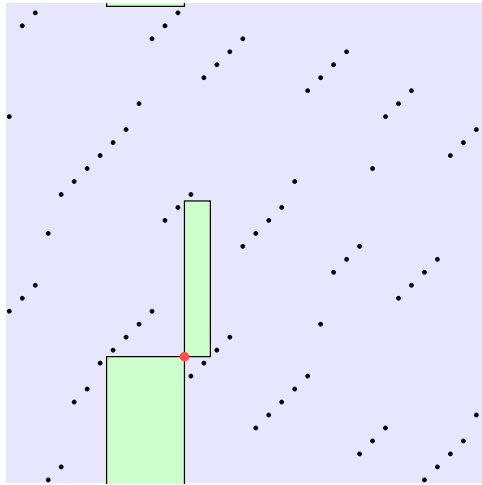

$$x_{8,36,13,10} = x_{13,10,16,21}$$

(329)

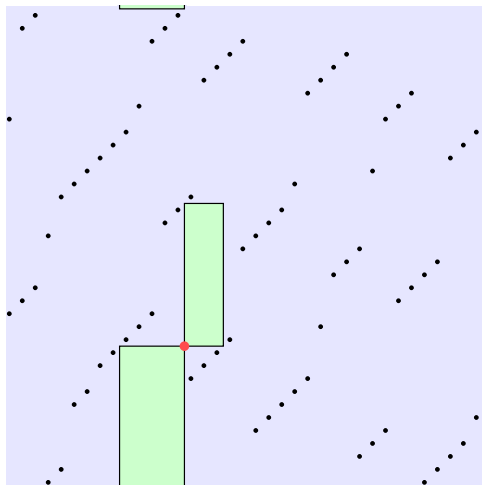

$$x_{9,36,13,11} = x_{13,11,17,21} \tag{330}$$

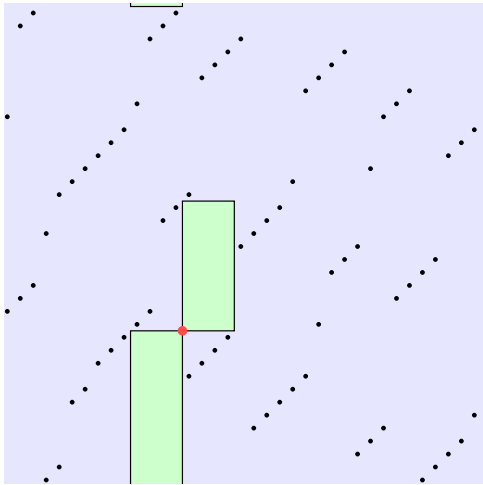

$$x_{10,36,13,12} = 0 \tag{331}$$

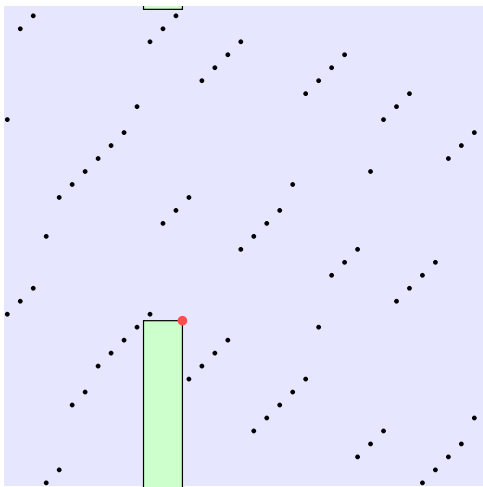

$$0 = x_{13,18,18,21} \tag{332}$$



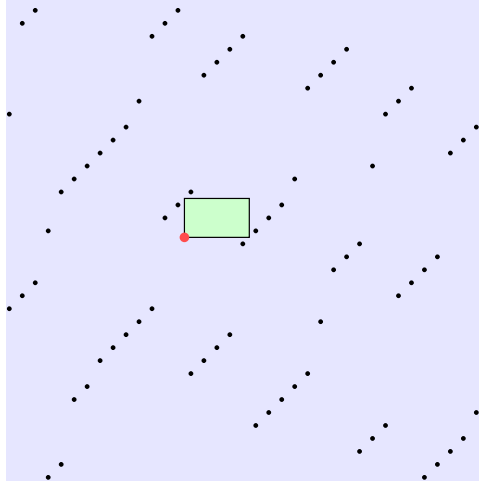

$$x_{11,36,13,19} = x_{13,19,19,21}$$

(333)

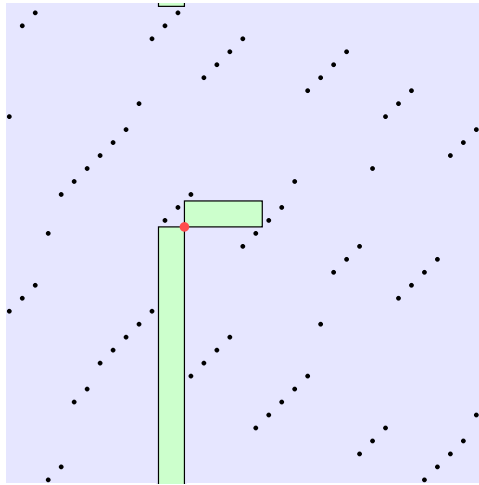

$$x_{12,36,13,20} = x_{13,20,20,21}$$

(334)

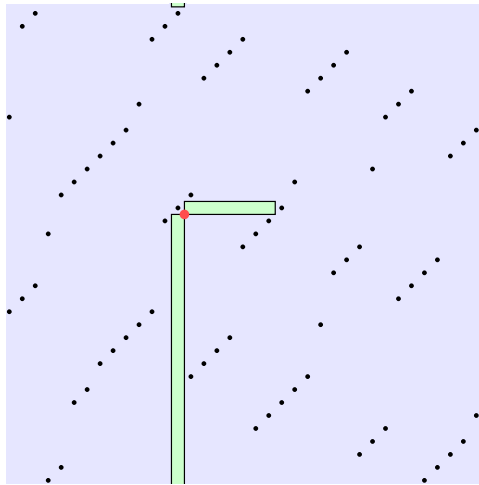

$$\begin{aligned}
& x_{4,21,13,22} + x_{5,21,13,23} + x_{6,21,13,24} + x_{7,21,13,25} + x_{8,21,13,26} + x_{9,21,13,28} + x_{10,21,13,33} + x_{11,21,13,34} + x_{12,21,13,35} = \\
& = x_{13,8,14,21} + x_{13,9,15,21} + x_{13,10,16,21} + x_{13,11,17,21} + x_{13,18,18,21} + x_{13,19,19,21} + x_{13,20,20,21}
\end{aligned} \tag{335}$$

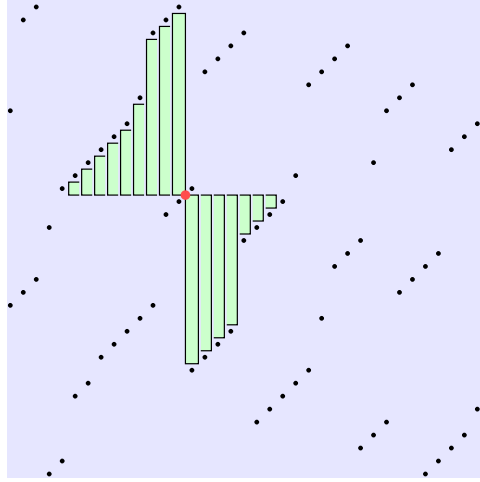

$$x_{4,21,13,22} = x_{13,22,14,7} \tag{336}$$

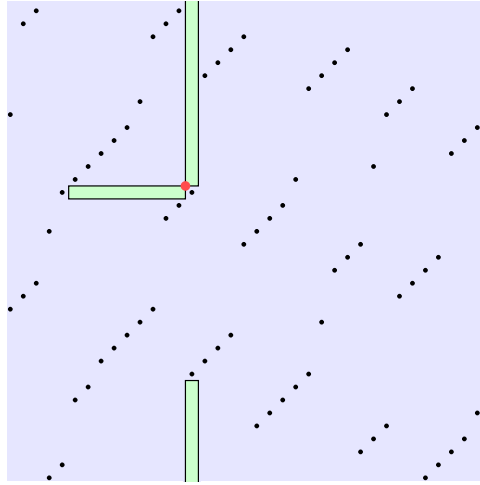

$$x_{5,21,13,23} = 0 \tag{337}$$

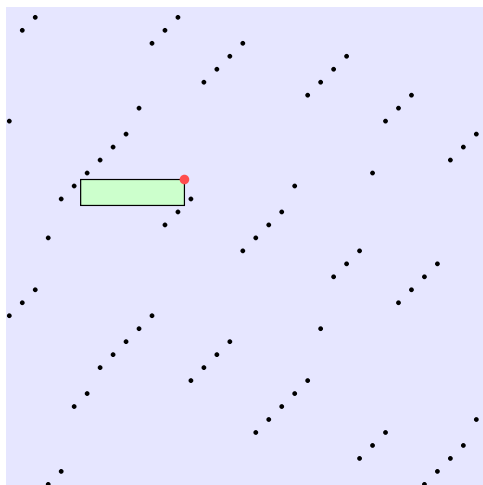

$$x_{6,21,13,24} = 0$$

(338)

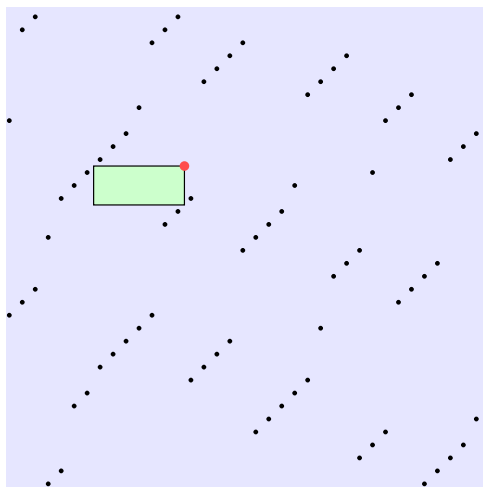

$$x_{7,21,13,25} = 0$$

(339)

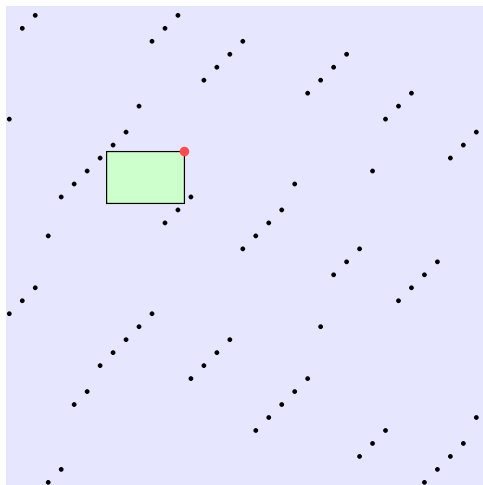

$$x_{8,21,13,26} = 0 \tag{340}$$

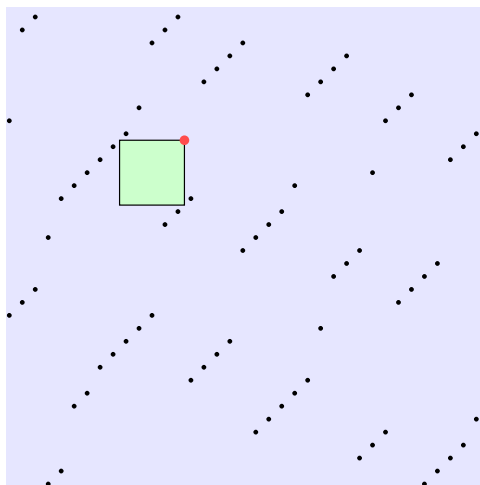

$$x_{9,21,13,28} = 0 \tag{341}$$

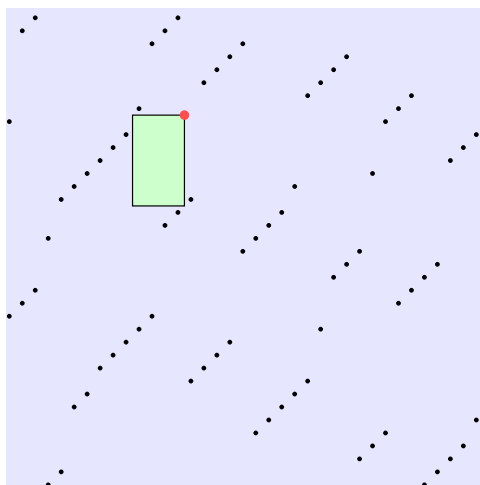

$$0 = x_{13,31,15,7} \tag{342}$$

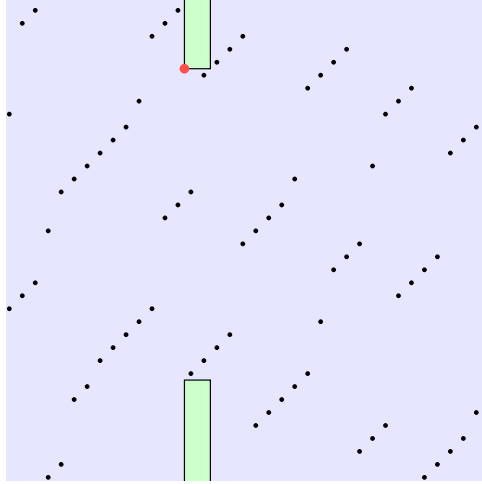

$$0 = x_{13,32,16,7}$$

(343)

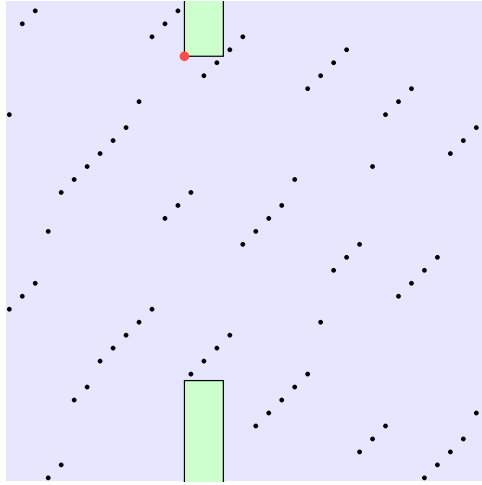

$$x_{10,21,13,33} = x_{13,33,17,7}$$

(344)

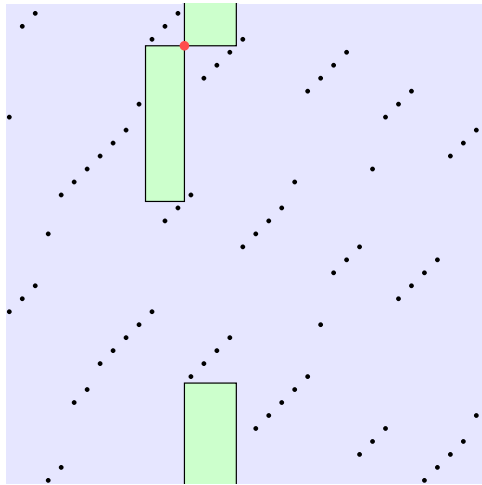

$$x_{11,21,13,34} = x_{13,34,0,36} + x_{13,34,18,7} + x_{13,34,26,3} + x_{13,34,31,1} \quad (345)$$

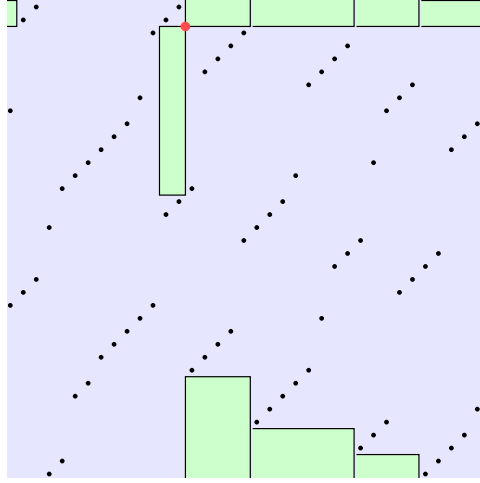

$$x_{12,21,13,35} = x_{13,35,1,36} \quad (346)$$

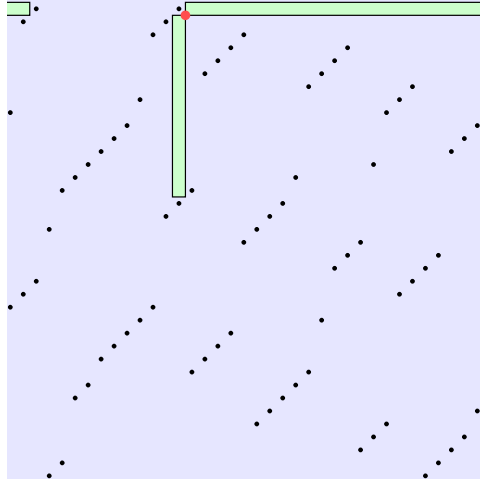

$$x_{6,36,13,8} + x_{7,36,13,9} + x_{8,36,13,10} + x_{9,36,13,11} + x_{10,36,13,12} + x_{11,36,13,19} + x_{12,36,13,20} = x_{13,34,0,36} + x_{13,35,1,36} \quad (347)$$

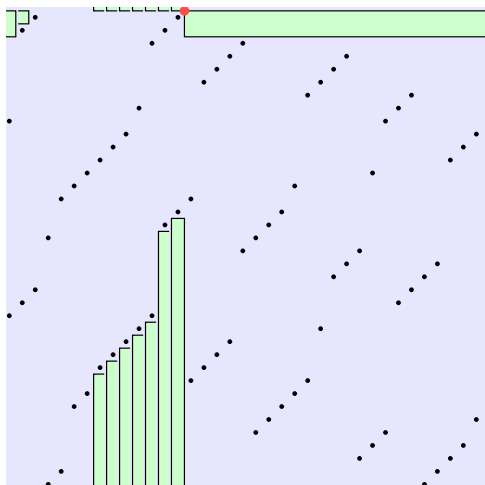

$$0 = x_{14,4,19,8}$$

(348)

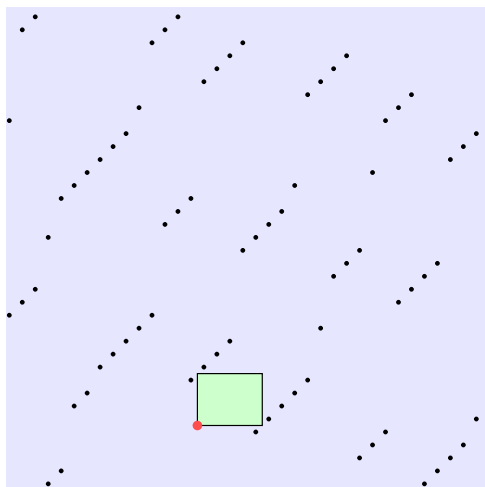

$$0 = x_{14,5,20,8}$$

(349)

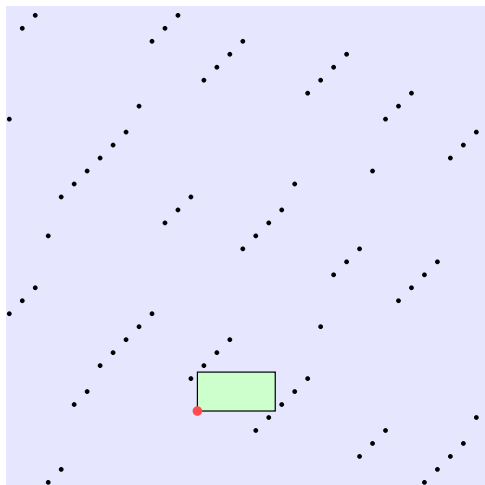

$$0 = x_{14,6,21,8}$$

(350)

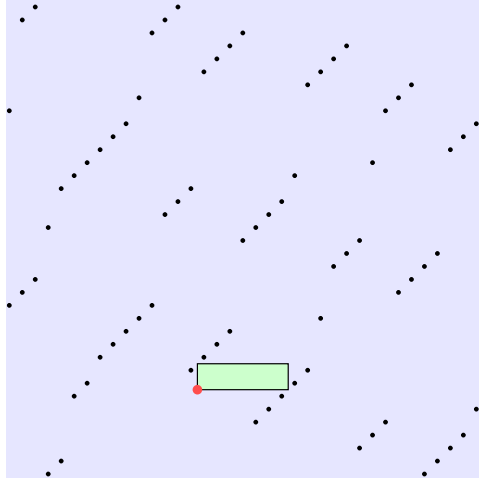

$$x_{13,22,14,7} = x_{14,7,22,8}$$

(351)

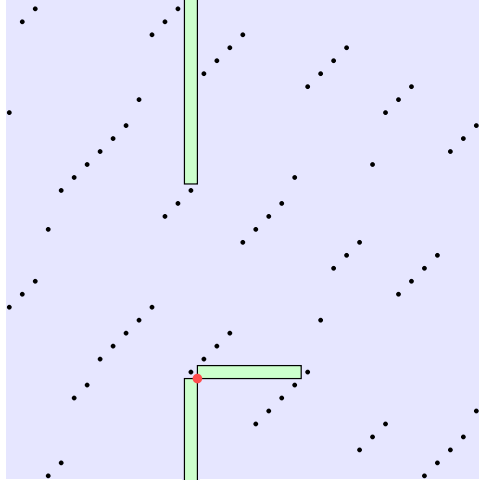

$$\begin{aligned} & x_{7,8,14,9} + x_{8,8,14,10} + x_{9,8,14,11} + x_{10,8,14,12} + x_{11,8,14,19} + x_{12,8,14,20} + x_{13,8,14,21} = \\ & = x_{14,4,19,8} + x_{14,5,20,8} + x_{14,6,21,8} + x_{14,7,22,8} + x_{14,31,15,8} + x_{14,32,16,8} + x_{14,33,17,8} + x_{14,34,18,8} \end{aligned} \quad (352)$$



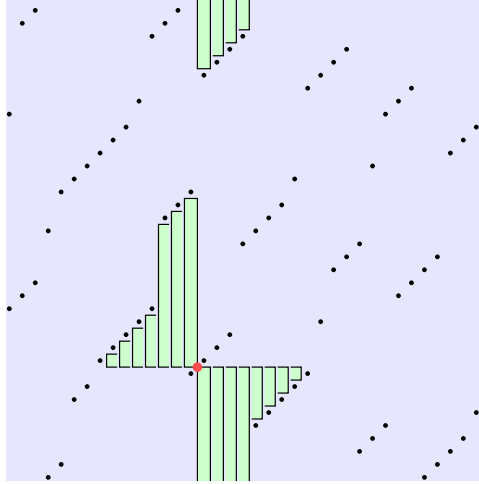

$$x_{7,8,14,9} = x_{14,9,15,30}$$

(353)

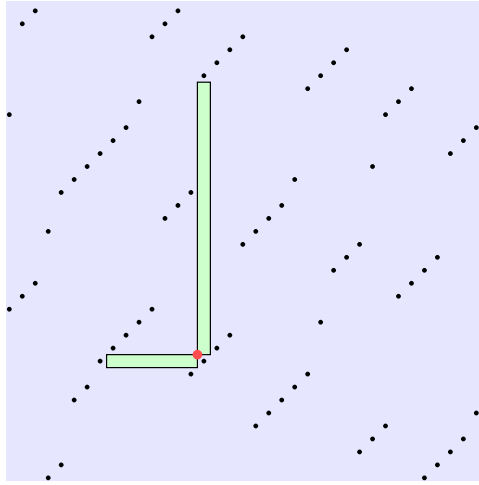

$$x_{8,8,14,10} = x_{14,10,16,30}$$

(354)

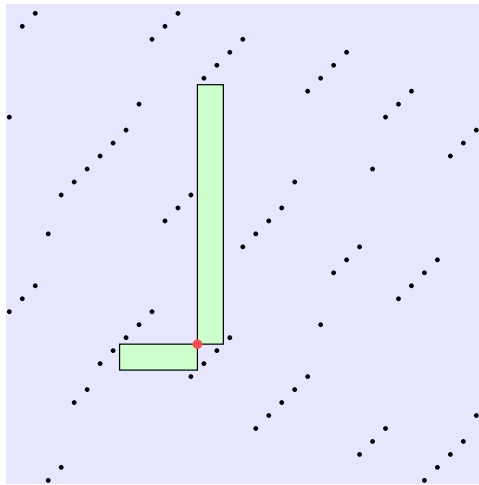

$$x_{9,8,14,11} = x_{14,11,17,30} \tag{355}$$

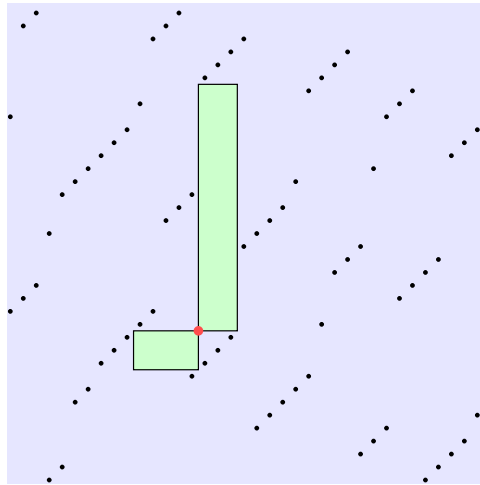

$$x_{10,8,14,12} = 0 \tag{356}$$

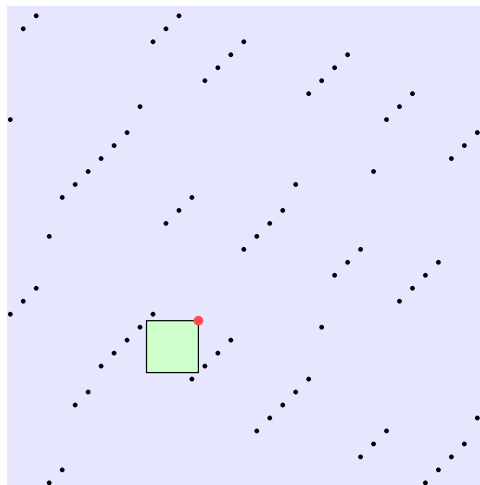

$$0 = x_{14,18,18,30} \tag{357}$$

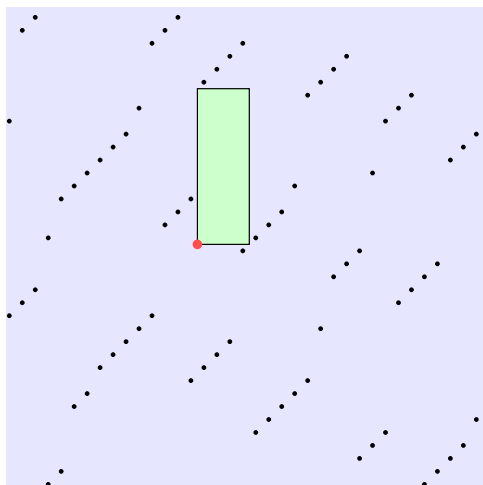

$$x_{11,8,14,19} = x_{14,19,19,30}$$

(358)

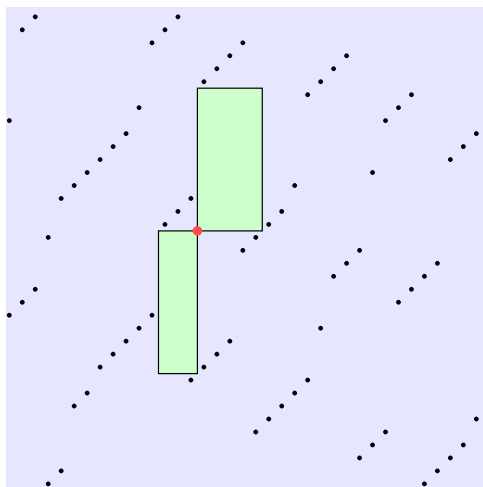

$$x_{12,8,14,20} = x_{14,20,20,30}$$

(359)

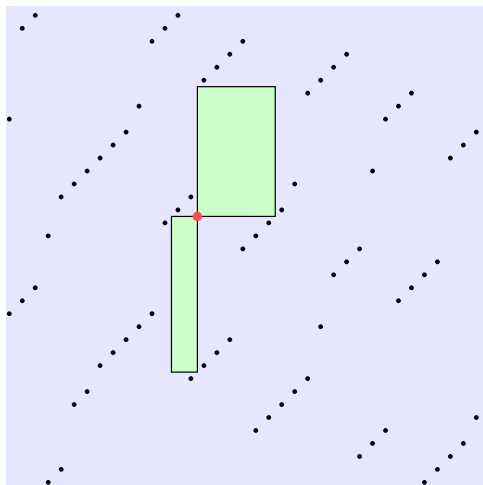

$$x_{13,8,14,21} = x_{14,21,3,22} + x_{14,21,21,30}$$

(360)

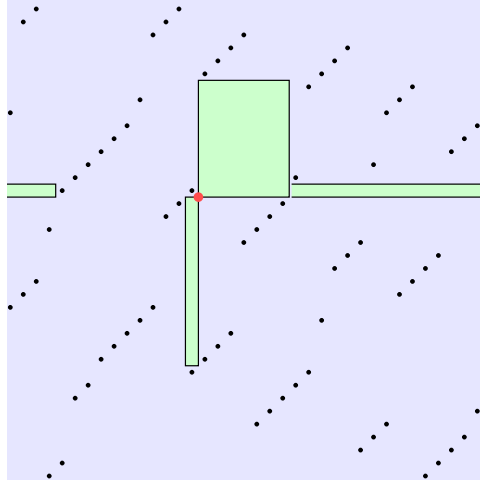

$$x_{10,22,14,33} + x_{11,22,14,34} + x_{12,22,14,35} + x_{13,22,14,7} = x_{14,21,3,22}$$

(361)

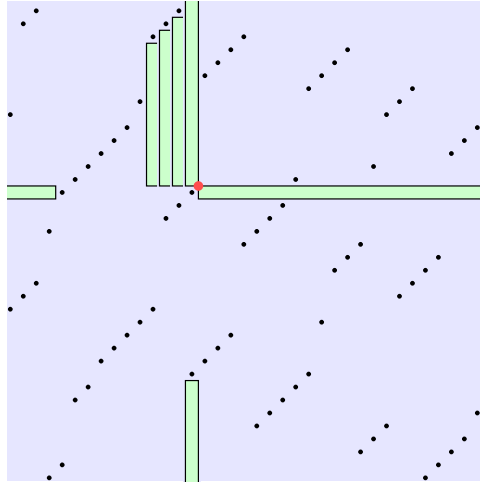

$$x_{31,29,14,33} = 0$$

(362)

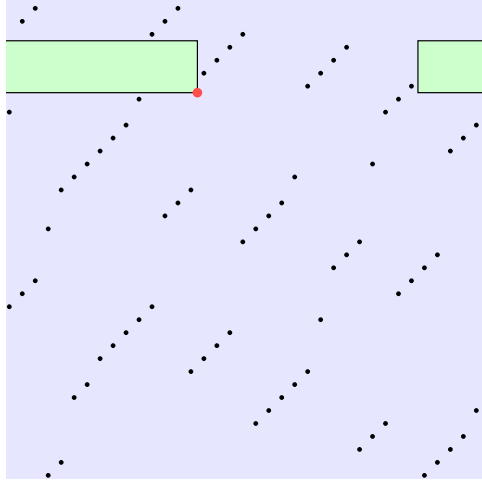

$$\begin{aligned}
 x_{24,30,14,31} + x_{25,30,14,32} + x_{26,30,14,33} = \\
 = x_{14,9,15,30} + x_{14,10,16,30} + x_{14,11,17,30} + x_{14,18,18,30} + x_{14,19,19,30} + x_{14,20,20,30} + x_{14,21,21,30} \quad (363)
 \end{aligned}$$

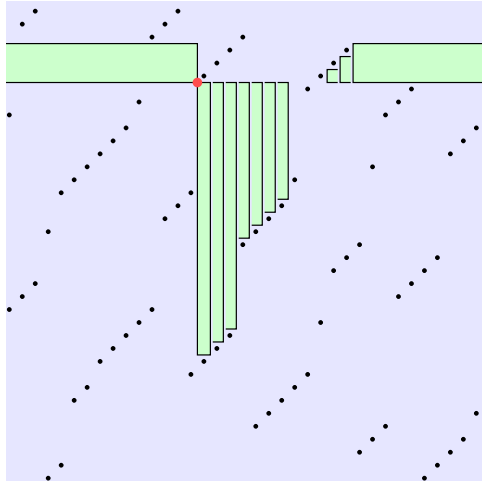

$$x_{24,30,14,31} = x_{14,31,15,8} \quad (364)$$

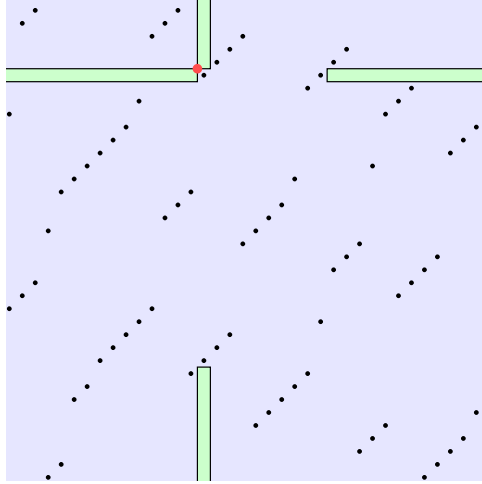

$$x_{25,30,14,32} = x_{14,32,16,8}$$

(365)

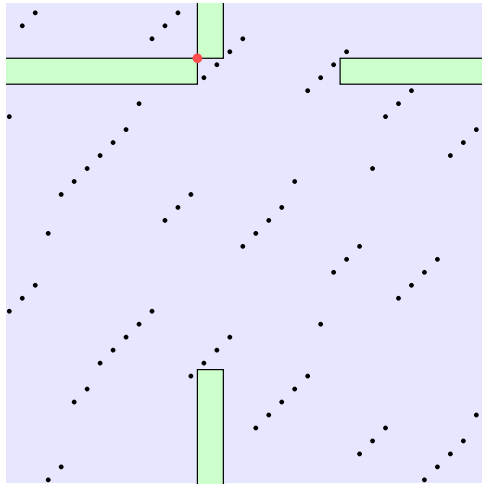

$$x_{10,22,14,33} + x_{26,30,14,33} + x_{31,29,14,33} = x_{14,33,17,8}$$

(366)

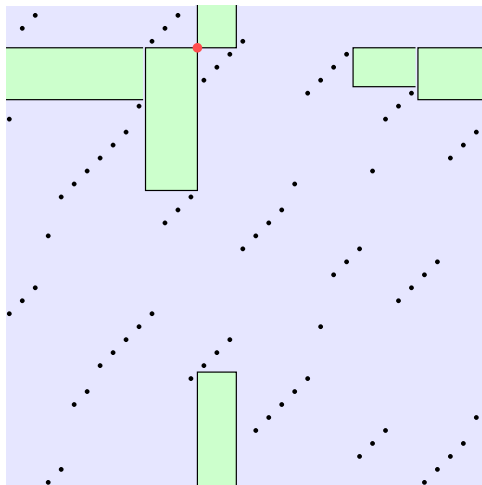

$$x_{11,22,14,34} = x_{14,34,18,8} \tag{367}$$

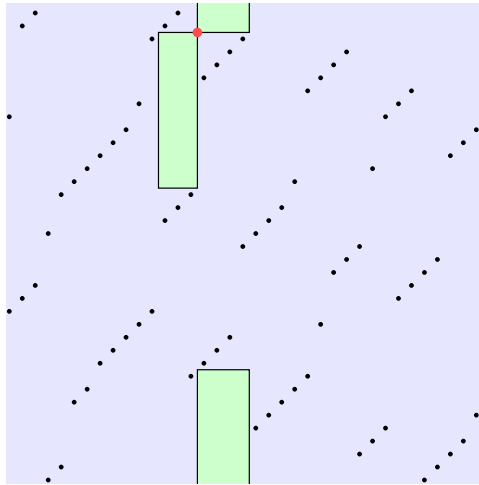

$$x_{12,22,14,35} = 0 \tag{368}$$

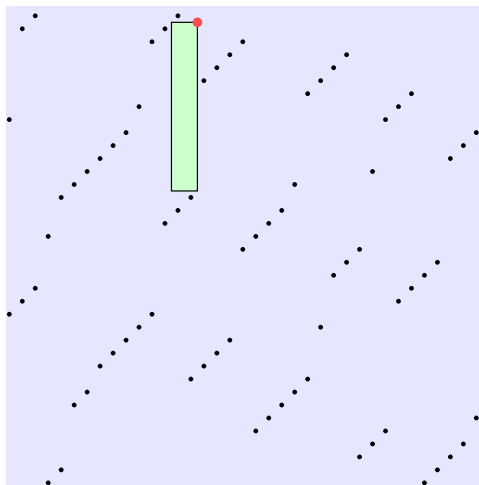

$$0 = x_{15,4,19,9} \tag{369}$$

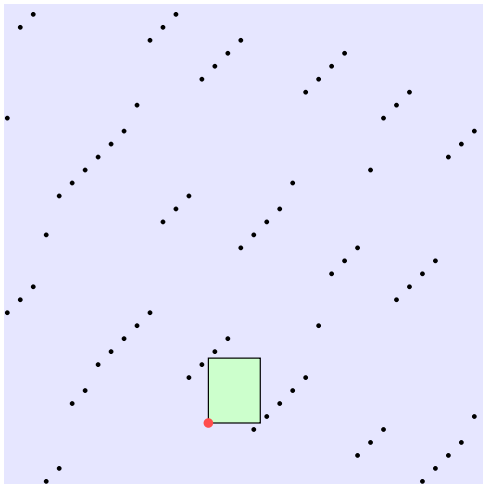

$$0 = x_{15,5,20,9}$$

(370)

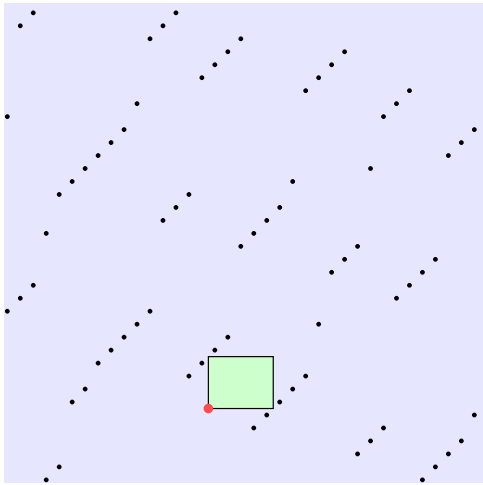

$$0 = x_{15,6,21,9}$$

(371)

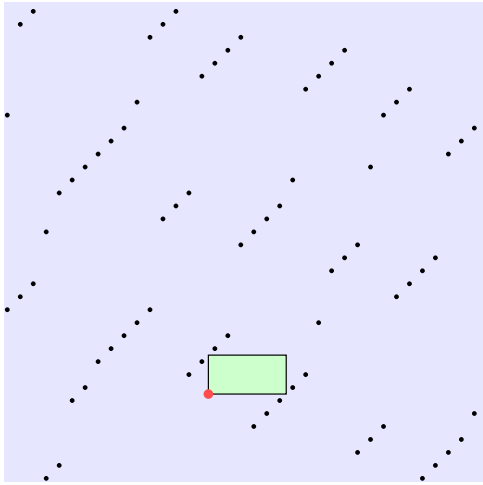



$$x_{13,31,15,7} = x_{15,7,22,9} \quad (372)$$

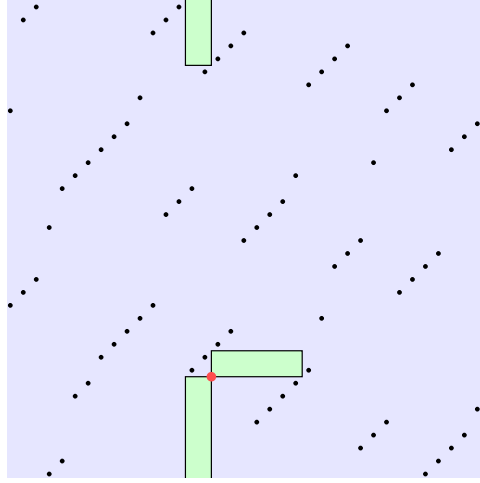

$$x_{14,31,15,8} = x_{15,8,6,9} \quad (373)$$

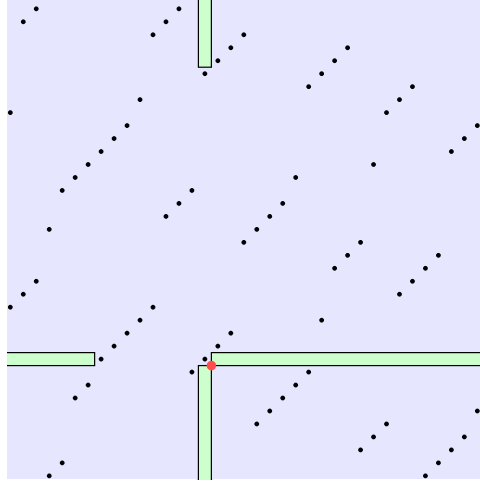

$$\begin{aligned} x_{8,9,15,10} + x_{9,9,15,11} + x_{10,9,15,12} + x_{11,9,15,19} + x_{12,9,15,20} + x_{13,9,15,21} + x_{14,9,15,30} = \\ = x_{15,4,19,9} + x_{15,5,20,9} + x_{15,6,21,9} + x_{15,7,22,9} + x_{15,8,6,9} + x_{15,32,16,9} + x_{15,33,17,9} + x_{15,34,18,9} \end{aligned} \quad (374)$$

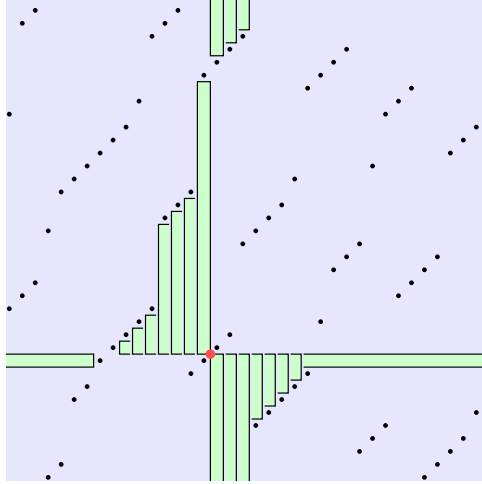

$$x_{8,9,15,10} = x_{15,10,16,31}$$

(375)

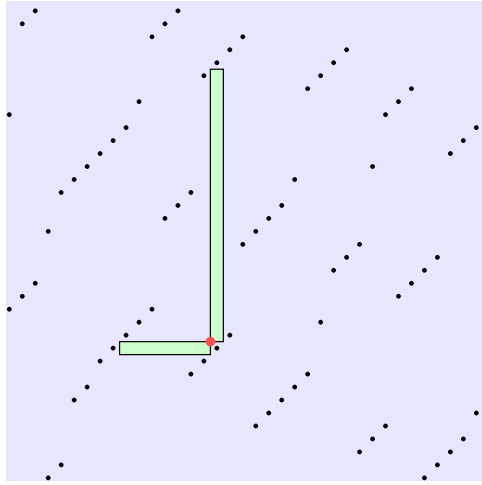

$$x_{9,9,15,11} = x_{15,11,17,31}$$

(376)

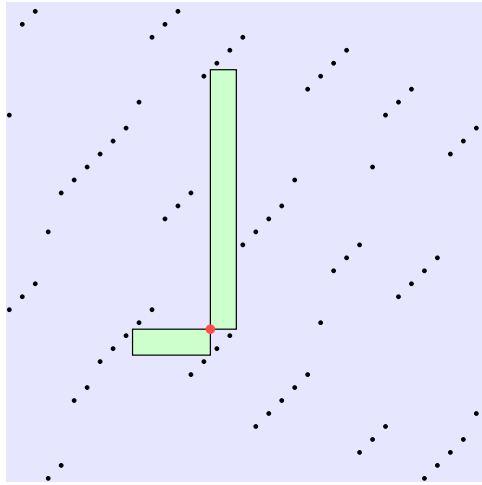

$$x_{10,9,15,12} = 0 \tag{377}$$

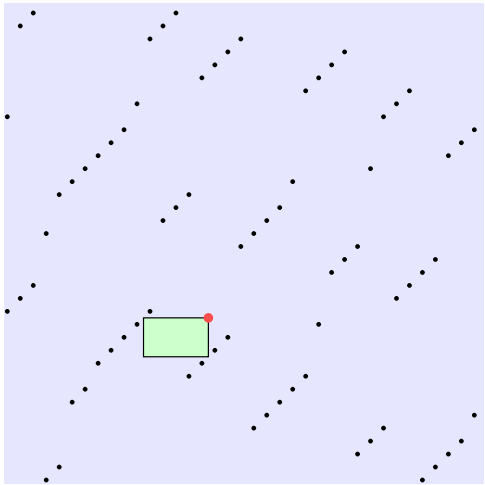

$$0 = x_{15,18,18,31} \tag{378}$$

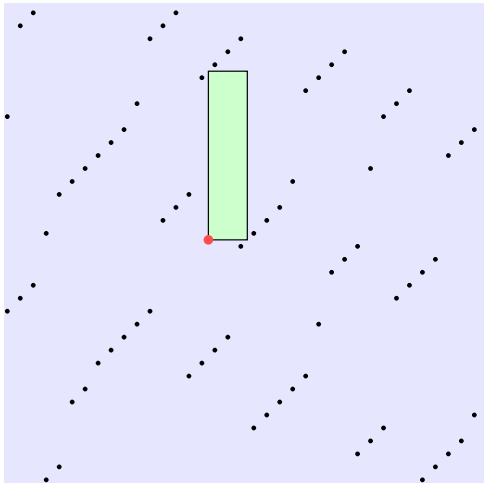

$$x_{11,9,15,19} = x_{15,19,19,31} \tag{379}$$

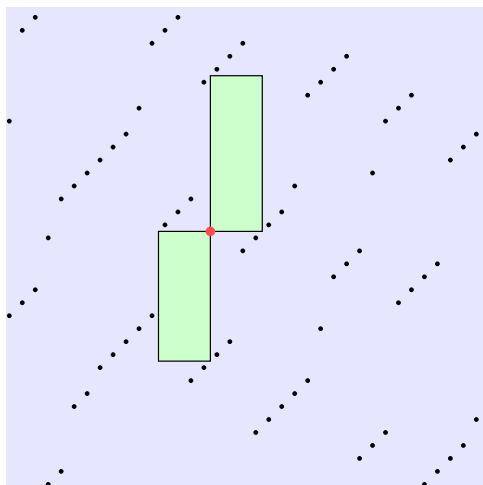

$$x_{12,9,15,20} = x_{15,20,20,31}$$

(380)

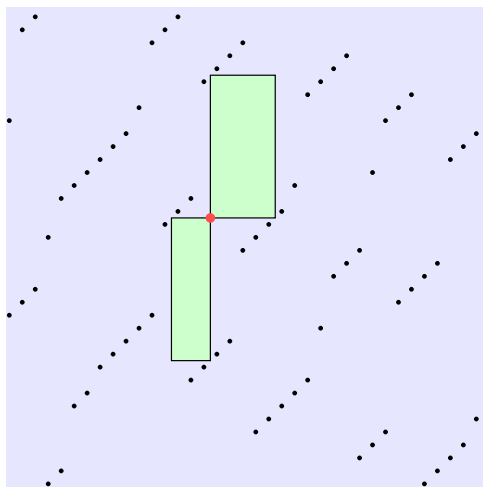

$$x_{13,9,15,21} = x_{15,21,21,31}$$

(381)

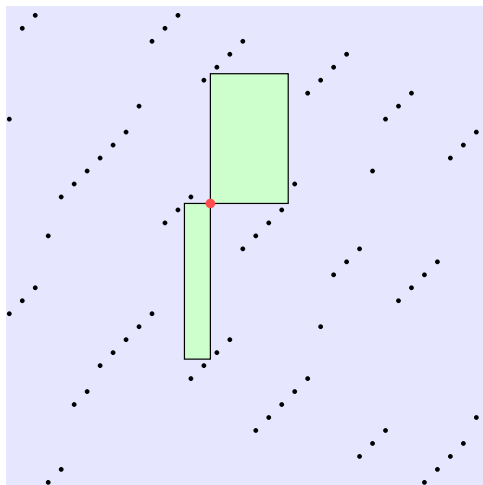

$$0 = x_{15,23,22,31} \quad (382)$$

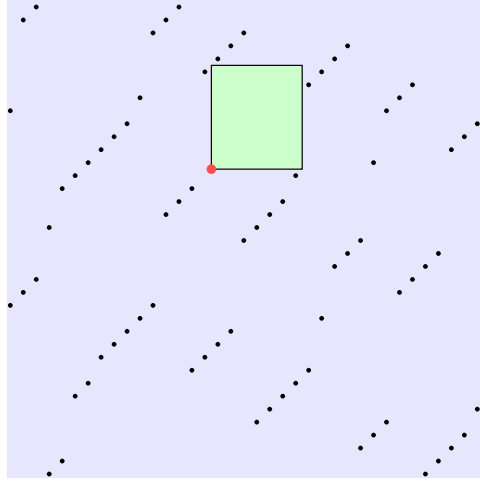

$$x_{14,9,15,30} = x_{15,30,23,31} \quad (383)$$

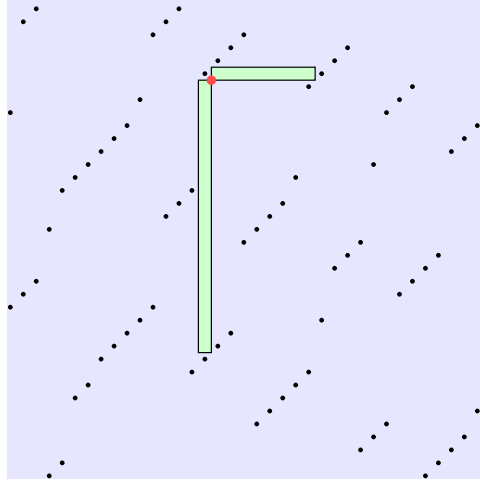

$$\begin{aligned} & x_{11,31,15,34} + x_{12,31,15,35} + x_{13,31,15,7} + x_{14,31,15,8} + x_{25,31,15,32} + x_{26,31,15,33} = \\ & = x_{15,10,16,31} + x_{15,11,17,31} + x_{15,18,18,31} + x_{15,19,19,31} + x_{15,20,20,31} + x_{15,21,21,31} + x_{15,23,22,31} + x_{15,30,23,31} \end{aligned} \quad (384)$$

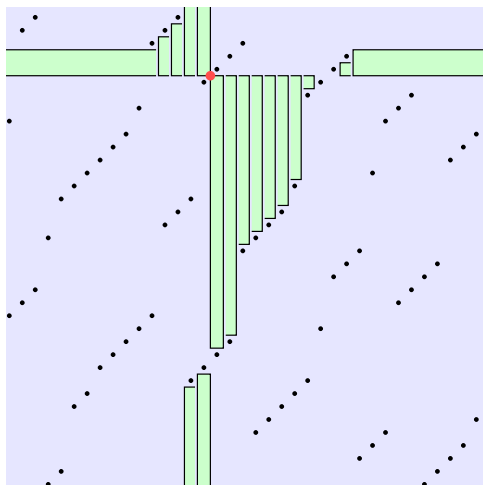

$$x_{25,31,15,32} = x_{15,32,16,9}$$

(385)

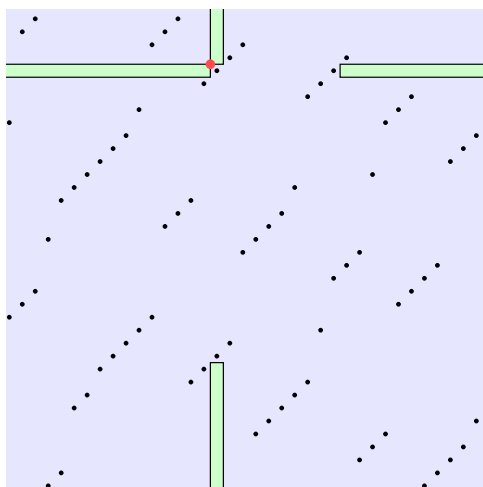

$$x_{26,31,15,33} = x_{15,33,17,9}$$

(386)

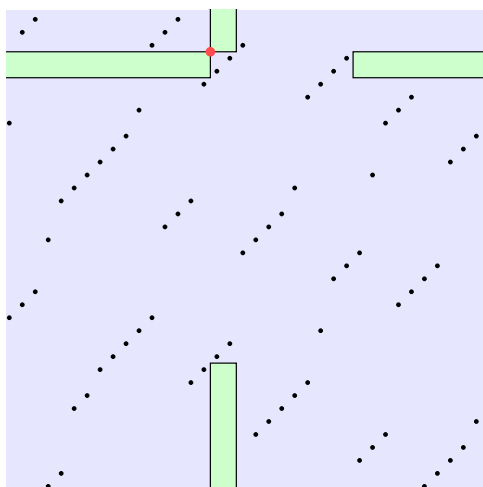

$$x_{11,31,15,34} = x_{15,34,18,9} \tag{387}$$

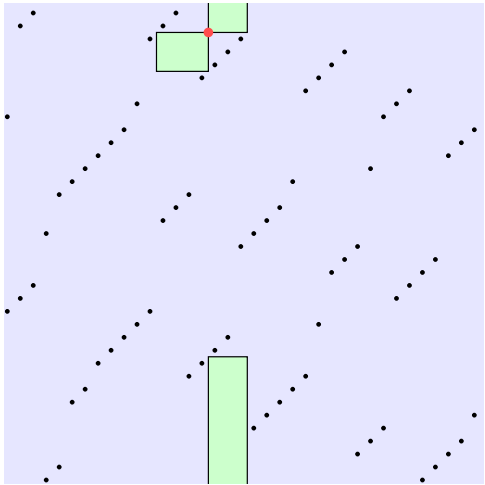

$$x_{12,31,15,35} = 0 \tag{388}$$

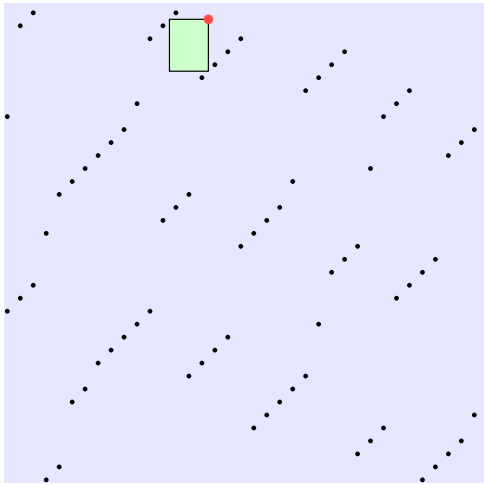

$$0 = x_{16,4,19,10} \tag{389}$$

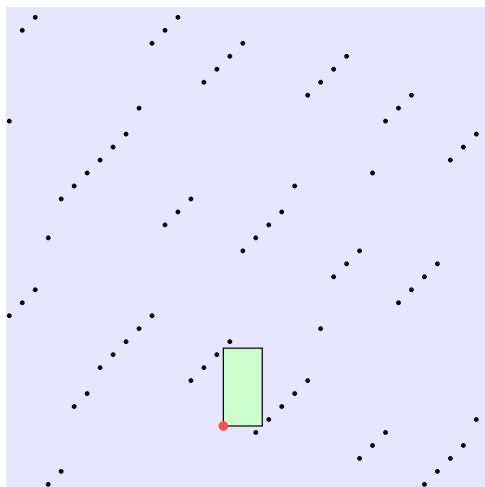

$$0 = x_{16,5,20,10}$$

(390)

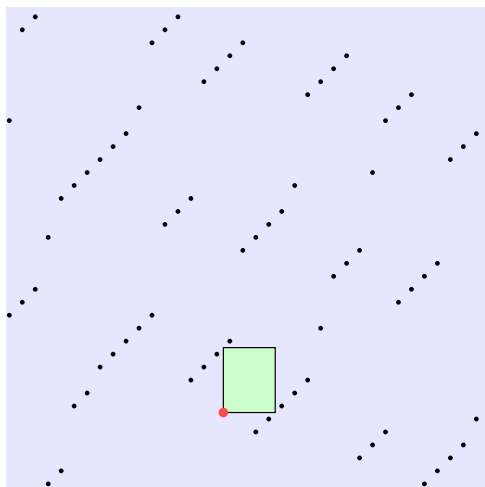

$$0 = x_{16,6,21,10}$$

(391)

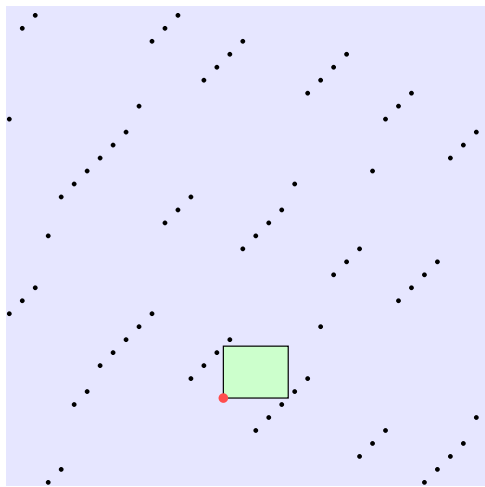



$$x_{13,32,16,7} = x_{16,7,22,10} \tag{392}$$

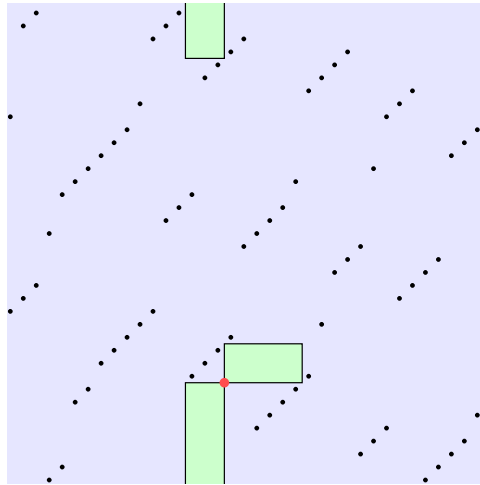

$$x_{14,32,16,8} = x_{16,8,6,10} \tag{393}$$

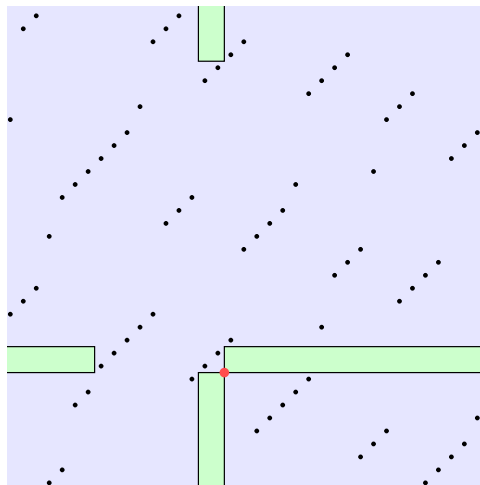

$$x_{15,32,16,9} = x_{16,9,7,10} \tag{394}$$

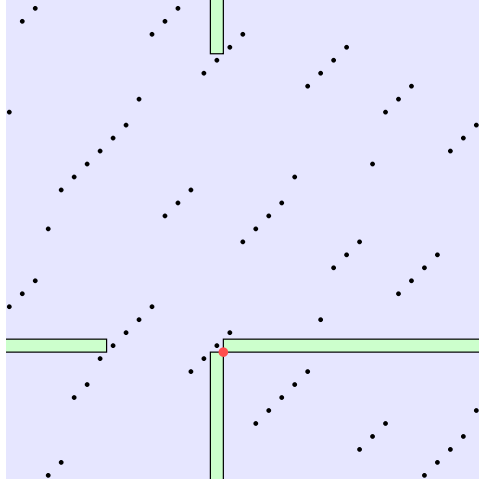

$$\begin{aligned}
 & x_{9,10,16,11} + x_{10,10,16,12} + x_{11,10,16,19} + x_{12,10,16,20} + x_{13,10,16,21} + x_{14,10,16,30} + x_{15,10,16,31} = \\
 & = x_{16,4,19,10} + x_{16,5,20,10} + x_{16,6,21,10} + x_{16,7,22,10} + x_{16,8,6,10} + x_{16,9,7,10} + x_{16,33,17,10} + x_{16,34,18,10} \quad (395)
 \end{aligned}$$

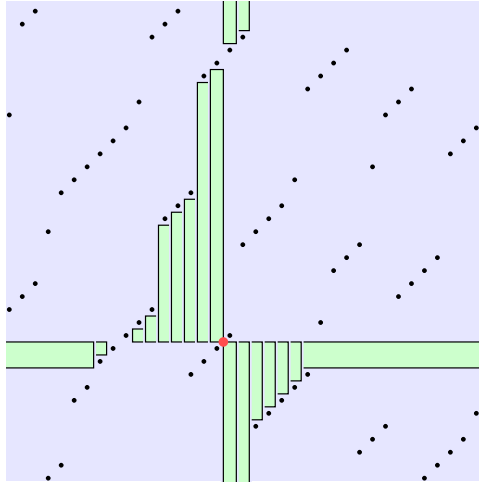

$$x_{9,10,16,11} = x_{16,11,17,32} \quad (396)$$

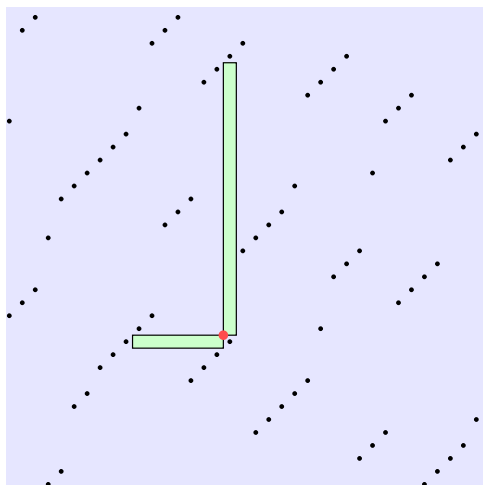

$$x_{10,10,16,12} = 0$$

(397)

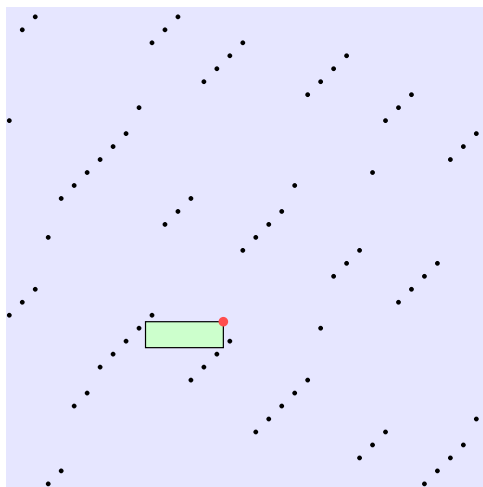

$$0 = x_{16,18,18,32}$$

(398)

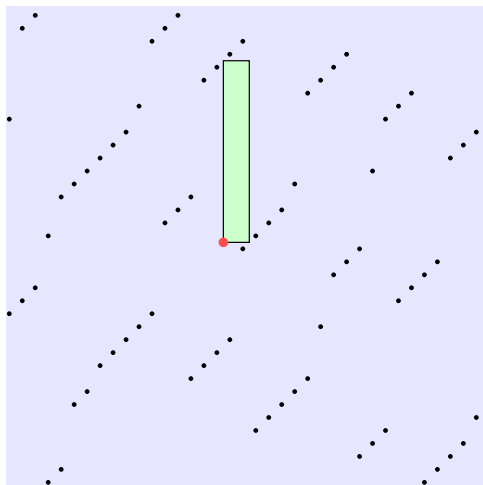

$$x_{11,10,16,19} = x_{16,19,19,32} \tag{399}$$

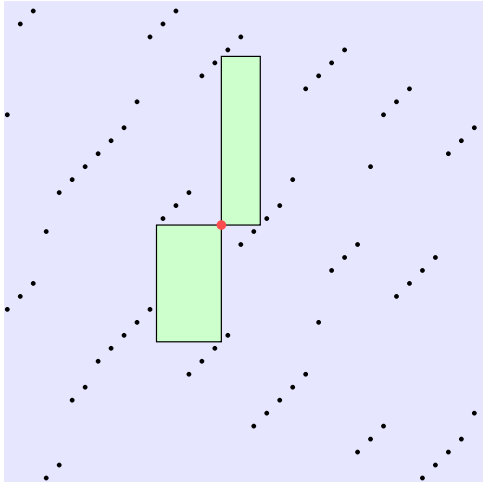

$$x_{12,10,16,20} = x_{16,20,20,32} \tag{400}$$

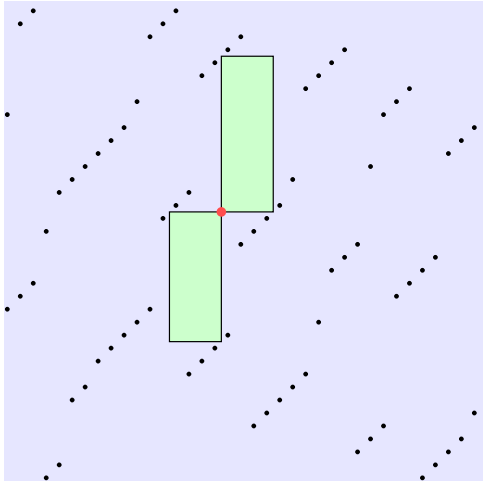

$$x_{13,10,16,21} = x_{16,21,21,32} \tag{401}$$

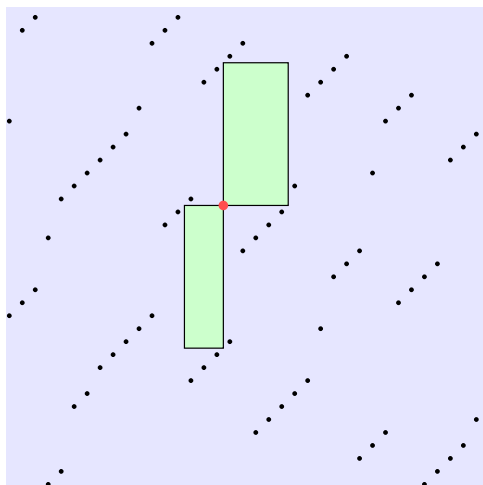

$$0 = x_{16,23,22,32}$$

(402)

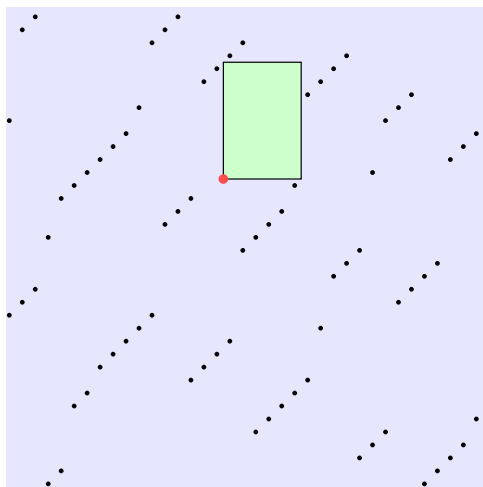

$$x_{14,10,16,30} = x_{16,30,23,32}$$

(403)

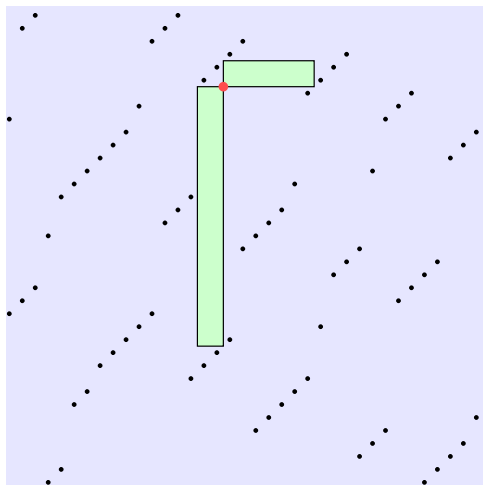

$$x_{15,10,16,31} = x_{16,31,24,32} \quad (404)$$

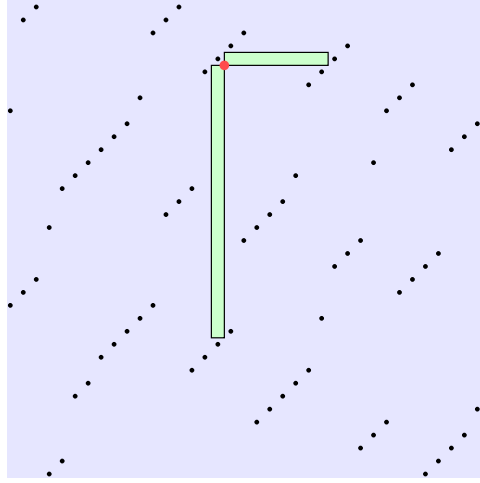

$$\begin{aligned} & x_{11,32,16,34} + x_{12,32,16,35} + x_{13,32,16,7} + x_{14,32,16,8} + x_{15,32,16,9} + x_{26,32,16,33} = \\ & = x_{16,11,17,32} + x_{16,18,18,32} + x_{16,19,19,32} + x_{16,20,20,32} + x_{16,21,21,32} + x_{16,23,22,32} + x_{16,30,23,32} + x_{16,31,24,32} \end{aligned} \quad (405)$$

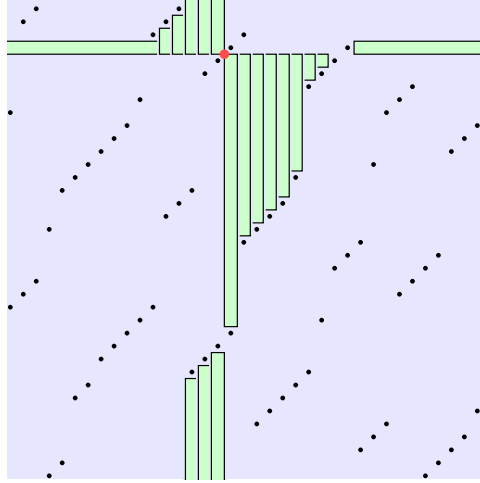

$$x_{26,32,16,33} = x_{16,33,17,10} \quad (406)$$

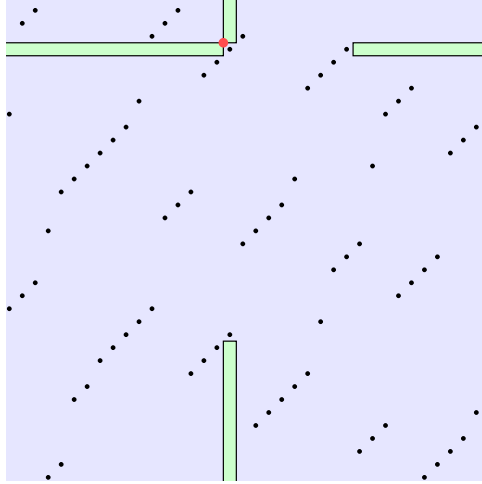

$$x_{11,32,16,34} = x_{16,34,18,10}$$

(407)

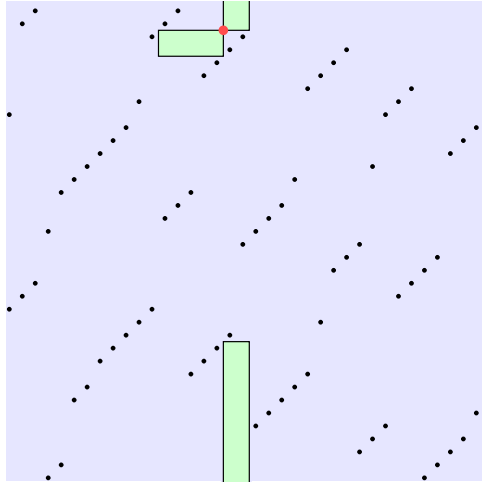

$$x_{12,32,16,35} = 0$$

(408)

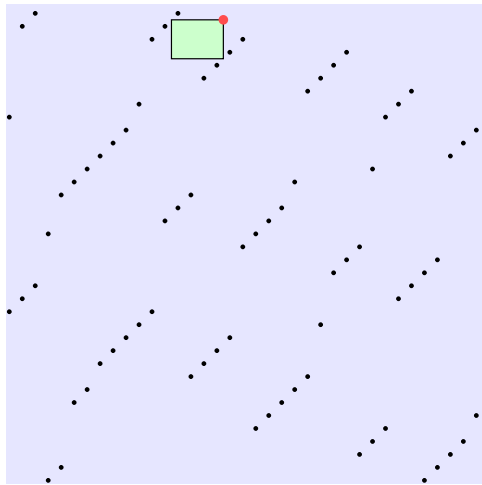

$$0 = x_{17,4,19,17}$$

(409)

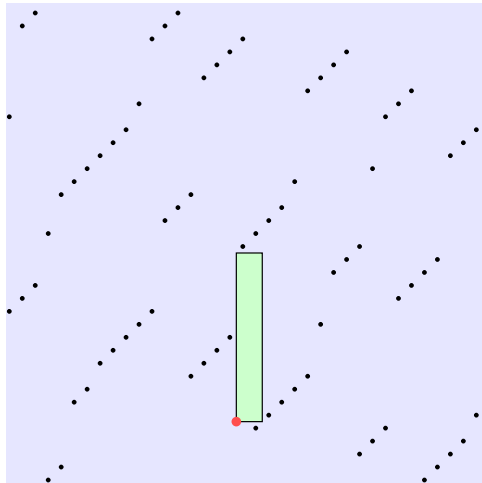

$$0 = x_{17,5,20,17}$$

(410)

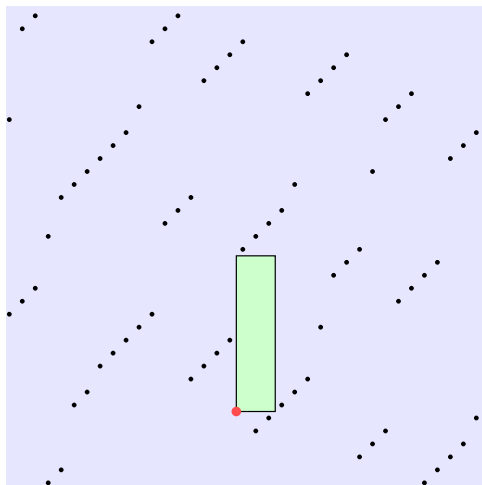

$$0 = x_{17,6,21,17}$$

(411)



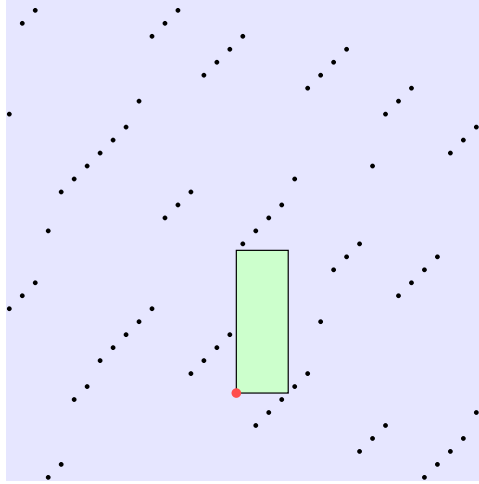

$$x_{13,33,17,7} = x_{17,7,22,17}$$

(412)

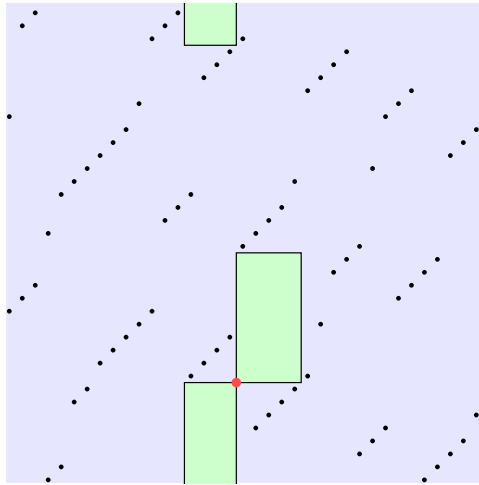

$$x_{14,33,17,8} = x_{17,8,6,11} + x_{17,8,23,17}$$

(413)

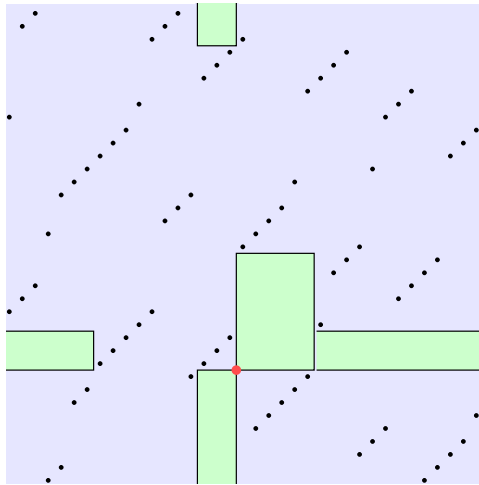

$$x_{15,33,17,9} = x_{17,9,7,11} \quad (414)$$

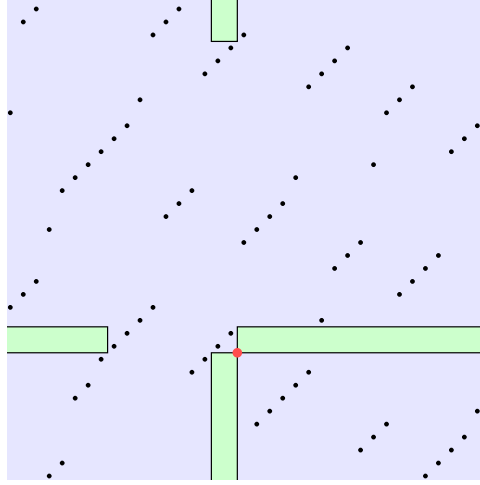

$$x_{16,33,17,10} = x_{17,10,8,11} \quad (415)$$

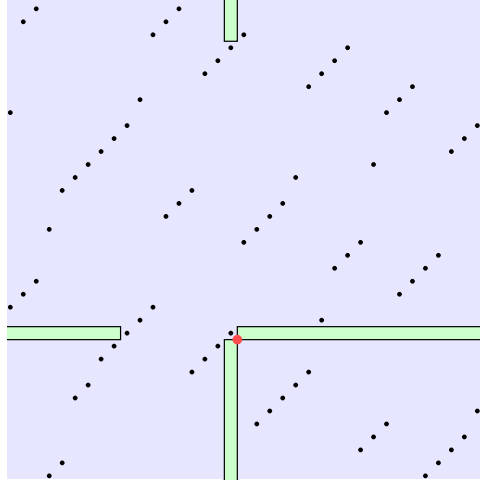

$$x_{11,11,17,19} + x_{12,11,17,20} + x_{13,11,17,21} + x_{14,11,17,30} + x_{15,11,17,31} + x_{16,11,17,32} = x_{17,8,6,11} + x_{17,9,7,11} + x_{17,10,8,11} \quad (416)$$

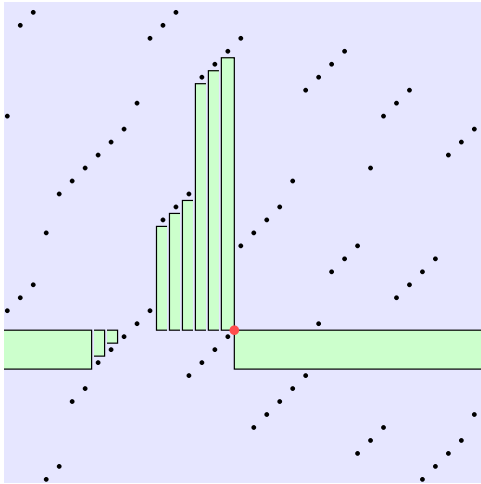

$$x_{2,13,17,18} + x_{3,13,17,19} = 0$$

(417)

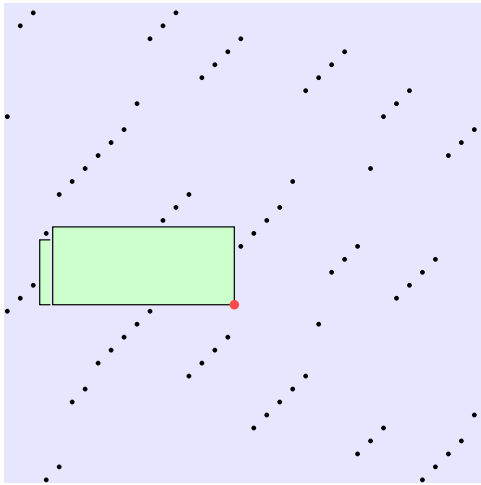

$$x_{33,15,17,18} = 0$$

(418)

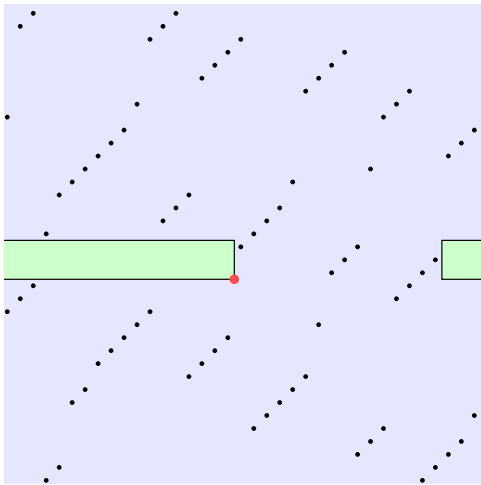

$$x_{27,17,17,18} = x_{17,4,19,17} + x_{17,5,20,17} + x_{17,6,21,17} + x_{17,7,22,17} + x_{17,8,23,17} + x_{17,34,18,17} \quad (419)$$

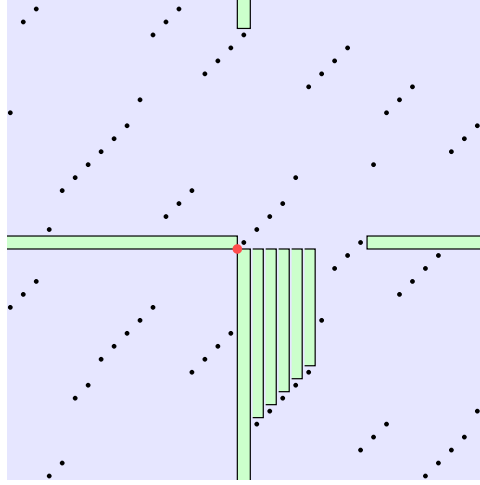

$$x_{2,13,17,18} + x_{27,17,17,18} + x_{33,15,17,18} = x_{17,18,18,33} \quad (420)$$

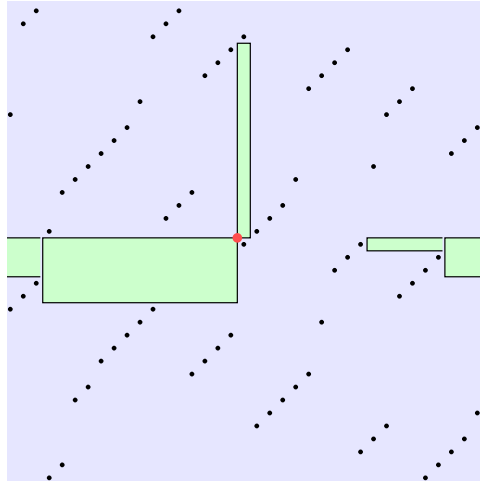

$$x_{3,13,17,19} + x_{11,11,17,19} = x_{17,19,19,33} \quad (421)$$

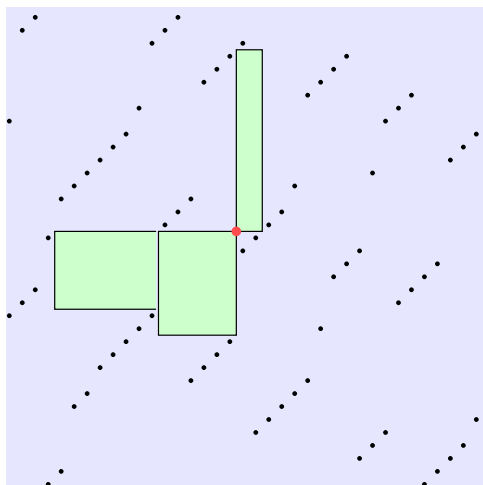

$$x_{12,11,17,20} = x_{17,20,20,33}$$

(422)

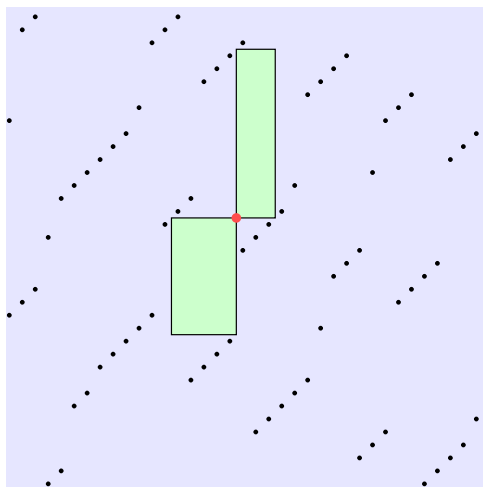

$$x_{13,11,17,21} = x_{17,21,21,33}$$

(423)

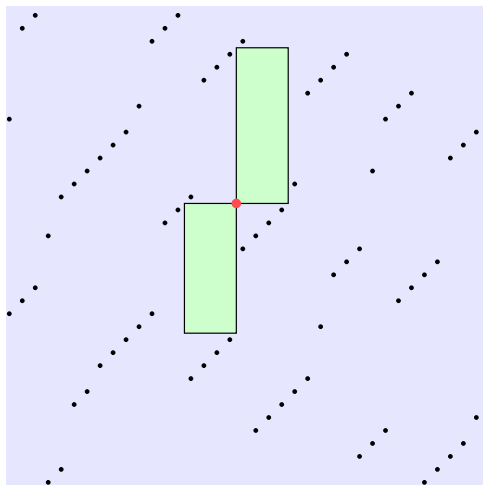

$$0 = x_{17,23,22,33} \tag{424}$$

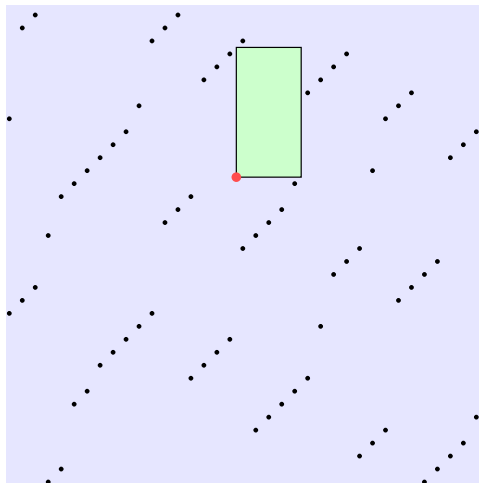

$$x_{14,11,17,30} = x_{17,30,23,33} \tag{425}$$

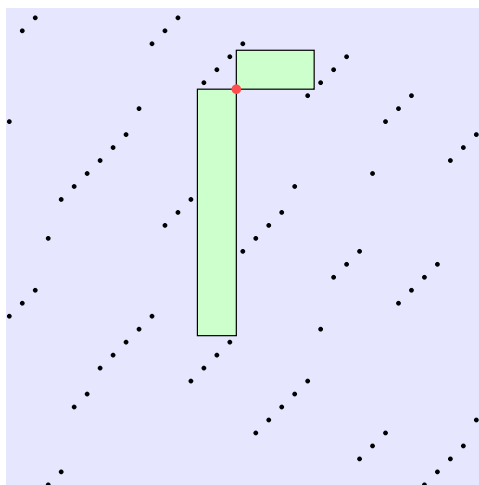

$$x_{15,11,17,31} = x_{17,31,24,33} \tag{426}$$

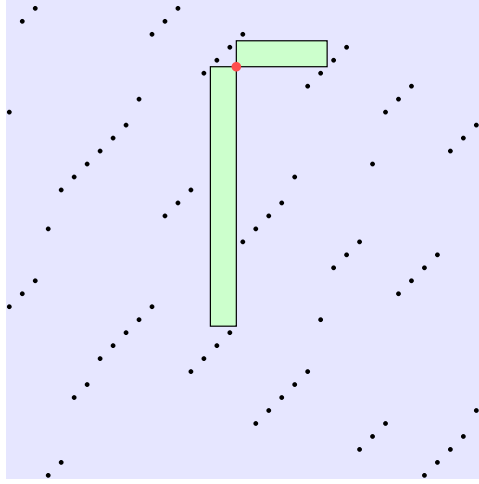

$$x_{16,11,17,32} = x_{17,32,25,33}$$

(427)

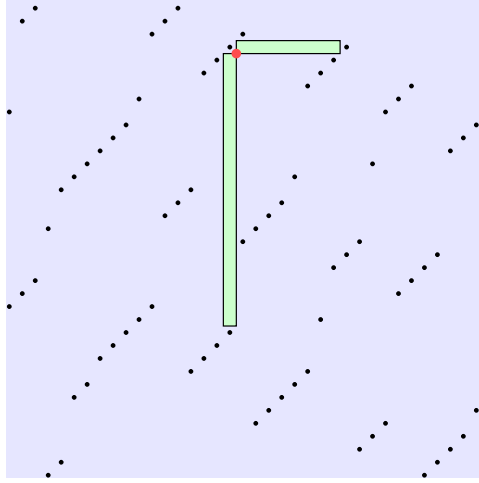

$$\begin{aligned} & x_{11,33,17,34} + x_{12,33,17,35} + x_{13,33,17,7} + x_{14,33,17,8} + x_{15,33,17,9} + x_{16,33,17,10} = \\ & = x_{17,18,18,33} + x_{17,19,19,33} + x_{17,20,20,33} + x_{17,21,21,33} + x_{17,23,22,33} + x_{17,30,23,33} + x_{17,31,24,33} + x_{17,32,25,33} \end{aligned} \quad (428)$$

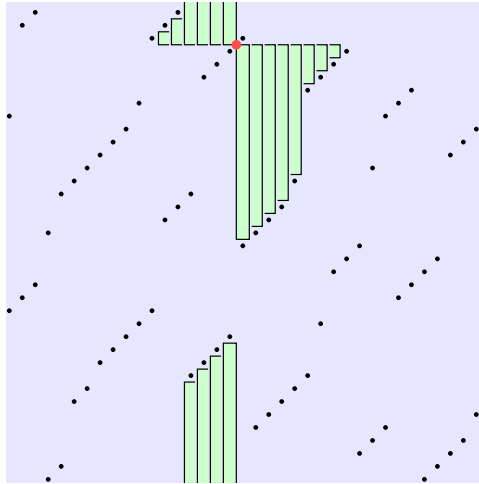

$$x_{11,33,17,34} = x_{17,34,18,17}$$

(429)

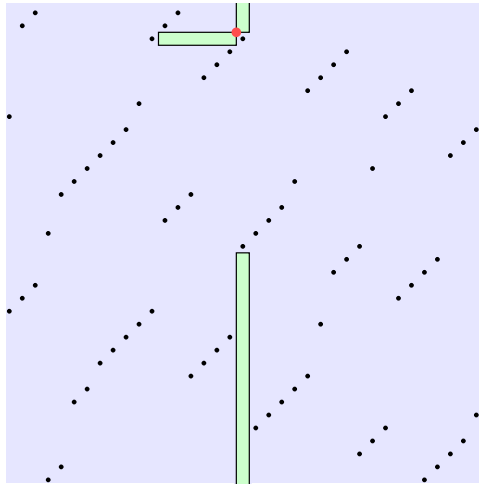

$$x_{12,33,17,35} = 0$$

(430)

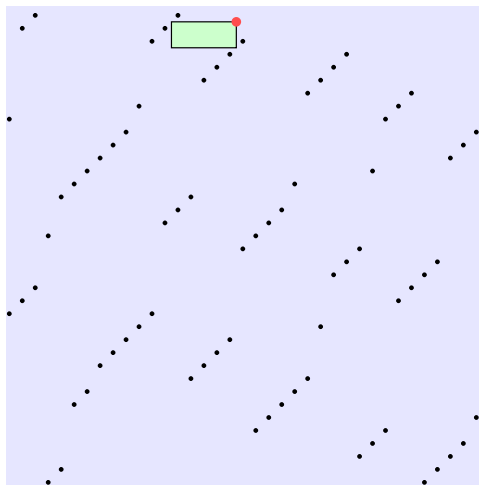



$$x_{35,1,18,4} + x_{36,1,18,5} = x_{18,33,31,1} \quad (431)$$

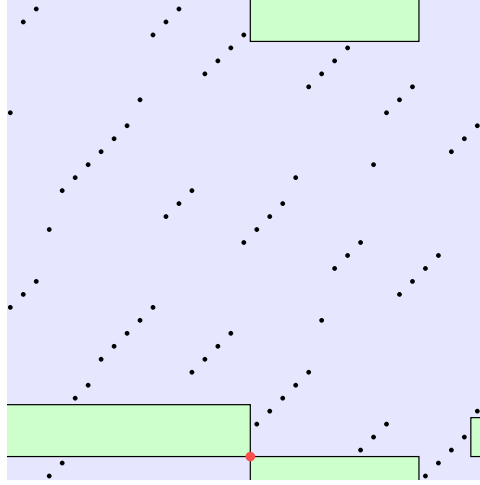

$$x_{29,3,18,4} = x_{18,19,19,3} + x_{18,20,20,3} + x_{18,21,21,3} + x_{18,23,22,3} + x_{18,30,23,3} + x_{18,31,24,3} + x_{18,32,25,3} + x_{18,33,26,3} \quad (432)$$

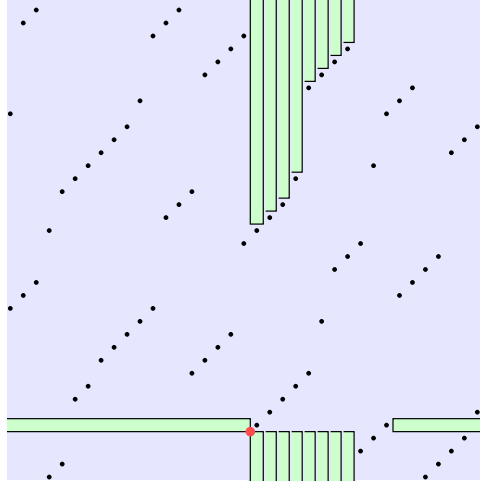

$$x_{29,3,18,4} + x_{35,1,18,4} = x_{18,4,19,18} \quad (433)$$

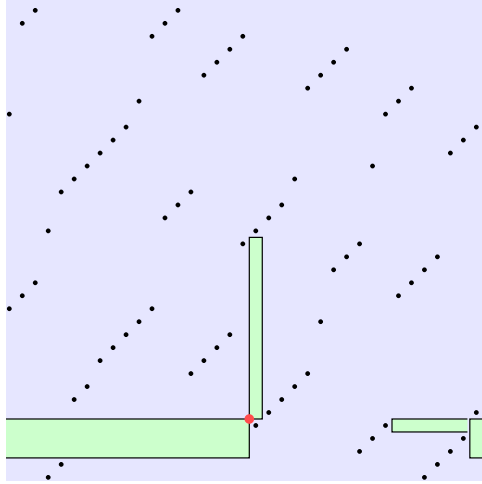

$$x_{4,36,18,5} + x_{36,1,18,5} = x_{18,5,20,18}$$

(434)

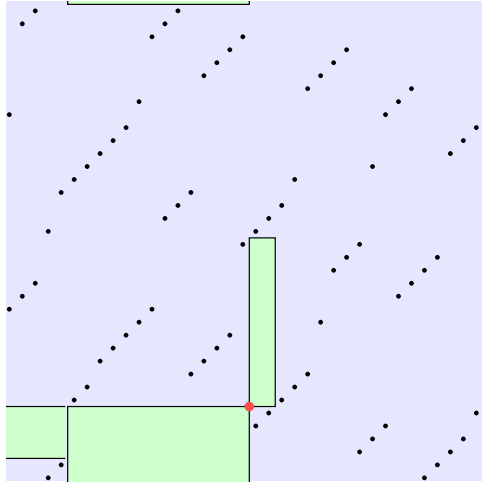

$$x_{5,36,18,6} = x_{18,6,21,18}$$

(435)

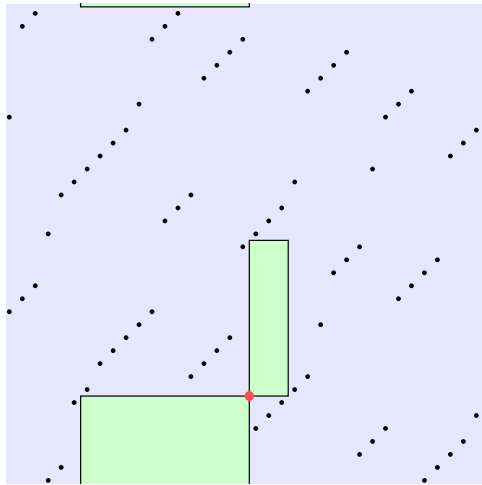

$$x_{6,36,18,7} + x_{13,34,18,7} = x_{18,7,22,18}$$

(436)

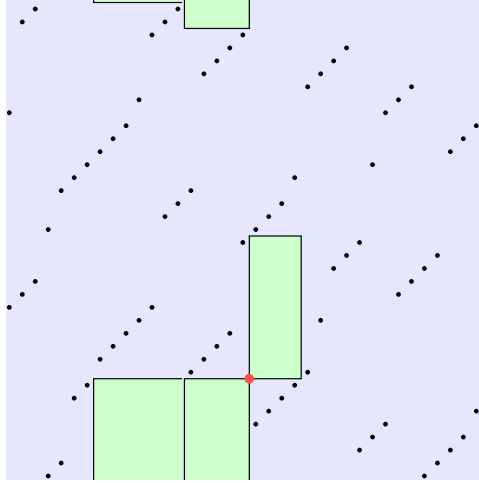

$$x_{14,34,18,8} = x_{18,8,23,18}$$

(437)

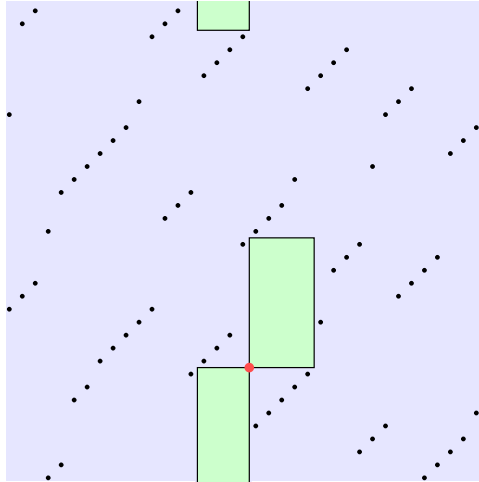

$$x_{15,34,18,9} = 0$$

(438)

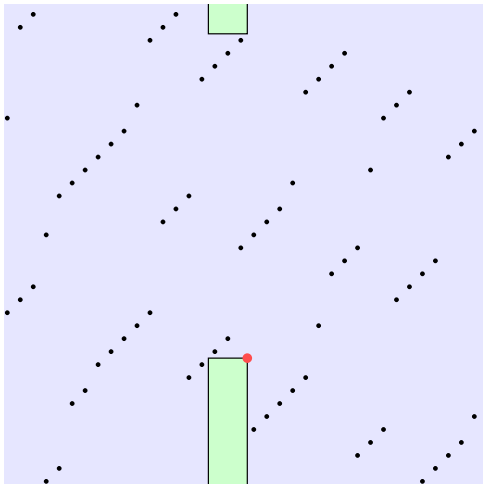

$$x_{16,34,18,10} = 0$$

(439)

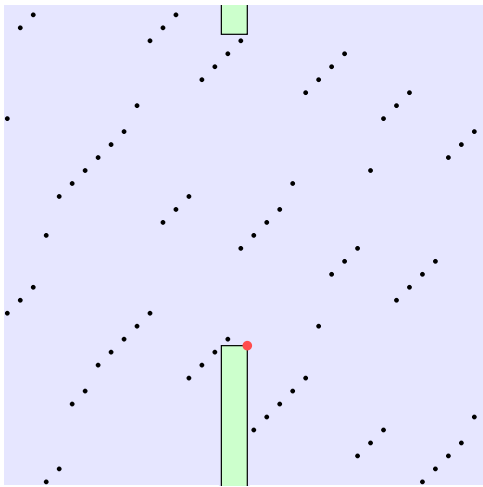

$$0 = x_{18,12,24,18}$$

(440)

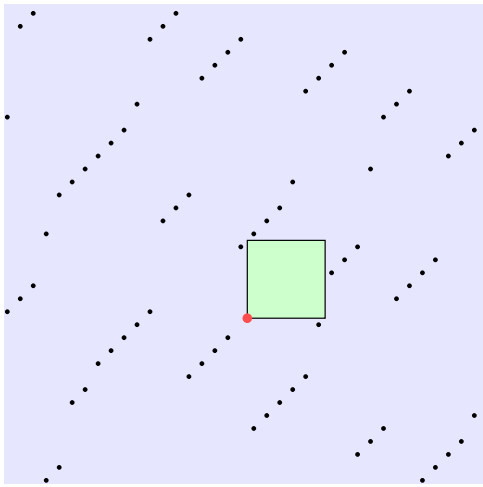

$$0 = x_{18,16,25,18} \quad (441)$$

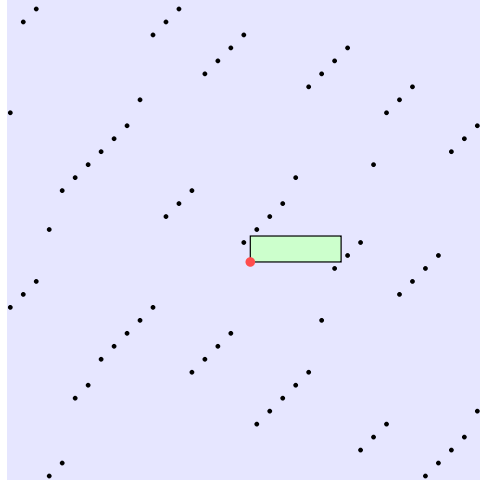

$$x_{17,34,18,17} = x_{18,17,26,18} \quad (442)$$

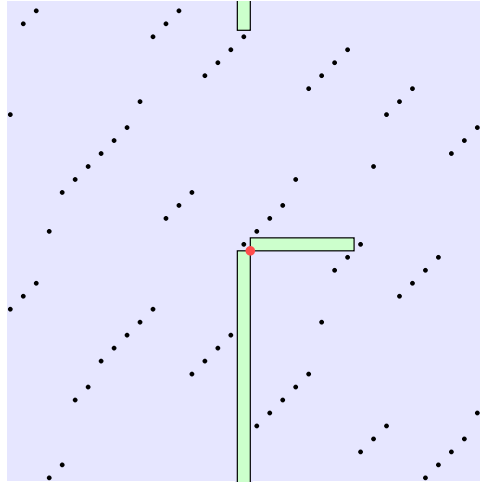

$$\begin{aligned} & x_{3,18,18,19} + x_{12,18,18,20} + x_{13,18,18,21} + x_{14,18,18,30} + x_{15,18,18,31} + x_{16,18,18,32} + x_{17,18,18,33} = \\ & = x_{18,4,19,18} + x_{18,5,20,18} + x_{18,6,21,18} + x_{18,7,22,18} + x_{18,8,23,18} + x_{18,12,24,18} + x_{18,16,25,18} + x_{18,17,26,18} \end{aligned} \quad (443)$$

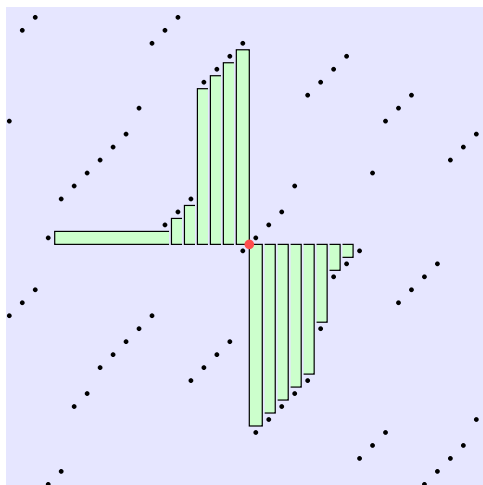

$$x_{3,18,18,19} = x_{18,19,19,3}$$

(444)

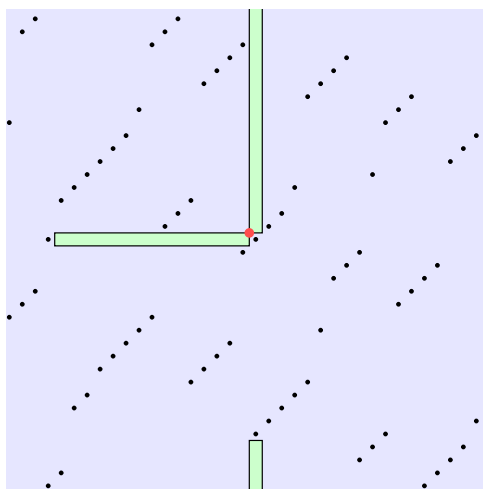

$$x_{12,18,18,20} = x_{18,20,20,3}$$

(445)

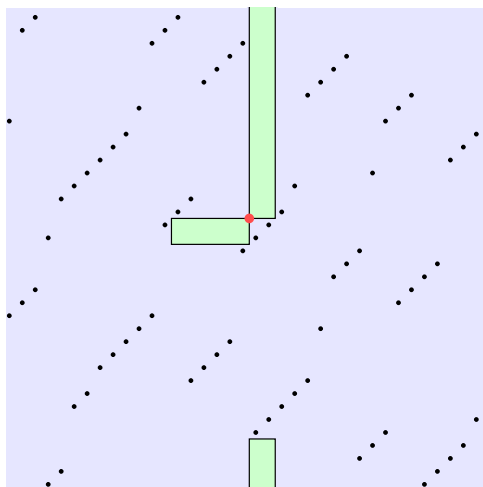

$$x_{13,18,18,21} = x_{18,21,21,3} \quad (446)$$

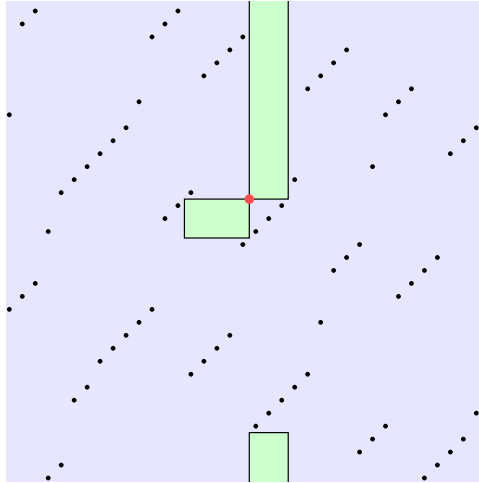

$$0 = x_{18,23,22,3} \quad (447)$$

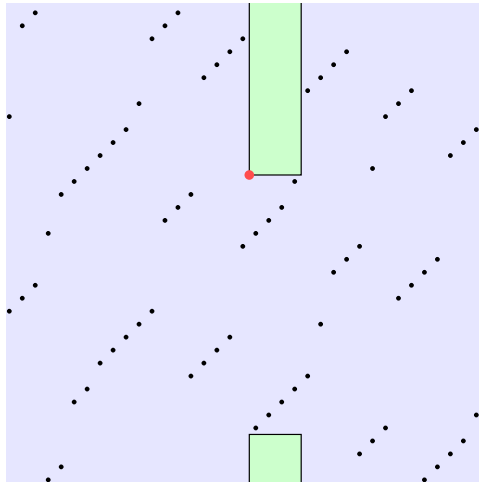

$$x_{14,18,18,30} = x_{18,30,23,3} \quad (448)$$

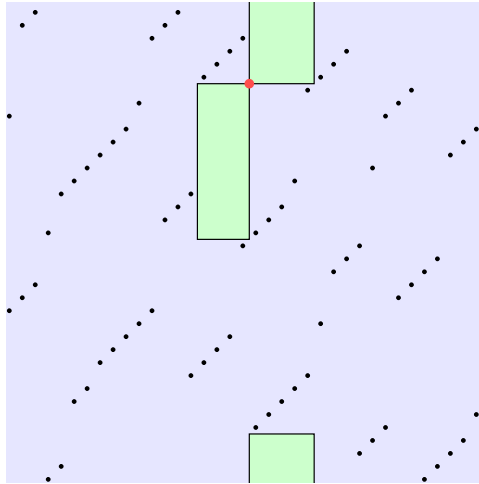

$$x_{15,18,18,31} = x_{18,31,24,3}$$

(449)

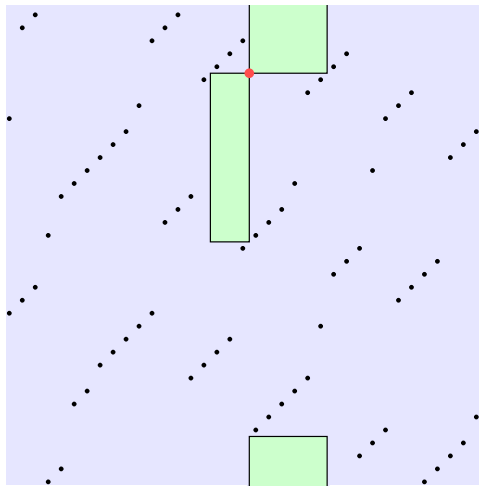

$$x_{16,18,18,32} = x_{18,32,25,3}$$

(450)

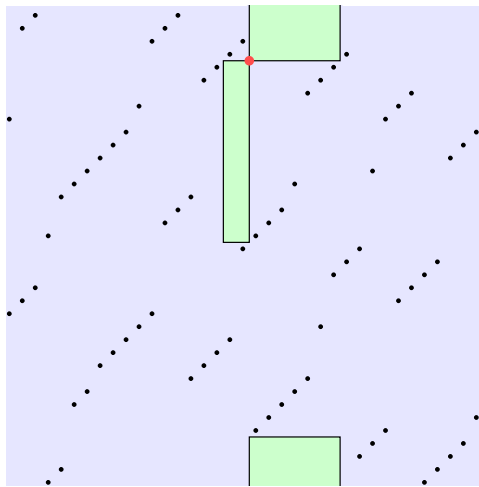



$$x_{17,18,18,33} = x_{18,33,0,36} + x_{18,33,10,34} + x_{18,33,26,3} + x_{18,33,31,1} \quad (451)$$

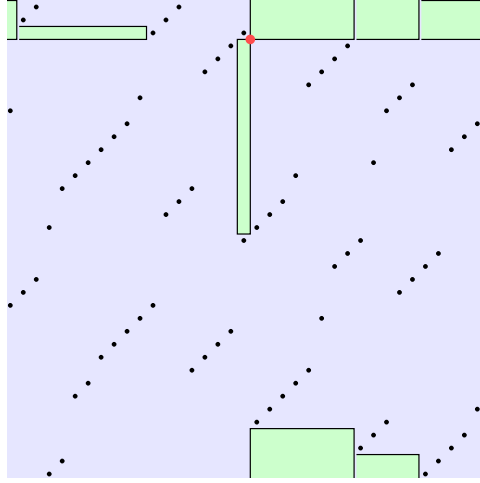

$$x_{13,34,18,7} + x_{14,34,18,8} + x_{15,34,18,9} + x_{16,34,18,10} + x_{17,34,18,17} = x_{18,33,10,34} \quad (452)$$

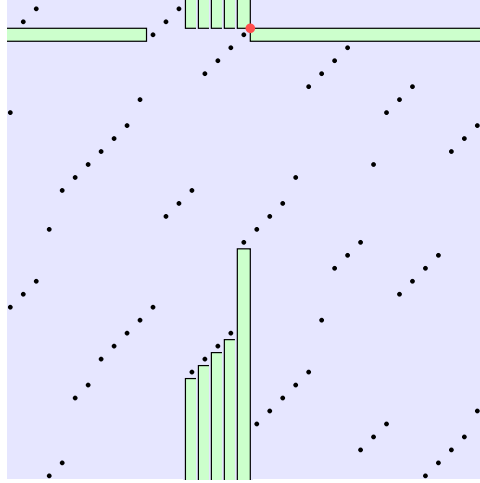

$$x_{4,36,18,5} + x_{5,36,18,6} + x_{6,36,18,7} = x_{18,33,0,36} \quad (453)$$

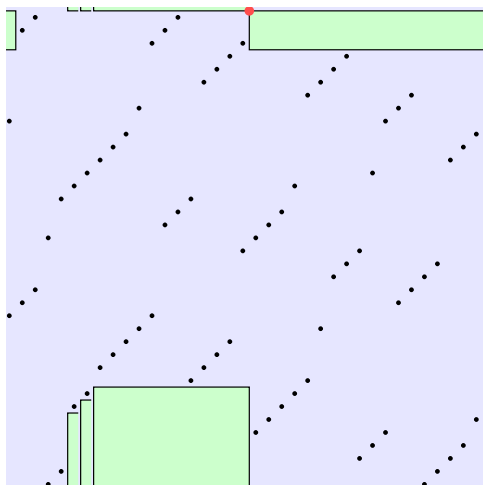

$$0 = x_{19,2,27,4}$$

(454)

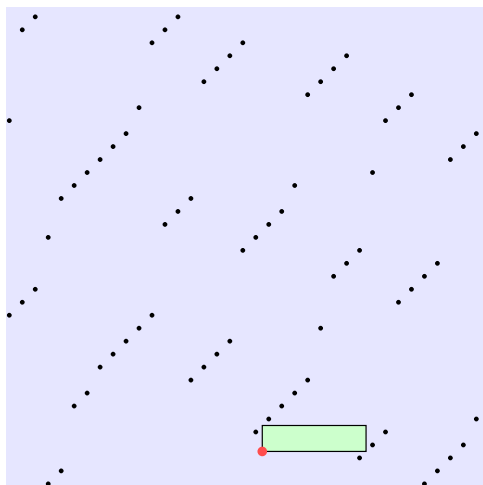

$$x_{18,19,19,3} = x_{19,3,28,4}$$

(455)

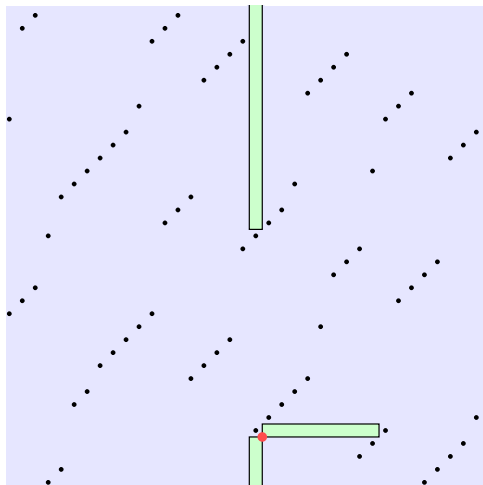

$$\begin{aligned}
& x_{5,4,19,6} + x_{6,4,19,7} + x_{14,4,19,8} + x_{15,4,19,9} + x_{16,4,19,10} + x_{17,4,19,17} + x_{18,4,19,18} + x_{36,4,19,5} = \\
& = x_{19,2,27,4} + x_{19,3,28,4} + x_{19,20,20,4} + x_{19,21,21,4} + x_{19,23,22,4} + x_{19,30,23,4} + x_{19,31,24,4} + x_{19,32,25,4} + x_{19,33,26,4} \quad (456)
\end{aligned}$$

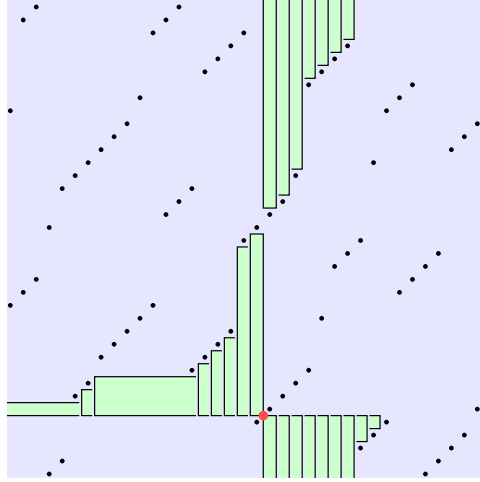

$$x_{36,4,19,5} = x_{19,5,20,19} \quad (457)$$

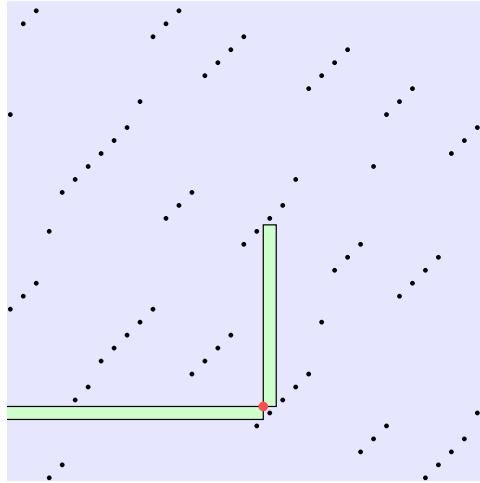

$$x_{5,4,19,6} = x_{19,6,21,19} \quad (458)$$

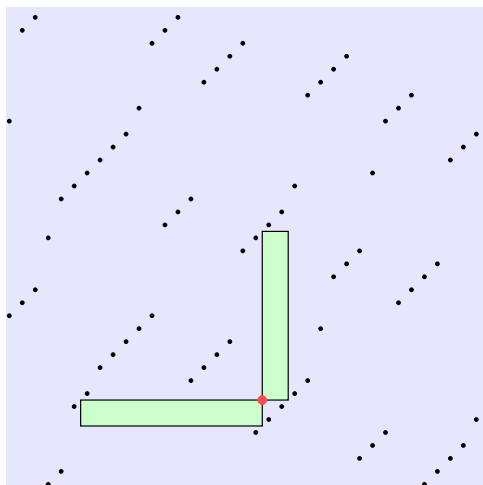

$$x_{6,4,19,7} = x_{19,7,22,19}$$

(459)

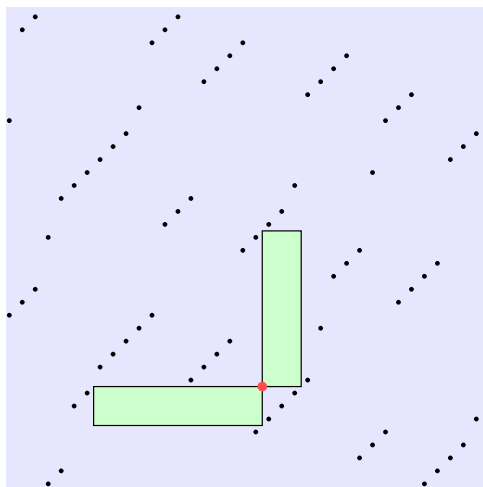

$$x_{14,4,19,8} = x_{19,8,23,19}$$

(460)

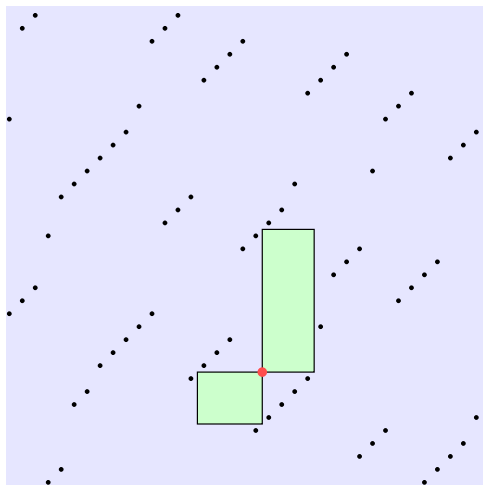

$$x_{15,4,19,9} = 0 \tag{461}$$

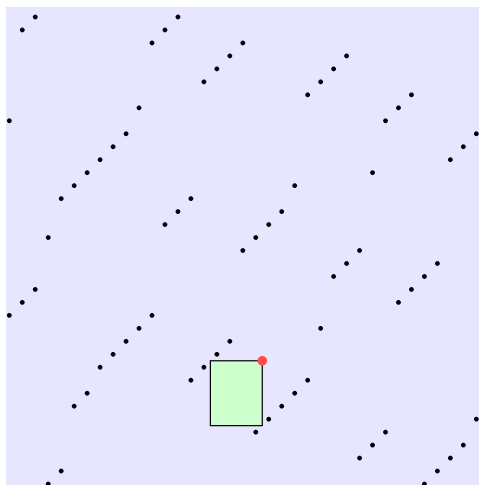

$$x_{16,4,19,10} = 0 \tag{462}$$

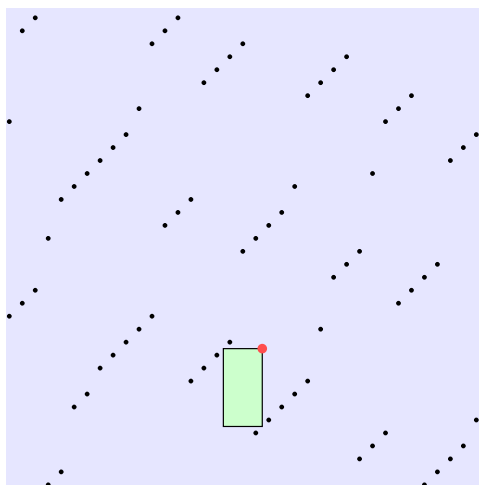

$$0 = x_{19,12,24,19} \tag{463}$$

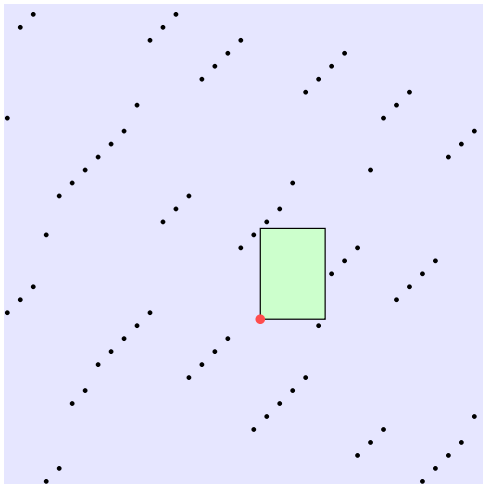

$$0 = x_{19,16,25,19}$$

(464)

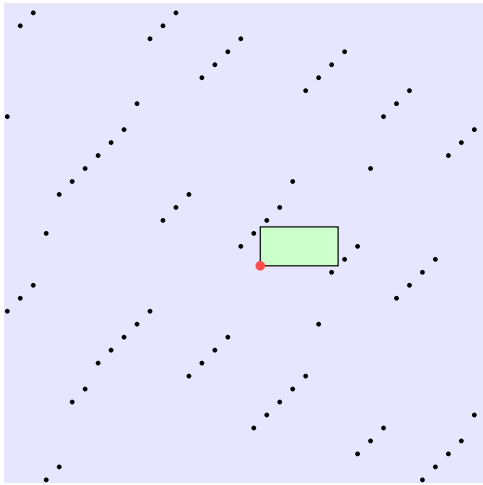

$$x_{17,4,19,17} = x_{19,17,26,19}$$

(465)

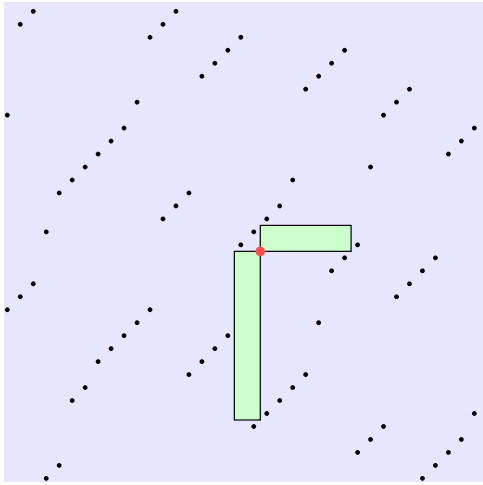

$$x_{18,4,19,18} = x_{19,18,2,19} \quad (466)$$

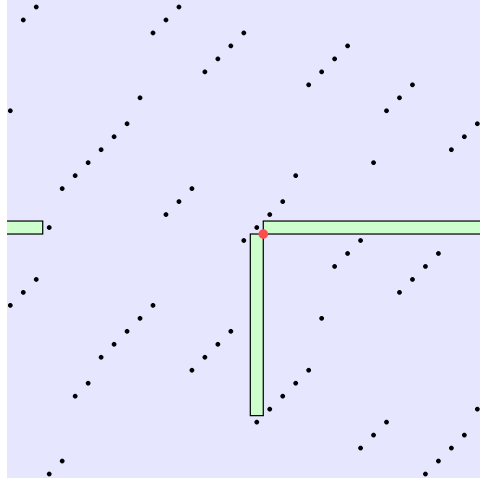

$$\begin{aligned} & x_{12,19,19,20} + x_{13,19,19,21} + x_{14,19,19,30} + x_{15,19,19,31} + x_{16,19,19,32} + x_{17,19,19,33} + x_{18,19,19,3} = \\ & = x_{19,5,20,19} + x_{19,6,21,19} + x_{19,7,22,19} + x_{19,8,23,19} + x_{19,12,24,19} + x_{19,16,25,19} + x_{19,17,26,19} + x_{19,18,2,19} \end{aligned} \quad (467)$$

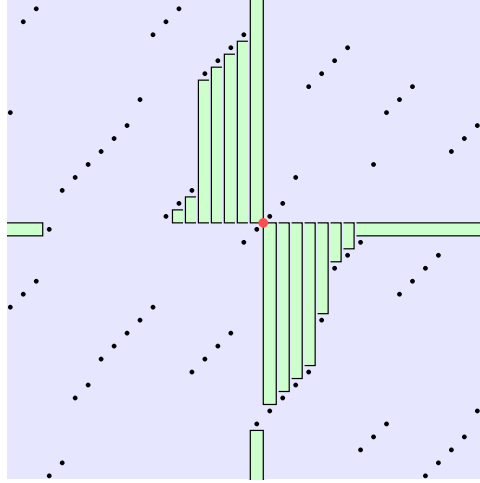

$$x_{12,19,19,20} = x_{19,20,20,4} \quad (468)$$

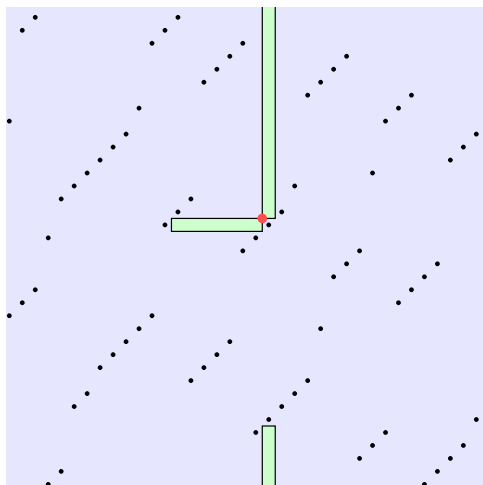

$$x_{13,19,19,21} = x_{19,21,21,4}$$

(469)

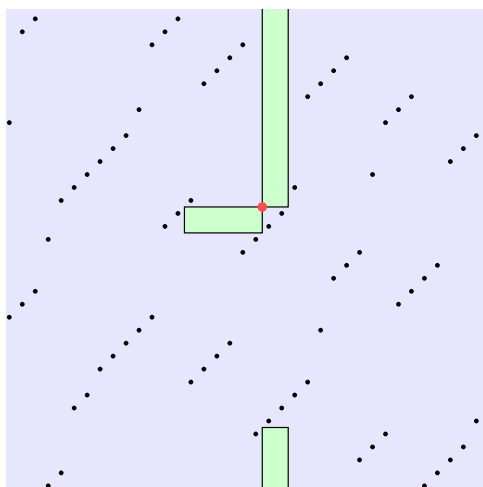

$$0 = x_{19,23,22,4}$$

(470)

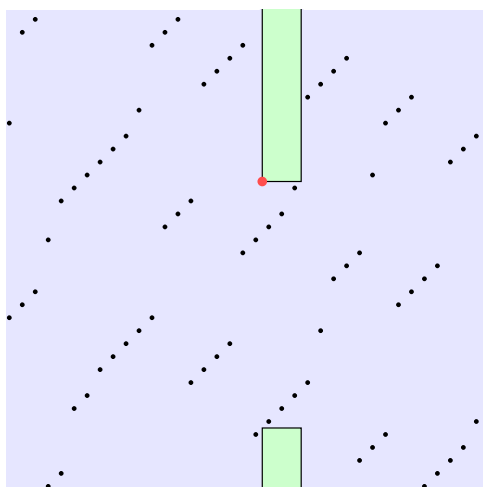



$$x_{14,19,19,30} = x_{19,30,23,4} \tag{471}$$

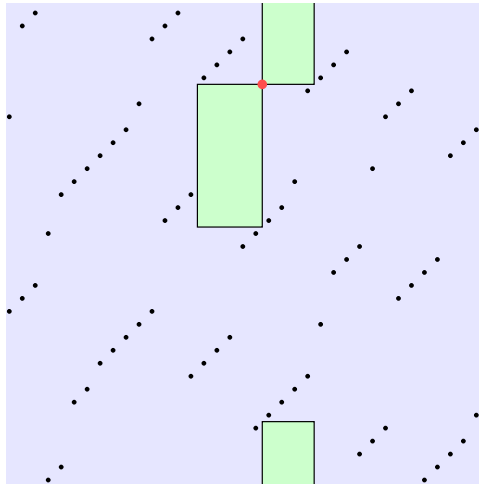

$$x_{15,19,19,31} = x_{19,31,24,4} \tag{472}$$

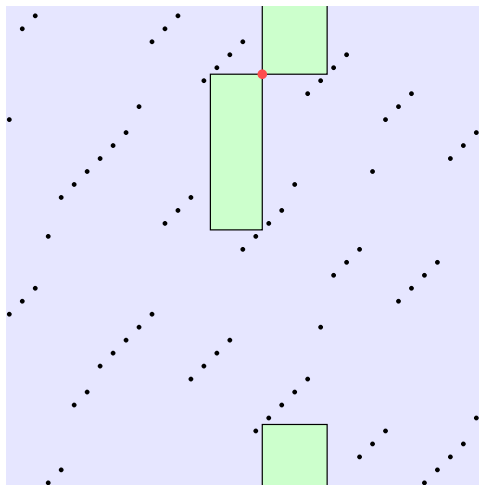

$$x_{16,19,19,32} = x_{19,32,25,4} \tag{473}$$

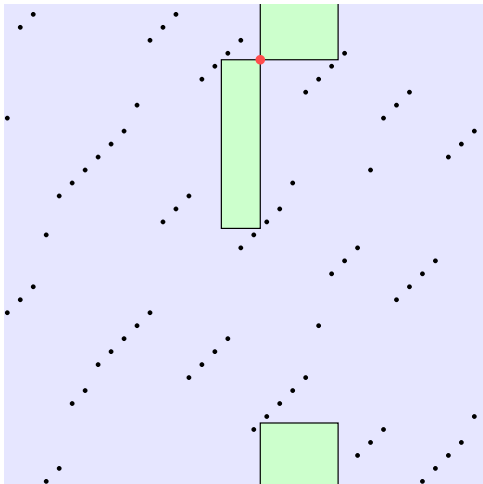

$$x_{17,19,19,33} = x_{19,33,26,4}$$

(474)

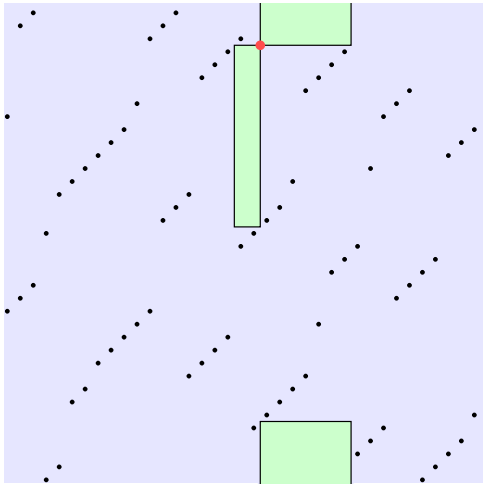

$$0 = x_{20,2,27,5}$$

(475)

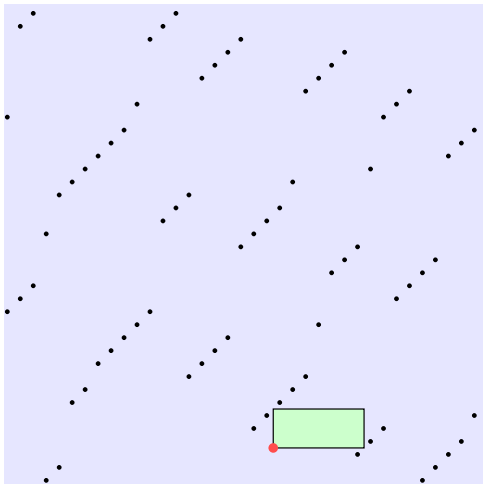

$$x_{18,20,20,3} = x_{20,3,28,5} \quad (476)$$

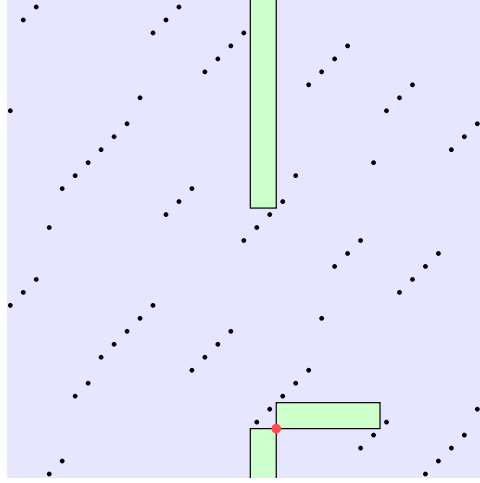

$$x_{19,20,20,4} = x_{20,4,35,5} \quad (477)$$

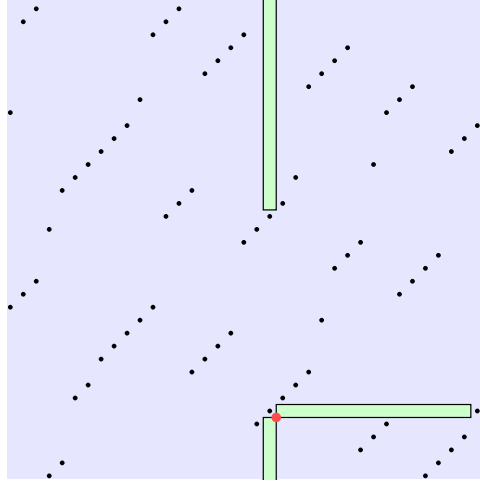

$$\begin{aligned} & x_{5,5,20,6} + x_{6,5,20,7} + x_{14,5,20,8} + x_{15,5,20,9} + x_{16,5,20,10} + x_{17,5,20,17} + x_{18,5,20,18} + x_{19,5,20,19} = \\ & = x_{20,2,27,5} + x_{20,3,28,5} + x_{20,4,35,5} + x_{20,21,21,5} + x_{20,23,22,5} + x_{20,30,23,5} + x_{20,31,24,5} + x_{20,32,25,5} + x_{20,33,26,5} \end{aligned} \quad (478)$$

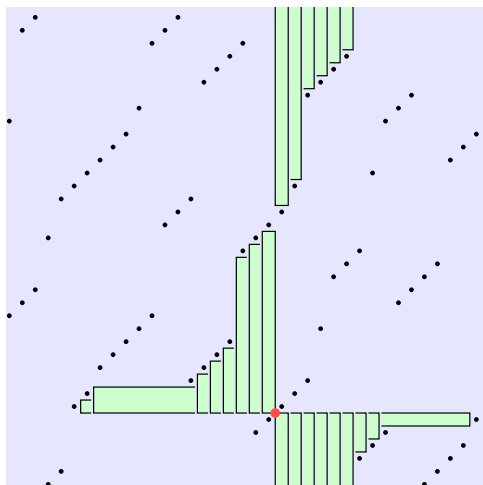

$$x_{5,5,20,6} = x_{20,6,21,20}$$

(479)

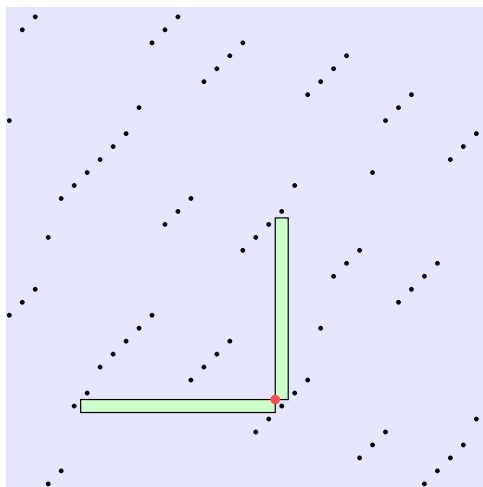

$$x_{6,5,20,7} = x_{20,7,22,20}$$

(480)

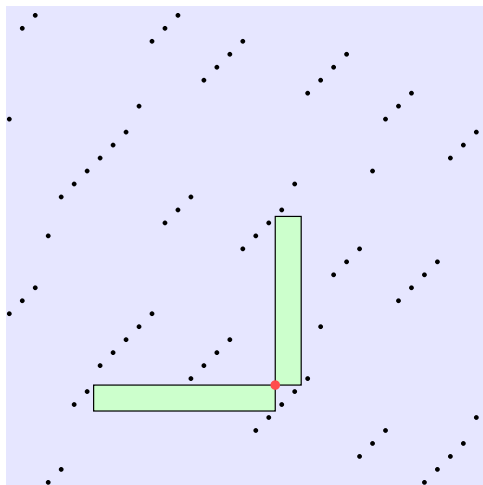

$$x_{14,5,20,8} = x_{20,8,23,20} \tag{481}$$

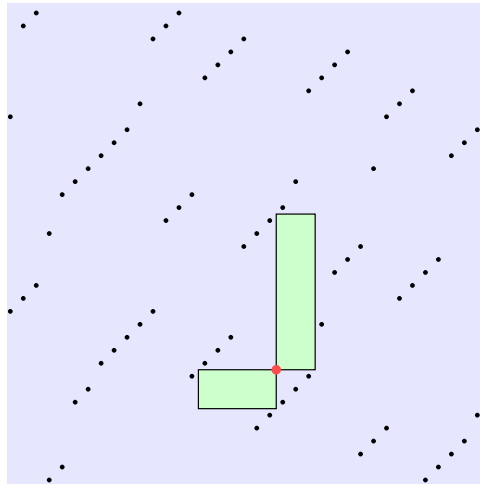

$$x_{15,5,20,9} = 0 \tag{482}$$

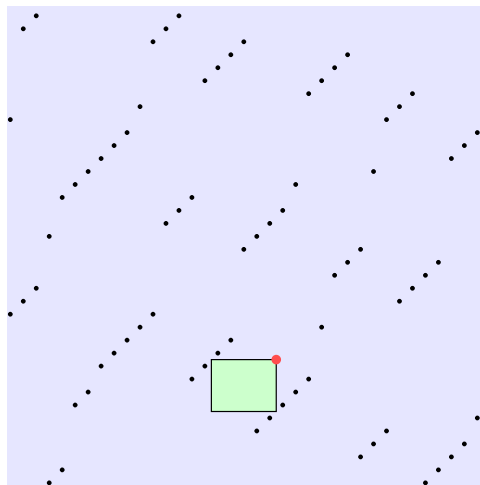

$$x_{16,5,20,10} = 0 \tag{483}$$

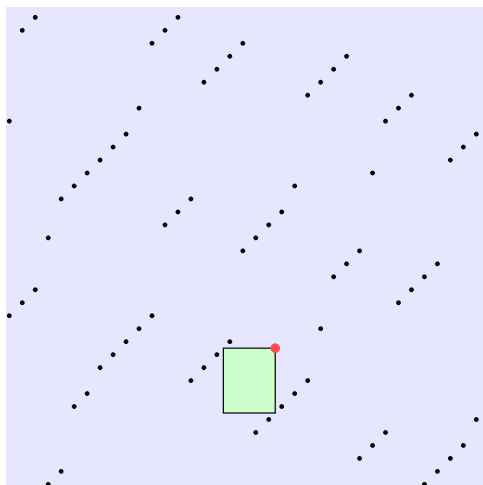

$$0 = x_{20,12,24,20}$$

(484)

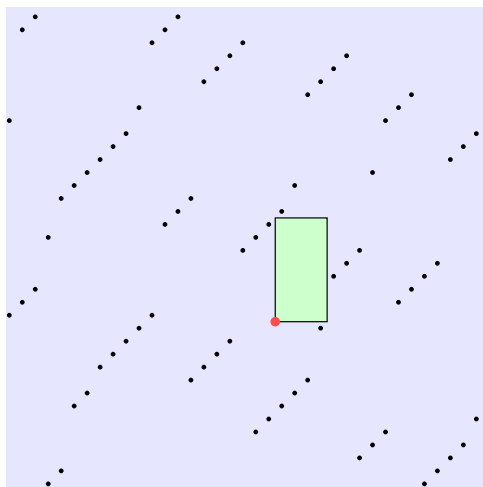

$$0 = x_{20,16,25,20}$$

(485)

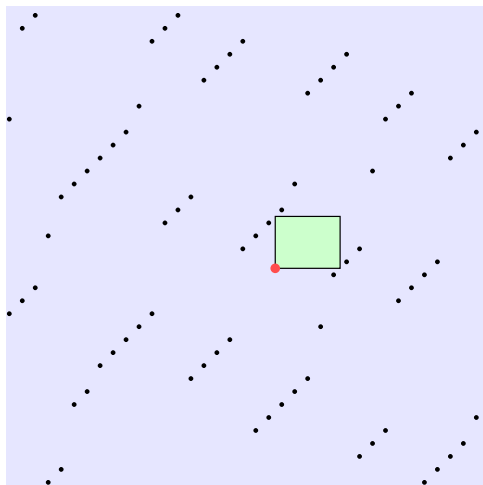

$$x_{17,5,20,17} = x_{20,17,26,20} \tag{486}$$

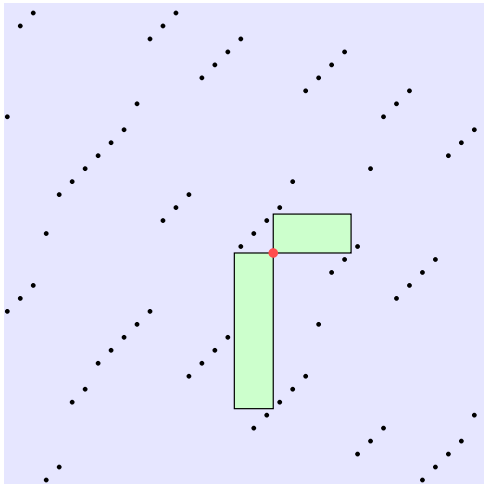

$$x_{18,5,20,18} = x_{20,18,2,20} \tag{487}$$

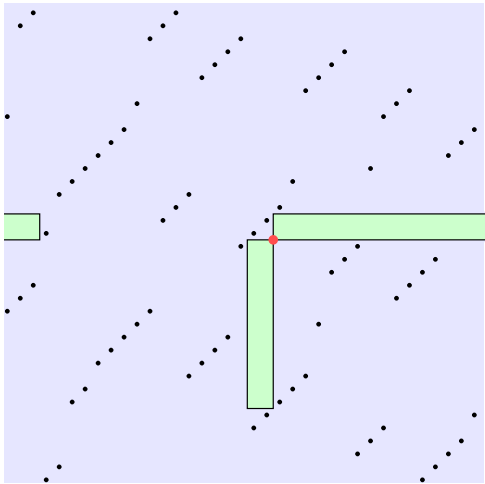

$$x_{19,5,20,19} = x_{20,19,11,20} \tag{488}$$

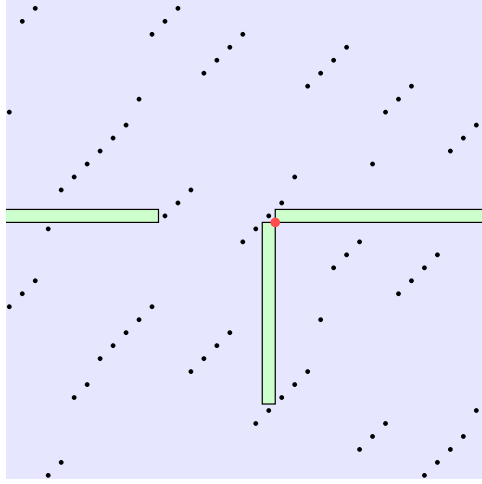

$$\begin{aligned}
 & x_{13,20,20,21} + x_{14,20,20,30} + x_{15,20,20,31} + x_{16,20,20,32} + x_{17,20,20,33} + x_{18,20,20,3} + x_{19,20,20,4} = \\
 & = x_{20,6,21,20} + x_{20,7,22,20} + x_{20,8,23,20} + x_{20,12,24,20} + x_{20,16,25,20} + x_{20,17,26,20} + x_{20,18,2,20} + x_{20,19,11,20} \quad (489)
 \end{aligned}$$

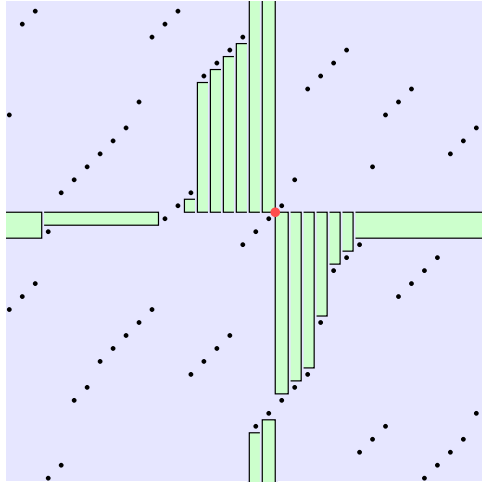

$$x_{13,20,20,21} = x_{20,21,21,5} \quad (490)$$



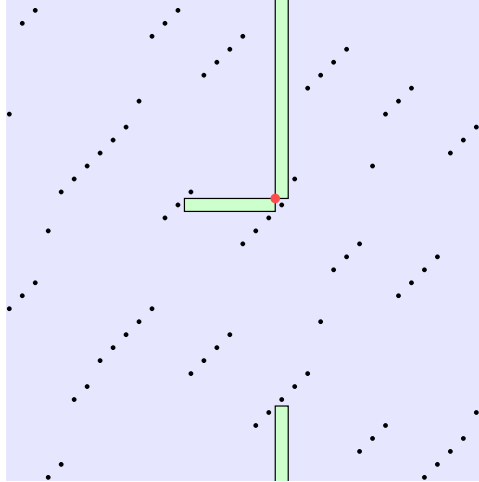

$$0 = x_{20,23,22,5}$$

(491)

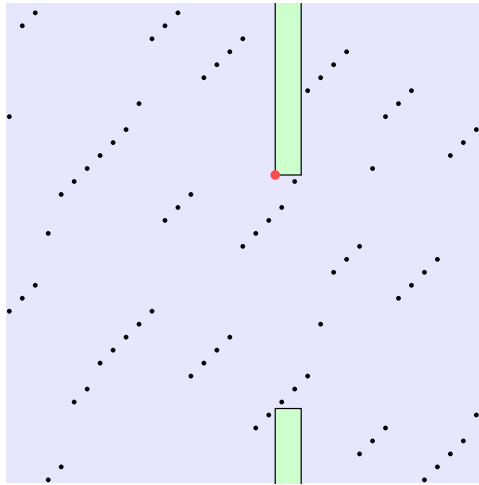

$$x_{14,20,20,30} = x_{20,30,23,5}$$

(492)

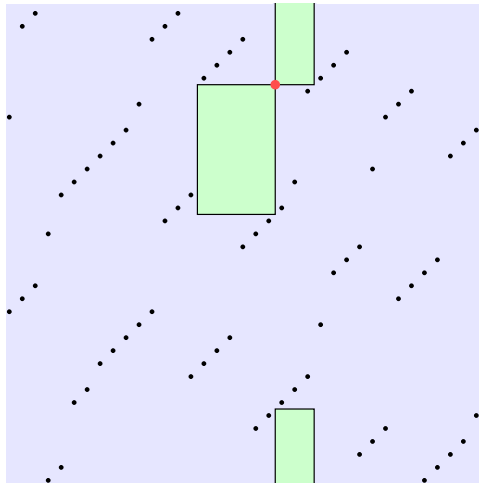

$$x_{15,20,20,31} = x_{20,31,24,5} \tag{493}$$

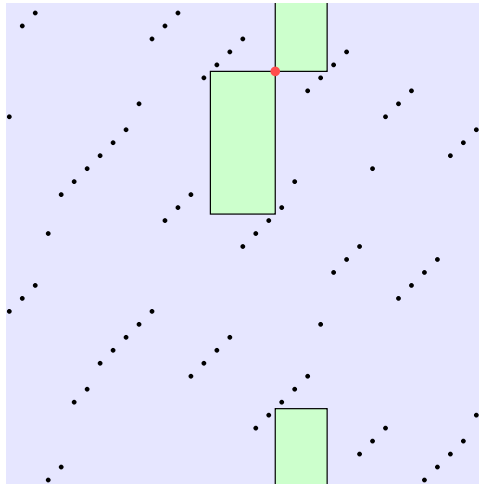

$$x_{16,20,20,32} = x_{20,32,25,5} \tag{494}$$

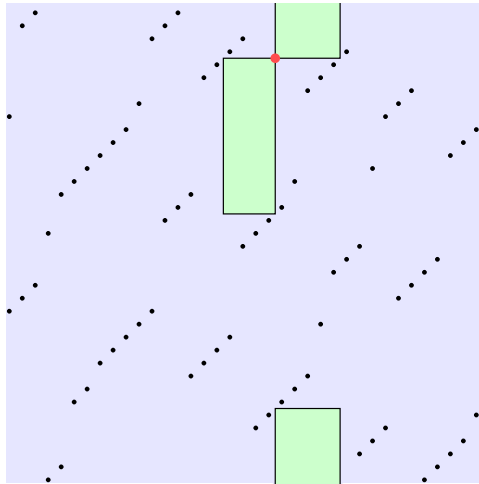

$$x_{17,20,20,33} = x_{20,33,26,5} \tag{495}$$

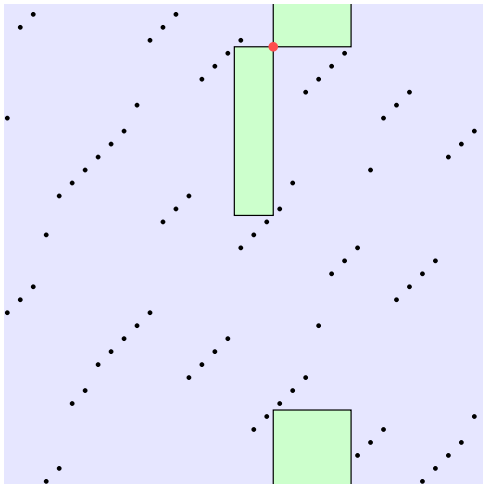

$$0 = x_{21,2,27,6}$$

(496)

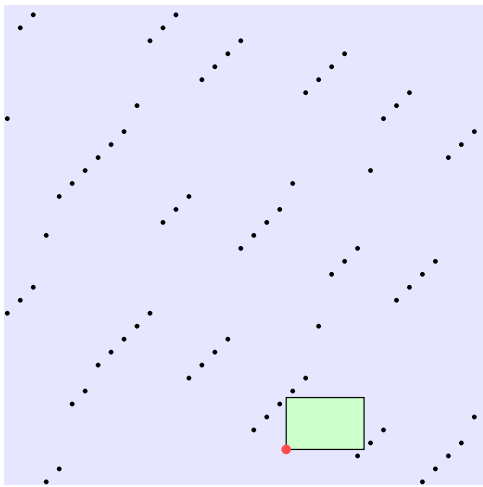

$$x_{18,21,21,3} = x_{21,3,28,6}$$

(497)

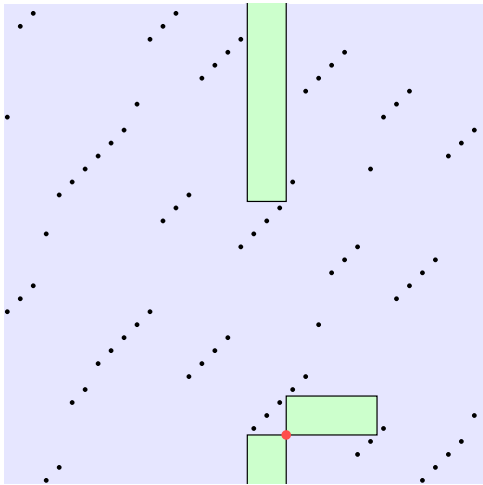

$$x_{19,21,21,4} = x_{21,4,35,6} \quad (498)$$

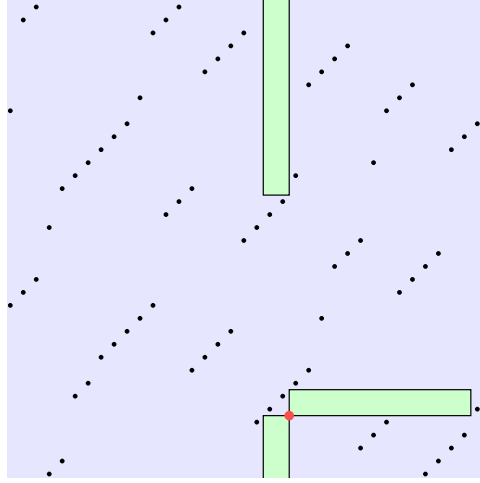

$$x_{20,21,21,5} = x_{21,5,4,6} \quad (499)$$

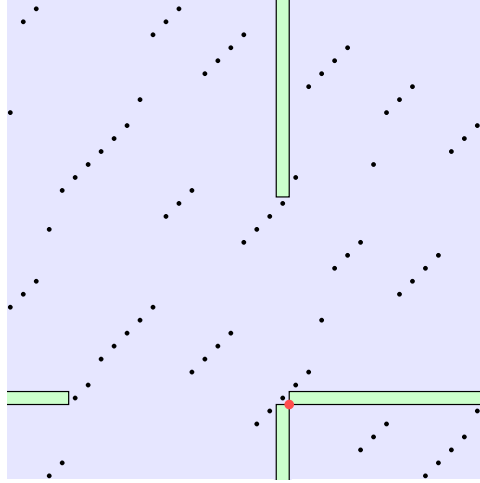

$$\begin{aligned} & x_{6,6,21,7} + x_{14,6,21,8} + x_{15,6,21,9} + x_{16,6,21,10} + x_{17,6,21,17} + x_{18,6,21,18} + x_{19,6,21,19} + x_{20,6,21,20} = \\ & = x_{21,2,27,6} + x_{21,3,28,6} + x_{21,4,35,6} + x_{21,5,4,6} + x_{21,23,22,6} + x_{21,30,23,6} + x_{21,31,24,6} + x_{21,32,25,6} + x_{21,33,26,6} \end{aligned} \quad (500)$$

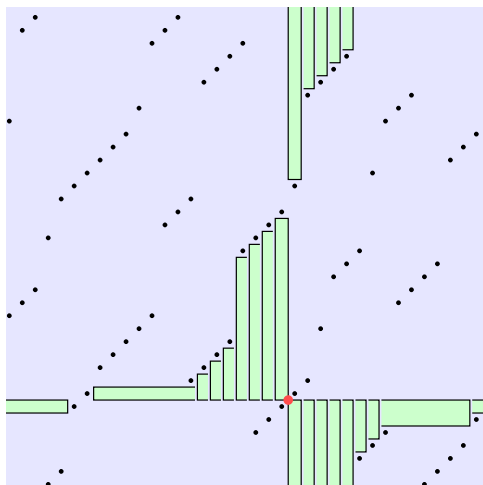

$$x_{6,6,21,7} = x_{21,7,22,22}$$

(501)

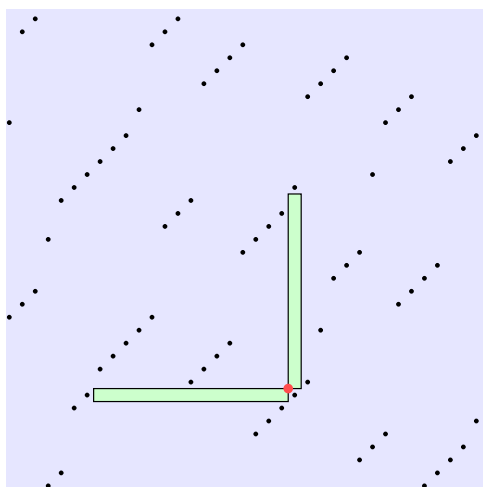

$$x_{14,6,21,8} = x_{21,8,23,22}$$

(502)

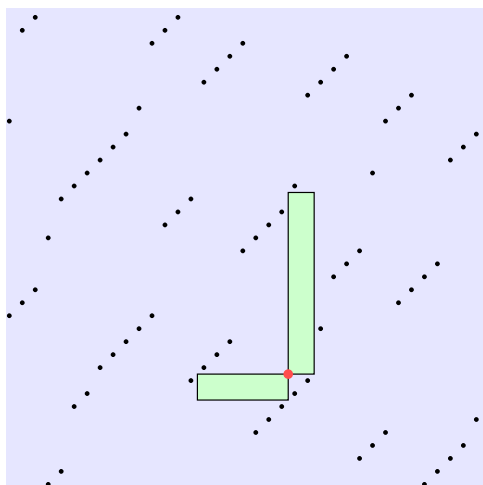

$$x_{15,6,21,9} = 0 \tag{503}$$

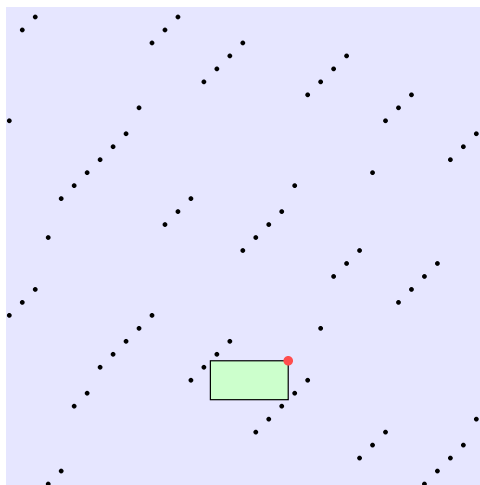

$$x_{16,6,21,10} = 0 \tag{504}$$

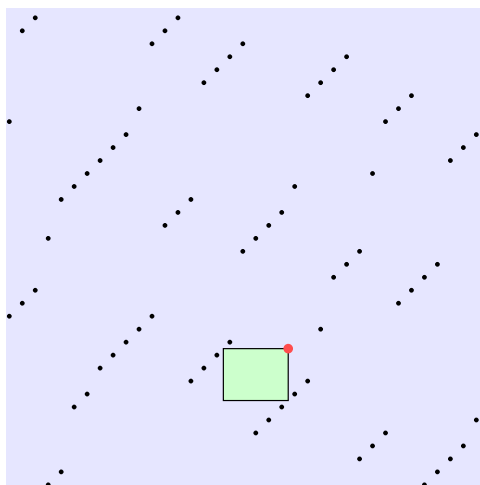

$$0 = x_{21,12,24,22} \tag{505}$$

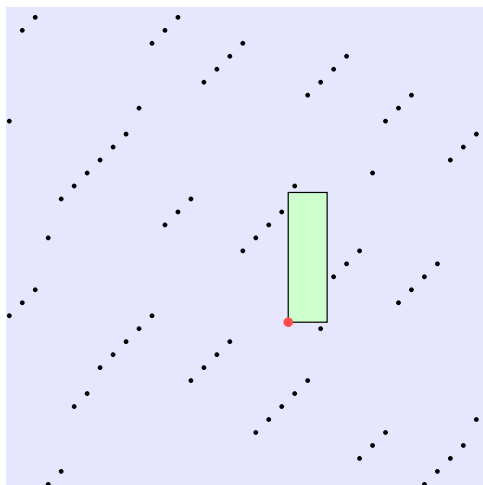

$$0 = x_{21,16,25,22}$$

(506)

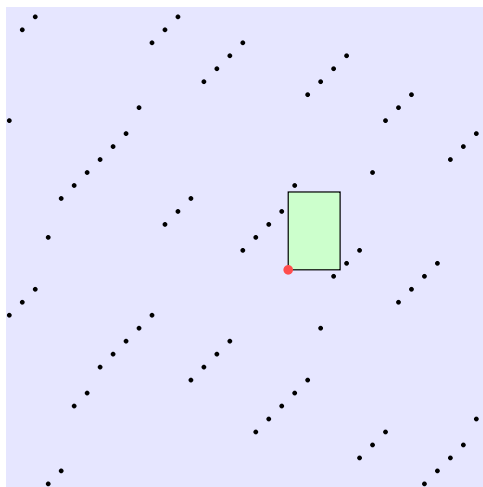

$$x_{17,6,21,17} = x_{21,17,26,22}$$

(507)

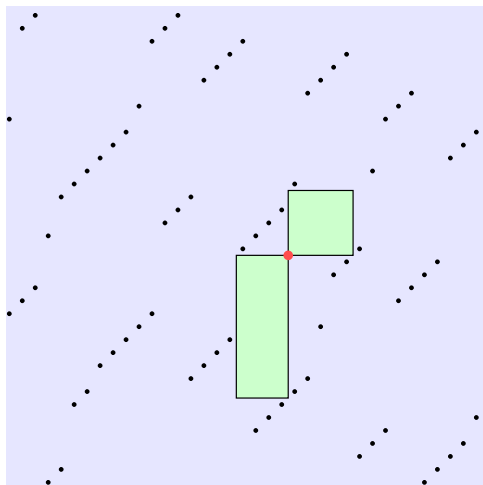

$$x_{18,6,21,18} = x_{21,18,2,22} \quad (508)$$

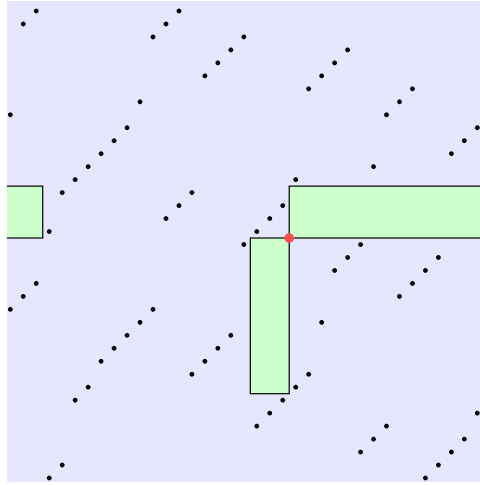

$$x_{19,6,21,19} = x_{21,19,3,22} + x_{21,19,11,21} \quad (509)$$

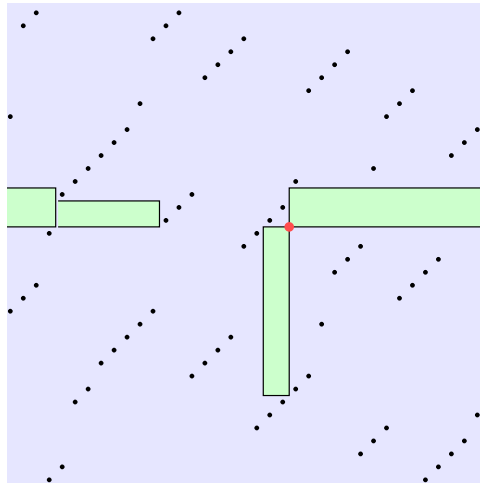

$$x_{20,6,21,20} = x_{21,20,12,21} \quad (510)$$



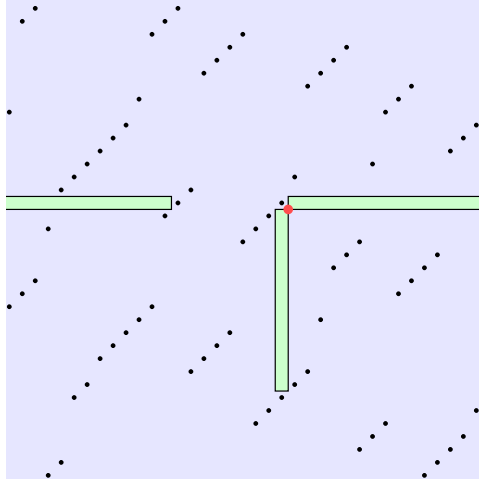

$$x_{14,21,21,30} + x_{15,21,21,31} + x_{16,21,21,32} + x_{17,21,21,33} + x_{18,21,21,3} + x_{19,21,21,4} + x_{20,21,21,5} = x_{21,19,11,21} + x_{21,20,12,21} \quad (511)$$

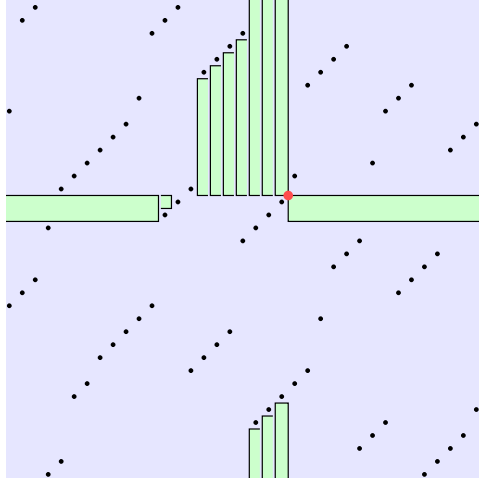

$$\begin{aligned} x_{5,22,21,23} + x_{6,22,21,24} + x_{7,22,21,25} + x_{8,22,21,26} + x_{9,22,21,28} + x_{10,22,21,30} = \\ = x_{21,7,22,22} + x_{21,8,23,22} + x_{21,12,24,22} + x_{21,16,25,22} + x_{21,17,26,22} + x_{21,18,2,22} + x_{21,19,3,22} \end{aligned} \quad (512)$$

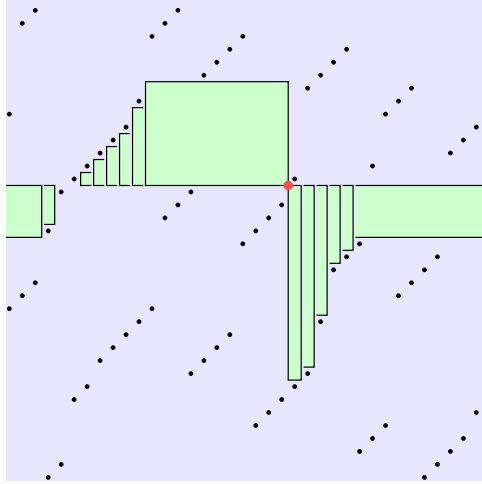

$$x_{5,22,21,23} = x_{21,23,22,6}$$

(513)

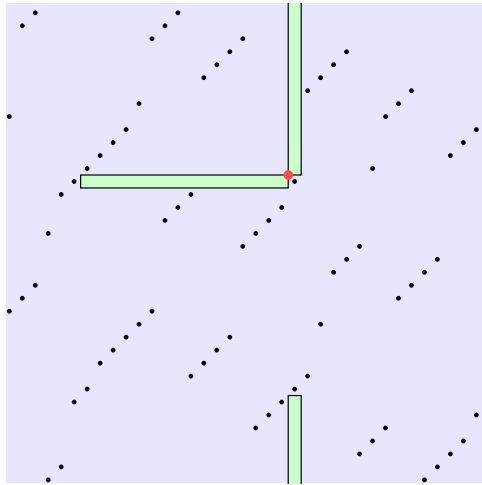

$$x_{6,22,21,24} = 0$$

(514)

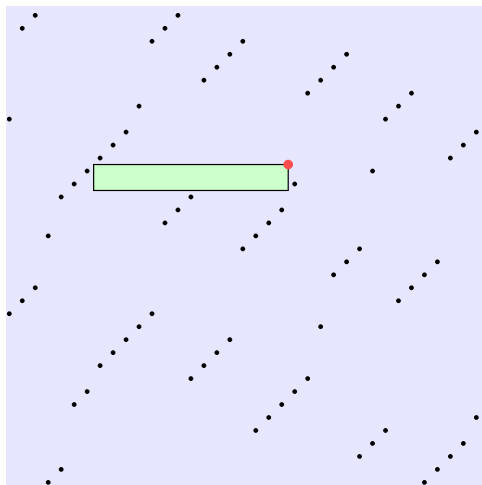

$$x_{7,22,21,25} = 0 \tag{515}$$

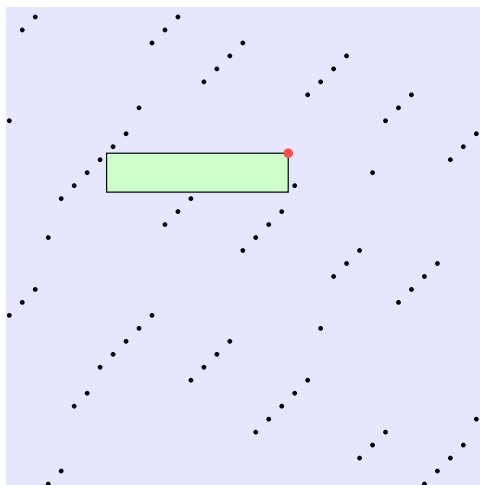

$$x_{8,22,21,26} = 0 \tag{516}$$

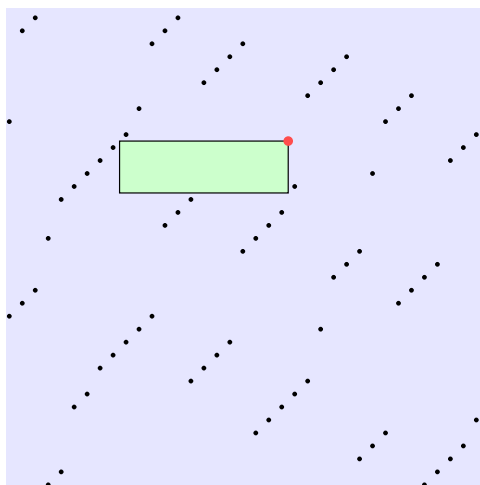

$$x_{9,22,21,28} = 0 \tag{517}$$

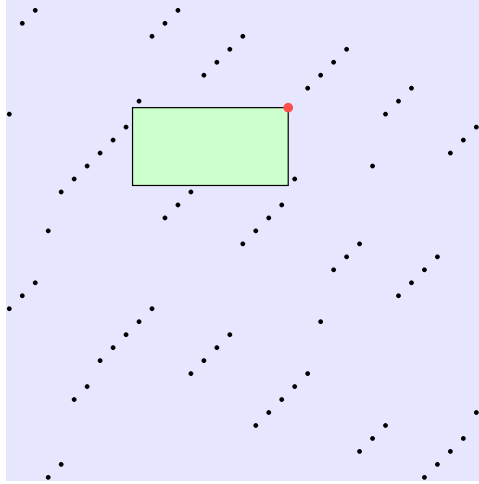

$$x_{10,22,21,30} + x_{14,21,21,30} = x_{21,30,23,6}$$

(518)

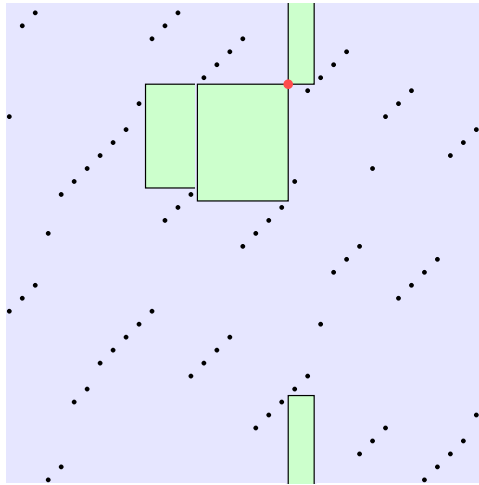

$$x_{15,21,21,31} = x_{21,31,24,6}$$

(519)

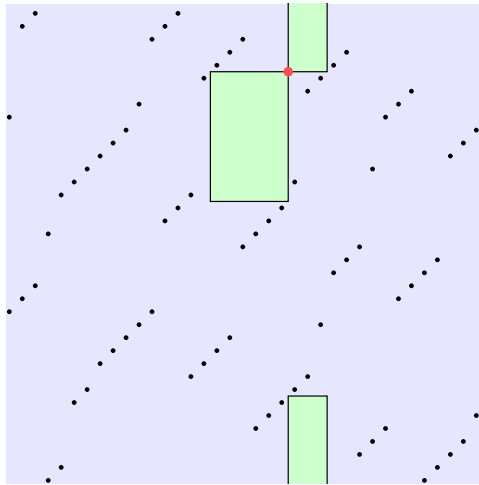

$$x_{16,21,21,32} = x_{21,32,25,6} \tag{520}$$

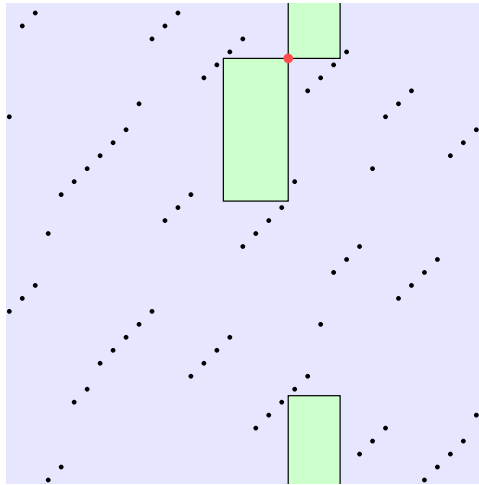

$$x_{17,21,21,33} = x_{21,33,26,6} \tag{521}$$

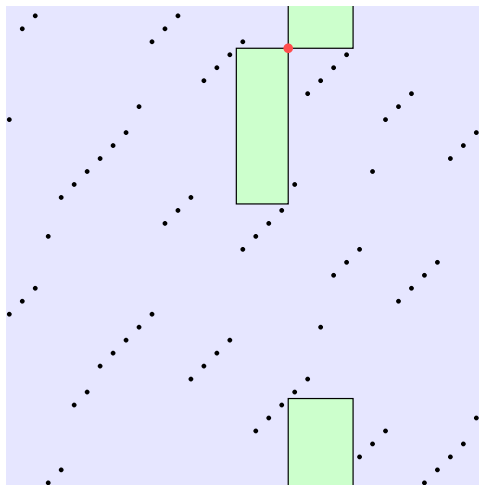

$$0 = x_{22,2,27,7} \tag{522}$$

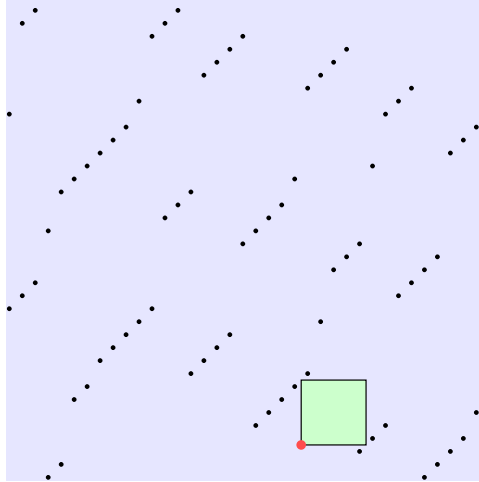

$$x_{18,23,22,3} = x_{22,3,28,7}$$

(523)

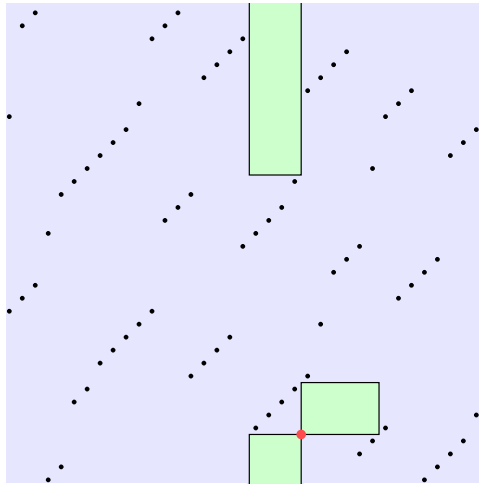

$$x_{19,23,22,4} = x_{22,4,35,7}$$

(524)

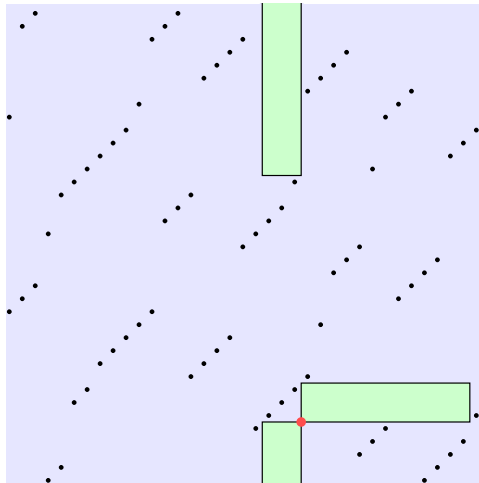

$$x_{20,23,22,5} = x_{22,5,4,7}$$

(525)

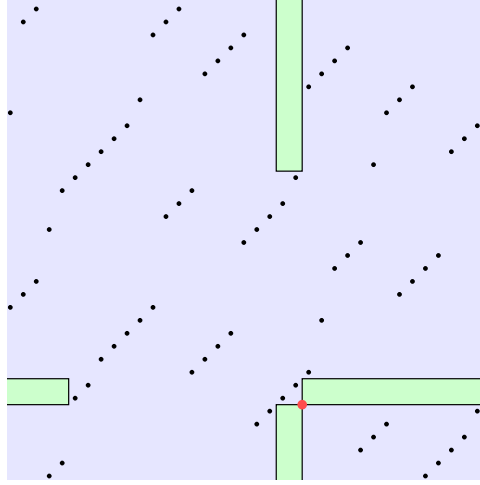

$$x_{21,23,22,6} = x_{22,6,5,7}$$

(526)

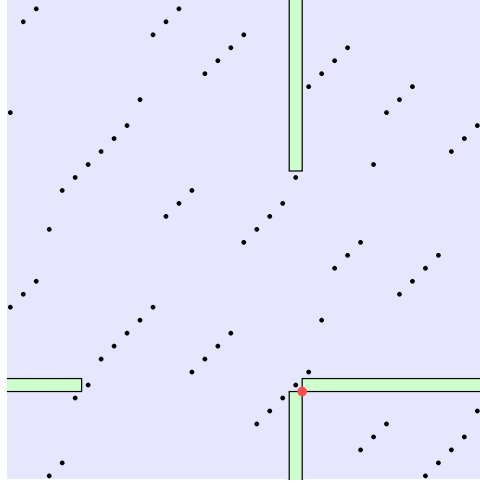

$$\begin{aligned} & x_{14,7,22,8} + x_{15,7,22,9} + x_{16,7,22,10} + x_{17,7,22,17} + x_{18,7,22,18} + x_{19,7,22,19} + x_{20,7,22,20} + x_{21,7,22,22} = \\ & = x_{22,2,27,7} + x_{22,3,28,7} + x_{22,4,35,7} + x_{22,5,4,7} + x_{22,6,5,7} + x_{22,30,23,7} + x_{22,31,24,7} + x_{22,32,25,7} + x_{22,33,26,7} \end{aligned} \quad (527)$$

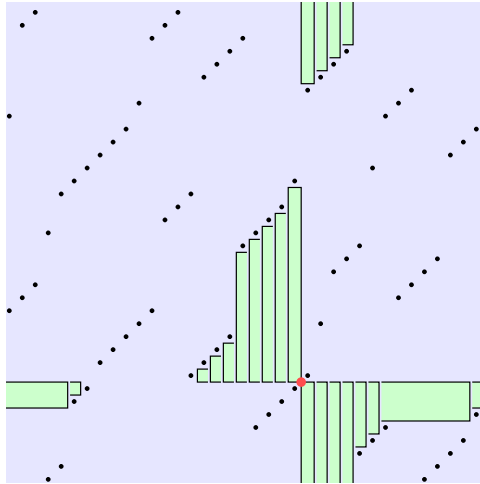

$$x_{14,7,22,8} = x_{22,8,23,29}$$

(528)

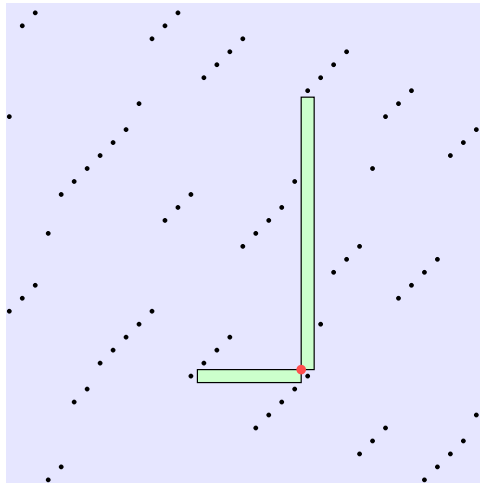

$$x_{15,7,22,9} = 0$$

(529)

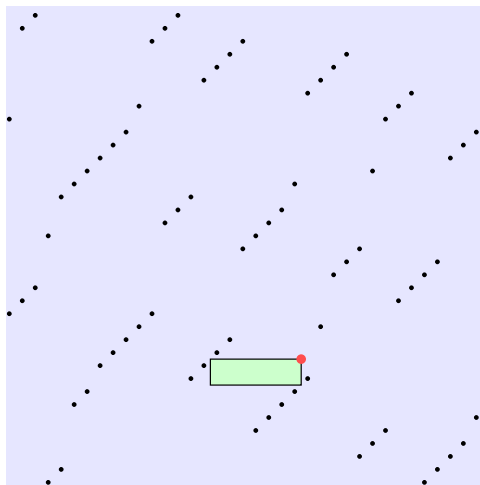



$$x_{16,7,22,10} = 0 \tag{530}$$

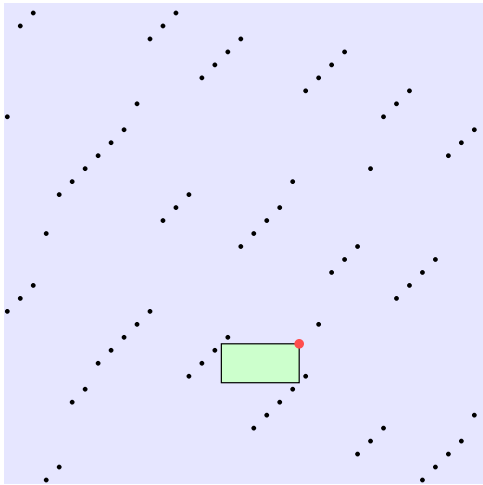

$$0 = x_{22,12,24,29} \tag{531}$$

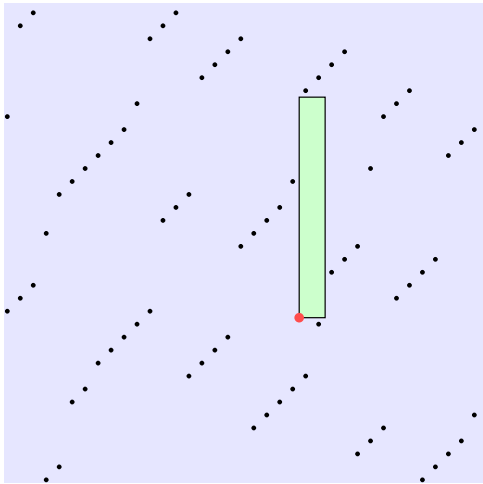

$$0 = x_{22,16,25,29} \tag{532}$$

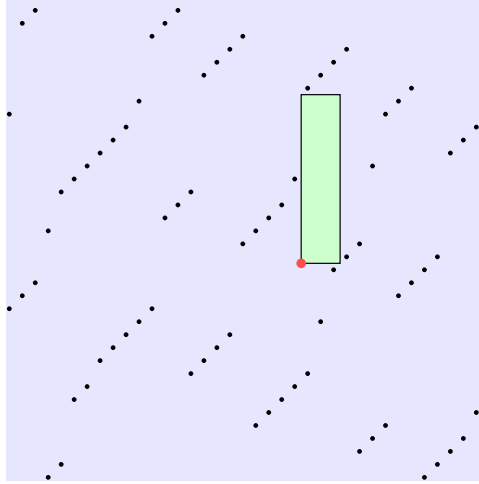

$$x_{17,7,22,17} = x_{22,17,26,29}$$

(533)

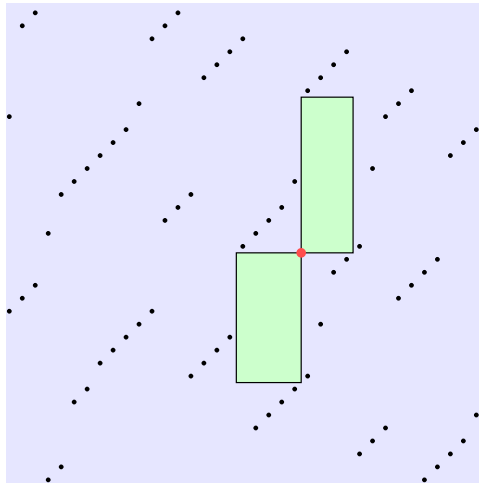

$$x_{18,7,22,18} = x_{22,18,2,23} + x_{22,18,27,29}$$

(534)

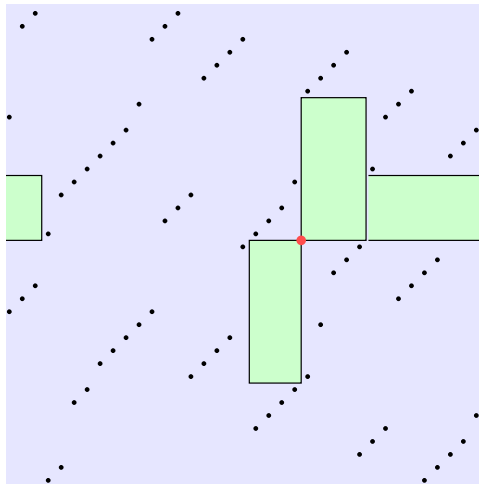

$$x_{19,7,22,19} = x_{22,19,3,23} \tag{535}$$

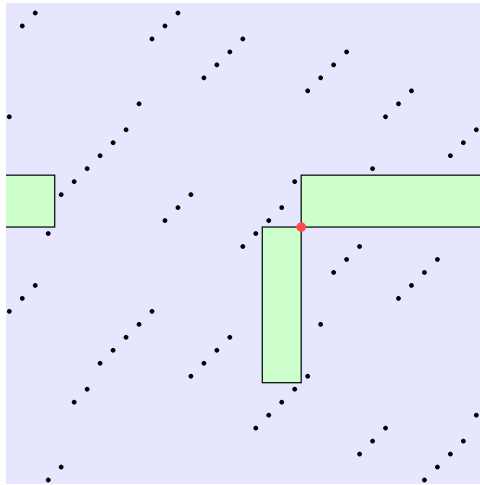

$$x_{20,7,22,20} = 0 \tag{536}$$

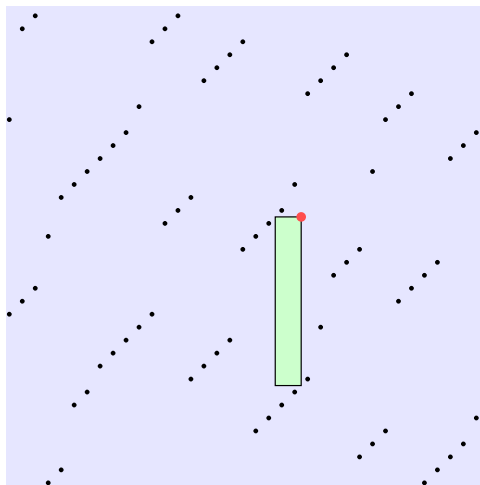

$$x_{21,7,22,22} = x_{22,22,4,23} \tag{537}$$

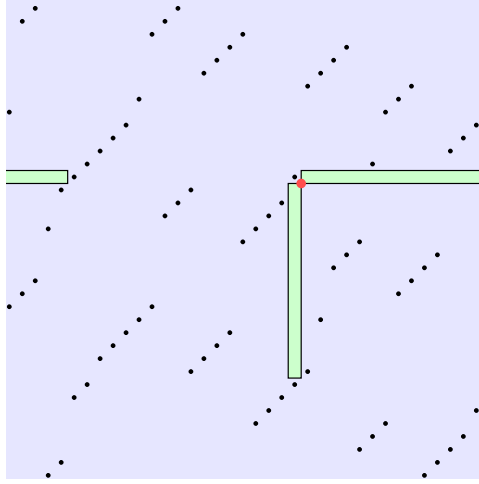

$$\begin{aligned}
 x_{10,23,22,30} + x_{15,23,22,31} + x_{16,23,22,32} + x_{17,23,22,33} + x_{18,23,22,3} + x_{19,23,22,4} + x_{20,23,22,5} + x_{21,23,22,6} = \\
 = x_{22,18,2,23} + x_{22,19,3,23} + x_{22,22,4,23} \quad (538)
 \end{aligned}$$

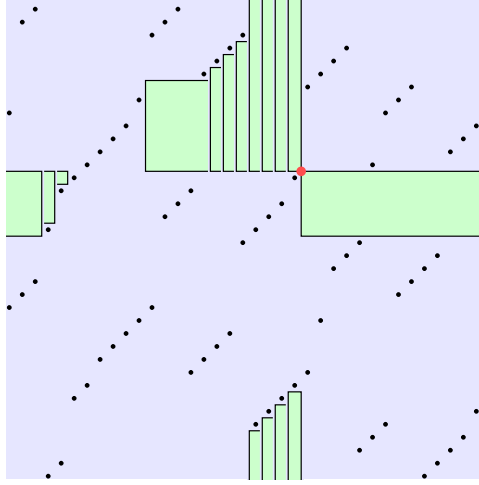

$$x_{31,29,22,30} = x_{22,8,23,29} + x_{22,12,24,29} + x_{22,16,25,29} + x_{22,17,26,29} + x_{22,18,27,29} \quad (539)$$

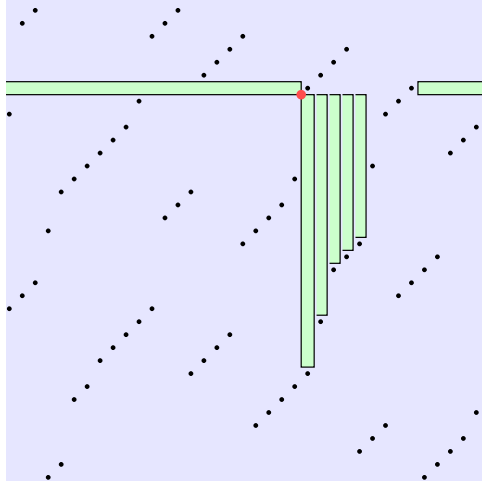

$$x_{10,23,22,30} + x_{31,29,22,30} = x_{22,30,23,7}$$

(540)

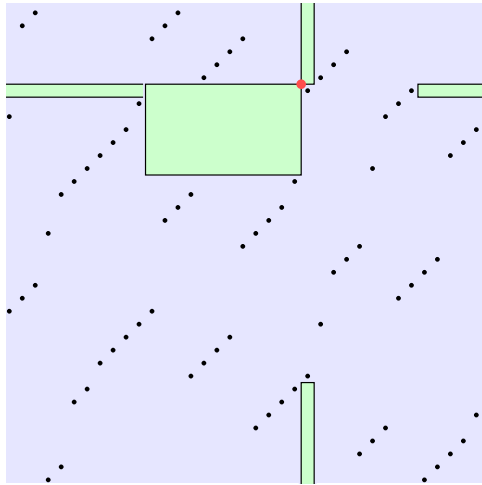

$$x_{15,23,22,31} = x_{22,31,24,7}$$

(541)

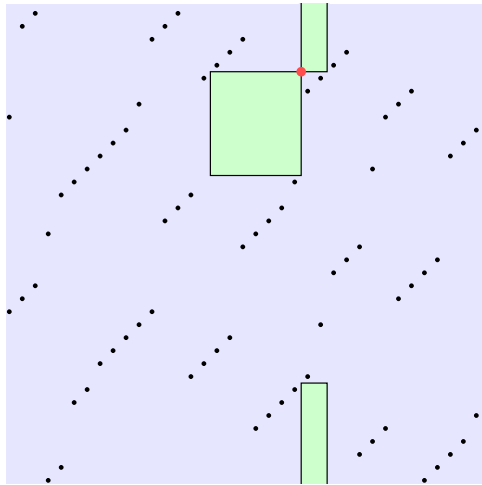

$$x_{16,23,22,32} = x_{22,32,25,7} \tag{542}$$

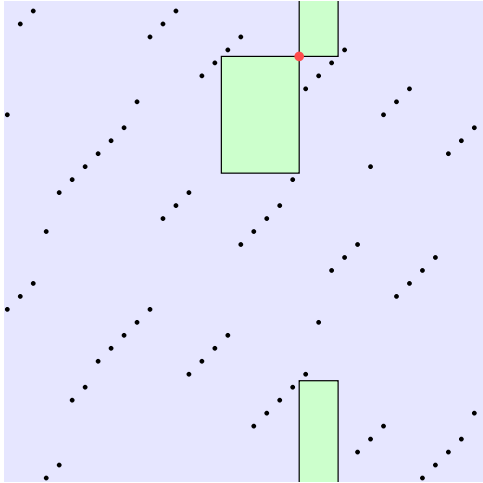

$$x_{17,23,22,33} = x_{22,33,26,7} \tag{543}$$

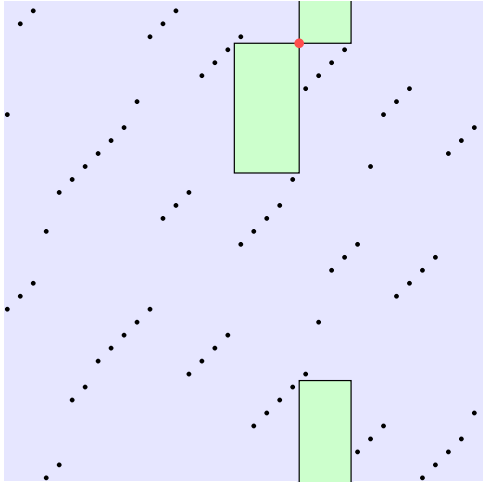

$$0 = x_{23,2,27,11} \tag{544}$$

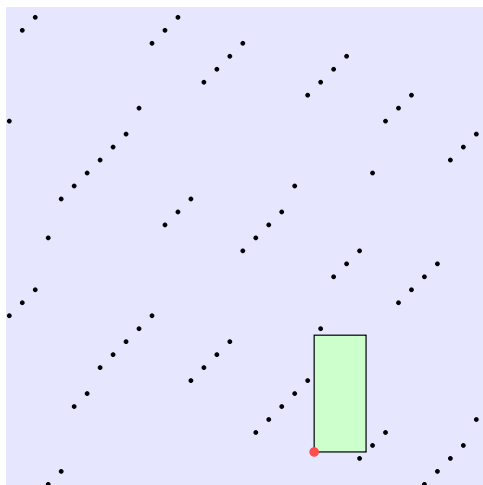

$$x_{18,30,23,3} = x_{23,3,28,11}$$

(545)

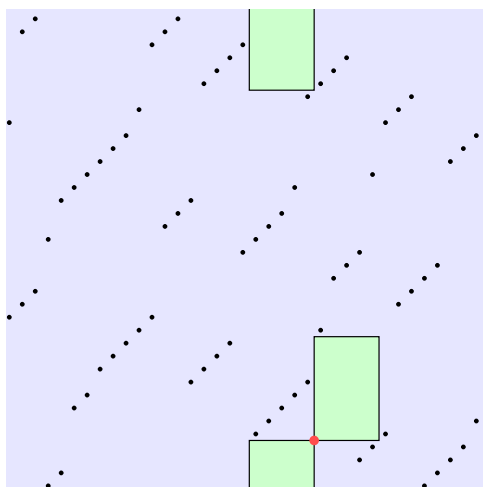

$$x_{19,30,23,4} = x_{23,4,35,11}$$

(546)

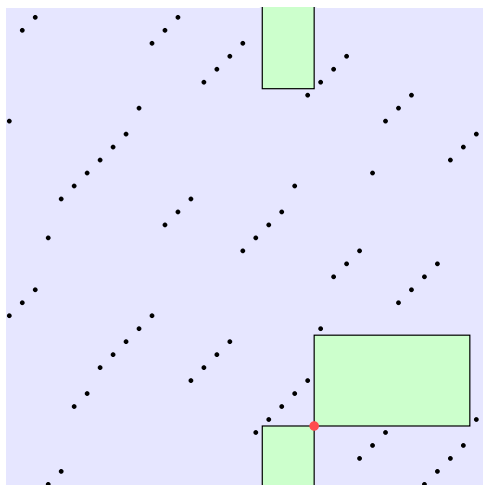

$$x_{20,30,23,5} = x_{23,5,4,11} \tag{547}$$

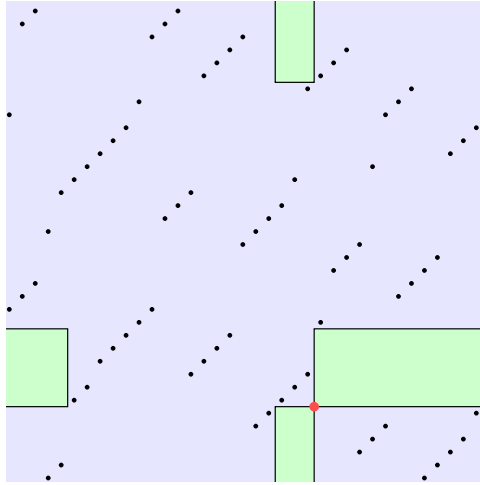

$$x_{21,30,23,6} = x_{23,6,5,11} \tag{548}$$

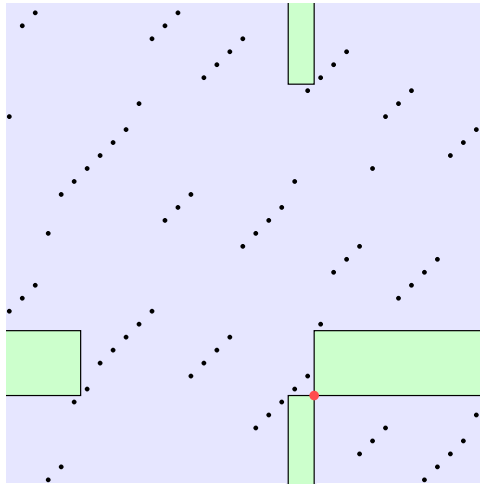

$$x_{22,30,23,7} = x_{23,7,6,11} + x_{23,7,13,8} \tag{549}$$



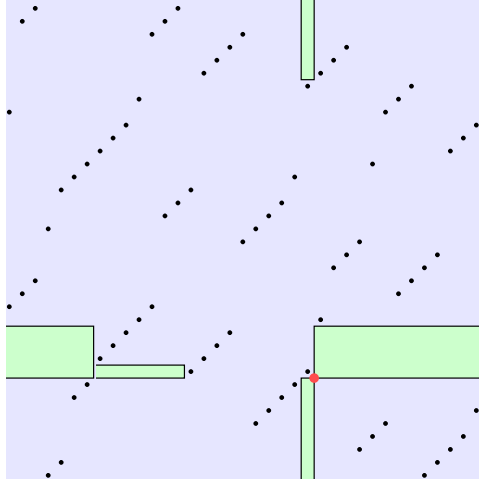

$$x_{17,8,23,17} + x_{18,8,23,18} + x_{19,8,23,19} + x_{20,8,23,20} + x_{21,8,23,22} + x_{22,8,23,29} = x_{23,7,13,8} \quad (550)$$

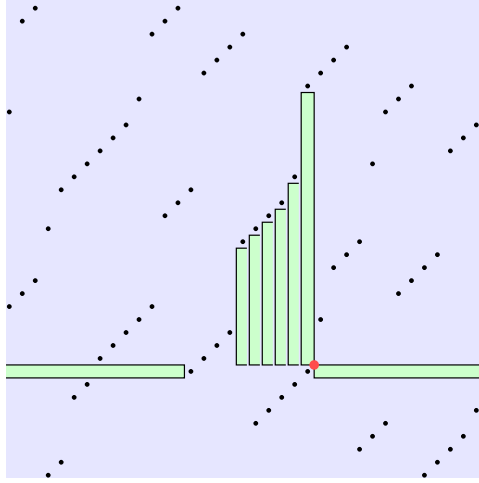

$$\begin{aligned} x_{10,11,23,12} + x_{11,11,23,17} = \\ = x_{23,2,27,11} + x_{23,3,28,11} + x_{23,4,35,11} + x_{23,5,4,11} + x_{23,6,5,11} + x_{23,7,6,11} + x_{23,31,24,11} + x_{23,32,25,11} + x_{23,33,26,11} \end{aligned} \quad (551)$$

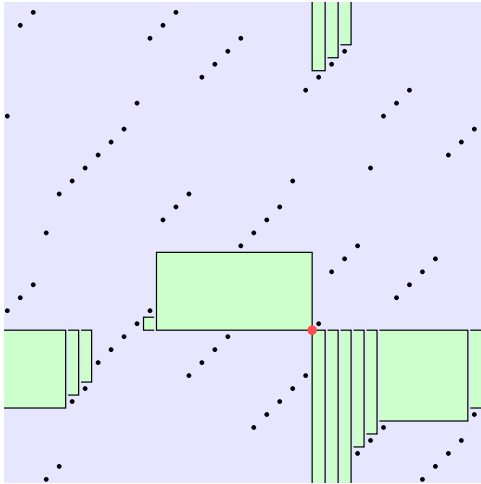

$$x_{10,11,23,12} = x_{23,12,24,30}$$

(552)

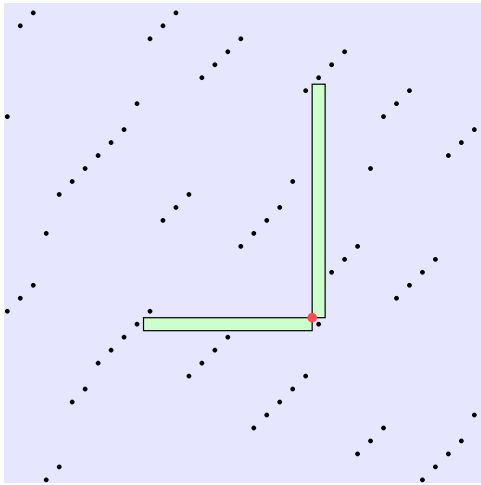

$$0 = x_{23,16,25,30}$$

(553)

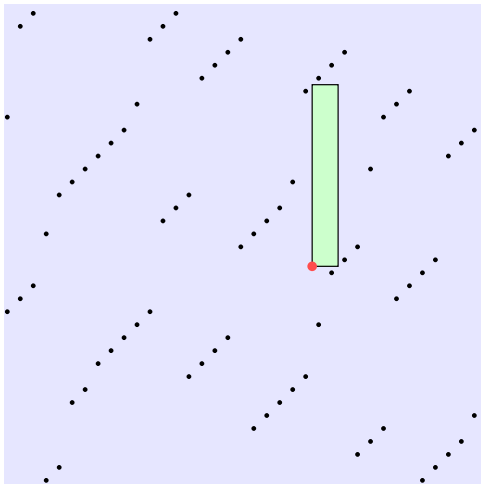

$$x_{11,11,23,17} + x_{17,8,23,17} = x_{23,17,26,30} \quad (554)$$

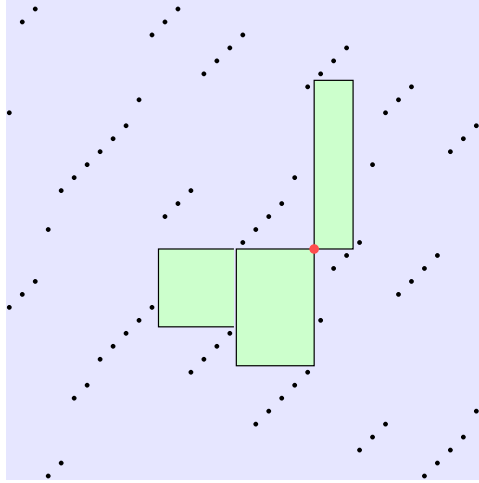

$$x_{18,8,23,18} = x_{23,18,27,30} \quad (555)$$

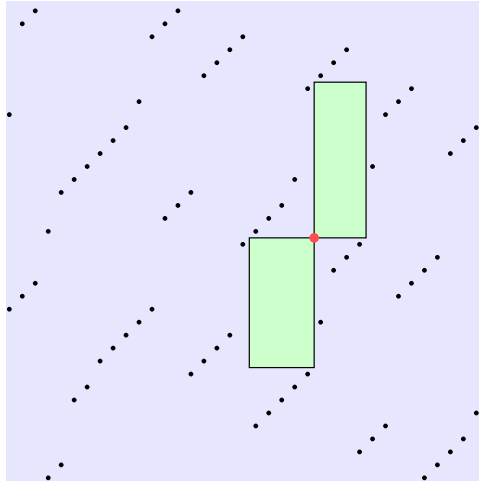

$$x_{19,8,23,19} = 0 \quad (556)$$

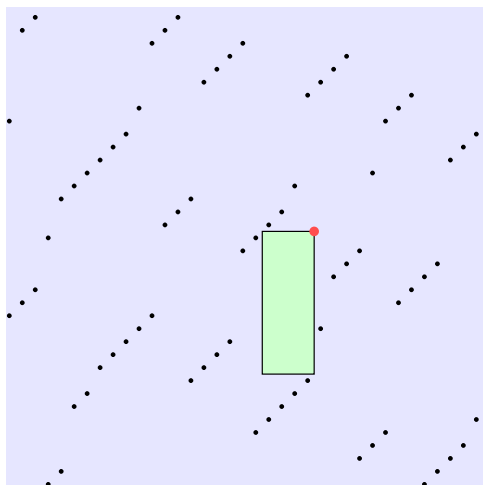

$$x_{20,8,23,20} = 0$$

(557)

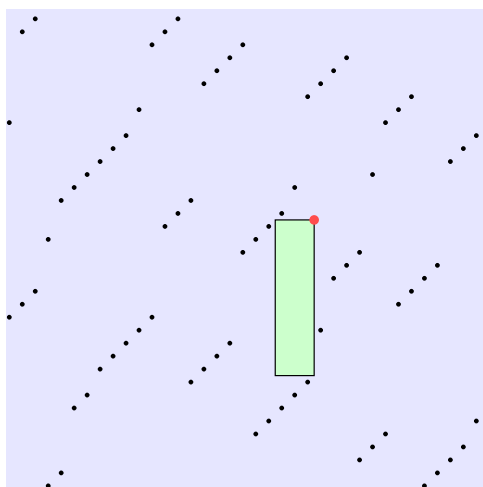

$$x_{21,8,23,22} = 0$$

(558)

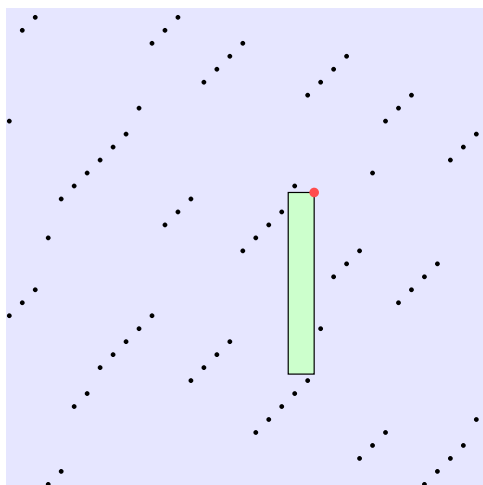

$$0 = x_{23,24,28,30} \tag{559}$$

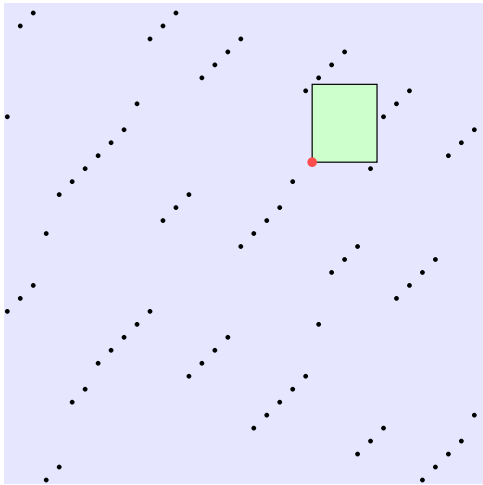

$$0 = x_{23,28,29,30} \tag{560}$$

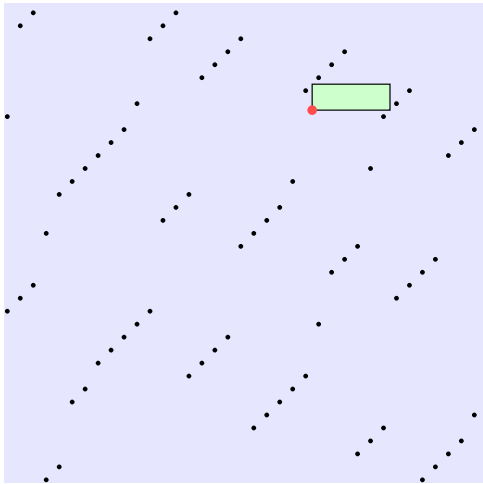

$$x_{22,8,23,29} = x_{23,29,30,30} \tag{561}$$

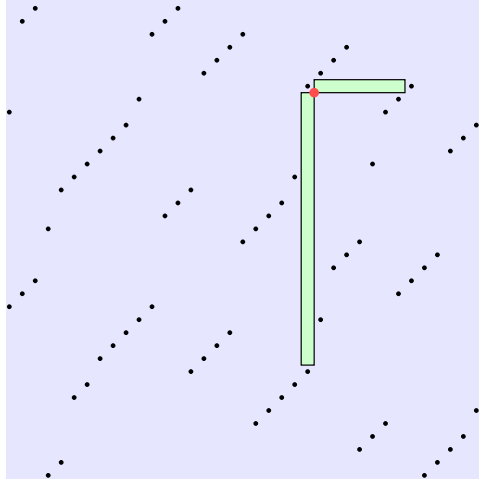

$$\begin{aligned}
 & x_{15,30,23,31} + x_{16,30,23,32} + x_{17,30,23,33} + x_{18,30,23,3} + x_{19,30,23,4} + x_{20,30,23,5} + x_{21,30,23,6} + x_{22,30,23,7} = \\
 & = x_{23,12,24,30} + x_{23,16,25,30} + x_{23,17,26,30} + x_{23,18,27,30} + x_{23,24,28,30} + x_{23,28,29,30} + x_{23,29,30,30} \quad (562)
 \end{aligned}$$

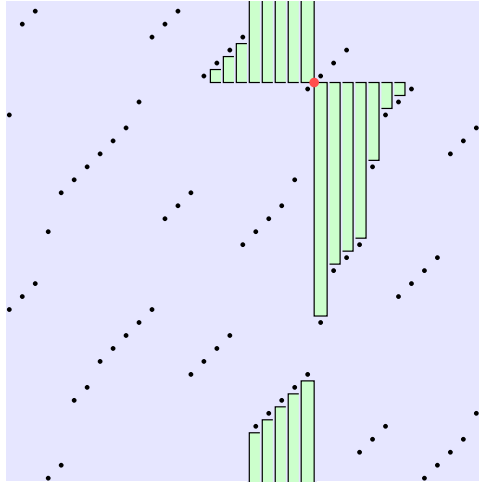

$$x_{15,30,23,31} = x_{23,31,24,11} \quad (563)$$

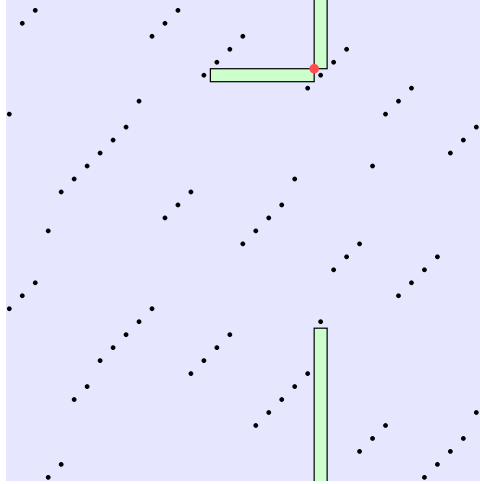

$$x_{16,30,23,32} = x_{23,32,25,11}$$

(564)

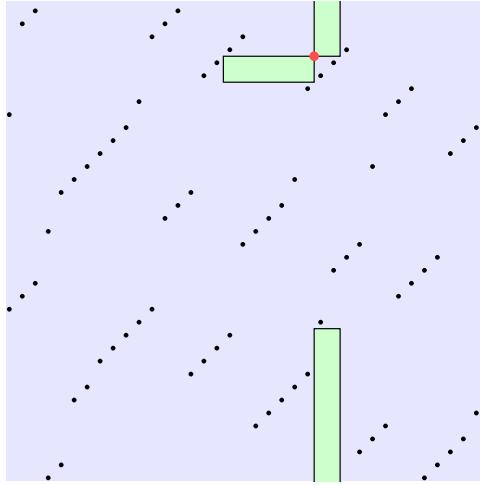

$$x_{17,30,23,33} = x_{23,33,26,11}$$

(565)

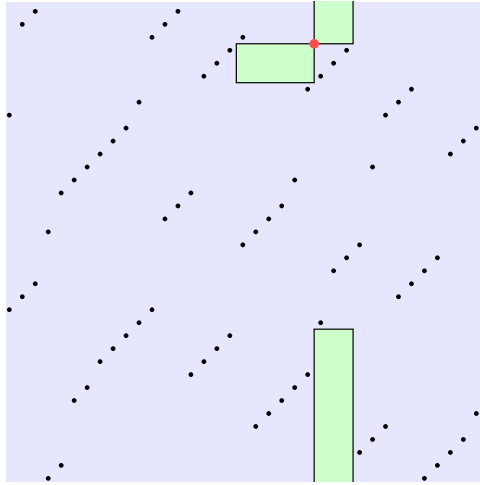

$$0 = x_{24,2,27,15} \tag{566}$$

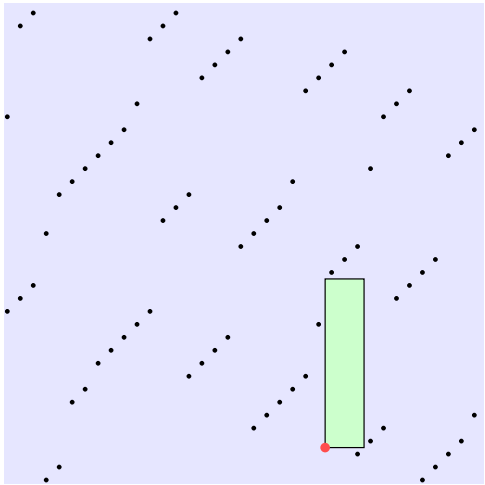

$$x_{18,31,24,3} = x_{24,3,28,15} \tag{567}$$

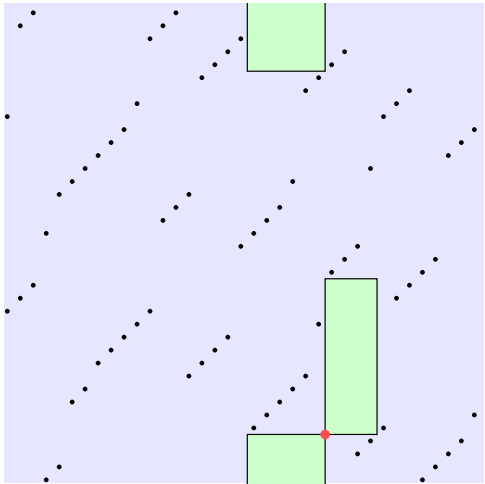

$$x_{19,31,24,4} = x_{24,4,29,15} + x_{24,4,35,13} \tag{568}$$



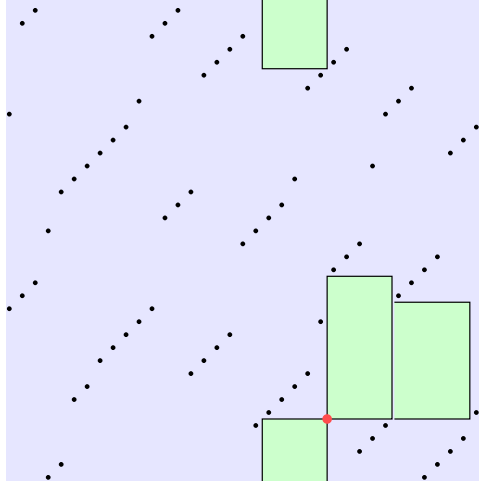

$$x_{20,31,24,5} = x_{24,5,4,12} + x_{24,5,36,13}$$

(569)

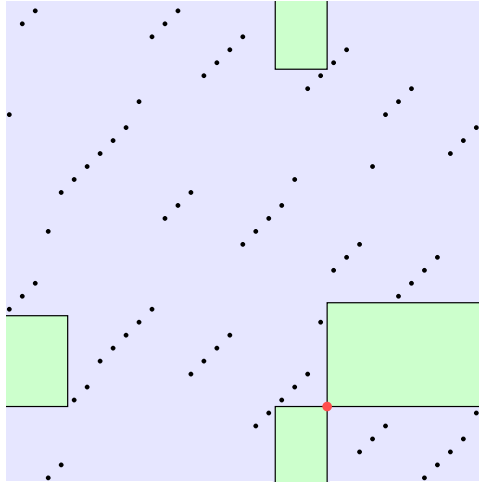

$$x_{21,31,24,6} = x_{24,6,5,12}$$

(570)

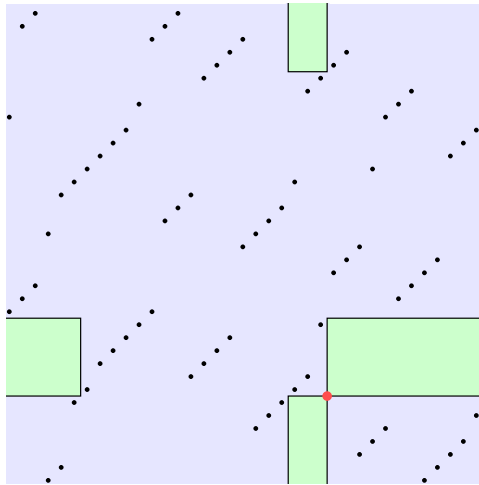

$$x_{22,31,24,7} = x_{24,7,6,12} \tag{571}$$

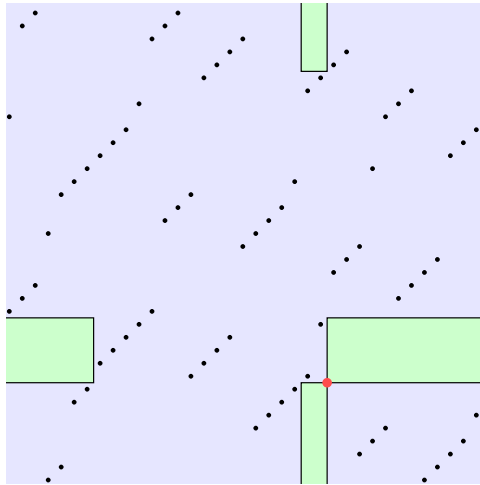

$$0 = x_{24,9,7,12} \tag{572}$$

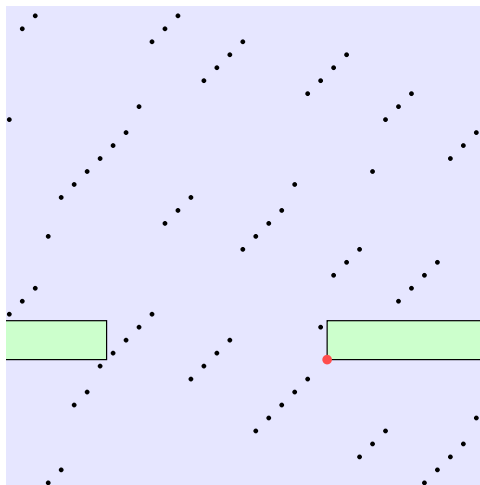

$$0 = x_{24,10,8,12} \tag{573}$$

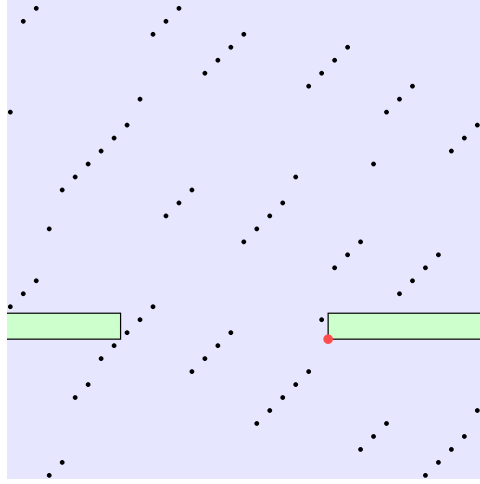

$$x_{23,31,24,11} = x_{24,11,9,12}$$

(574)

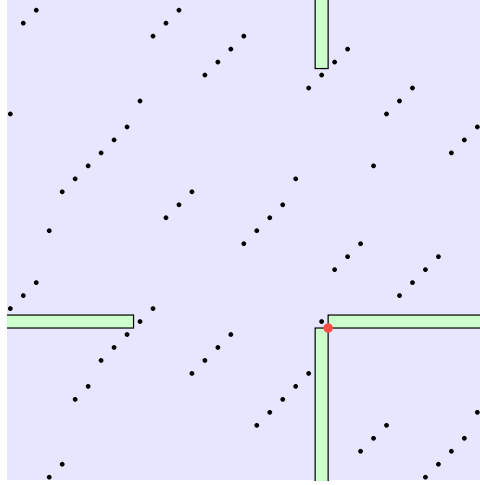

$$\begin{aligned} x_{11,12,24,17} + x_{18,12,24,18} + x_{19,12,24,19} + x_{20,12,24,20} + x_{21,12,24,22} + x_{22,12,24,29} + x_{23,12,24,30} = \\ = x_{24,5,4,12} + x_{24,6,5,12} + x_{24,7,6,12} + x_{24,9,7,12} + x_{24,10,8,12} + x_{24,11,9,12} \end{aligned} \quad (575)$$

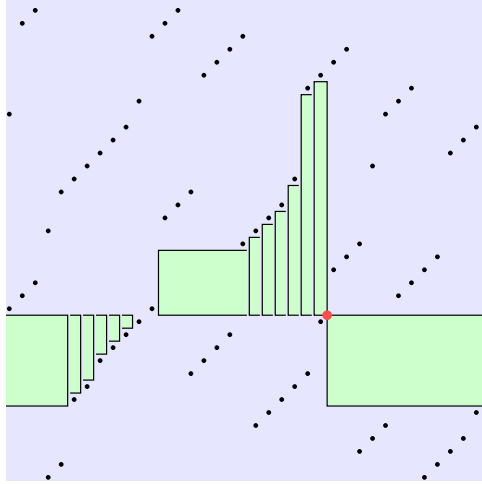

$$x_{2,13,24,17} = x_{24,4,35,13} + x_{24,5,36,13}$$

(576)

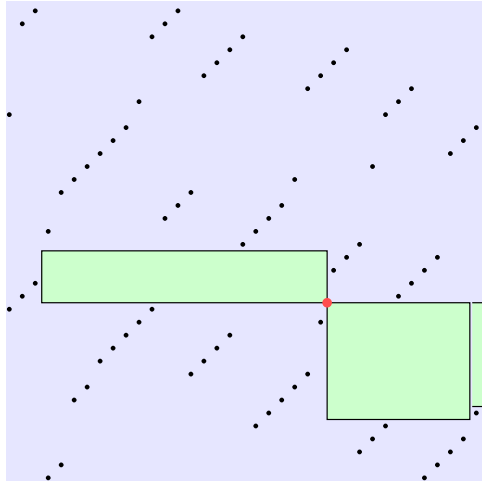

$$x_{32,15,24,16} + x_{33,15,24,17} = x_{24,2,27,15} + x_{24,3,28,15} + x_{24,4,29,15} + x_{24,32,25,15} + x_{24,33,26,15}$$

(577)

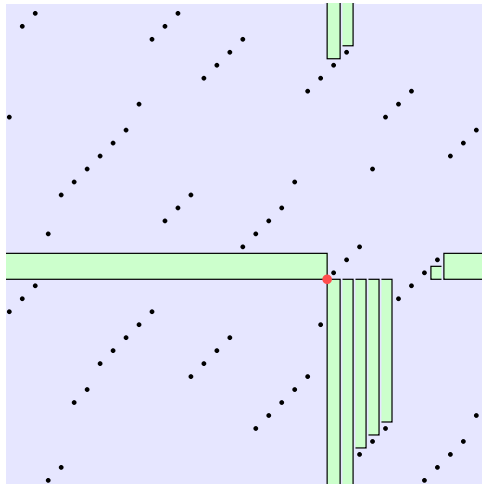

$$x_{32,15,24,16} = x_{24,16,25,31}$$

(578)

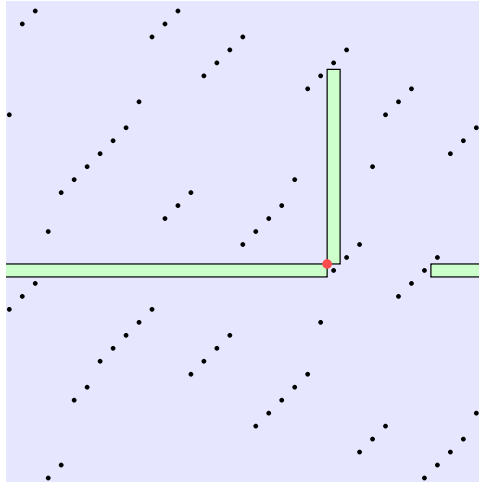

$$x_{2,13,24,17} + x_{11,12,24,17} + x_{33,15,24,17} = x_{24,17,26,31}$$

(579)

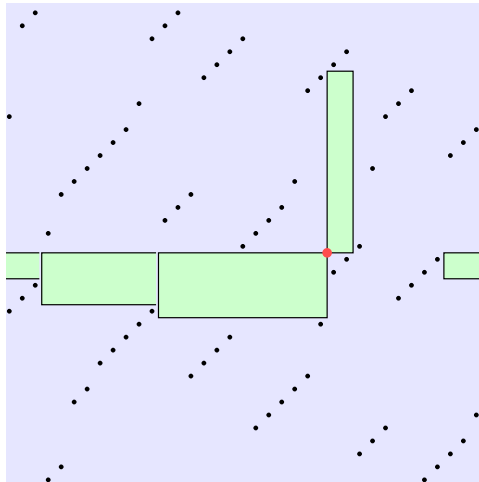

$$x_{18,12,24,18} = x_{24,18,27,31}$$

(580)

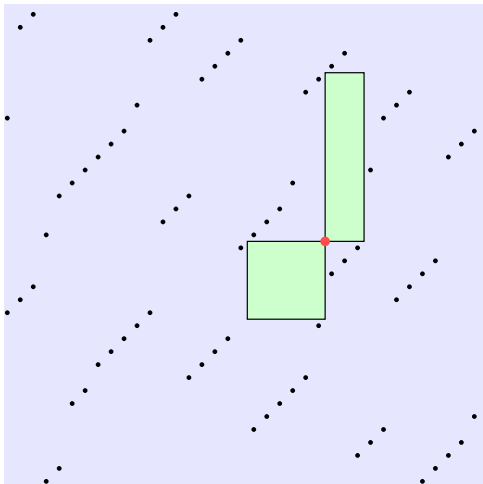

$$x_{19,12,24,19} = 0$$

(581)

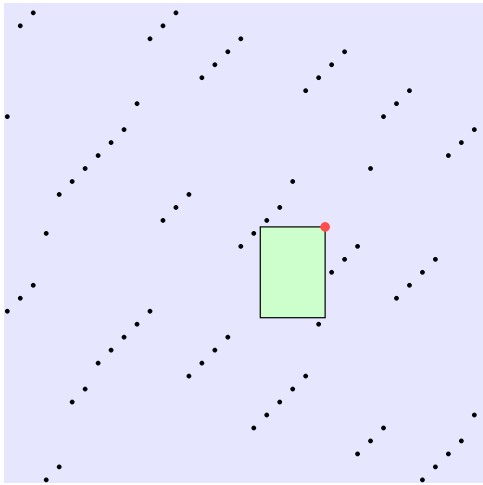

$$x_{20,12,24,20} = 0$$

(582)

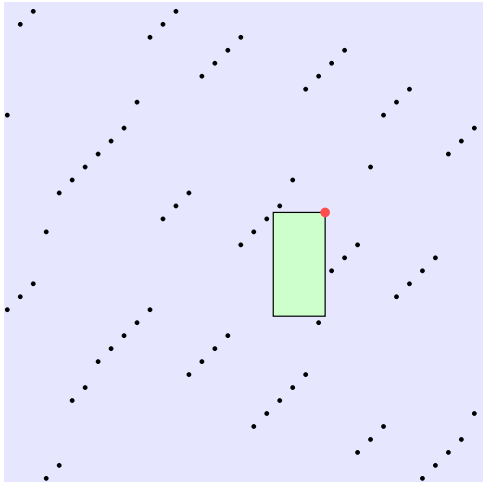

$$x_{21,12,24,22} = 0 \tag{583}$$

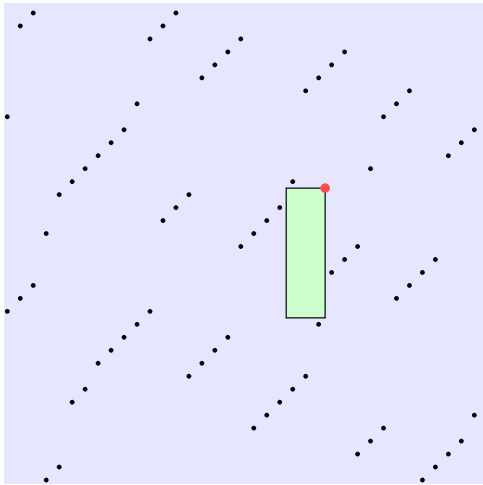

$$0 = x_{24,24,28,31} \tag{584}$$

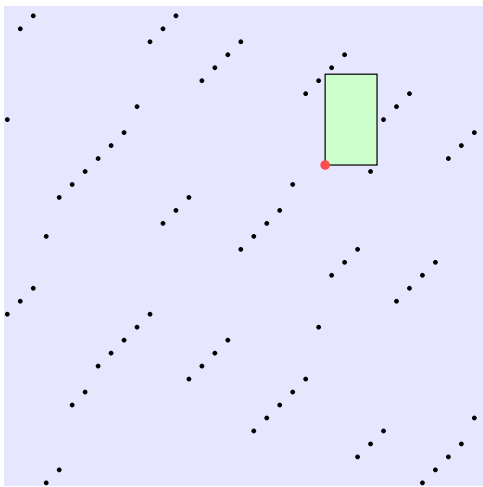

$$0 = x_{24,28,29,31} \tag{585}$$

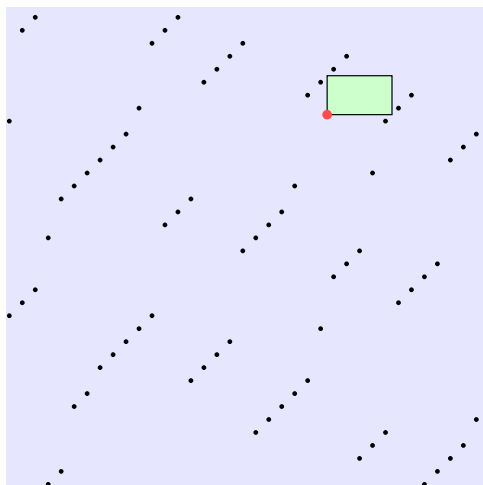

$$x_{22,12,24,29} = x_{24,29,30,31}$$

(586)

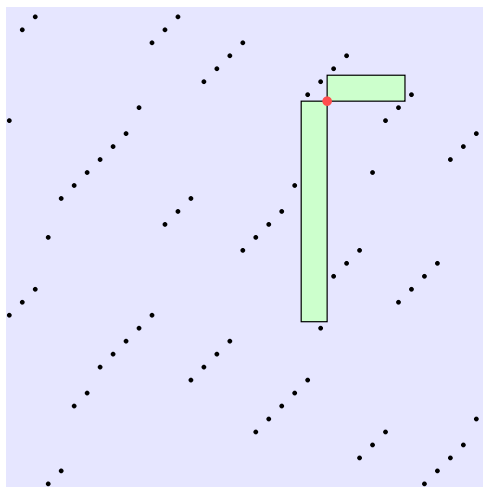

$$x_{23,12,24,30} = x_{24,30,14,31}$$

(587)

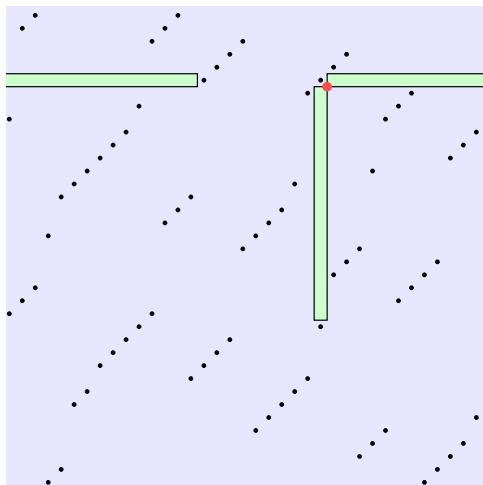



$$\begin{aligned}
& x_{16,31,24,32} + x_{17,31,24,33} + x_{18,31,24,3} + x_{19,31,24,4} + x_{20,31,24,5} + x_{21,31,24,6} + x_{22,31,24,7} + x_{23,31,24,11} = \\
& = x_{24,16,25,31} + x_{24,17,26,31} + x_{24,18,27,31} + x_{24,24,28,31} + x_{24,28,29,31} + x_{24,29,30,31} + x_{24,30,14,31} \quad (588)
\end{aligned}$$

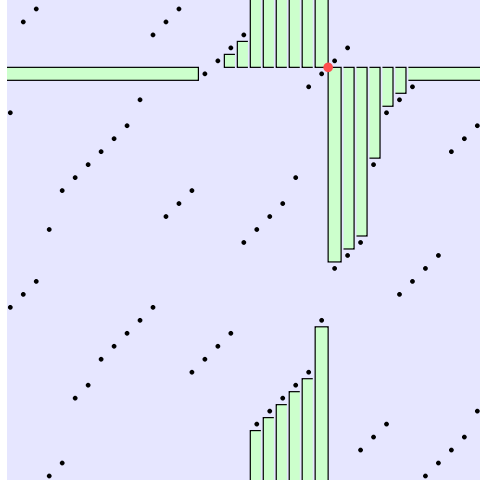

$$x_{16,31,24,32} = x_{24,32,25,15} \quad (589)$$

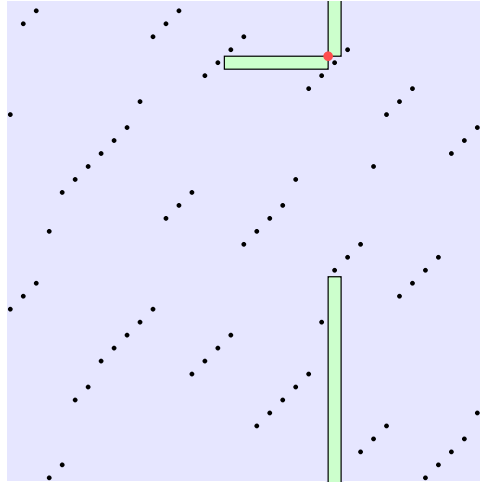

$$x_{17,31,24,33} = x_{24,33,26,15} \quad (590)$$

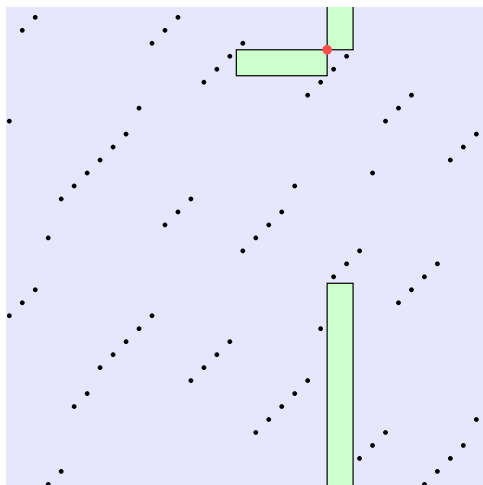

$$0 = x_{25,2,27,16}$$

(591)

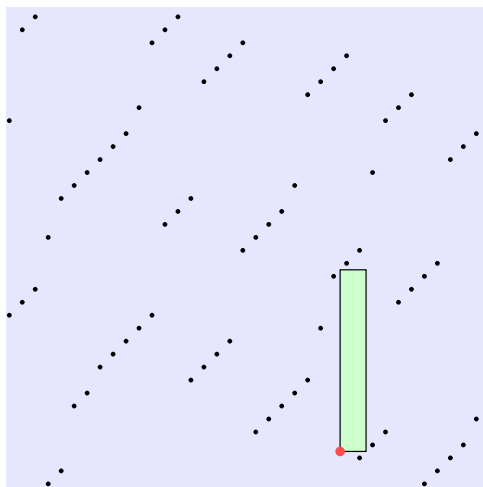

$$x_{18,32,25,3} = x_{25,3,28,16}$$

(592)

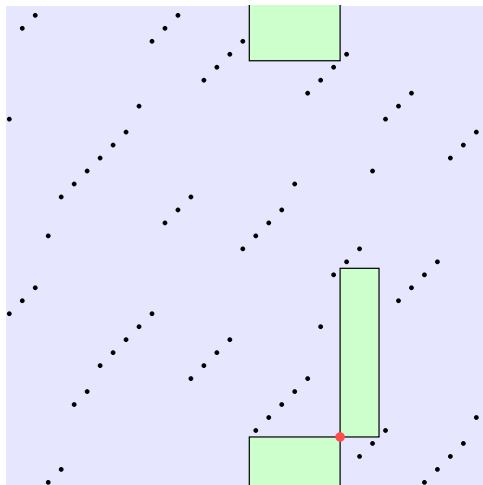

$$x_{19,32,25,4} = x_{25,4,29,16} \tag{593}$$

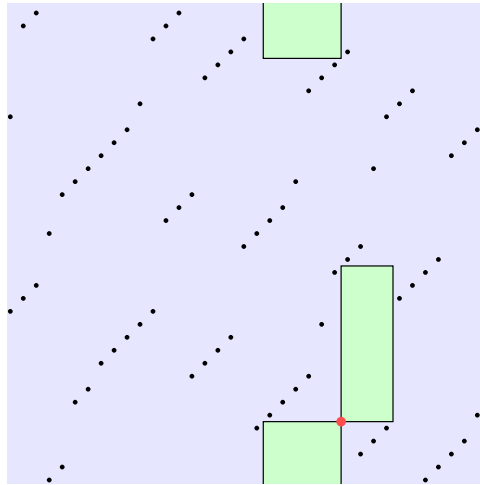

$$x_{20,32,25,5} = 0 \tag{594}$$

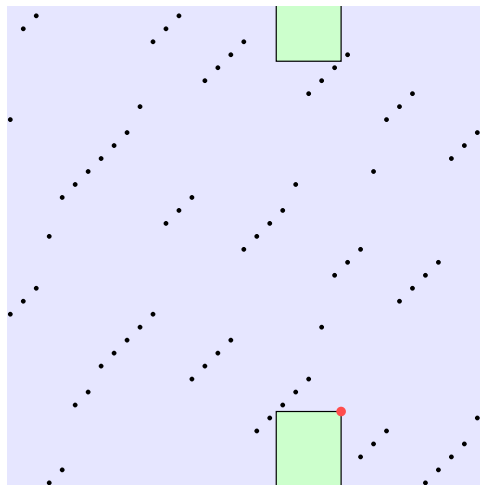

$$x_{21,32,25,6} = 0 \tag{595}$$

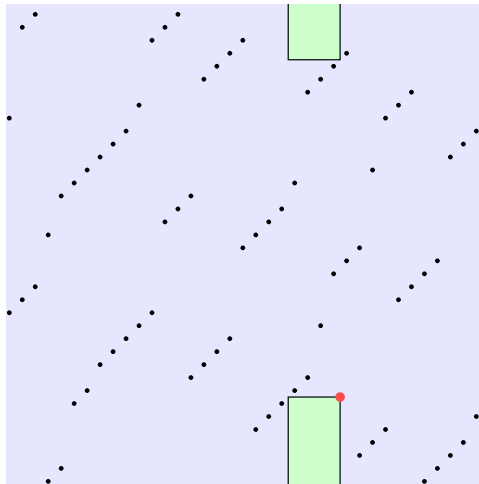

$$x_{22,32,25,7} = 0$$

(596)

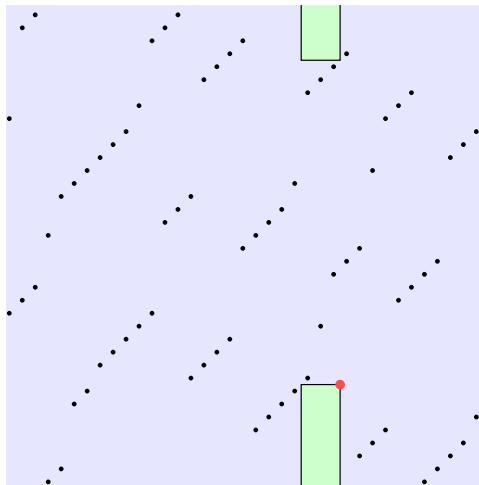

$$x_{23,32,25,11} = 0$$

(597)

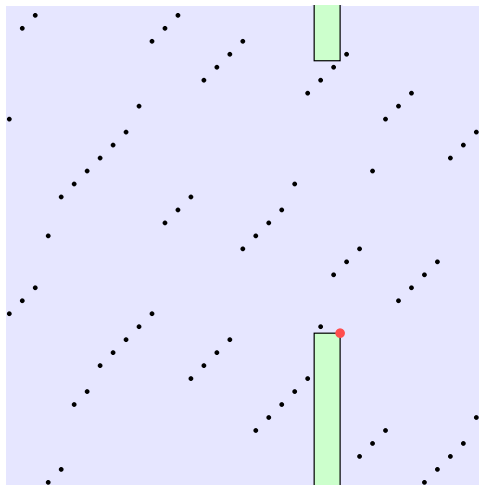

$$0 = x_{25,14,30,16}$$

(598)

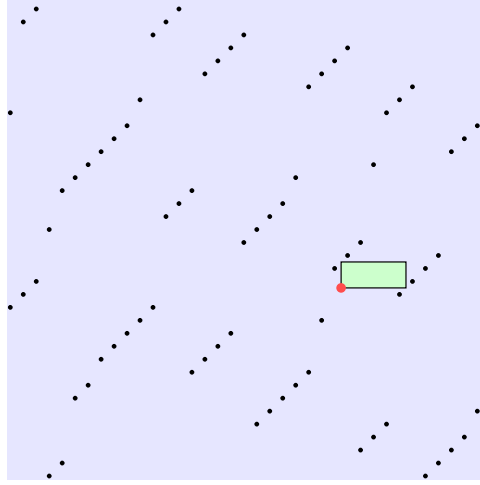

$$x_{24,32,25,15} = x_{25,15,31,16}$$

(599)

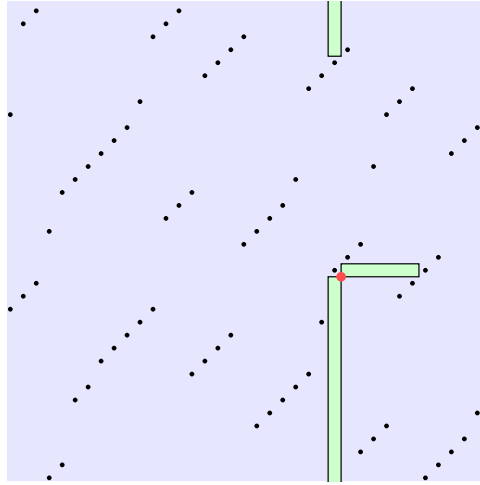

$$\begin{aligned} & x_{18,16,25,18} + x_{19,16,25,19} + x_{20,16,25,20} + x_{21,16,25,22} + x_{22,16,25,29} + x_{23,16,25,30} + x_{24,16,25,31} + x_{33,16,25,17} = \\ & = x_{25,2,27,16} + x_{25,3,28,16} + x_{25,4,29,16} + x_{25,14,30,16} + x_{25,15,31,16} + x_{25,33,26,16} \end{aligned} \quad (600)$$

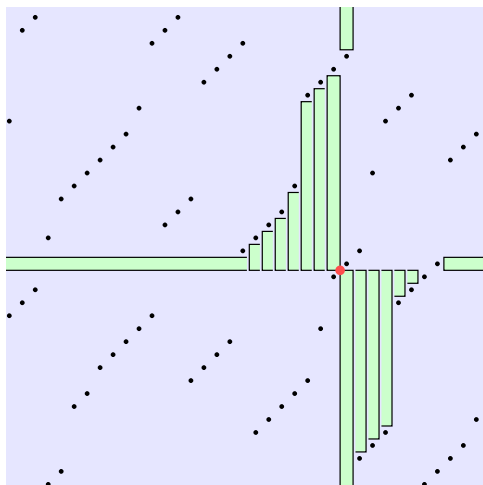

$$x_{33,16,25,17} = x_{25,17,26,32}$$

(601)

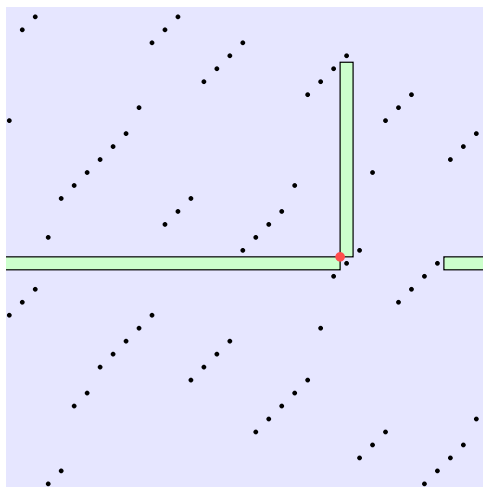

$$x_{18,16,25,18} = x_{25,18,27,32}$$

(602)

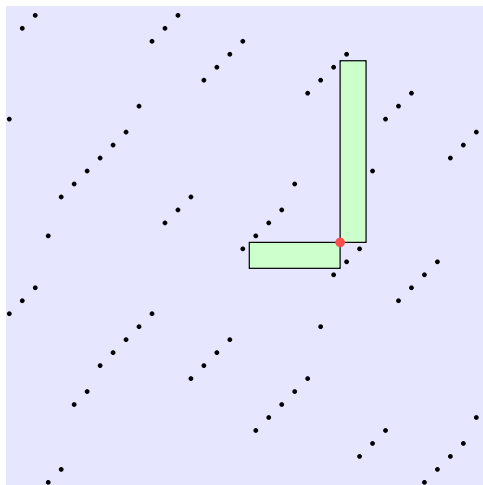

$$x_{19,16,25,19} = 0 \tag{603}$$

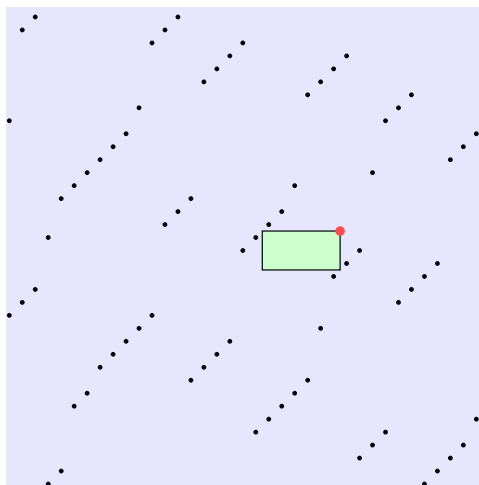

$$x_{20,16,25,20} = 0 \tag{604}$$

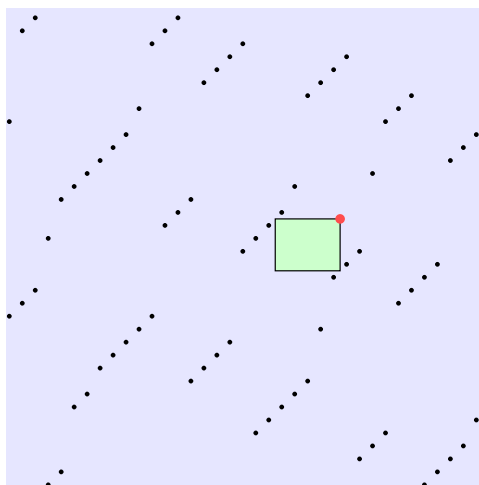

$$x_{21,16,25,22} = 0 \tag{605}$$

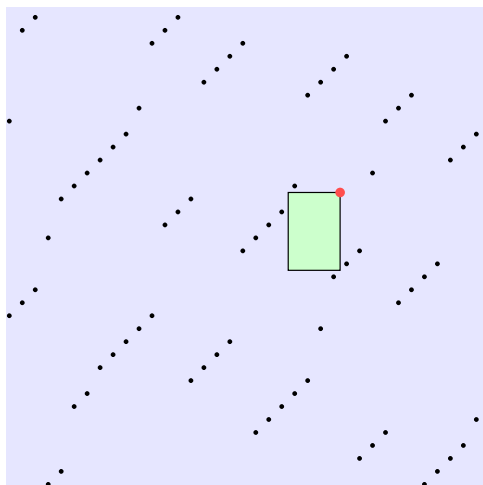

$$0 = x_{25,24,28,32}$$

(606)

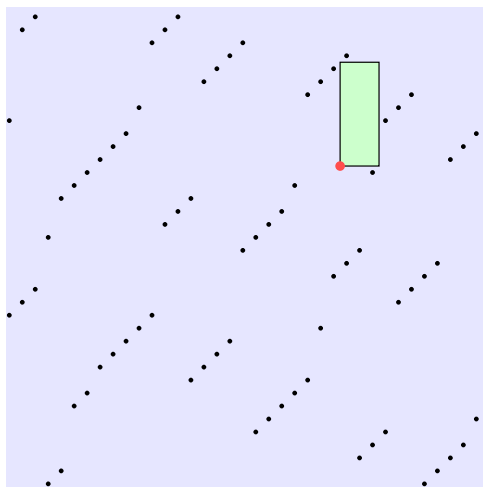

$$0 = x_{25,28,29,32}$$

(607)

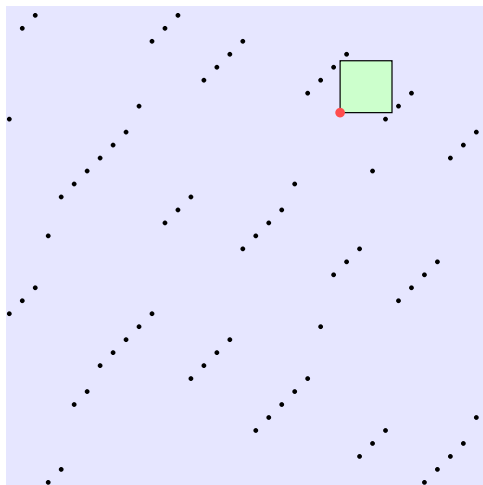



$$x_{22,16,25,29} = x_{25,29,30,32} \tag{608}$$

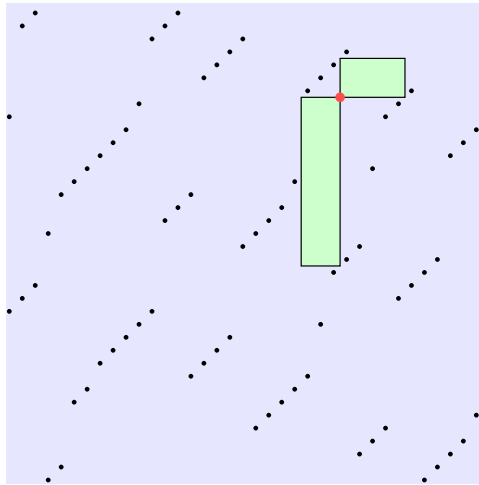

$$x_{23,16,25,30} = x_{25,30,14,32} \tag{609}$$

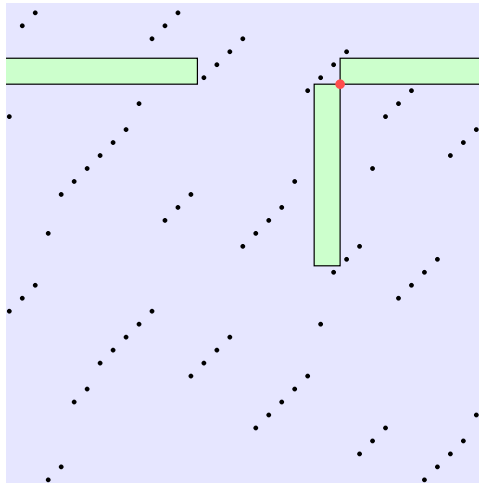

$$x_{24,16,25,31} = x_{25,31,15,32} \tag{610}$$

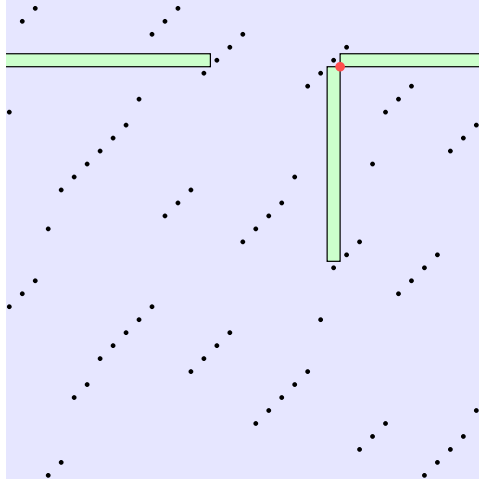

$$\begin{aligned}
 & x_{17,32,25,33} + x_{18,32,25,3} + x_{19,32,25,4} + x_{20,32,25,5} + x_{21,32,25,6} + x_{22,32,25,7} + x_{23,32,25,11} + x_{24,32,25,15} = \\
 & = x_{25,17,26,32} + x_{25,18,27,32} + x_{25,24,28,32} + x_{25,28,29,32} + x_{25,29,30,32} + x_{25,30,14,32} + x_{25,31,15,32} \quad (611)
 \end{aligned}$$

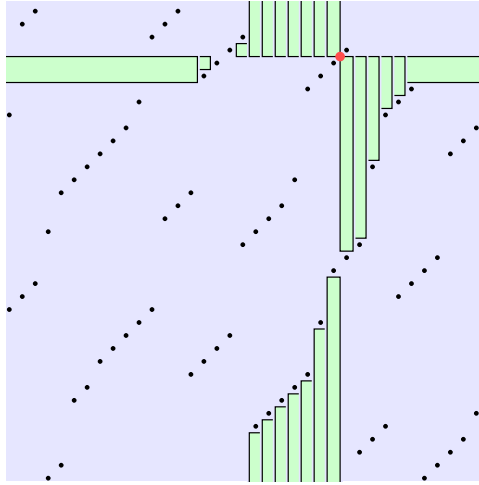

$$x_{17,32,25,33} = x_{25,33,26,16} \quad (612)$$

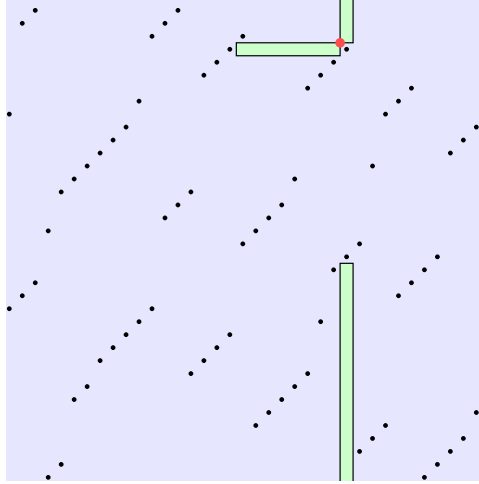

$$x_{34,1,26,2} + x_{35,1,26,3} = x_{26,18,27,1} + x_{26,24,28,1} + x_{26,28,29,1} + x_{26,29,30,1} + x_{26,30,31,1} \quad (613)$$

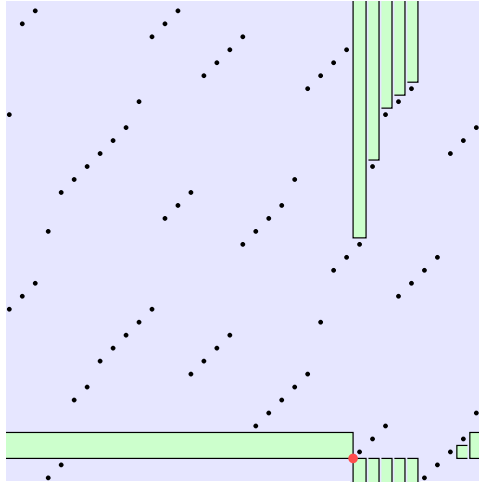

$$x_{34,1,26,2} = x_{26,2,27,17} \quad (614)$$

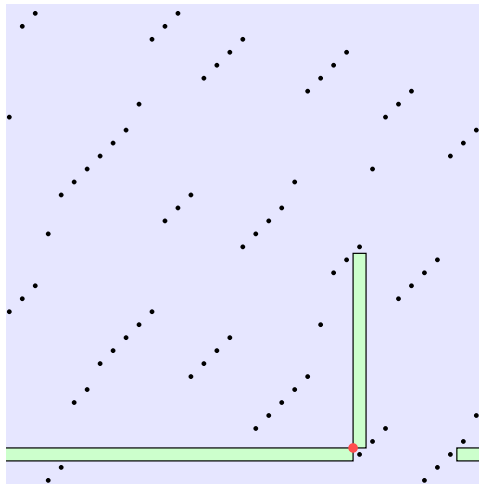

$$x_{4,36,26,3} + x_{13,34,26,3} + x_{18,33,26,3} + x_{35,1,26,3} = x_{26,3,28,17} \quad (615)$$

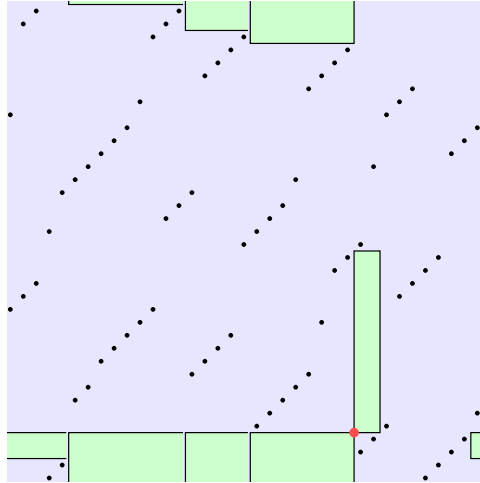

$$x_{19,33,26,4} = x_{26,4,29,17} \quad (616)$$

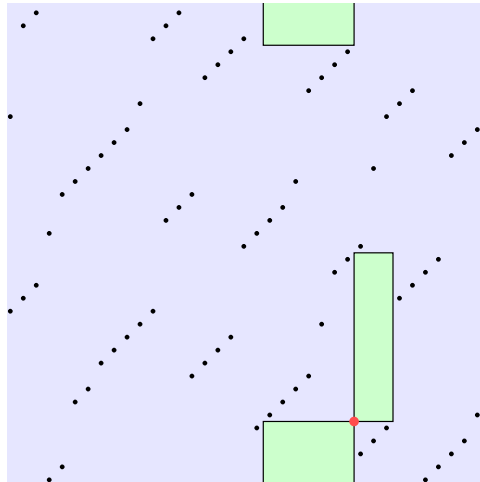

$$x_{20,33,26,5} = 0 \quad (617)$$

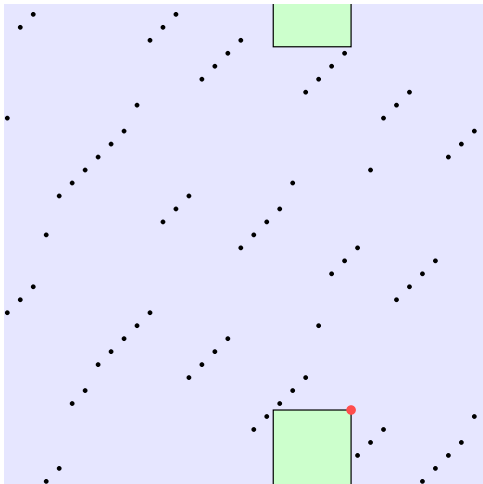

$$x_{21,33,26,6} = 0$$

(618)

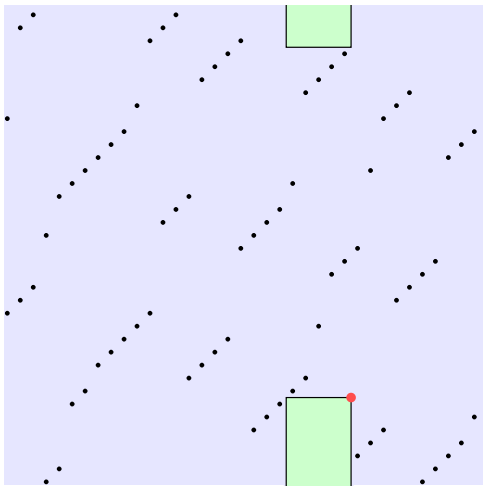

$$x_{22,33,26,7} = 0$$

(619)

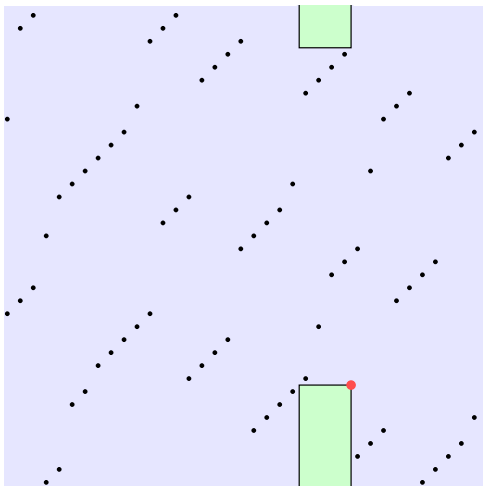

$$x_{23,33,26,11} = 0 \tag{620}$$

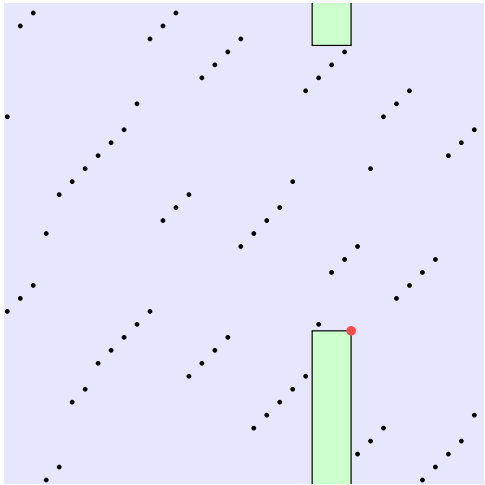

$$0 = x_{26,14,30,17} \tag{621}$$

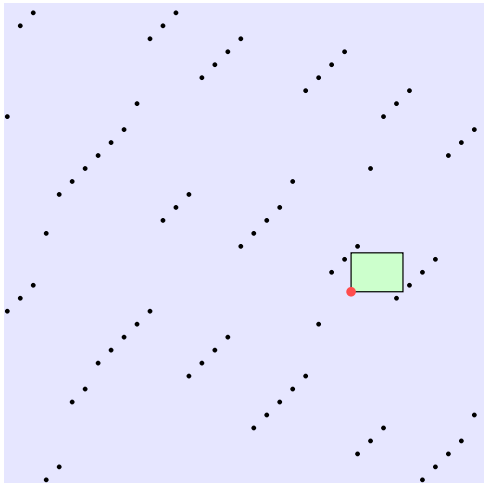

$$x_{24,33,26,15} = x_{26,15,31,17} \tag{622}$$

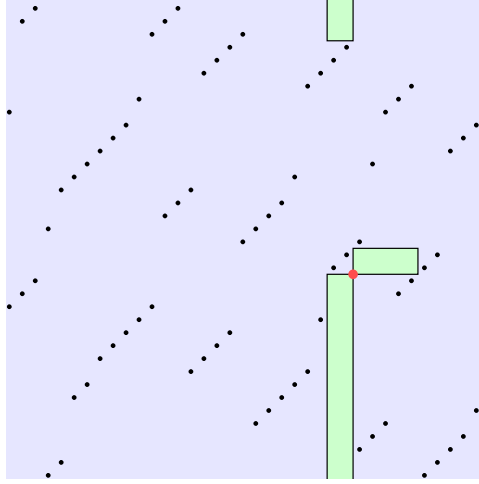

$$x_{25,33,26,16} = x_{26,16,32,17}$$

(623)

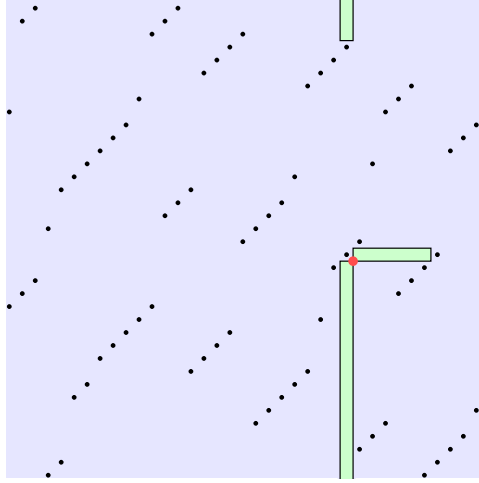

$$\begin{aligned} x_{18,17,26,18} + x_{19,17,26,19} + x_{20,17,26,20} + x_{21,17,26,22} + x_{22,17,26,29} + x_{23,17,26,30} + x_{24,17,26,31} + x_{25,17,26,32} = \\ = x_{26,2,27,17} + x_{26,3,28,17} + x_{26,4,29,17} + x_{26,14,30,17} + x_{26,15,31,17} + x_{26,16,32,17} \end{aligned} \quad (624)$$

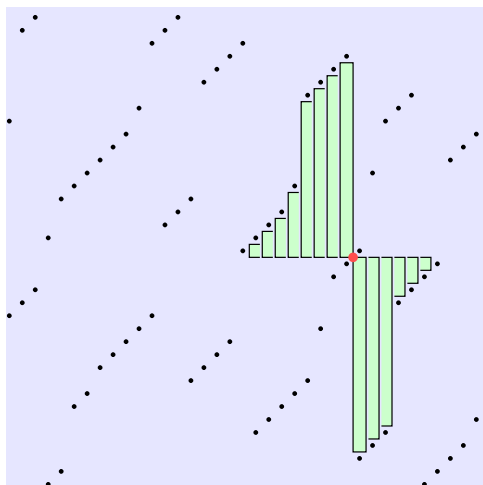

$$x_{18,17,26,18} = x_{26,18,27,1}$$

(625)

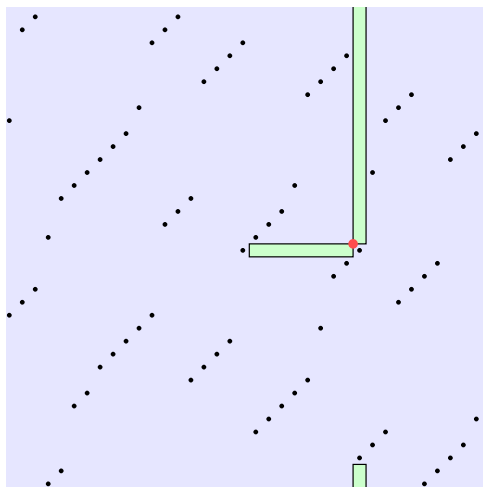

$$x_{19,17,26,19} = 0$$

(626)

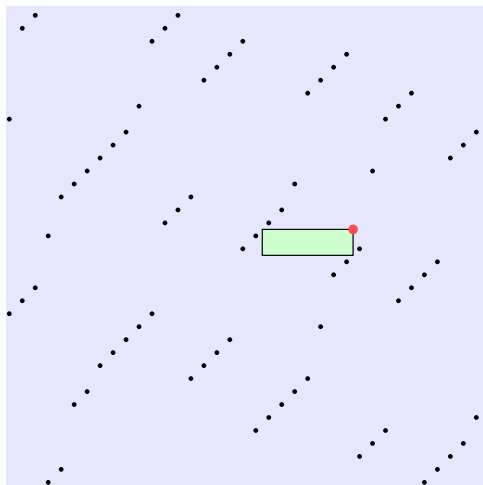



$$x_{20,17,26,20} = 0 \tag{627}$$

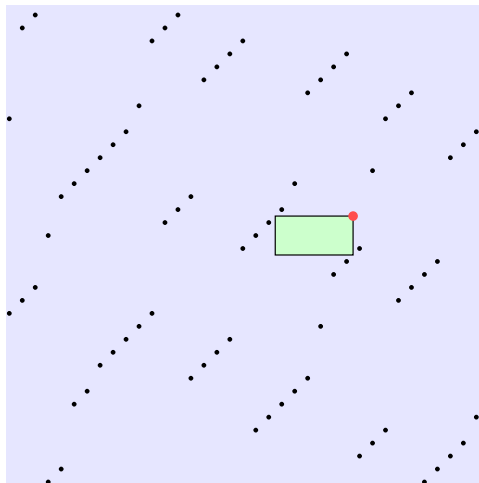

$$x_{21,17,26,22} = 0 \tag{628}$$

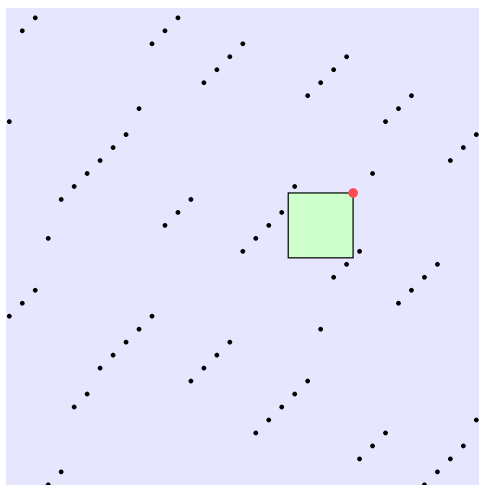

$$0 = x_{26,24,28,1} \tag{629}$$

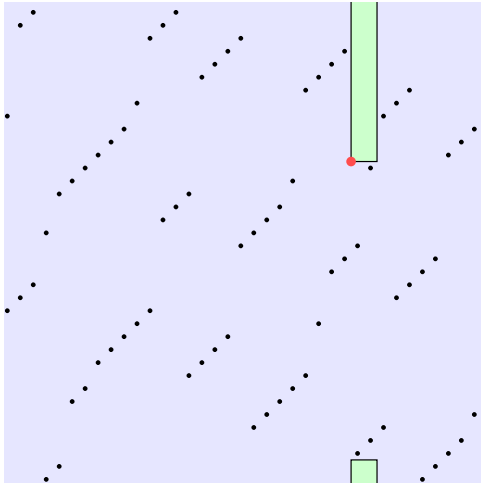

$$0 = x_{26,28,29,1}$$

(630)

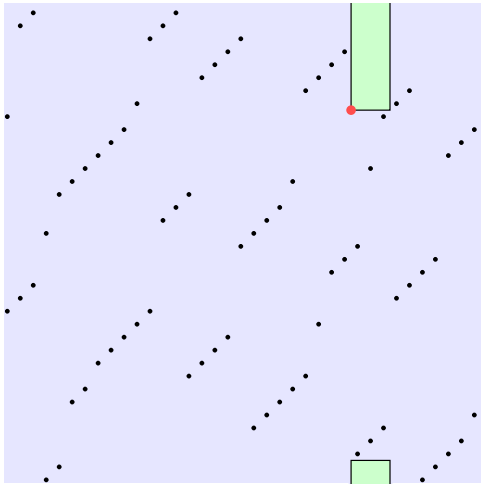

$$x_{22,17,26,29} = x_{26,29,30,1}$$

(631)

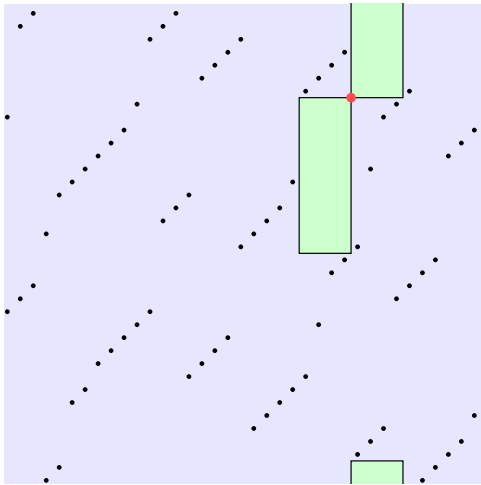

$$x_{23,17,26,30} = x_{26,30,0,36} + x_{26,30,10,34} + x_{26,30,14,33} + x_{26,30,31,1} \quad (632)$$

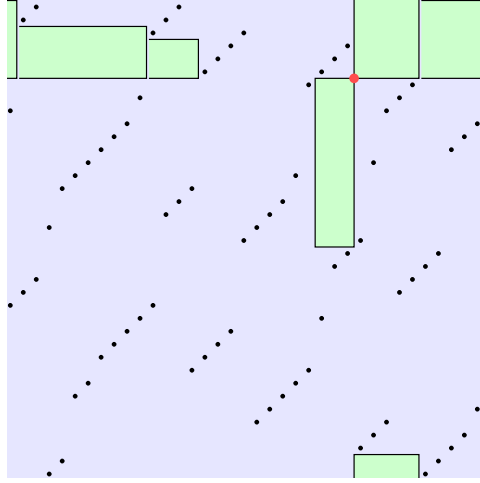

$$x_{24,17,26,31} = x_{26,31,15,33} \quad (633)$$

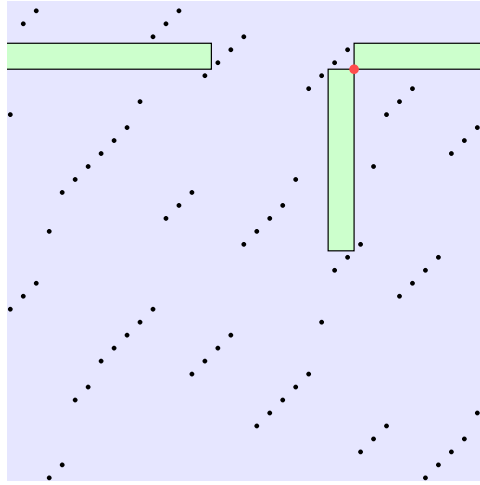

$$x_{25,17,26,32} = x_{26,32,16,33} \quad (634)$$

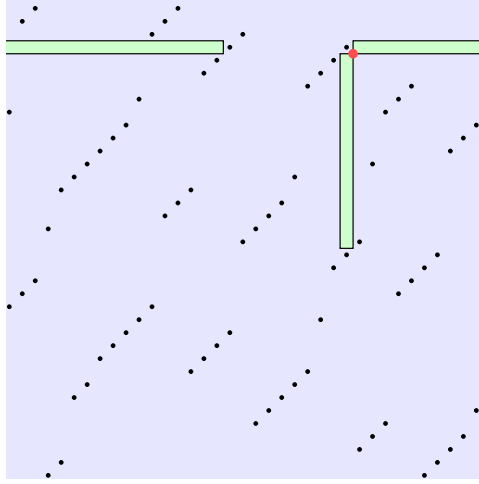

$$\begin{aligned}
 x_{18,33,26,3} + x_{19,33,26,4} + x_{20,33,26,5} + x_{21,33,26,6} + x_{22,33,26,7} + x_{23,33,26,11} + x_{24,33,26,15} + x_{25,33,26,16} = \\
 = x_{26,30,14,33} + x_{26,31,15,33} + x_{26,32,16,33} \quad (635)
 \end{aligned}$$

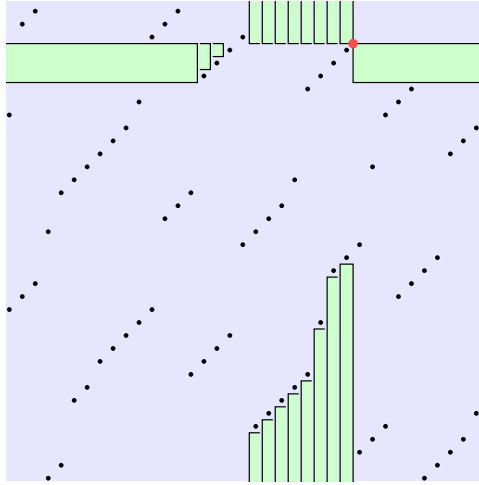

$$x_{13,34,26,3} = x_{26,30,10,34} \quad (636)$$

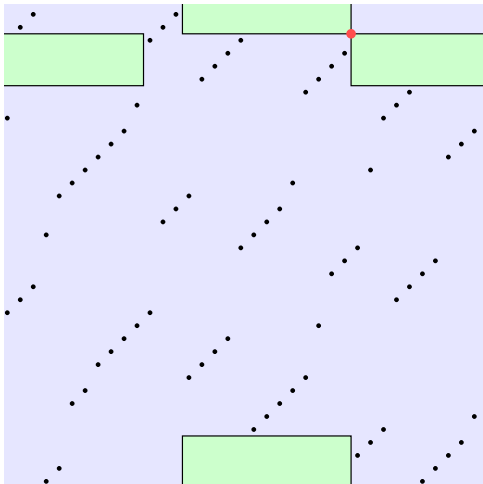

$$x_{4,36,26,3} = x_{26,30,0,36}$$

(637)

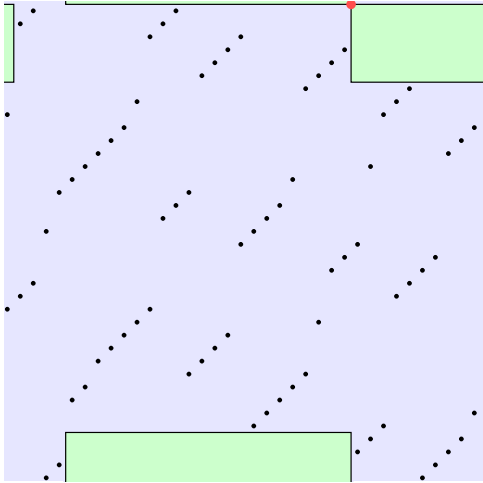

$$0 = x_{27,0,32,2}$$

(638)

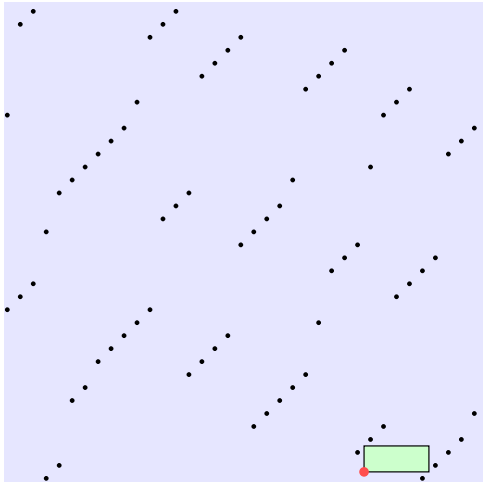

$$x_{26,18,27,1} = x_{27,1,33,2}$$

(639)

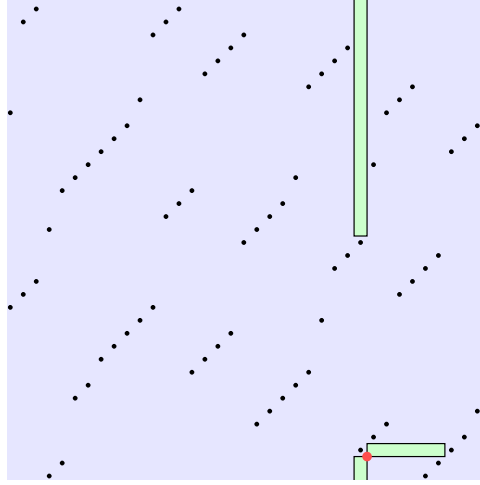

$$\begin{aligned} x_{19,2,27,4} + x_{20,2,27,5} + x_{21,2,27,6} + x_{22,2,27,7} + x_{23,2,27,11} + x_{24,2,27,15} + x_{25,2,27,16} + x_{26,2,27,17} + x_{35,2,27,3} = \\ = x_{27,0,32,2} + x_{27,1,33,2} + x_{27,24,28,2} + x_{27,28,29,2} + x_{27,29,30,2} + x_{27,30,31,2} \end{aligned} \quad (640)$$

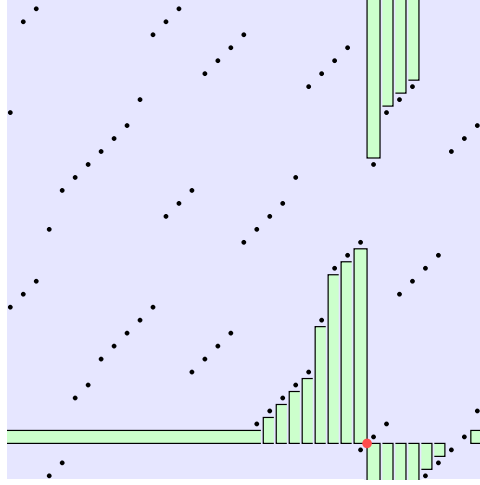

$$x_{35,2,27,3} = x_{27,3,28,23}$$

(641)

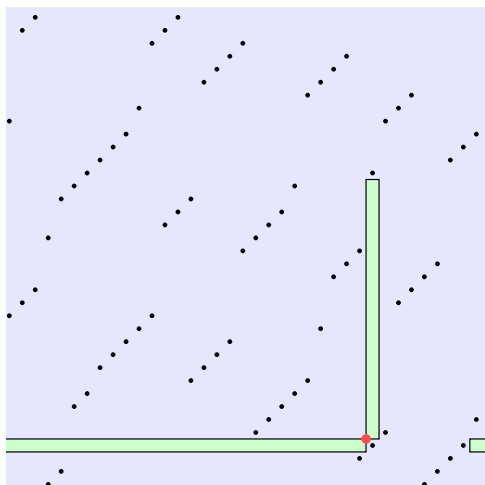

$$x_{19,2,27,4} = x_{27,4,29,23}$$

(642)

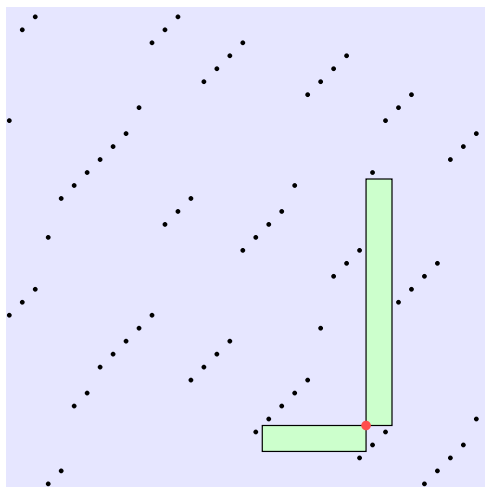

$$x_{20,2,27,5} = 0$$

(643)

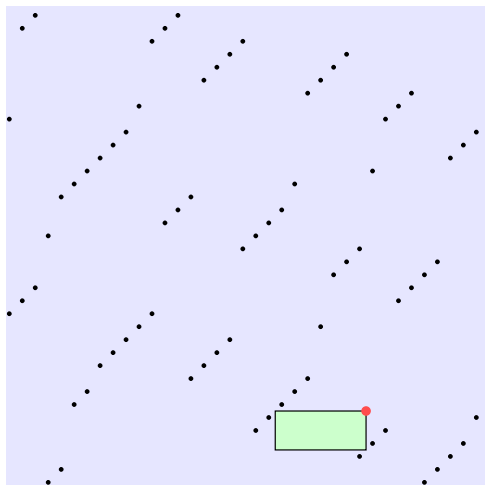

$$x_{21,2,27,6} = 0 \tag{644}$$

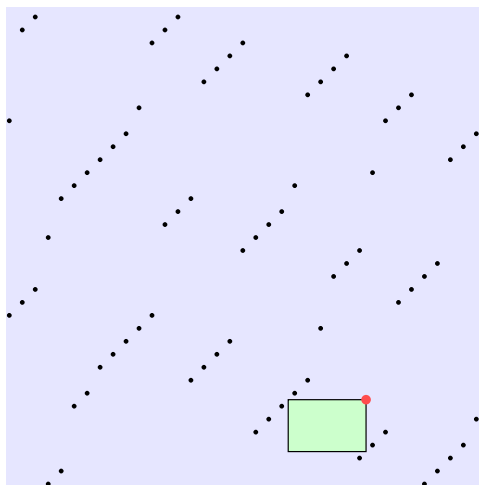

$$x_{22,2,27,7} = 0 \tag{645}$$

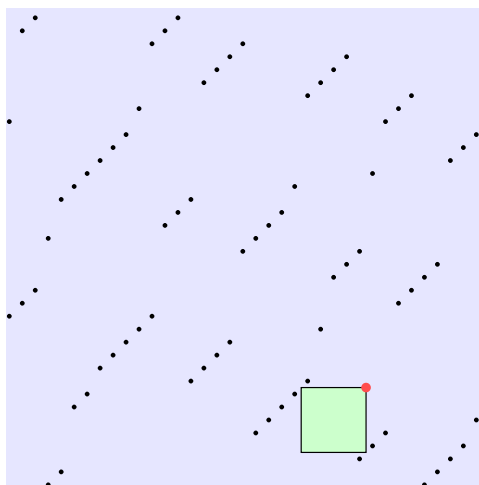

$$x_{23,2,27,11} = 0 \tag{646}$$



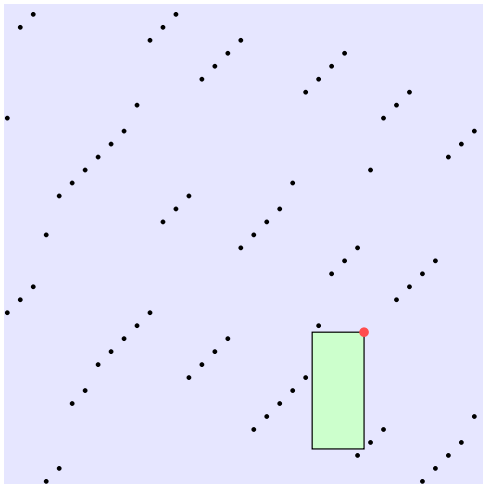

$$0 = x_{27,14,30,23}$$

(647)

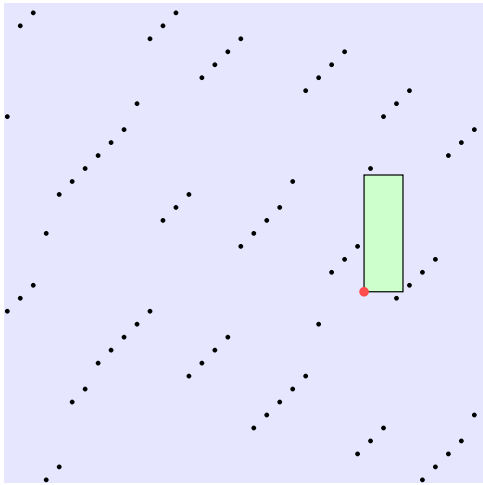

$$x_{24,2,27,15} = x_{27,15,31,23}$$

(648)

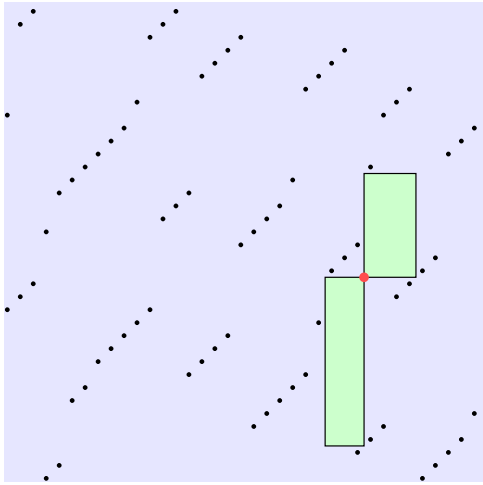

$$x_{25,2,27,16} = x_{27,16,32,23} \quad (649)$$

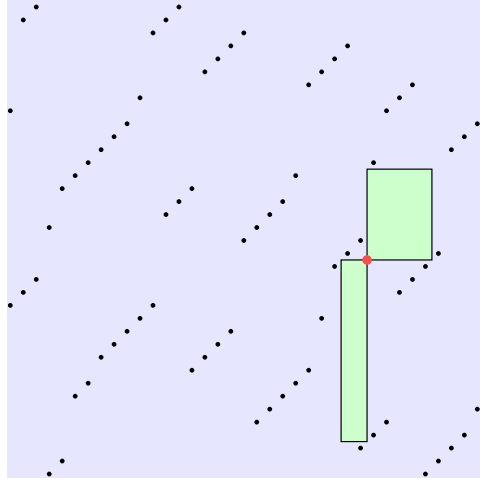

$$x_{26,2,27,17} = x_{27,17,2,23} + x_{27,17,17,18} \quad (650)$$

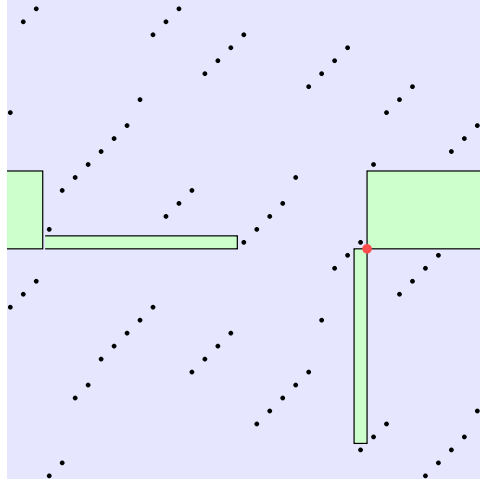

$$x_{22,18,27,29} + x_{23,18,27,30} + x_{24,18,27,31} + x_{25,18,27,32} + x_{26,18,27,1} = x_{27,17,17,18} \quad (651)$$

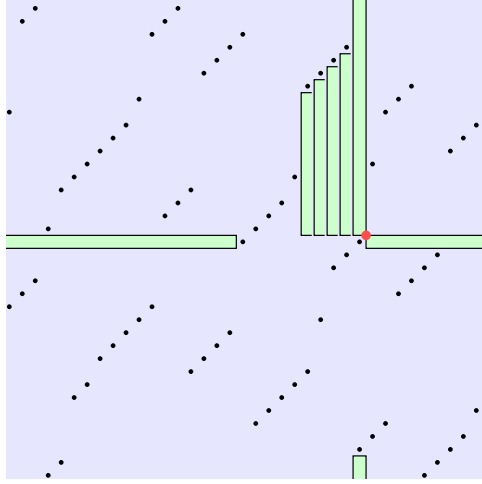

$$\begin{aligned}
 & x_{6,23,27,24} + x_{7,23,27,25} + x_{8,23,27,26} + x_{9,23,27,28} + x_{10,23,27,29} = \\
 & = x_{27,3,28,23} + x_{27,4,29,23} + x_{27,14,30,23} + x_{27,15,31,23} + x_{27,16,32,23} + x_{27,17,2,23} \quad (652)
 \end{aligned}$$

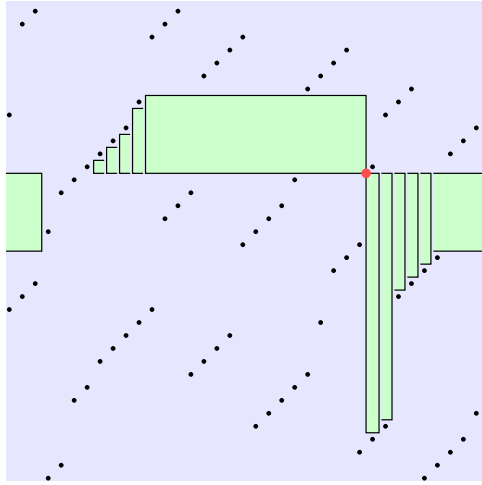

$$x_{6,23,27,24} = x_{27,24,28,2} \quad (653)$$

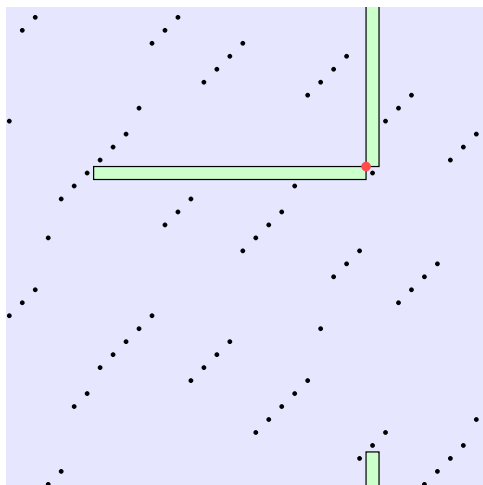

$$x_{7,23,27,25} = 0$$

(654)

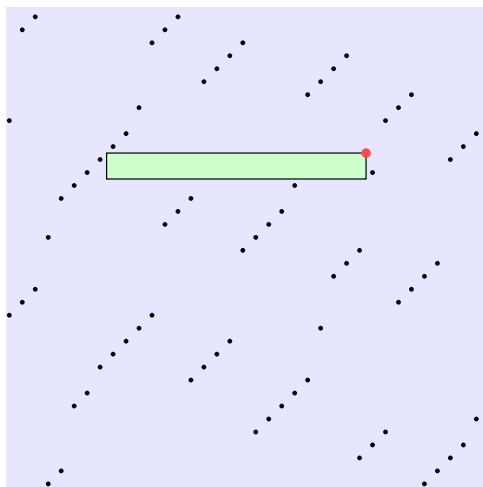

$$x_{8,23,27,26} = 0$$

(655)

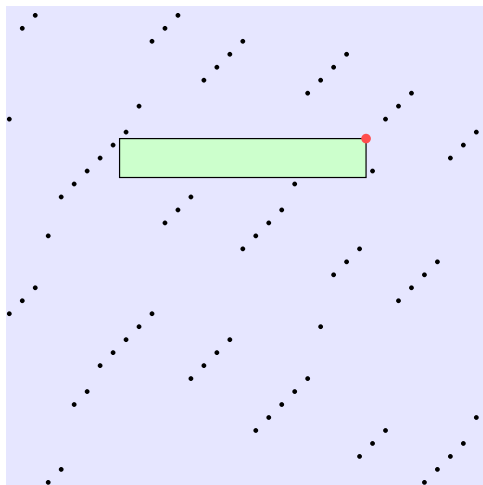

$$x_{9,23,27,28} = x_{27,28,29,2} \quad (656)$$

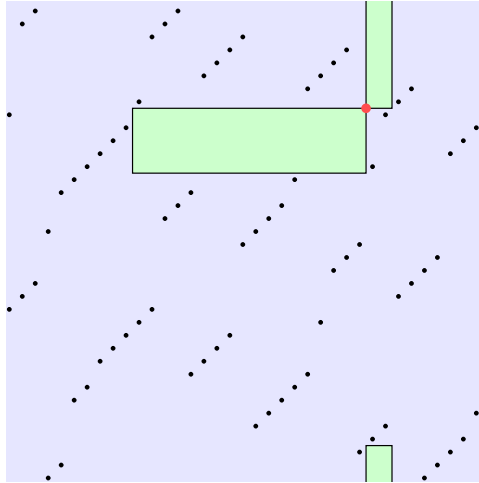

$$x_{10,23,27,29} + x_{22,18,27,29} = x_{27,29,30,2} \quad (657)$$

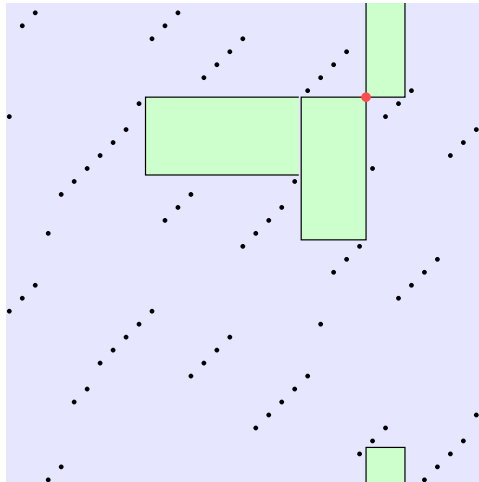

$$x_{23,18,27,30} = x_{27,30,31,2} \quad (658)$$

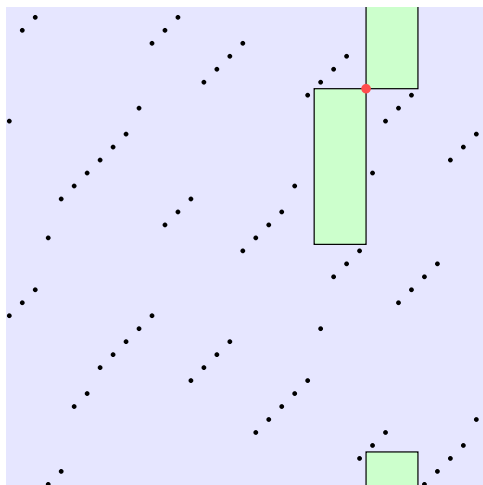

$$x_{24,18,27,31} = 0$$

(659)

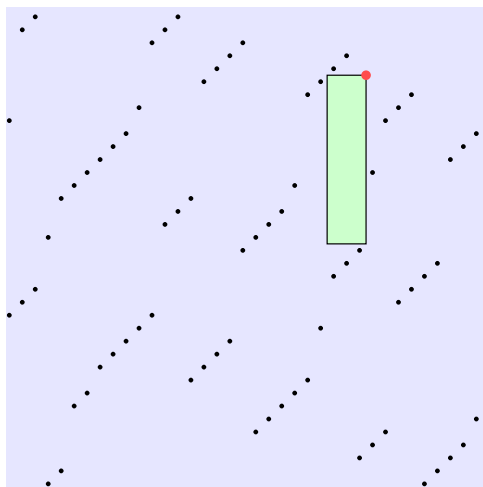

$$x_{25,18,27,32} = 0$$

(660)

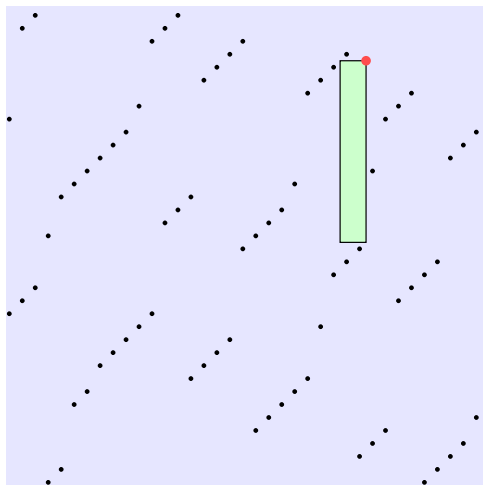

$$0 = x_{28,0,32,3}$$

(661)

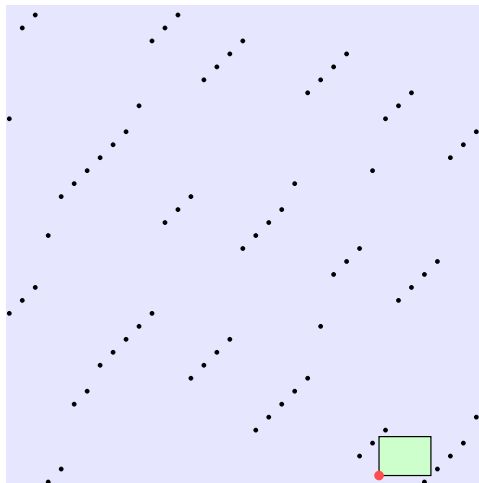

$$x_{26,24,28,1} = x_{28,1,33,3}$$

(662)

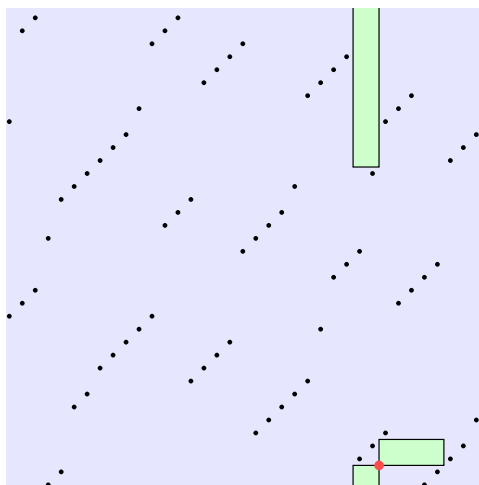

$$x_{27,24,28,2} = x_{28,2,34,3}$$

(663)

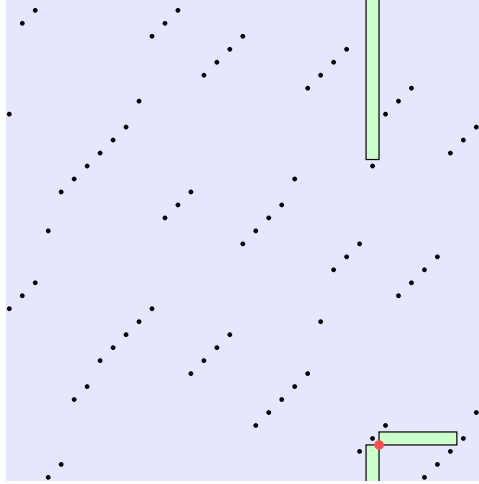

$$\begin{aligned}
 x_{19,3,28,4} + x_{20,3,28,5} + x_{21,3,28,6} + x_{22,3,28,7} + x_{23,3,28,11} + x_{24,3,28,15} + x_{25,3,28,16} + x_{26,3,28,17} + x_{27,3,28,23} = \\
 = x_{28,0,32,3} + x_{28,1,33,3} + x_{28,2,34,3} + x_{28,28,29,3} + x_{28,29,30,3} + x_{28,30,31,3} \quad (664)
 \end{aligned}$$

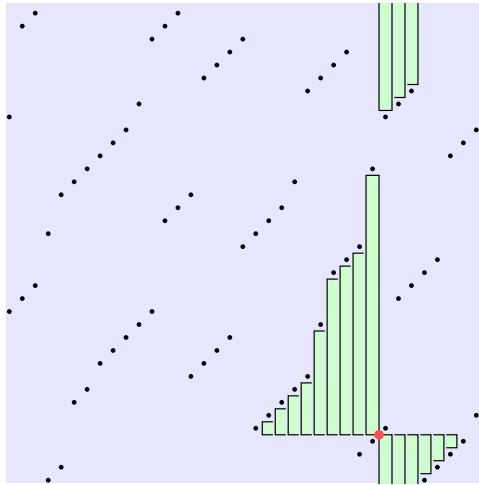

$$x_{19,3,28,4} = x_{28,4,29,27} \quad (665)$$



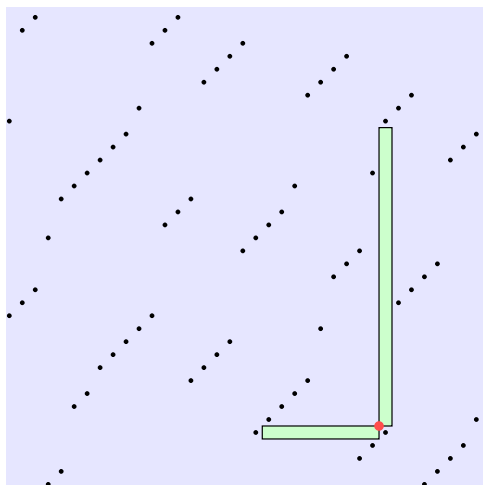

$$x_{20,3,28,5} = 0$$

(666)

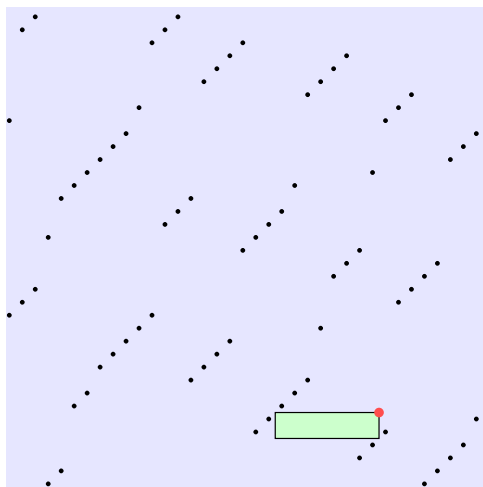

$$x_{21,3,28,6} = 0$$

(667)

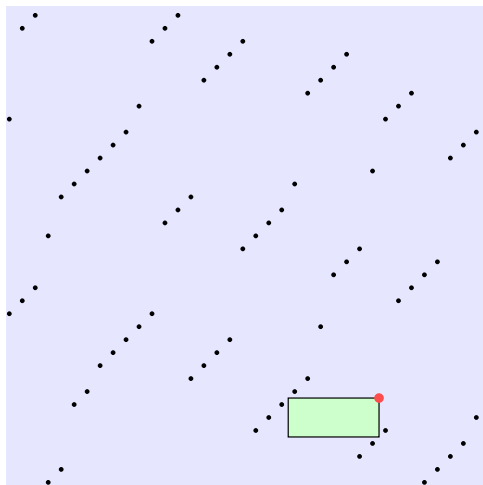

$$x_{22,3,28,7} = 0$$

(668)

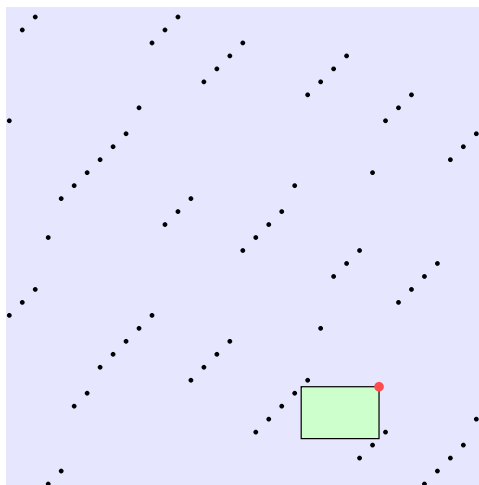

$$x_{23,3,28,11} = 0$$

(669)

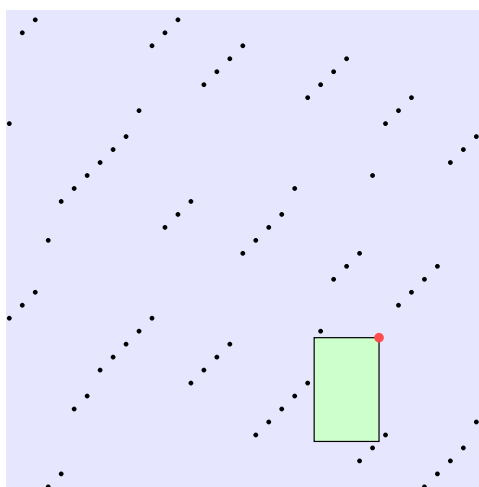

$$0 = x_{28,14,30,27}$$

(670)

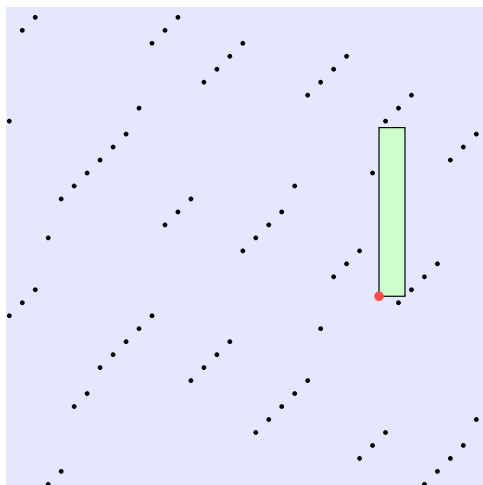

$$x_{24,3,28,15} = x_{28,15,31,27}$$

(671)

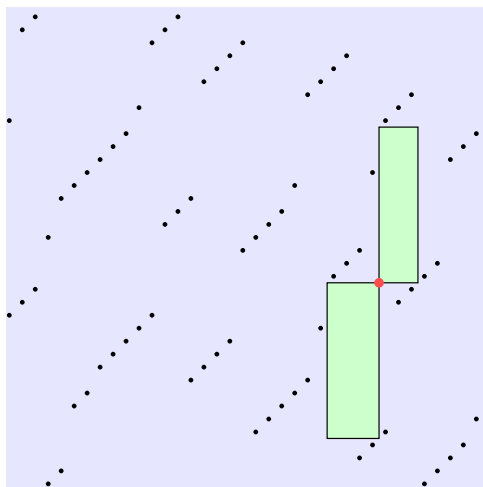

$$x_{25,3,28,16} = x_{28,16,32,27}$$

(672)

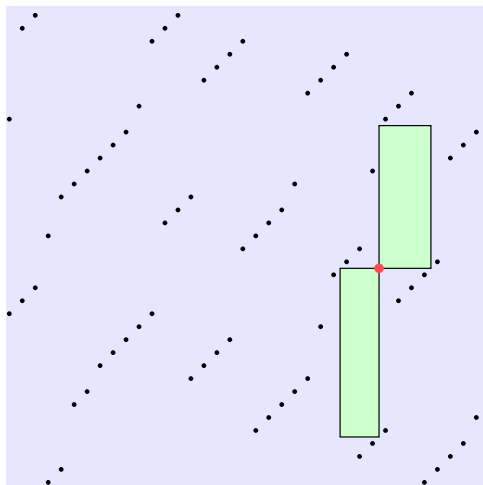

$$x_{26,3,28,17} = x_{28,17,2,24} + x_{28,17,33,27}$$

(673)

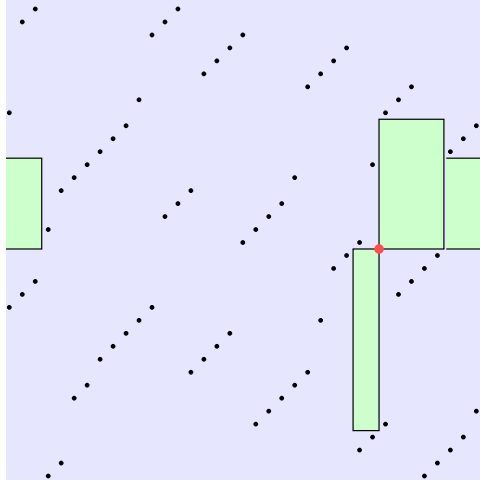

$$0 = x_{28,19,3,24}$$

(674)

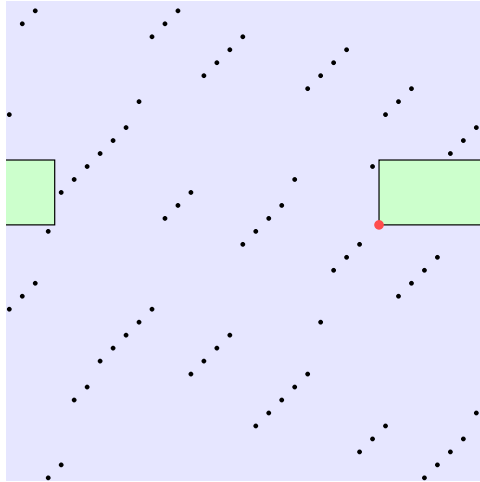

$$0 = x_{28,22,4,24}$$

(675)

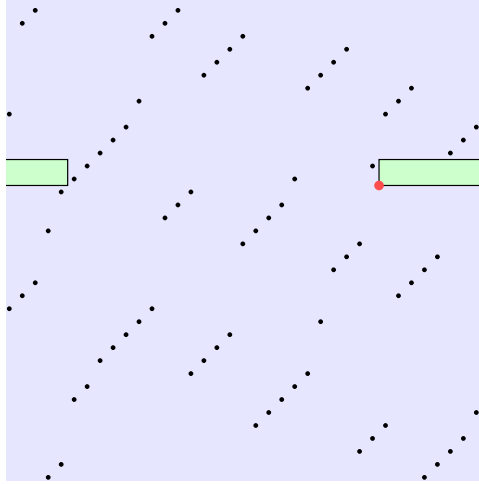

$$x_{27,3,28,23} = x_{28,23,5,24}$$

(676)

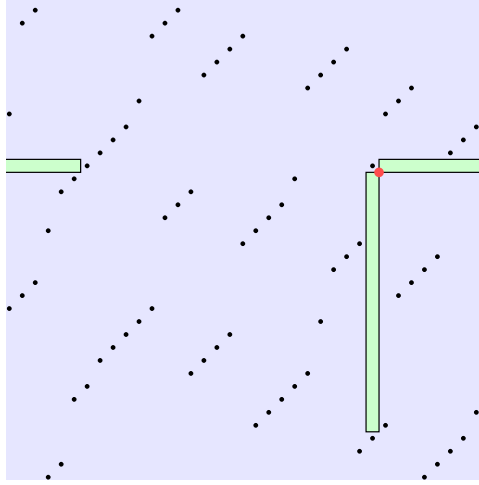

$$\begin{aligned} x_{9,24,28,28} + x_{10,24,28,29} + x_{23,24,28,30} + x_{24,24,28,31} + x_{25,24,28,32} + x_{26,24,28,1} + x_{27,24,28,2} = \\ = x_{28,17,2,24} + x_{28,19,3,24} + x_{28,22,4,24} + x_{28,23,5,24} \end{aligned} \quad (677)$$

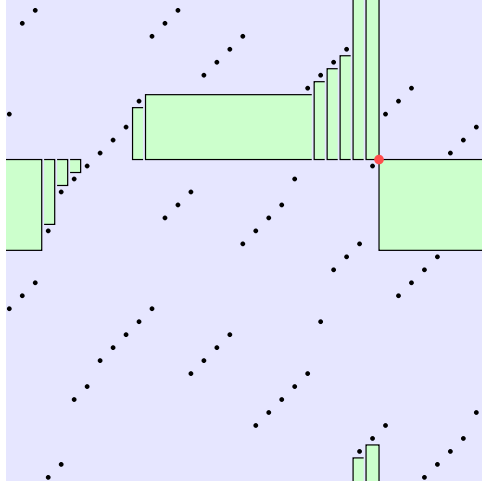

$$x_{0,27,28,28} = x_{28,4,29,27} + x_{28,14,30,27} + x_{28,15,31,27} + x_{28,16,32,27} + x_{28,17,33,27}$$

(678)

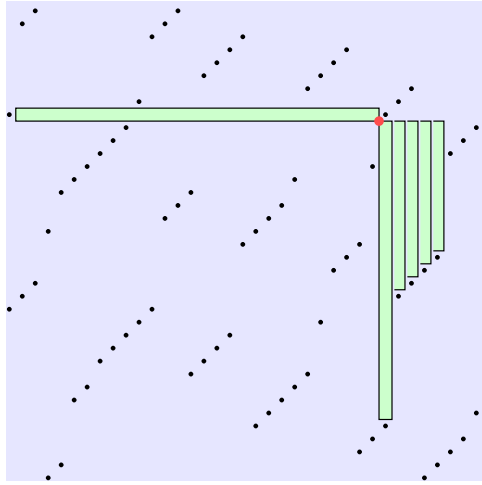

$$x_{0,27,28,28} + x_{9,24,28,28} = x_{28,28,29,3}$$

(679)

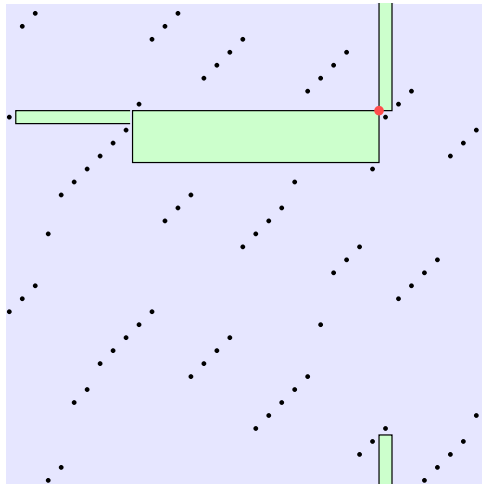

$$x_{10,24,28,29} = x_{28,29,30,3} \tag{680}$$

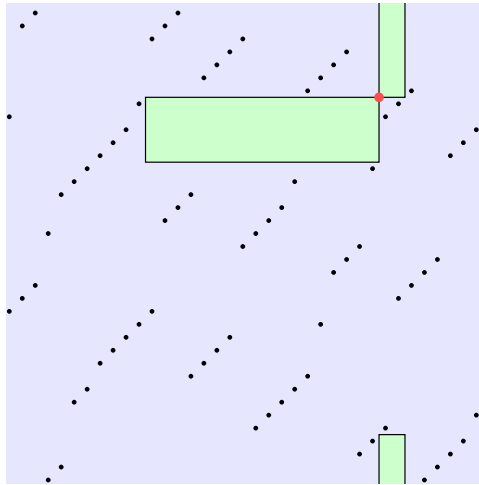

$$x_{23,24,28,30} = x_{28,30,31,3} \tag{681}$$

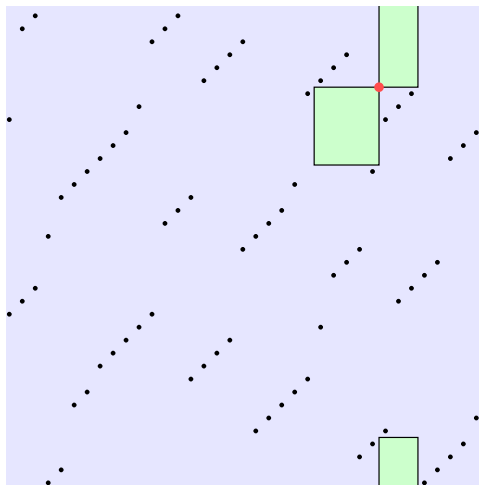

$$x_{24,24,28,31} = 0 \tag{682}$$

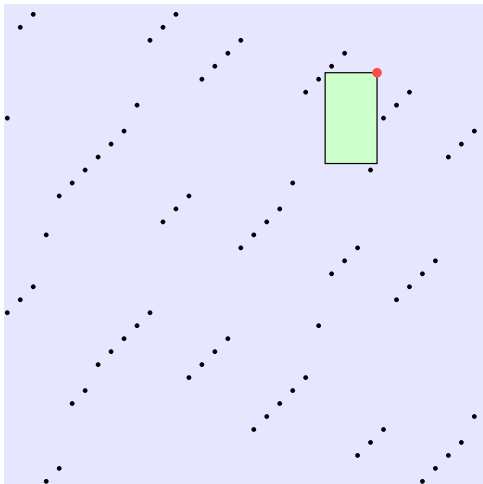

$$x_{25,24,28,32} = 0$$

(683)

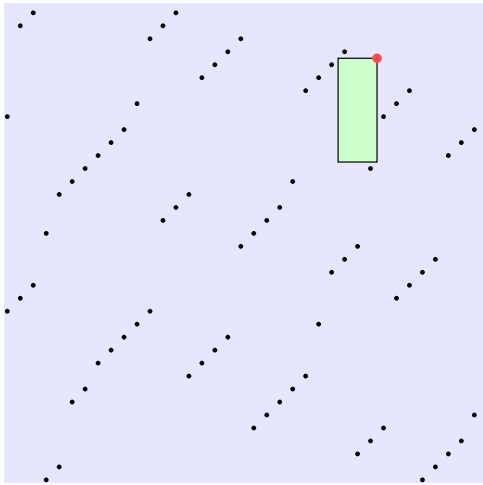

$$0 = x_{29,0,32,13}$$

(684)

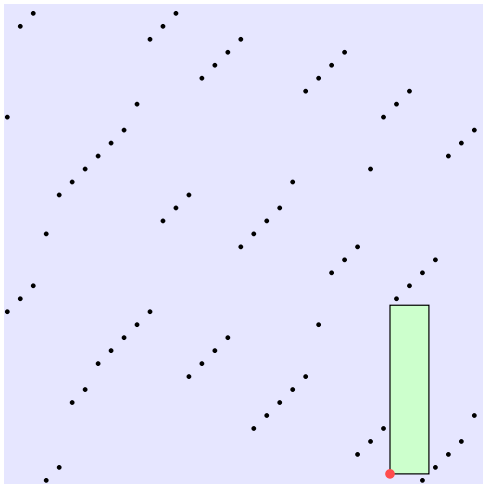



$$x_{26,28,29,1} = x_{29,1,33,13} \tag{685}$$

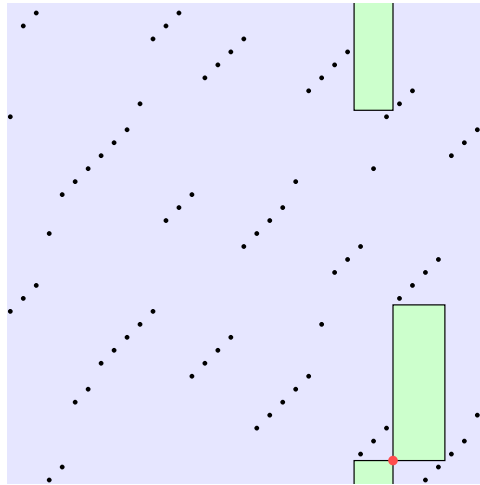

$$x_{27,28,29,2} = x_{29,2,34,13} \tag{686}$$

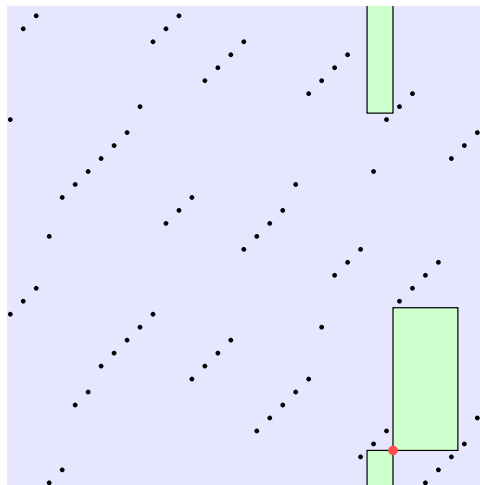

$$x_{28,28,29,3} = x_{29,3,18,4} + x_{29,3,35,13} \tag{687}$$

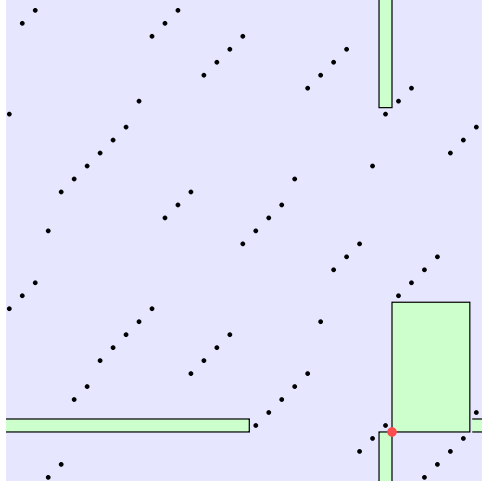

$$x_{24,4,29,15} + x_{25,4,29,16} + x_{26,4,29,17} + x_{27,4,29,23} + x_{28,4,29,27} = x_{29,3,18,4} \quad (688)$$

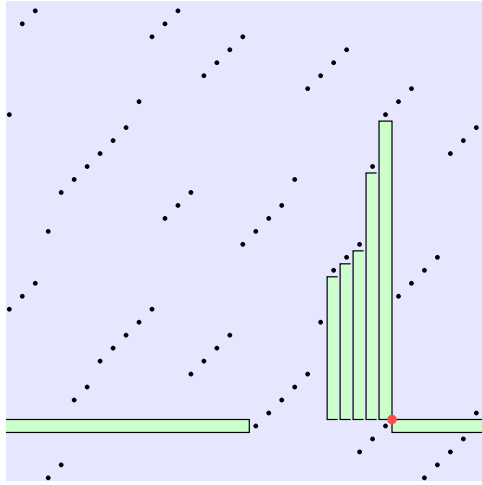

$$x_{11,12,29,15} = 0 \quad (689)$$

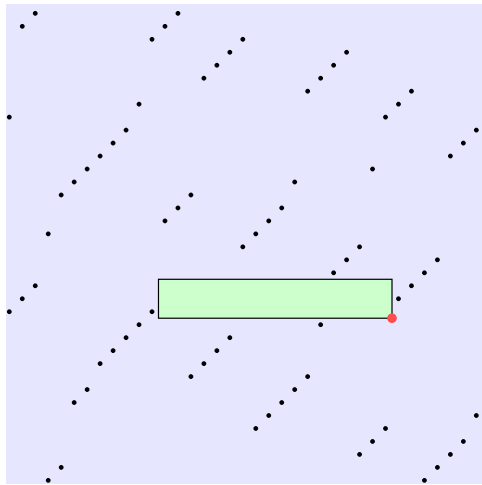

$$x_{1,13,29,14} + x_{2,13,29,15} = x_{29,0,32,13} + x_{29,1,33,13} + x_{29,2,34,13} + x_{29,3,35,13} + x_{29,29,30,13} + x_{29,30,31,13} \quad (690)$$

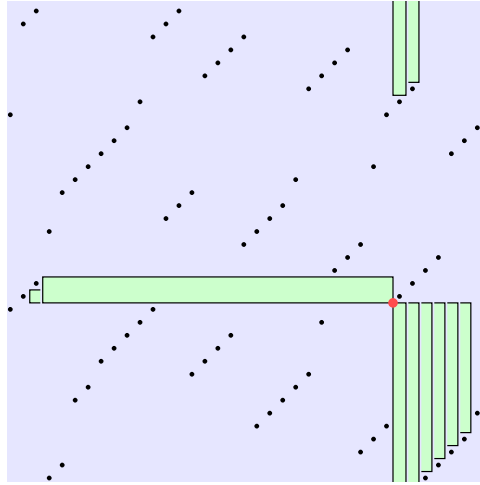

$$x_{1,13,29,14} = x_{29,14,30,28} \quad (691)$$

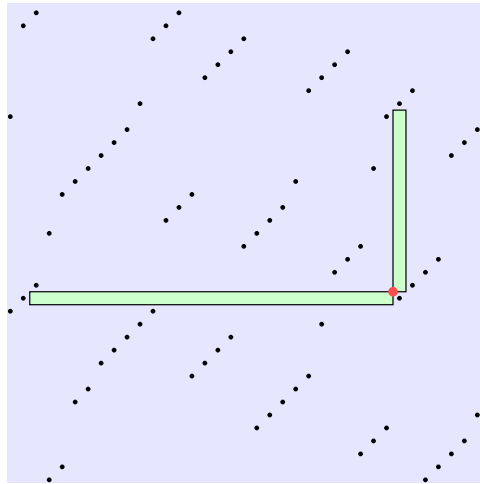

$$x_{2,13,29,15} + x_{11,12,29,15} + x_{24,4,29,15} = x_{29,15,31,28} \quad (692)$$

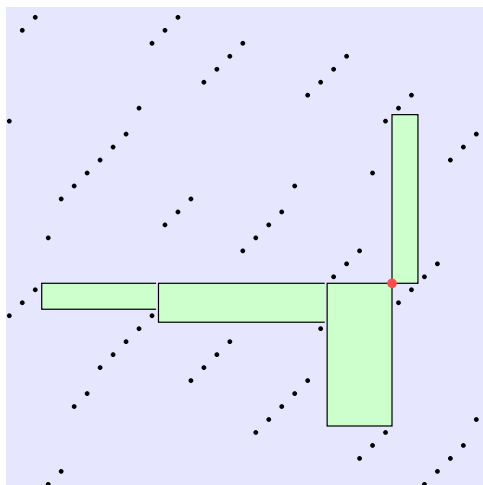

$$x_{25,4,29,16} = x_{29,16,32,28}$$

(693)

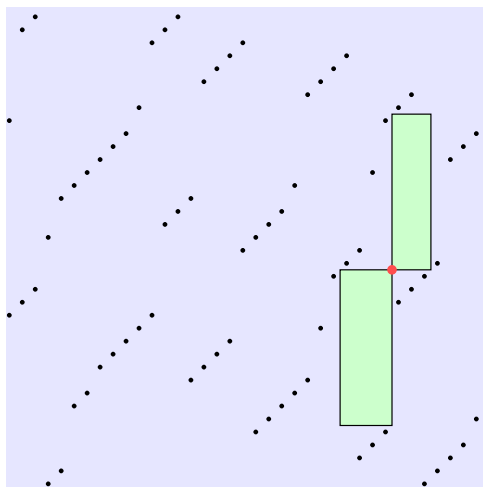

$$x_{26,4,29,17} = x_{29,17,33,28}$$

(694)

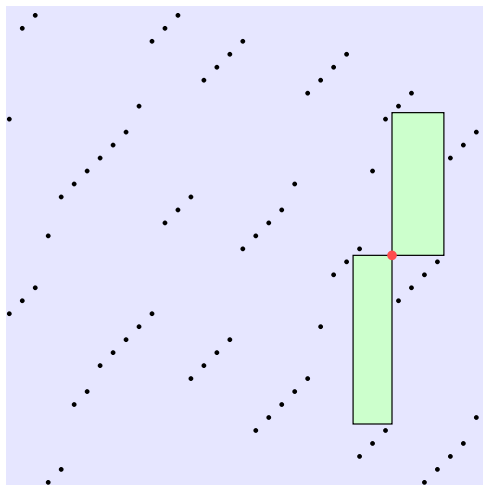

$$x_{27,4,29,23} = 0$$

(695)

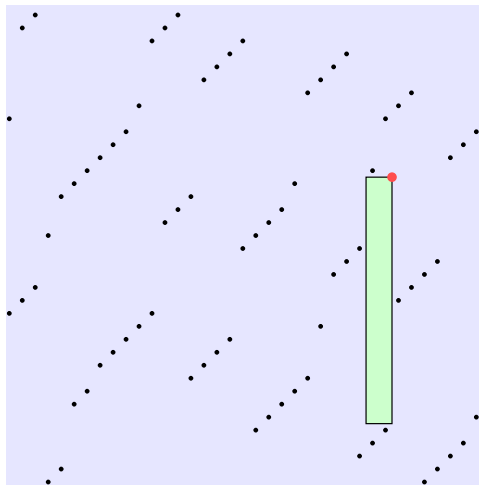

$$0 = x_{29,25,34,28}$$

(696)

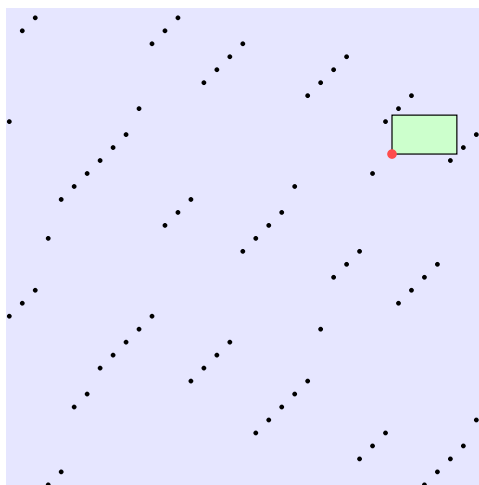

$$0 = x_{29,26,35,28}$$

(697)

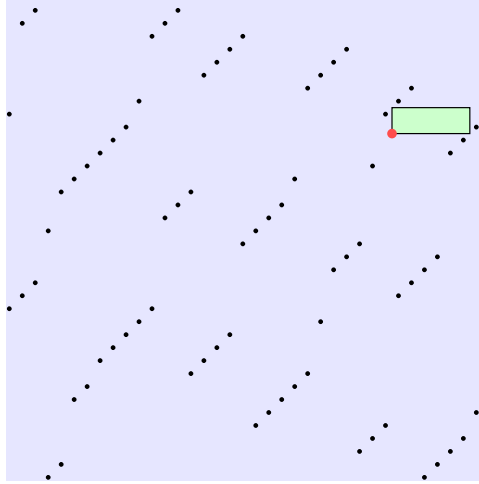

$$x_{28,4,29,27} = x_{29,27,36,28}$$

(698)

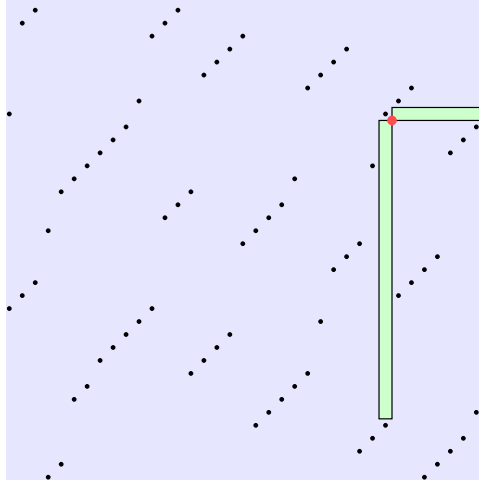

$$\begin{aligned} & x_{10,28,29,29} + x_{23,28,29,30} + x_{24,28,29,31} + x_{25,28,29,32} + x_{26,28,29,1} + x_{27,28,29,2} + x_{28,28,29,3} = \\ & = x_{29,14,30,28} + x_{29,15,31,28} + x_{29,16,32,28} + x_{29,17,33,28} + x_{29,25,34,28} + x_{29,26,35,28} + x_{29,27,36,28} \end{aligned} \quad (699)$$

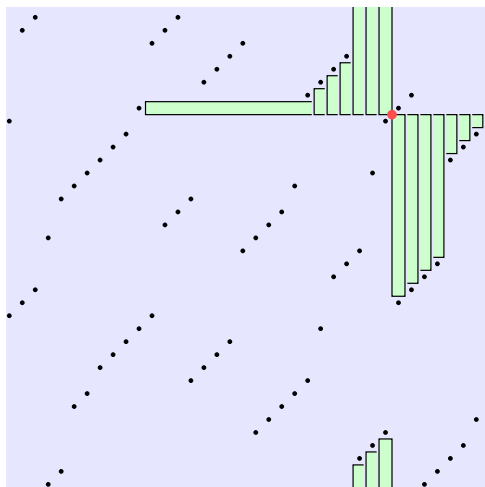

$$x_{10,28,29,29} = x_{29,29,30,13}$$

(700)

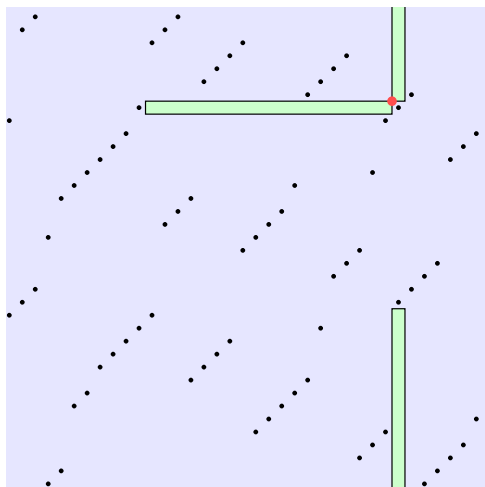

$$x_{23,28,29,30} = x_{29,30,31,13}$$

(701)

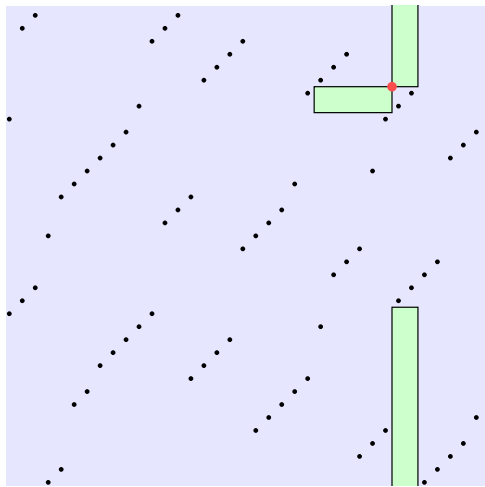

$$x_{24,28,29,31} = 0 \tag{702}$$

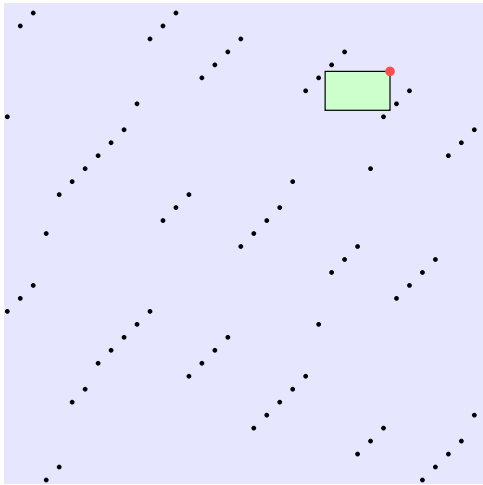

$$x_{25,28,29,32} = 0 \tag{703}$$

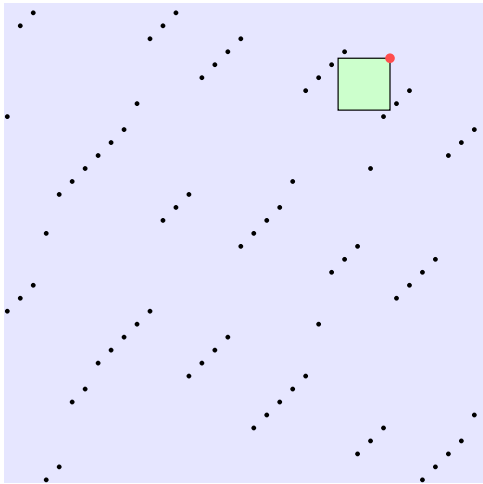

$$0 = x_{30,0,32,14} \tag{704}$$



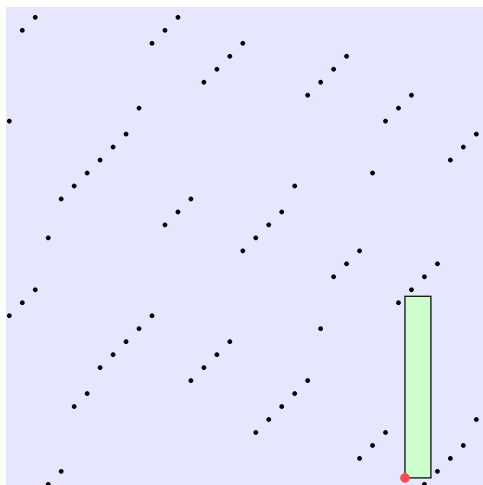

$$x_{26,29,30,1} = x_{30,1,33,14}$$

(705)

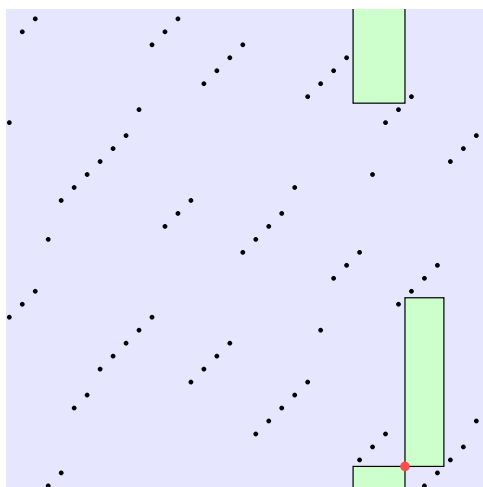

$$x_{27,29,30,2} = x_{30,2,34,14}$$

(706)

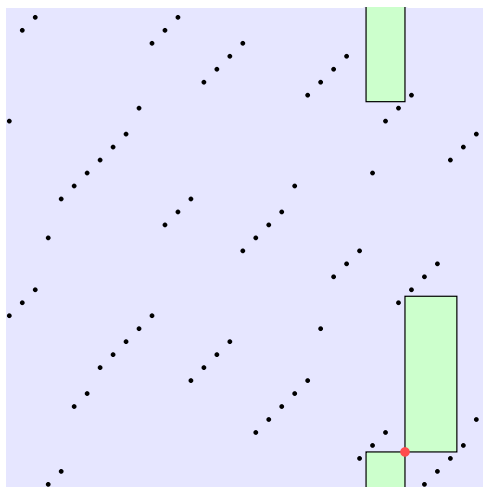

$$x_{28,29,30,3} = x_{30,3,35,14} \tag{707}$$

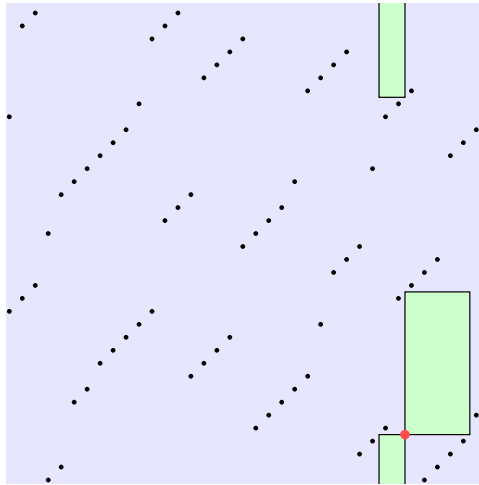

$$0 = x_{30,5,36,14} \tag{708}$$

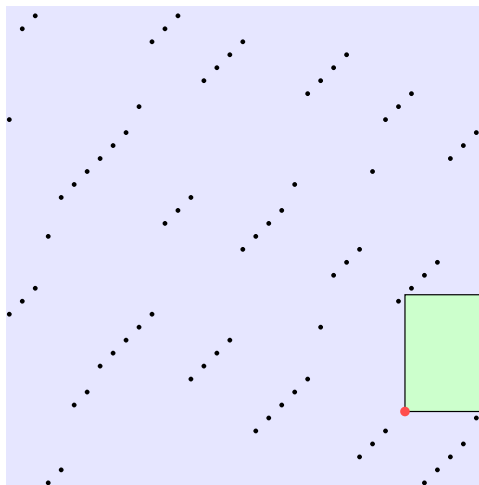

$$x_{29,29,30,13} = x_{30,13,0,14} \tag{709}$$

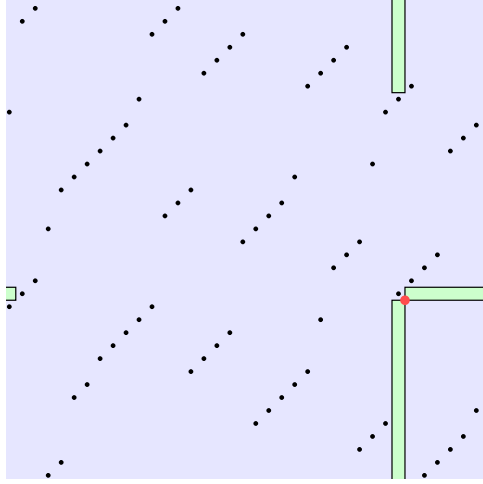

$$\begin{aligned}
 & x_{2,14,30,15} + x_{25,14,30,16} + x_{26,14,30,17} + x_{27,14,30,23} + x_{28,14,30,27} + x_{29,14,30,28} = \\
 & = x_{30,0,32,14} + x_{30,1,33,14} + x_{30,2,34,14} + x_{30,3,35,14} + x_{30,5,36,14} + x_{30,13,0,14} + x_{30,30,31,14} \quad (710)
 \end{aligned}$$

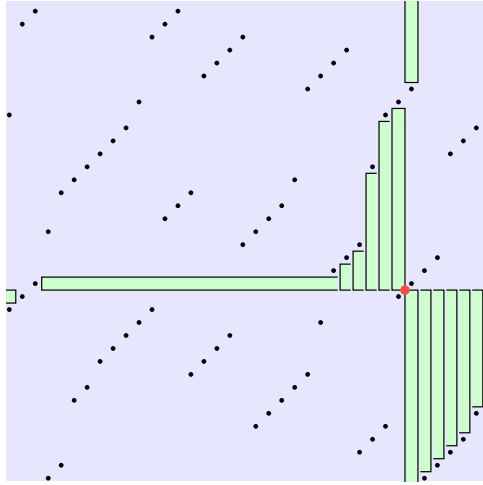

$$x_{2,14,30,15} = x_{30,15,31,29} \quad (711)$$

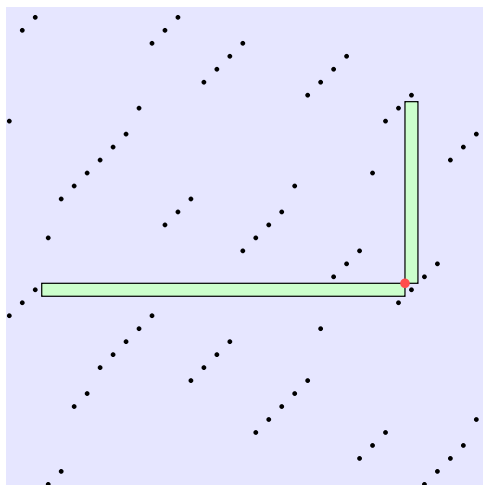

$$x_{25,14,30,16} = x_{30,16,32,29}$$

(712)

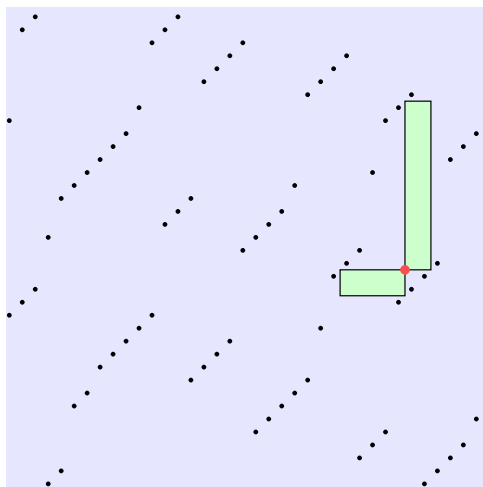

$$x_{26,14,30,17} = x_{30,17,33,29}$$

(713)

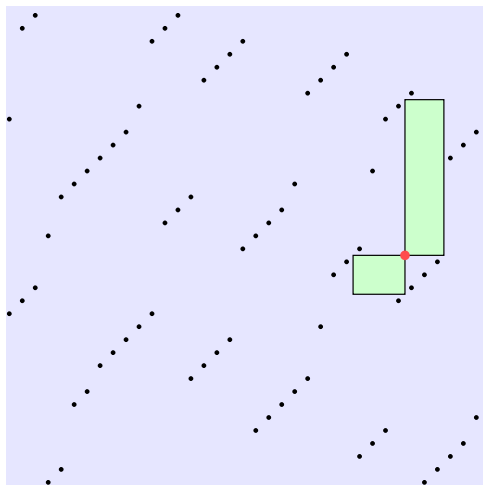

$$x_{27,14,30,23} = 0 \tag{714}$$

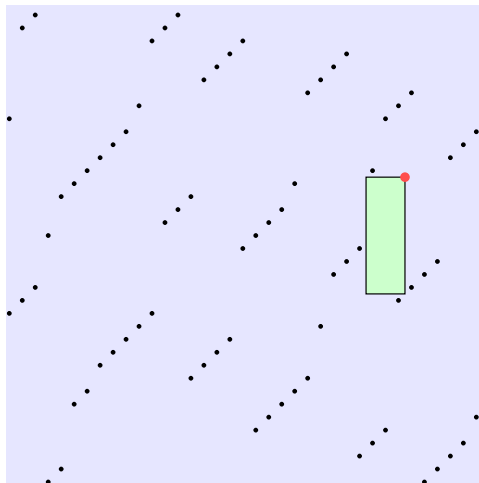

$$0 = x_{30,25,34,29} \tag{715}$$

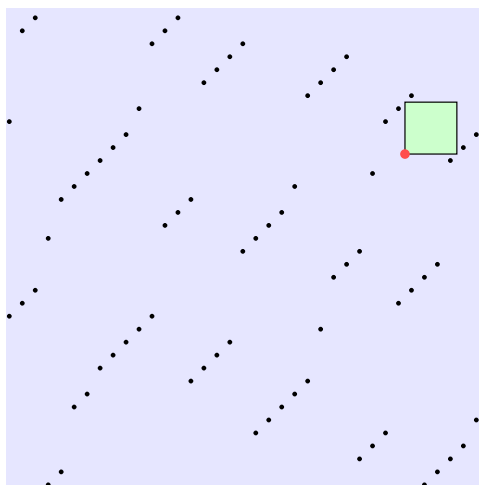

$$0 = x_{30,26,35,29} \tag{716}$$

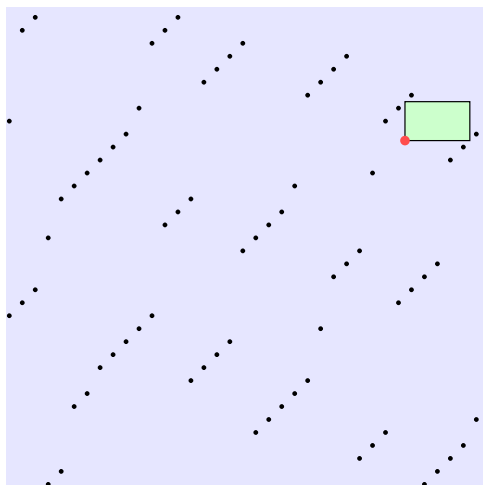

$$x_{28,14,30,27} = x_{30,27,36,29}$$

(717)

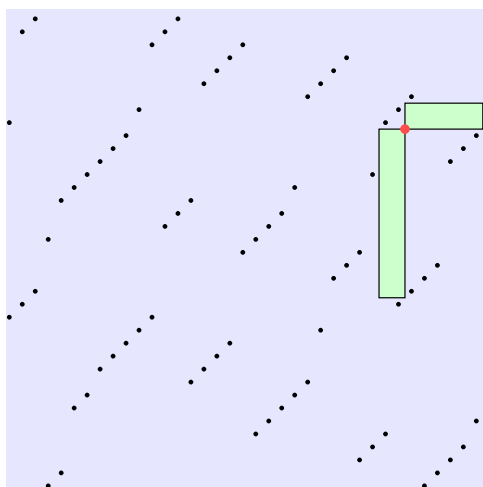

$$x_{29,14,30,28} = x_{30,28,9,29}$$

(718)

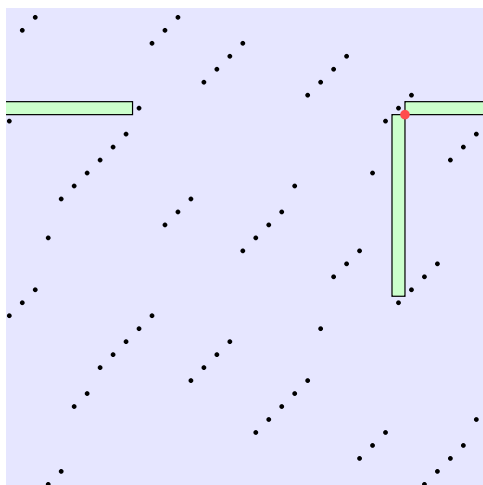

$$\begin{aligned}
& x_{23,29,30,30} + x_{24,29,30,31} + x_{25,29,30,32} + x_{26,29,30,1} + x_{27,29,30,2} + x_{28,29,30,3} + x_{29,29,30,13} = \\
& = x_{30,15,31,29} + x_{30,16,32,29} + x_{30,17,33,29} + x_{30,25,34,29} + x_{30,26,35,29} + x_{30,27,36,29} + x_{30,28,9,29} \quad (719)
\end{aligned}$$

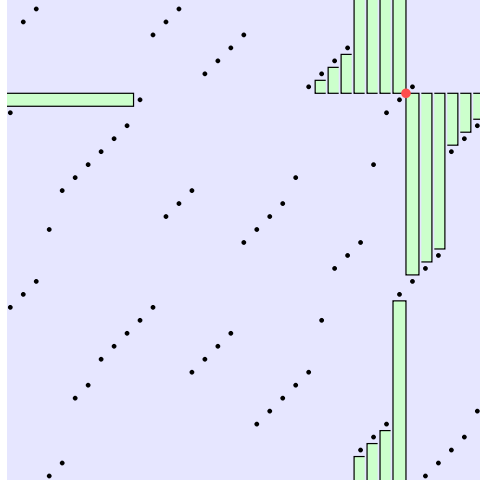

$$x_{23,29,30,30} = x_{30,30,31,14} \quad (720)$$

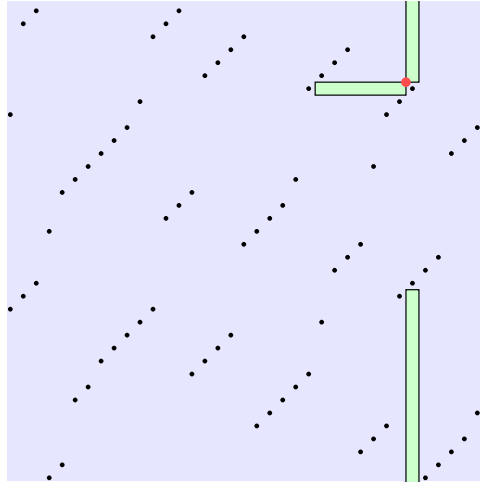

$$x_{24,29,30,31} = 0 \quad (721)$$

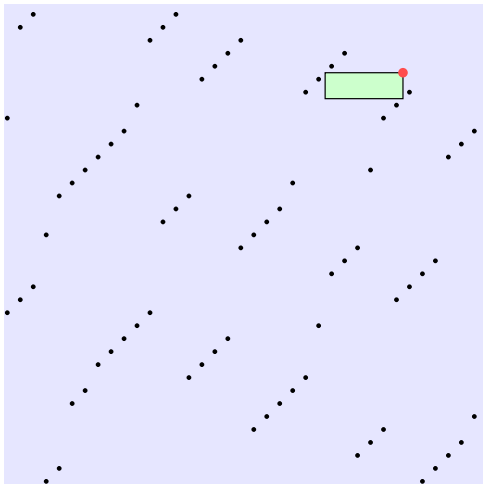

$$x_{25,29,30,32} = 0$$

(722)

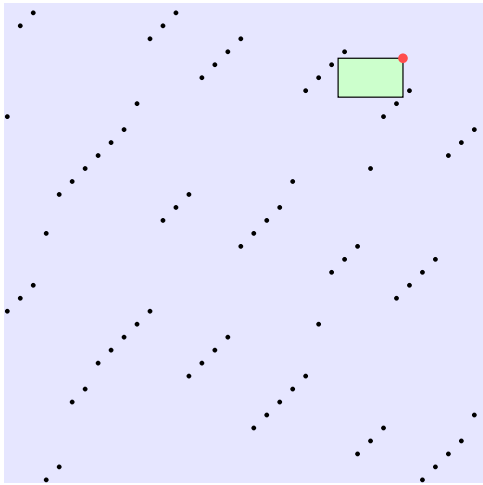

$$x_{3,36,31,0} = x_{31,0,32,15}$$

(723)

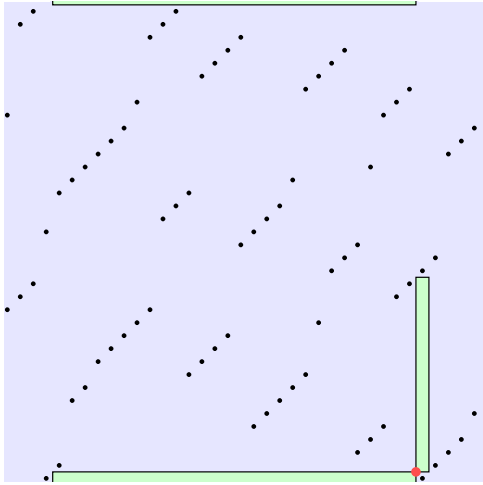



$$x_{4,36,31,1} + x_{13,34,31,1} + x_{18,33,31,1} + x_{26,30,31,1} = x_{31,1,33,15} \quad (724)$$

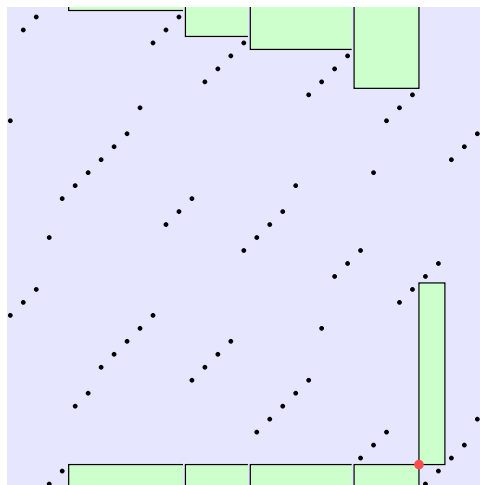

$$x_{27,30,31,2} = x_{31,2,34,15} \quad (725)$$

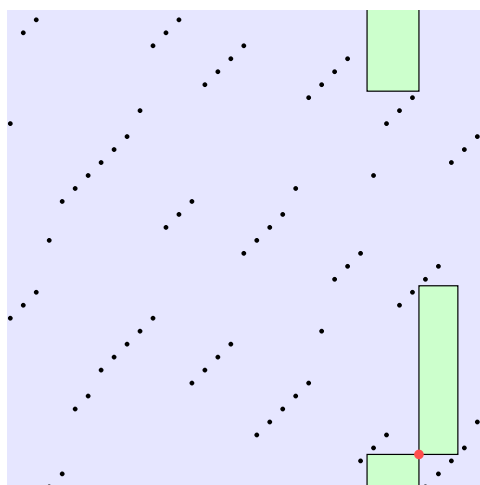

$$x_{28,30,31,3} = x_{31,3,35,15} \quad (726)$$

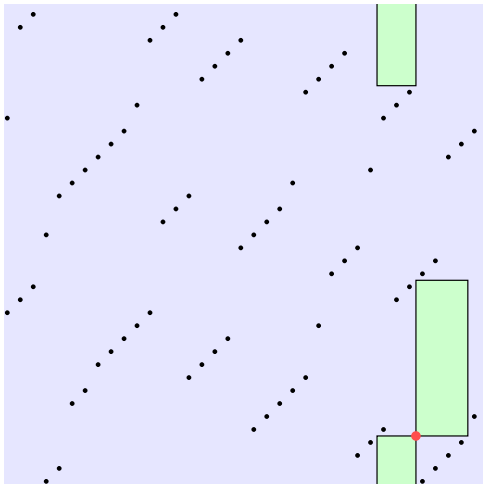

$$0 = x_{31,5,36,15}$$

(727)

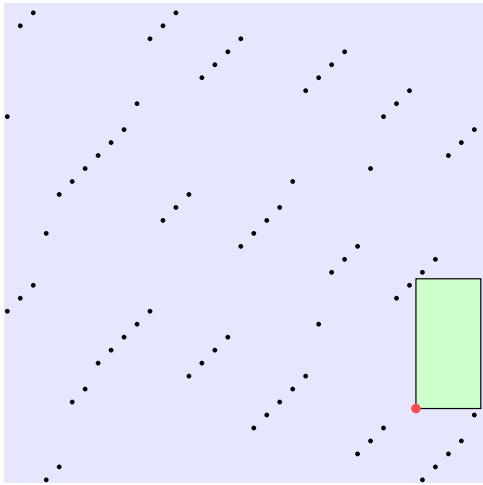

$$x_{29,30,31,13} = x_{31,13,0,15}$$

(728)

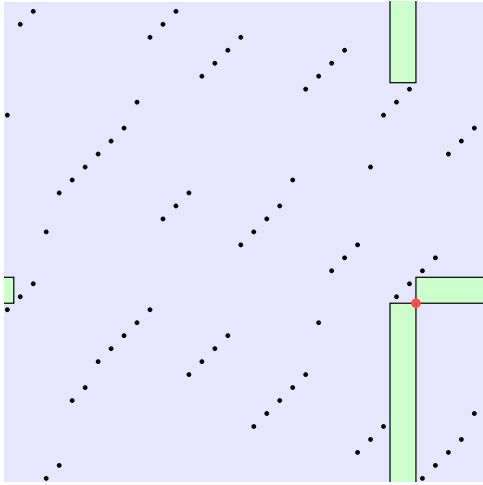

$$x_{30,30,31,14} = x_{31,14,1,15} \quad (729)$$

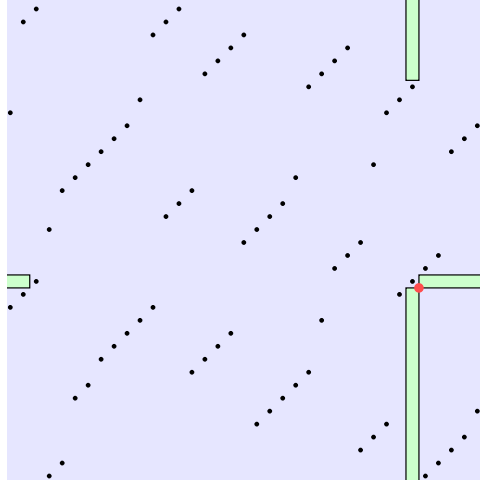

$$\begin{aligned} x_{25,15,31,16} + x_{26,15,31,17} + x_{27,15,31,23} + x_{28,15,31,27} + x_{29,15,31,28} + x_{30,15,31,29} = \\ = x_{31,0,32,15} + x_{31,1,33,15} + x_{31,2,34,15} + x_{31,3,35,15} + x_{31,5,36,15} + x_{31,13,0,15} + x_{31,14,1,15} \end{aligned} \quad (730)$$

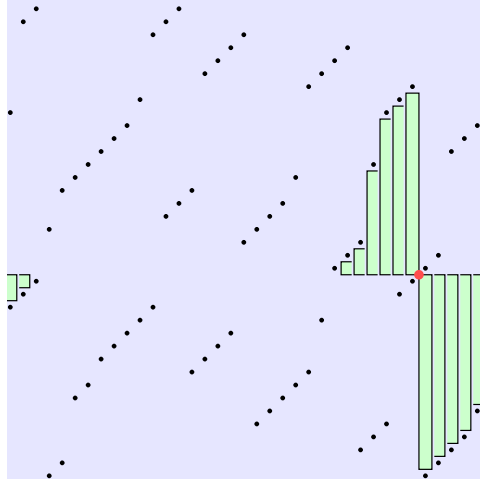

$$x_{25,15,31,16} = x_{31,16,32,36} \quad (731)$$

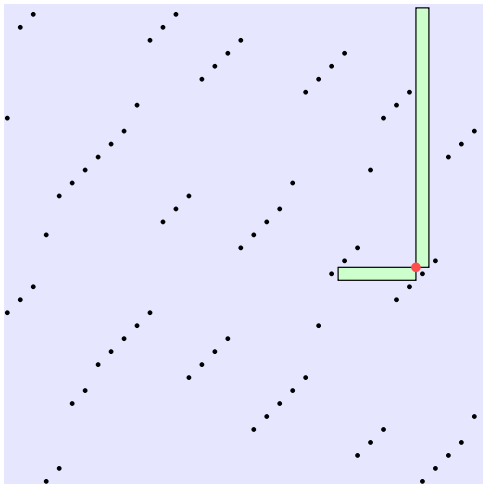

$$x_{26,15,31,17} = x_{31,17,33,36}$$

(732)

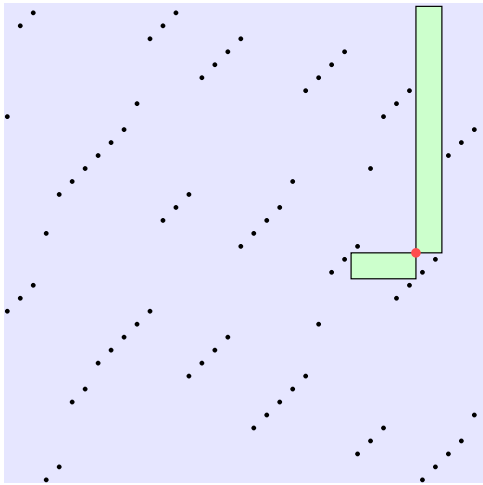

$$x_{27,15,31,23} = 0$$

(733)

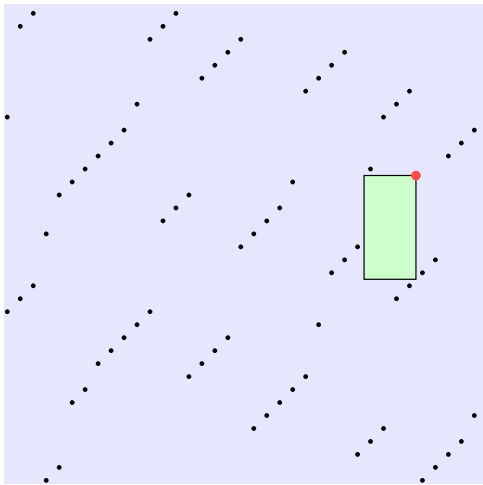

$$0 = x_{31,25,34,36}$$

(734)

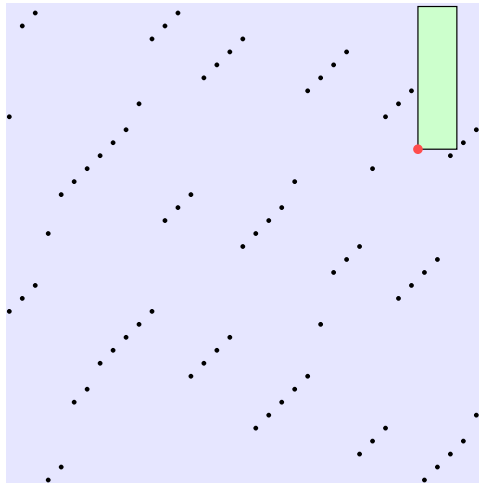

$$0 = x_{31,26,35,36}$$

(735)

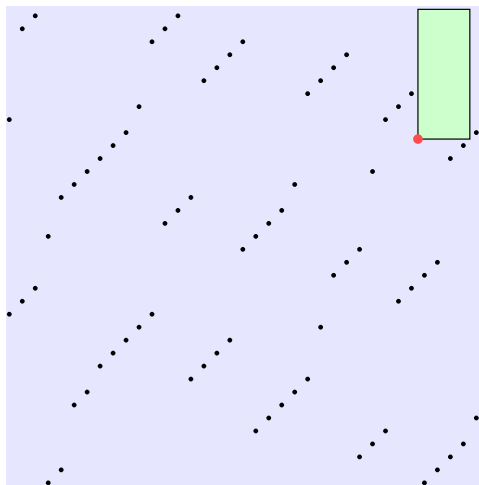

$$x_{28,15,31,27} = x_{31,27,36,36}$$

(736)

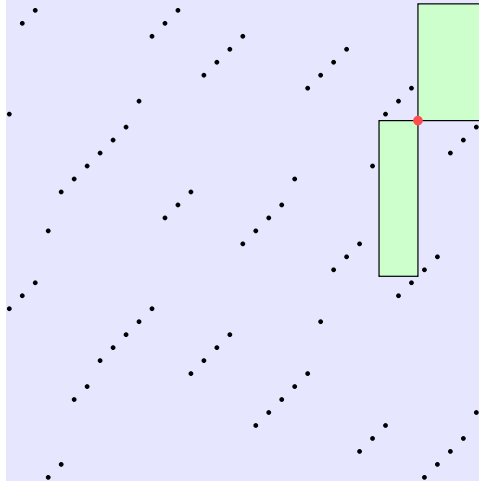

$$x_{29,15,31,28} = x_{31,28,0,36} + x_{31,28,9,34}$$

(737)

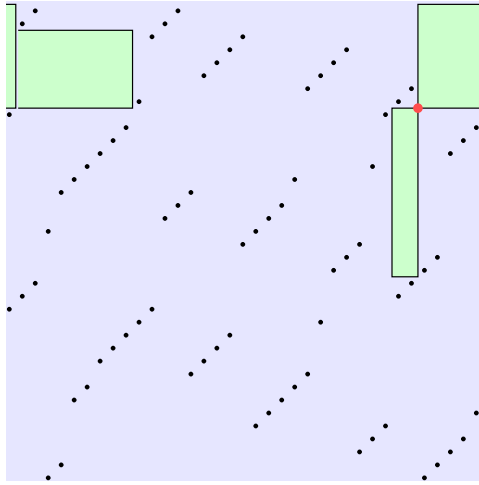

$$x_{30,15,31,29} = x_{31,29,10,34} + x_{31,29,14,33} + x_{31,29,22,30}$$

(738)

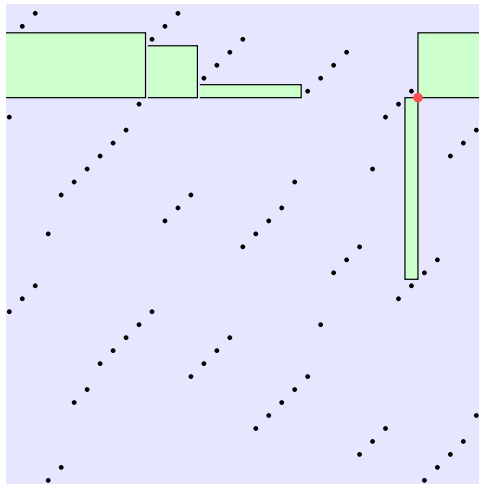

$$x_{26,30,31,1} + x_{27,30,31,2} + x_{28,30,31,3} + x_{29,30,31,13} + x_{30,30,31,14} = x_{31,29,22,30} \quad (739)$$

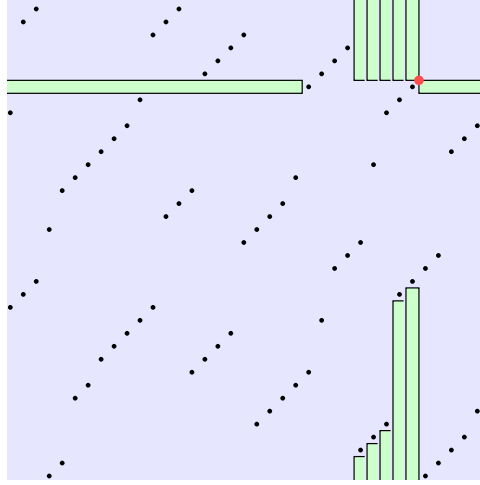

$$x_{18,33,31,1} = x_{31,29,14,33} \quad (740)$$

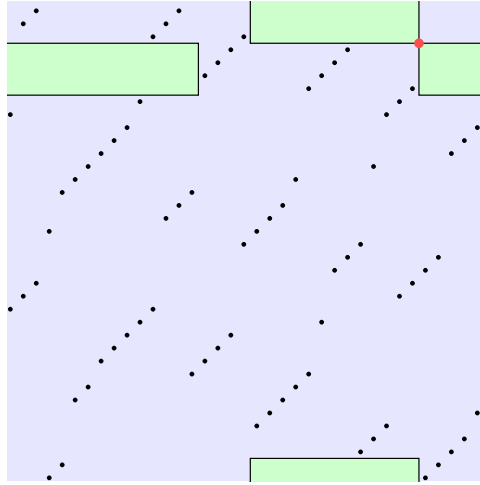

$$x_{13,34,31,1} = x_{31,28,9,34} + x_{31,29,10,34} \quad (741)$$

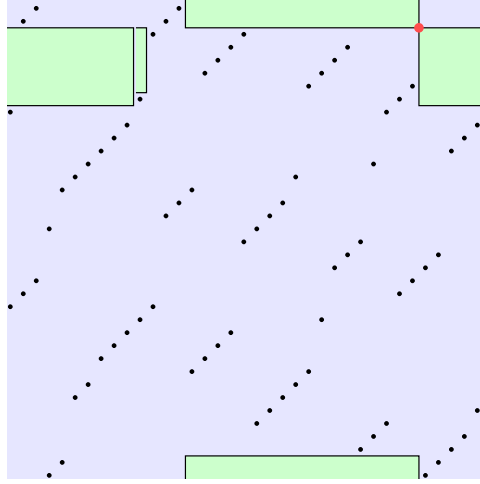

$$x_{3,36,31,0} + x_{4,36,31,1} = x_{31,16,32,36} + x_{31,17,33,36} + x_{31,25,34,36} + x_{31,26,35,36} + x_{31,27,36,36} + x_{31,28,0,36} \quad (742)$$

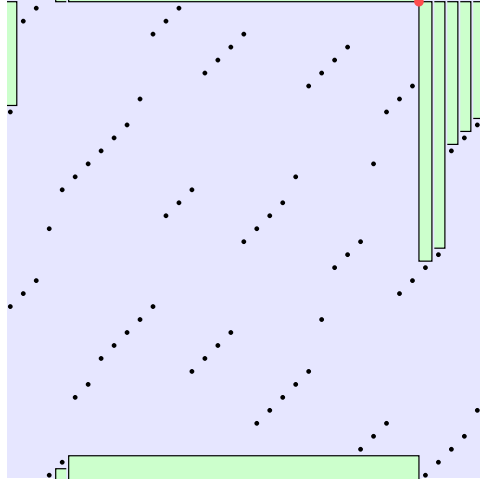

$$\begin{aligned} x_{4,0,32,1} + x_{27,0,32,2} + x_{28,0,32,3} + x_{29,0,32,13} + x_{30,0,32,14} + x_{31,0,32,15} = \\ = x_{32,17,33,0} + x_{32,25,34,0} + x_{32,26,35,0} + x_{32,27,36,0} + x_{32,28,0,0} + x_{32,35,1,0} + x_{32,36,2,0} \end{aligned} \quad (743)$$



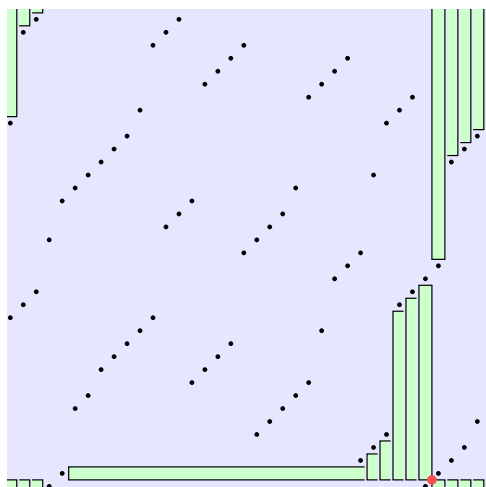

$$x_{4,0,32,1} = x_{32,1,33,16}$$

(744)

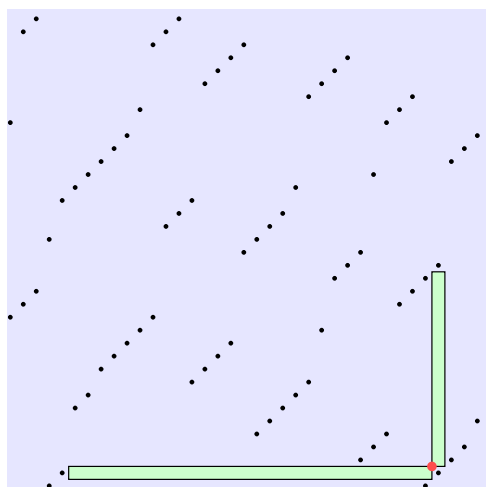

$$x_{27,0,32,2} = x_{32,2,34,16}$$

(745)

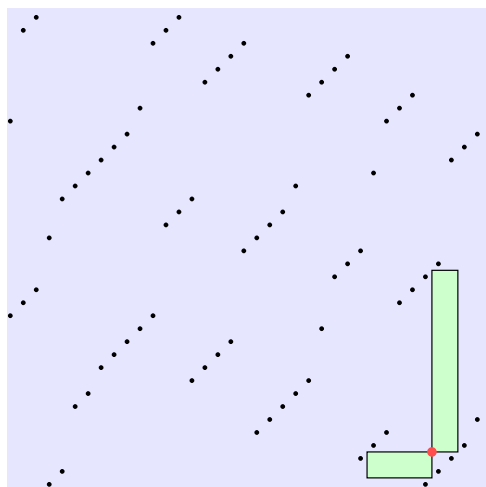

$$x_{28,0,32,3} = x_{32,3,35,16}$$

(746)

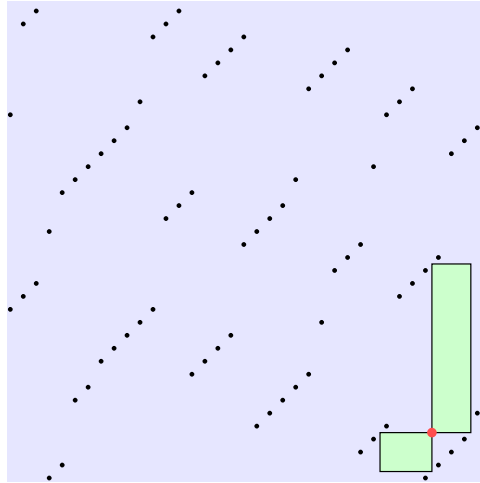

$$0 = x_{32,5,36,16}$$

(747)

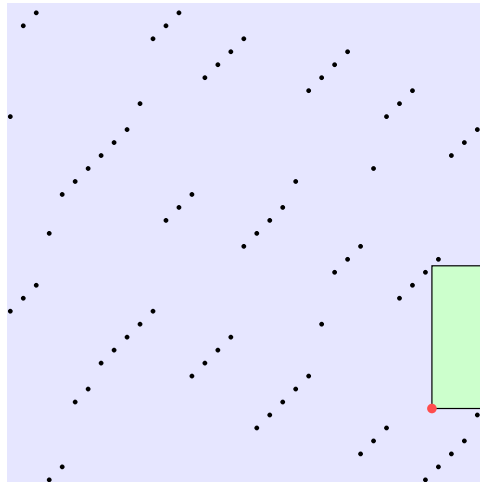

$$x_{29,0,32,13} = x_{32,13,0,16}$$

(748)

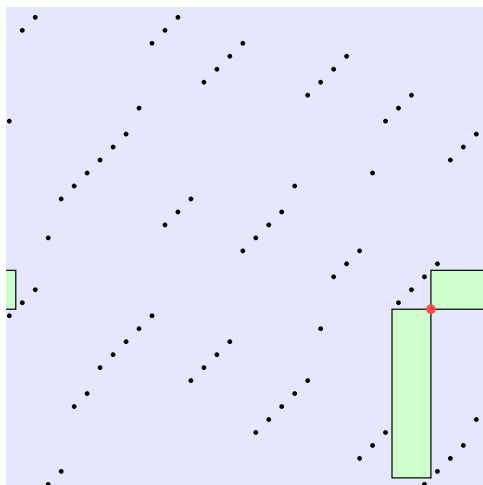

$$x_{30,0,32,14} = x_{32,14,1,16}$$

(749)

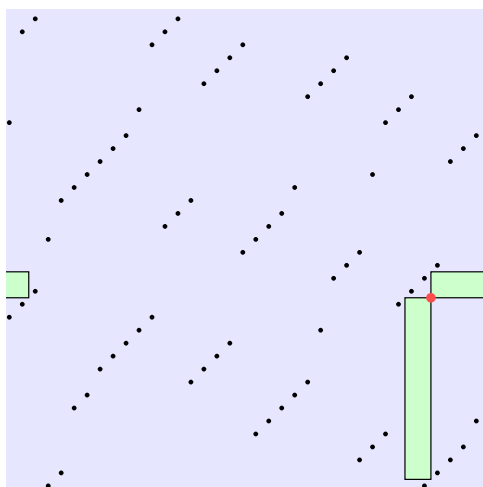

$$x_{31,0,32,15} = x_{32,15,24,16}$$

(750)

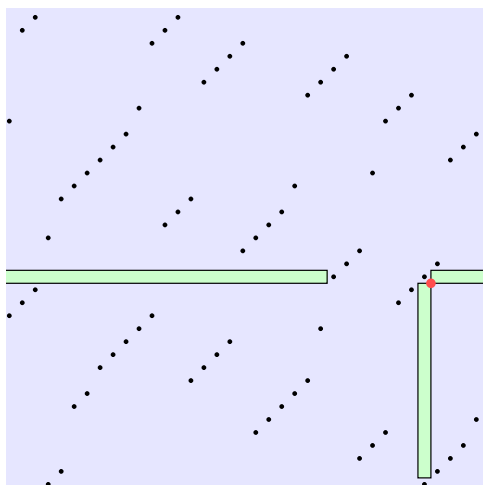

$$\begin{aligned}
& x_{26,16,32,17} + x_{27,16,32,23} + x_{28,16,32,27} + x_{29,16,32,28} + x_{30,16,32,29} + x_{31,16,32,36} = \\
& = x_{32,1,33,16} + x_{32,2,34,16} + x_{32,3,35,16} + x_{32,5,36,16} + x_{32,13,0,16} + x_{32,14,1,16} + x_{32,15,24,16} \quad (751)
\end{aligned}$$

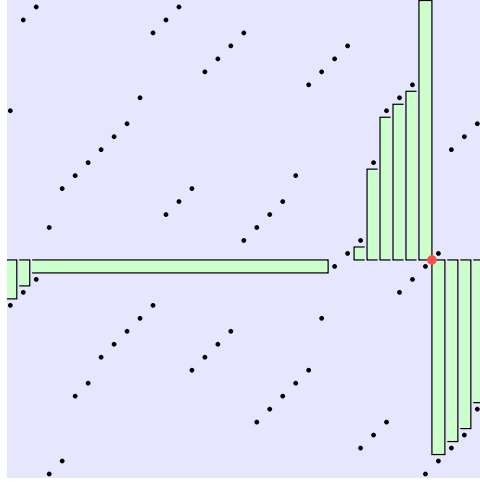

$$x_{26,16,32,17} = x_{32,17,33,0} \quad (752)$$

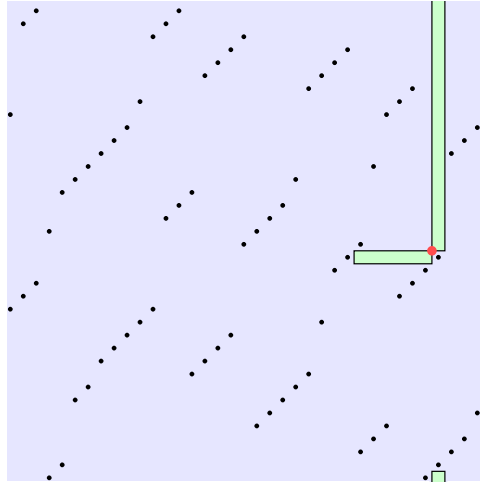

$$x_{27,16,32,23} = 0 \quad (753)$$

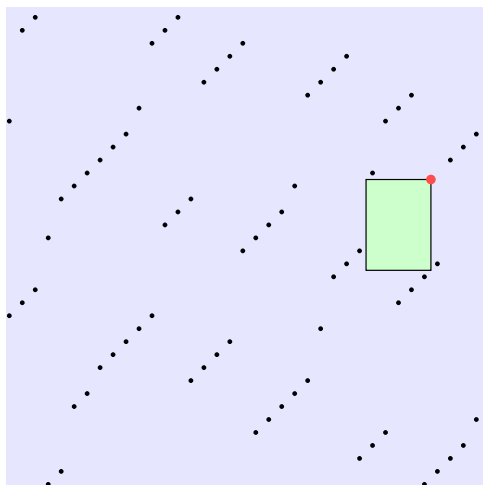

$$0 = x_{32,25,34,0}$$

(754)

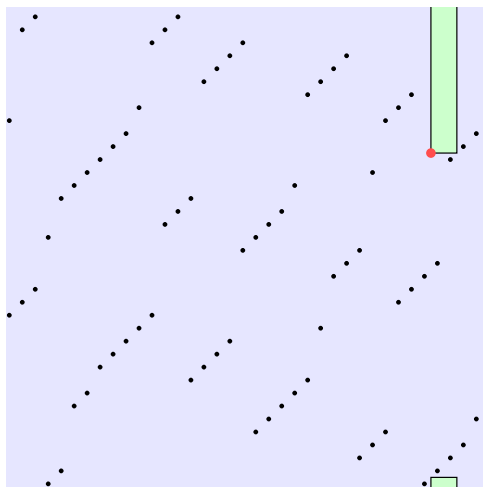

$$0 = x_{32,26,35,0}$$

(755)

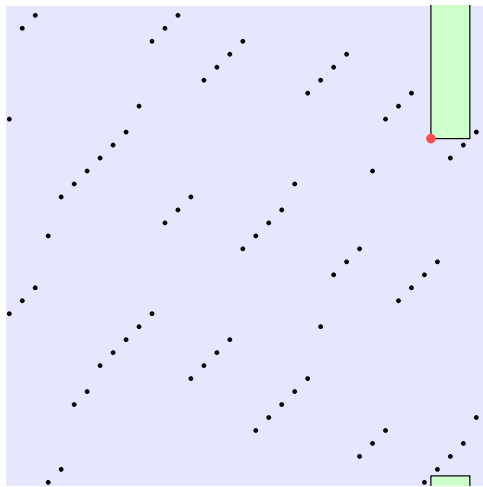

$$x_{28,16,32,27} = x_{32,27,36,0} \tag{756}$$

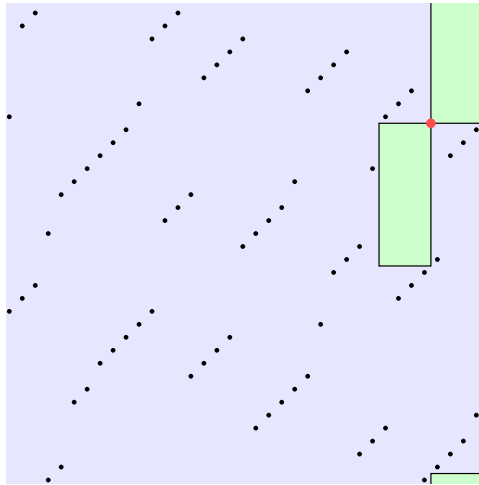

$$x_{29,16,32,28} = x_{32,28,0,0} \tag{757}$$

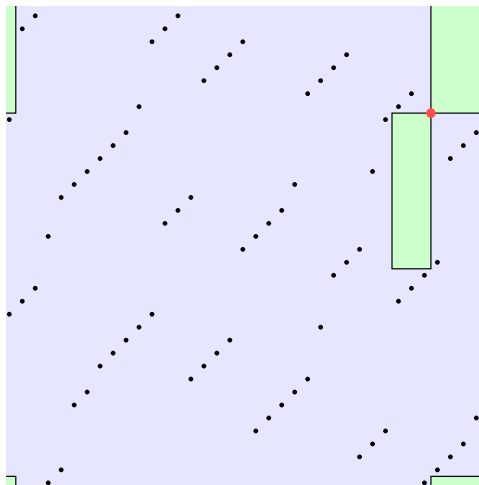

$$x_{30,16,32,29} = 0 \tag{758}$$

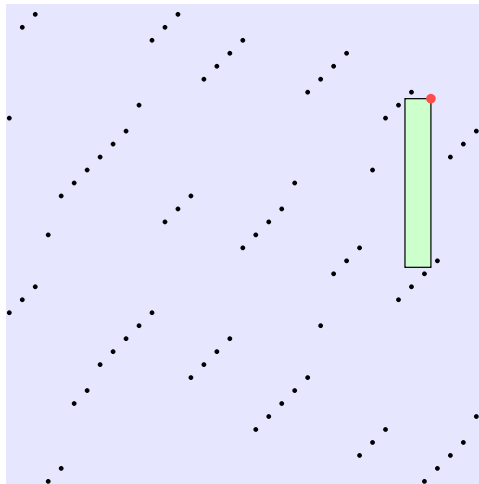

$$0 = x_{32,35,1,0}$$

(759)

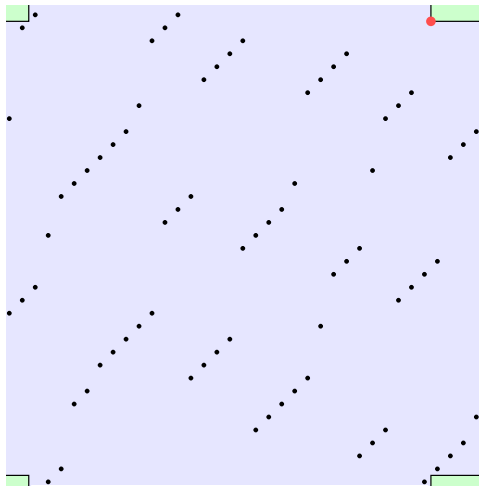

$$x_{31,16,32,36} = x_{32,36,2,0}$$

(760)

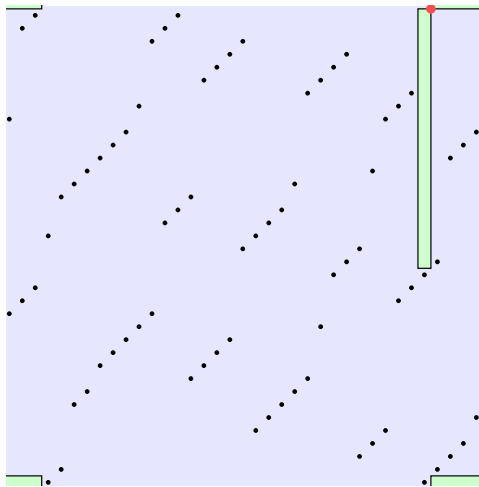

$$x_{32,17,33,0} = x_{33,0,3,1}$$

(761)

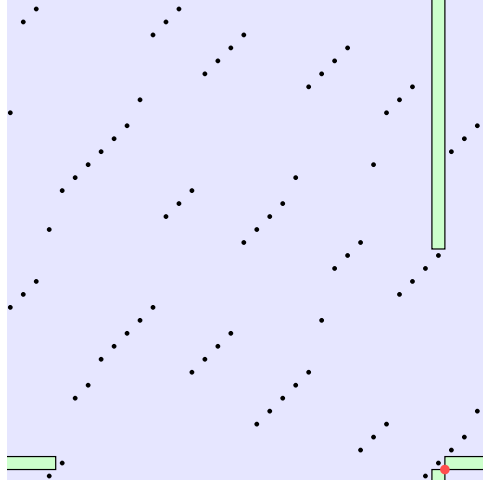

$$\begin{aligned} x_{27,1,33,2} + x_{28,1,33,3} + x_{29,1,33,13} + x_{30,1,33,14} + x_{31,1,33,15} + x_{32,1,33,16} = \\ = x_{33,0,3,1} + x_{33,25,34,1} + x_{33,26,35,1} + x_{33,27,36,1} + x_{33,28,0,1} + x_{33,35,1,1} + x_{33,36,2,1} \end{aligned} \quad (762)$$

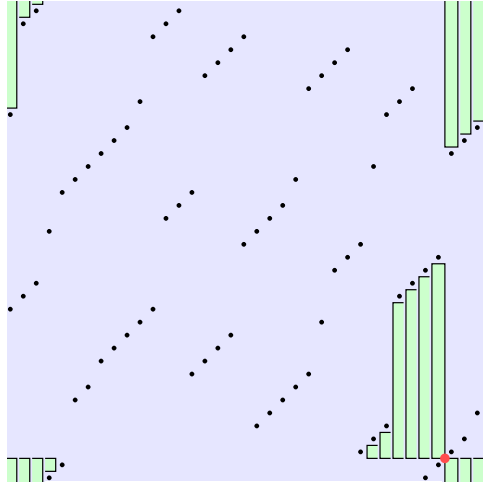

$$x_{27,1,33,2} = x_{33,2,34,24}$$

(763)



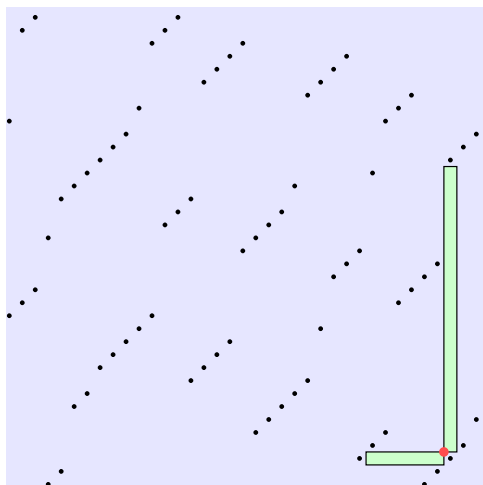

$$x_{28,1,33,3} = x_{33,3,35,24}$$

(764)

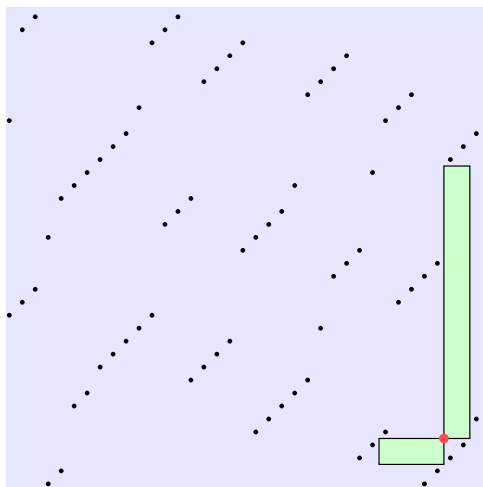

$$0 = x_{33,5,36,24}$$

(765)

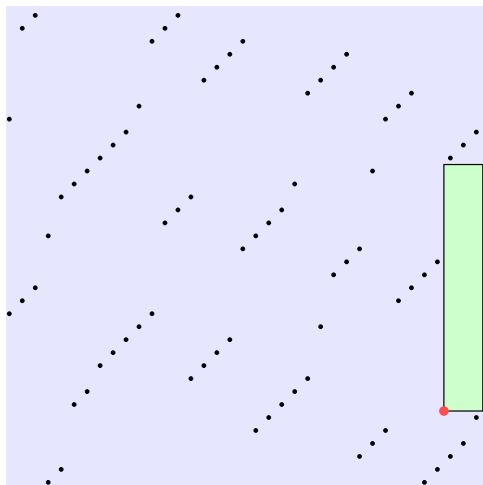

$$x_{29,1,33,13} = x_{33,13,0,24} \quad (766)$$

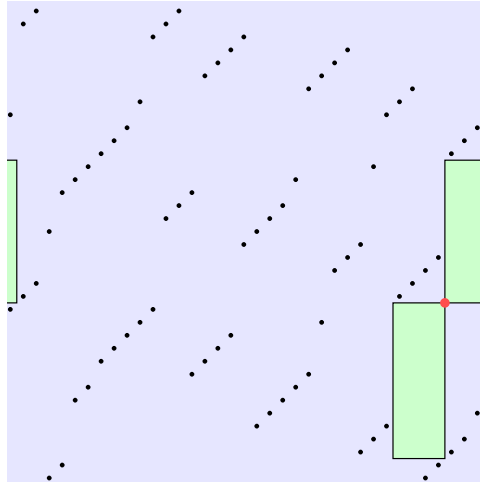

$$x_{30,1,33,14} = x_{33,14,1,24} \quad (767)$$

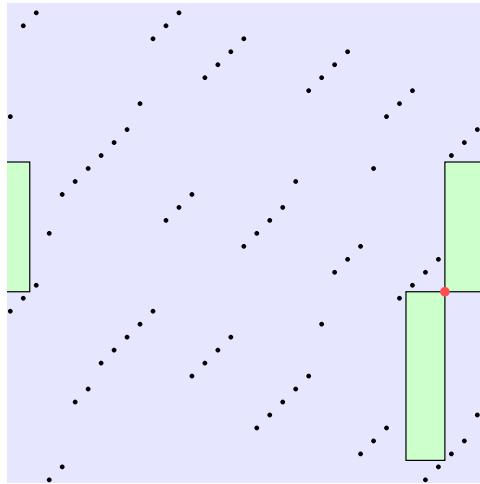

$$x_{31,1,33,15} = x_{33,15,2,24} + x_{33,15,17,18} + x_{33,15,24,17} \quad (768)$$

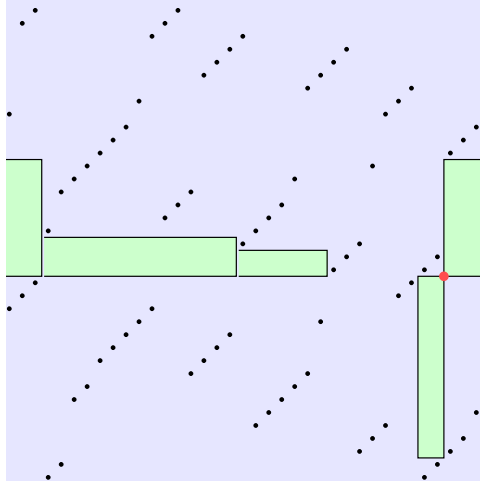

$$x_{32,1,33,16} = x_{33,16,25,17}$$

(769)

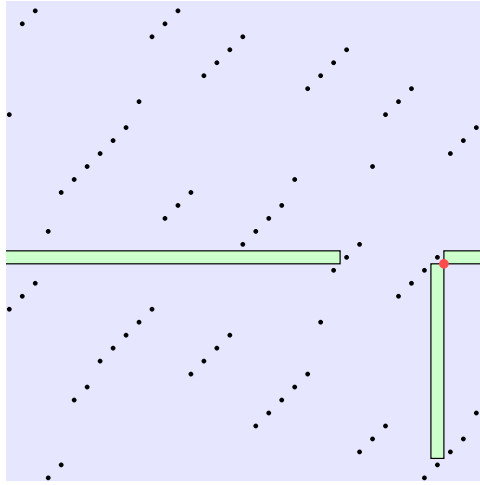

$$x_{28,17,33,27} + x_{29,17,33,28} + x_{30,17,33,29} + x_{31,17,33,36} + x_{32,17,33,0} = x_{33,15,24,17} + x_{33,16,25,17}$$

(770)

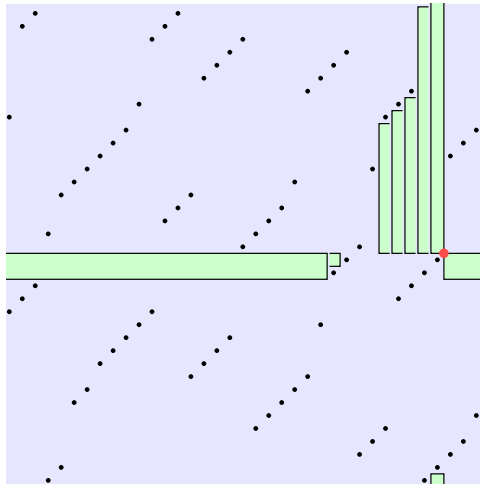

$$0 = x_{33,15,17,18}$$

(771)

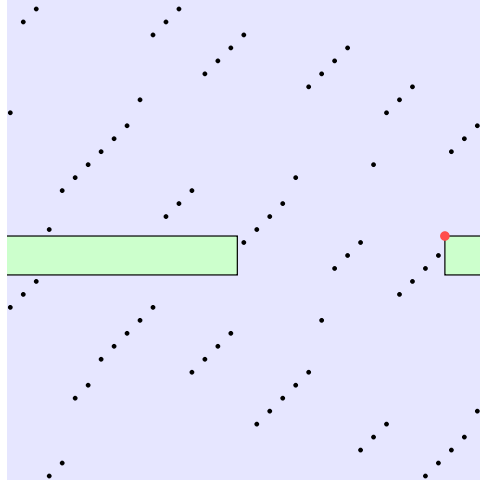

$$x_{7,24,33,25} + x_{8,24,33,26} + x_{9,24,33,27} = x_{33,2,34,24} + x_{33,3,35,24} + x_{33,5,36,24} + x_{33,13,0,24} + x_{33,14,1,24} + x_{33,15,2,24}$$

(772)

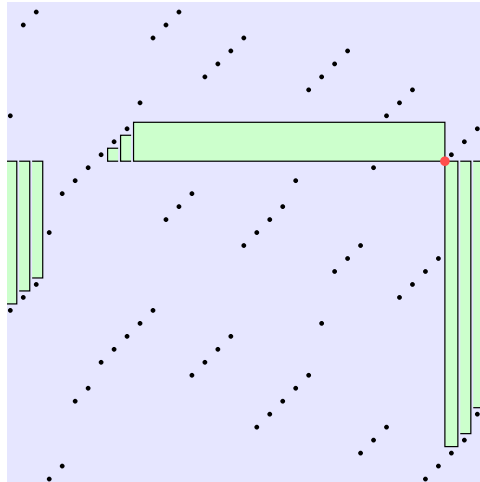

$$x_{7,24,33,25} = x_{33,25,34,1}$$

(773)

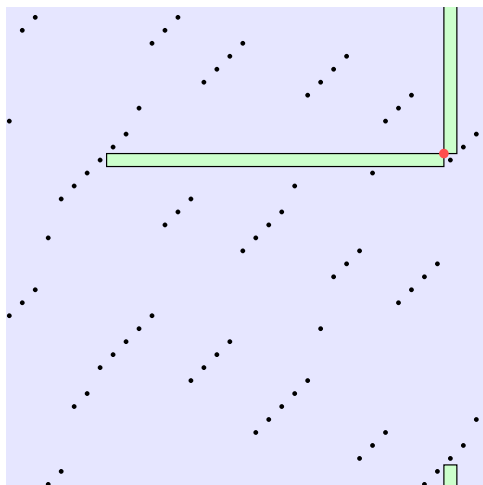

$$x_{8,24,33,26} = x_{33,26,35,1}$$

(774)

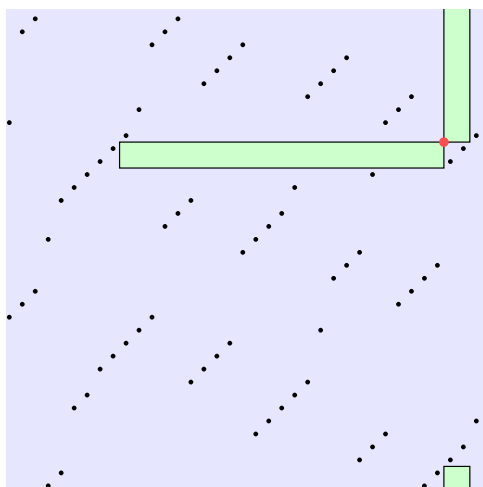

$$x_{9,24,33,27} + x_{28,17,33,27} = x_{33,27,36,1}$$

(775)

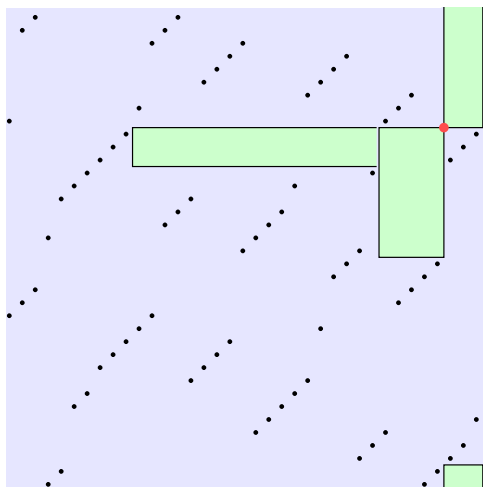

$$x_{29,17,33,28} = x_{33,28,0,1} \tag{776}$$

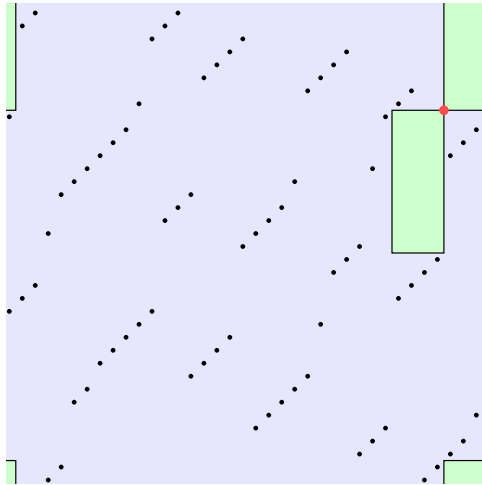

$$x_{30,17,33,29} = 0 \tag{777}$$

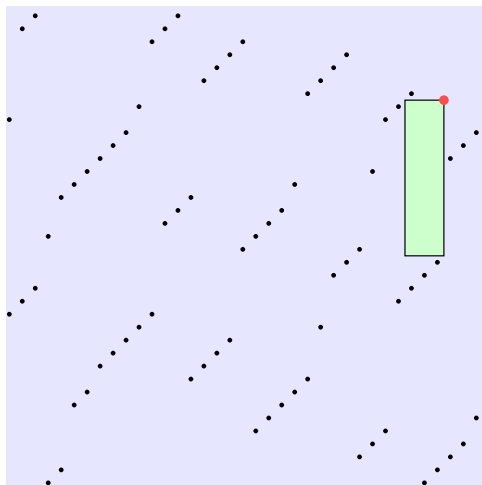

$$0 = x_{33,35,1,1} \tag{778}$$

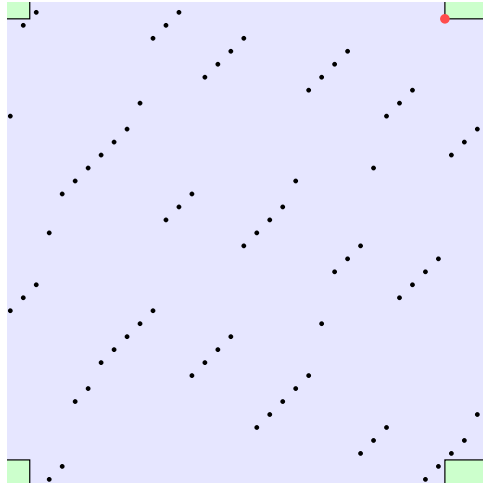

$$x_{31,17,33,36} = x_{33,36,2,1}$$

(779)

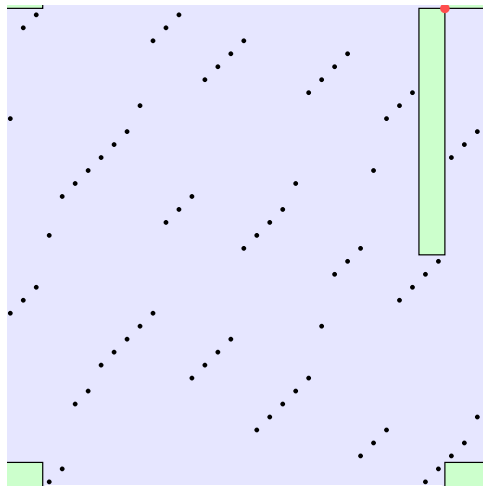

$$x_{32,25,34,0} = x_{34,0,3,2}$$

(780)

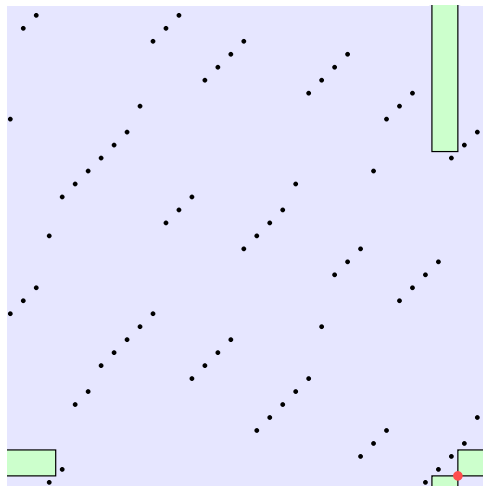

$$x_{33,25,34,1} = x_{34,1,26,2} \quad (781)$$

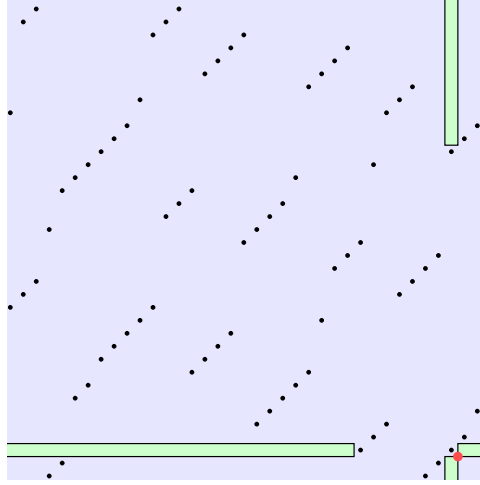

$$\begin{aligned} x_{28,2,34,3} + x_{29,2,34,13} + x_{30,2,34,14} + x_{31,2,34,15} + x_{32,2,34,16} + x_{33,2,34,24} = \\ = x_{34,0,3,2} + x_{34,1,26,2} + x_{34,26,35,2} + x_{34,27,36,2} + x_{34,28,0,2} + x_{34,35,1,2} + x_{34,36,2,2} \end{aligned} \quad (782)$$

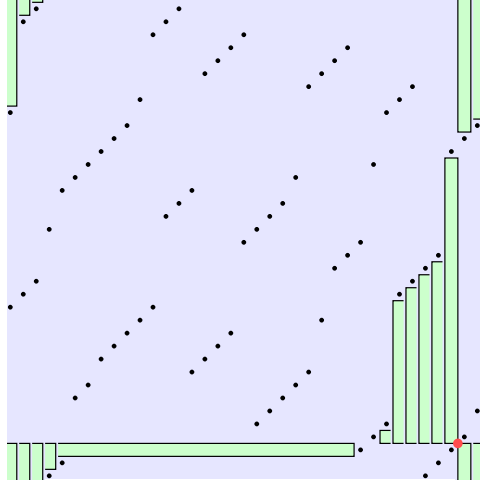

$$x_{28,2,34,3} = x_{34,3,35,25} \quad (783)$$



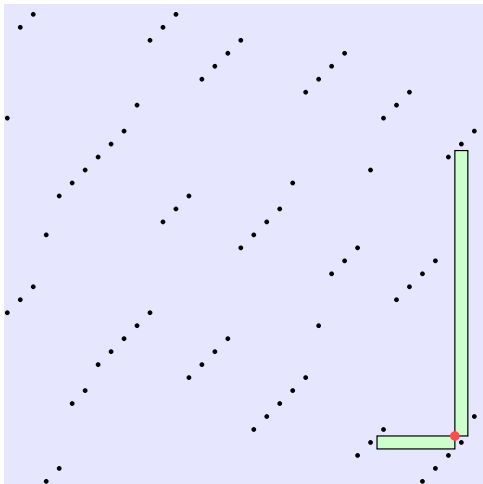

$$0 = x_{34,5,36,25}$$

(784)

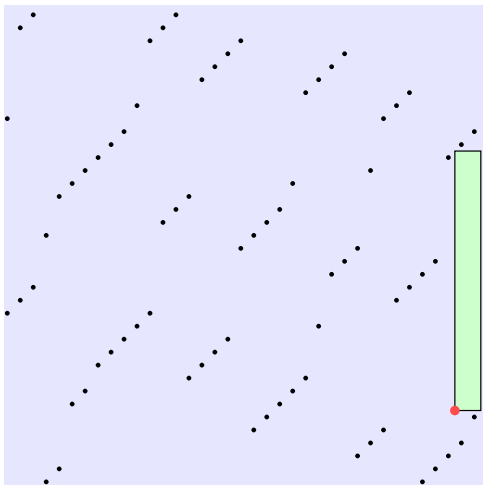

$$x_{29,2,34,13} = x_{34,13,0,25}$$

(785)

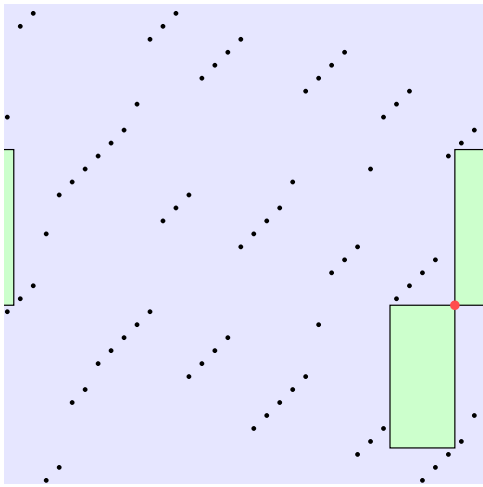

$$x_{30,2,34,14} = x_{34,14,1,25} \quad (786)$$

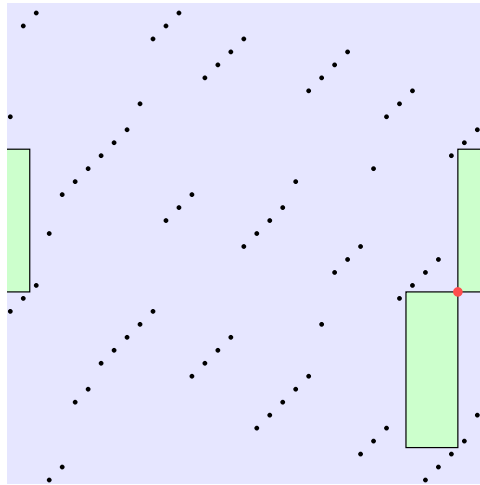

$$x_{31,2,34,15} = x_{34,15,2,25} \quad (787)$$

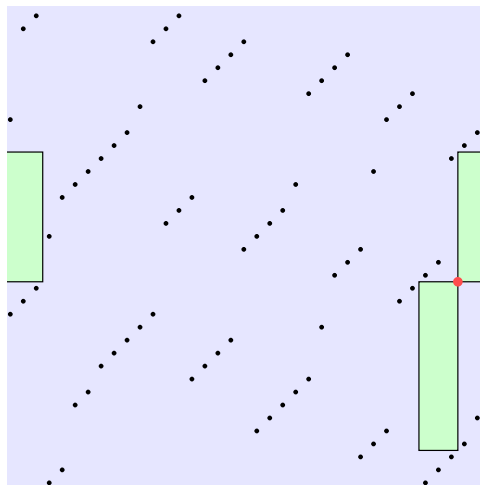

$$x_{32,2,34,16} = 0 \quad (788)$$

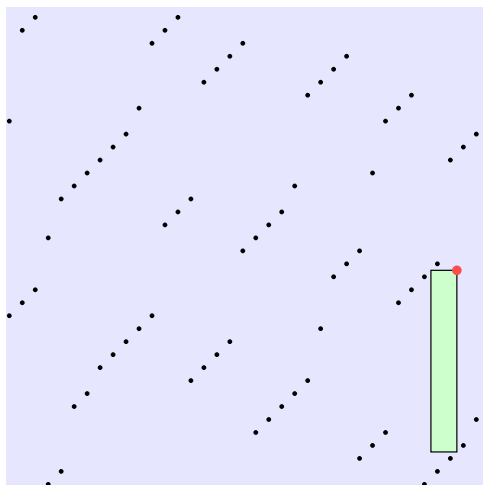

$$0 = x_{34,19,3,25}$$

(789)

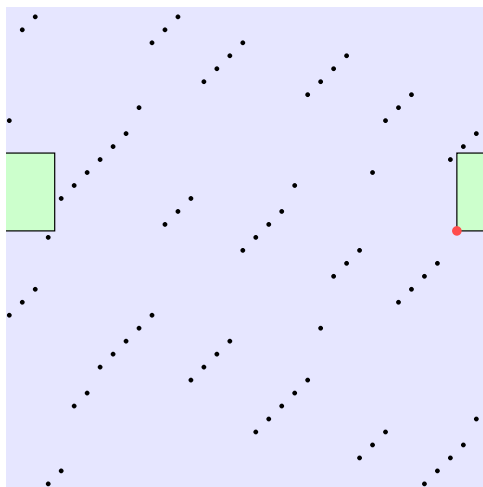

$$0 = x_{34,22,4,25}$$

(790)

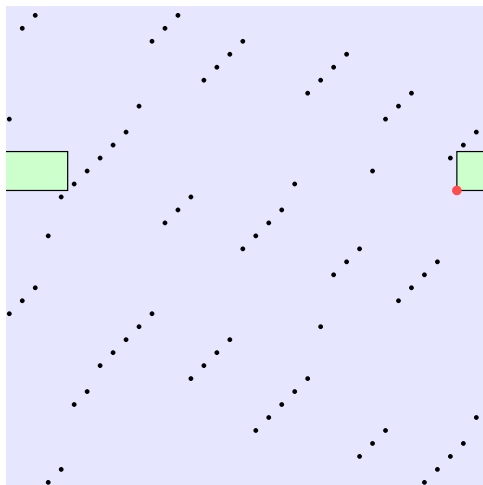

$$0 = x_{34,23,5,25}$$

(791)

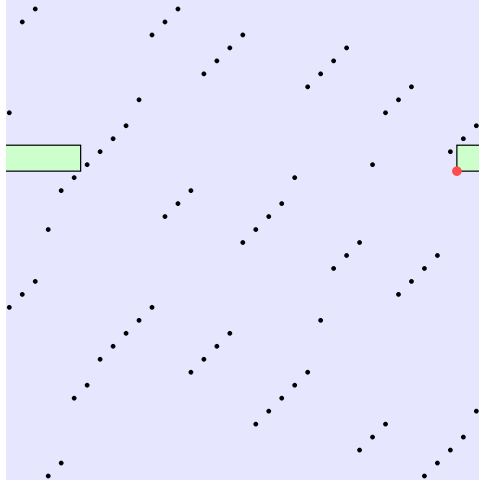

$$x_{33,2,34,24} = x_{34,24,6,25}$$

(792)

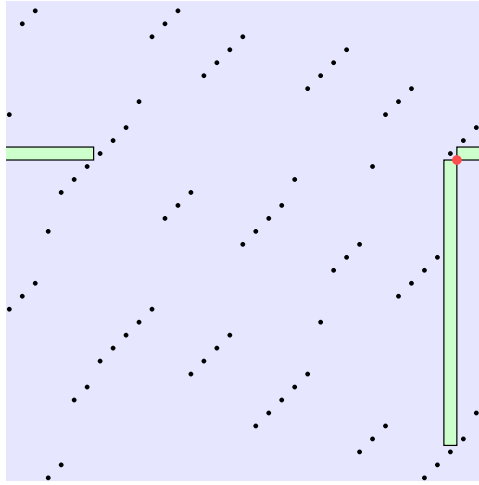

$$\begin{aligned} & x_{8,25,34,26} + x_{9,25,34,27} + x_{29,25,34,28} + x_{30,25,34,29} + x_{31,25,34,36} + x_{32,25,34,0} + x_{33,25,34,1} = \\ & = x_{34,3,35,25} + x_{34,5,36,25} + x_{34,13,0,25} + x_{34,14,1,25} + x_{34,15,2,25} + x_{34,19,3,25} + x_{34,22,4,25} + x_{34,23,5,25} + x_{34,24,6,25} \end{aligned} \quad (793)$$

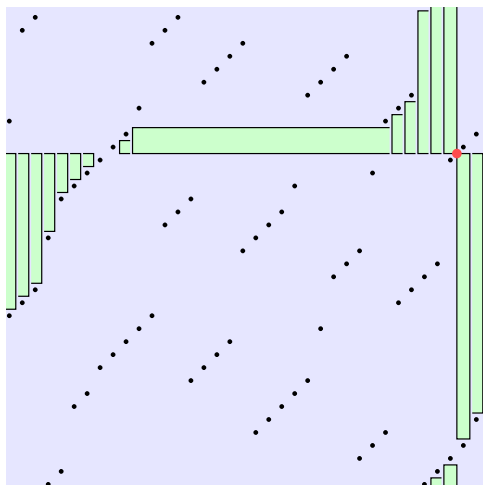

$$x_{8,25,34,26} = x_{34,26,35,2}$$

(794)

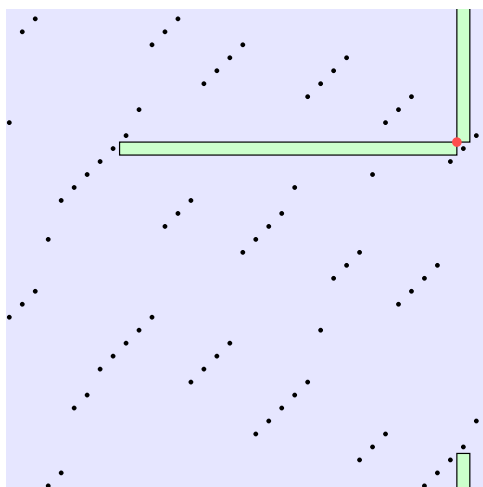

$$x_{9,25,34,27} = x_{34,27,36,2}$$

(795)

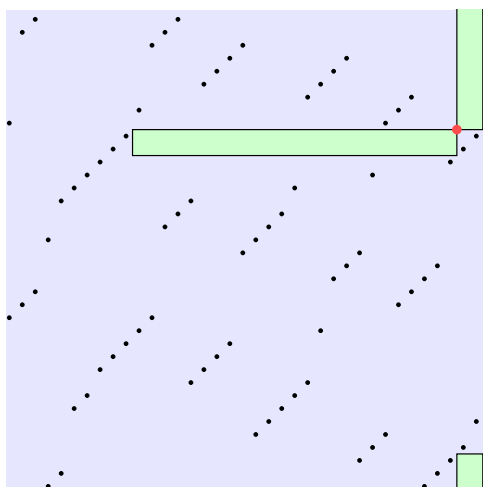

$$x_{29,25,34,28} = x_{34,28,0,2} \tag{796}$$

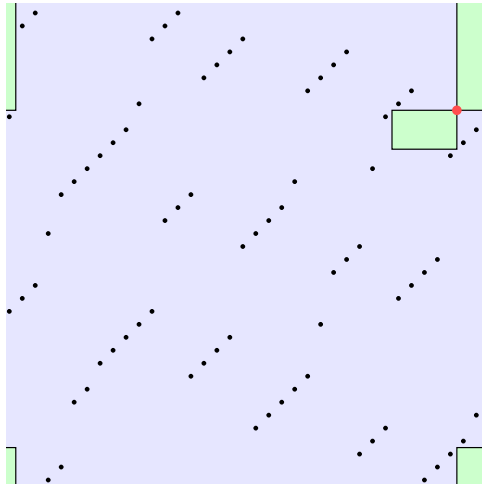

$$x_{30,25,34,29} = 0 \tag{797}$$

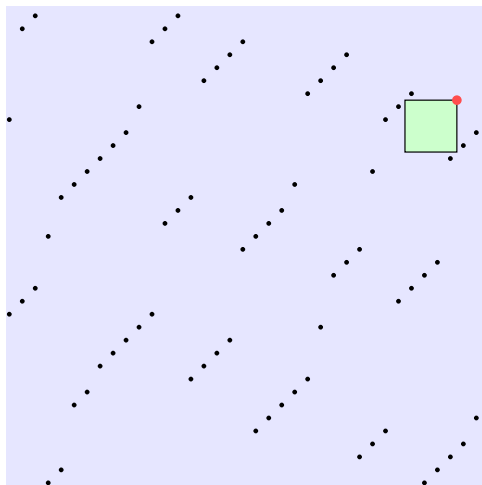

$$0 = x_{34,35,1,2} \tag{798}$$

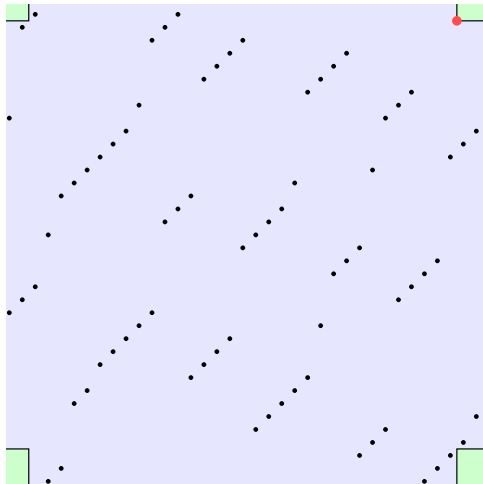

$$x_{31,25,34,36} = x_{34,36,2,2}$$

(799)

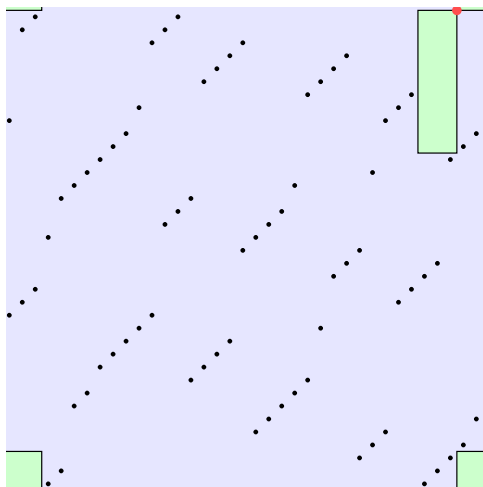

$$x_{32,26,35,0} = x_{35,0,3,4}$$

(800)

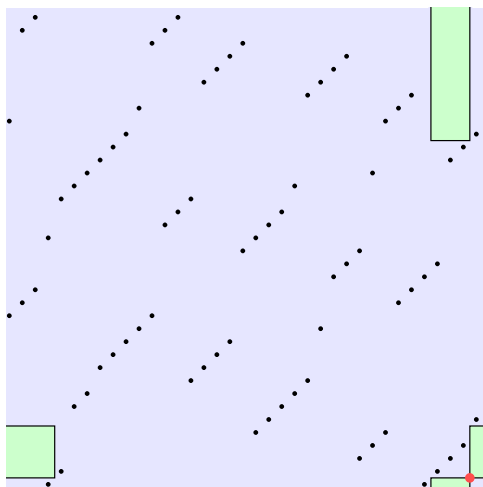

$$x_{33,26,35,1} = x_{35,1,18,4} + x_{35,1,26,3} \quad (801)$$

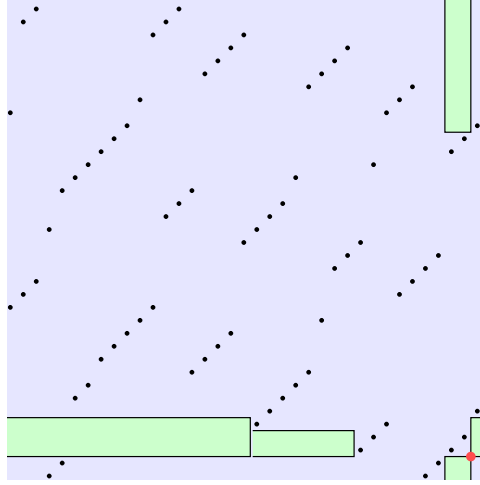

$$x_{34,26,35,2} = x_{35,2,27,3} \quad (802)$$

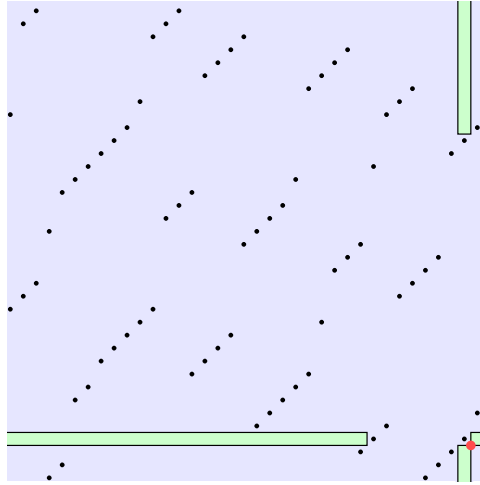

$$x_{29,3,35,13} + x_{30,3,35,14} + x_{31,3,35,15} + x_{32,3,35,16} + x_{33,3,35,24} + x_{34,3,35,25} = x_{35,1,26,3} + x_{35,2,27,3} \quad (803)$$



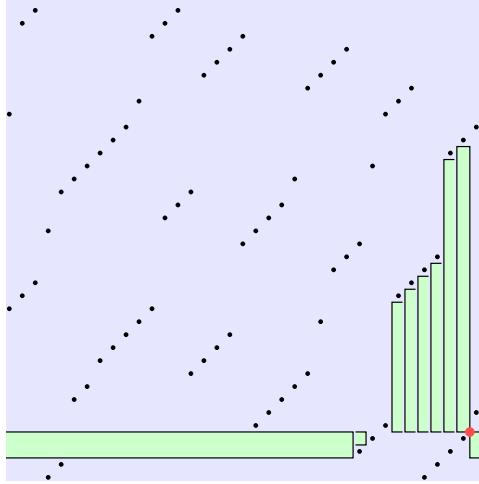

$$\begin{aligned}
 x_{20,4,35,5} + x_{21,4,35,6} + x_{22,4,35,7} + x_{23,4,35,11} + x_{24,4,35,13} = \\
 = x_{35,0,3,4} + x_{35,1,18,4} + x_{35,27,36,4} + x_{35,28,0,4} + x_{35,35,1,4} + x_{35,36,2,4} \quad (804)
 \end{aligned}$$

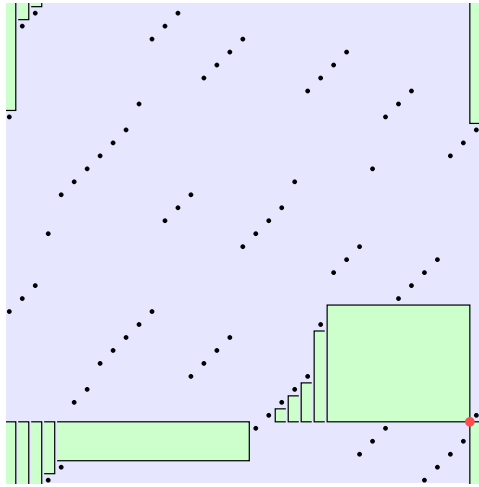

$$x_{20,4,35,5} = x_{35,5,36,26} \quad (805)$$

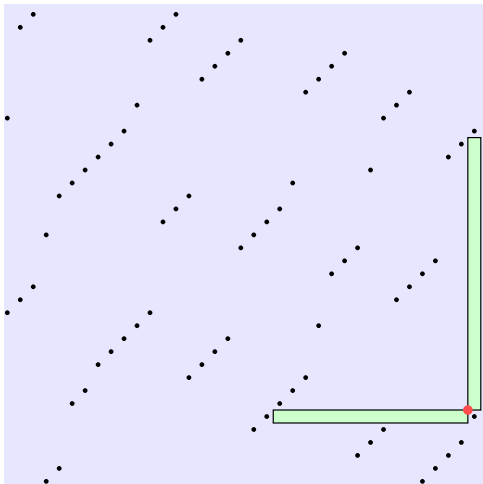

$$x_{21,4,35,6} = 0$$

(806)

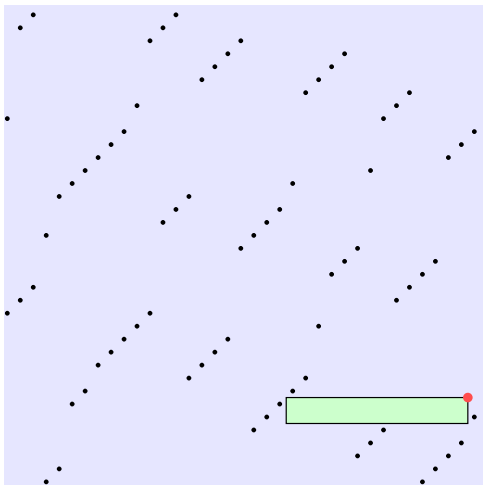

$$x_{22,4,35,7} = 0$$

(807)

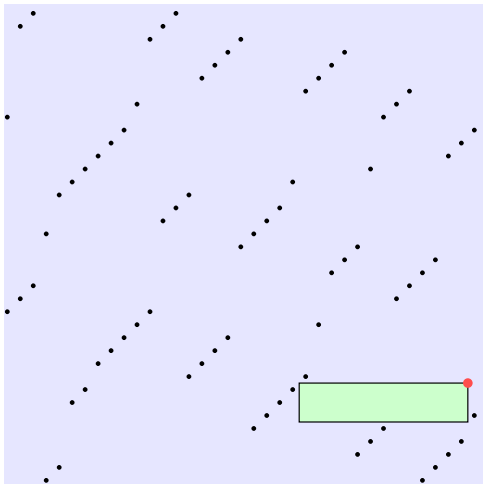

$$x_{23,4,35,11} = 0 \tag{808}$$

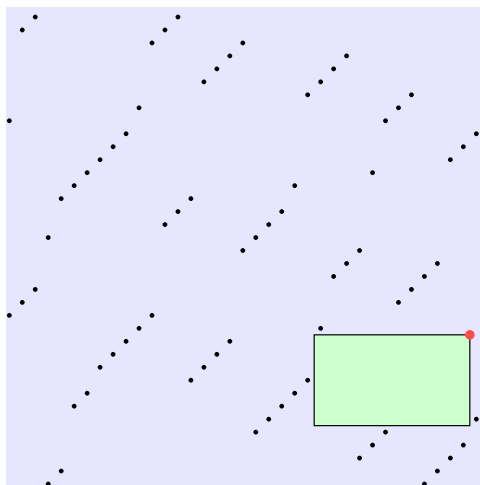

$$x_{24,4,35,13} + x_{29,3,35,13} = x_{35,13,0,26} \tag{809}$$

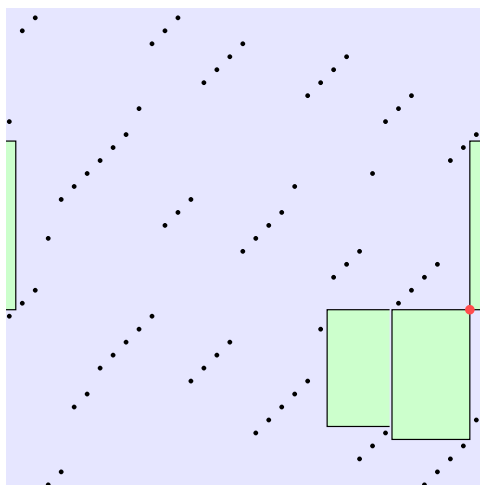

$$x_{30,3,35,14} = x_{35,14,1,26} \tag{810}$$

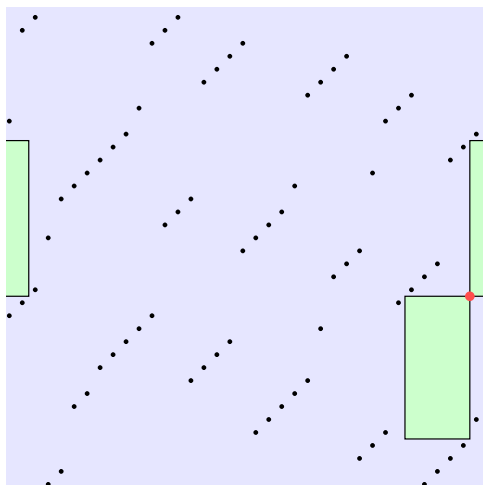

$$x_{31,3,35,15} = x_{35,15,2,26}$$

(811)

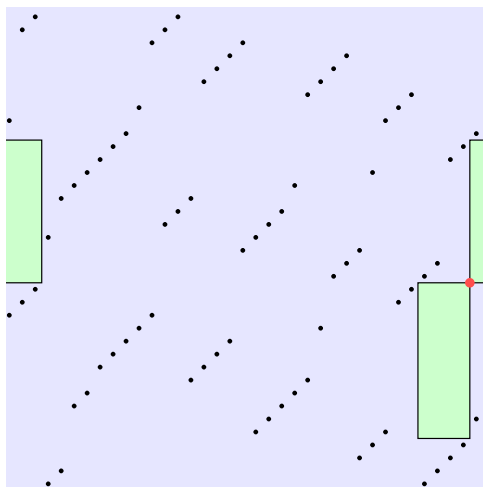

$$x_{32,3,35,16} = 0$$

(812)

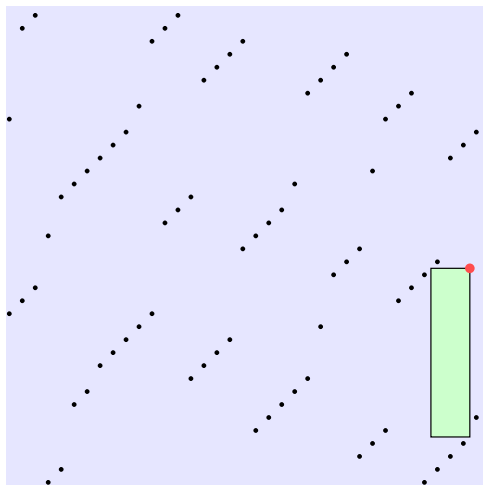

$$0 = x_{35,19,3,26} \tag{813}$$

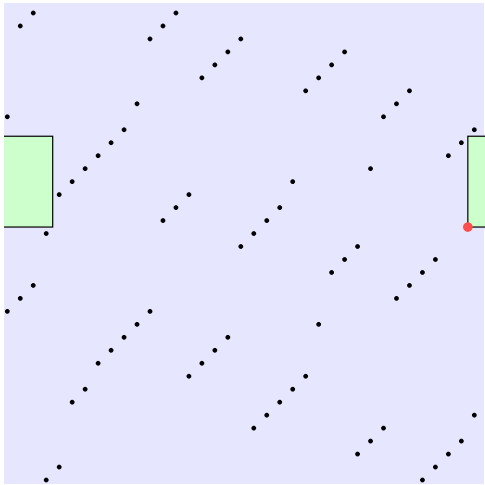

$$0 = x_{35,22,4,26} \tag{814}$$

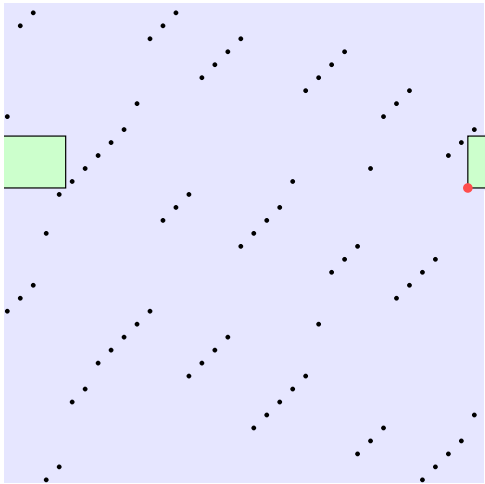

$$0 = x_{35,23,5,26} \tag{815}$$

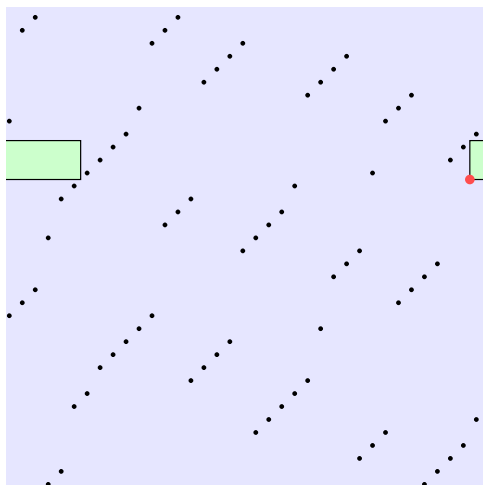

$$x_{33,3,35,24} = x_{35,24,6,26}$$

(816)

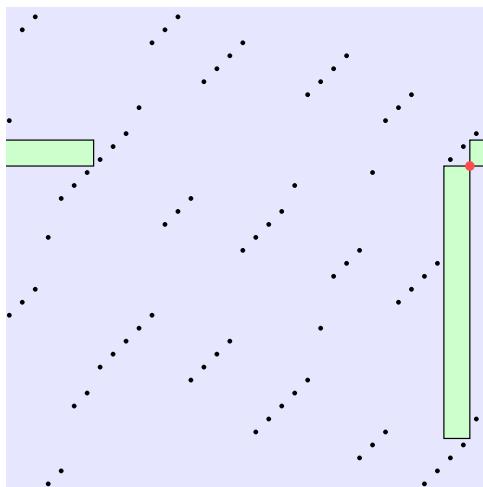

$$x_{34,3,35,25} = x_{35,25,7,26}$$

(817)

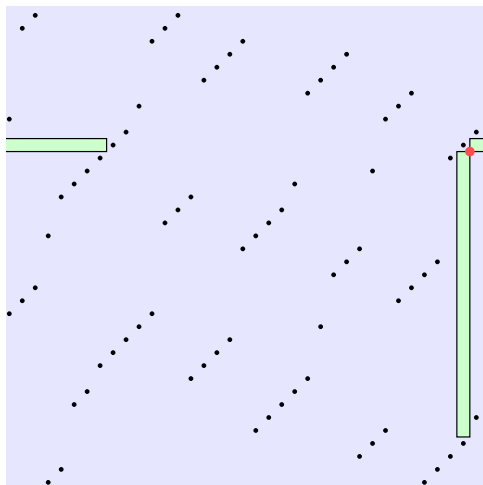

$$\begin{aligned}
& x_{9,26,35,27} + x_{29,26,35,28} + x_{30,26,35,29} + x_{31,26,35,36} + x_{32,26,35,0} + x_{33,26,35,1} + x_{34,26,35,2} = \\
& = x_{35,5,36,26} + x_{35,13,0,26} + x_{35,14,1,26} + x_{35,15,2,26} + x_{35,19,3,26} + x_{35,22,4,26} + x_{35,23,5,26} + x_{35,24,6,26} + x_{35,25,7,26} \quad (818)
\end{aligned}$$

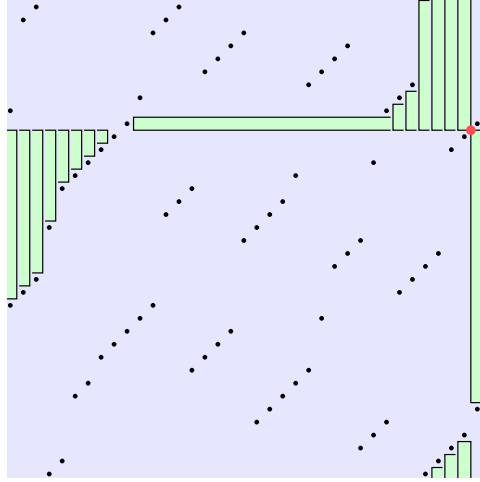

$$x_{9,26,35,27} = x_{35,27,36,4} \quad (819)$$

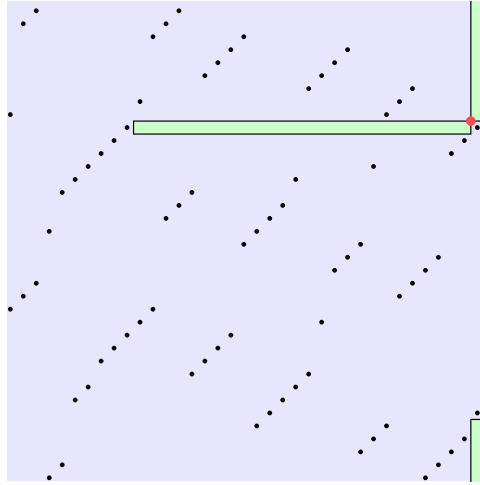

$$x_{29,26,35,28} = x_{35,28,0,4} \quad (820)$$

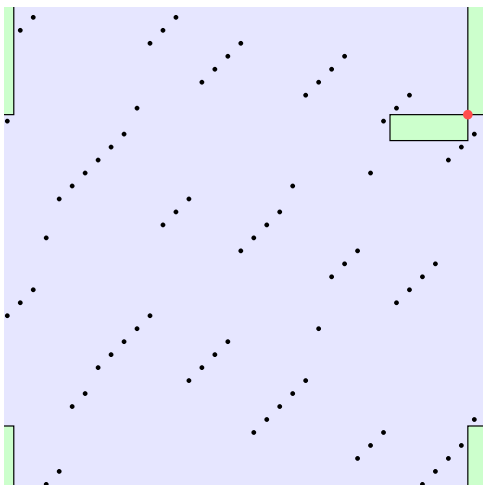

$$x_{30,26,35,29} = 0$$

(821)

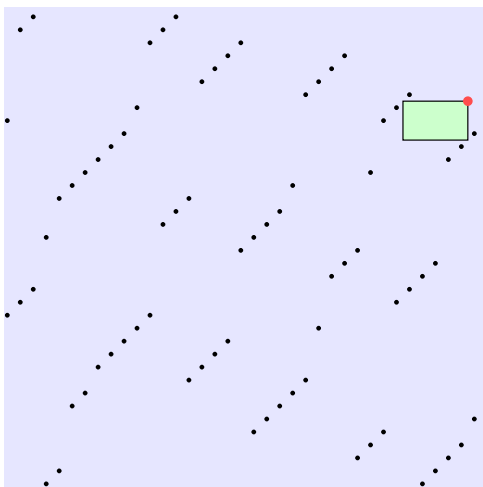

$$0 = x_{35,35,1,4}$$

(822)

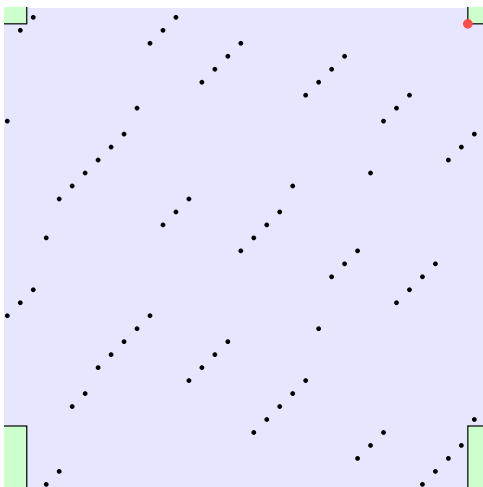



$$x_{31,26,35,36} = x_{35,36,2,4} \quad (823)$$

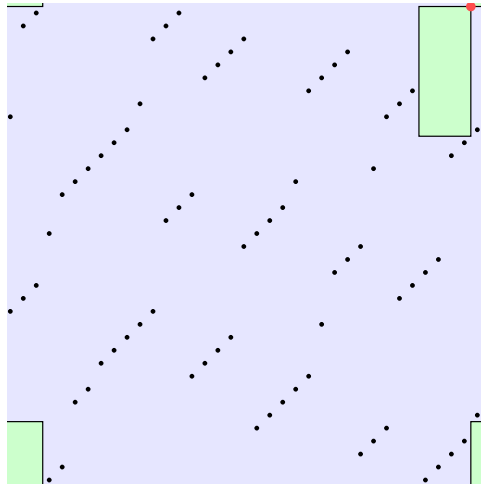

$$x_{32,27,36,0} = x_{36,0,3,12} \quad (824)$$

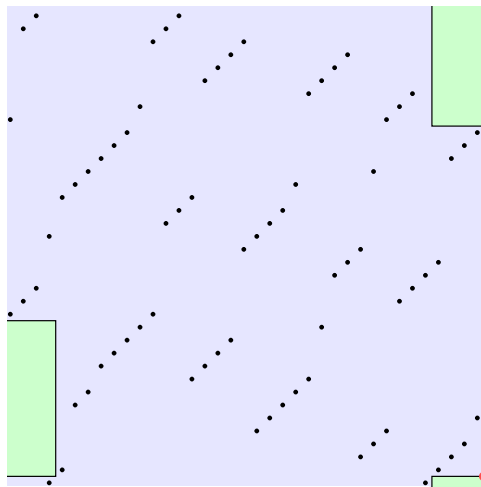

$$x_{33,27,36,1} = x_{36,1,4,12} + x_{36,1,18,5} \quad (825)$$

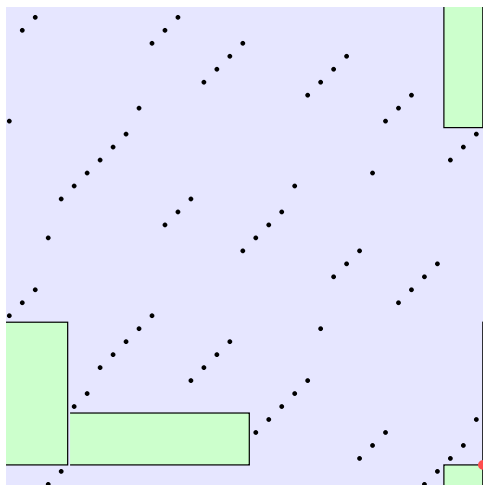

$$x_{34,27,36,2} = 0$$

(826)

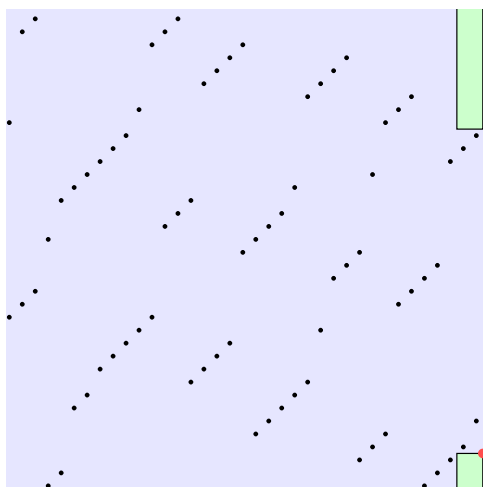

$$x_{35,27,36,4} = x_{36,4,19,5}$$

(827)

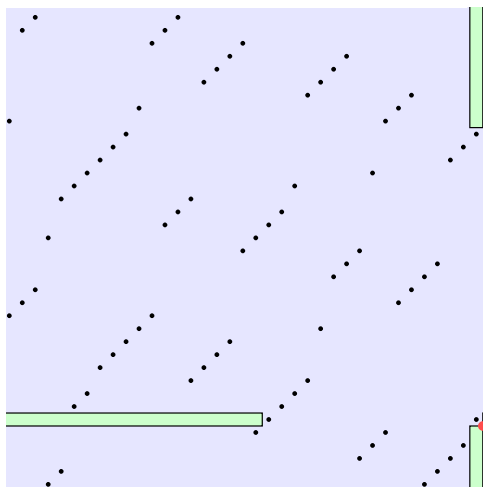

$$x_{24,5,36,13} + x_{30,5,36,14} + x_{31,5,36,15} + x_{32,5,36,16} + x_{33,5,36,24} + x_{34,5,36,25} + x_{35,5,36,26} = x_{36,1,18,5} + x_{36,4,19,5} \quad (828)$$

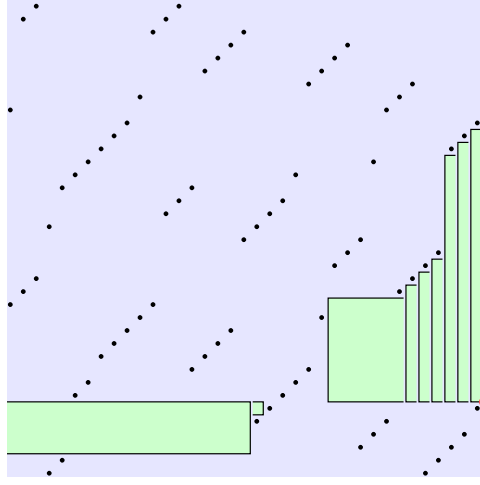

$$x_{11,12,36,13} = x_{36,0,3,12} + x_{36,1,4,12} + x_{36,28,0,12} + x_{36,35,1,12} + x_{36,36,2,12} \quad (829)$$

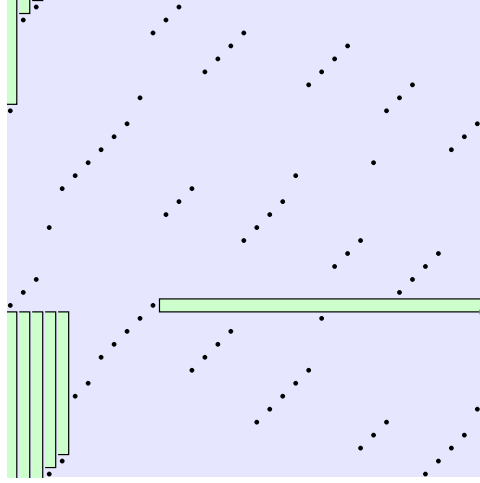

$$x_{11,12,36,13} + x_{24,5,36,13} = x_{36,13,0,27} \quad (830)$$

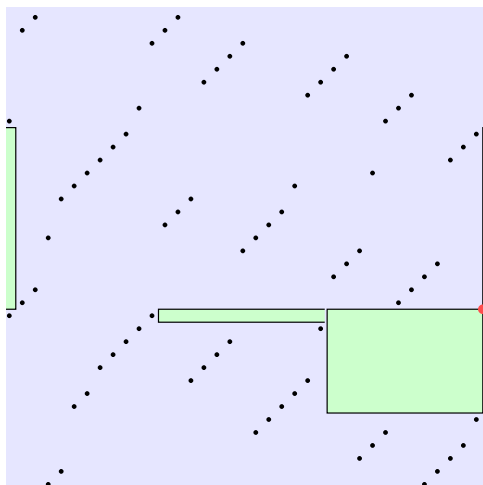

$$x_{30,5,36,14} = x_{36,14,1,27}$$

(831)

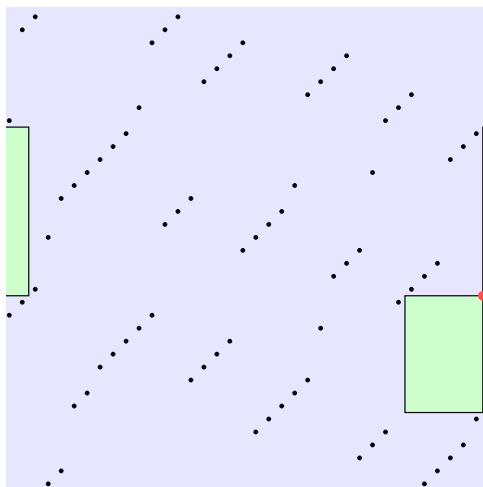

$$x_{31,5,36,15} = x_{36,15,2,27}$$

(832)

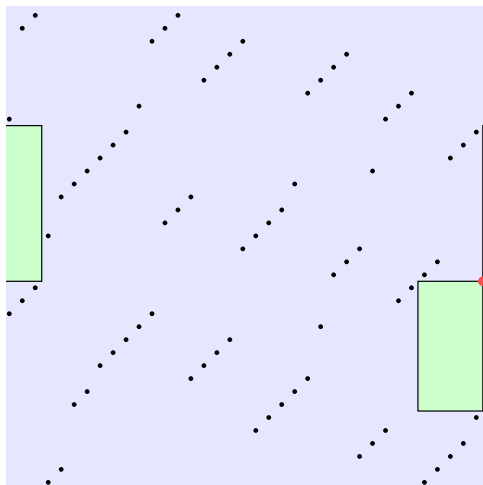

$$x_{32,5,36,16} = 0 \tag{833}$$

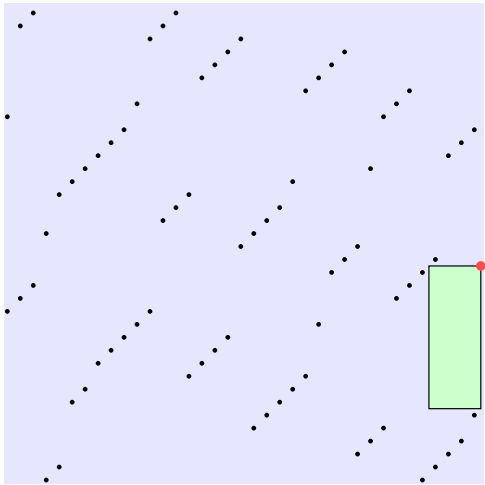

$$0 = x_{36,19,3,27} \tag{834}$$

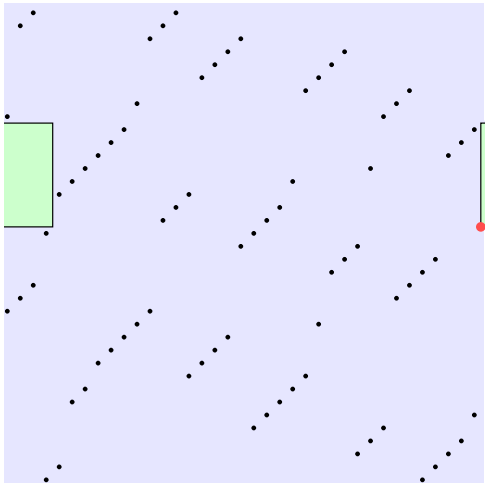

$$0 = x_{36,22,4,27} \tag{835}$$

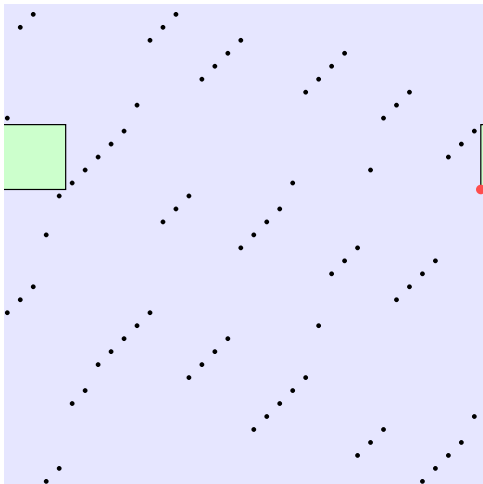

$$0 = x_{36,23,5,27}$$

(836)

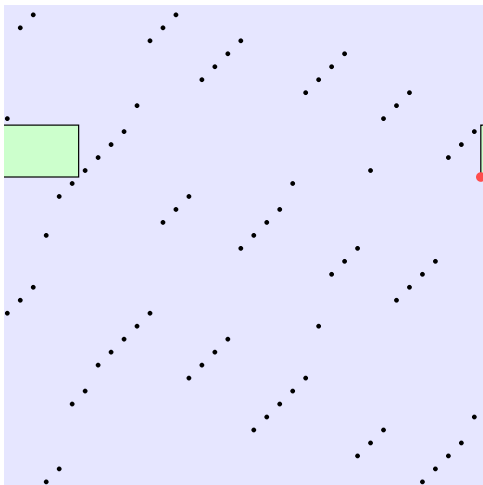

$$x_{33,5,36,24} = x_{36,24,6,27}$$

(837)

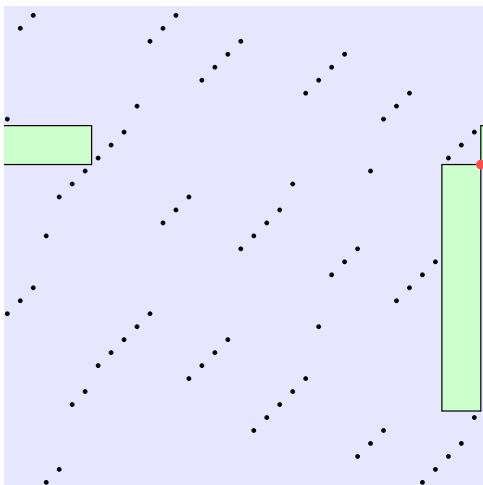

$$x_{34,5,36,25} = x_{36,25,7,27} \quad (838)$$

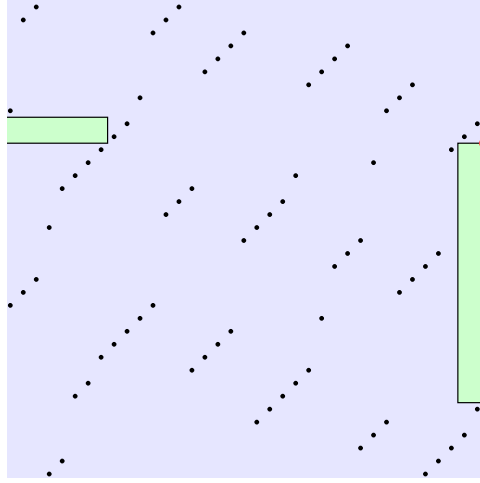

$$x_{35,5,36,26} = x_{36,26,8,27} \quad (839)$$

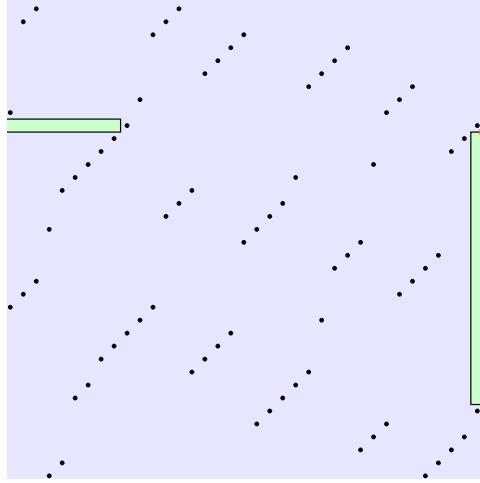

$$\begin{aligned} & x_{29,27,36,28} + x_{30,27,36,29} + x_{31,27,36,36} + x_{32,27,36,0} + x_{33,27,36,1} + x_{34,27,36,2} + x_{35,27,36,4} = \\ & = x_{36,13,0,27} + x_{36,14,1,27} + x_{36,15,2,27} + x_{36,19,3,27} + x_{36,22,4,27} + x_{36,23,5,27} + x_{36,24,6,27} + x_{36,25,7,27} + x_{36,26,8,27} \end{aligned} \quad (840)$$

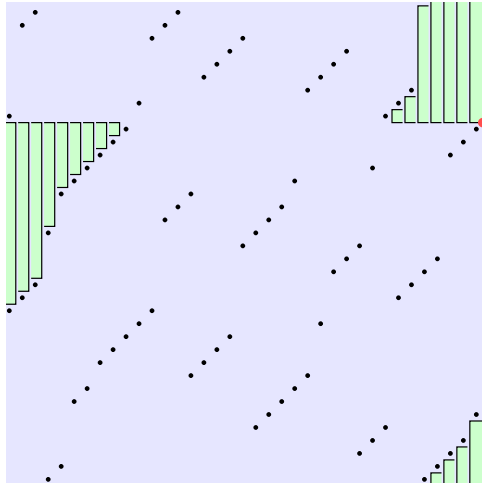

$$x_{29,27,36,28} = x_{36,28,0,12}$$

(841)

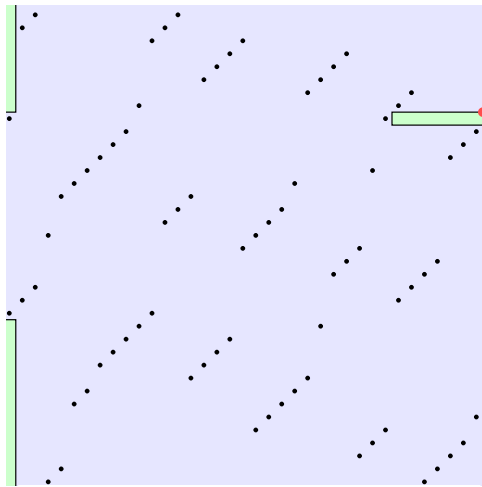

$$x_{30,27,36,29} = 0$$

(842)

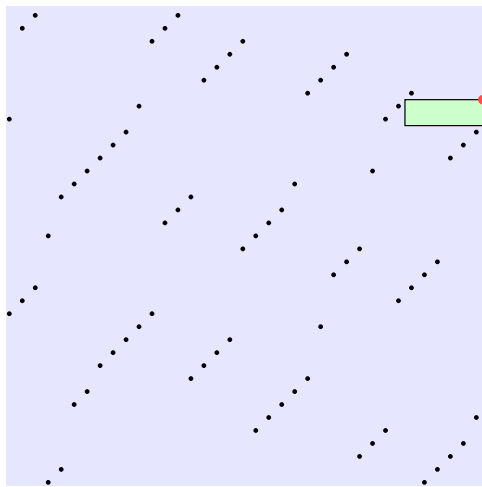



$$0 = x_{36,35,1,12}$$

(843)

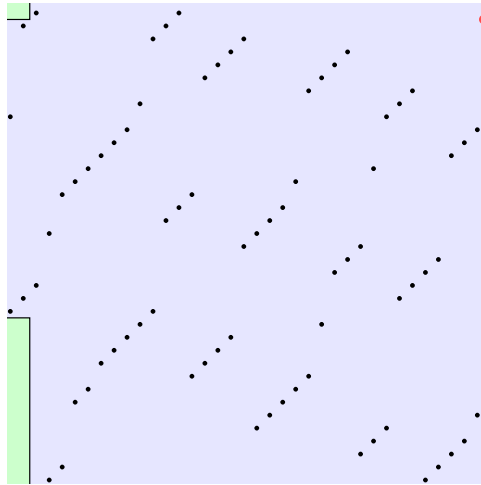

$$x_{31,27,36,36} = x_{36,36,2,12}$$

(844)

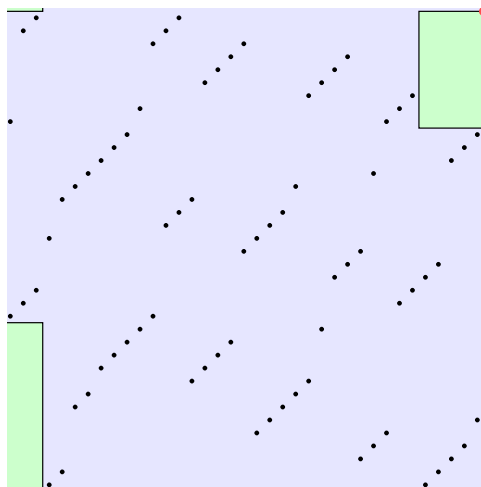

Supplement: Supplementary file 1 [file matching.pdf]
