# Supplementary material for: Distinguishing Legendrian knots with trivial orientation-preserving symmetry group
Source: arXiv:1810.06460 ancillary file (2021-09-14)

# Maximal types of rectangles

1.  $(0, 0, 3, 13)$

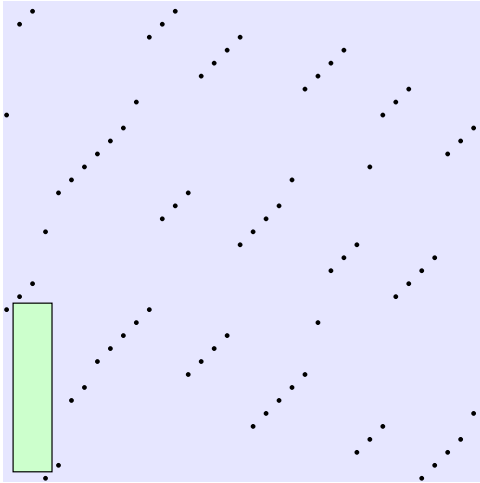

2.  $(0, 1, 4, 13)$

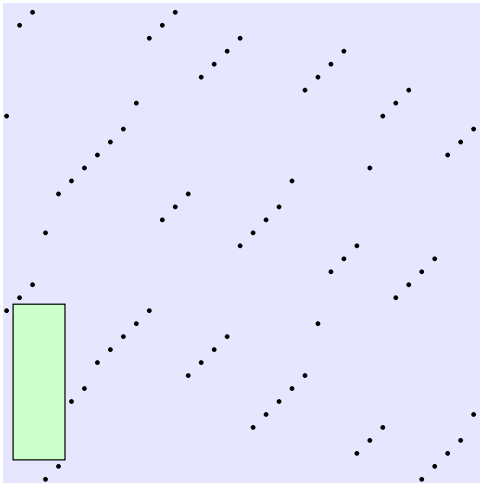

3.  $(0, 6, 5, 13)$

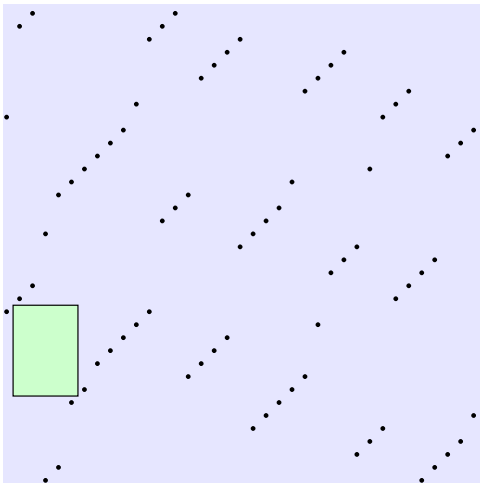

4.  $(0, 7, 6, 13)$

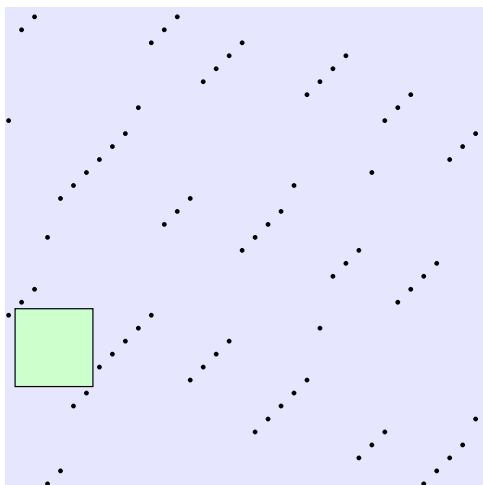

5.  $(0, 9, 7, 13)$

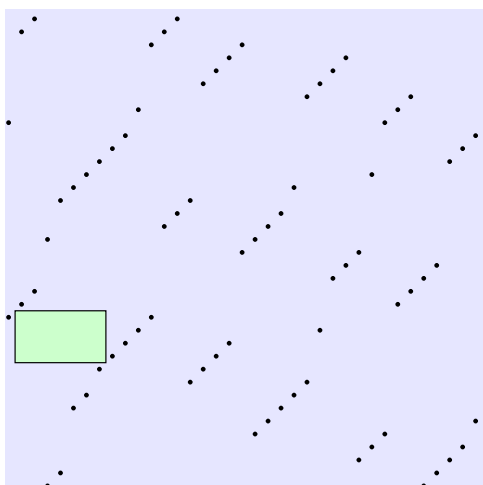

6.  $(0, 10, 8, 13)$

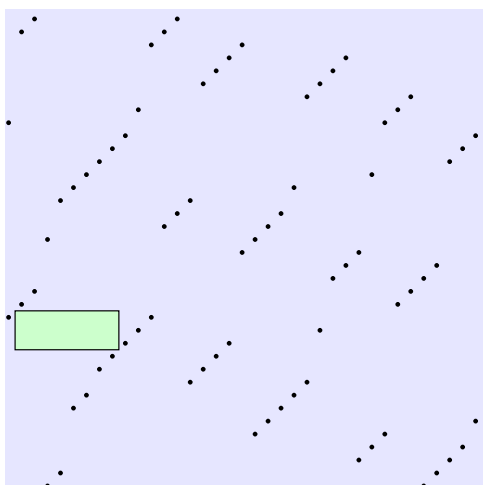

7.  $(0, 11, 9, 13)$

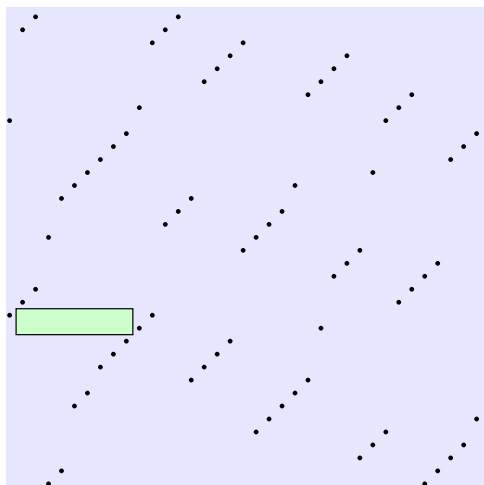

8.  $(0, 12, 10, 13)$

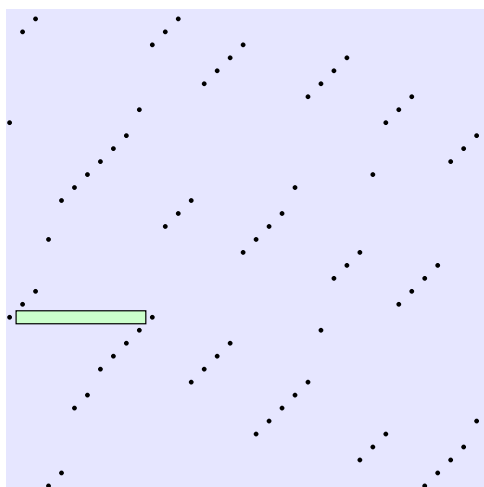

9.  $(0, 14, 1, 34)$

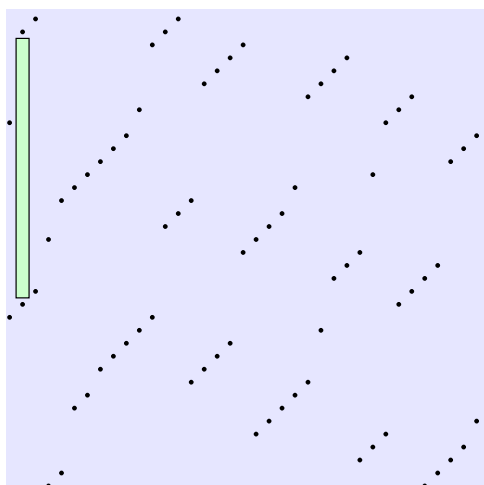

10.  $(0, 15, 2, 34)$

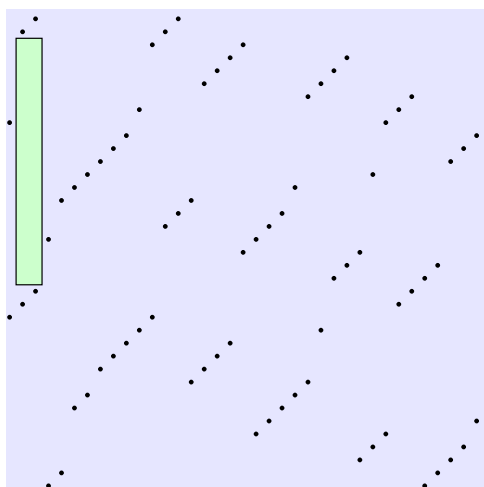

11.  $(0, 19, 3, 34)$

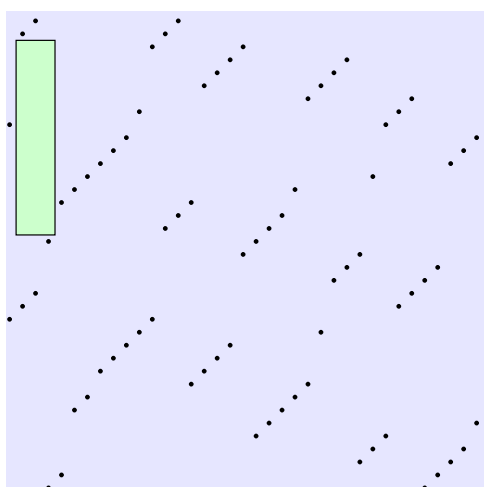

12.  $(0, 22, 4, 34)$

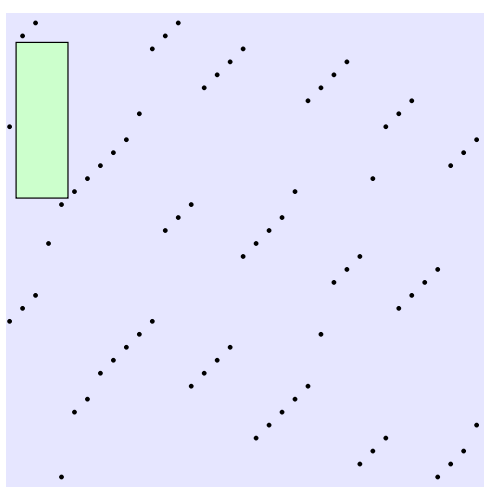

13.  $(0, 23, 5, 34)$

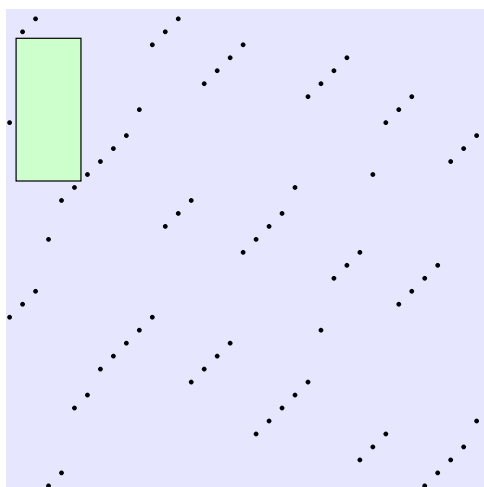

14.  $(0, 24, 6, 34)$

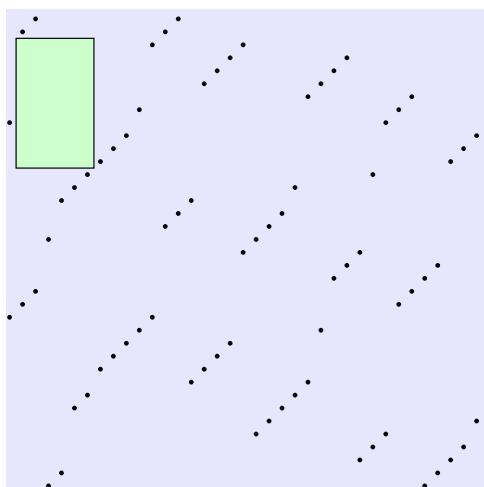

15.  $(0, 25, 7, 34)$

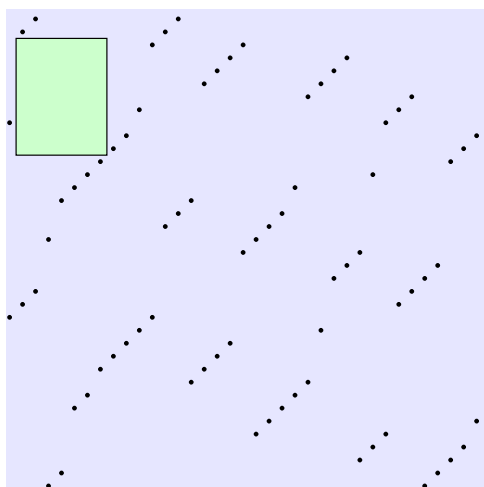

16.  $(0, 26, 8, 34)$

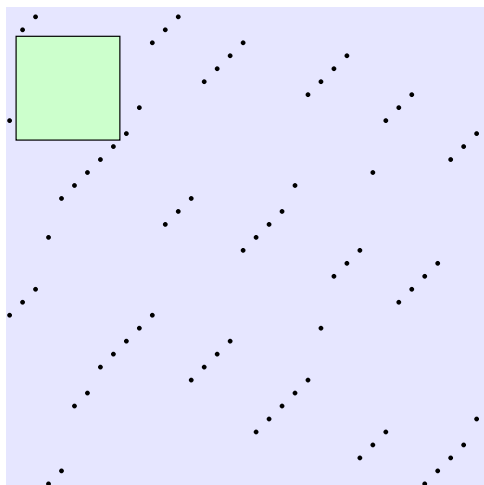

17.  $(0, 27, 9, 34)$

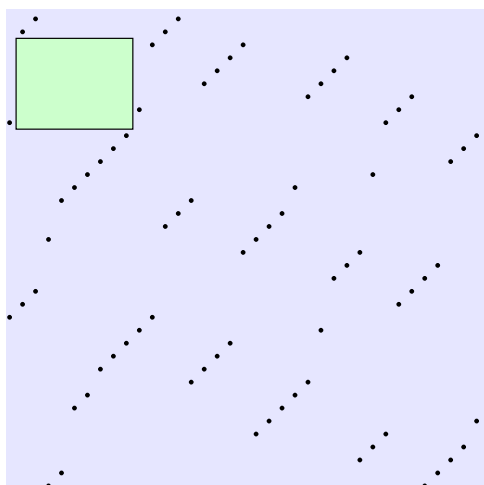

18.  $(0, 27, 28, 28)$

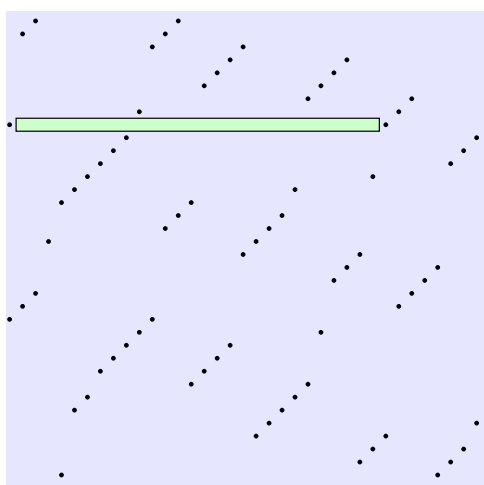

19.  $(0, 35, 1, 13)$

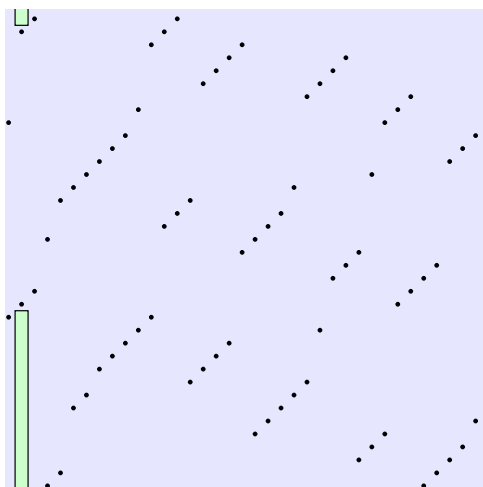

20.  $(0, 36, 2, 13)$

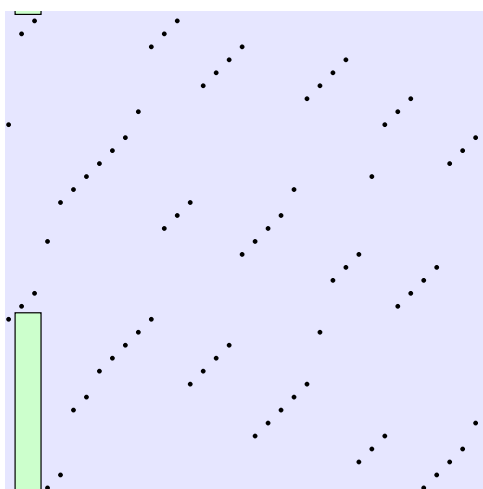

21.  $(1, 0, 3, 14)$

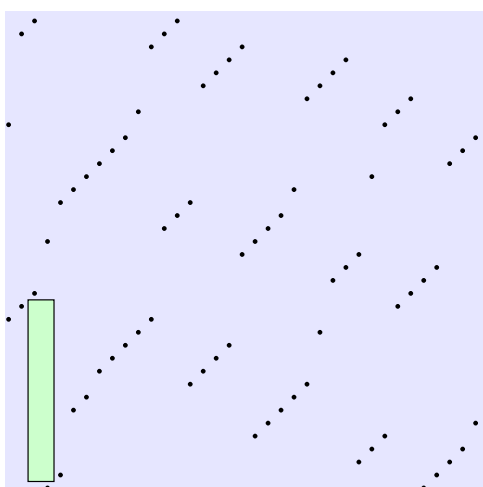

22.  $(1, 1, 4, 14)$

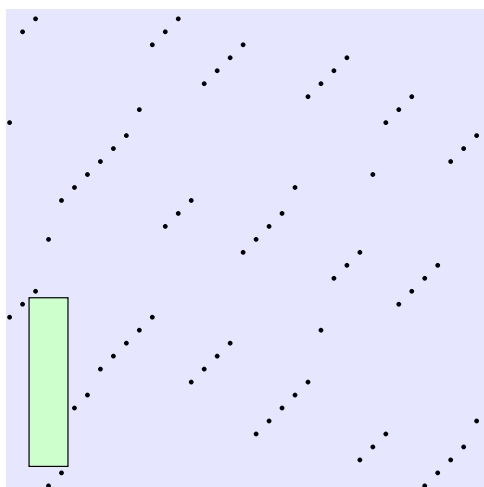

23.  $(1, 6, 5, 14)$

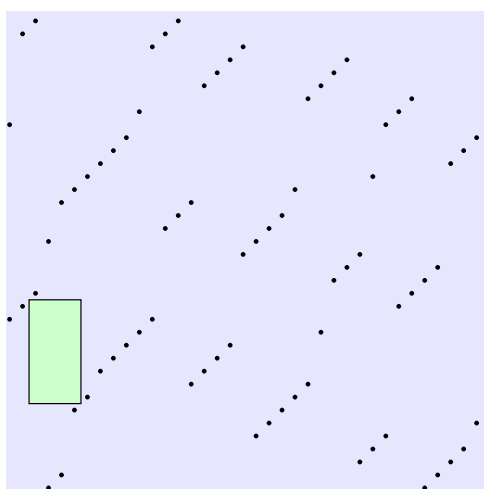

24.  $(1, 7, 6, 14)$

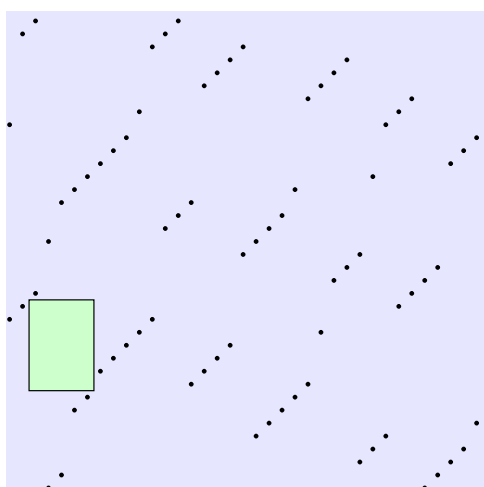



25. (1, 9, 7, 14)

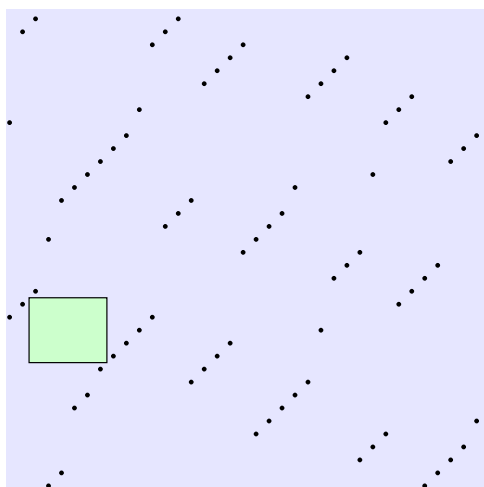

26. (1, 10, 8, 14)

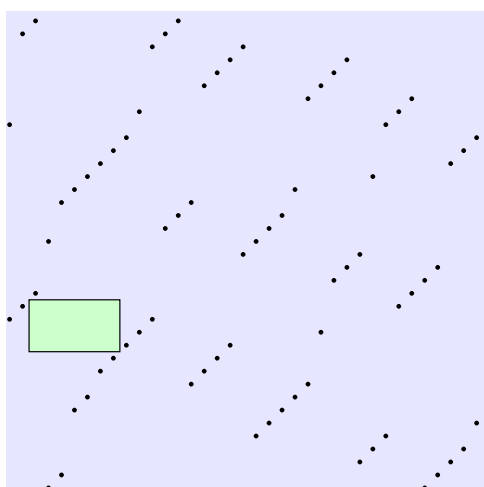

27. (1, 11, 9, 14)

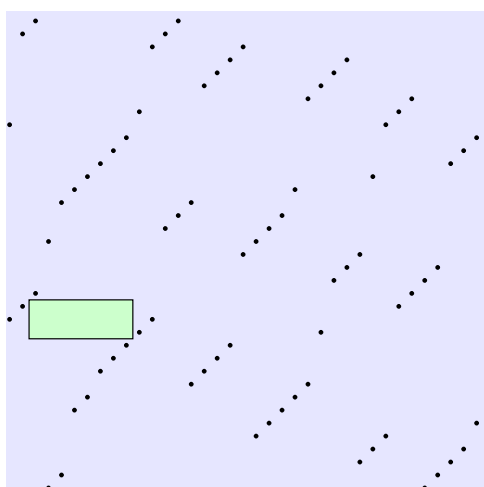

28.  $(1, 12, 10, 14)$

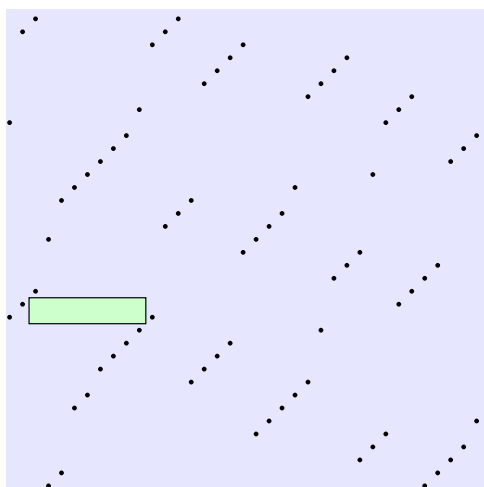

29.  $(1, 13, 29, 14)$

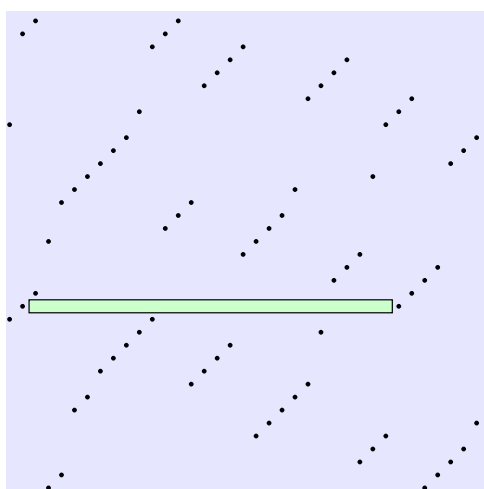

30.  $(1, 15, 2, 35)$

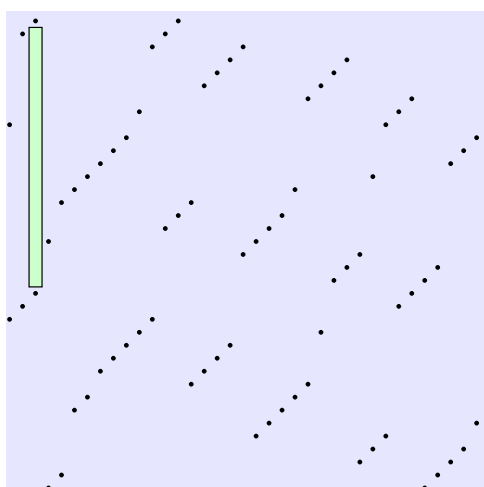

31.  $(1, 19, 3, 35)$

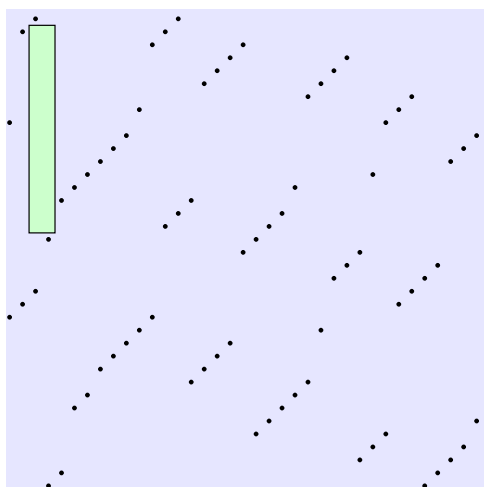

32.  $(1, 22, 4, 35)$

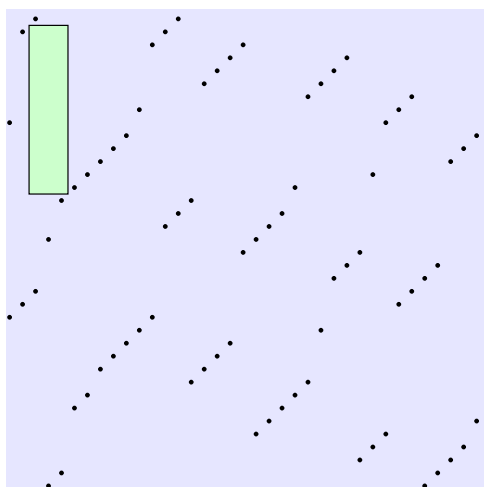

33.  $(1, 23, 5, 35)$

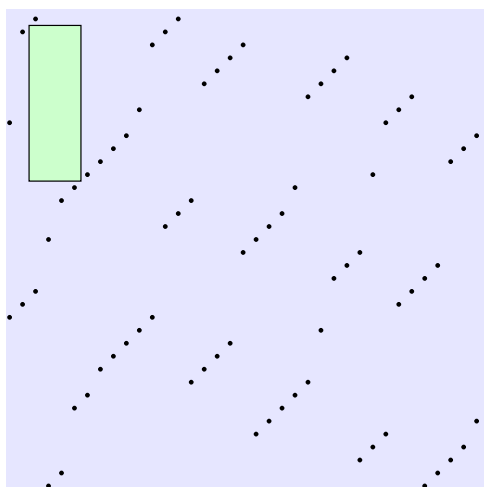

34. (1, 24, 6, 35)

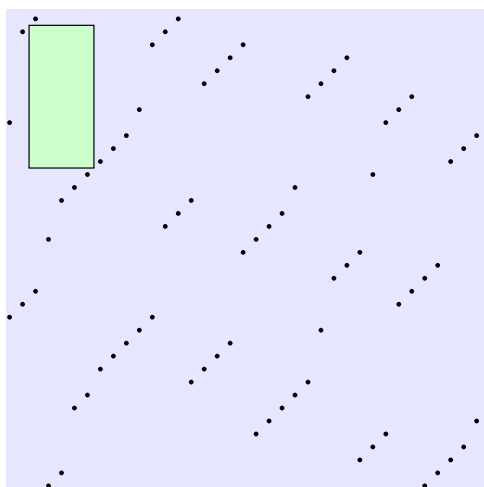

35. (1, 25, 7, 35)

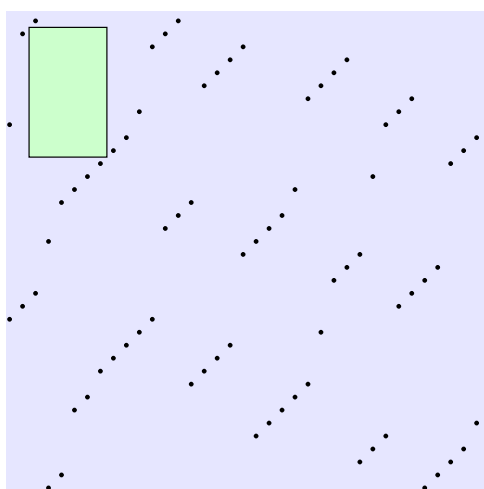

36. (1, 26, 8, 35)

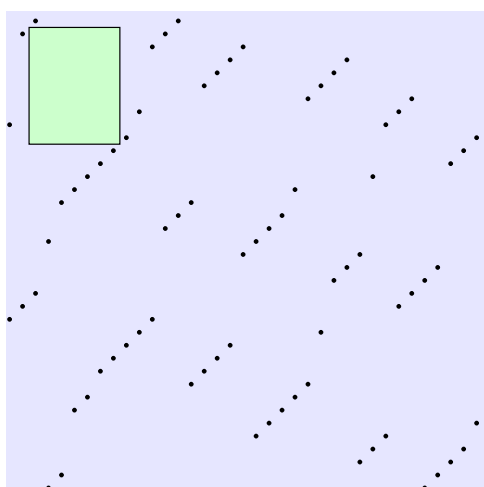

37. (1, 27, 9, 35)

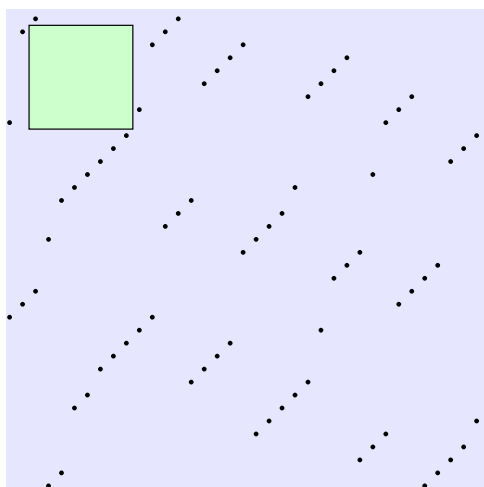

38. (1, 29, 10, 35)

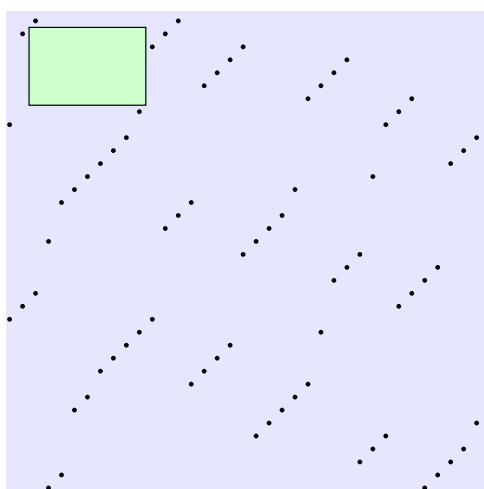

39. (1, 34, 11, 35)

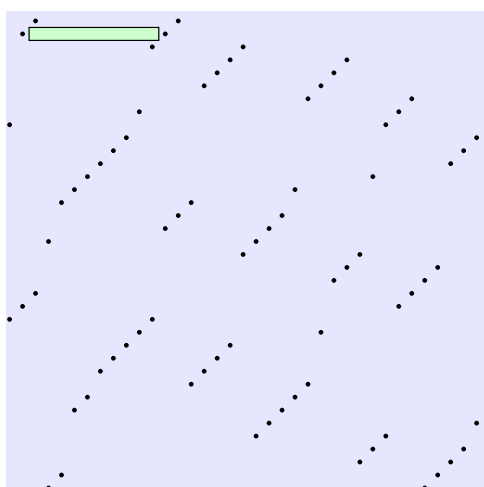

40.  $(1, 36, 2, 14)$

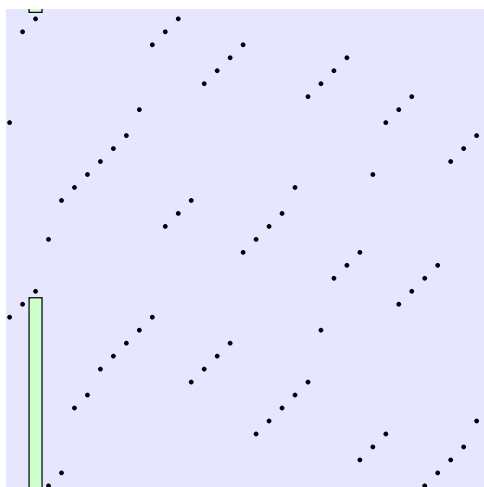

41.  $(2, 0, 3, 18)$

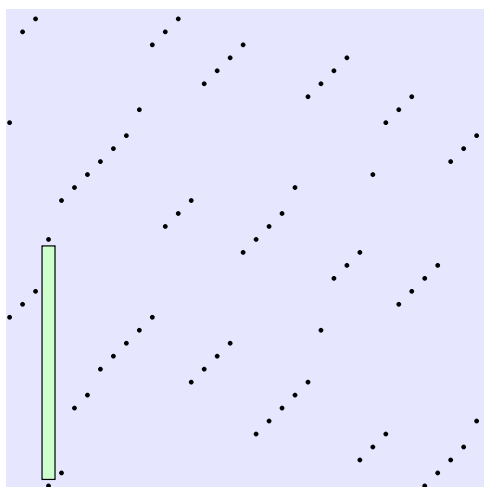

42.  $(2, 1, 4, 18)$

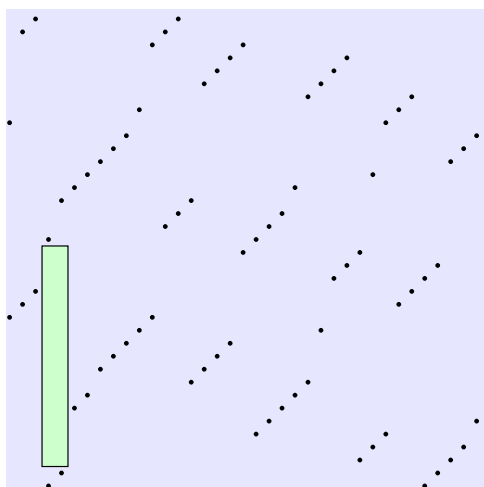

43. (2, 6, 5, 18)

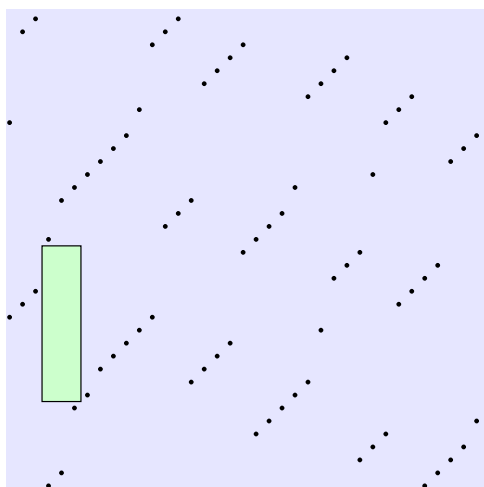

44. (2, 7, 6, 18)

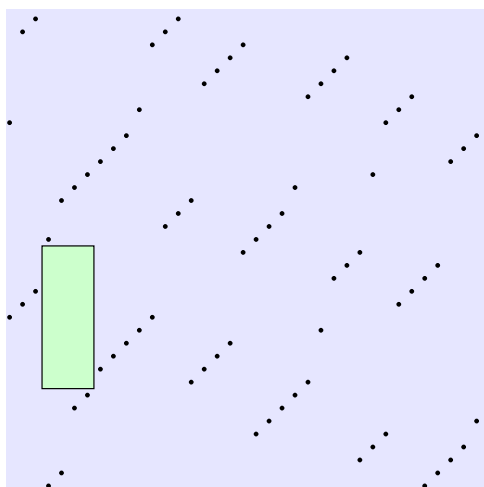

45. (2, 9, 7, 18)

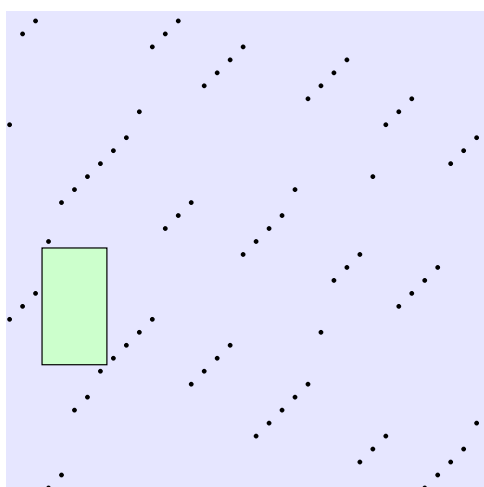

46. (2, 10, 8, 18)

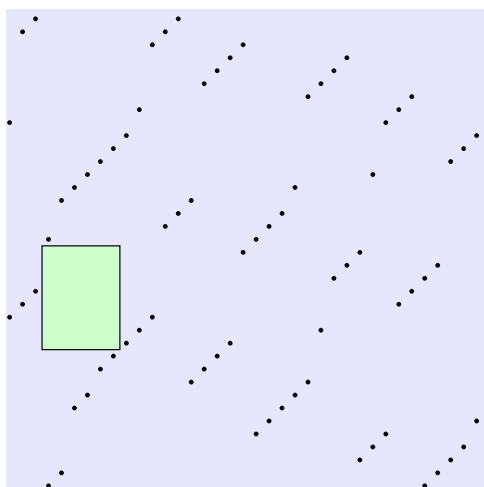

47. (2, 11, 9, 18)

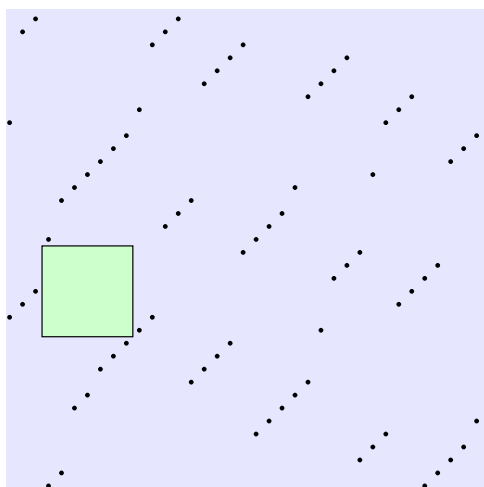

48. (2, 12, 10, 18)

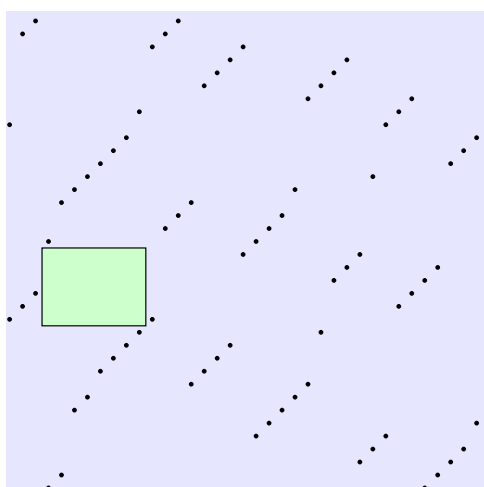



49. (2, 13, 17, 18)

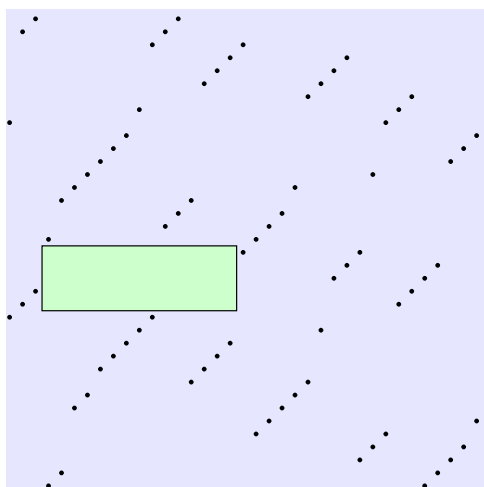

50. (2, 13, 24, 17)

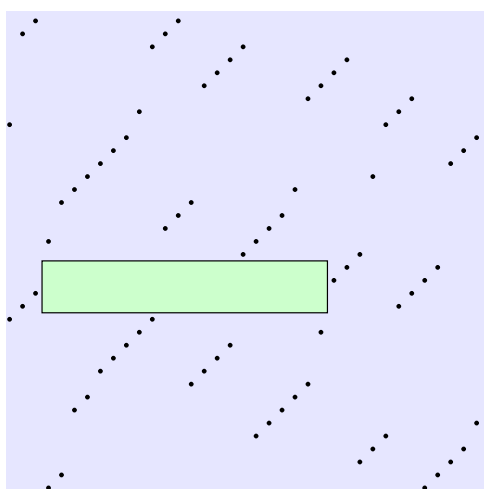

51. (2, 13, 29, 15)

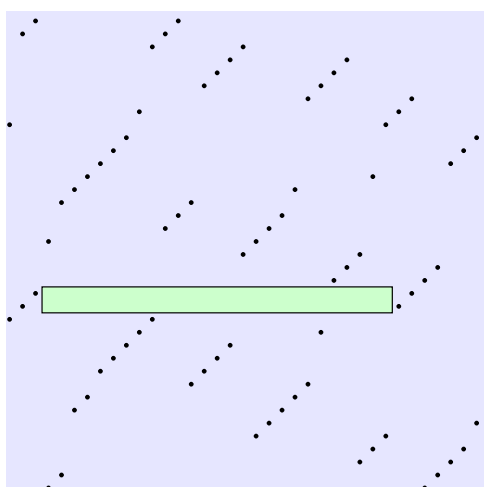

52.  $(2, 14, 30, 15)$

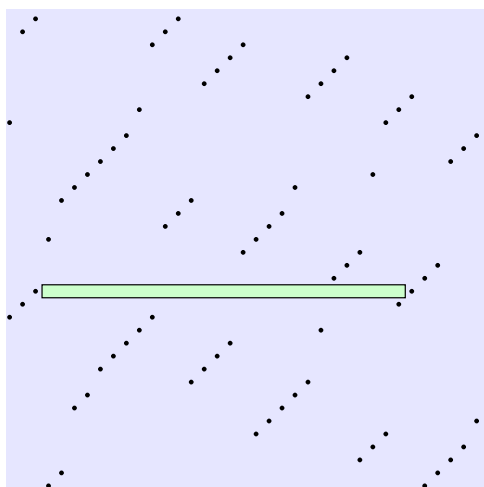

53.  $(2, 19, 3, 36)$

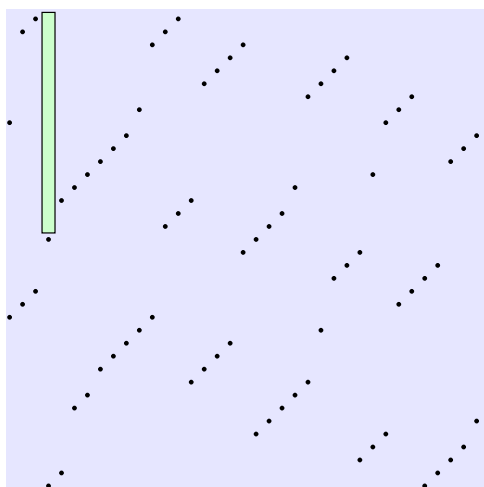

54.  $(2, 22, 4, 36)$

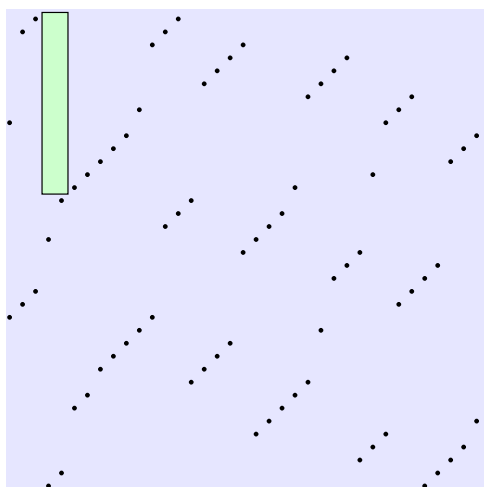

55.  $(2, 23, 5, 36)$

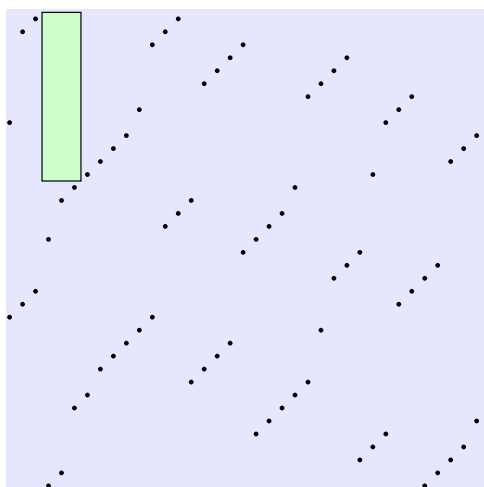

56.  $(2, 24, 6, 36)$

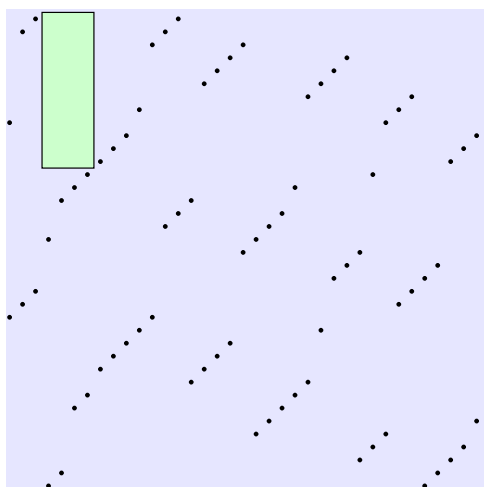

57.  $(2, 25, 7, 36)$

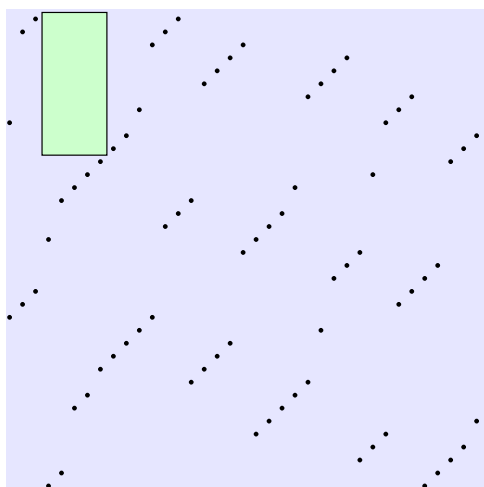

58. (2, 26, 8, 36)

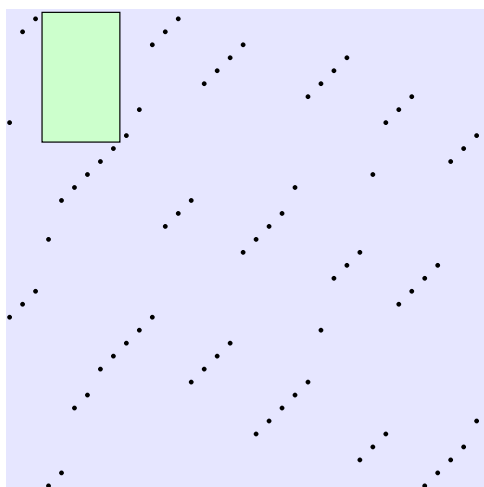

59. (2, 27, 9, 36)

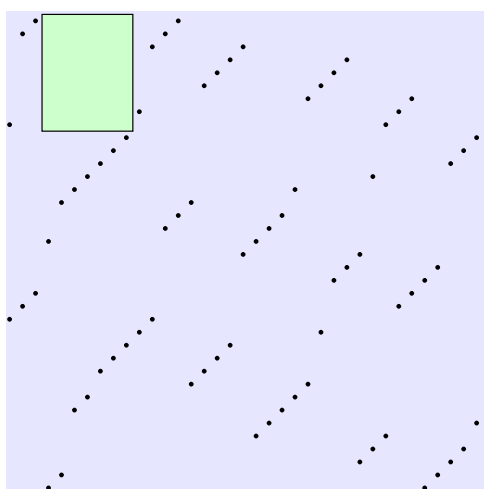

60. (2, 29, 10, 36)

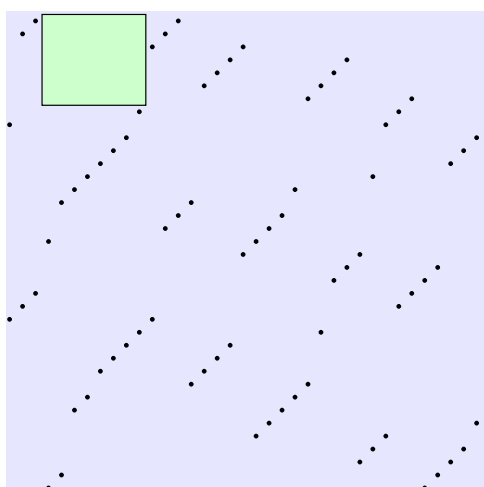

61.  $(2, 34, 11, 36)$

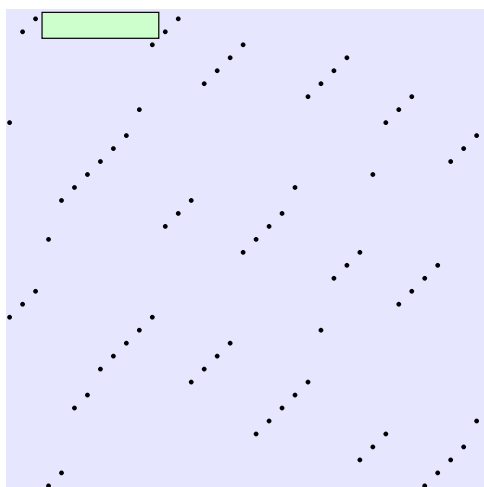

62.  $(2, 35, 12, 36)$

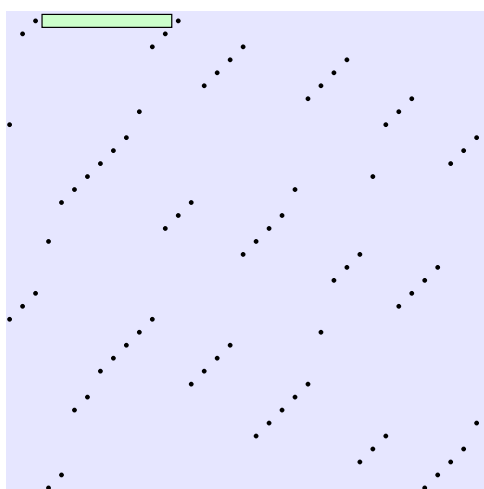

63.  $(3, 1, 4, 21)$

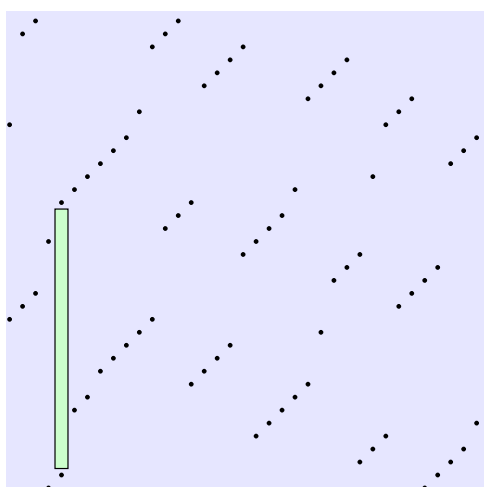

64.  $(3, 6, 5, 21)$

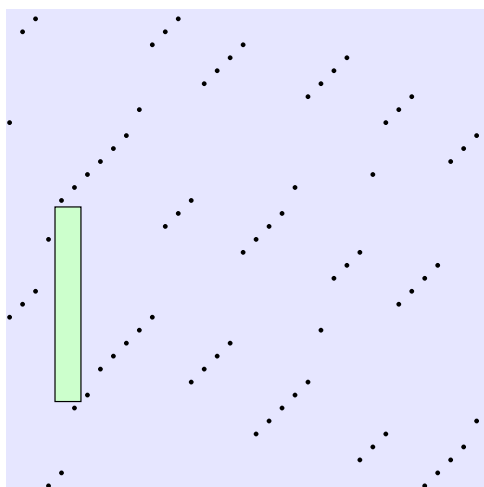

65.  $(3, 7, 6, 21)$

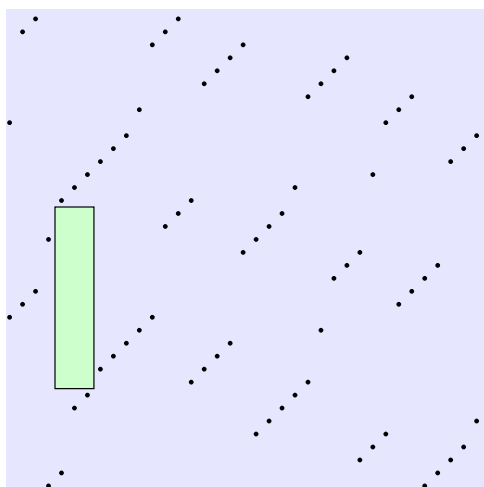

66.  $(3, 9, 7, 21)$

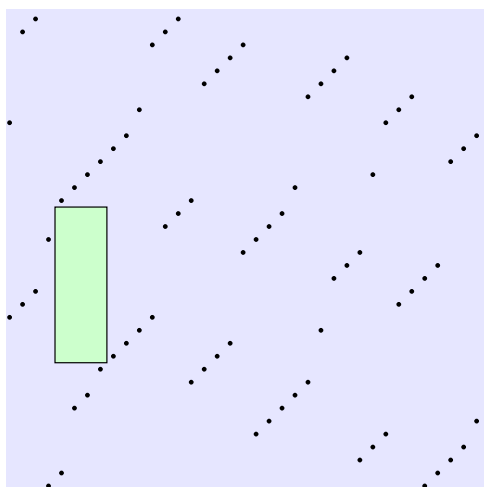

67.  $(3, 10, 8, 21)$

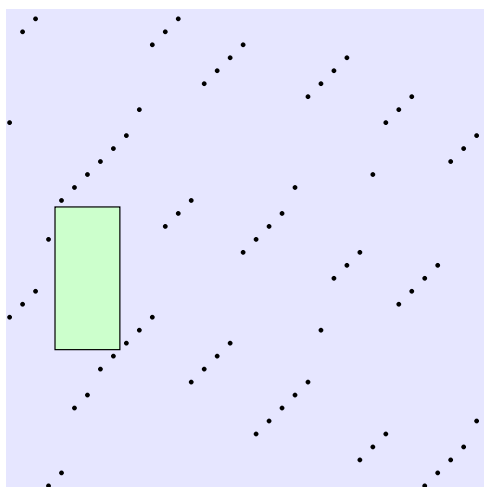

68.  $(3, 11, 9, 21)$

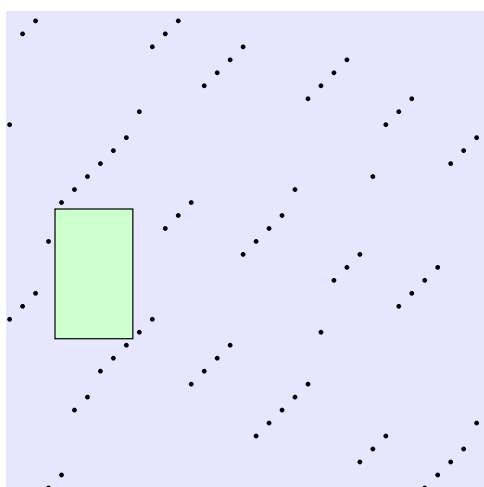

69.  $(3, 12, 10, 21)$

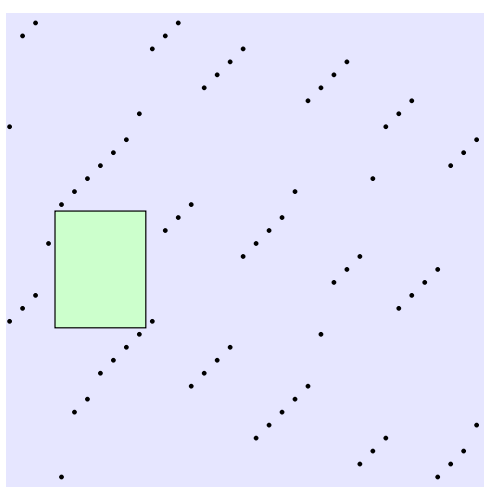

70.  $(3, 13, 11, 21)$

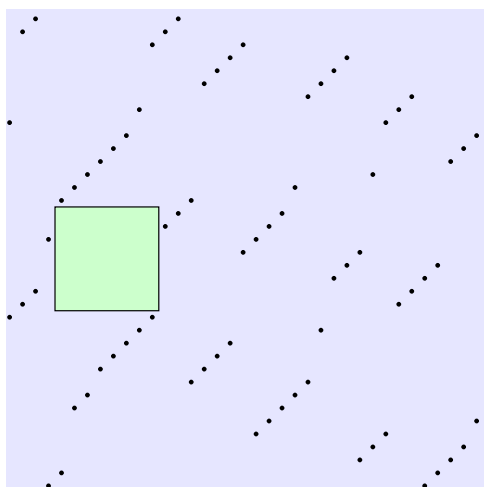

71.  $(3, 13, 17, 19)$

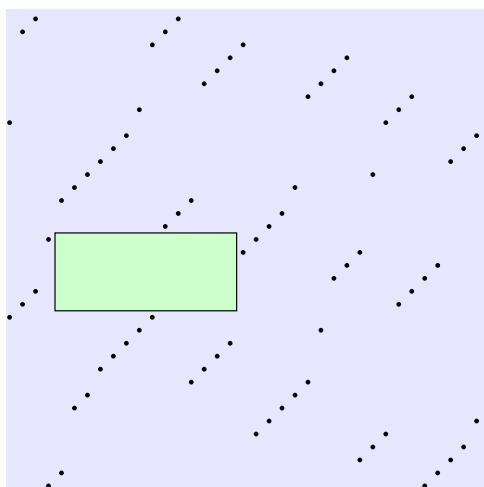

72.  $(3, 18, 18, 19)$

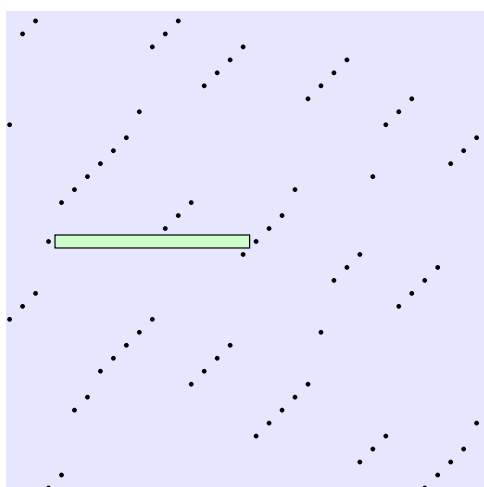



73.  $(3, 22, 4, 0)$

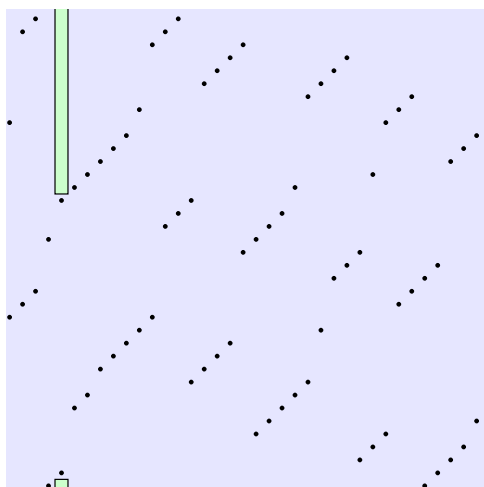

74.  $(3, 23, 5, 0)$

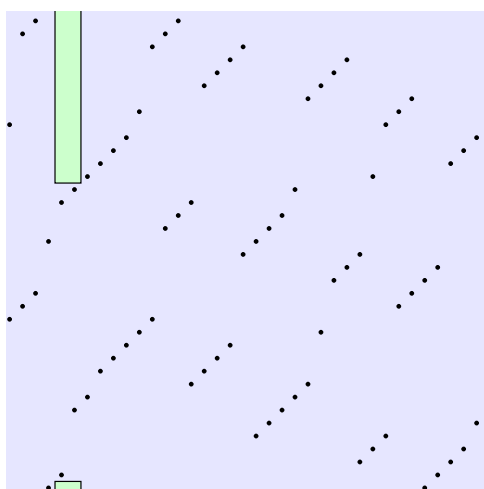

75.  $(3, 24, 6, 0)$

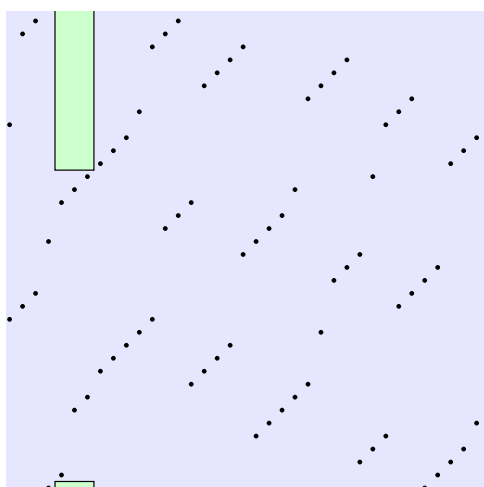

76.  $(3, 25, 7, 0)$

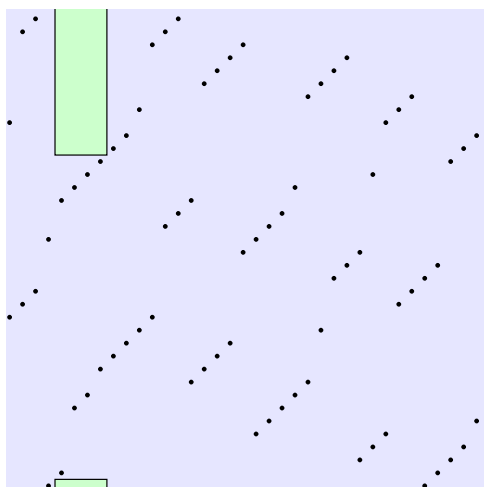

77.  $(3, 26, 8, 0)$

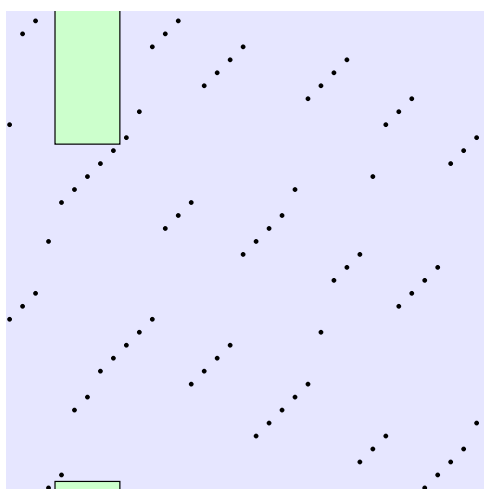

78.  $(3, 27, 9, 0)$

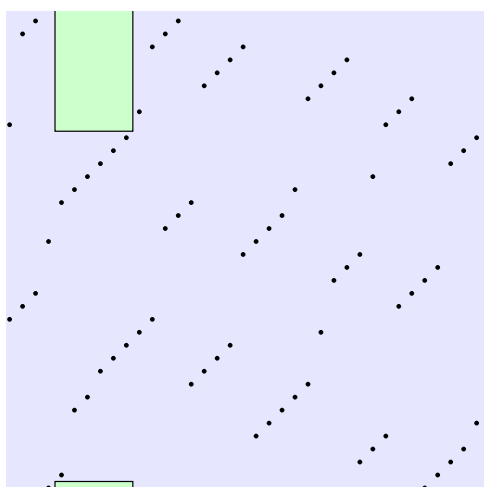

79.  $(3, 29, 10, 0)$

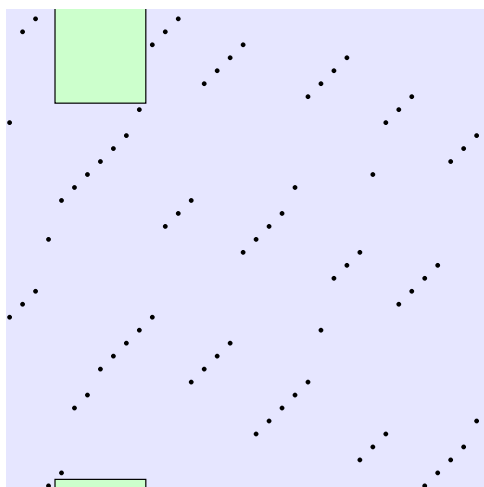

80.  $(3, 34, 11, 0)$

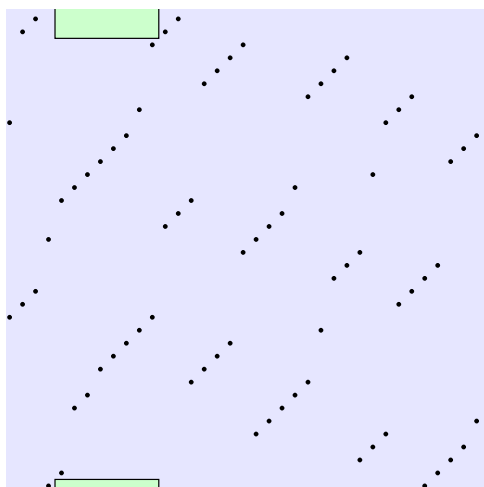

81.  $(3, 35, 12, 0)$

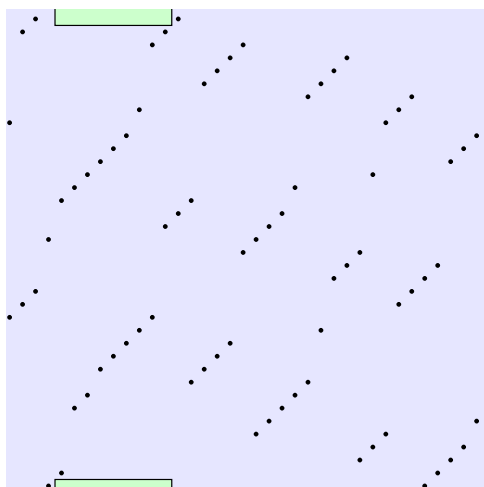

82.  $(3, 36, 31, 0)$

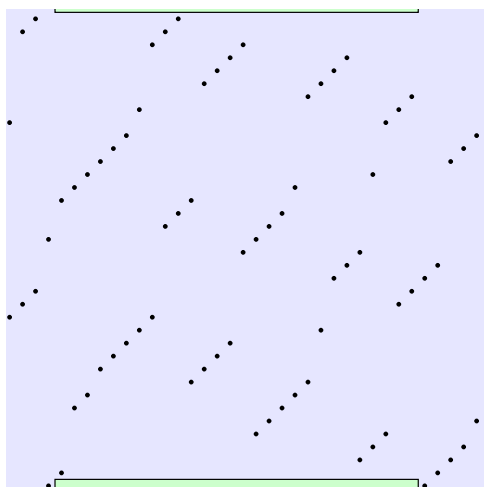

83.  $(4, 0, 32, 1)$

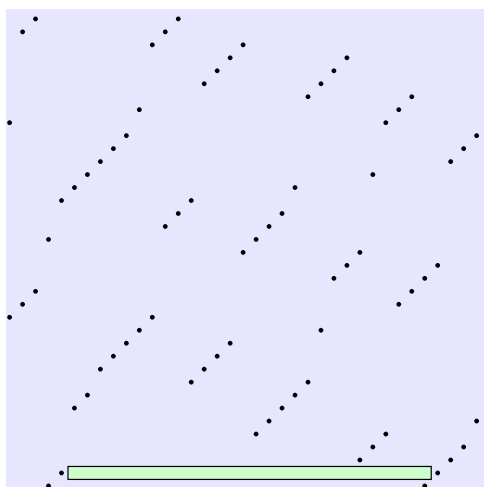

84.  $(4, 6, 5, 22)$

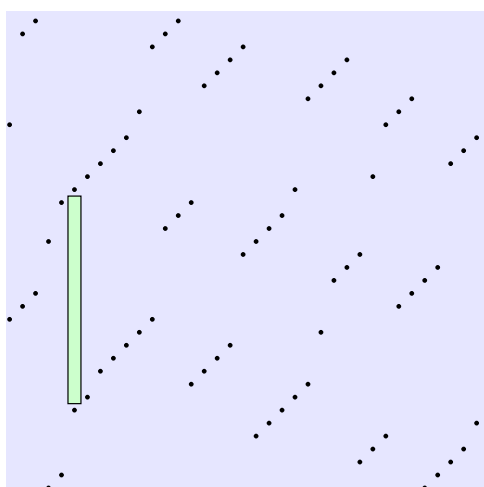

85. (4, 7, 6, 22)

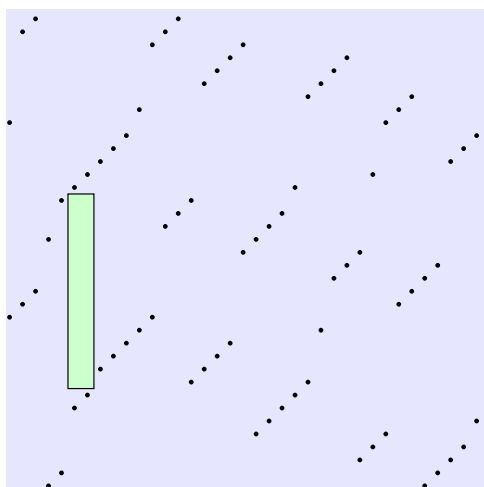

86. (4, 9, 7, 22)

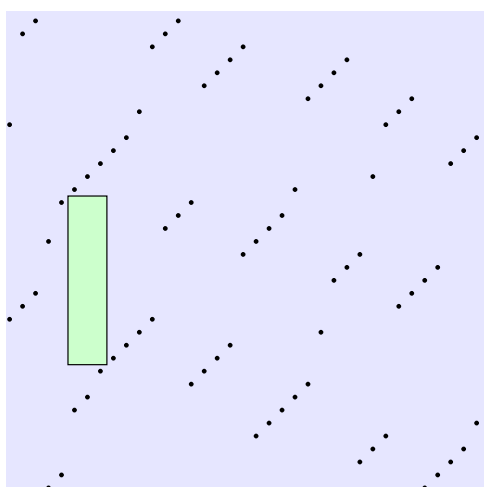

87. (4, 10, 8, 22)

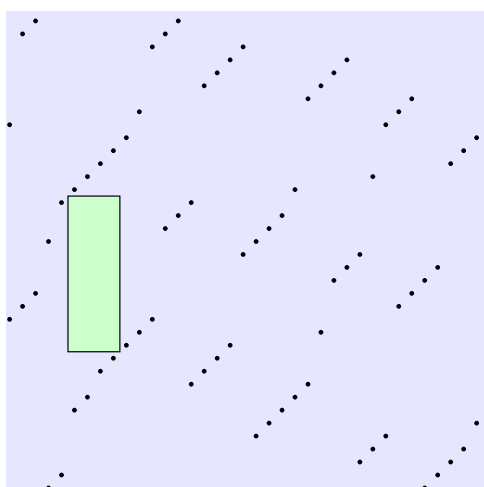

88. (4, 11, 9, 22)

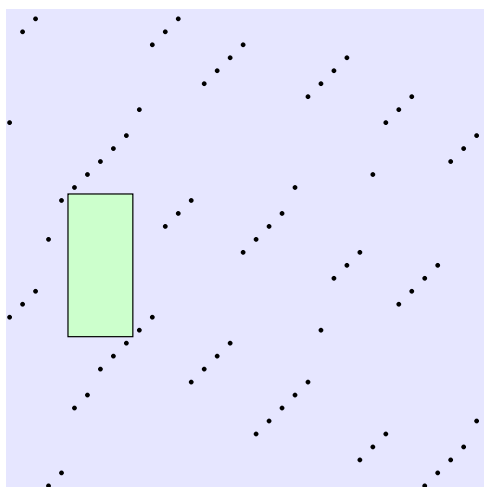

89. (4, 12, 10, 22)

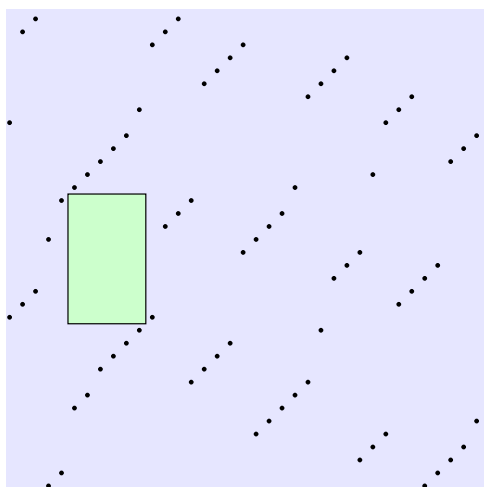

90. (4, 13, 11, 22)

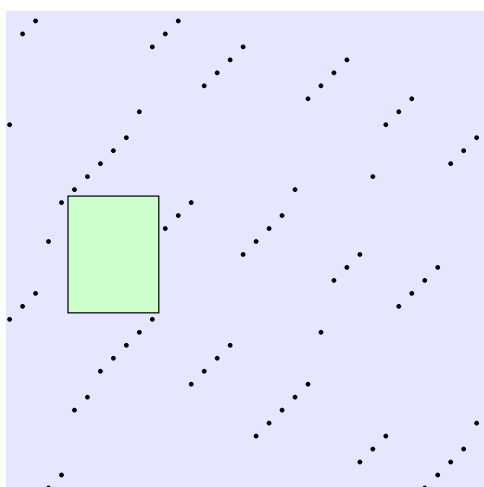

91.  $(4, 20, 12, 22)$

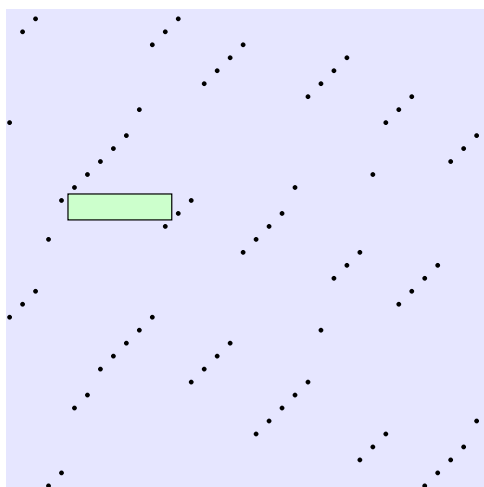

92.  $(4, 21, 13, 22)$

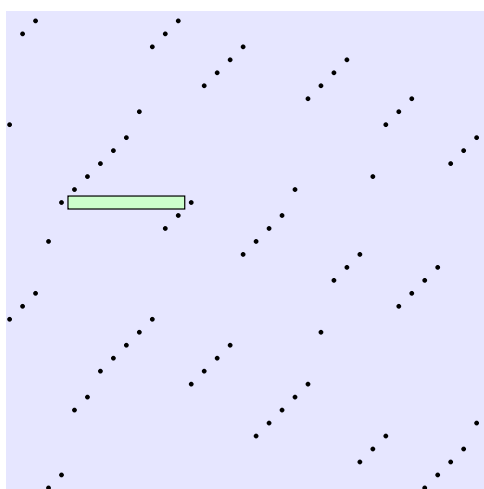

93.  $(4, 23, 5, 5)$

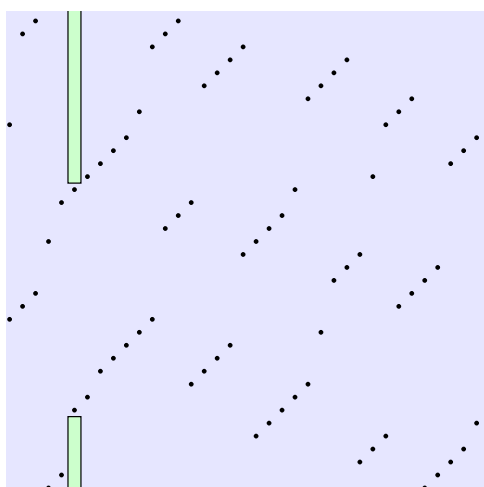

94. (4, 24, 6, 5)

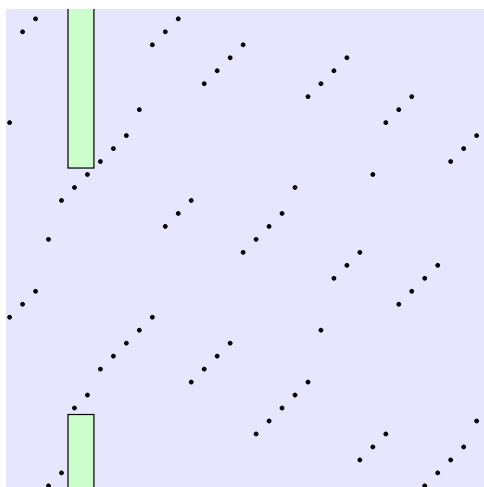

95. (4, 25, 7, 5)

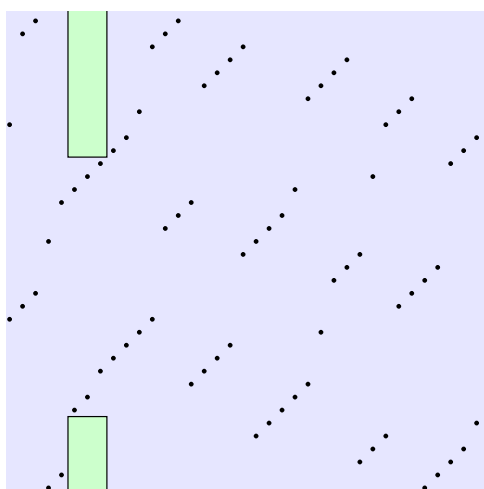

96. (4, 26, 8, 5)

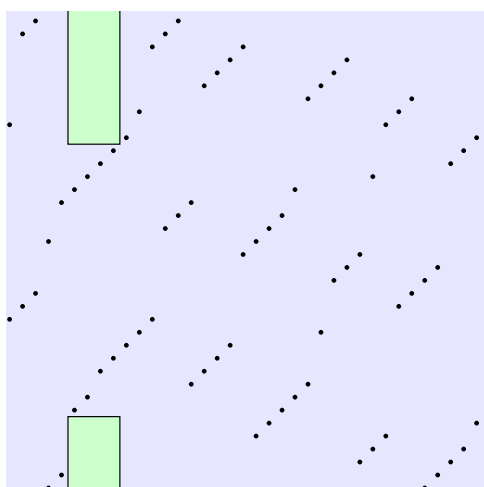



97. (4, 27, 9, 5)

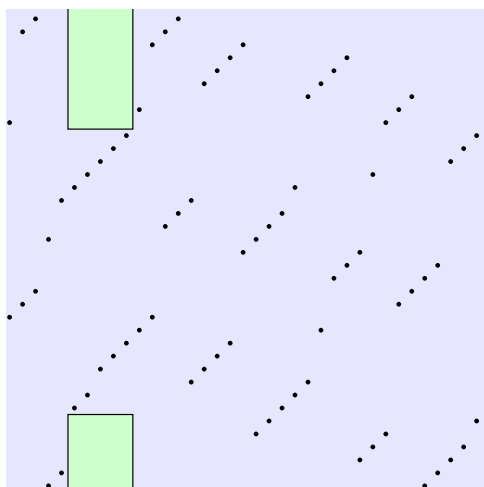

98. (4, 29, 10, 5)

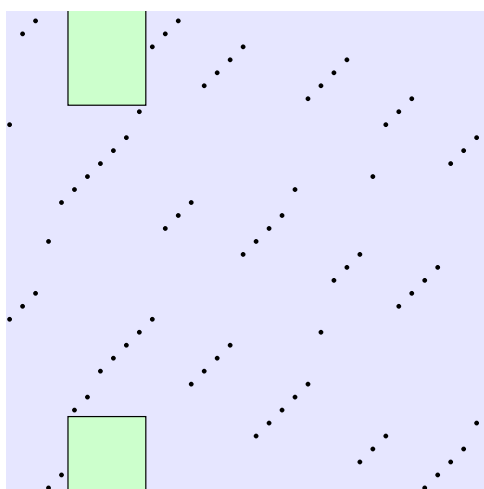

99. (4, 34, 11, 5)

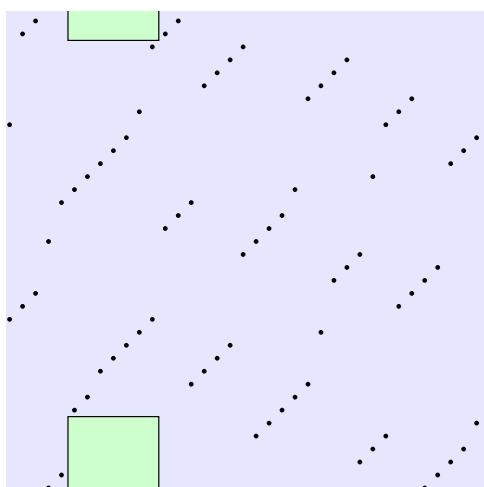

100.  $(4, 35, 12, 5)$

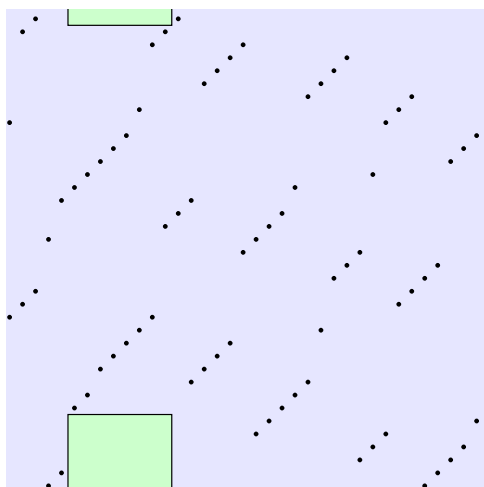

101.  $(4, 36, 18, 5)$

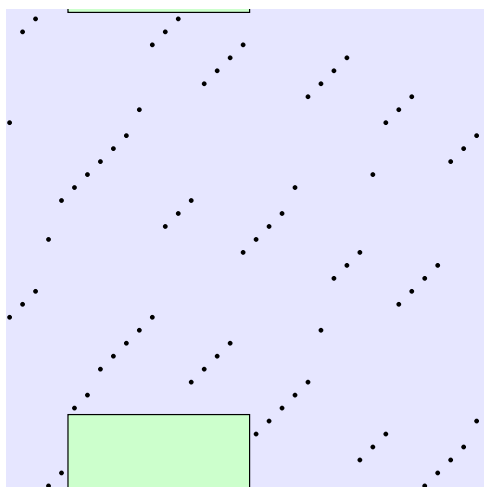

102.  $(4, 36, 26, 3)$

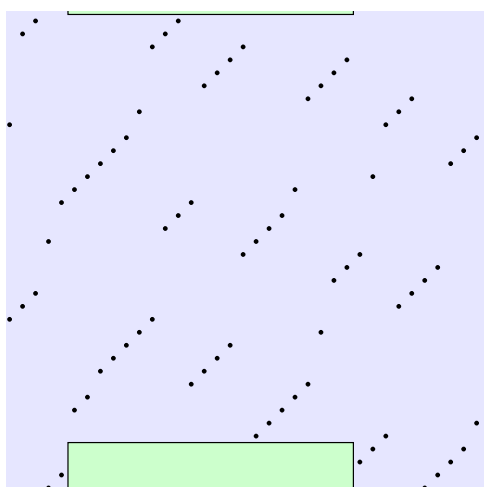

103.  $(4, 36, 31, 1)$

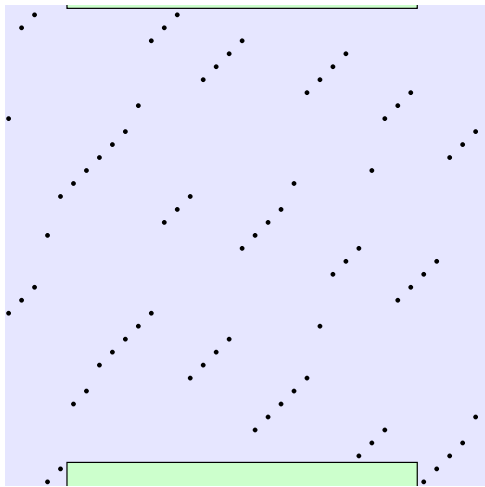

104.  $(5, 4, 19, 6)$

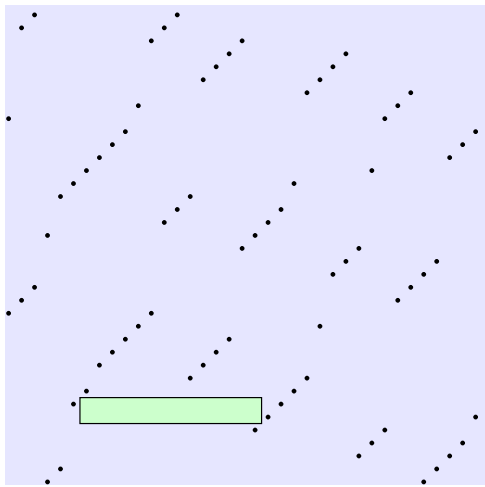

105.  $(5, 5, 20, 6)$

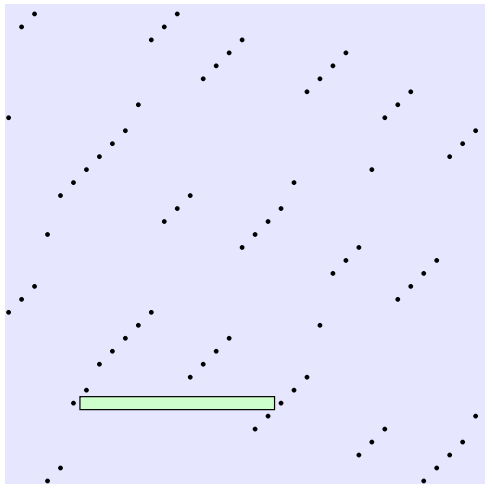

106. (5, 7, 6, 23)

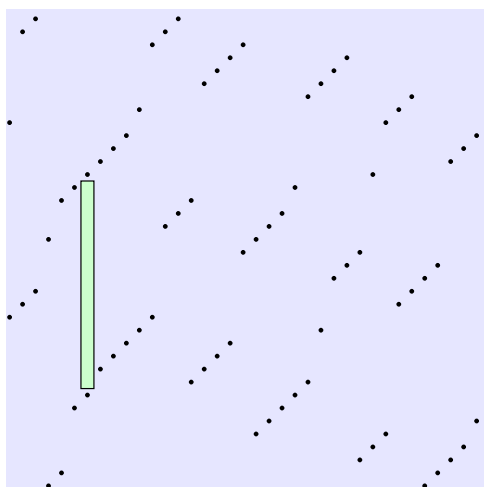

107. (5, 9, 7, 23)

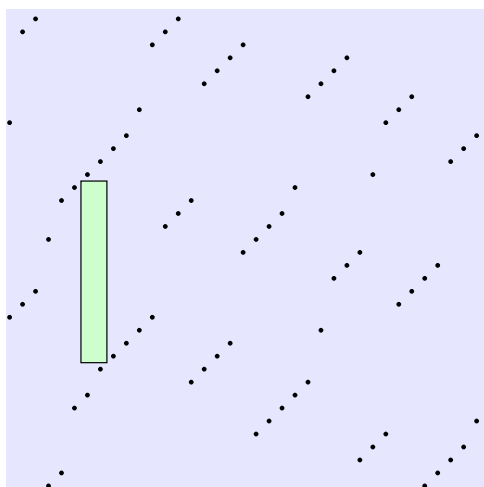

108. (5, 10, 8, 23)

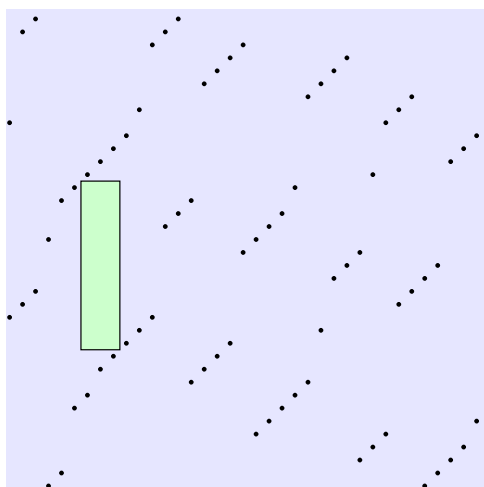

109. (5, 11, 9, 23)

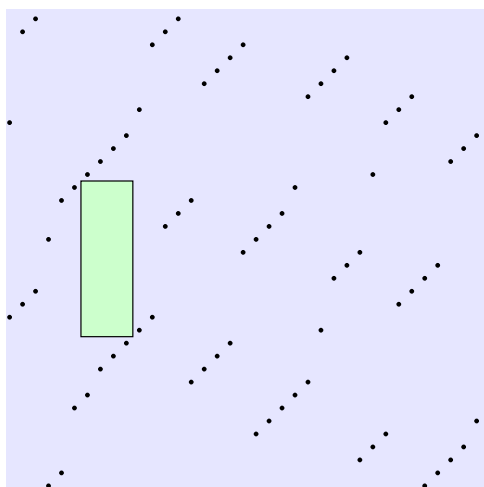

110. (5, 12, 10, 23)

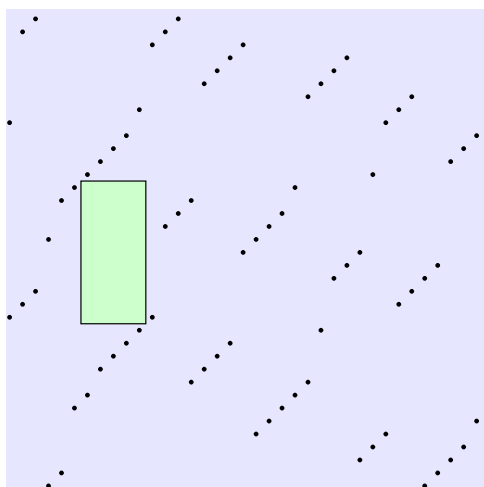

111. (5, 13, 11, 23)

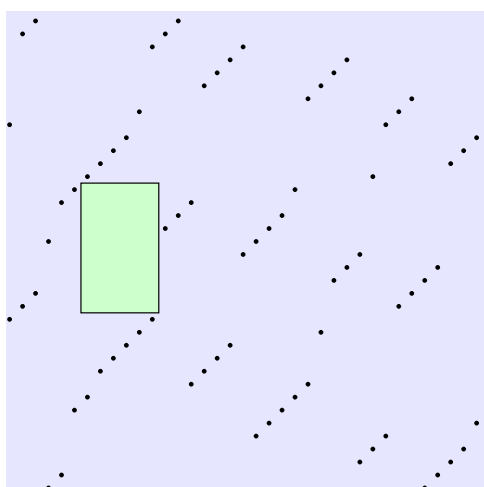

112. (5, 20, 12, 23)

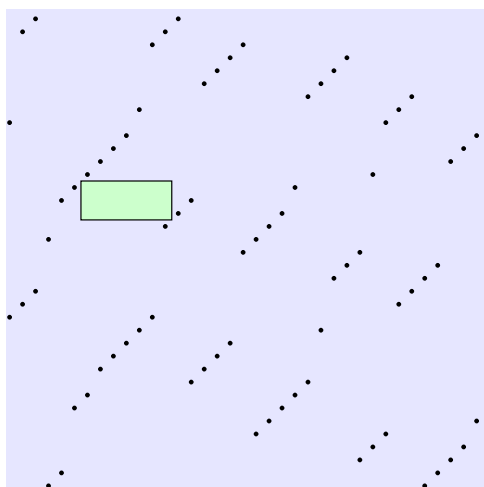

113. (5, 21, 13, 23)

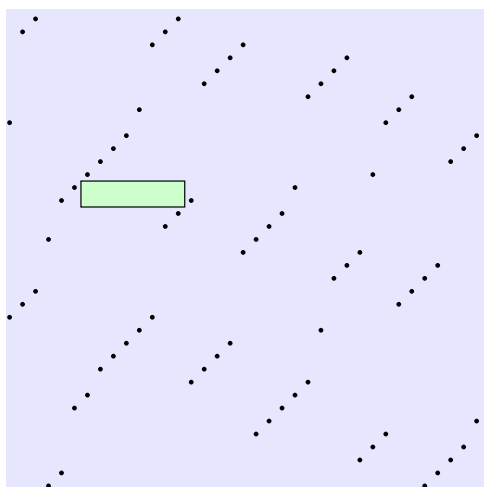

114. (5, 22, 21, 23)

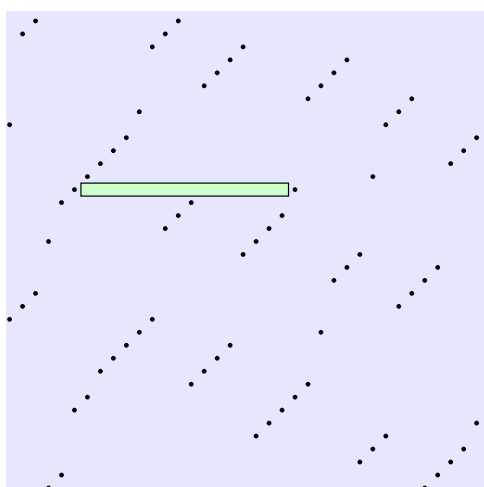

115. (5, 24, 6, 6)

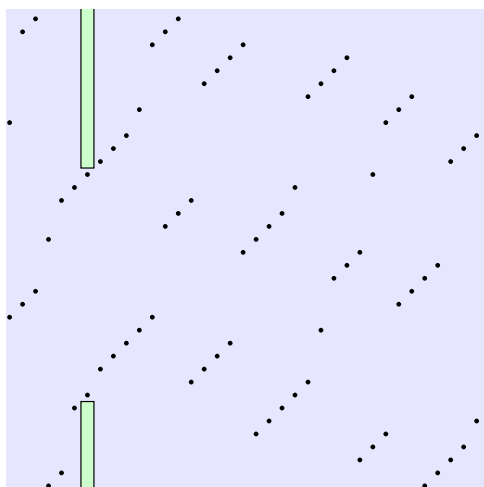

116. (5, 25, 7, 6)

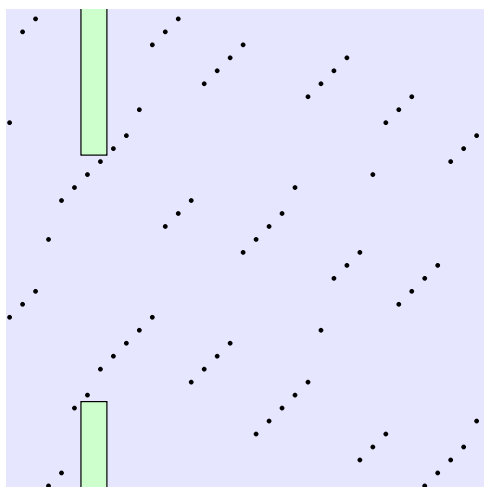

117. (5, 26, 8, 6)

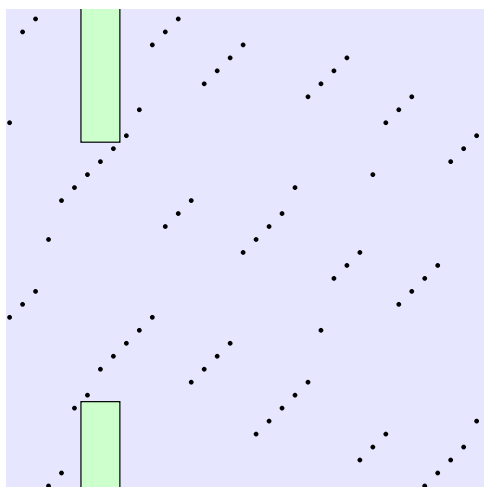

118. (5, 27, 9, 6)

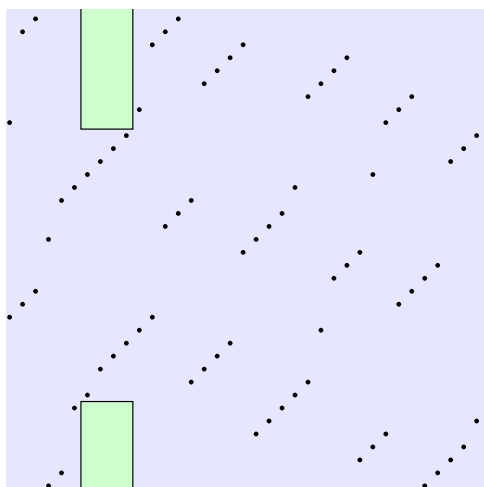

119. (5, 29, 10, 6)

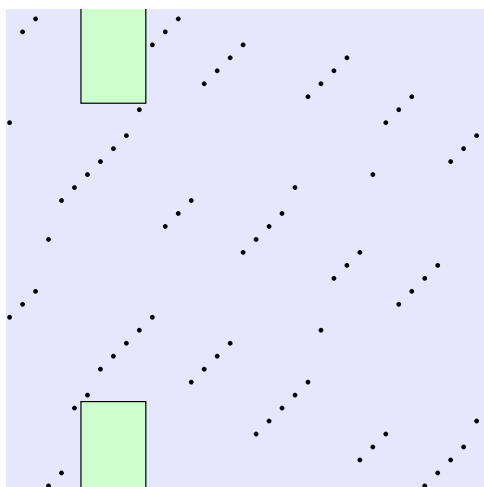

120. (5, 34, 11, 6)

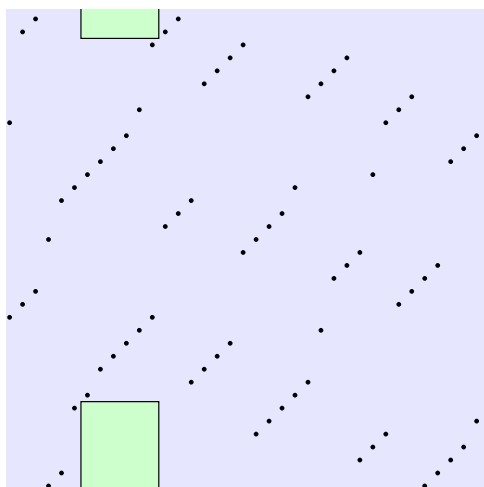



121. (5, 35, 12, 6)

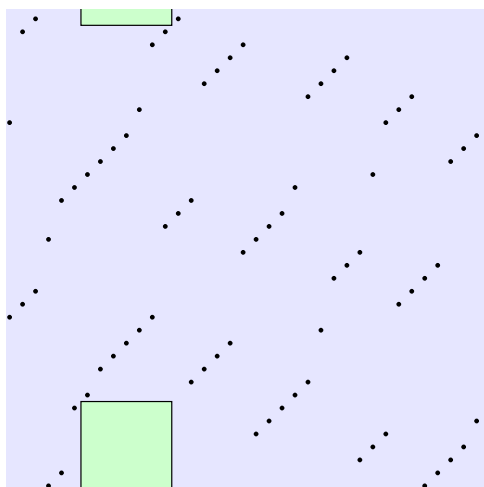

122. (5, 36, 18, 6)

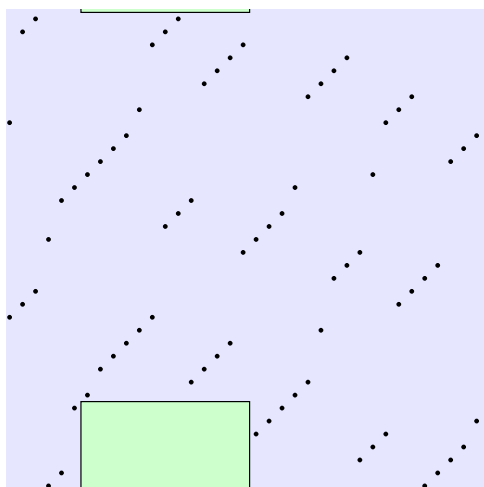

123. (6, 4, 19, 7)

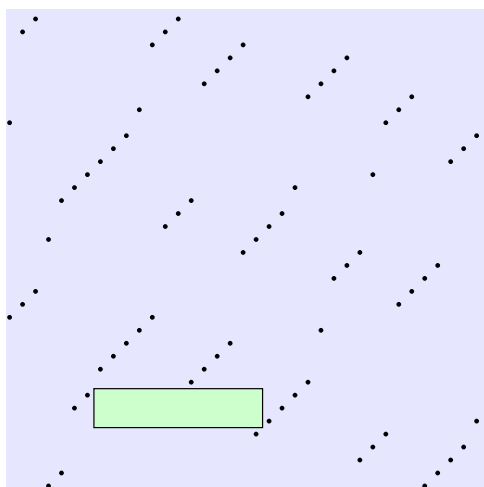

124. (6, 5, 20, 7)

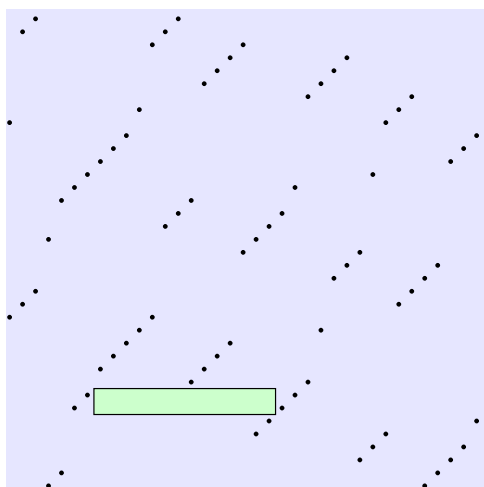

125. (6, 6, 21, 7)

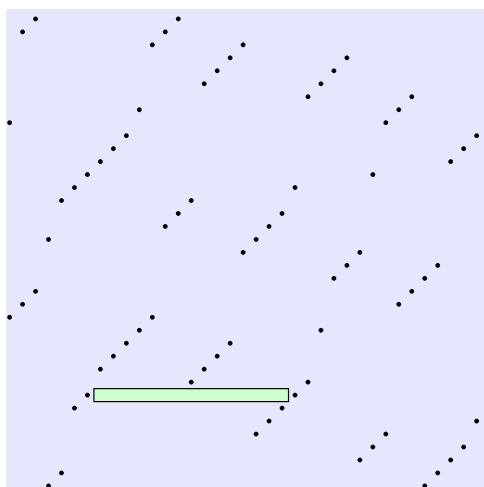

126. (6, 9, 7, 24)

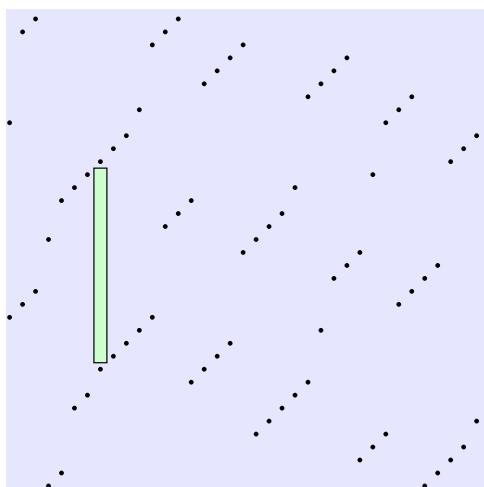

127. (6, 10, 8, 24)

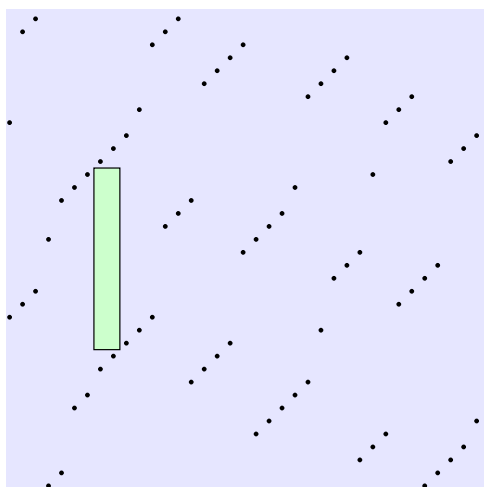

128. (6, 11, 9, 24)

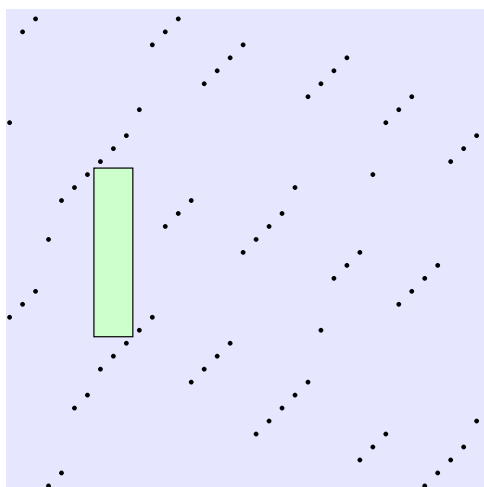

129. (6, 12, 10, 24)

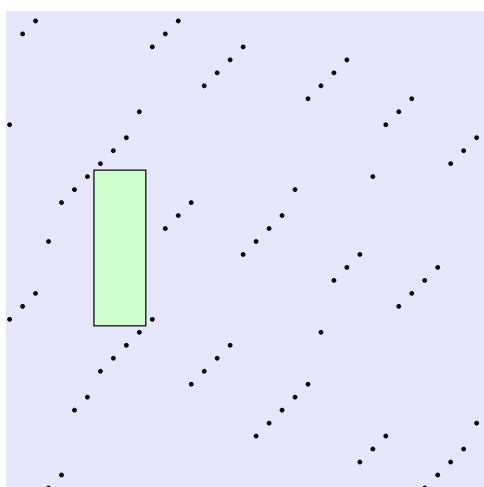

130. (6, 13, 11, 24)

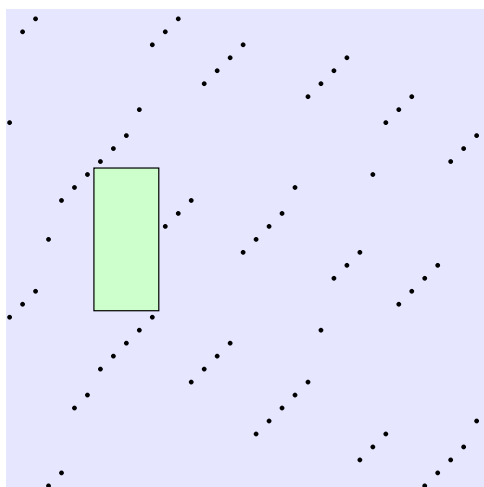

131. (6, 20, 12, 24)

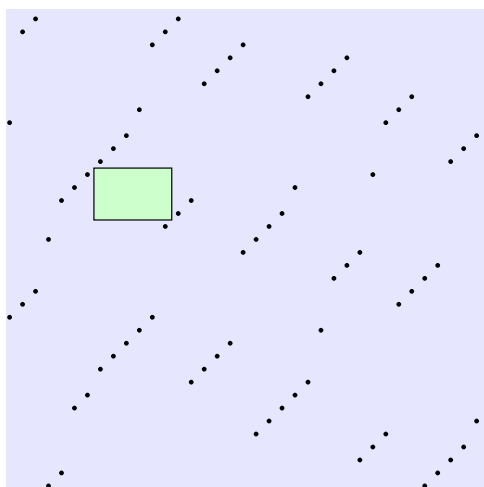

132. (6, 21, 13, 24)

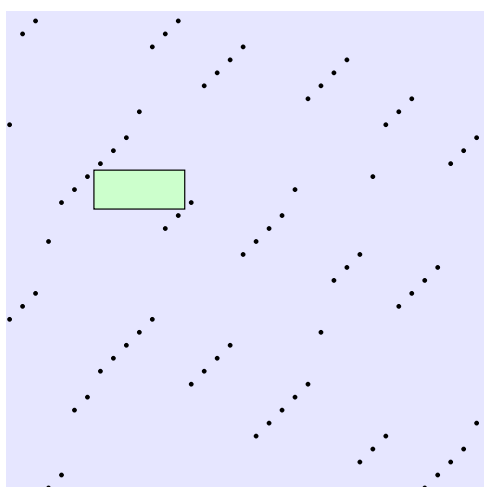

133. (6, 22, 21, 24)

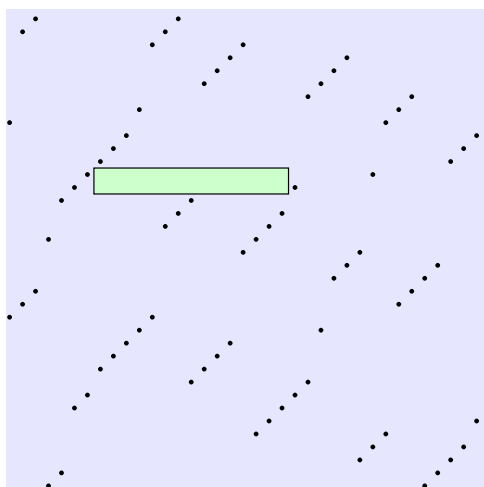

134. (6, 23, 27, 24)

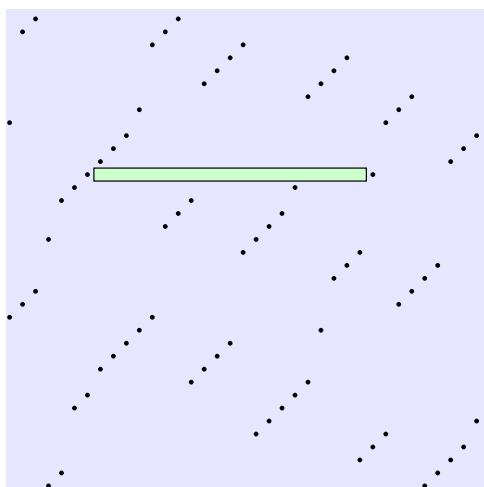

135. (6, 25, 7, 8)

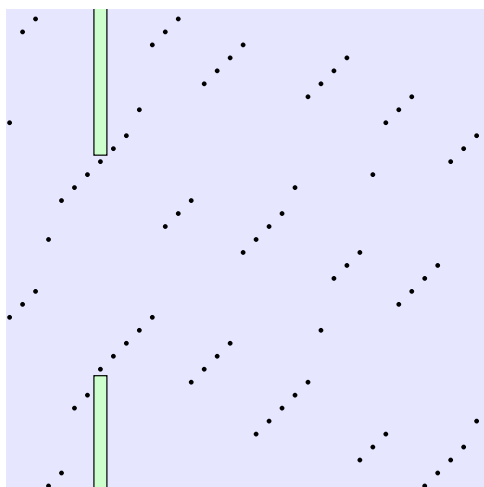

136. (6, 26, 8, 8)

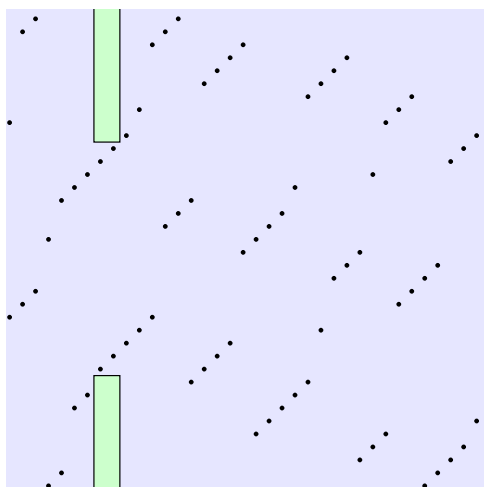

137. (6, 27, 9, 8)

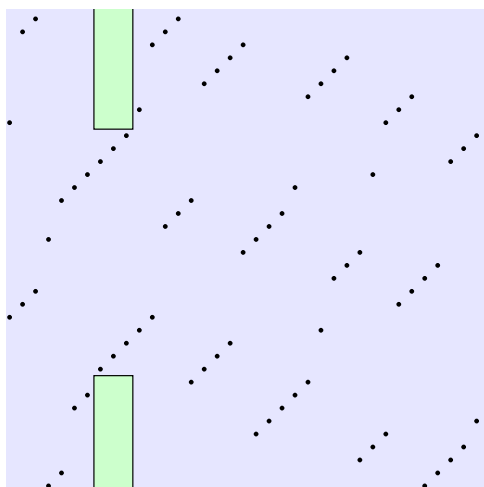

138. (6, 29, 10, 8)

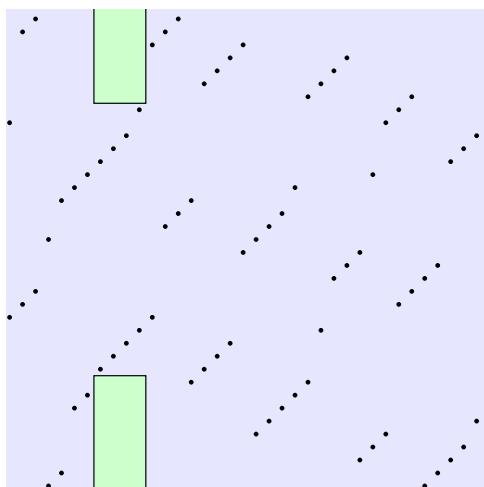

139. (6, 34, 11, 8)

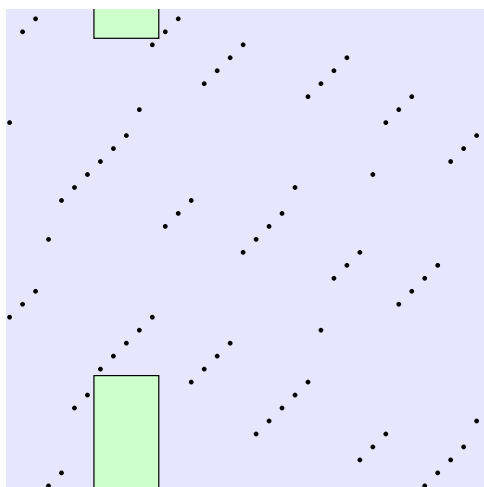

140. (6, 35, 12, 8)

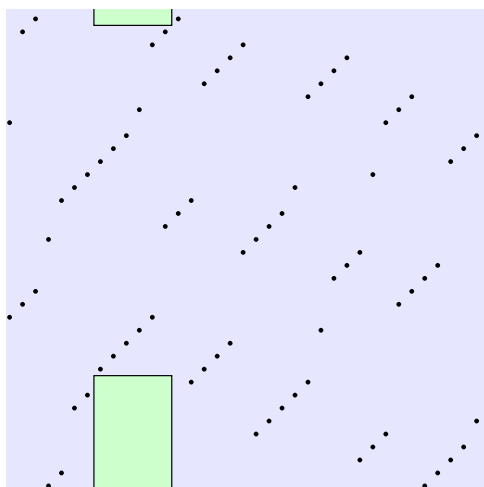

141. (6, 36, 13, 8)

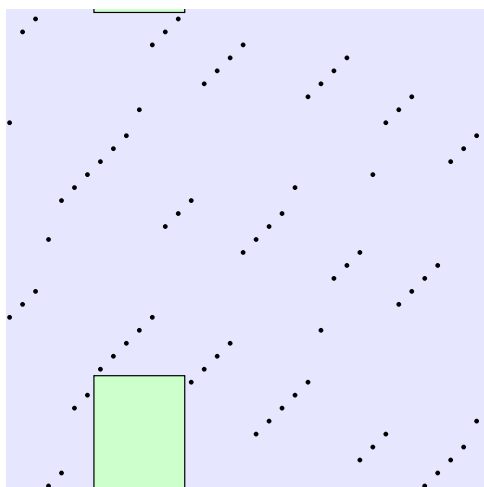

142. (6, 36, 18, 7)

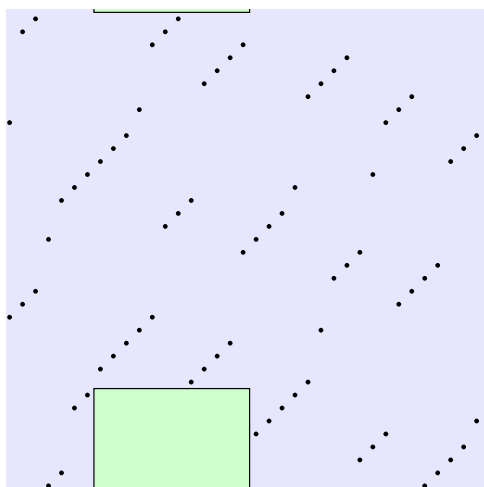

143. (7, 8, 14, 9)

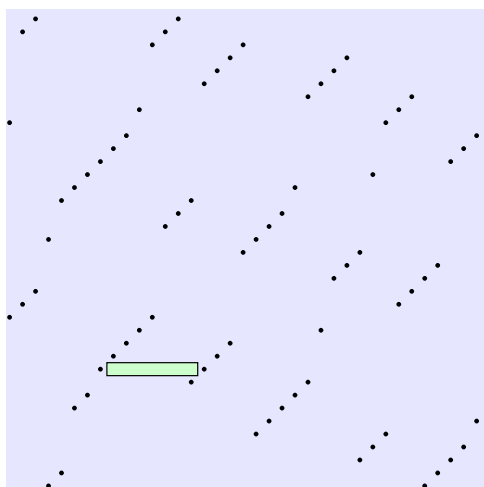

144. (7, 10, 8, 25)

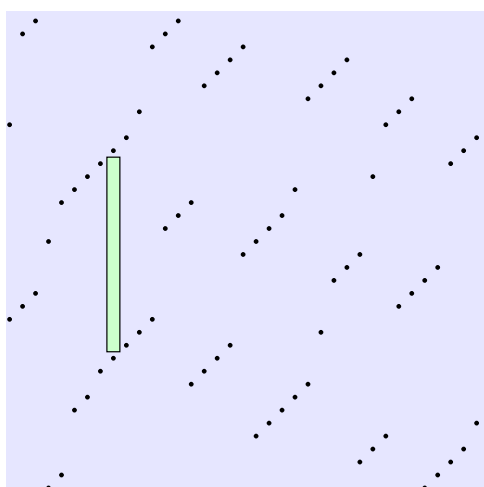



145. (7, 11, 9, 25)

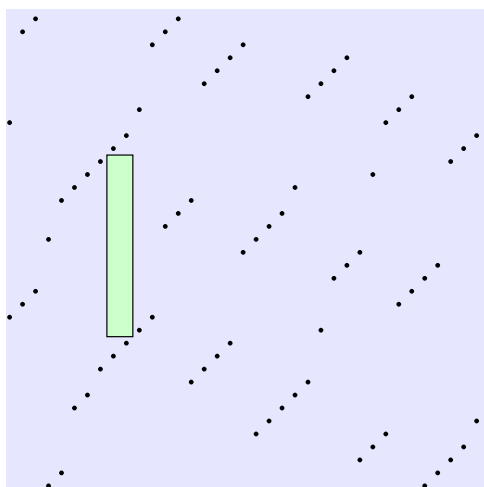

146. (7, 12, 10, 25)

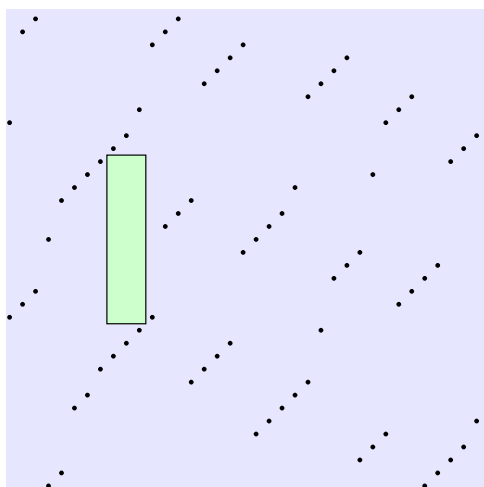

147. (7, 13, 11, 25)

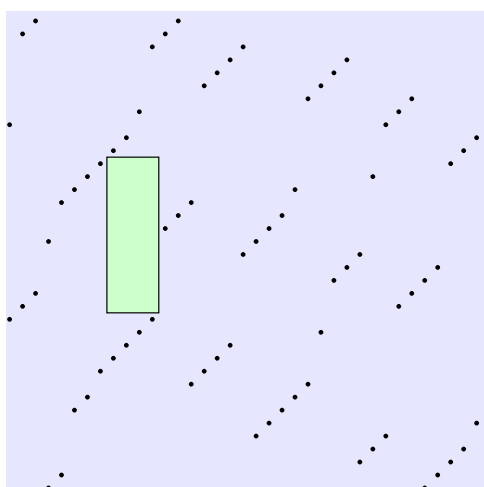

148. (7, 20, 12, 25)

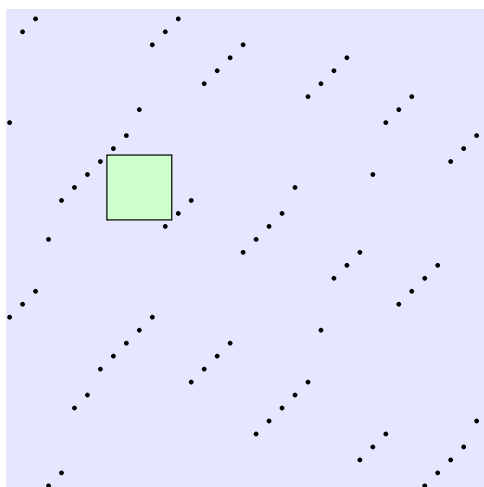

149. (7, 21, 13, 25)

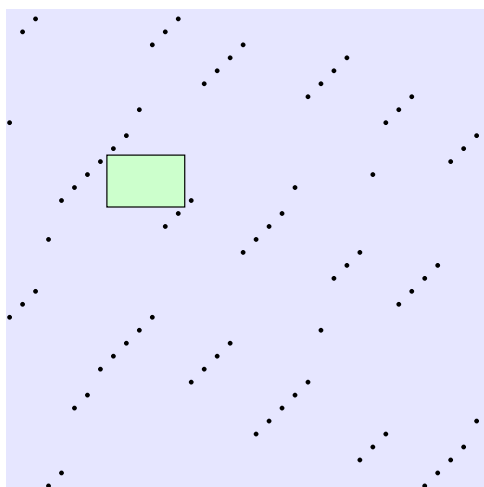

150. (7, 22, 21, 25)

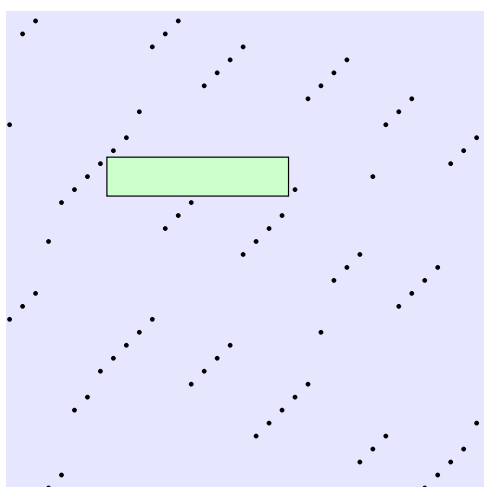

151. (7, 23, 27, 25)

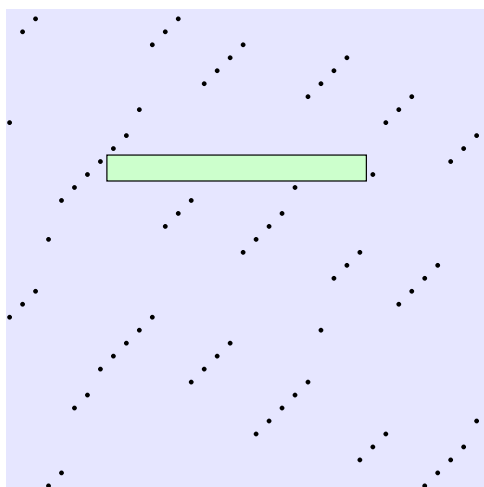

152. (7, 24, 33, 25)

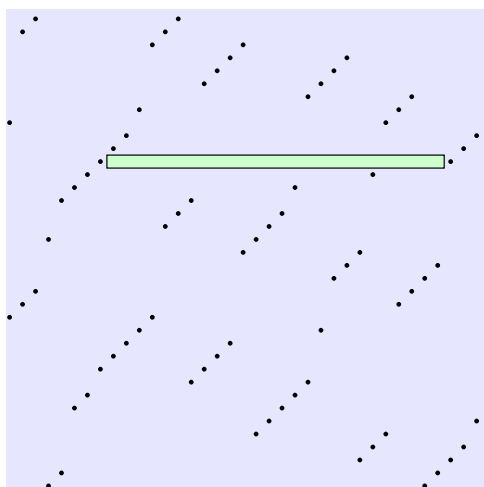

153. (7, 26, 8, 9)

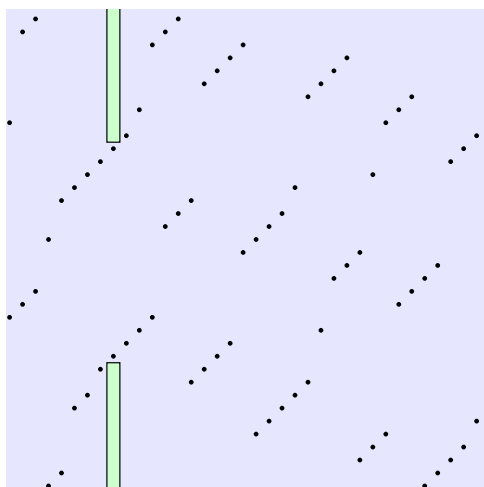

154. (7, 27, 9, 9)

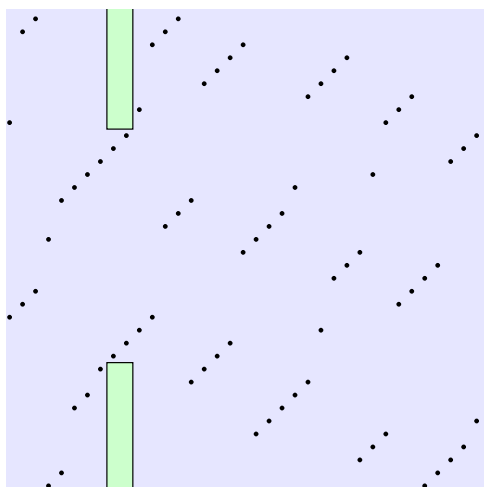

155. (7, 29, 10, 9)

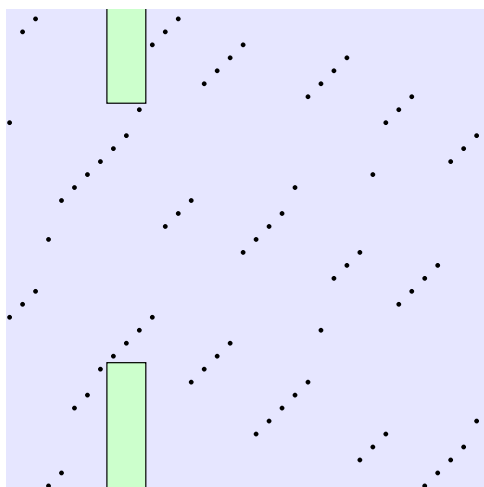

156. (7, 34, 11, 9)

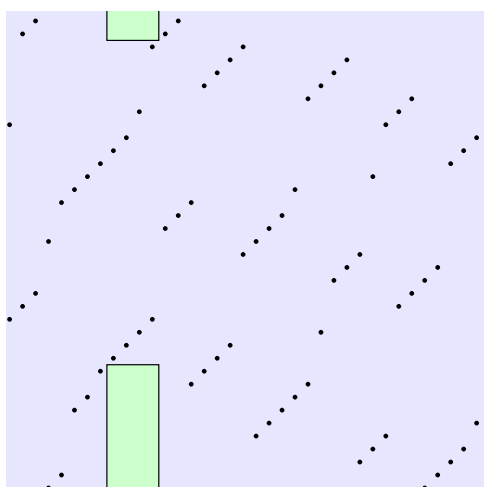

157. (7, 35, 12, 9)

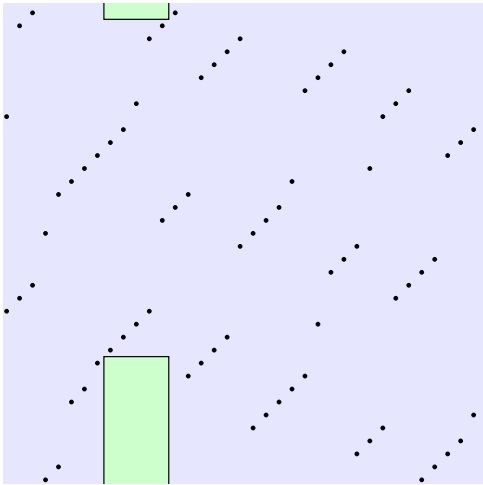

158. (7, 36, 13, 9)

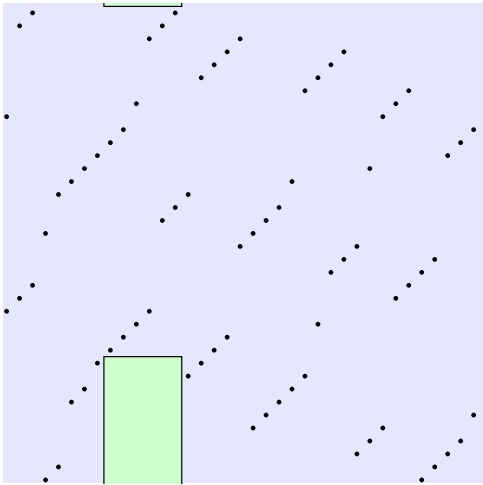

159. (8, 8, 14, 10)

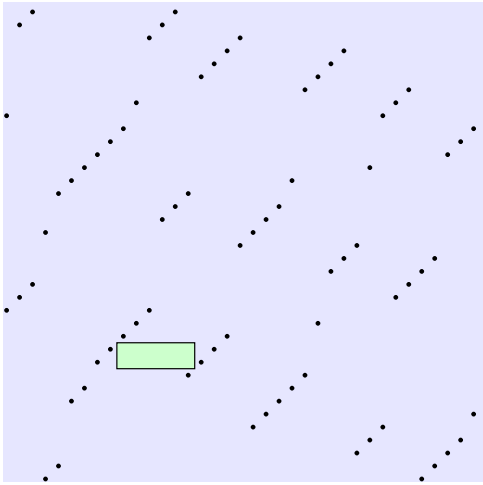

160. (8, 9, 15, 10)

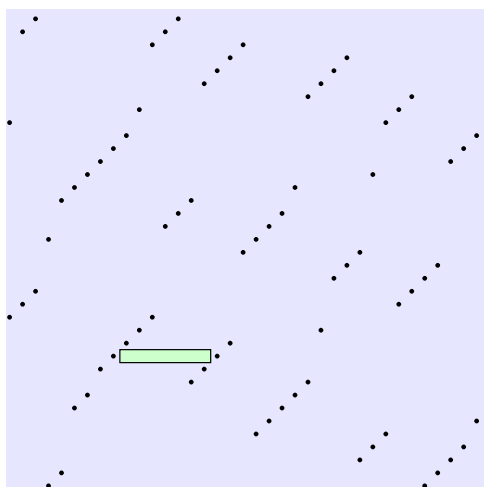

161. (8, 11, 9, 26)

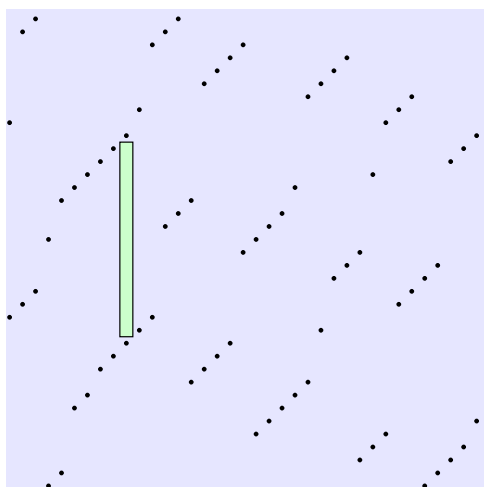

162. (8, 12, 10, 26)

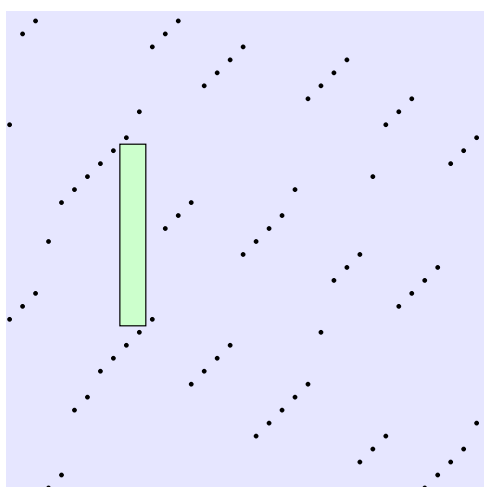

163. (8, 13, 11, 26)

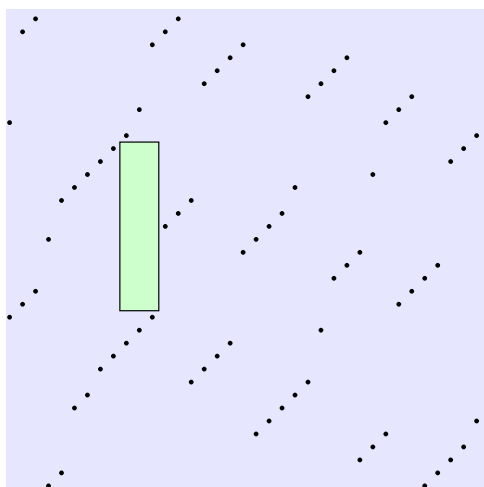

164. (8, 20, 12, 26)

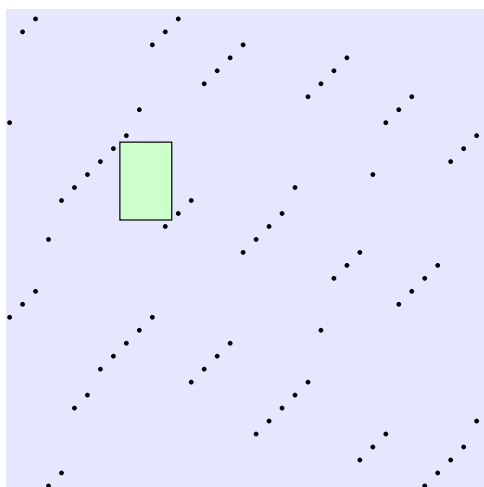

165. (8, 21, 13, 26)

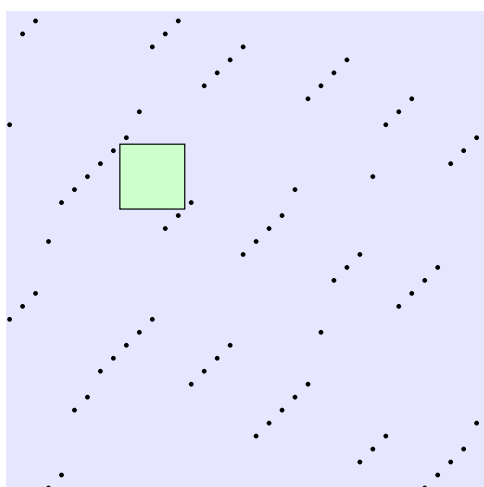

166. (8, 22, 21, 26)

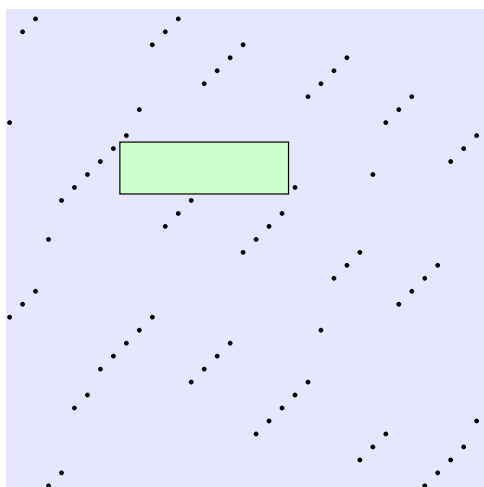

167. (8, 23, 27, 26)

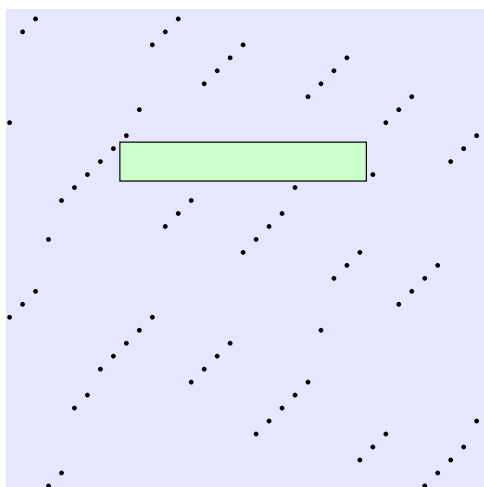

168. (8, 24, 33, 26)

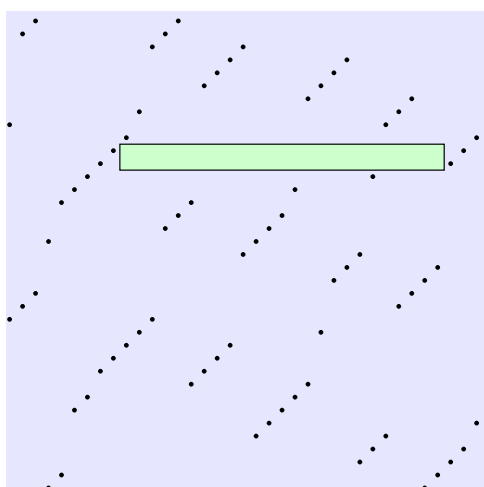



169. (8, 25, 34, 26)

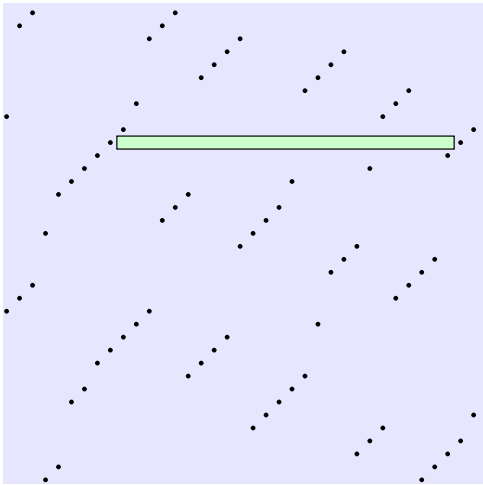

170. (8, 27, 9, 10)

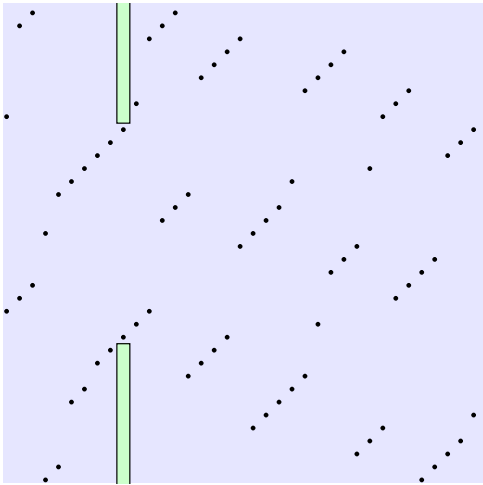

171. (8, 29, 10, 10)

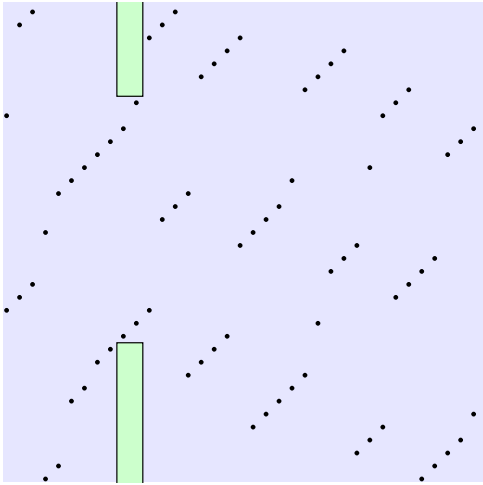

172. (8, 34, 11, 10)

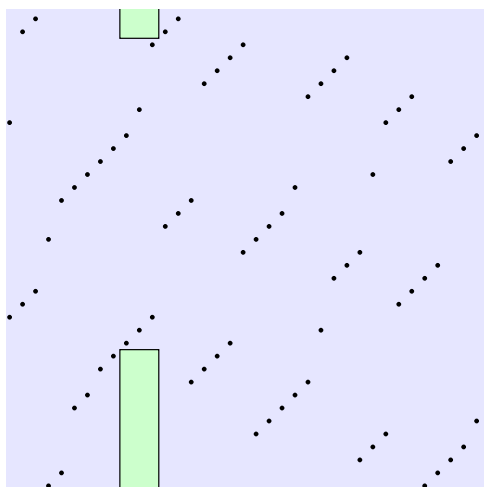

173. (8, 35, 12, 10)

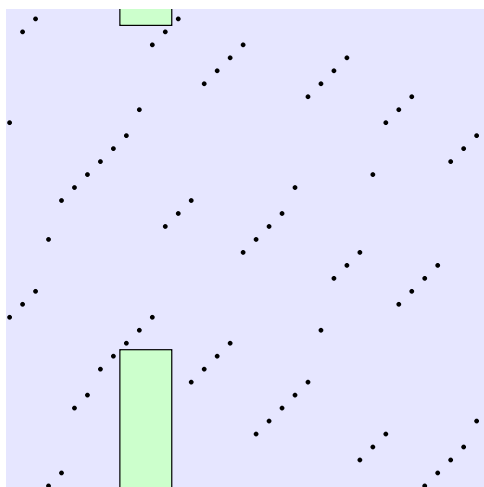

174. (8, 36, 13, 10)

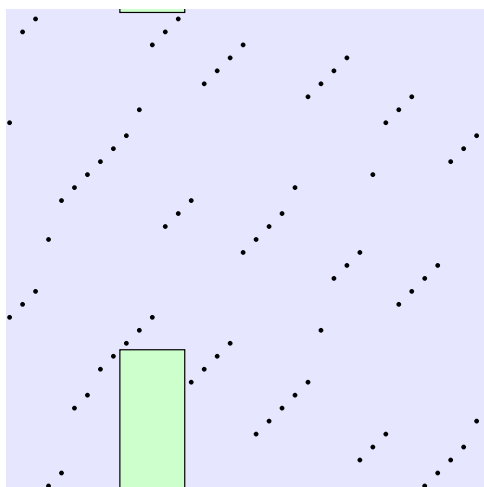

175. (9, 8, 14, 11)

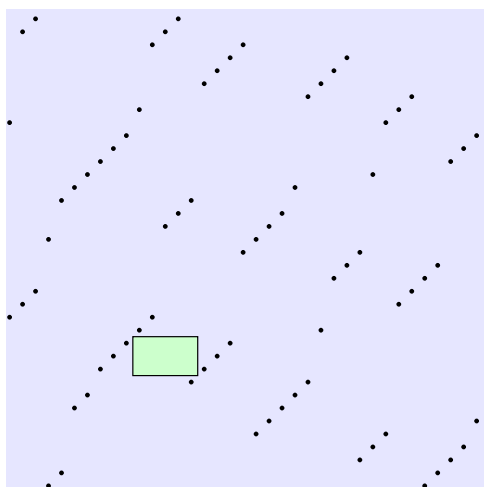

176. (9, 9, 15, 11)

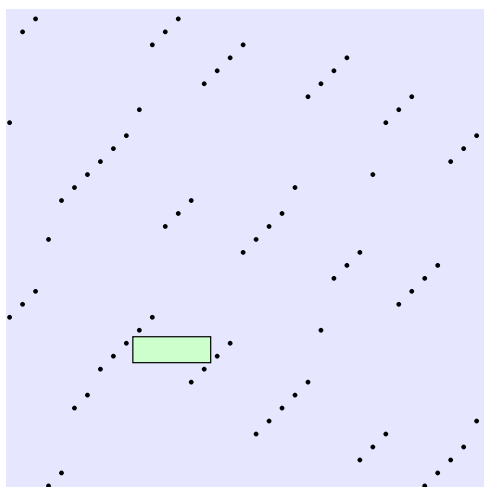

177. (9, 10, 16, 11)

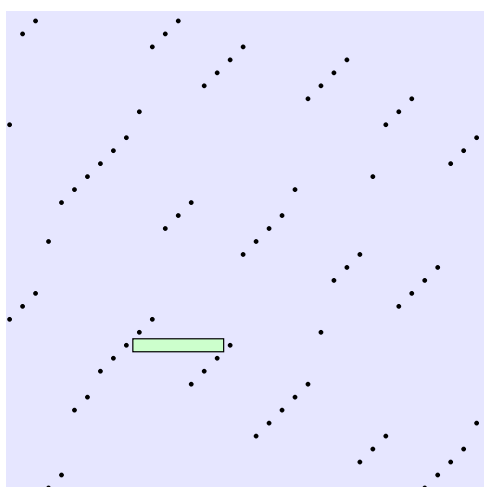

178. (9, 12, 10, 28)

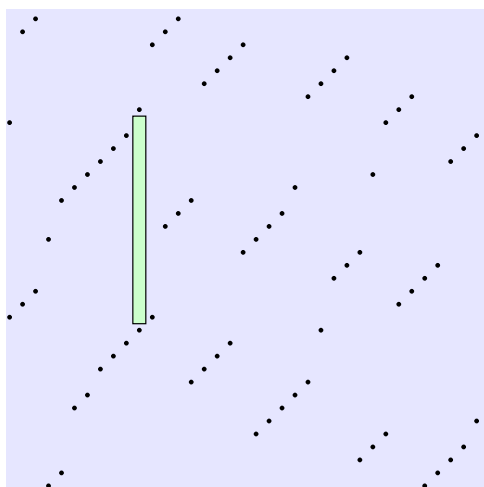

179. (9, 13, 11, 28)

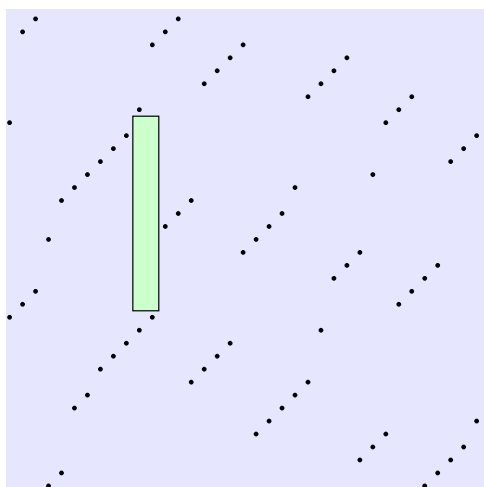

180. (9, 20, 12, 28)

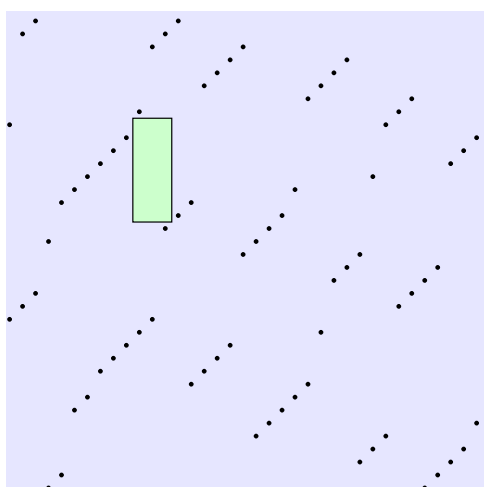

181. (9, 21, 13, 28)

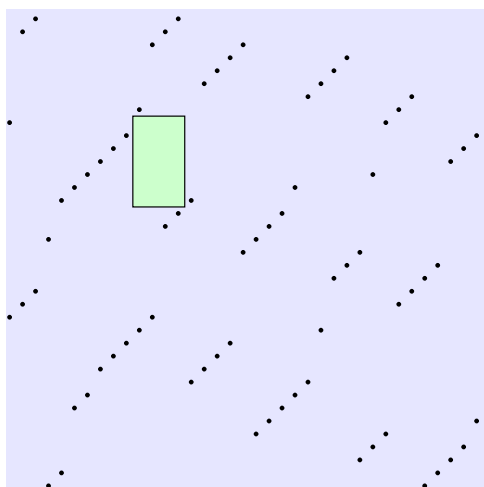

182. (9, 22, 21, 28)

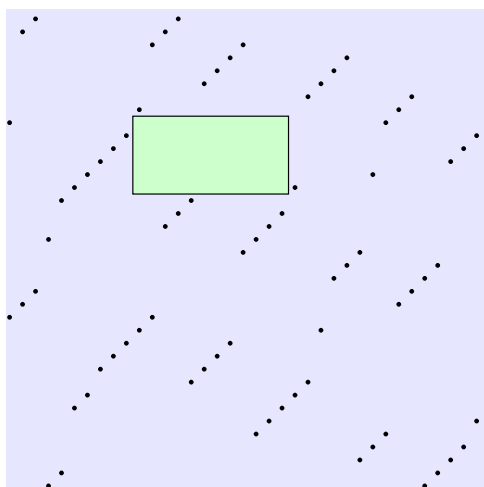

183. (9, 23, 27, 28)

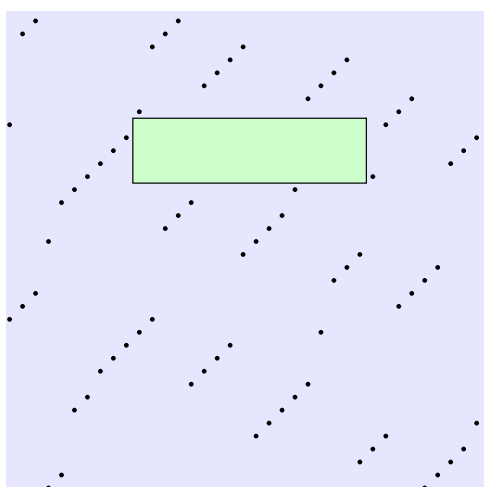

184. (9, 24, 28, 28)

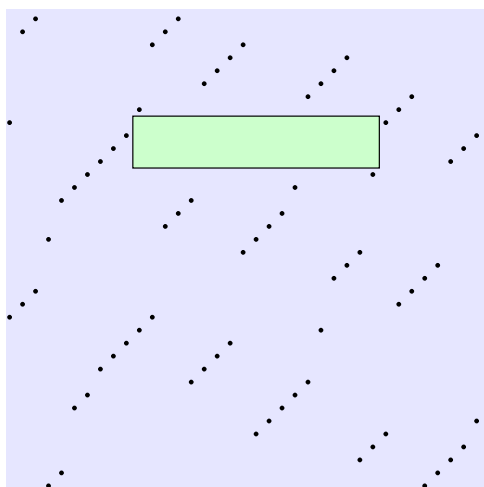

185. (9, 24, 33, 27)

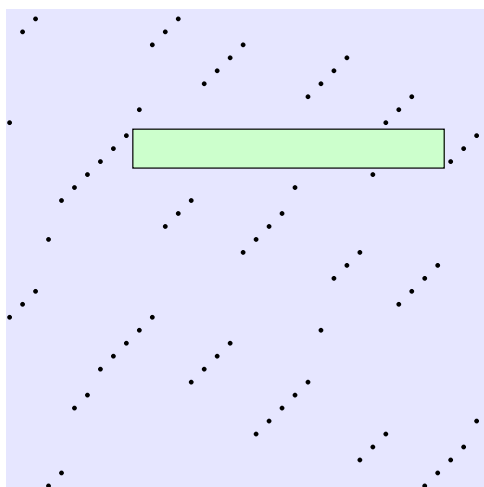

186. (9, 25, 34, 27)

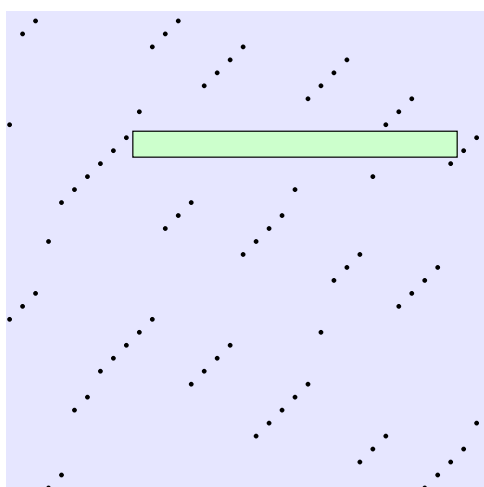

187. (9, 26, 35, 27)

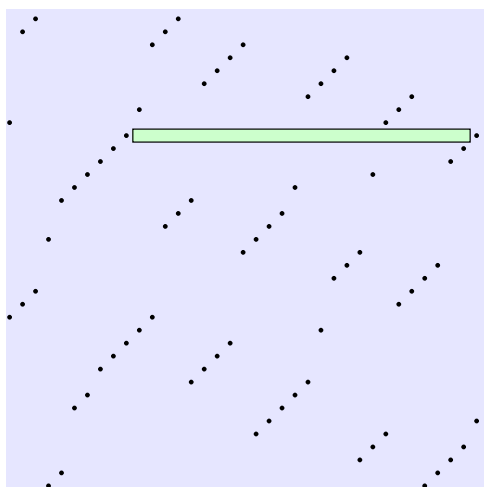

188. (9, 29, 10, 11)

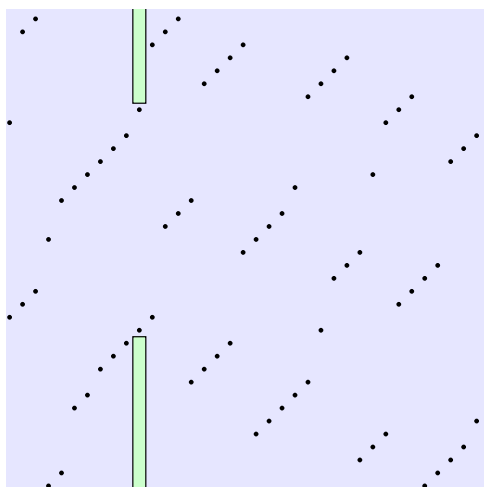

189. (9, 34, 11, 11)

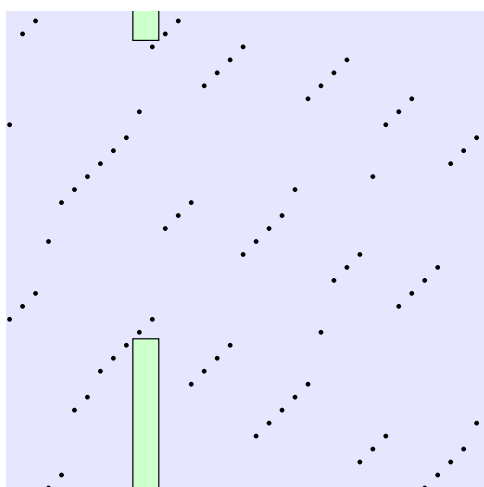

190. (9, 35, 12, 11)

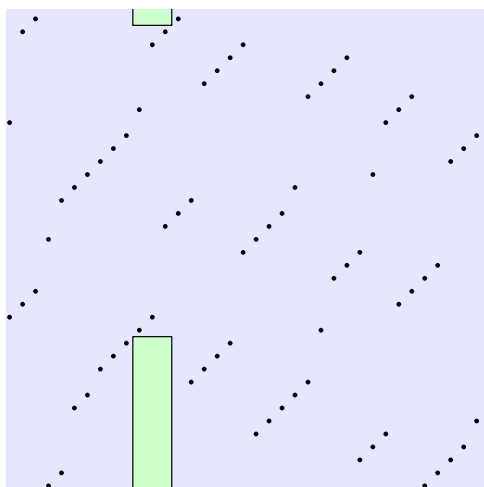

191. (9, 36, 13, 11)

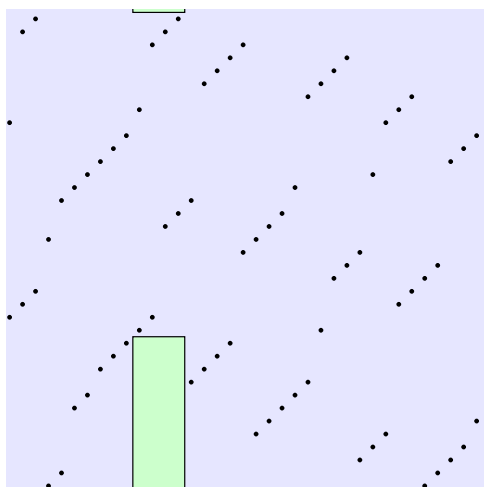

192. (10, 8, 14, 12)

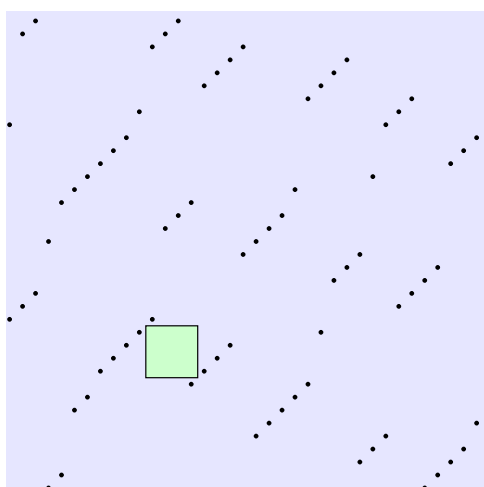



193. (10, 9, 15, 12)

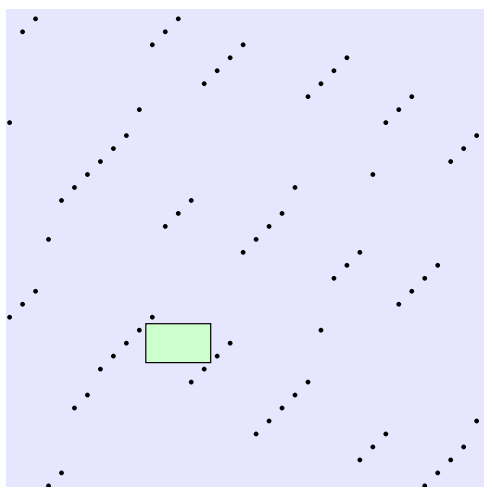

194. (10, 10, 16, 12)

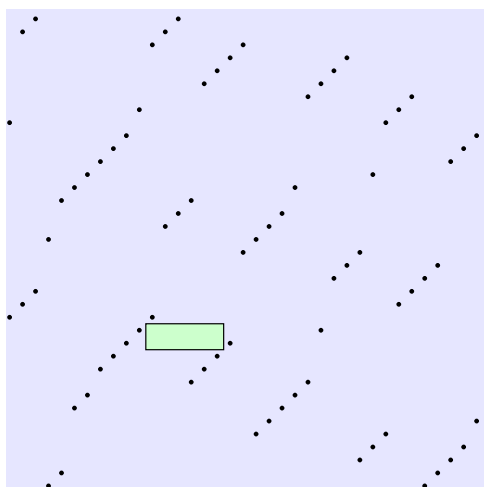

195. (10, 11, 23, 12)

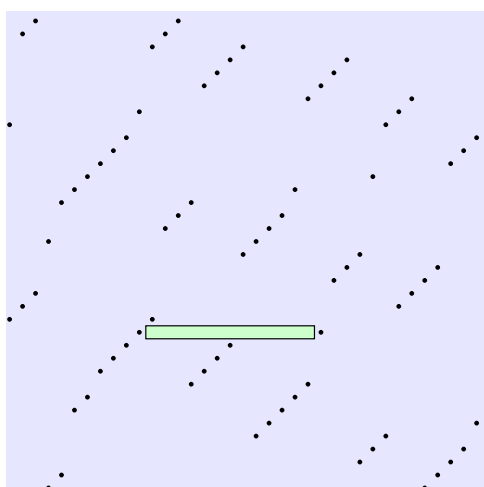

196. (10, 13, 11, 33)

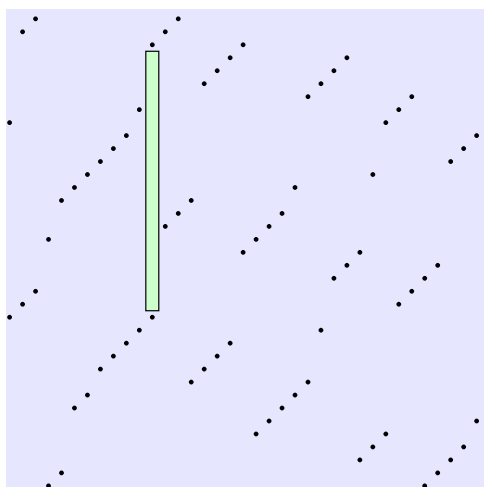

197. (10, 20, 12, 33)

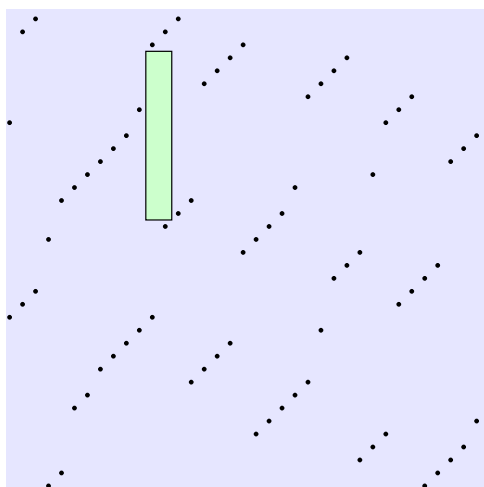

198. (10, 21, 13, 33)

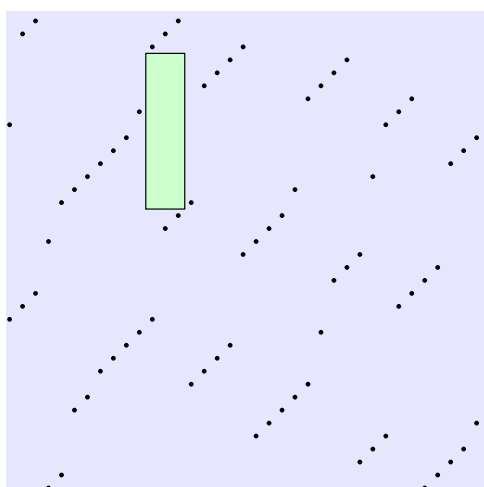

199. (10, 22, 14, 33)

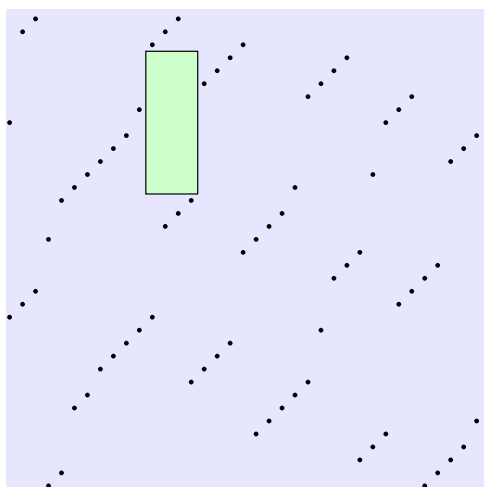

200. (10, 22, 21, 30)

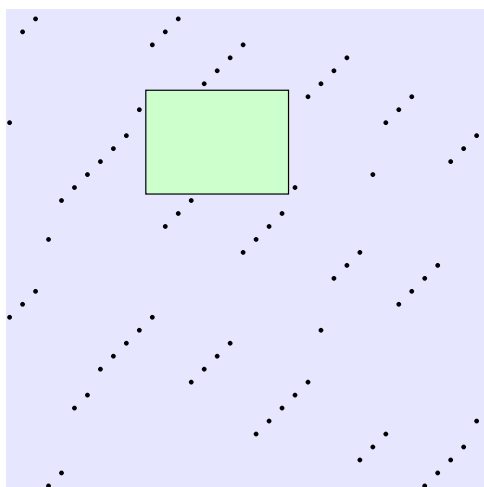

201. (10, 23, 22, 30)

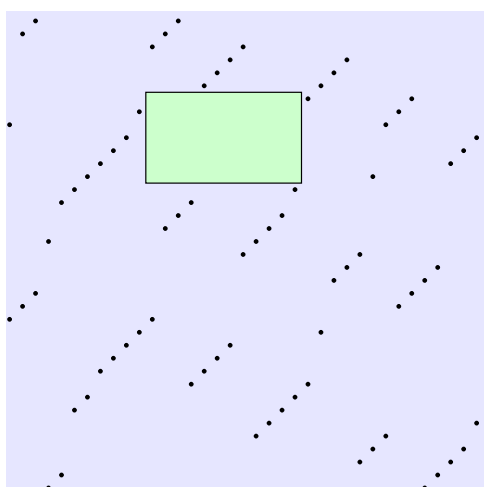

202. (10, 23, 27, 29)

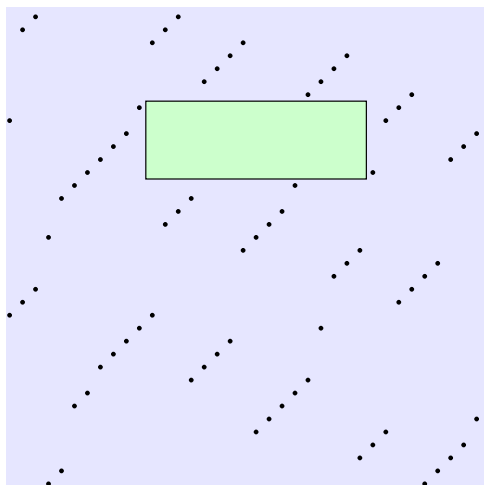

203. (10, 24, 28, 29)

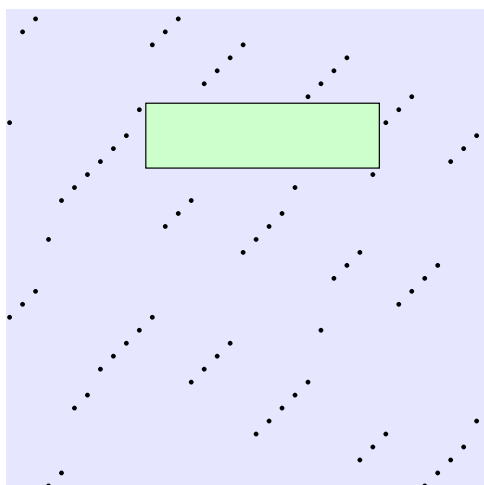

204. (10, 28, 29, 29)

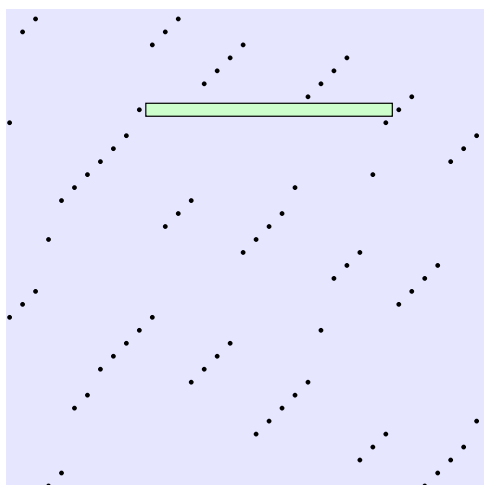

205. (10, 34, 11, 12)

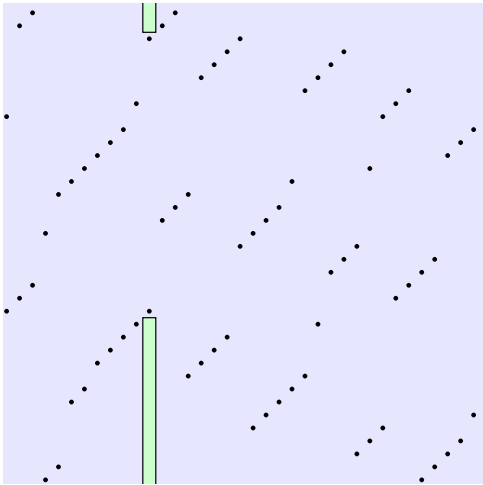

206. (10, 35, 12, 12)

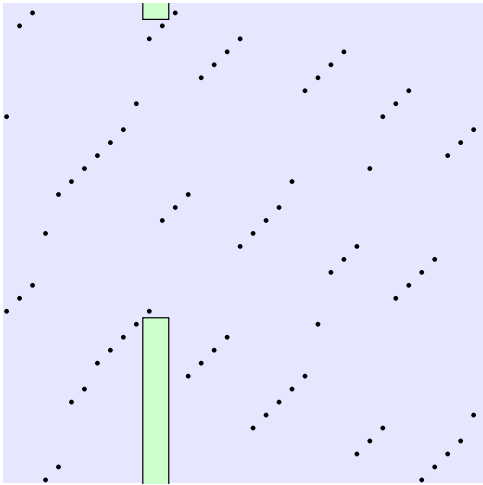

207. (10, 36, 13, 12)

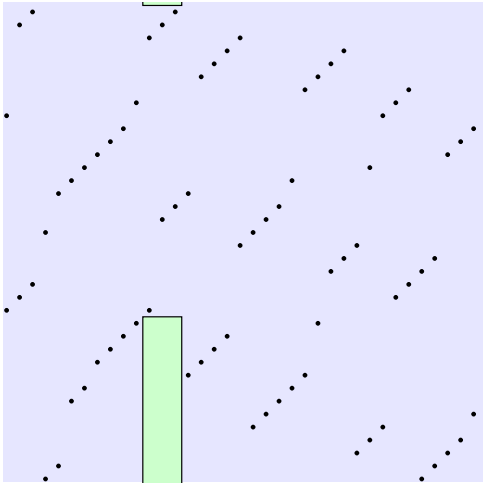

208. (11, 8, 14, 19)

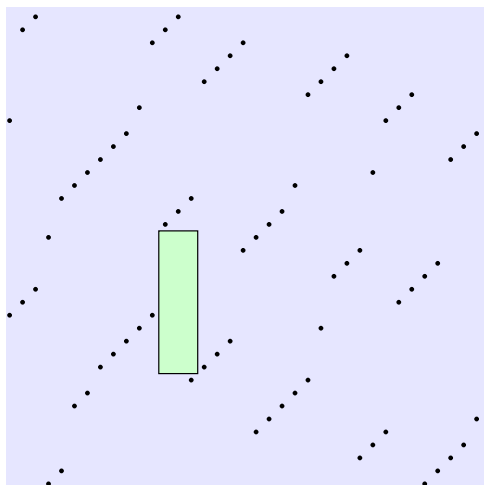

209. (11, 9, 15, 19)

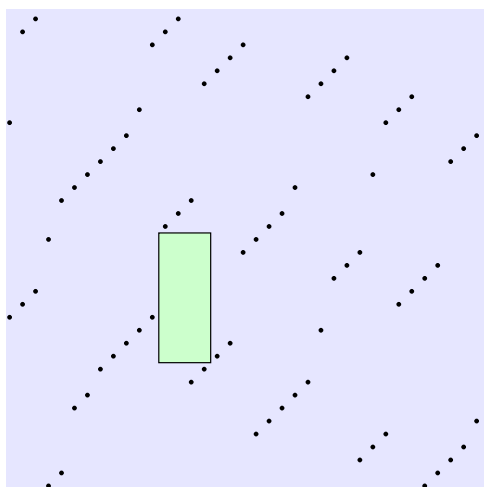

210. (11, 10, 16, 19)

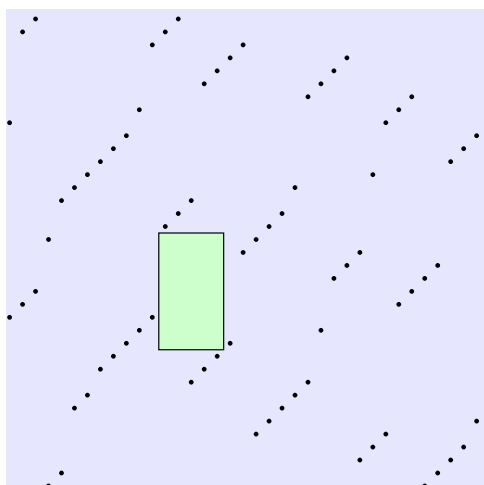

211. (11, 11, 17, 19)

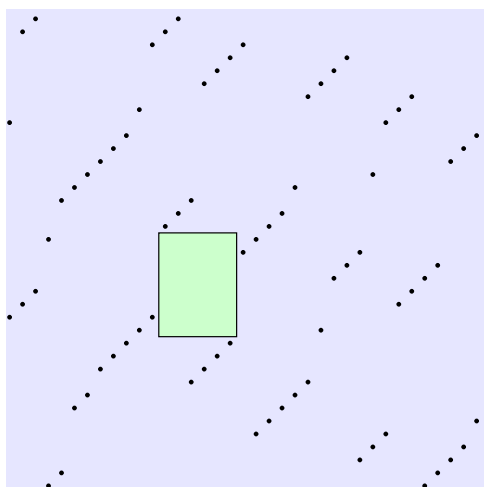

212. (11, 11, 23, 17)

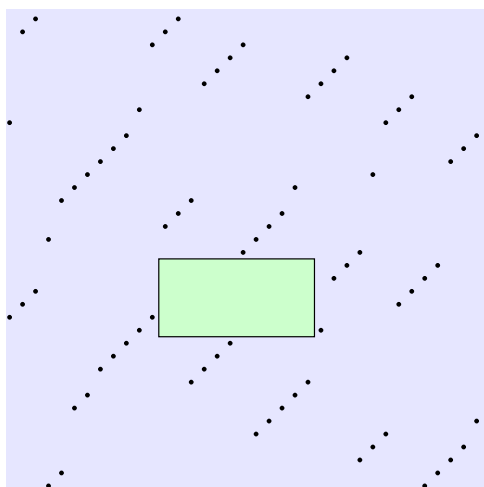

213. (11, 12, 24, 17)

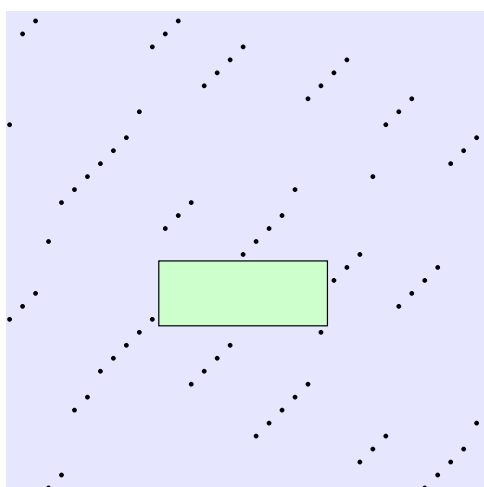

214. (11, 12, 29, 15)

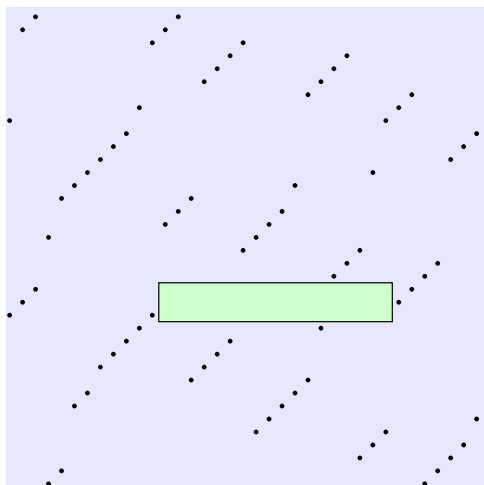

215. (11, 12, 36, 13)

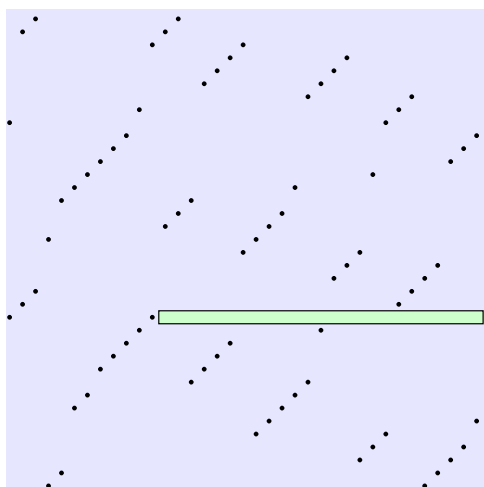

216. (11, 20, 12, 34)

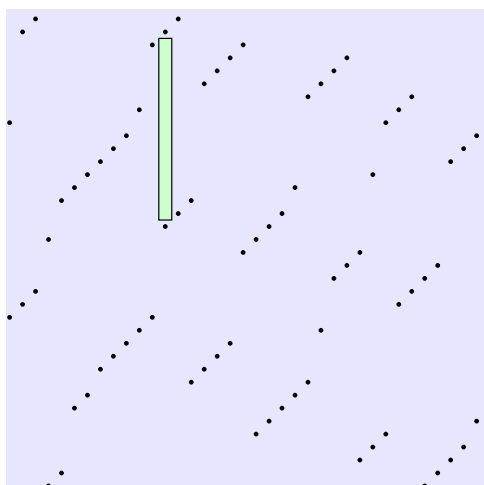



217. (11, 21, 13, 34)

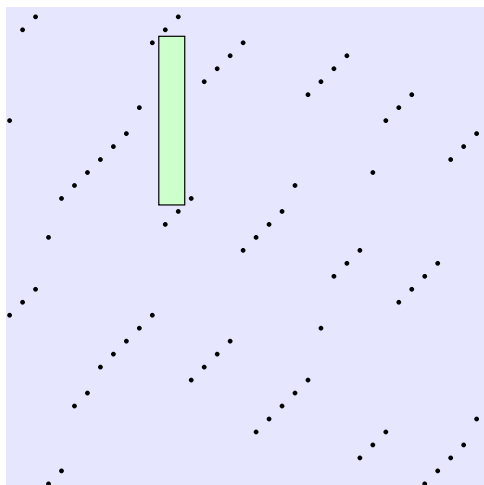

218. (11, 22, 14, 34)

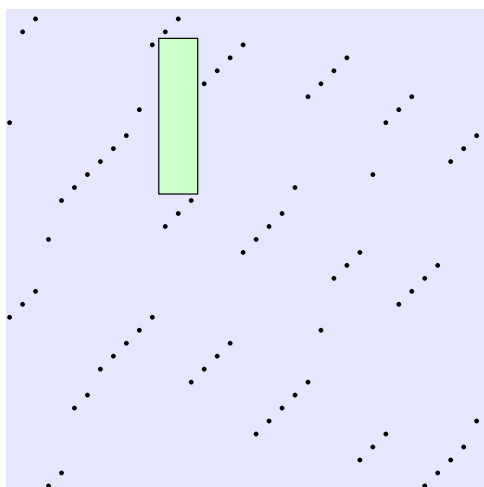

219. (11, 31, 15, 34)

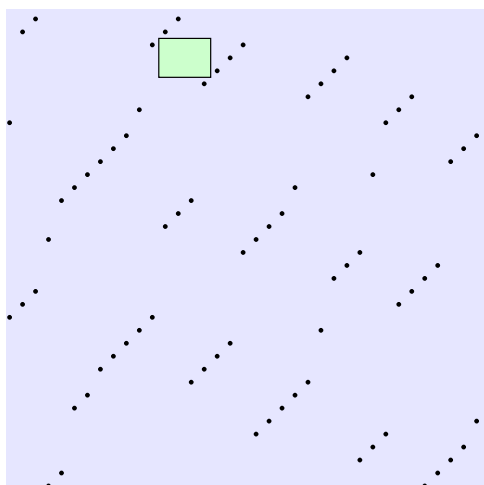

220. (11, 32, 16, 34)

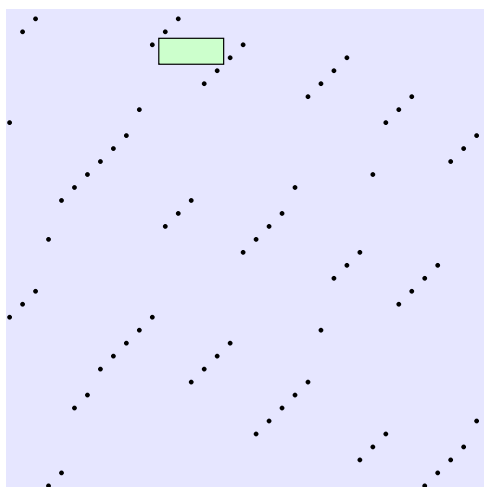

221. (11, 33, 17, 34)

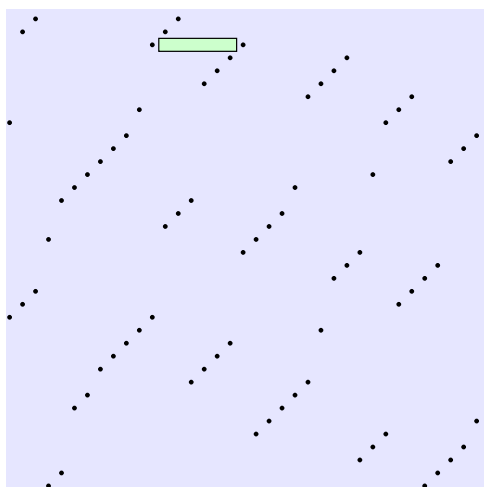

222. (11, 35, 12, 19)

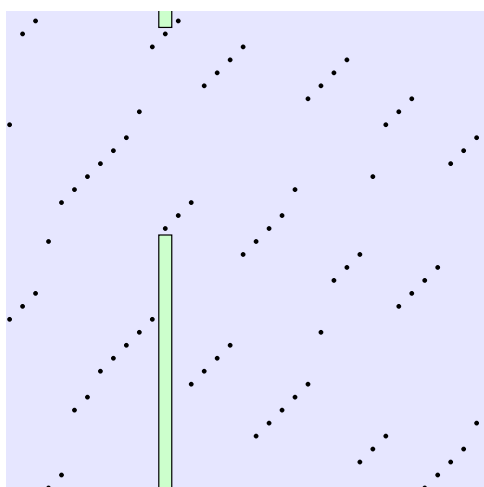

223. (11, 36, 13, 19)

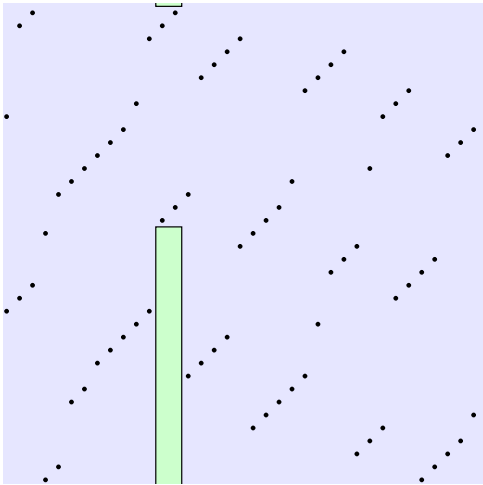

224. (12, 8, 14, 20)

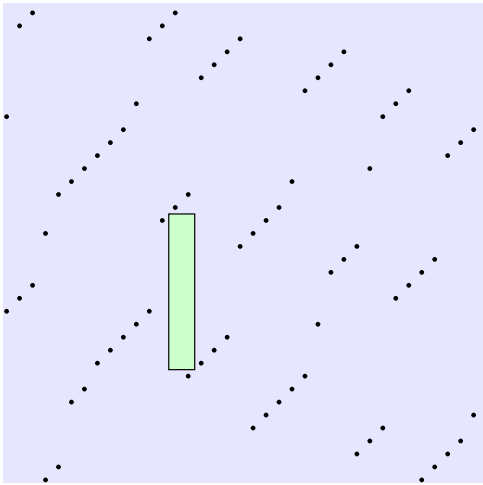

225. (12, 9, 15, 20)

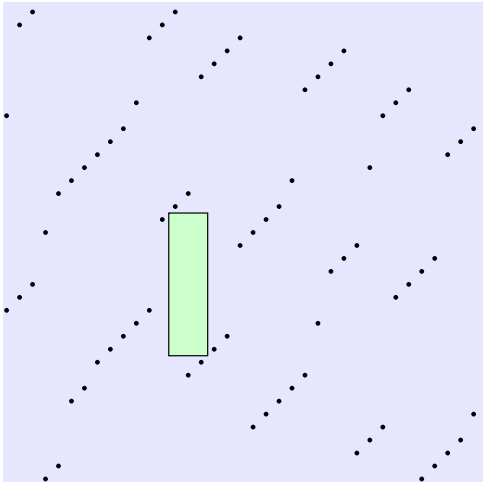

226. (12, 10, 16, 20)

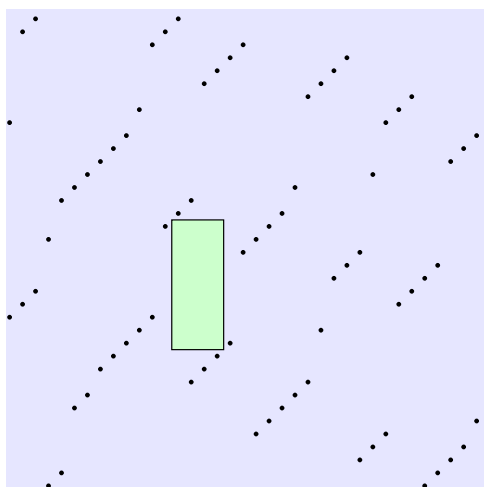

227. (12, 11, 17, 20)

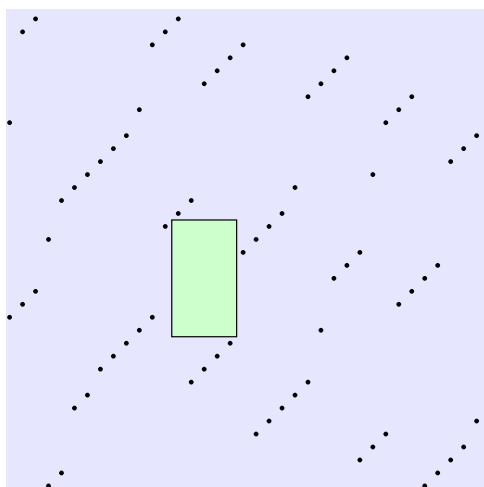

228. (12, 18, 18, 20)

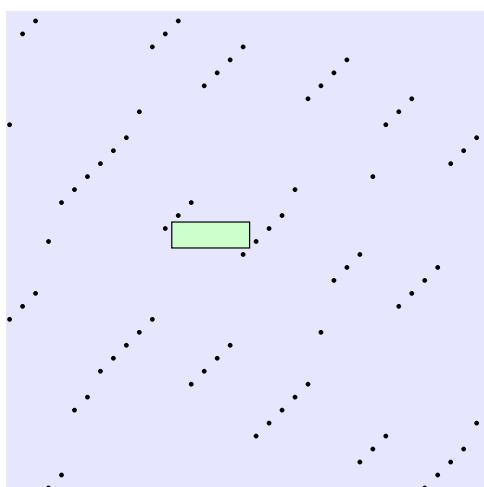

229. (12, 19, 19, 20)

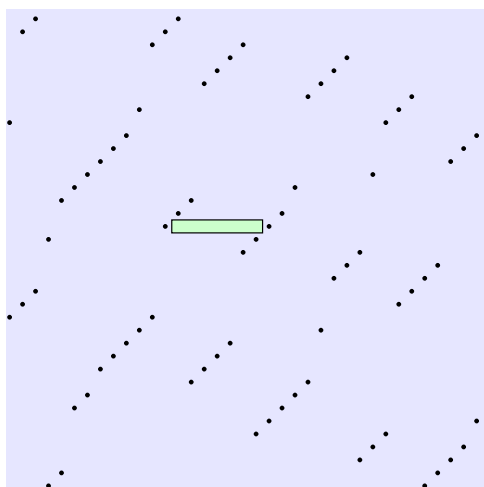

230. (12, 21, 13, 35)

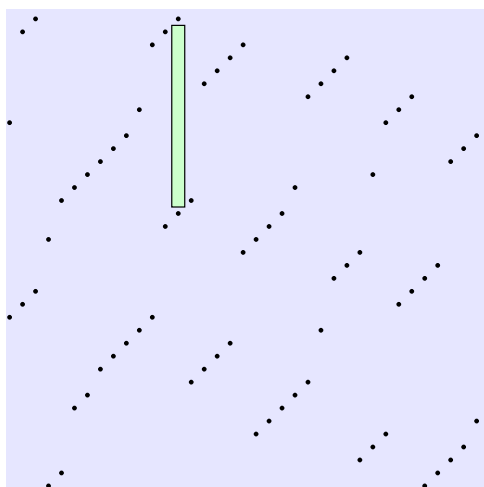

231. (12, 22, 14, 35)

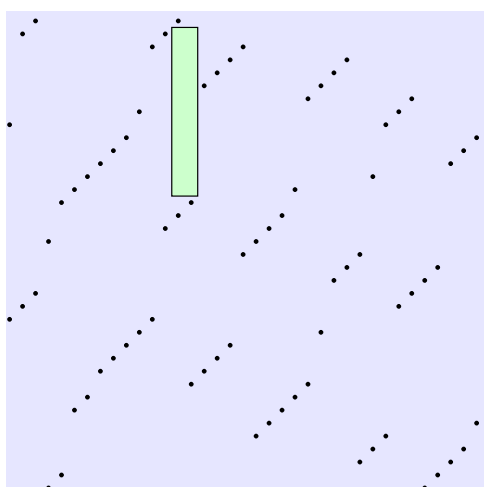

232. (12, 31, 15, 35)

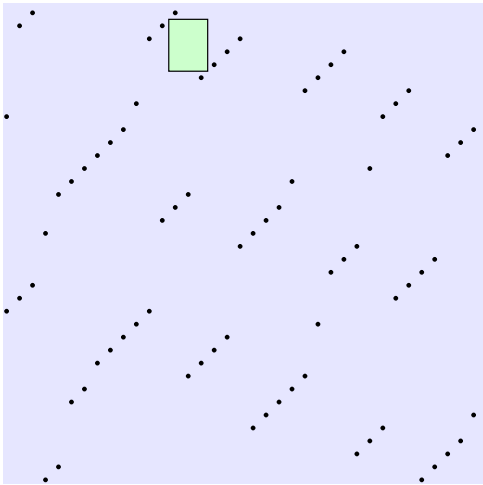

233. (12, 32, 16, 35)

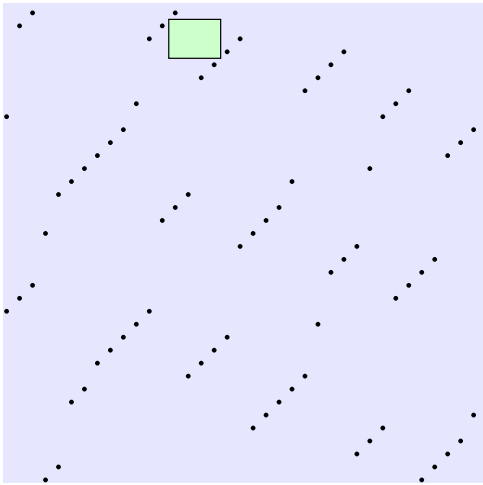

234. (12, 33, 17, 35)

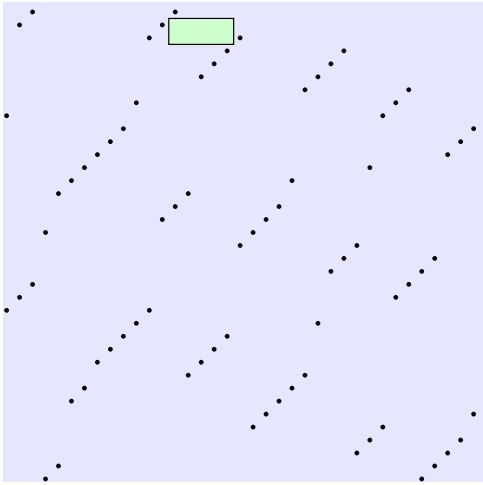

235. (12, 34, 0, 35)

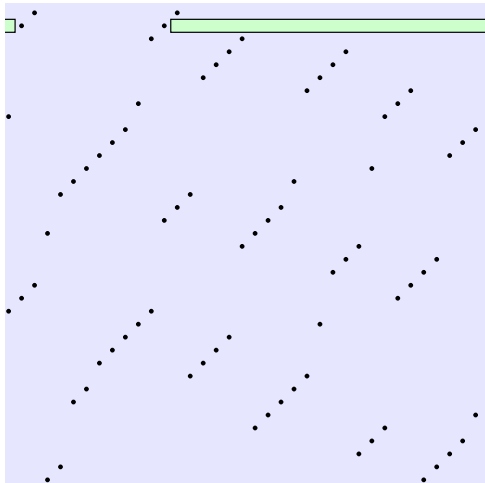

236. (12, 36, 13, 20)

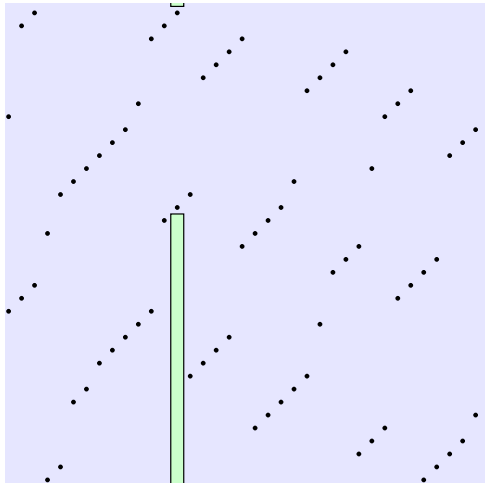

237. (13, 8, 14, 21)

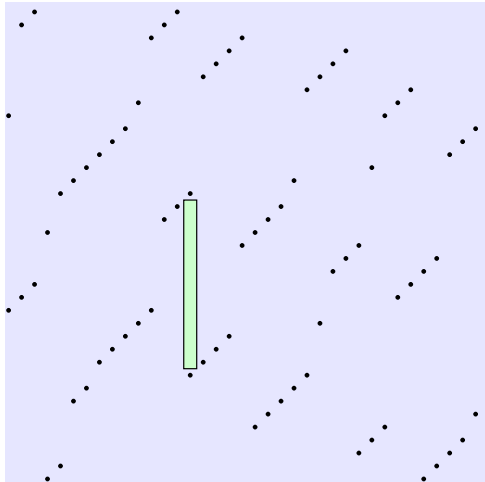

238. (13, 9, 15, 21)

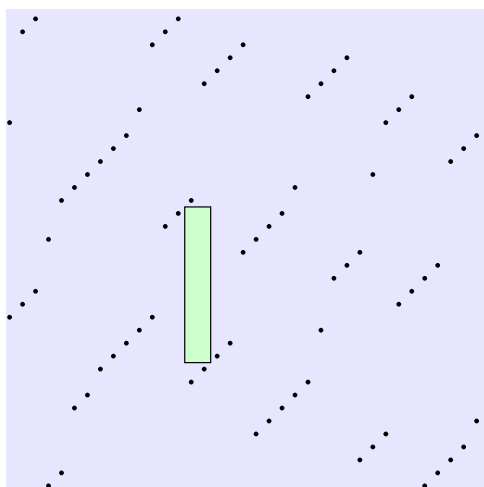

239. (13, 10, 16, 21)

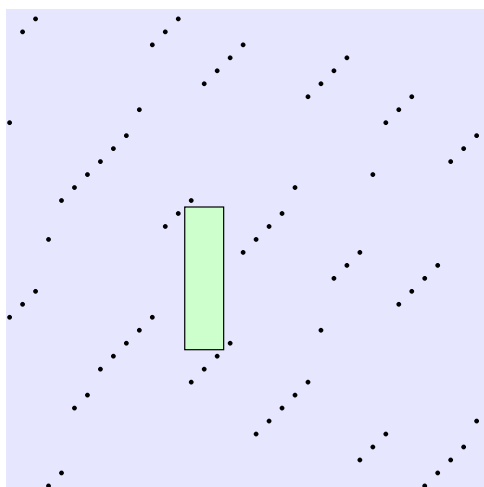

240. (13, 11, 17, 21)

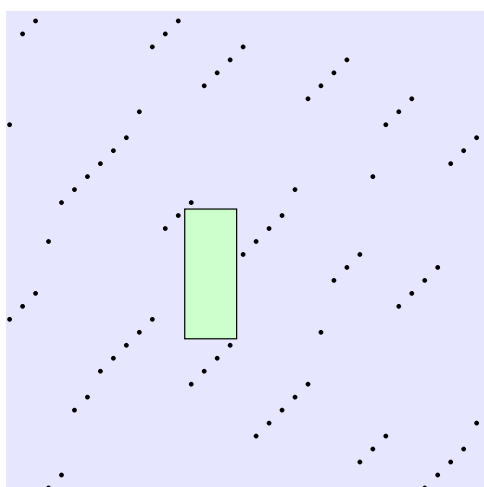



241. (13, 18, 18, 21)

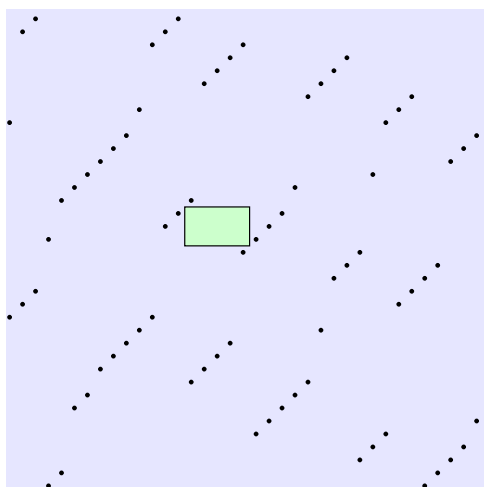

242. (13, 19, 19, 21)

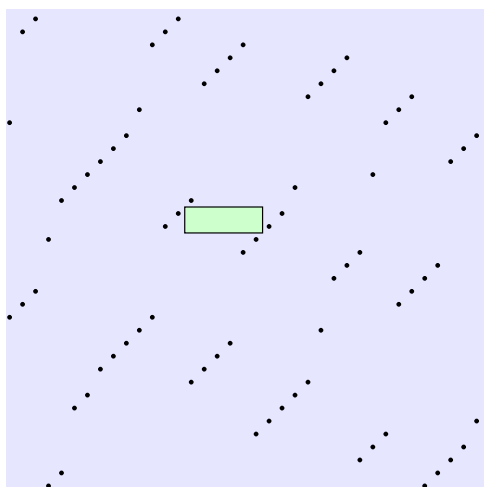

243. (13, 20, 20, 21)

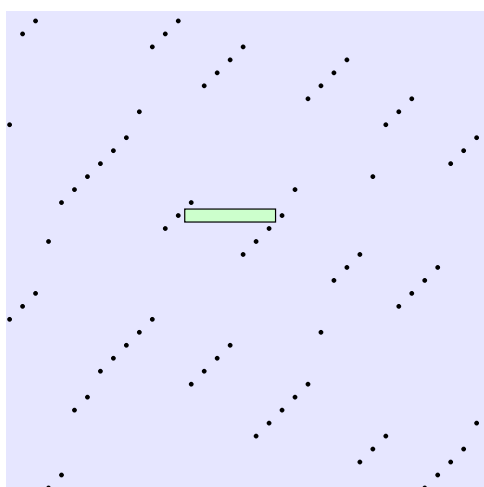

244. (13, 22, 14, 7)

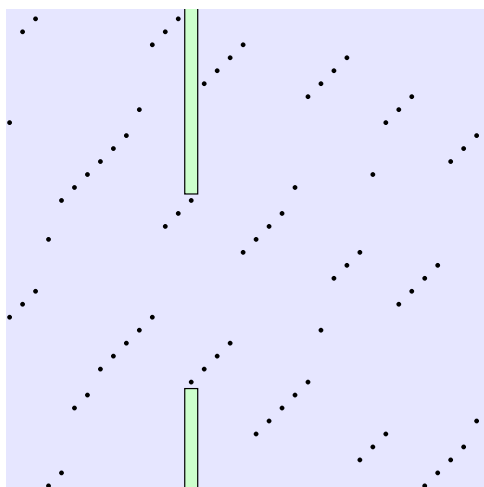

245. (13, 31, 15, 7)

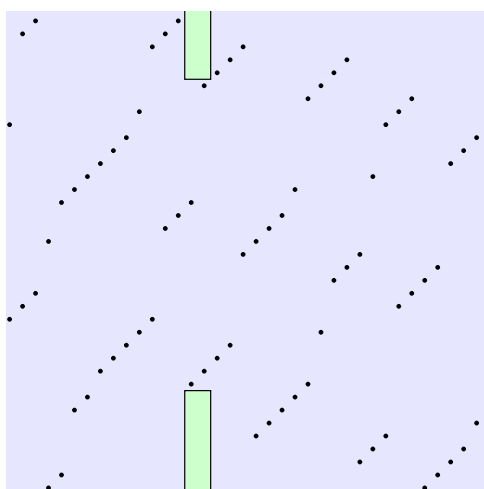

246. (13, 32, 16, 7)

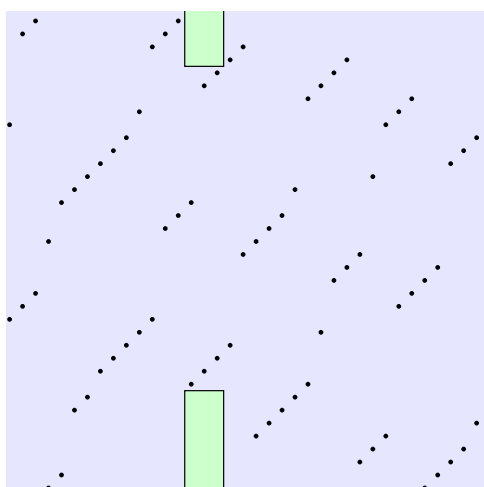

247. (13, 33, 17, 7)

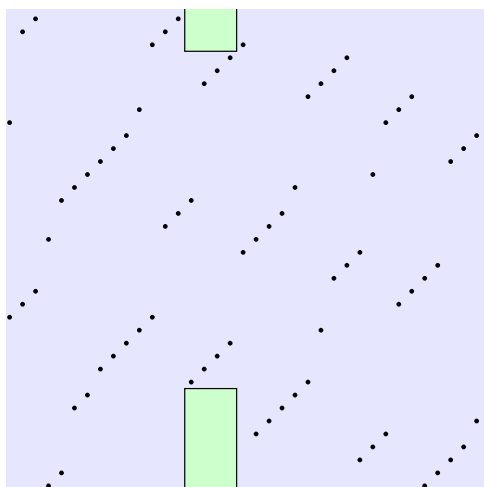

248. (13, 34, 0, 36)

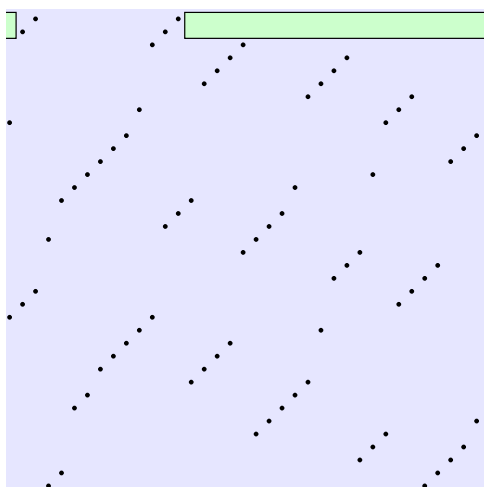

249. (13, 34, 18, 7)

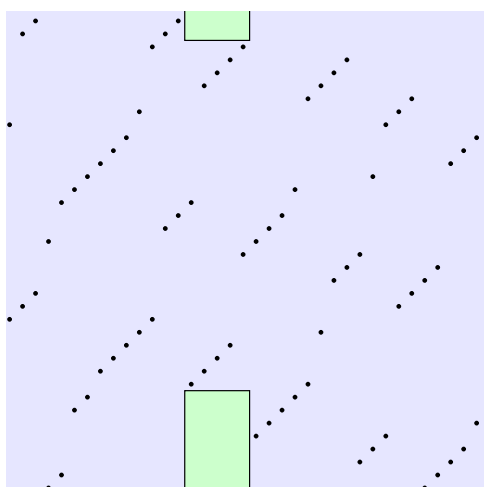

250. (13, 34, 26, 3)

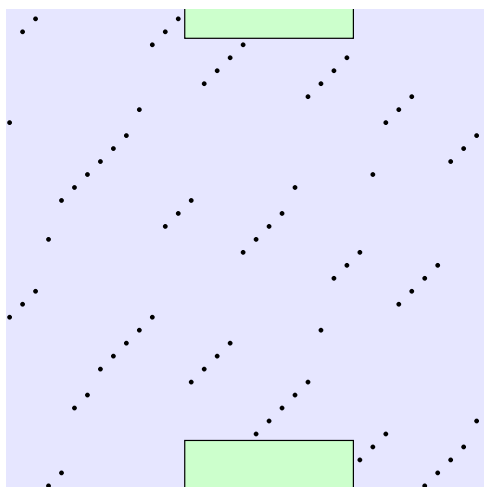

251. (13, 34, 31, 1)

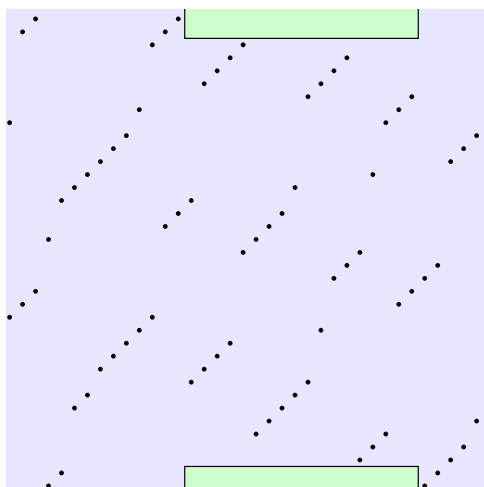

252. (13, 35, 1, 36)

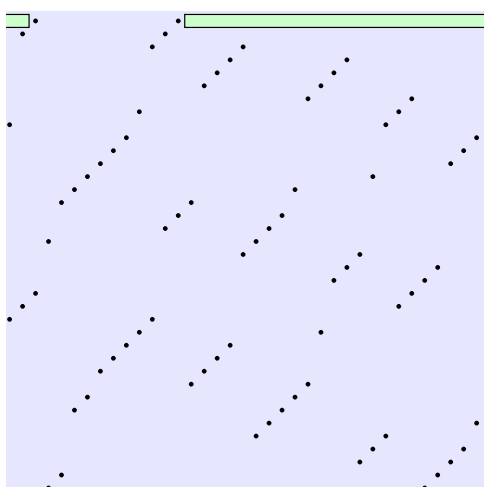

253. (14, 4, 19, 8)

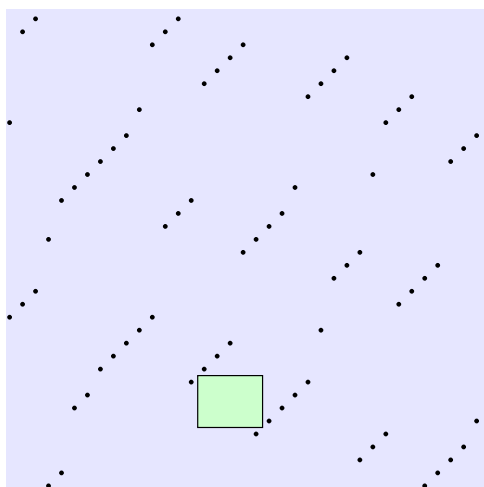

254. (14, 5, 20, 8)

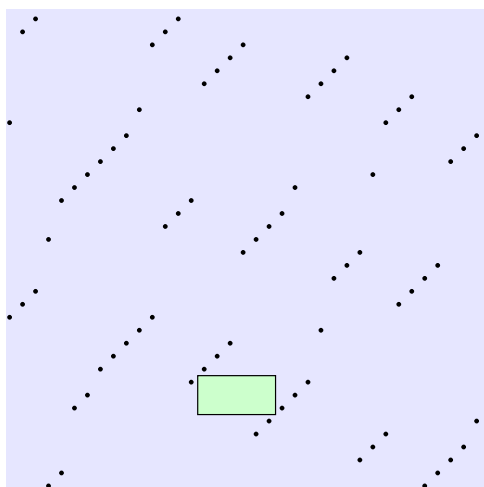

255. (14, 6, 21, 8)

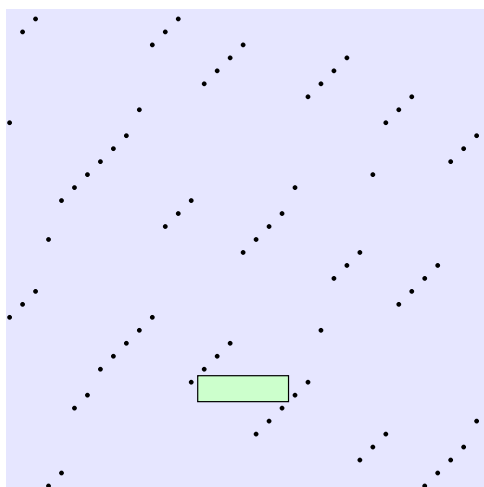

256. (14, 7, 22, 8)

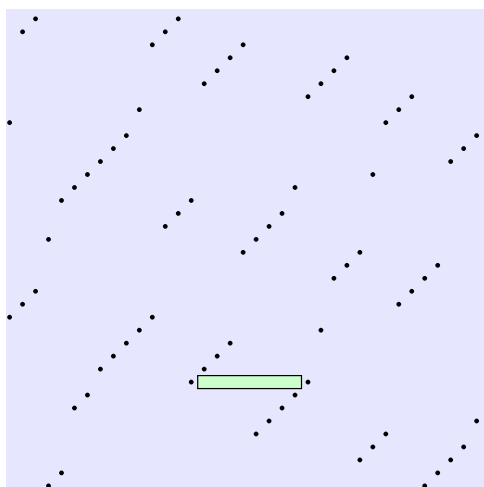

257. (14, 9, 15, 30)

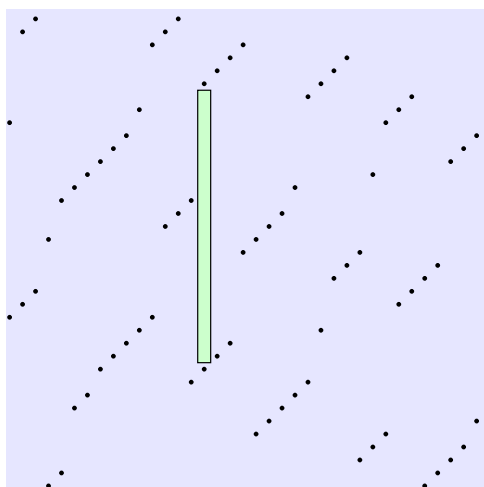

258. (14, 10, 16, 30)

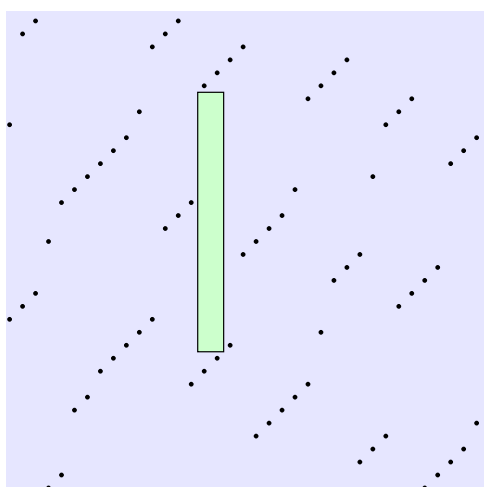

259. (14, 11, 17, 30)

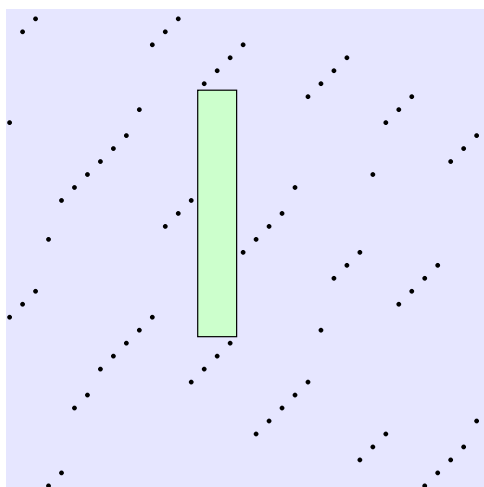

260. (14, 18, 18, 30)

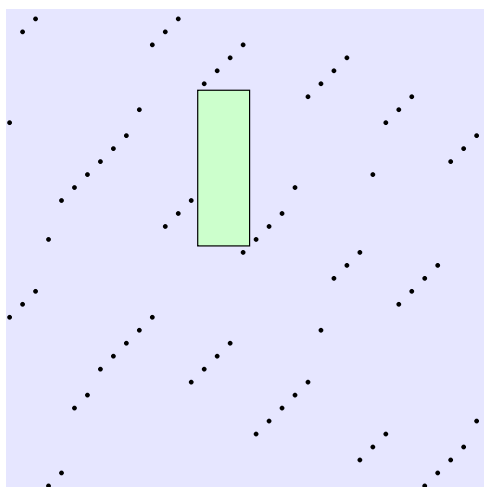

261. (14, 19, 19, 30)

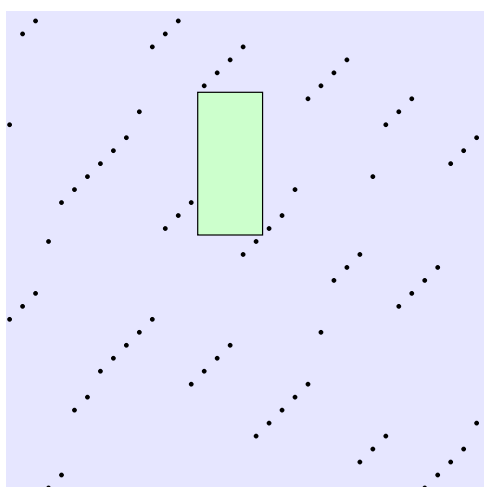

262. (14, 20, 20, 30)

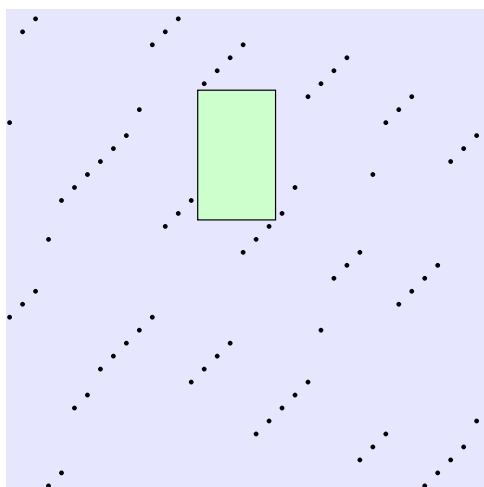

263. (14, 21, 3, 22)

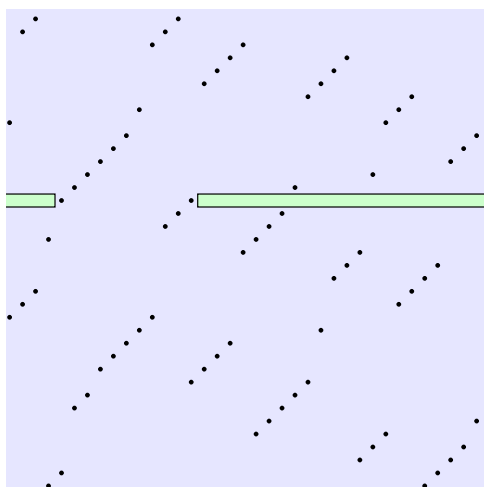

264. (14, 21, 21, 30)

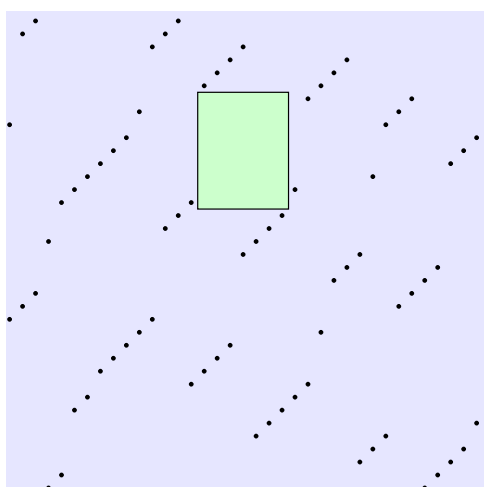



265. (14, 31, 15, 8)

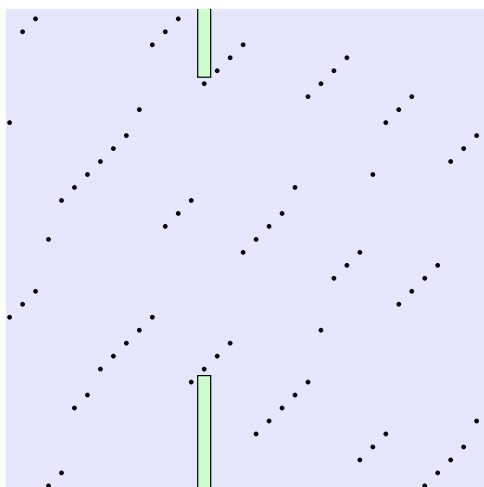

266. (14, 32, 16, 8)

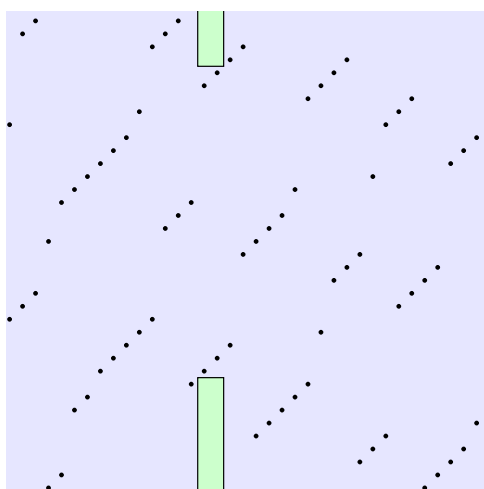

267. (14, 33, 17, 8)

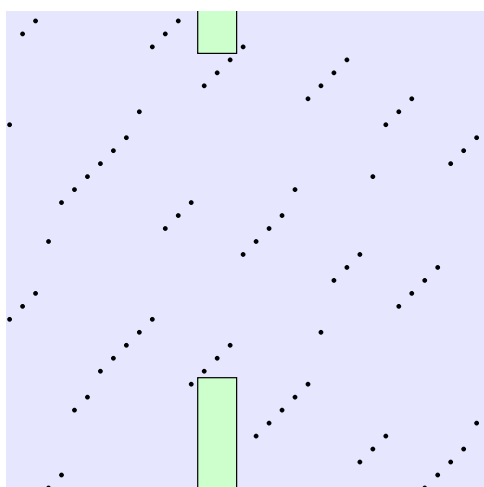

268. (14, 34, 18, 8)

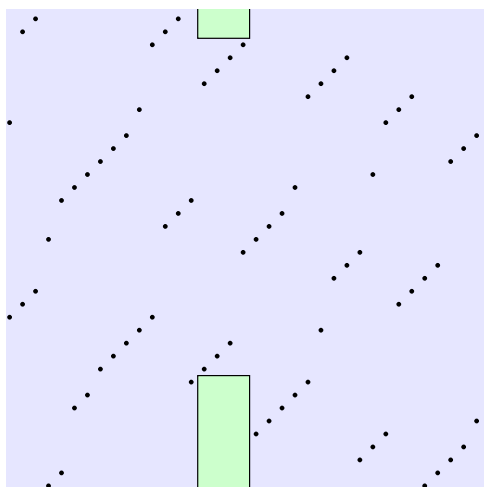

269. (15, 4, 19, 9)

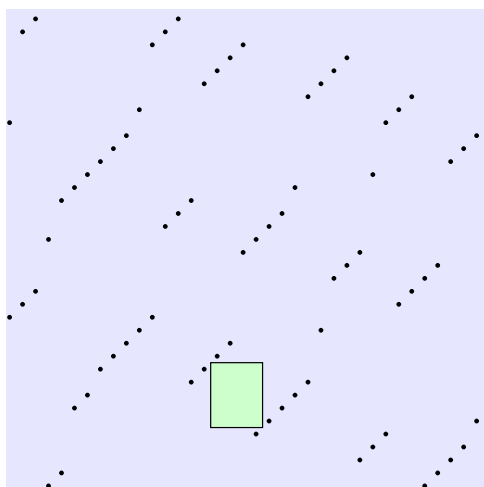

270. (15, 5, 20, 9)

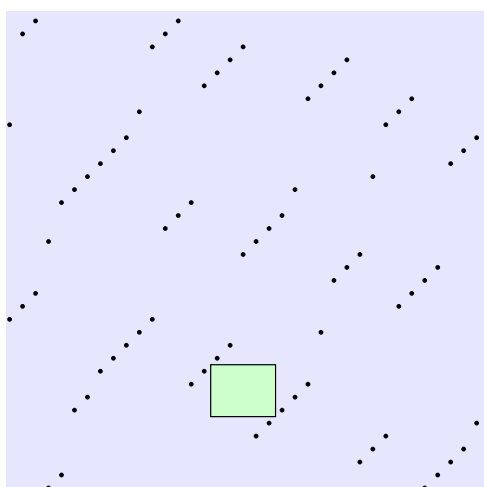

271. (15, 6, 21, 9)

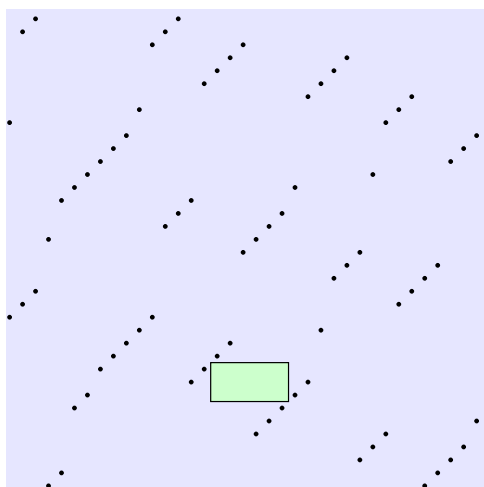

272. (15, 7, 22, 9)

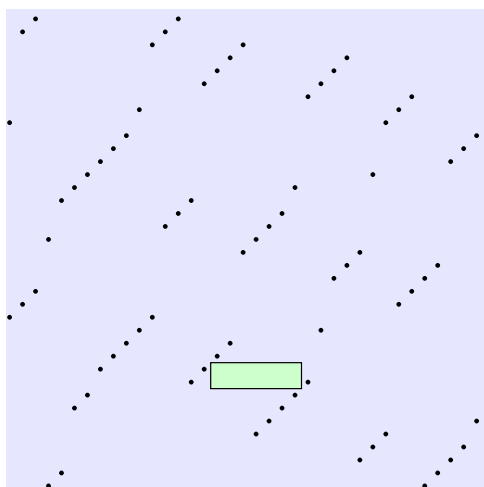

273. (15, 8, 6, 9)

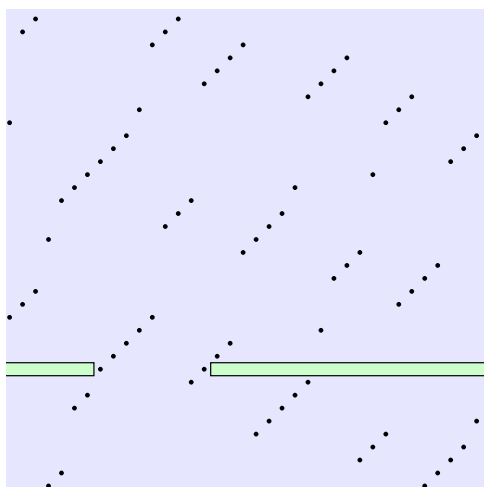

274. (15, 10, 16, 31)

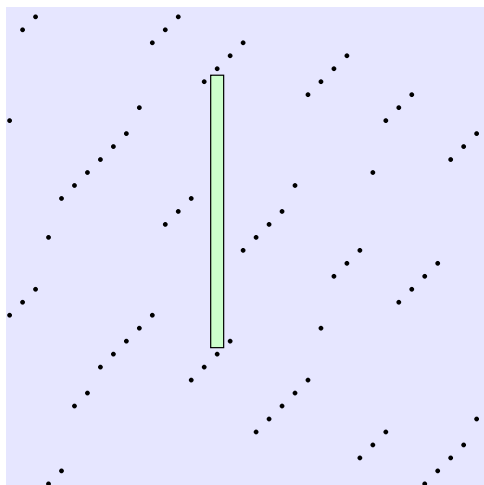

275. (15, 11, 17, 31)

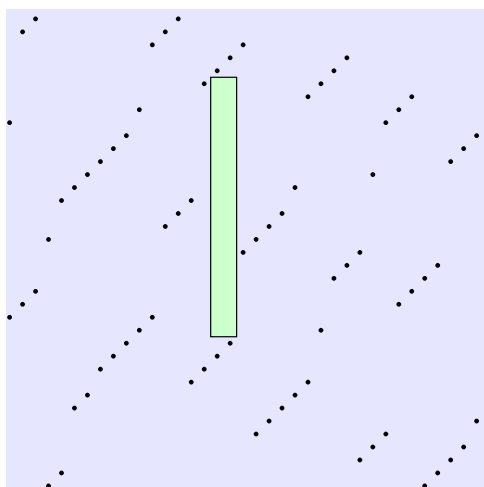

276. (15, 18, 18, 31)

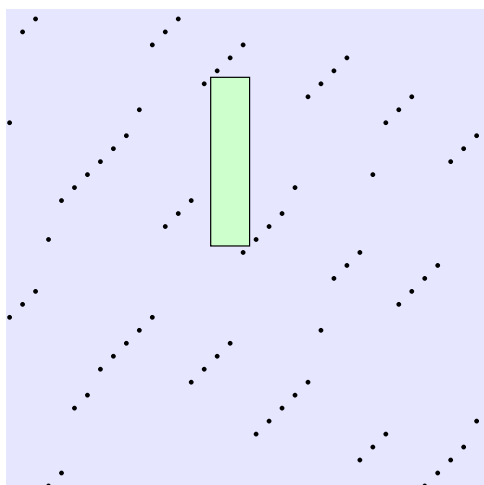

277. (15, 19, 19, 31)

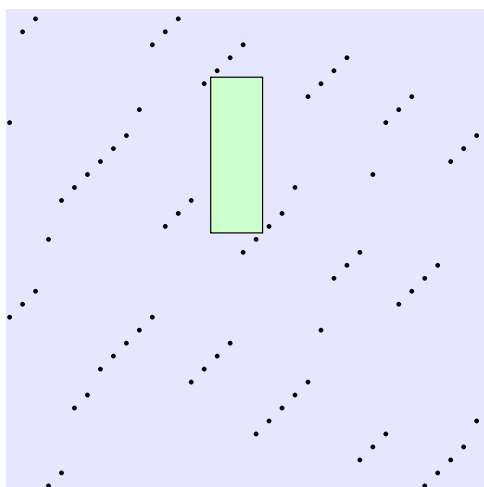

278. (15, 20, 20, 31)

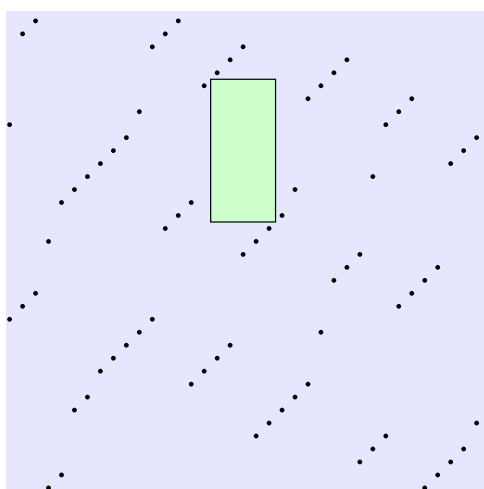

279. (15, 21, 21, 31)

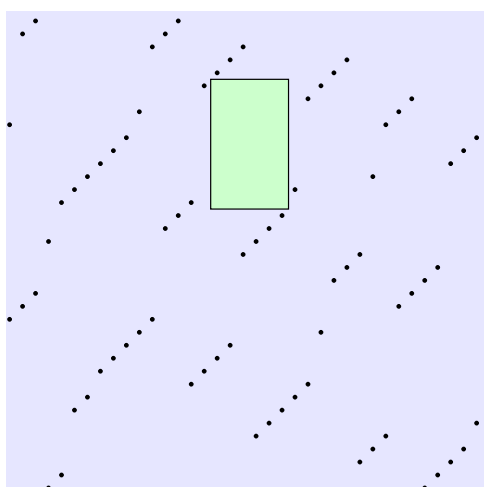

280. (15, 23, 22, 31)

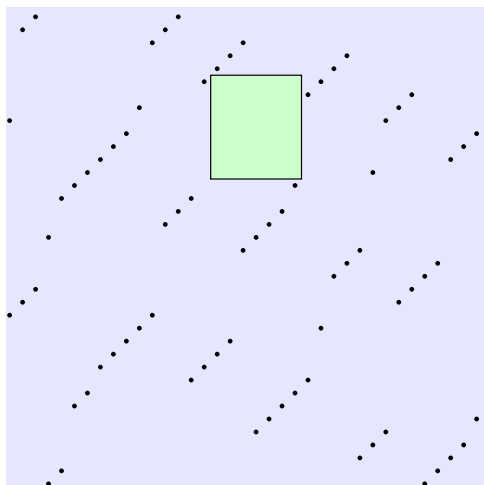

281. (15, 30, 23, 31)

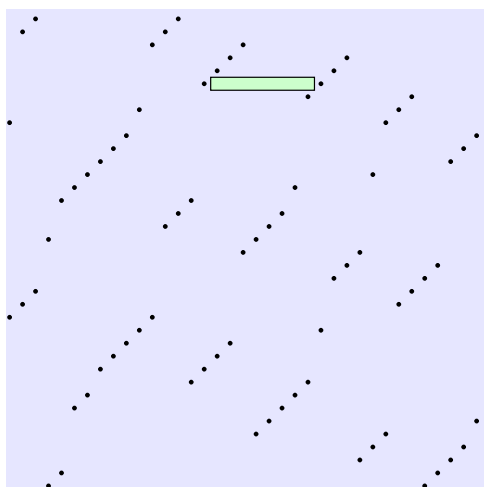

282. (15, 32, 16, 9)

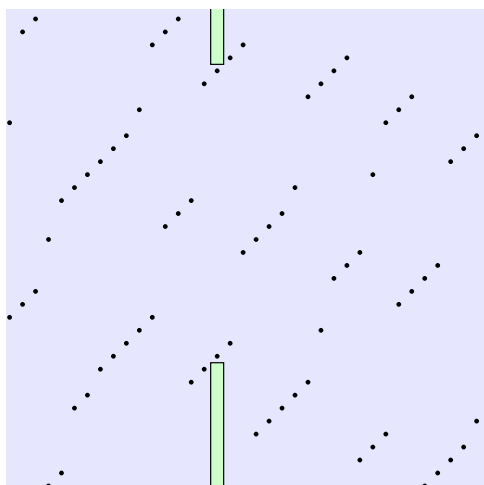

283. (15, 33, 17, 9)

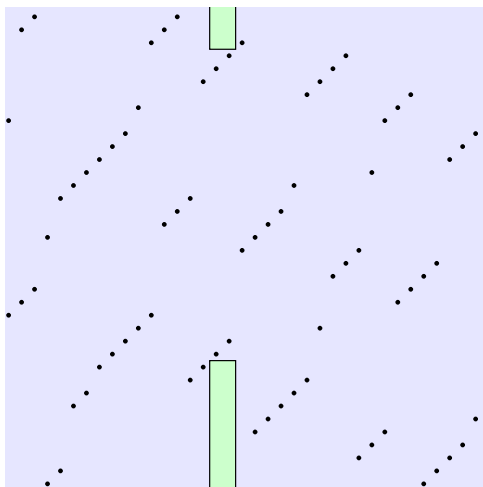

284. (15, 34, 18, 9)

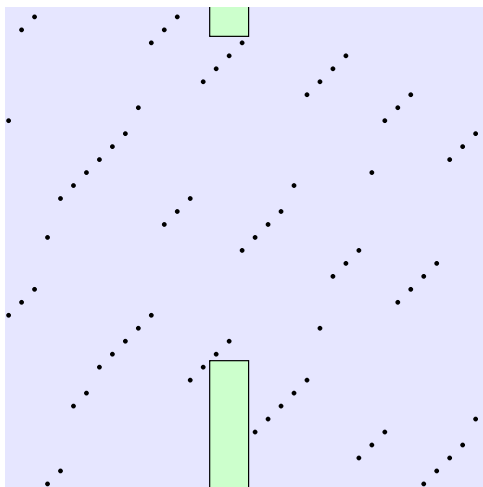

285. (16, 4, 19, 10)

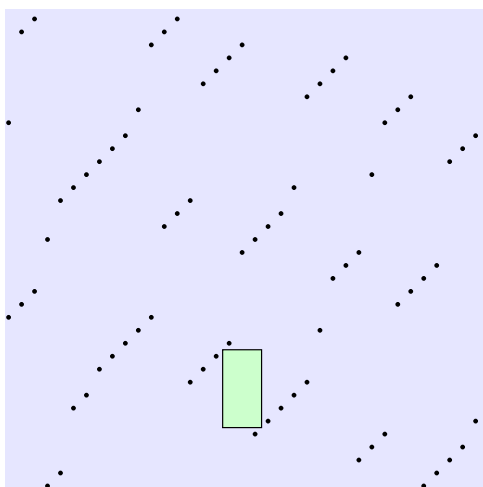

286. (16, 5, 20, 10)

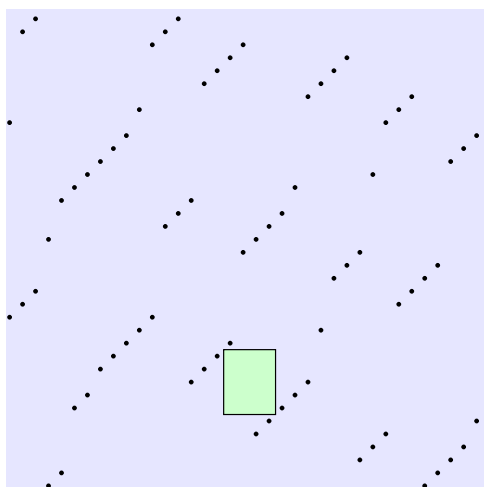

287. (16, 6, 21, 10)

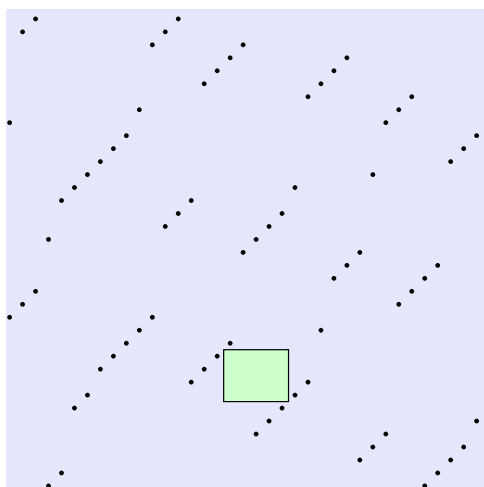

288. (16, 7, 22, 10)

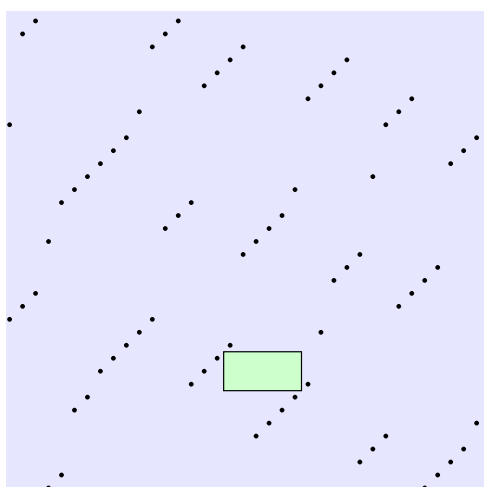



289. (16, 8, 6, 10)

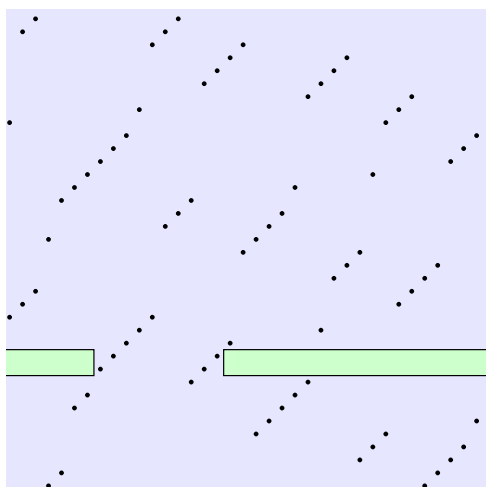

290. (16, 9, 7, 10)

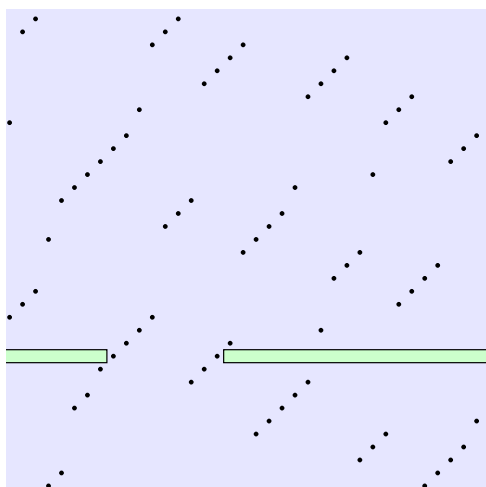

291. (16, 11, 17, 32)

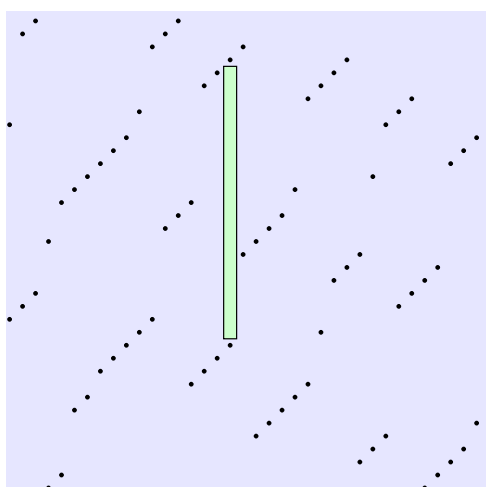

292. (16, 18, 18, 32)

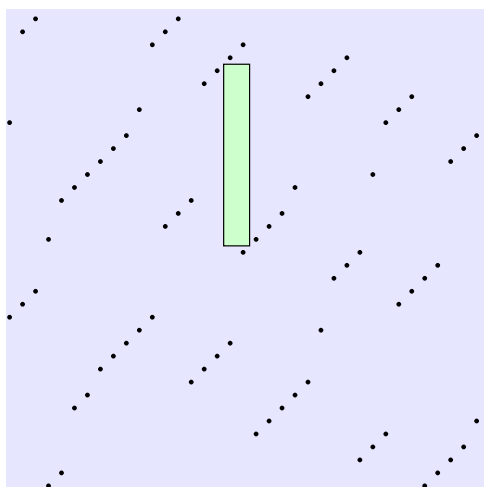

293. (16, 19, 19, 32)

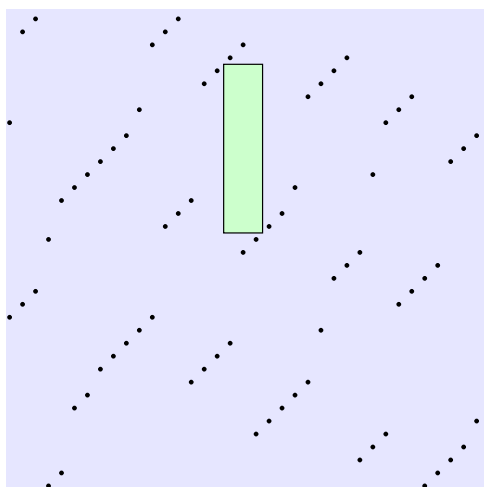

294. (16, 20, 20, 32)

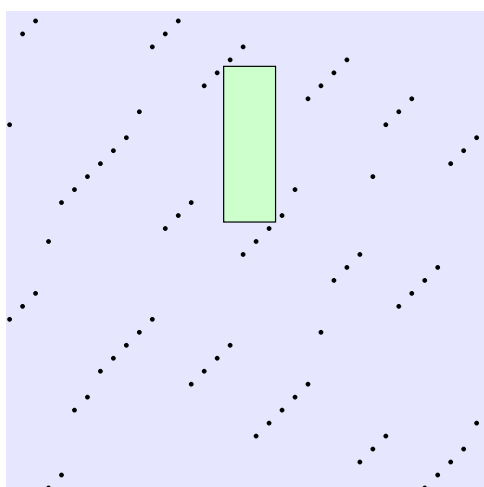

295. (16, 21, 21, 32)

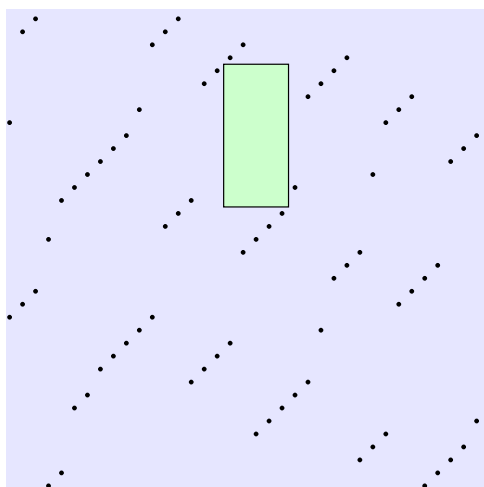

296. (16, 23, 22, 32)

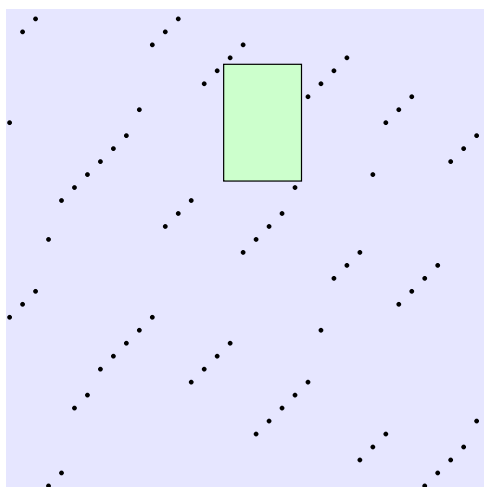

297. (16, 30, 23, 32)

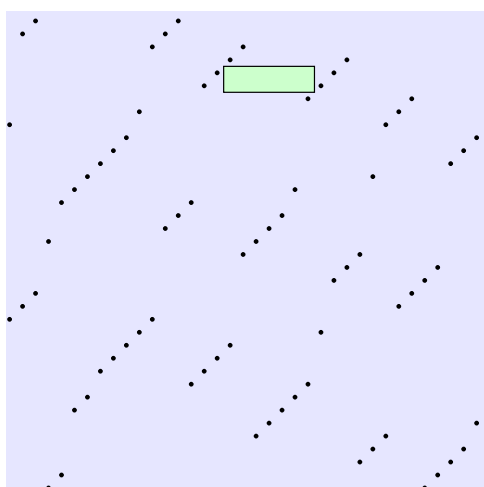

298. (16, 31, 24, 32)

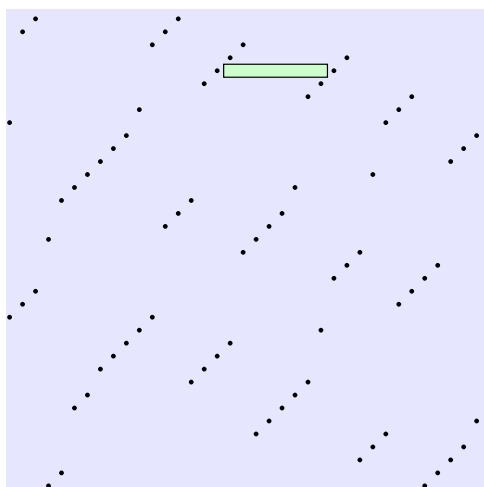

299. (16, 33, 17, 10)

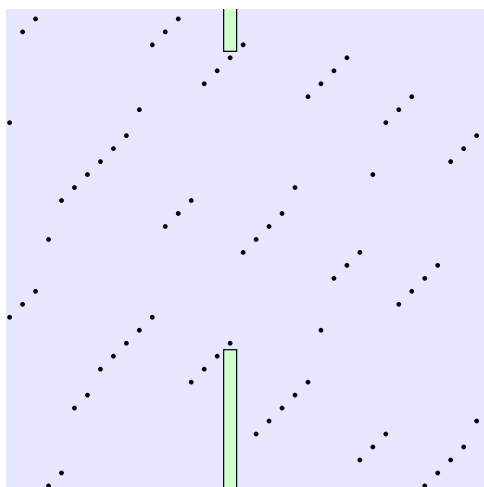

300. (16, 34, 18, 10)

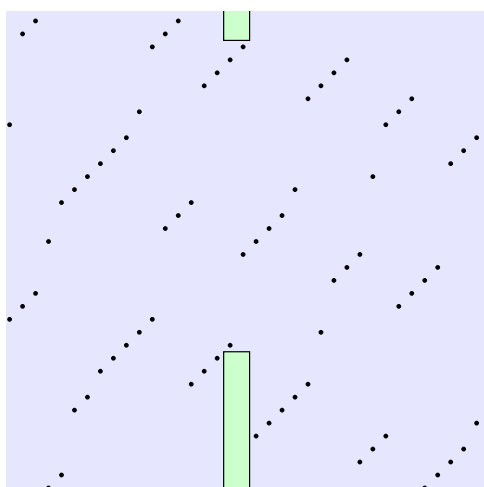

301. (17, 4, 19, 17)

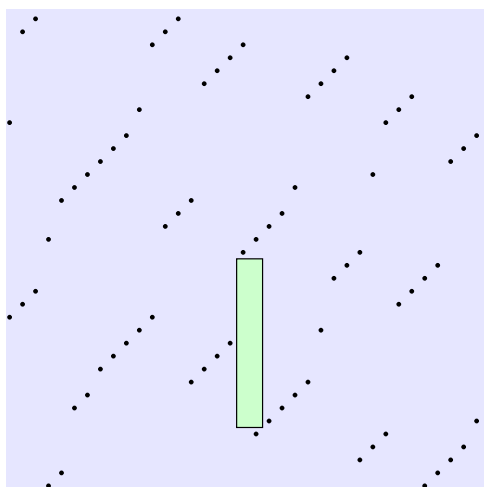

302. (17, 5, 20, 17)

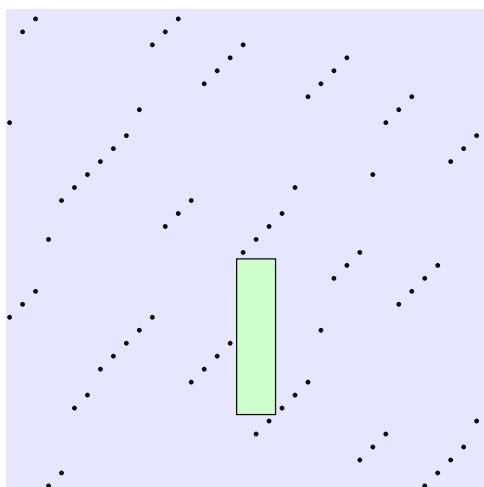

303. (17, 6, 21, 17)

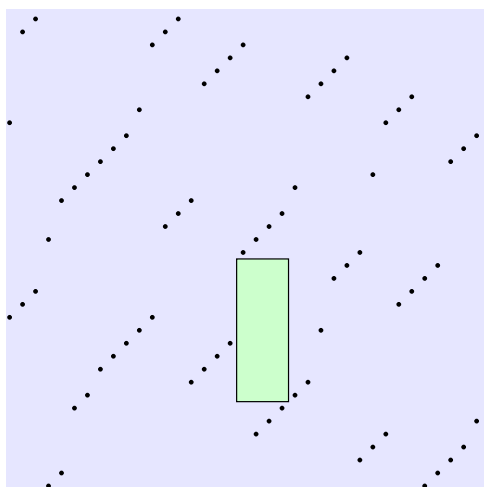

304. (17, 7, 22, 17)

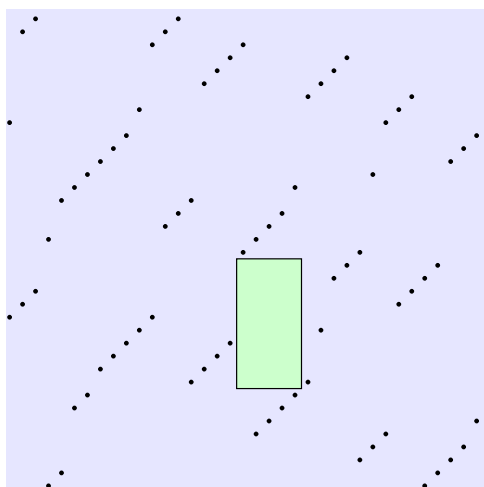

305. (17, 8, 6, 11)

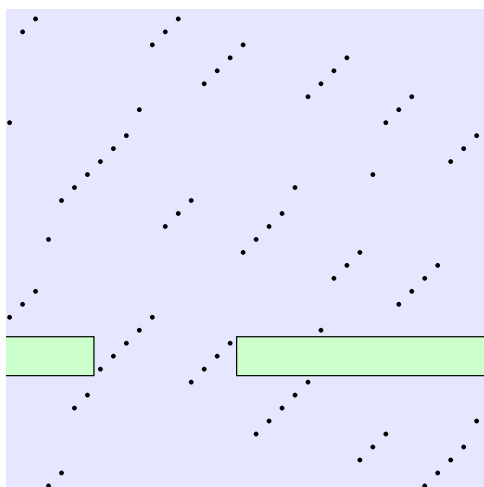

306. (17, 8, 23, 17)

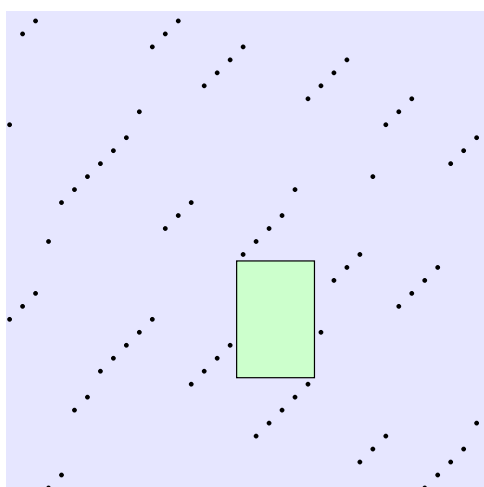

307. (17, 9, 7, 11)

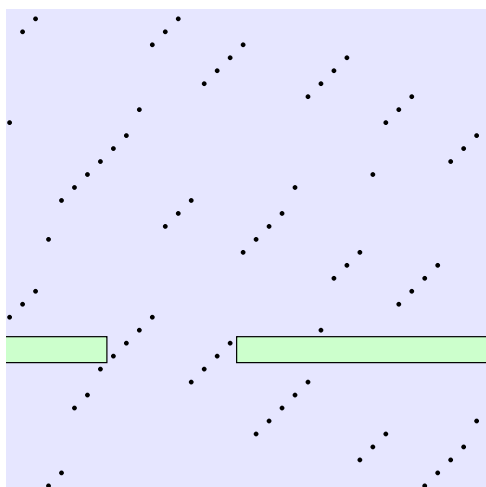

308. (17, 10, 8, 11)

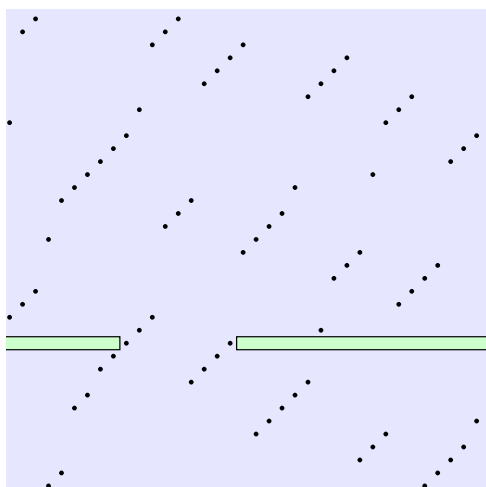

309. (17, 18, 18, 33)

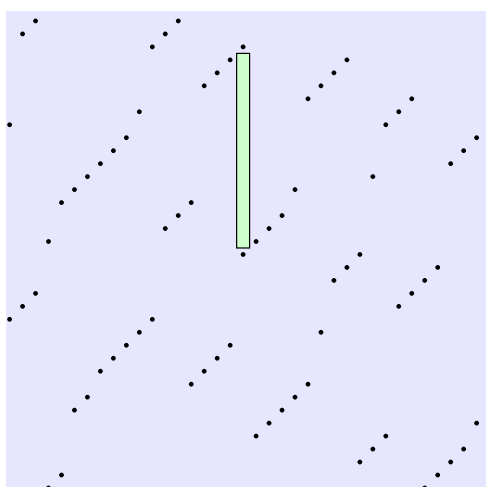

310. (17, 19, 19, 33)

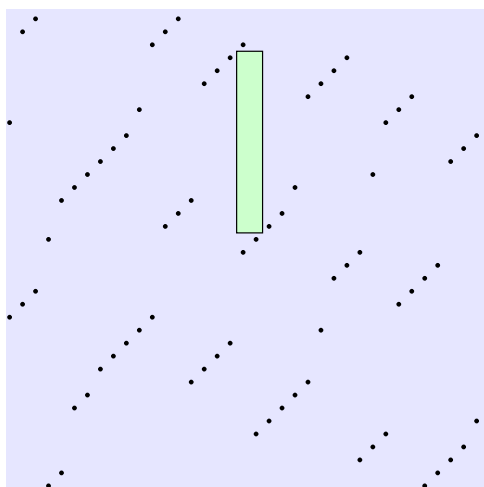

311. (17, 20, 20, 33)

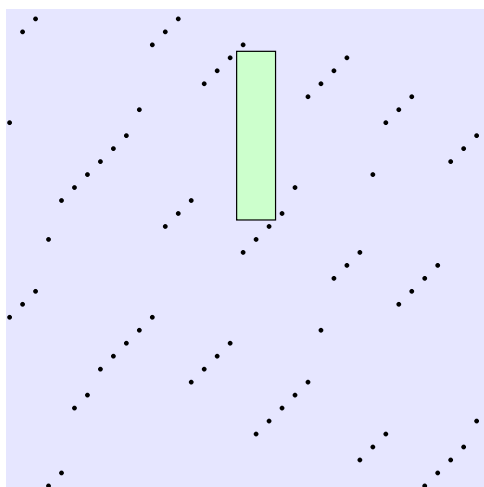

312. (17, 21, 21, 33)

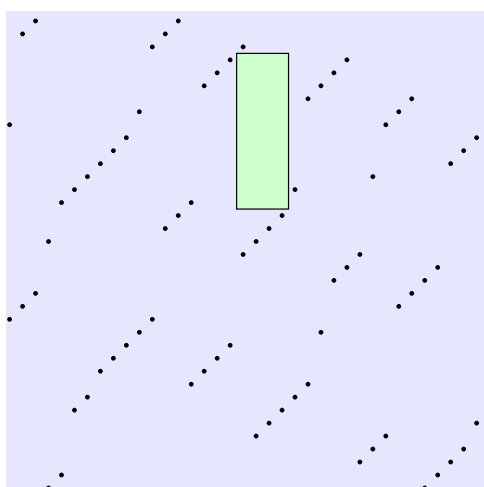



313. (17, 23, 22, 33)

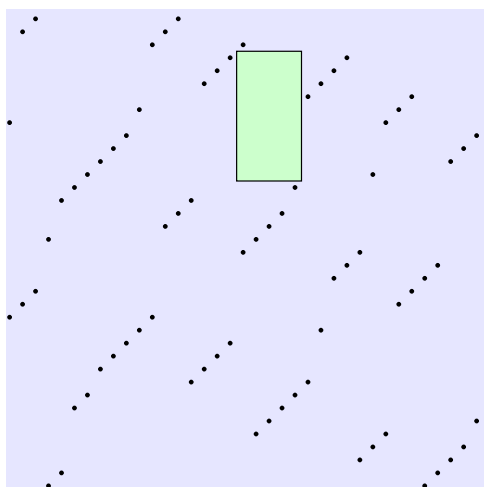

314. (17, 30, 23, 33)

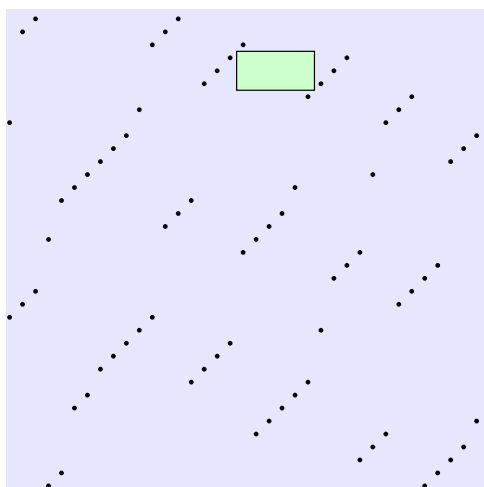

315. (17, 31, 24, 33)

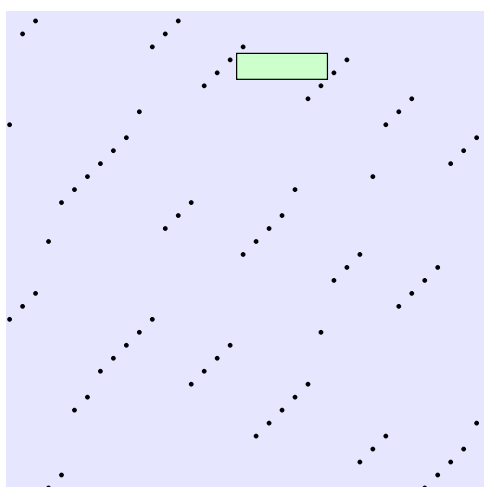

316. (17, 32, 25, 33)

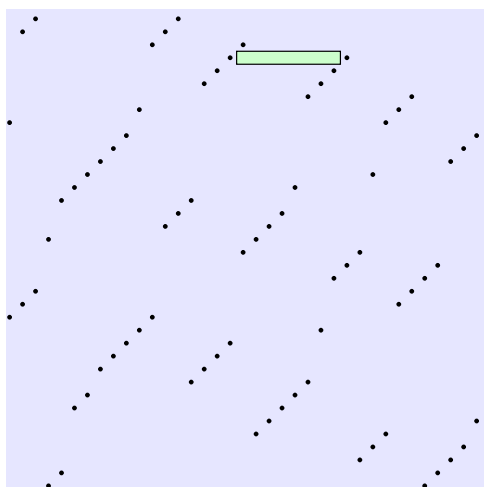

317. (17, 34, 18, 17)

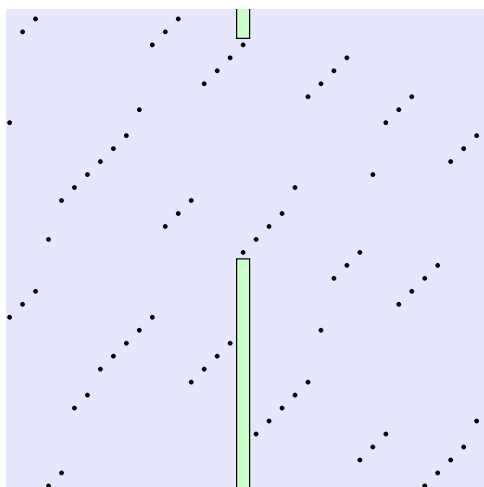

318. (18, 4, 19, 18)

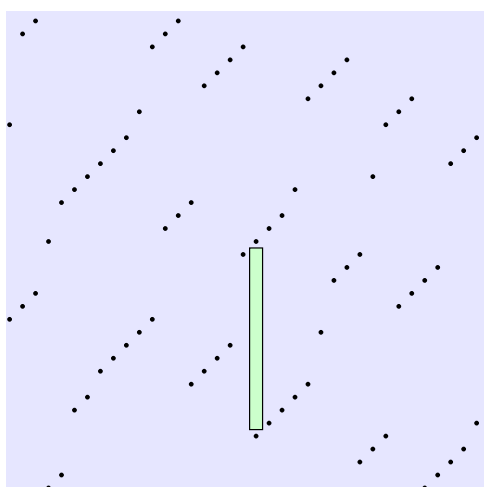

319. (18, 5, 20, 18)

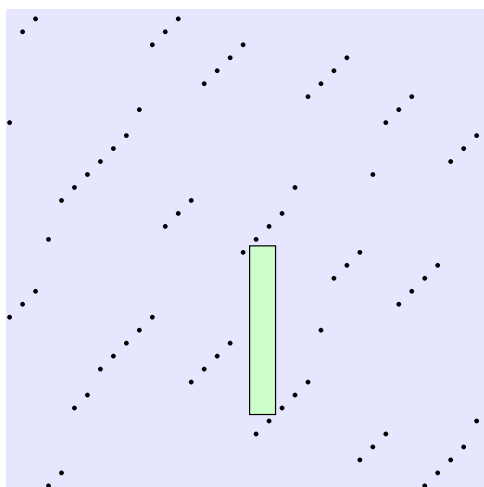

320. (18, 6, 21, 18)

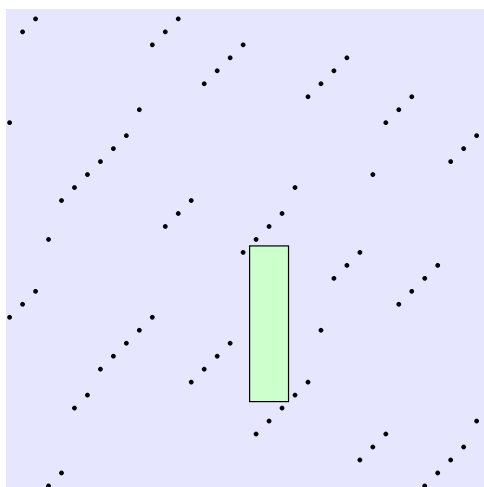

321. (18, 7, 22, 18)

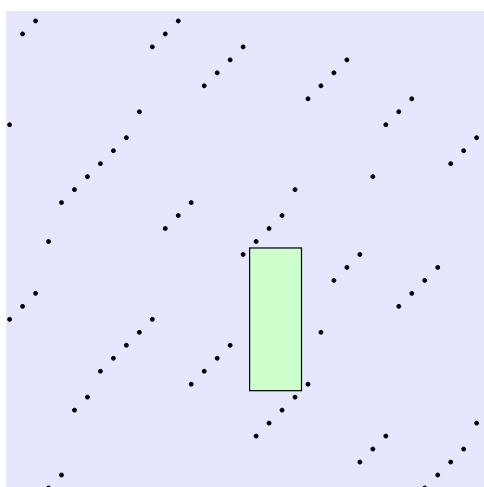

322. (18, 8, 23, 18)

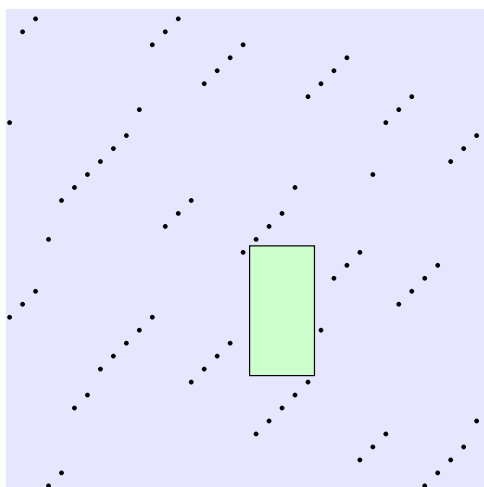

323. (18, 12, 24, 18)

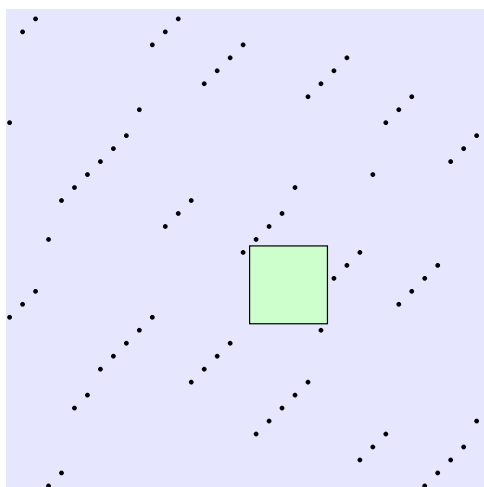

324. (18, 16, 25, 18)

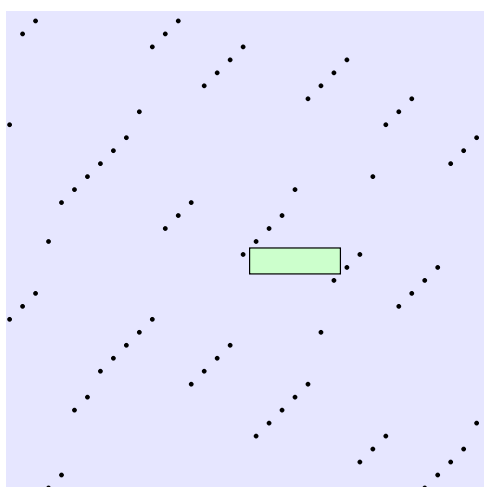

325. (18, 17, 26, 18)

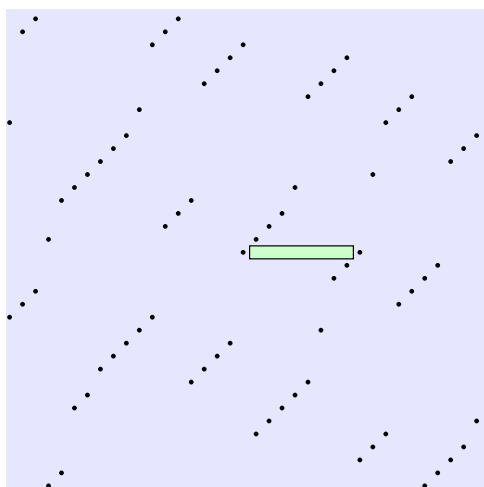

326. (18, 19, 19, 3)

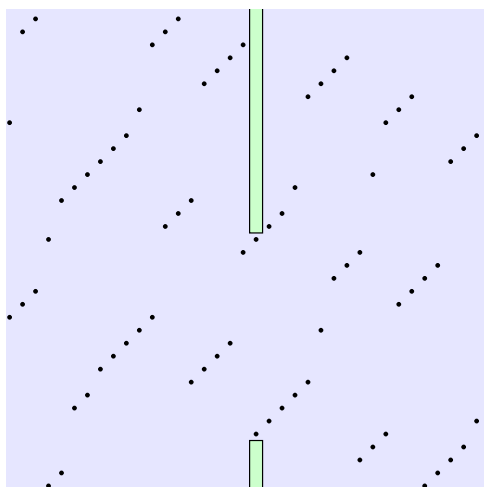

327. (18, 20, 20, 3)

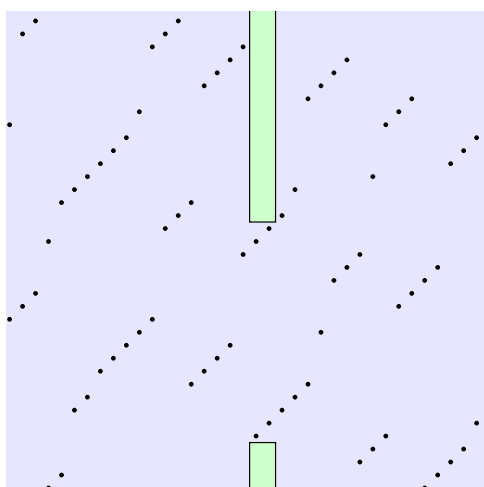

328. (18, 21, 21, 3)

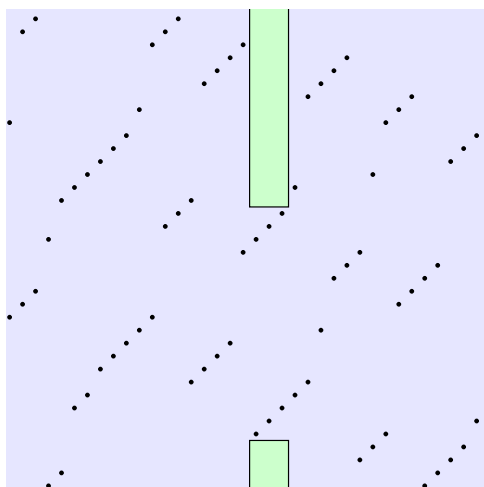

329. (18, 23, 22, 3)

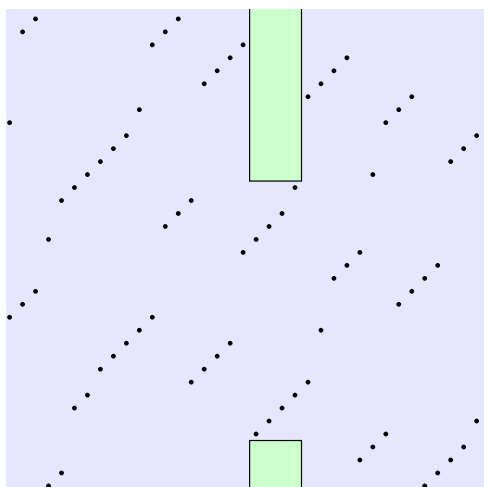

330. (18, 30, 23, 3)

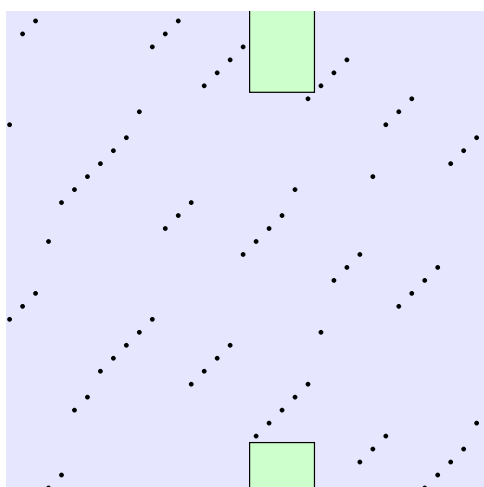

331. (18, 31, 24, 3)

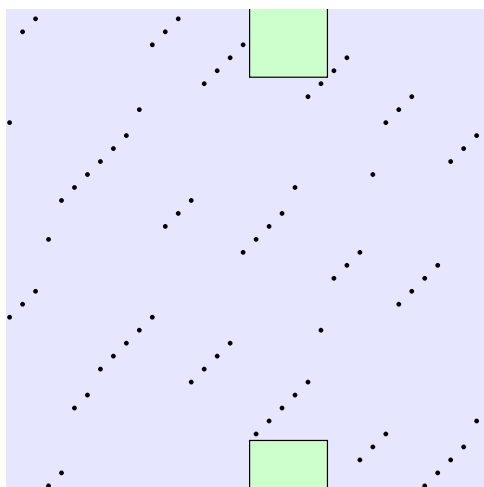

332. (18, 32, 25, 3)

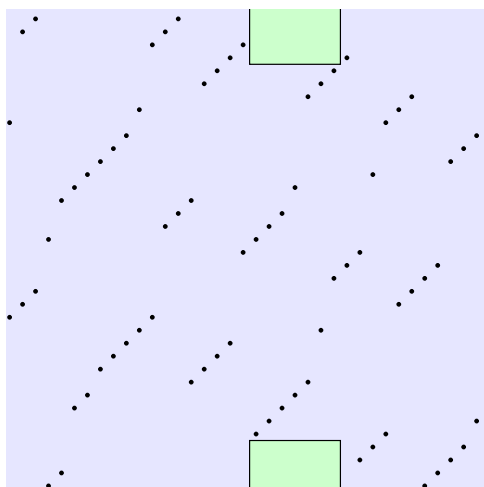

333. (18, 33, 0, 36)

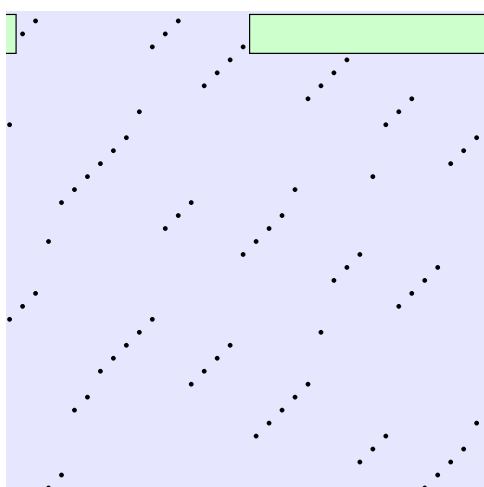

334.  $(18, 33, 10, 34)$

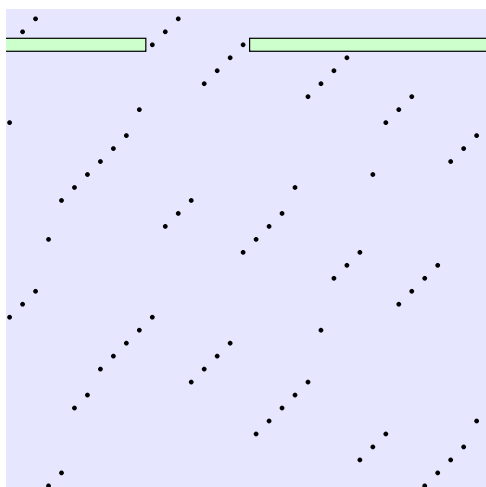

335.  $(18, 33, 26, 3)$

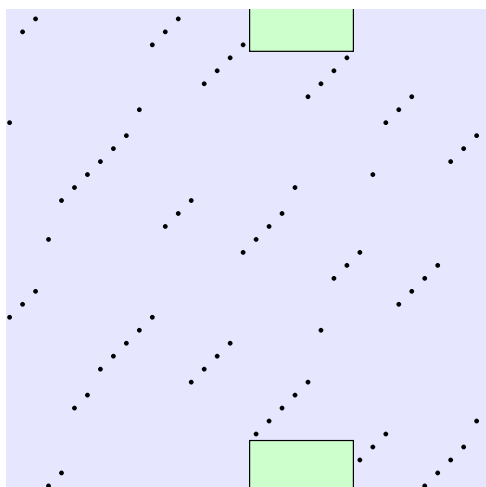

336.  $(18, 33, 31, 1)$

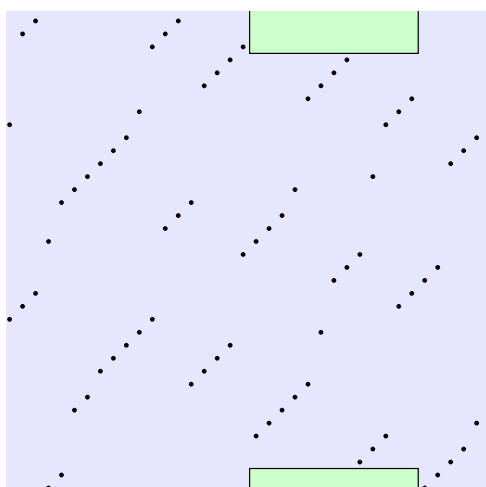



337. (19, 2, 27, 4)

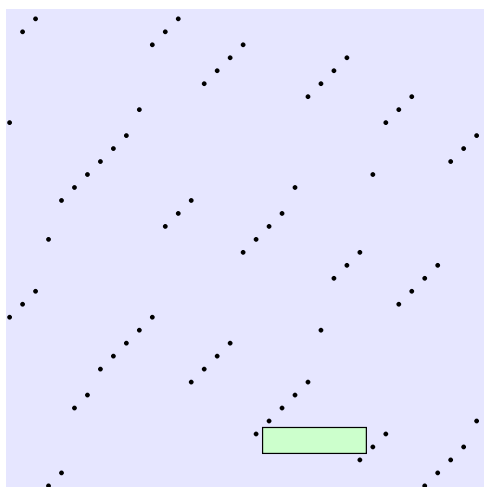

338. (19, 3, 28, 4)

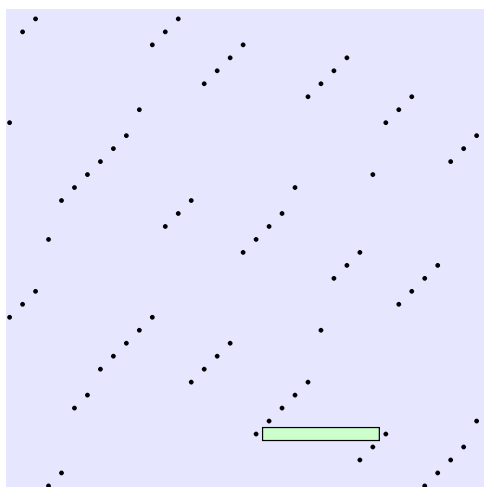

339. (19, 5, 20, 19)

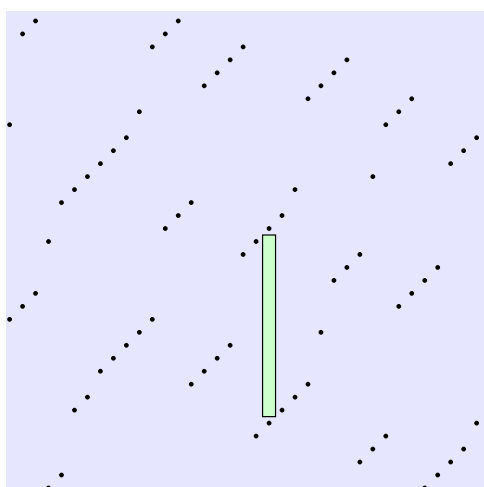

340. (19, 6, 21, 19)

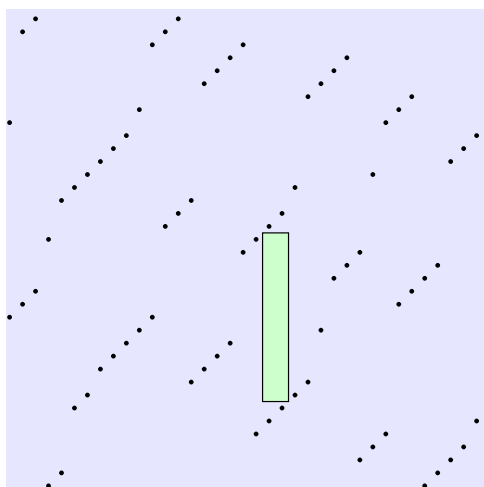

341. (19, 7, 22, 19)

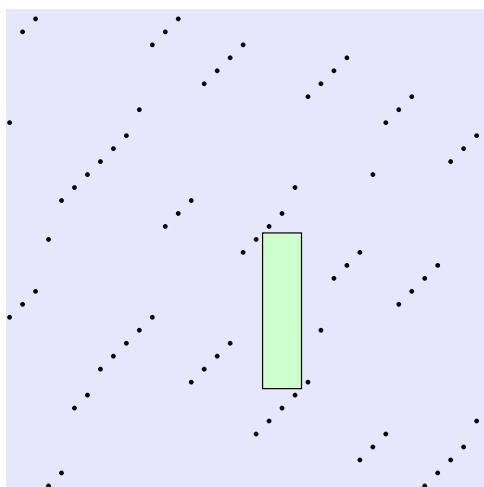

342. (19, 8, 23, 19)

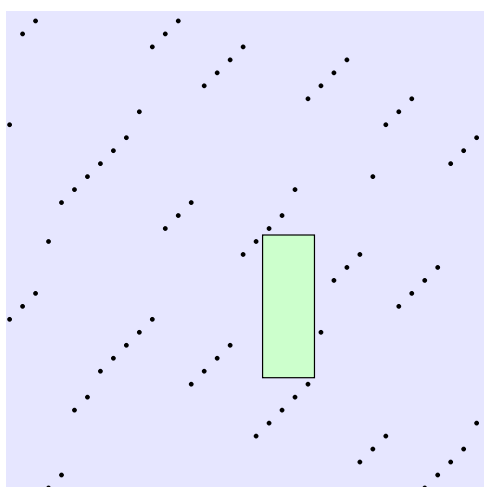

343. (19, 12, 24, 19)

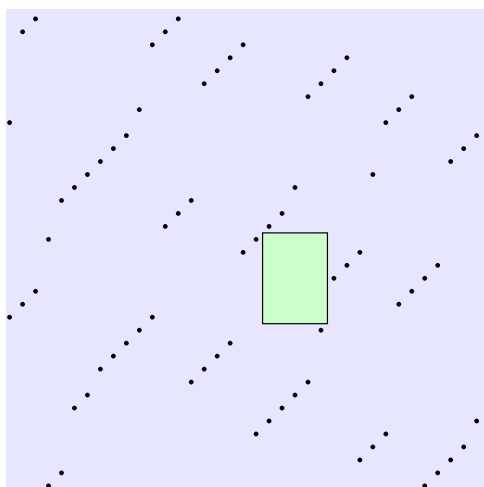

344. (19, 16, 25, 19)

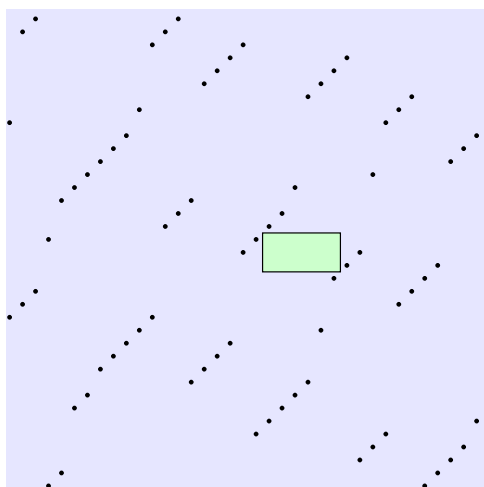

345. (19, 17, 26, 19)

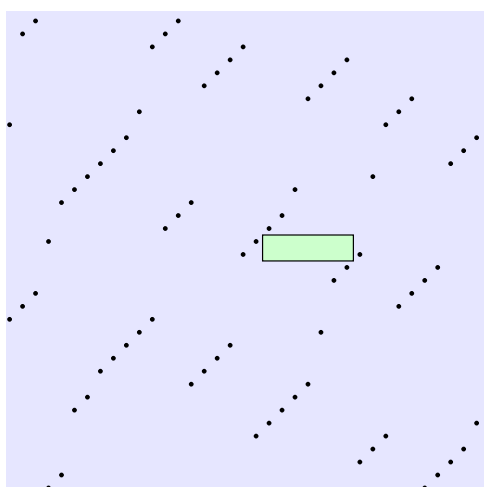

346. (19, 18, 2, 19)

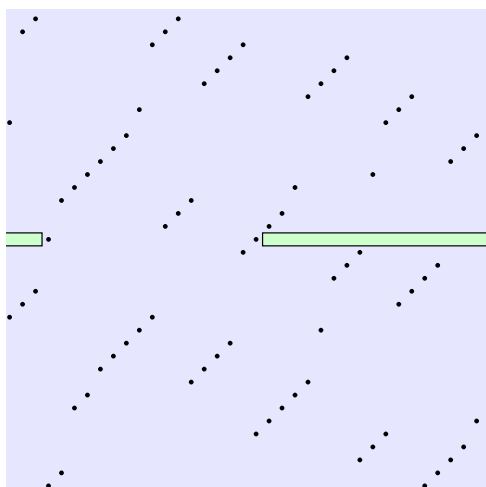

347. (19, 20, 20, 4)

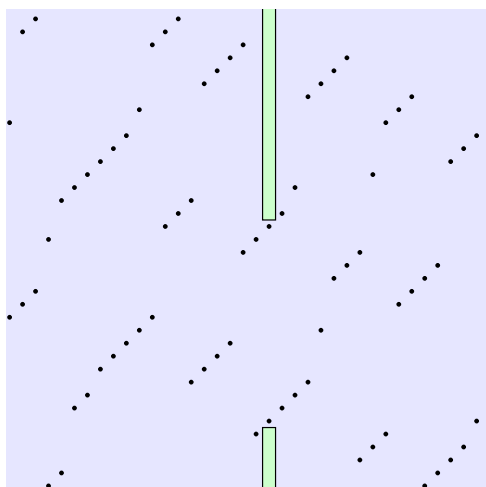

348. (19, 21, 21, 4)

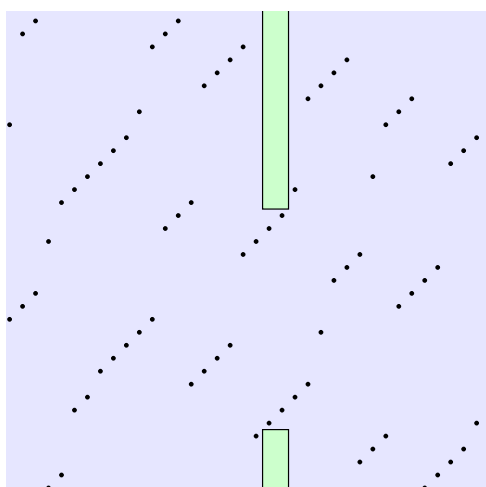

349. (19, 23, 22, 4)

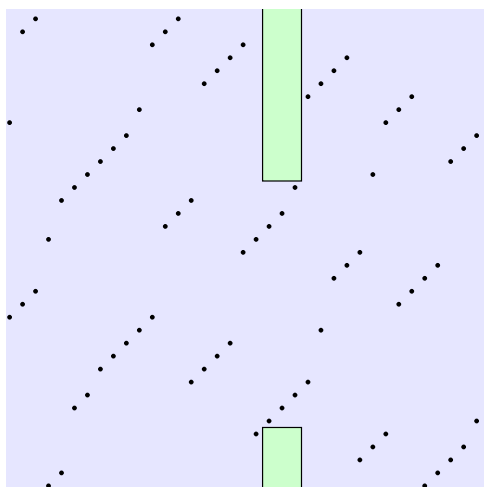

350. (19, 30, 23, 4)

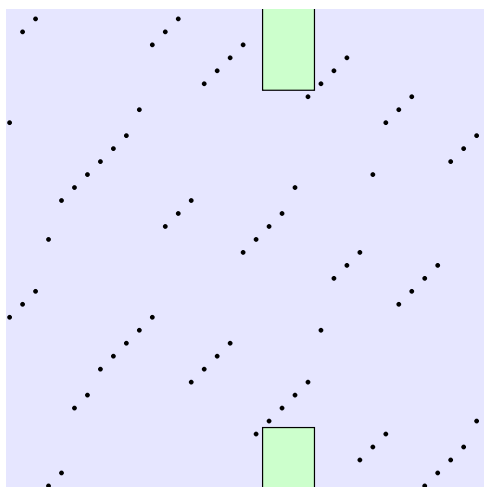

351. (19, 31, 24, 4)

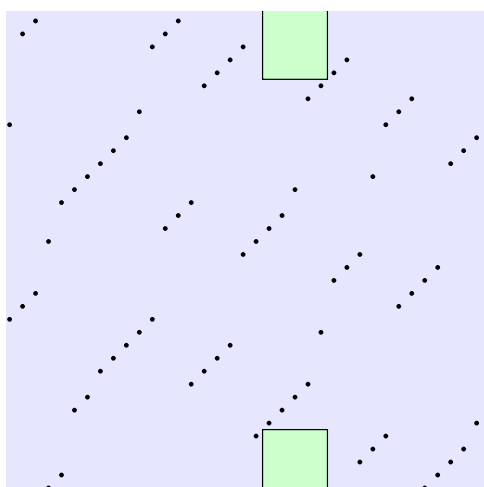

352. (19, 32, 25, 4)

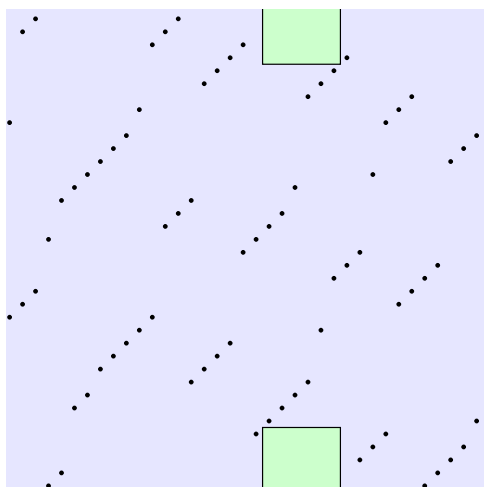

353. (19, 33, 26, 4)

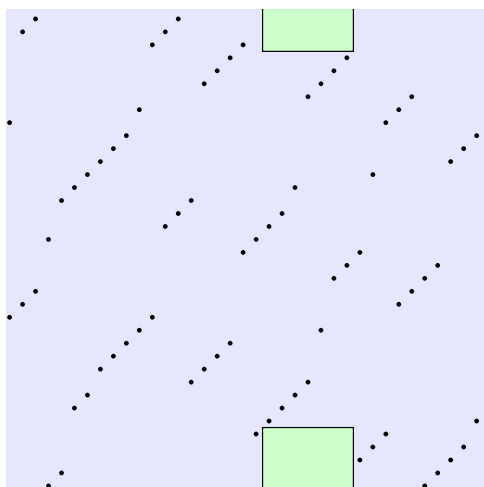

354. (20, 2, 27, 5)

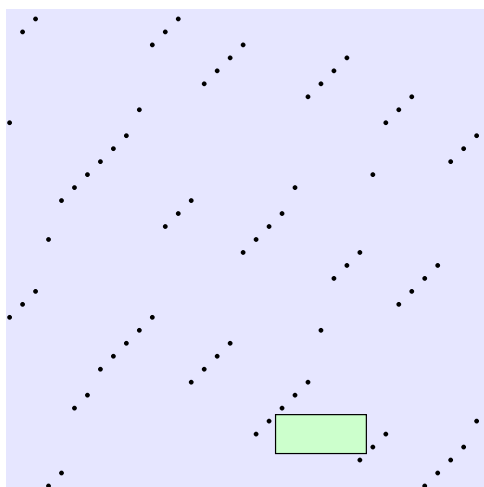

355.  $(20, 3, 28, 5)$

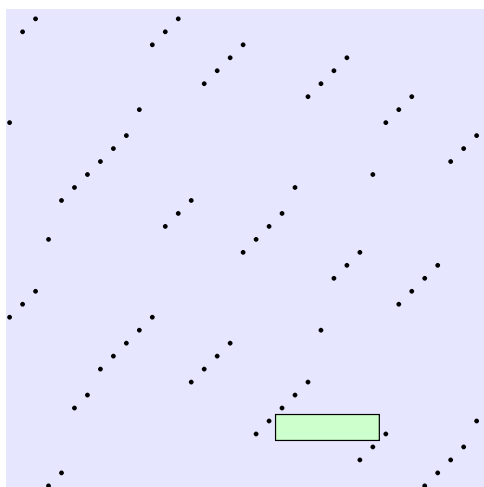

356.  $(20, 4, 35, 5)$

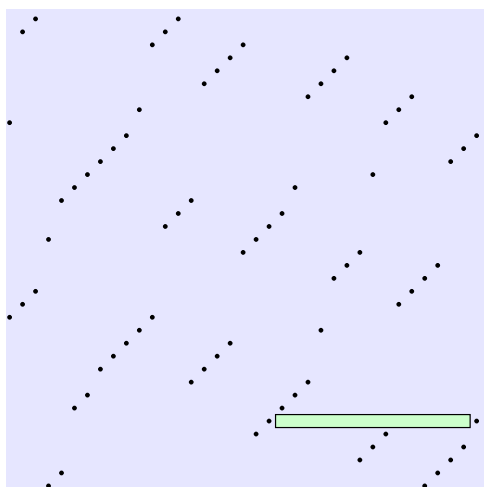

357.  $(20, 6, 21, 20)$

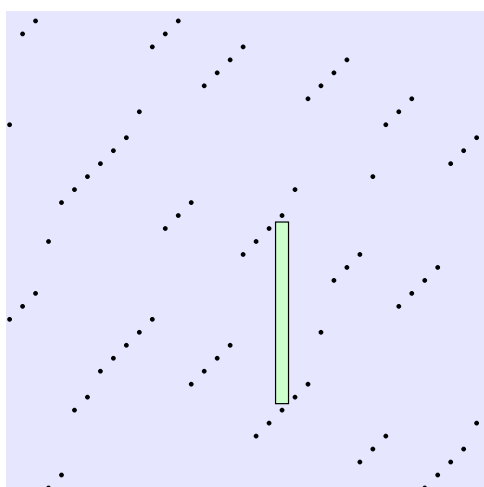

358. (20, 7, 22, 20)

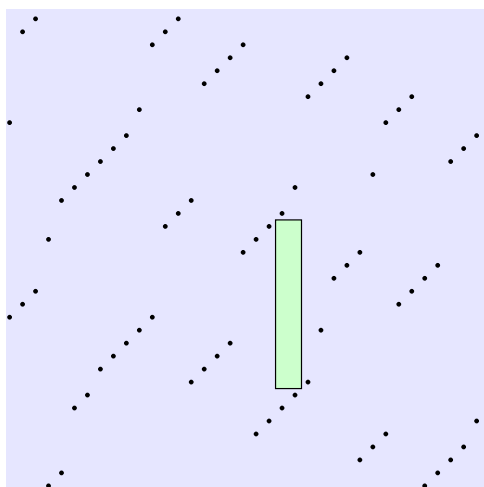

359. (20, 8, 23, 20)

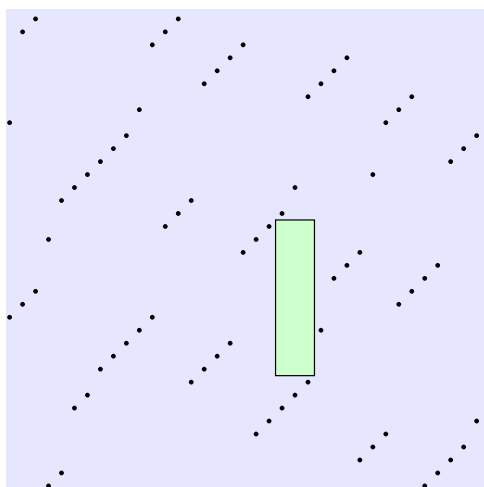

360. (20, 12, 24, 20)

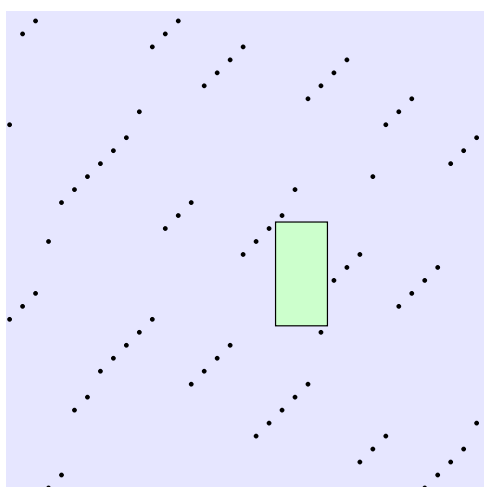



361. (20, 16, 25, 20)

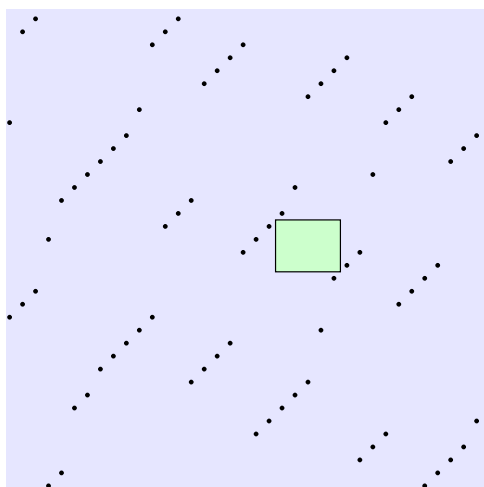

362. (20, 17, 26, 20)

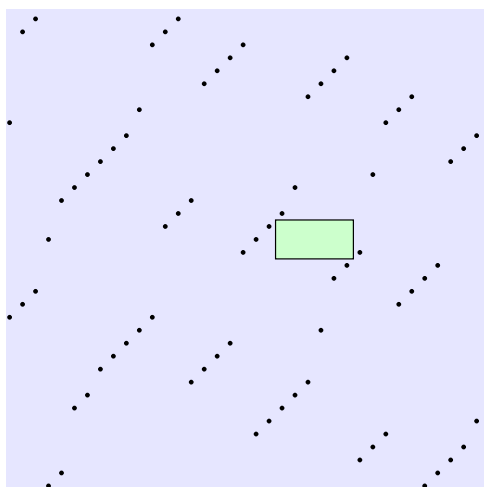

363. (20, 18, 2, 20)

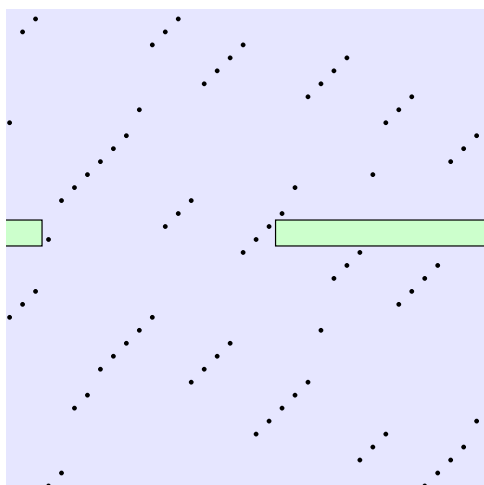

364. (20, 19, 11, 20)

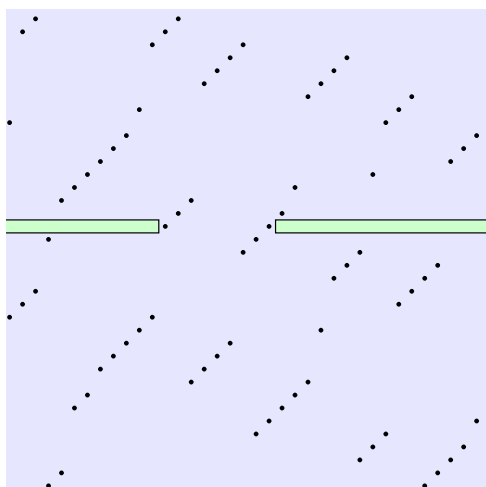

365. (20, 21, 21, 5)

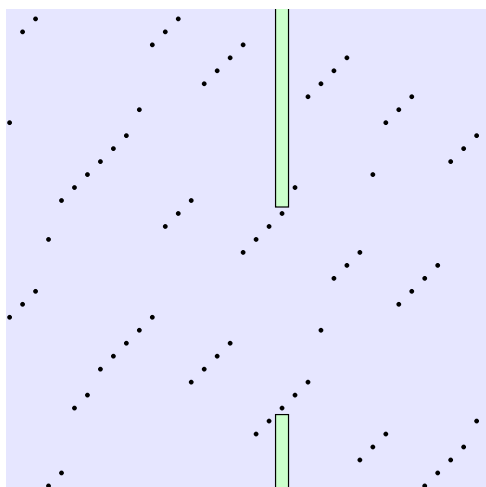

366. (20, 23, 22, 5)

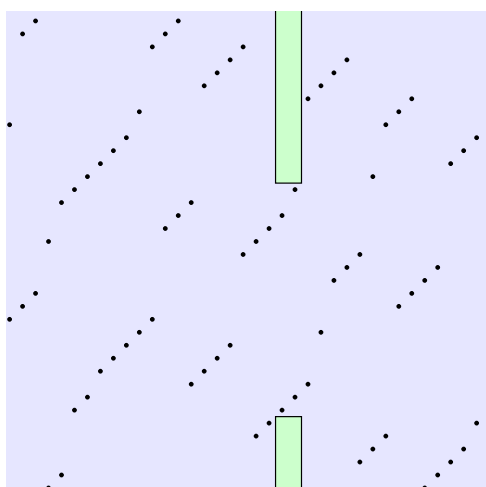

367. (20, 30, 23, 5)

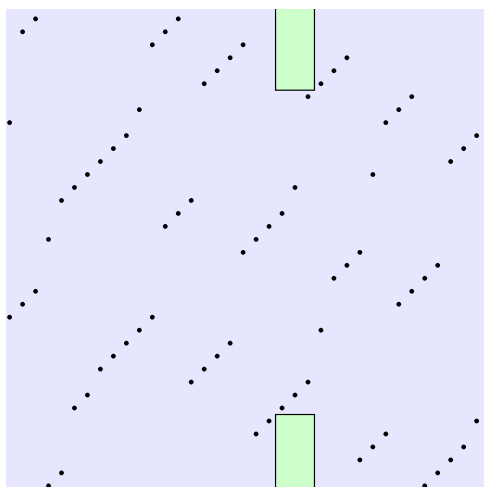

368. (20, 31, 24, 5)

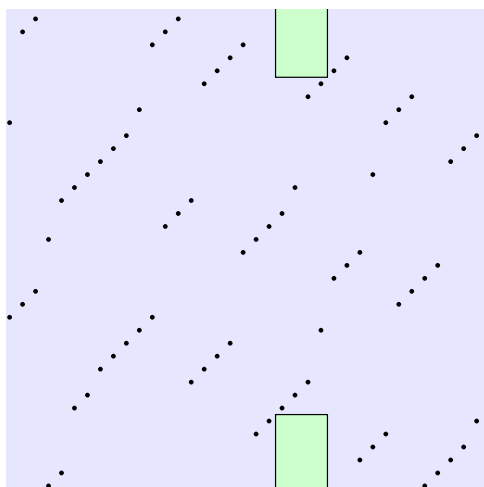

369. (20, 32, 25, 5)

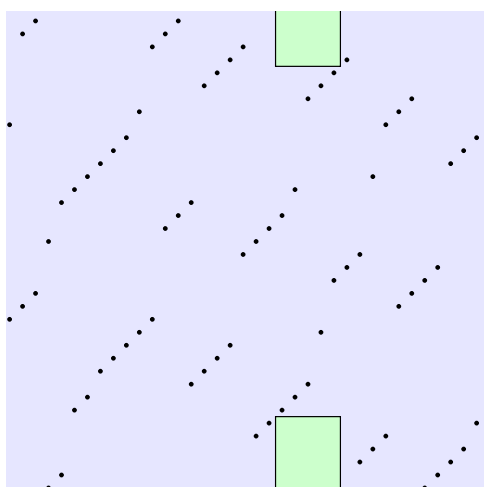

370. (20, 33, 26, 5)

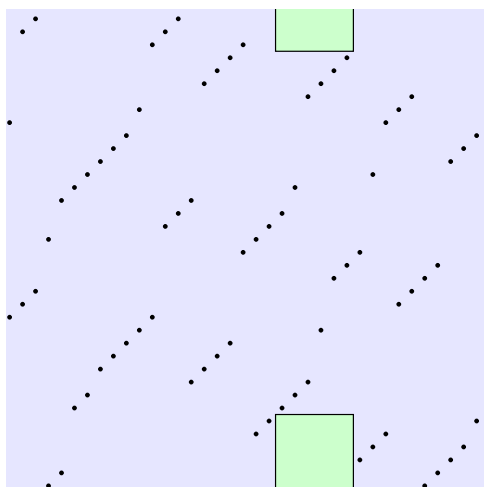

371. (21, 2, 27, 6)

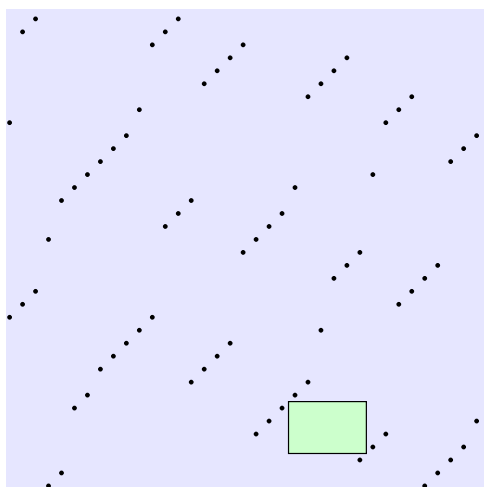

372. (21, 3, 28, 6)

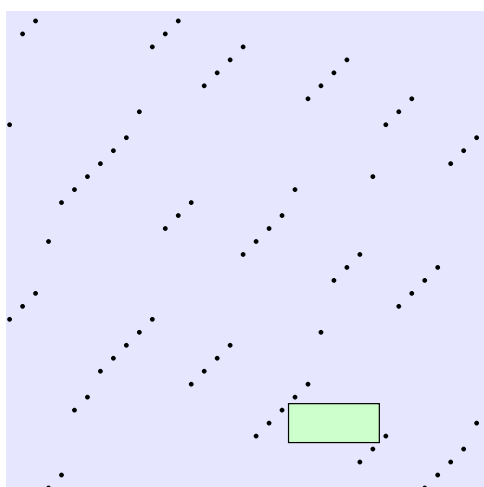

373. (21, 4, 35, 6)

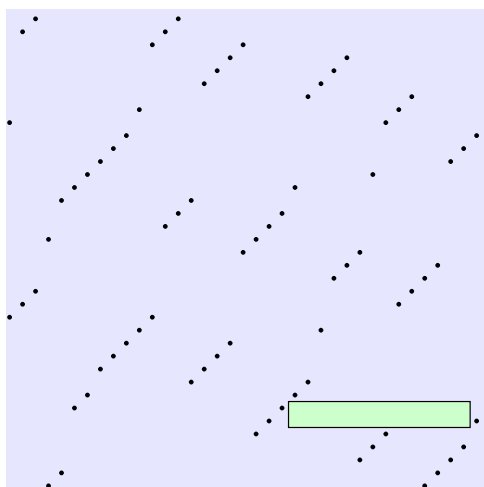

374. (21, 5, 4, 6)

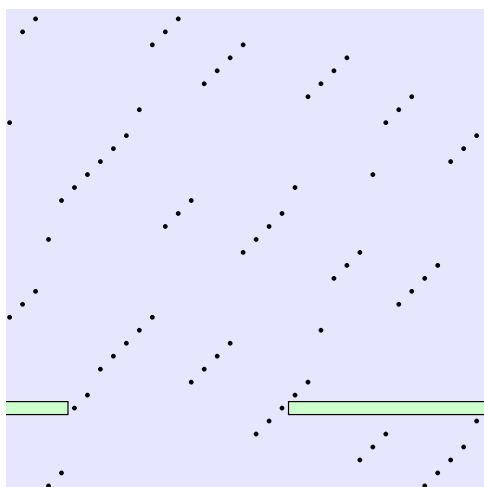

375. (21, 7, 22, 22)

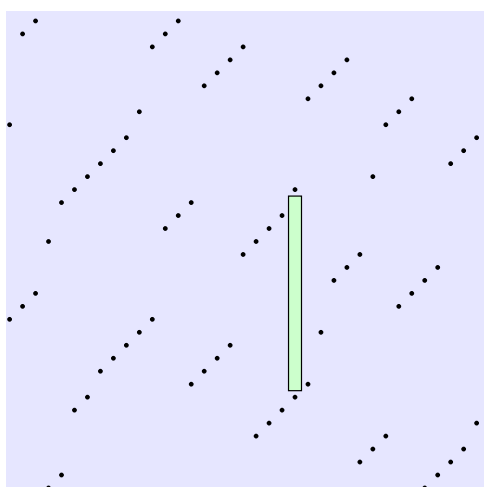

376. (21, 8, 23, 22)

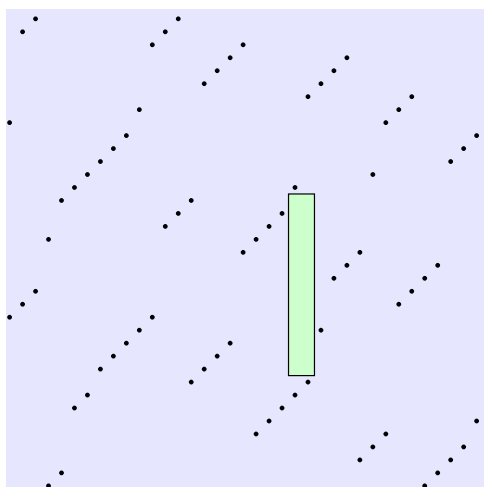

377. (21, 12, 24, 22)

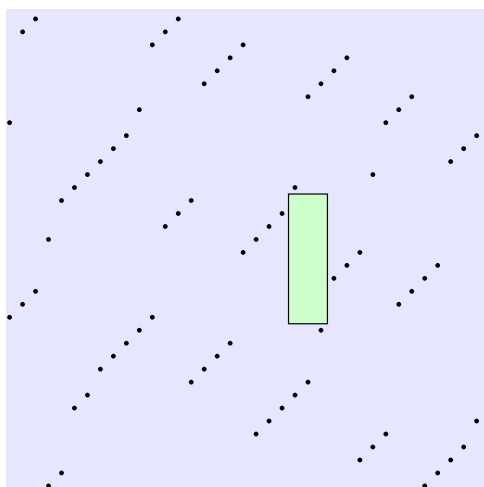

378. (21, 16, 25, 22)

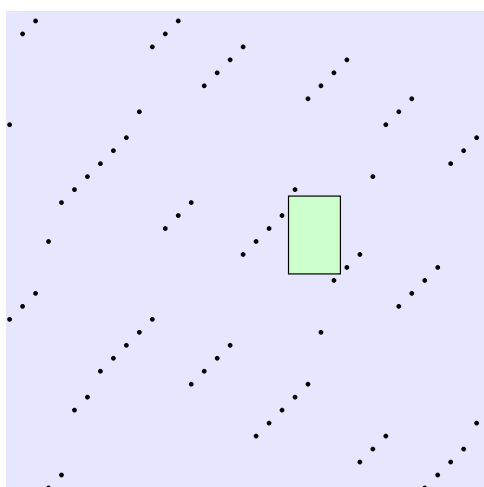

379. (21, 17, 26, 22)

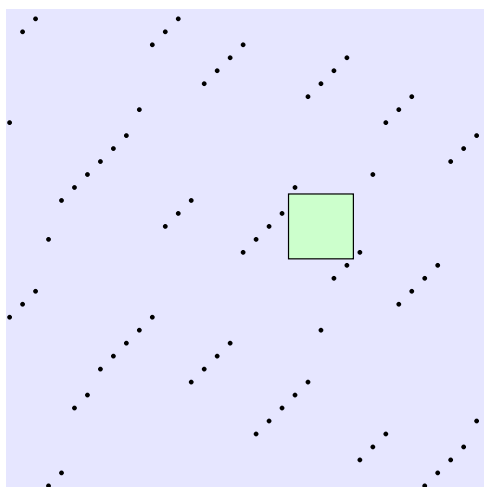

380. (21, 18, 2, 22)

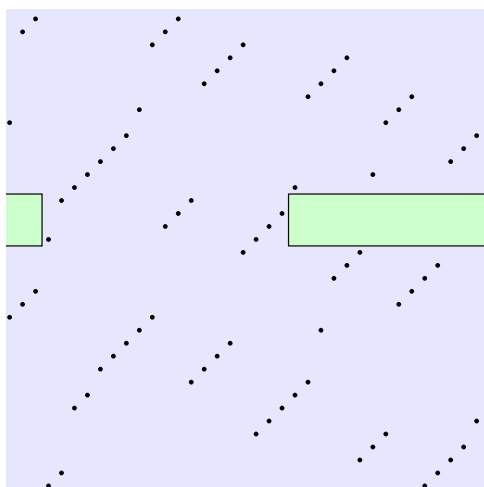

381. (21, 19, 3, 22)

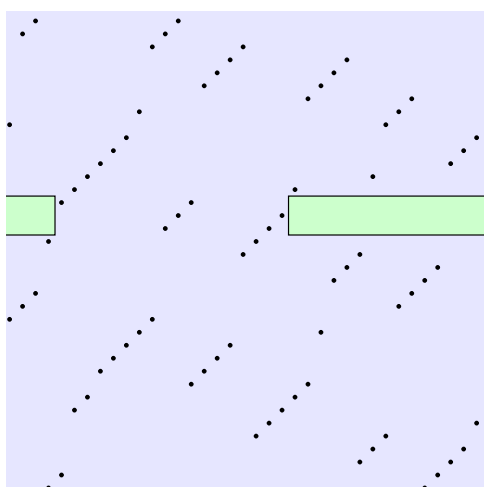

382. (21, 19, 11, 21)

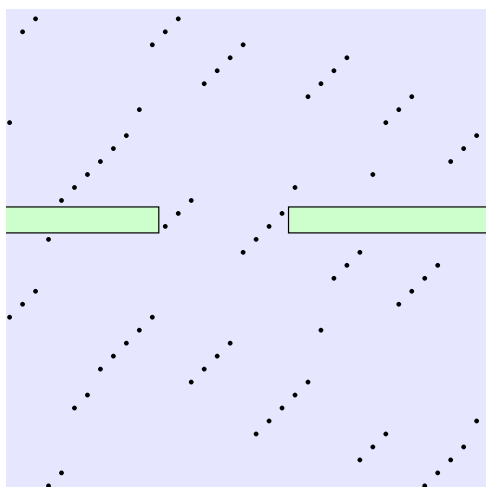

383. (21, 20, 12, 21)

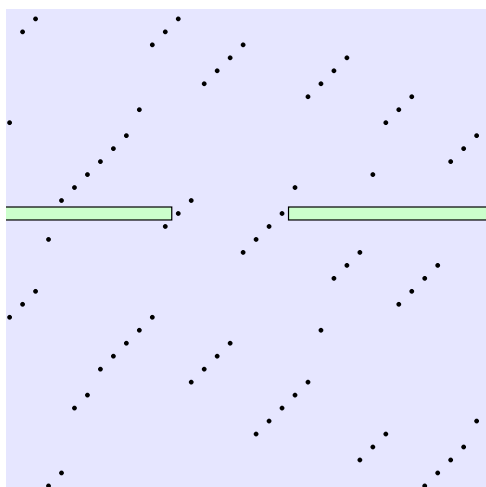

384. (21, 23, 22, 6)

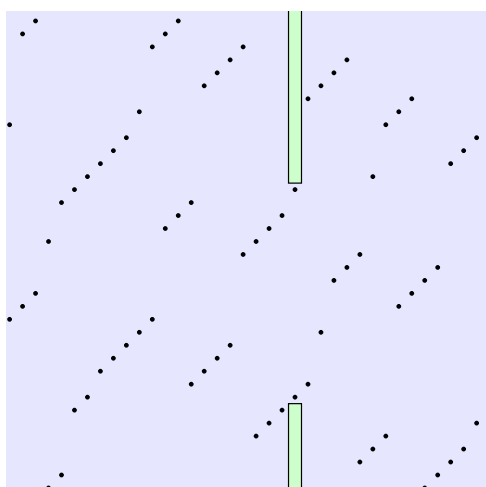



385. (21, 30, 23, 6)

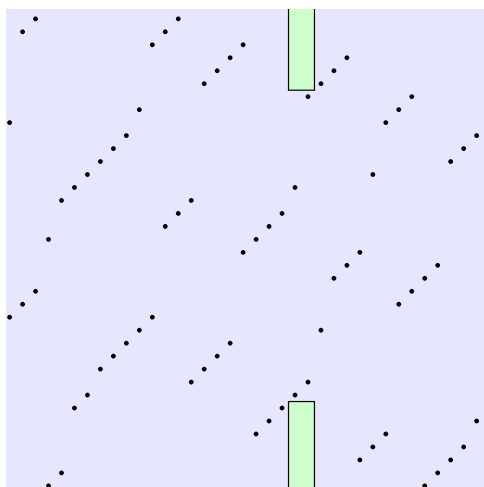

386. (21, 31, 24, 6)

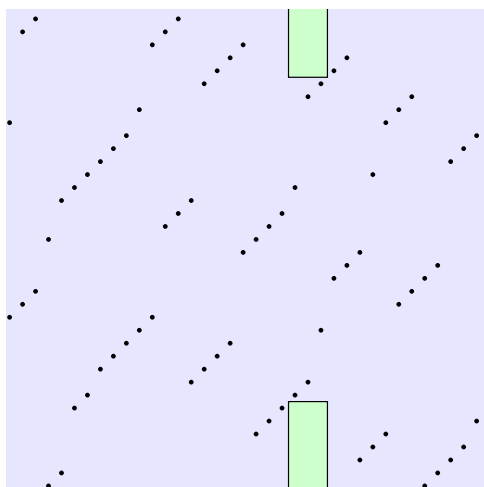

387. (21, 32, 25, 6)

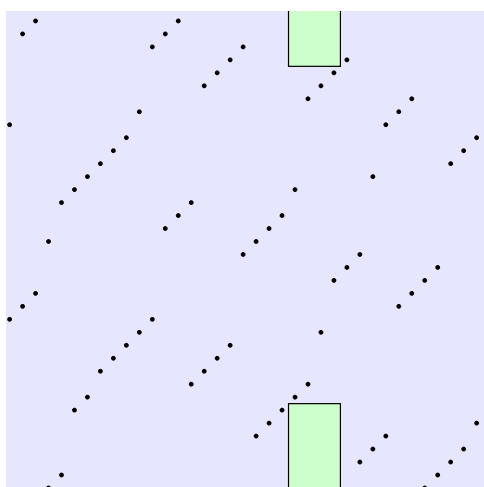

388. (21, 33, 26, 6)

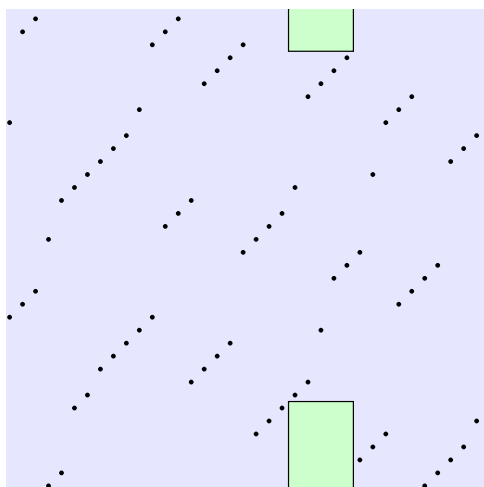

389. (22, 2, 27, 7)

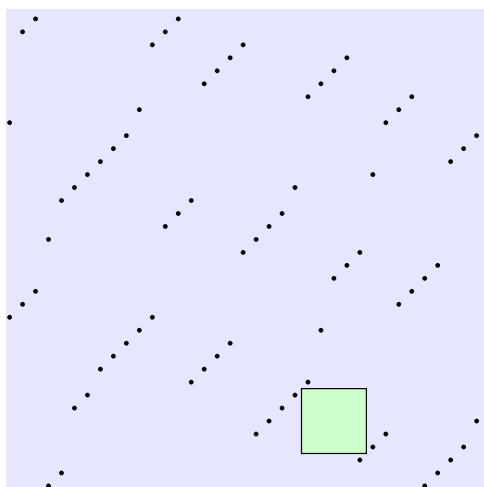

390. (22, 3, 28, 7)

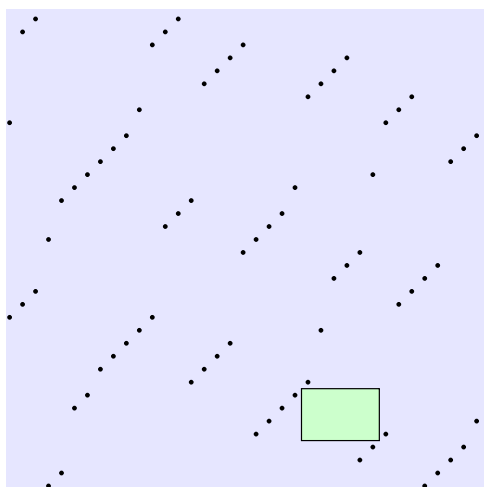

391. (22, 4, 35, 7)

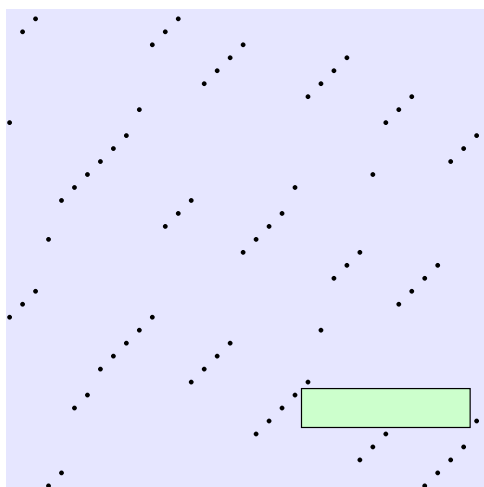

392. (22, 5, 4, 7)

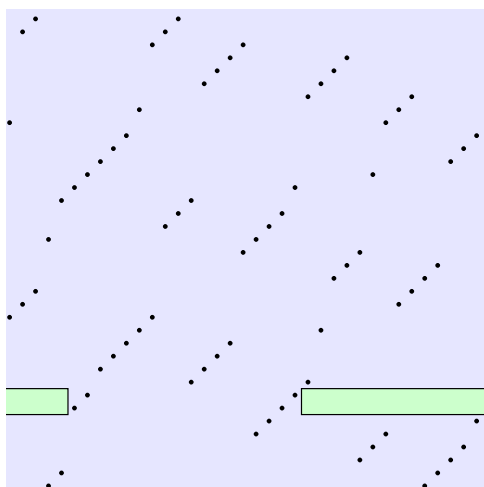

393. (22, 6, 5, 7)

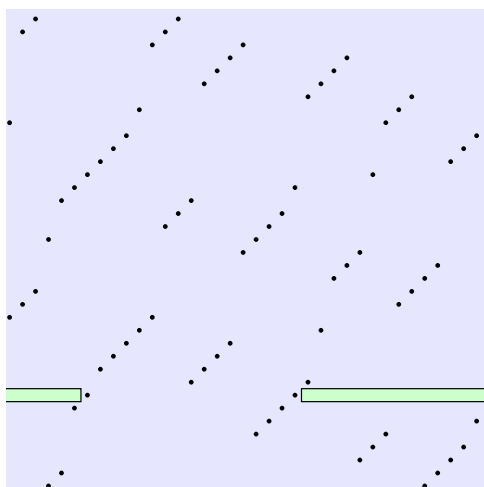

394. (22, 8, 23, 29)

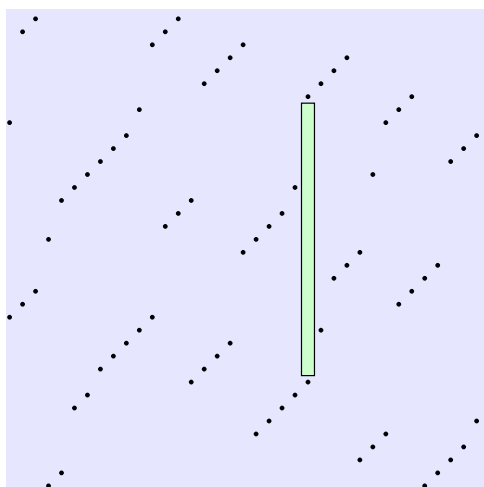

395. (22, 12, 24, 29)

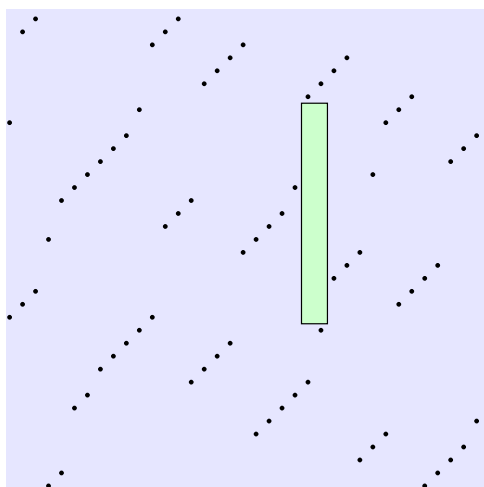

396. (22, 16, 25, 29)

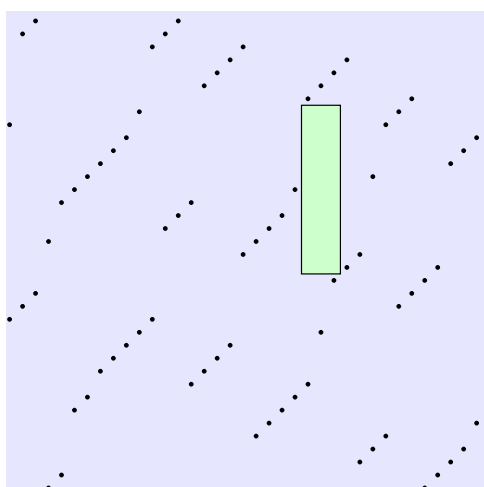

397. (22, 17, 26, 29)

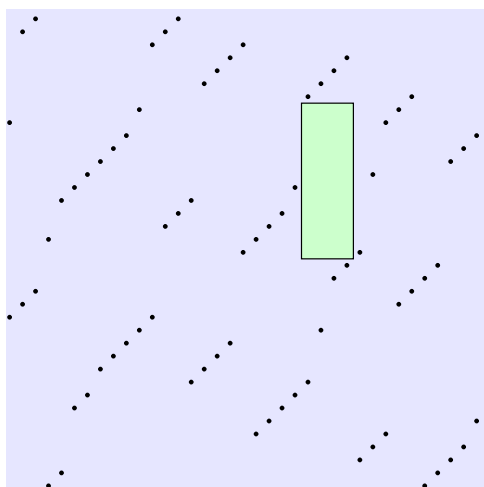

398. (22, 18, 2, 23)

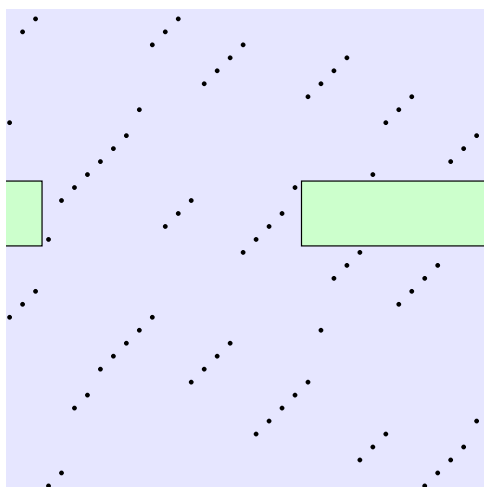

399. (22, 18, 27, 29)

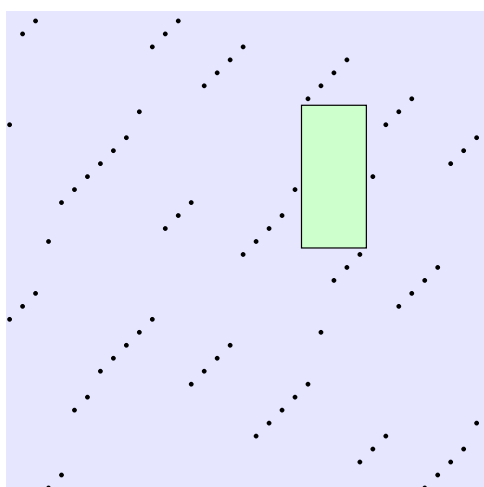

400. (22, 19, 3, 23)

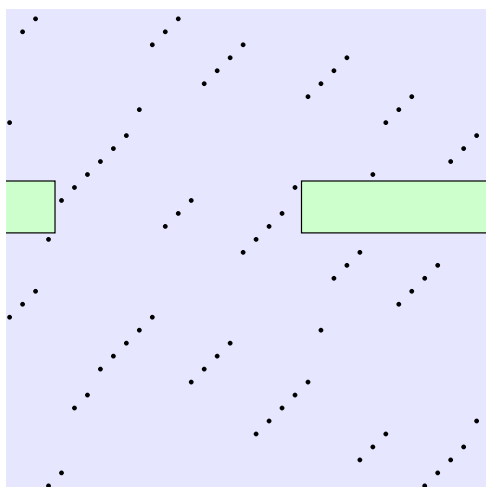

401. (22, 22, 4, 23)

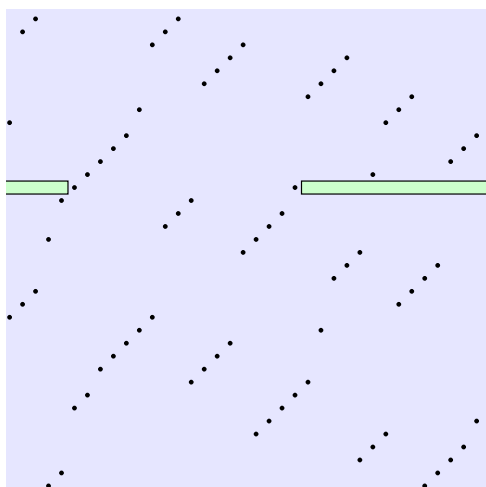

402. (22, 30, 23, 7)

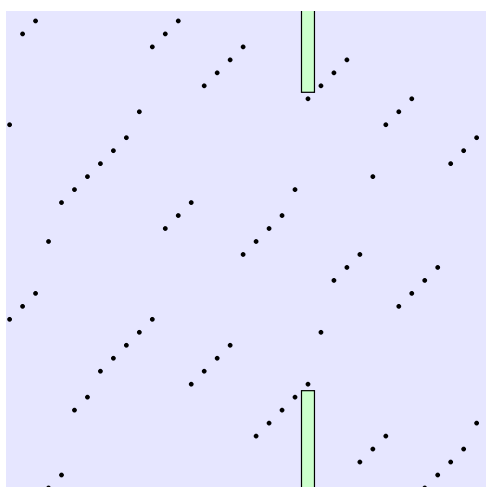

403. (22, 31, 24, 7)

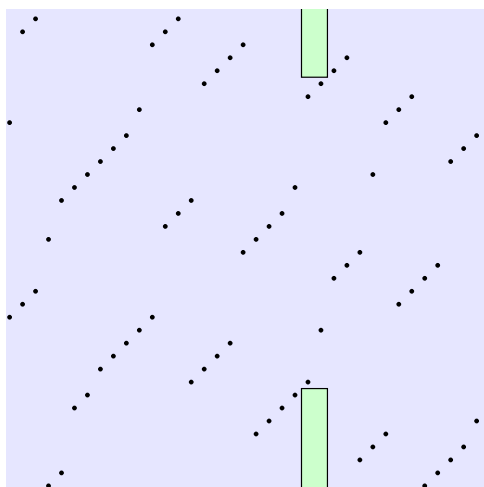

404. (22, 32, 25, 7)

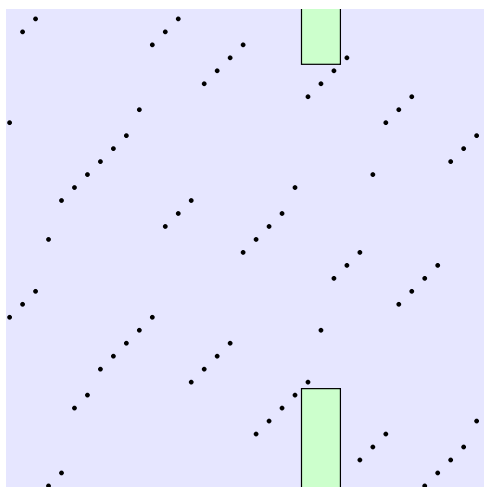

405. (22, 33, 26, 7)

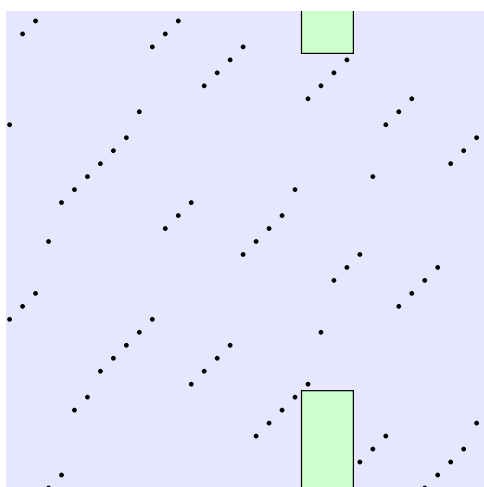

406. (23, 2, 27, 11)

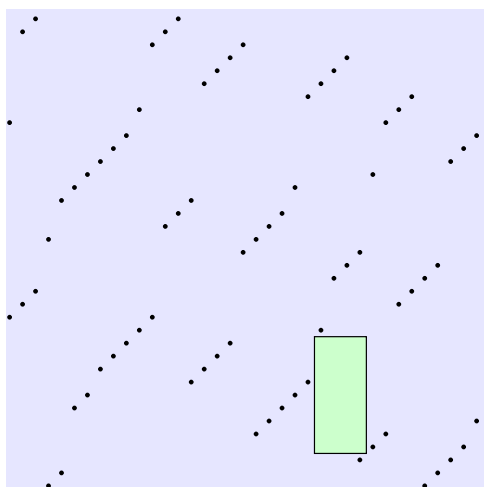

407. (23, 3, 28, 11)

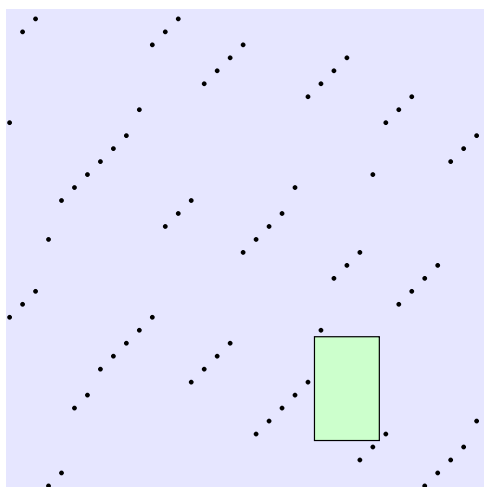

408. (23, 4, 35, 11)

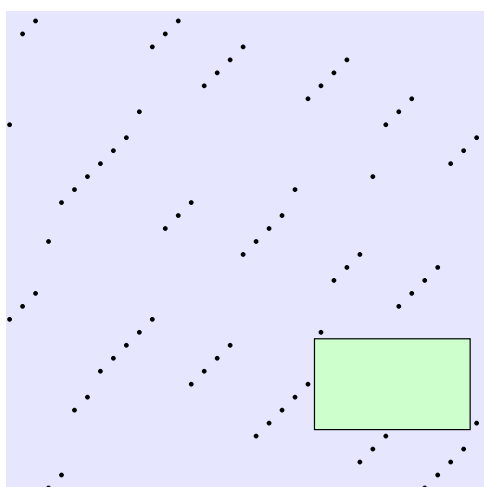



409.  $(23, 5, 4, 11)$

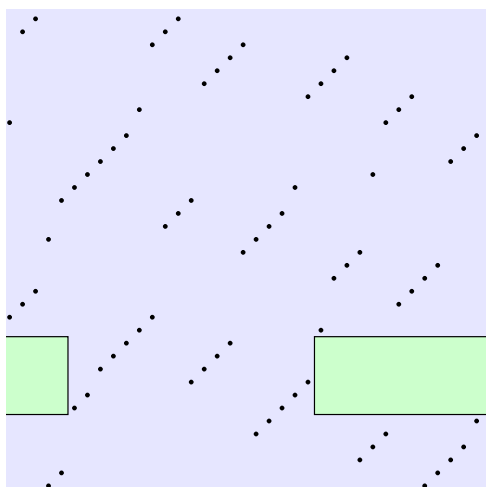

410.  $(23, 6, 5, 11)$

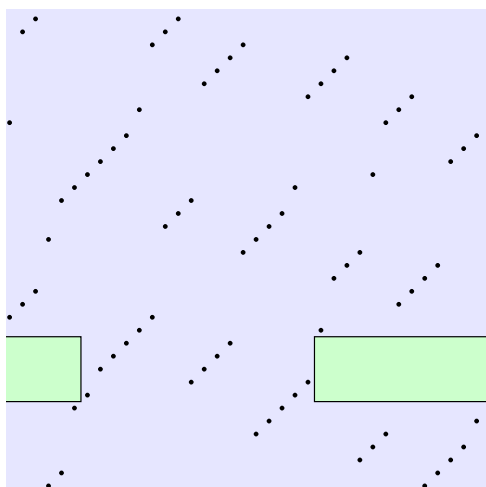

411.  $(23, 7, 6, 11)$

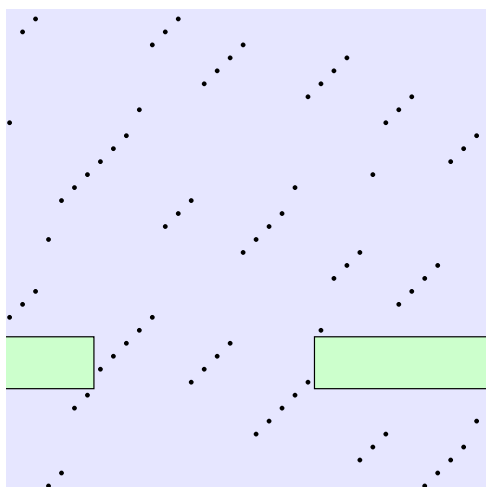

412. (23, 7, 13, 8)

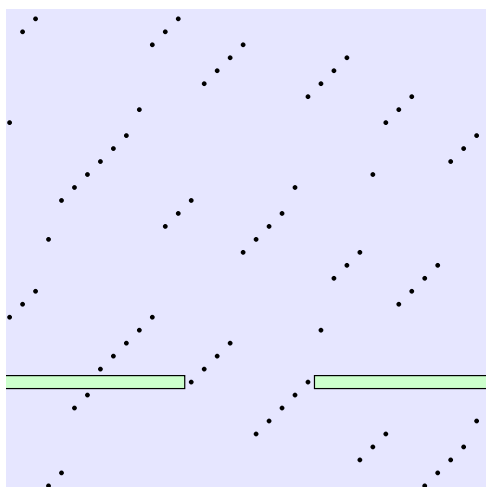

413. (23, 12, 24, 30)

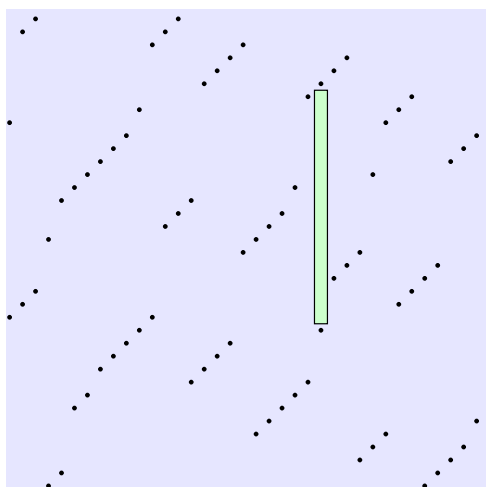

414. (23, 16, 25, 30)

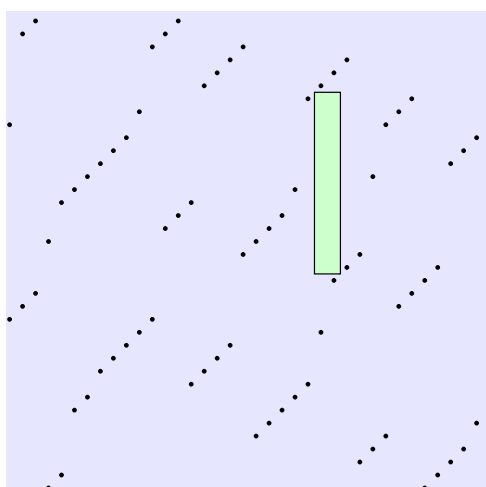

415. (23, 17, 26, 30)

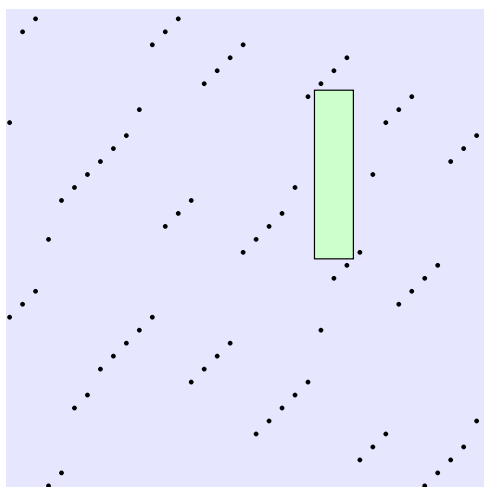

416. (23, 18, 27, 30)

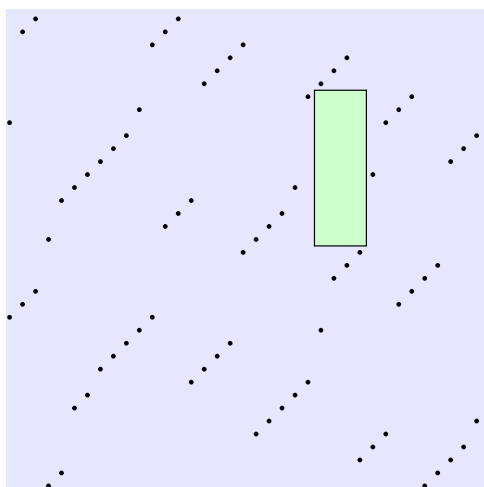

417. (23, 24, 28, 30)

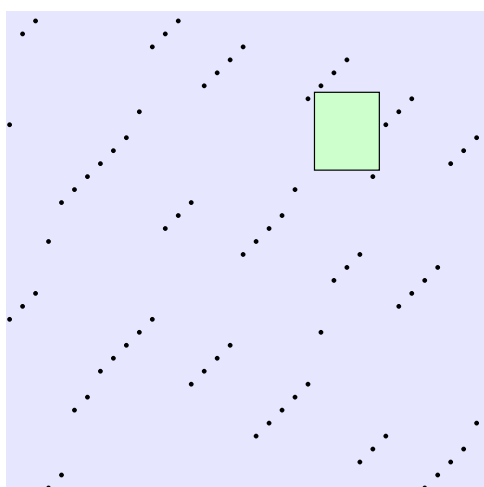

418. (23, 28, 29, 30)

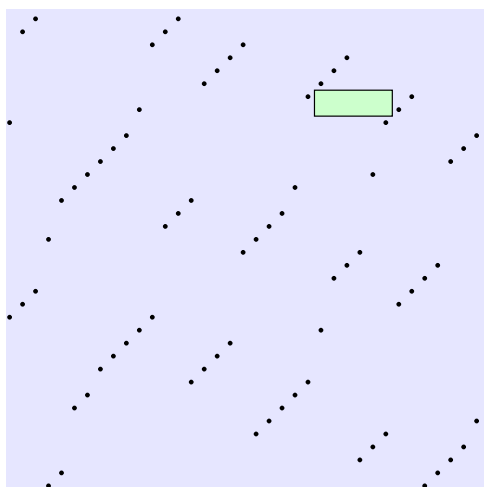

419. (23, 29, 30, 30)

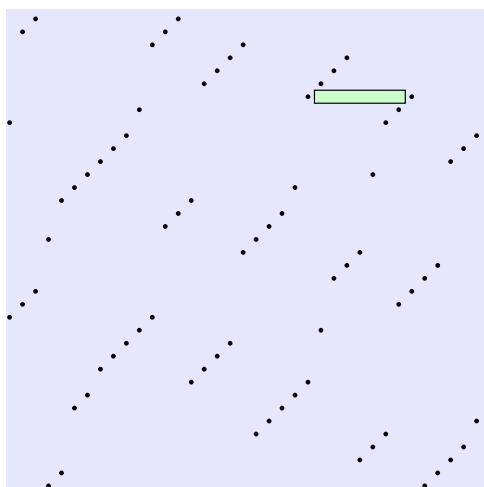

420. (23, 31, 24, 11)

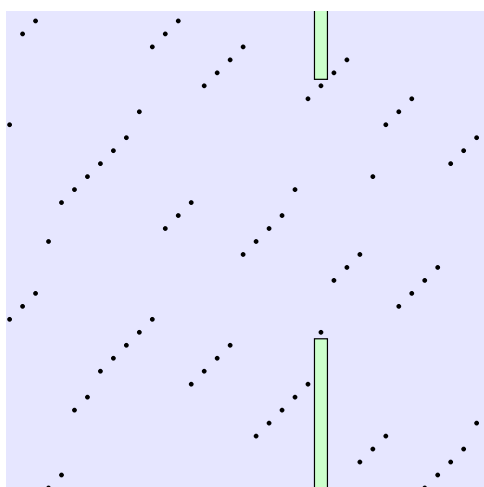

421. (23, 32, 25, 11)

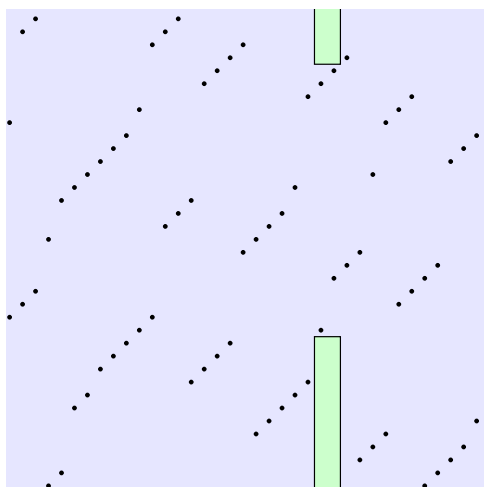

422. (23, 33, 26, 11)

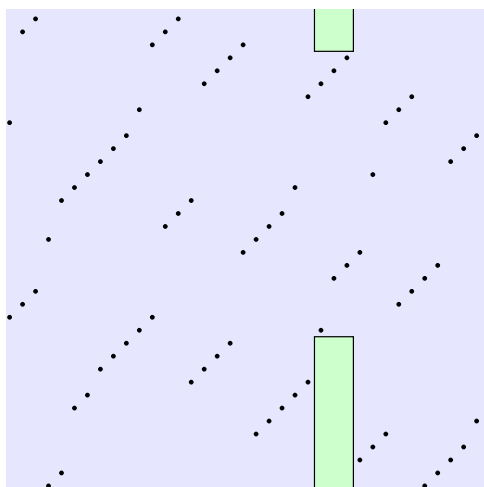

423. (24, 2, 27, 15)

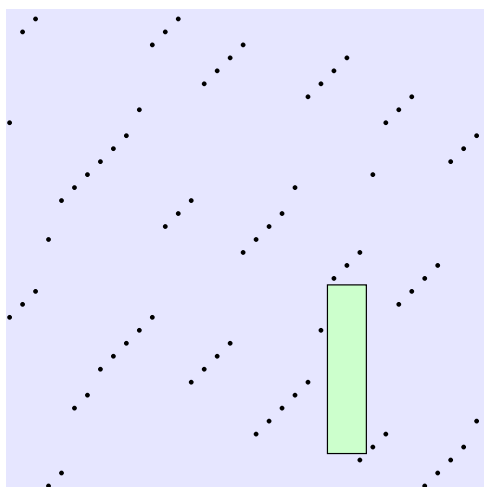

424. (24, 3, 28, 15)

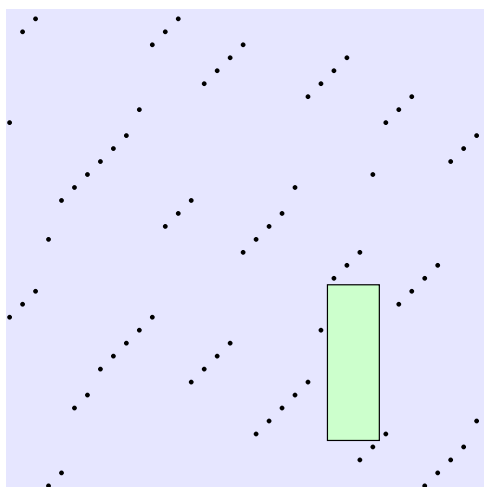

425. (24, 4, 29, 15)

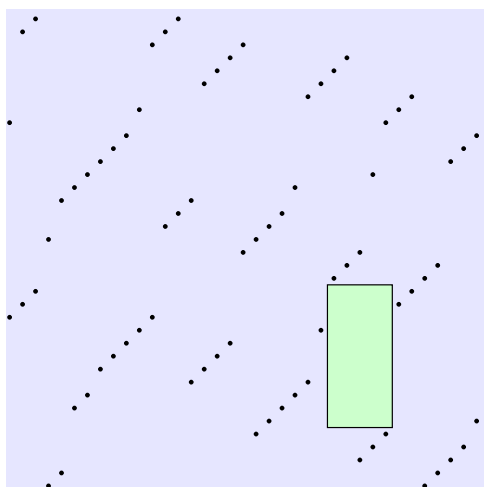

426. (24, 4, 35, 13)

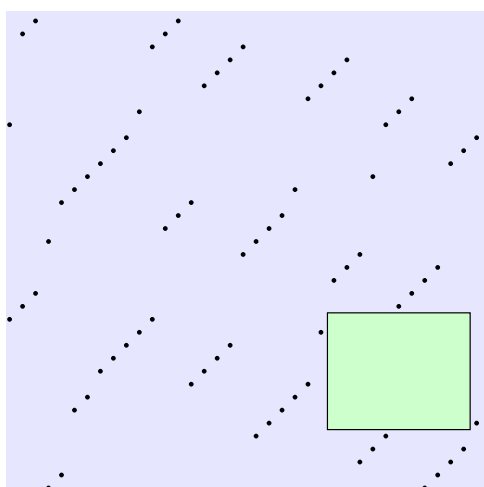

427.  $(24, 5, 4, 12)$

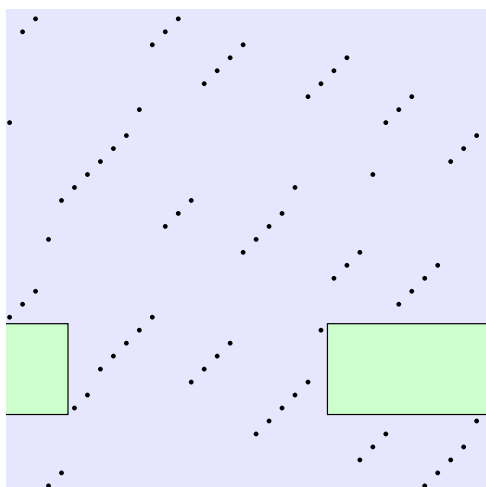

428.  $(24, 5, 36, 13)$

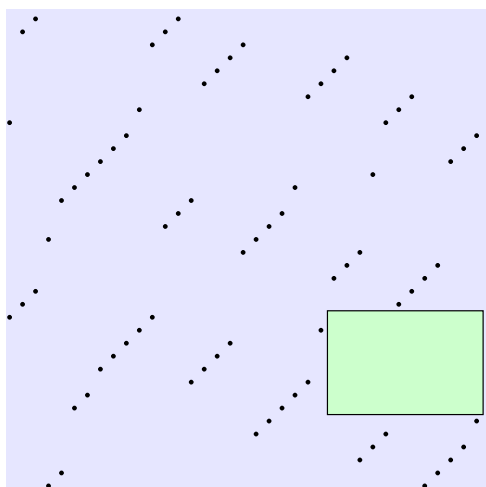

429.  $(24, 6, 5, 12)$

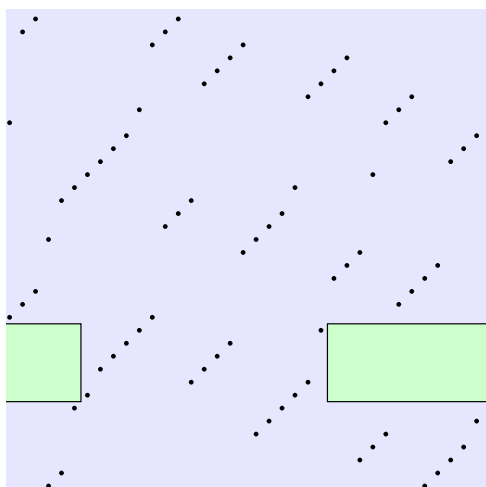

430. (24, 7, 6, 12)

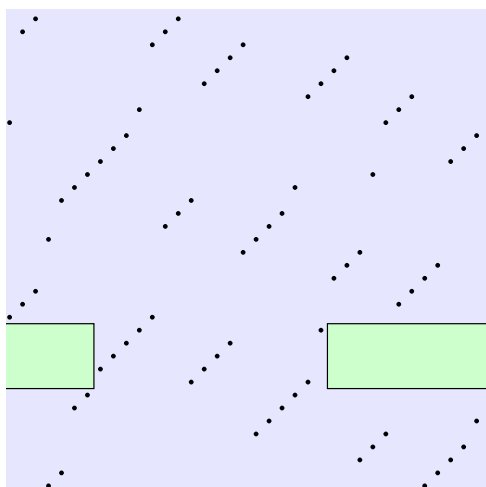

431. (24, 9, 7, 12)

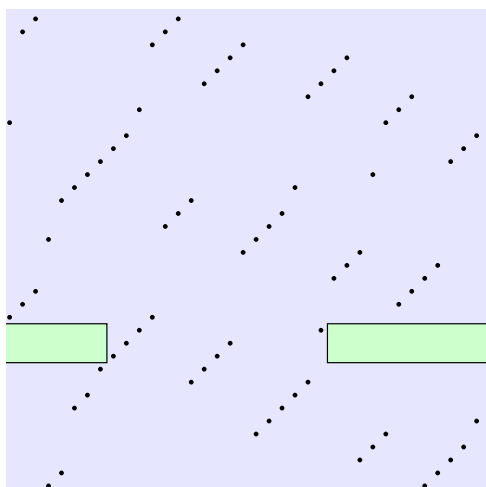

432. (24, 10, 8, 12)

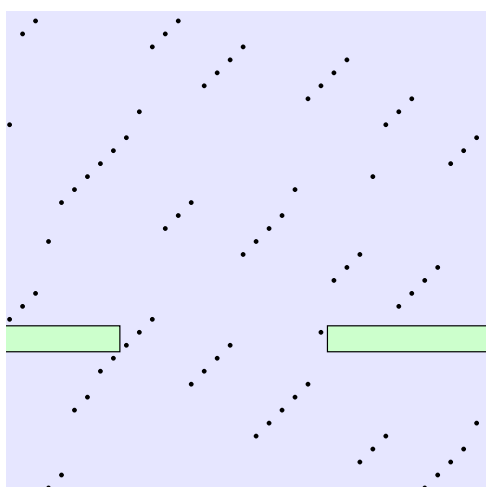



433. (24, 11, 9, 12)

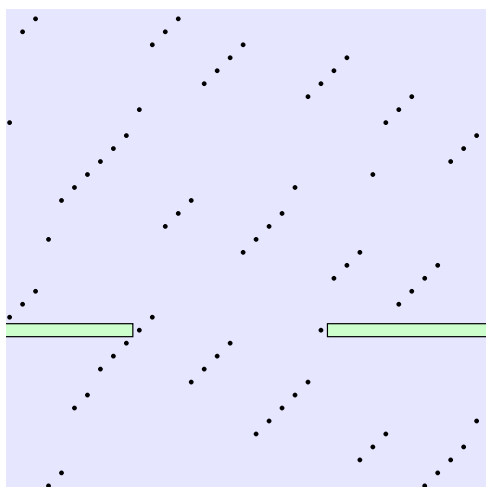

434. (24, 16, 25, 31)

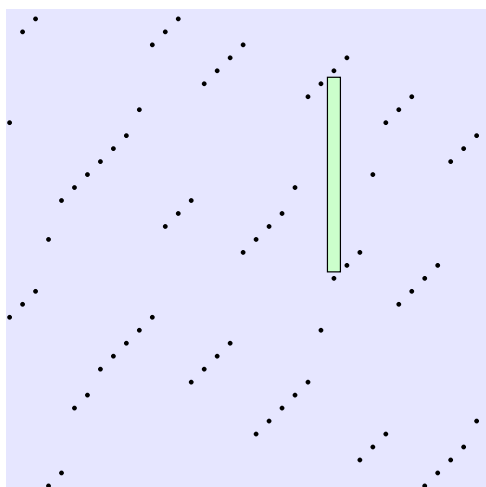

435. (24, 17, 26, 31)

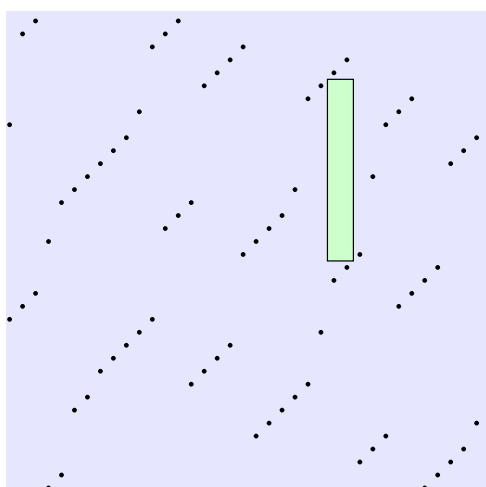

436. (24, 18, 27, 31)

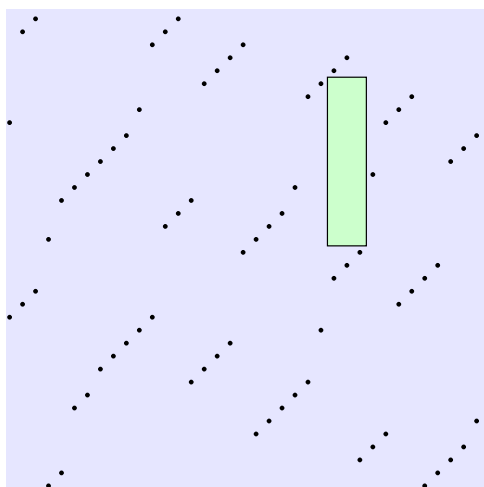

437. (24, 24, 28, 31)

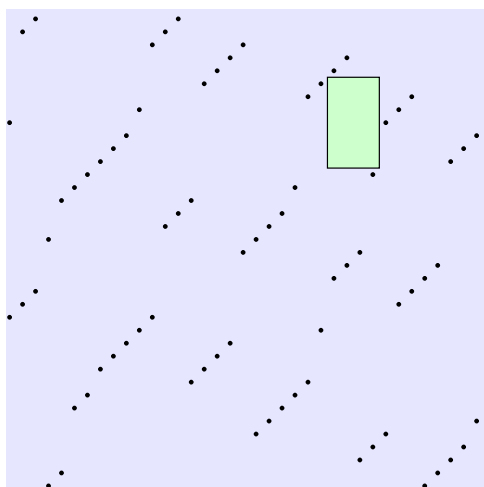

438. (24, 28, 29, 31)

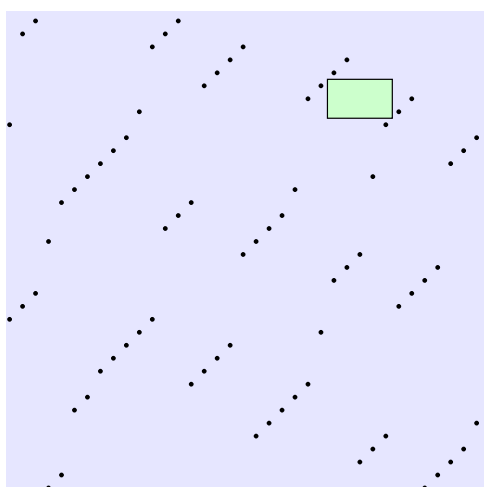

439. (24, 29, 30, 31)

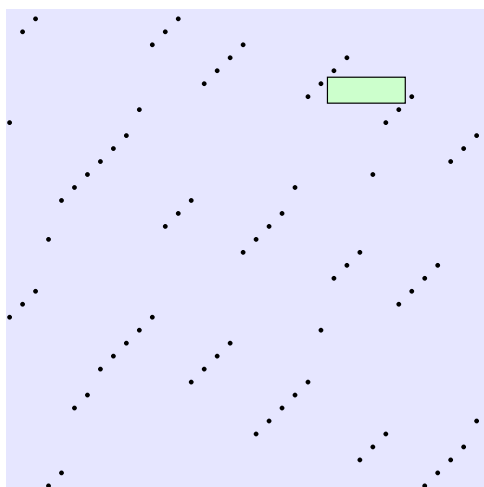

440. (24, 30, 14, 31)

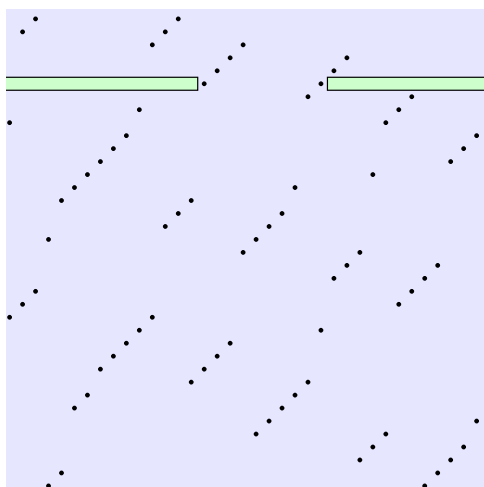

441. (24, 32, 25, 15)

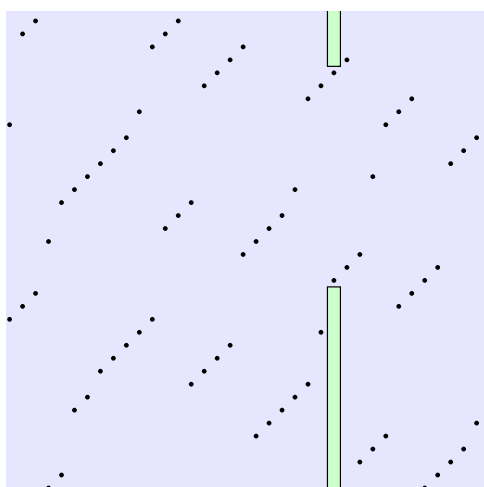

442. (24, 33, 26, 15)

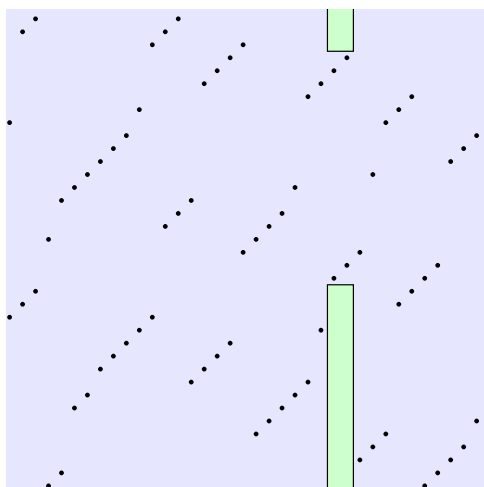

443. (25, 2, 27, 16)

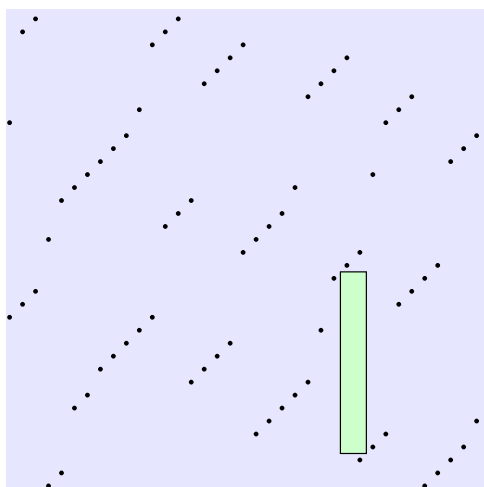

444. (25, 3, 28, 16)

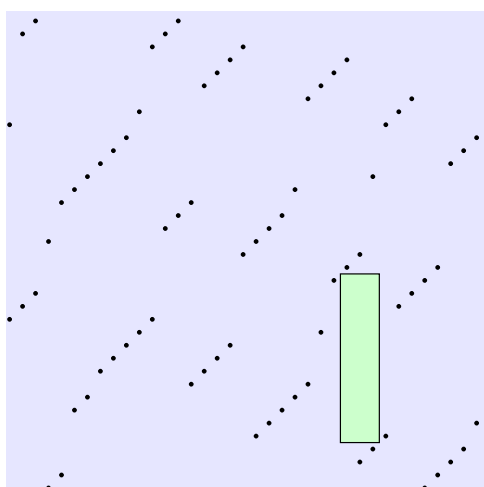

445. (25, 4, 29, 16)

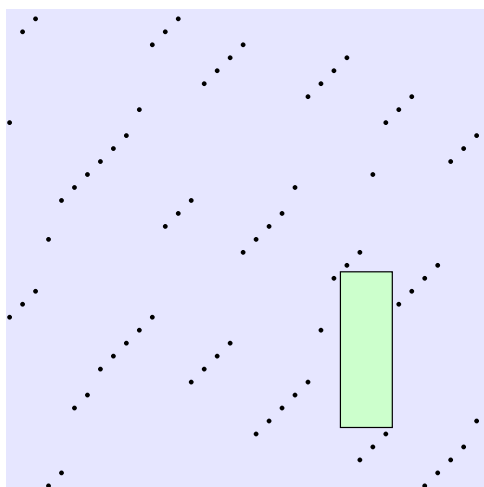

446. (25, 14, 30, 16)

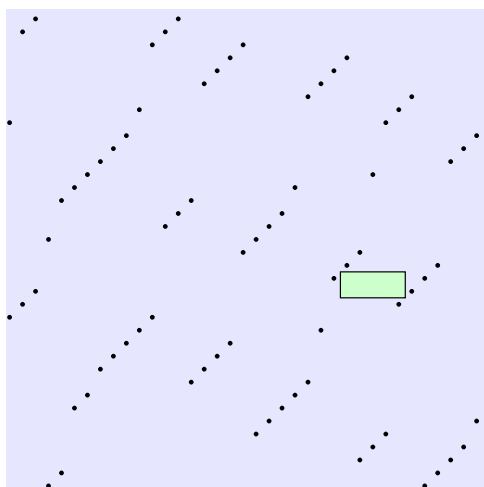

447. (25, 15, 31, 16)

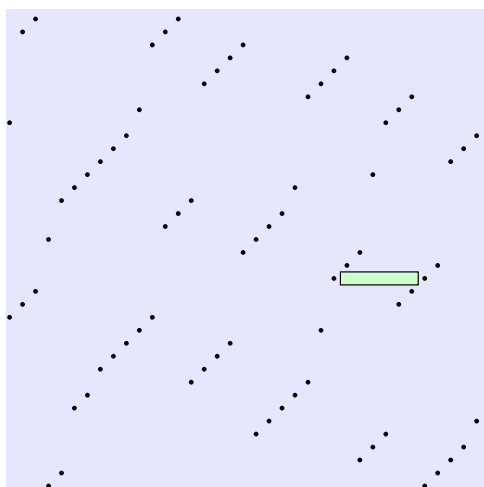

448. (25, 17, 26, 32)

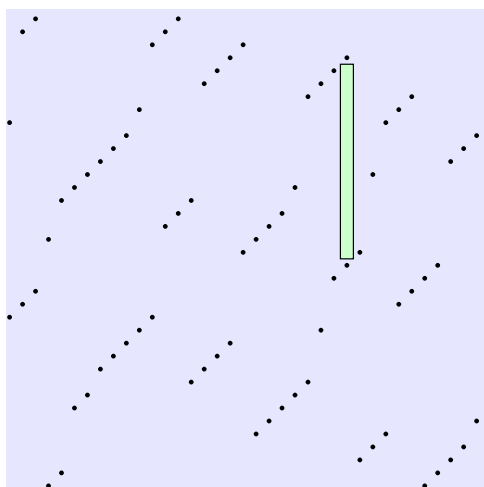

449. (25, 18, 27, 32)

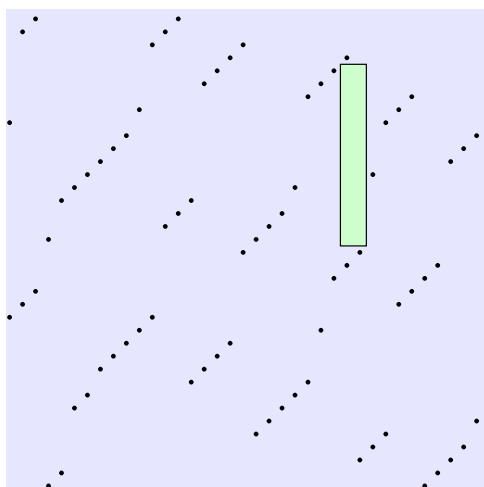

450. (25, 24, 28, 32)

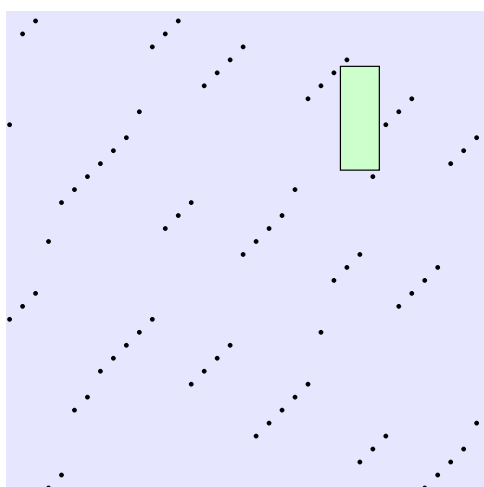

451. (25, 28, 29, 32)

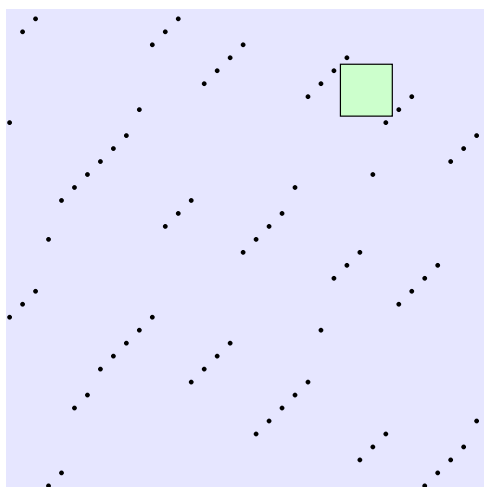

452. (25, 29, 30, 32)

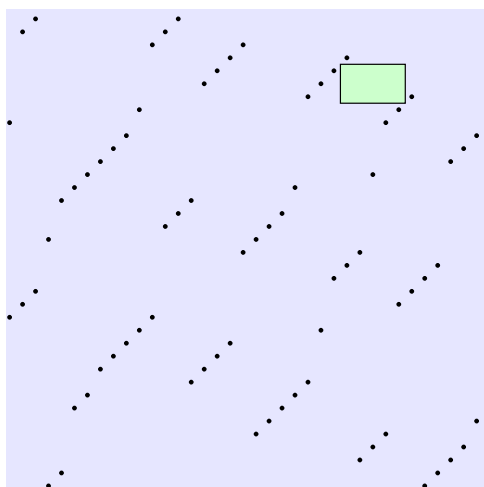

453. (25, 30, 14, 32)

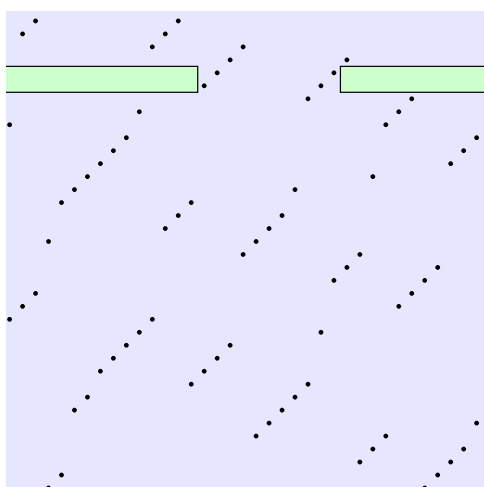

454. (25, 31, 15, 32)

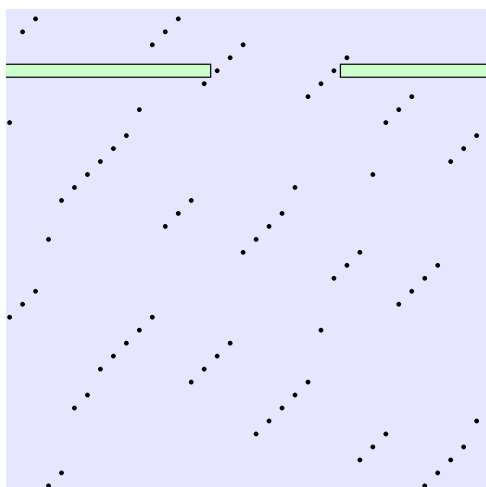

455. (25, 33, 26, 16)

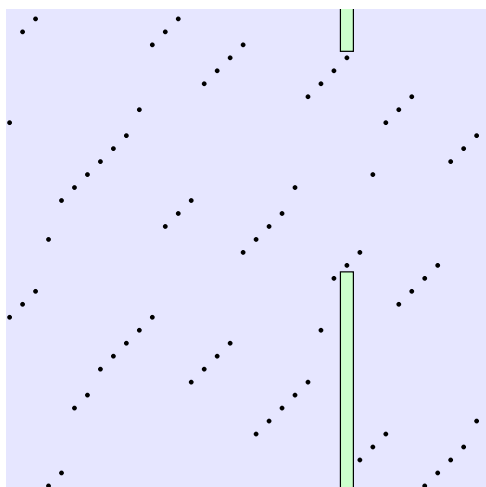

456. (26, 2, 27, 17)

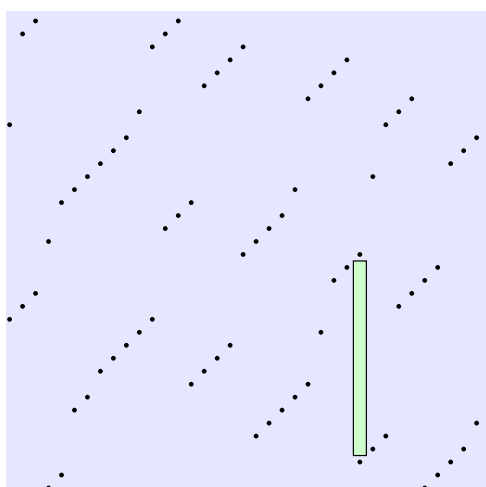



457. (26, 3, 28, 17)

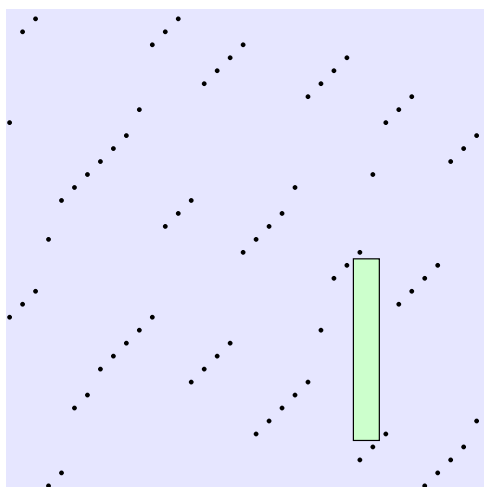

458. (26, 4, 29, 17)

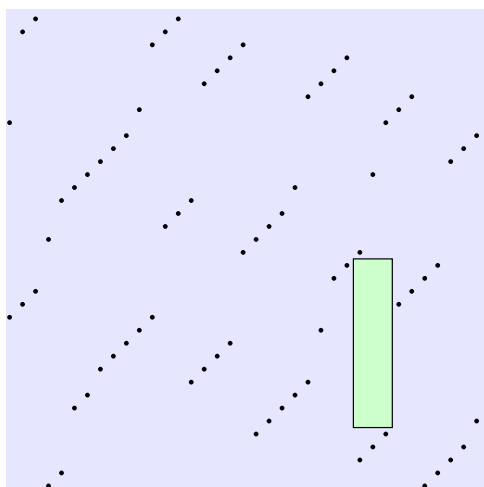

459. (26, 14, 30, 17)

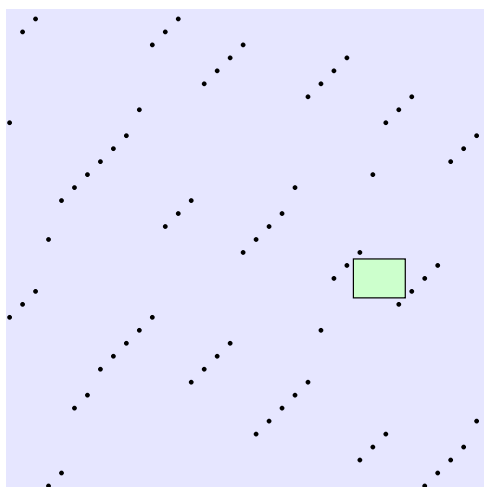

460. (26, 15, 31, 17)

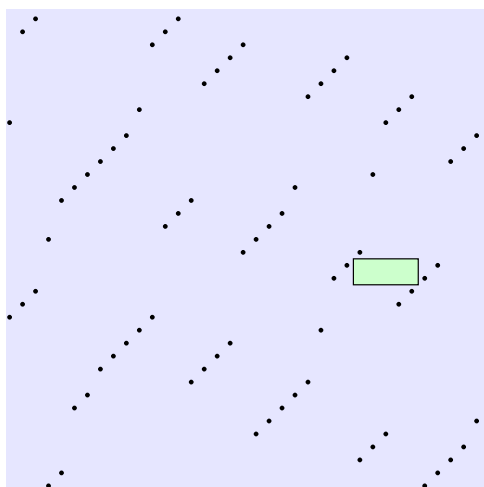

461. (26, 16, 32, 17)

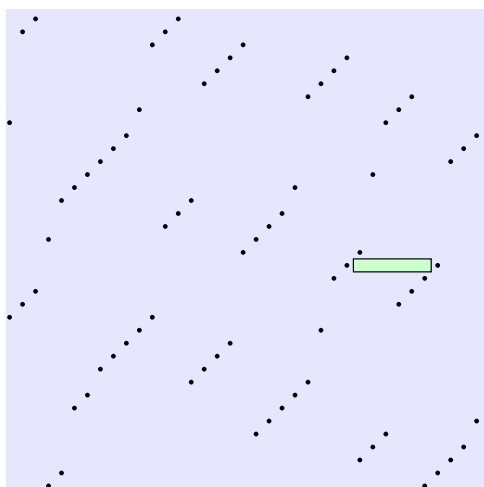

462. (26, 18, 27, 1)

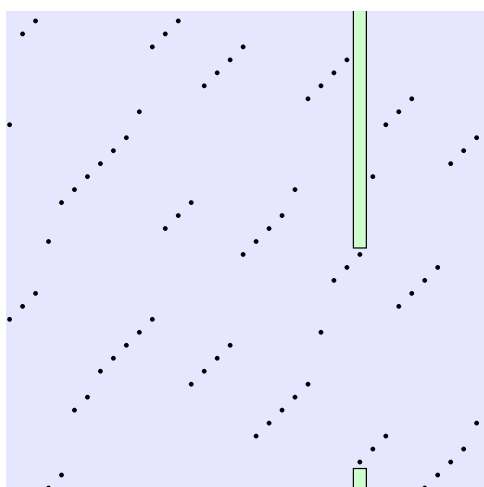

463. (26, 24, 28, 1)

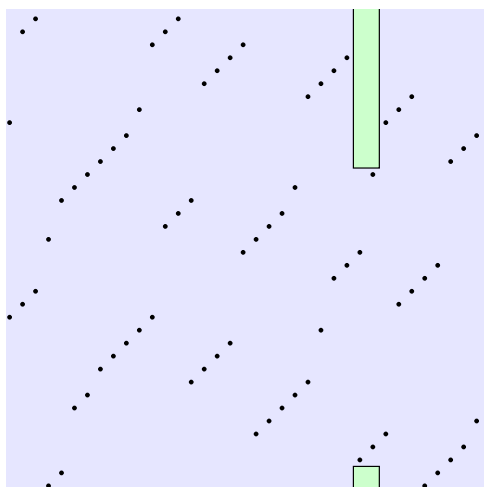

464. (26, 28, 29, 1)

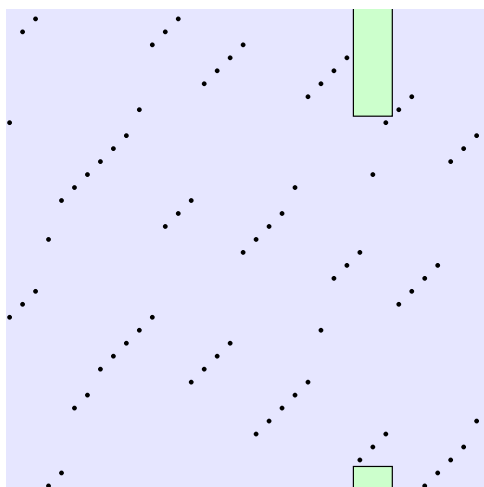

465. (26, 29, 30, 1)

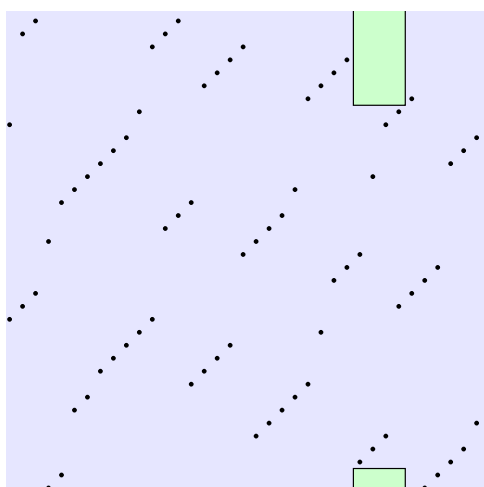

466. (26, 30, 0, 36)

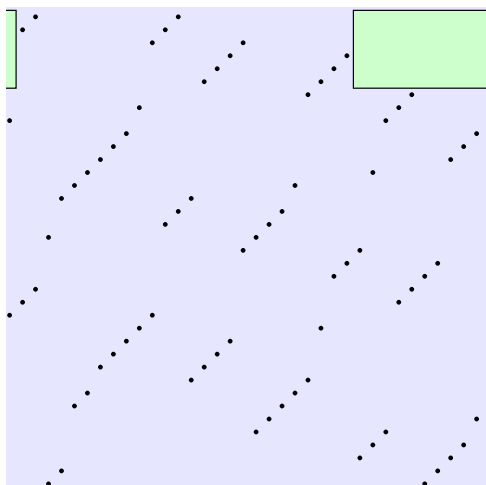

467. (26, 30, 10, 34)

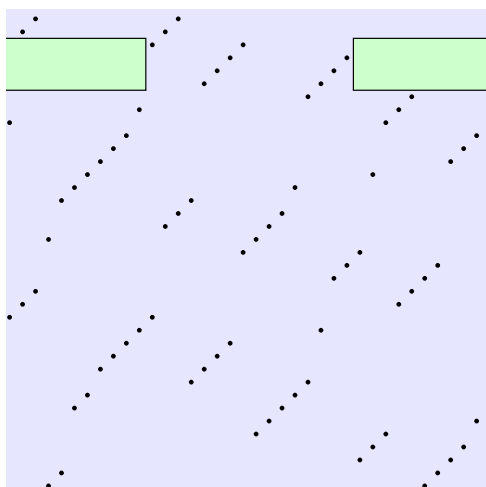

468. (26, 30, 14, 33)

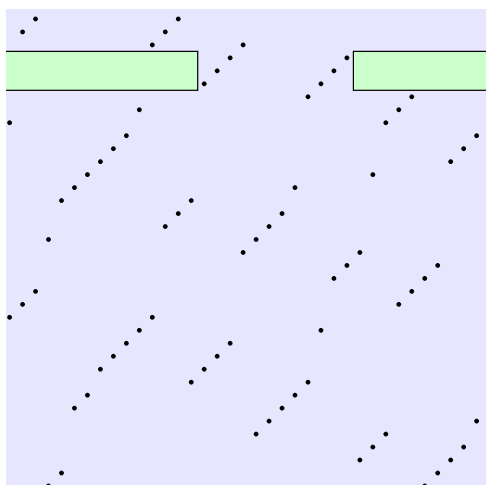

469. (26, 30, 31, 1)

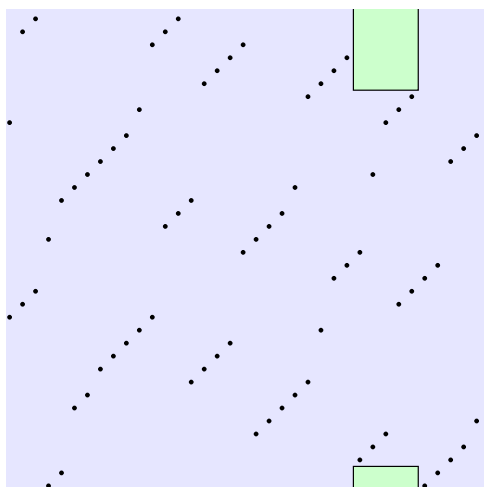

470. (26, 31, 15, 33)

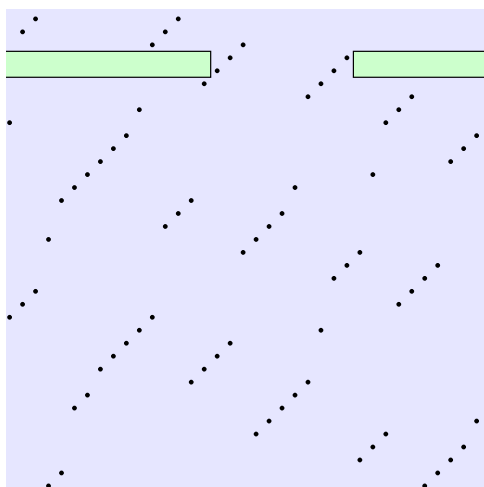

471. (26, 32, 16, 33)

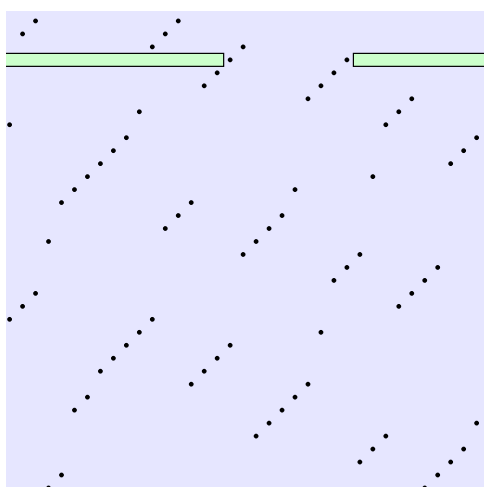

472.  $(27, 0, 32, 2)$

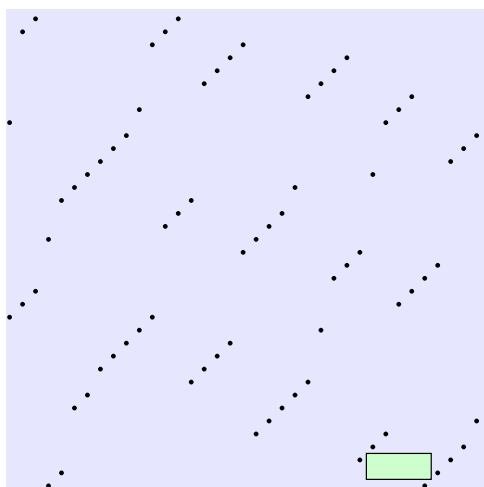

473.  $(27, 1, 33, 2)$

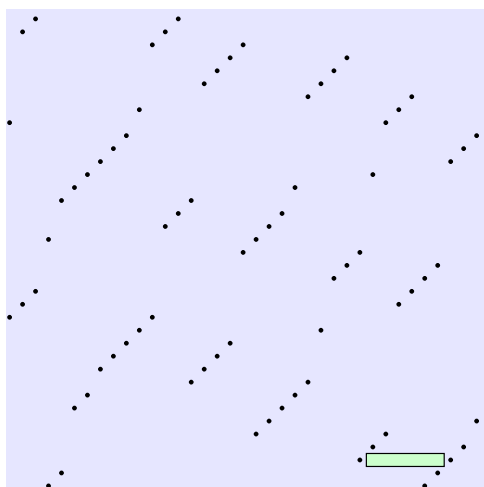

474.  $(27, 3, 28, 23)$

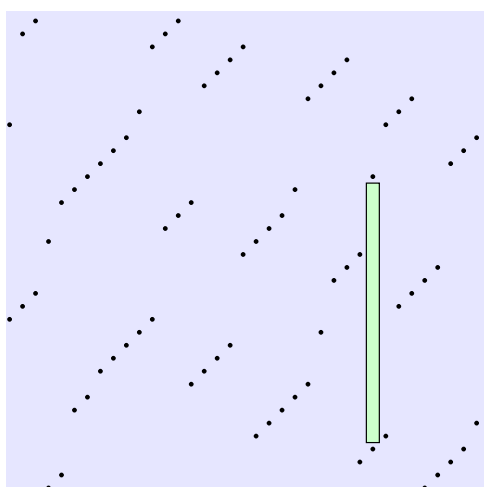

475. (27, 4, 29, 23)

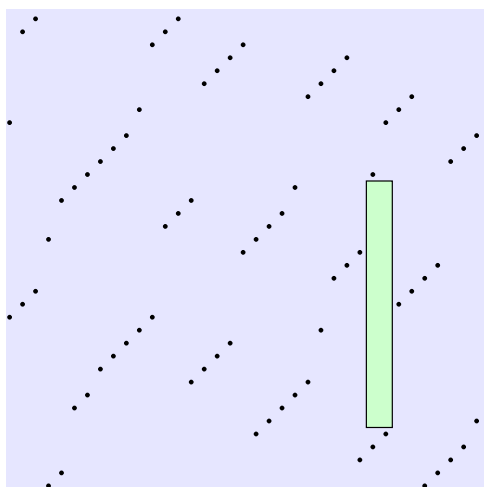

476. (27, 14, 30, 23)

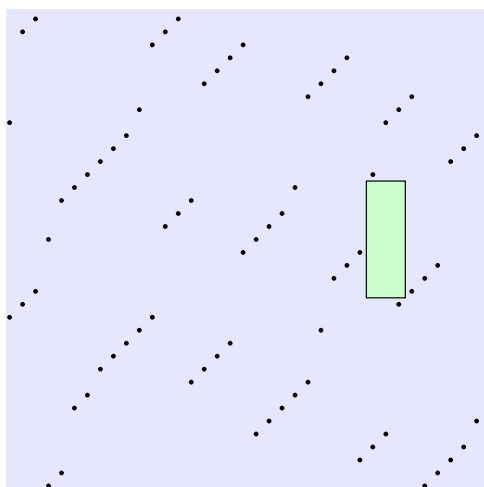

477. (27, 15, 31, 23)

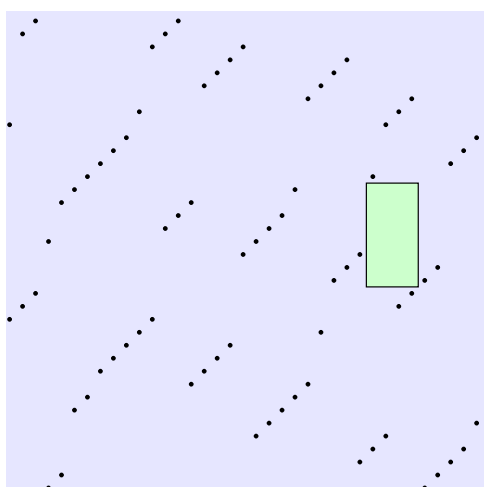

478. (27, 16, 32, 23)

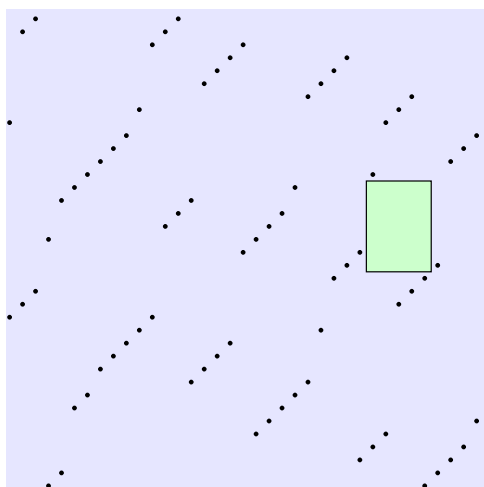

479. (27, 17, 2, 23)

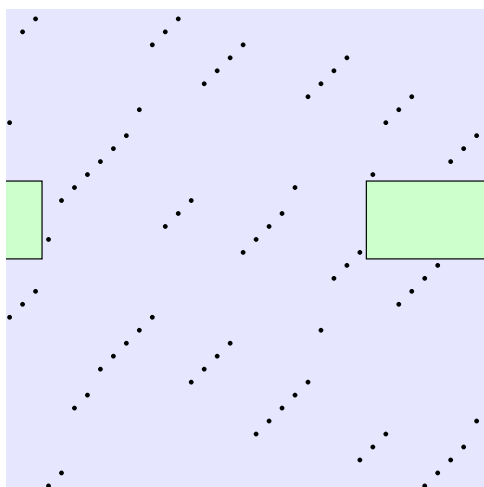

480. (27, 17, 17, 18)

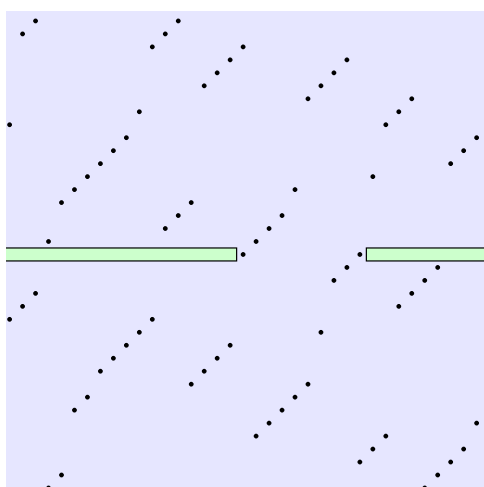



481. (27, 24, 28, 2)

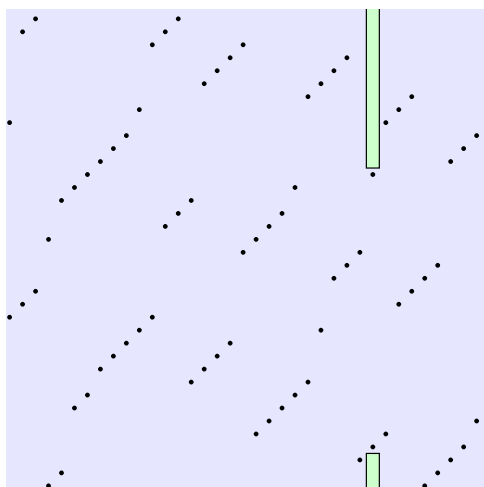

482. (27, 28, 29, 2)

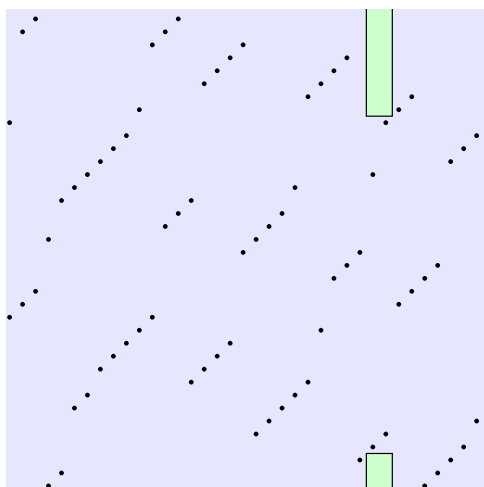

483. (27, 29, 30, 2)

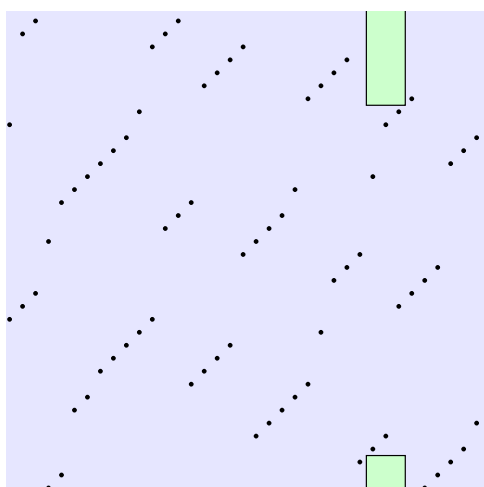

484.  $(27, 30, 31, 2)$

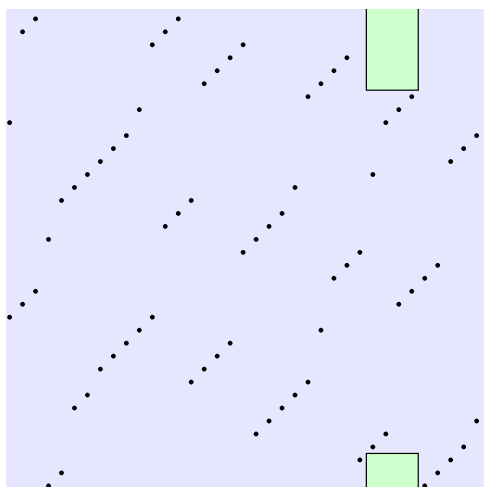

485.  $(28, 0, 32, 3)$

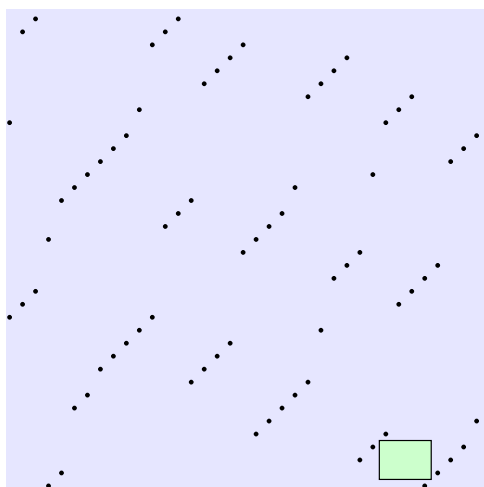

486.  $(28, 1, 33, 3)$

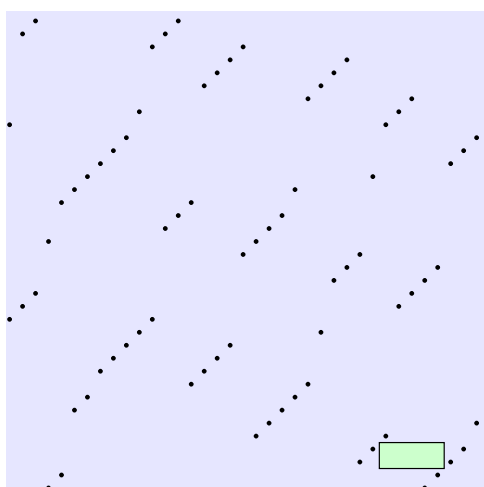

487. (28, 2, 34, 3)

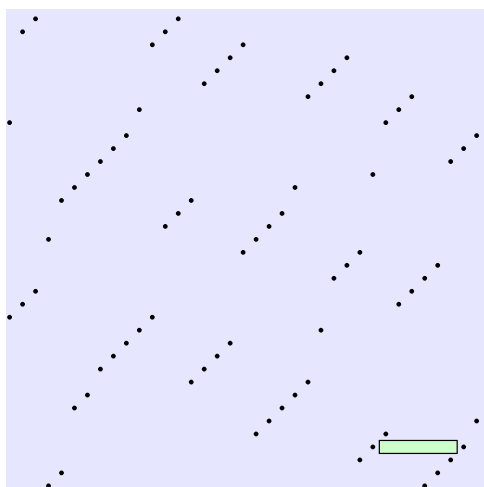

488. (28, 4, 29, 27)

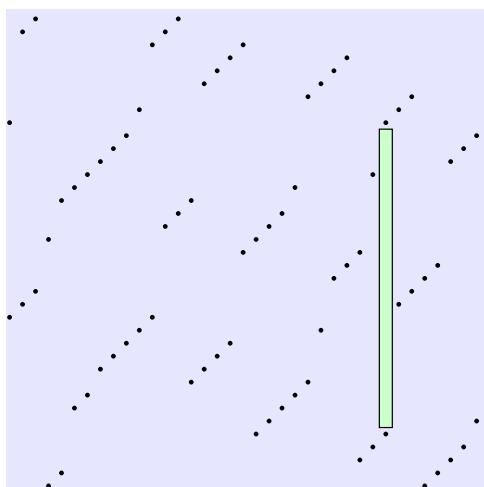

489. (28, 14, 30, 27)

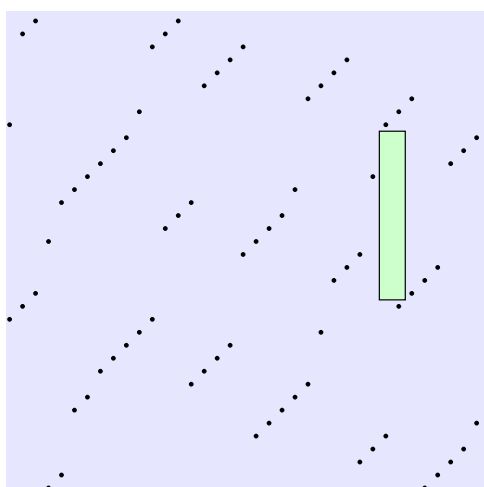

490. (28, 15, 31, 27)

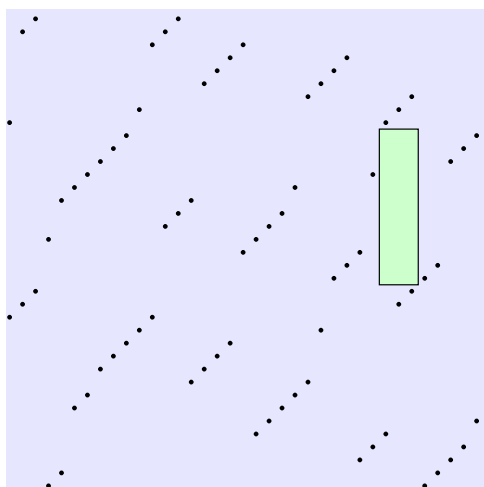

491. (28, 16, 32, 27)

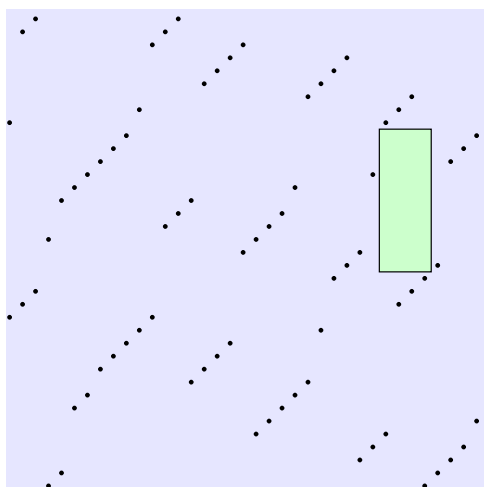

492. (28, 17, 2, 24)

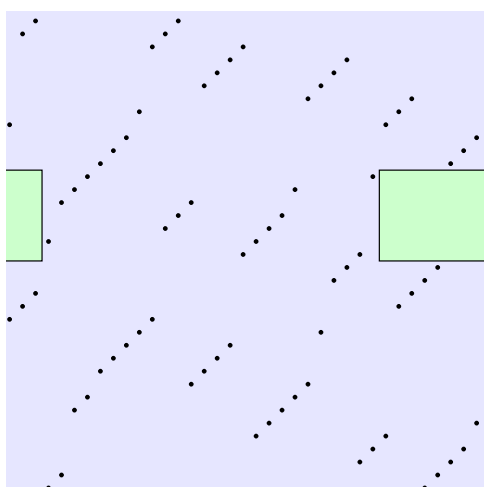

493. (28, 17, 33, 27)

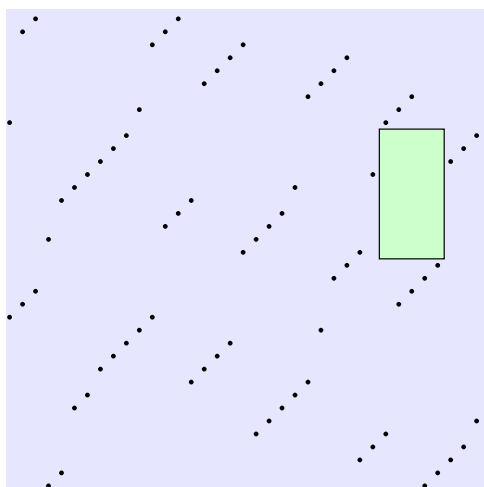

494. (28, 19, 3, 24)

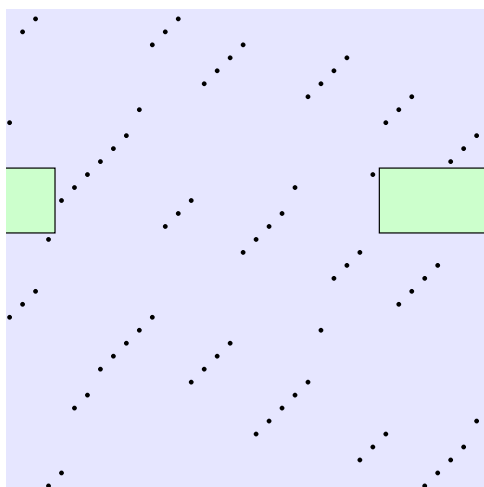

495. (28, 22, 4, 24)

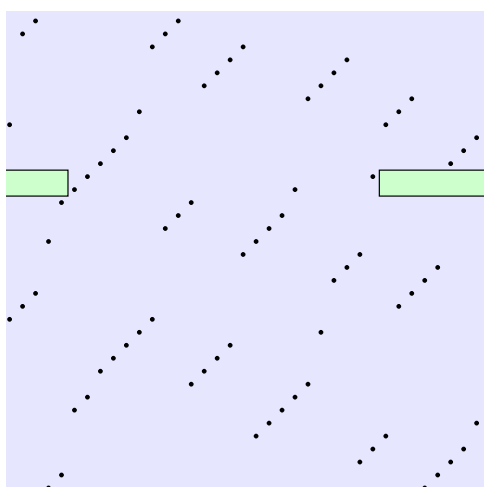

496. (28, 23, 5, 24)

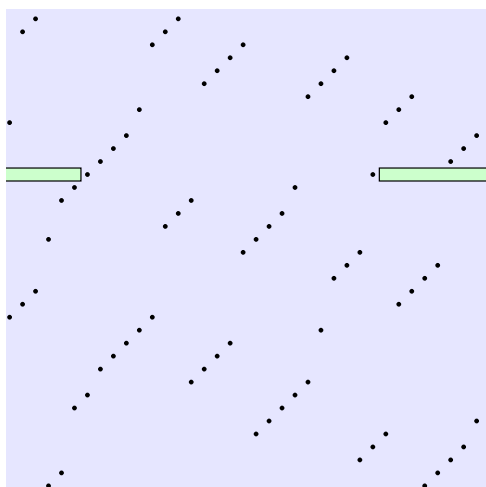

497. (28, 28, 29, 3)

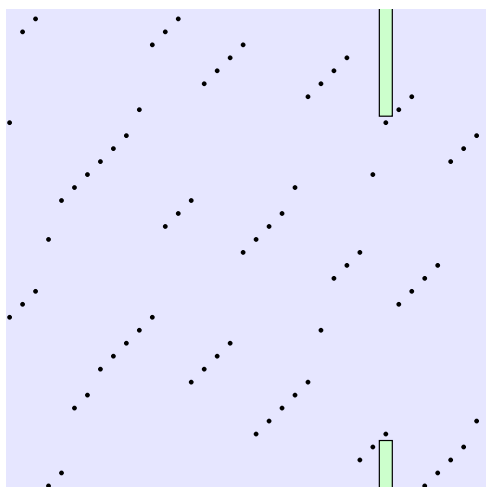

498. (28, 29, 30, 3)

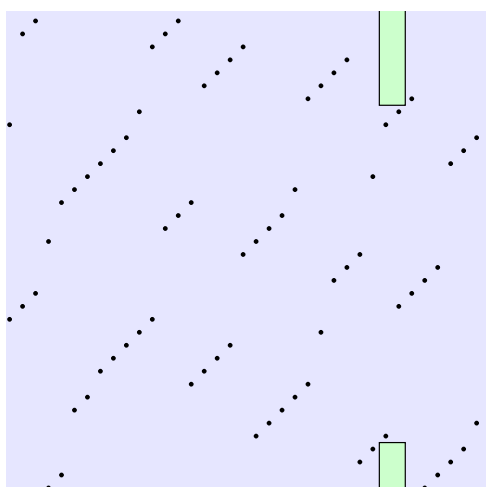

499. (28, 30, 31, 3)

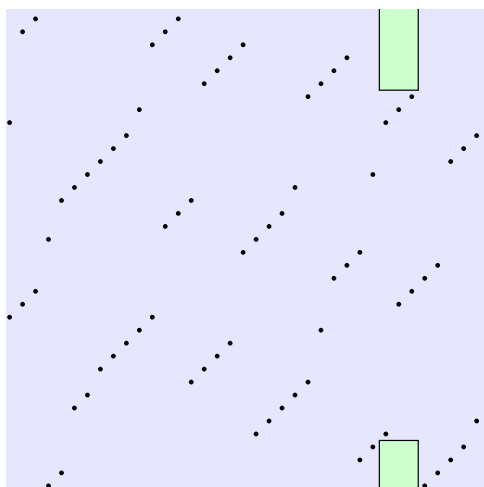

500. (29, 0, 32, 13)

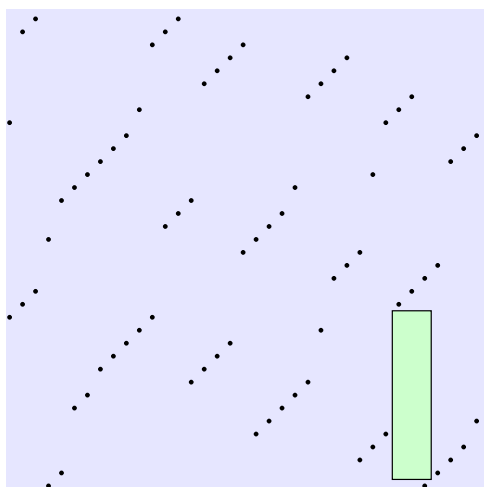

501. (29, 1, 33, 13)

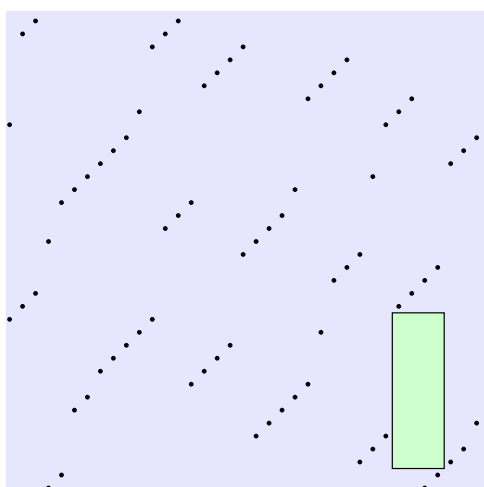

502. (29, 2, 34, 13)

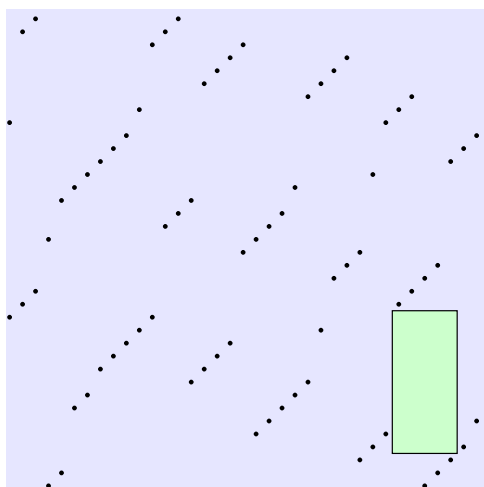

503. (29, 3, 18, 4)

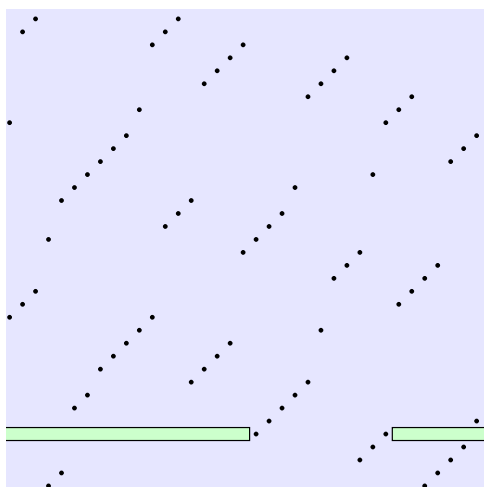

504. (29, 3, 35, 13)

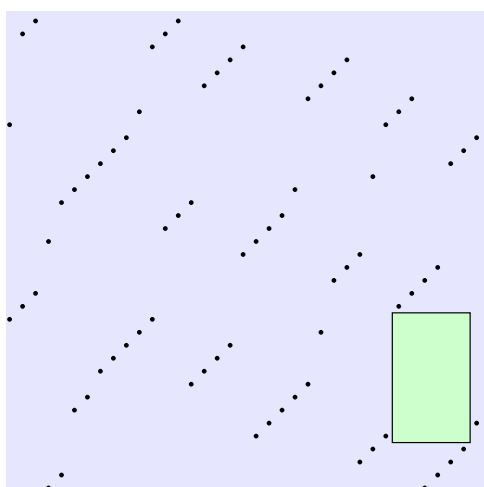



505. (29, 14, 30, 28)

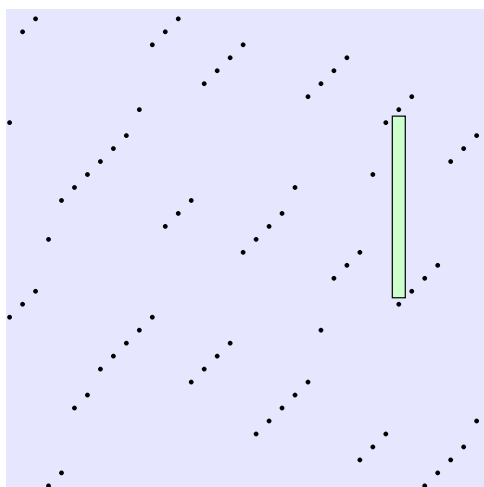

506. (29, 15, 31, 28)

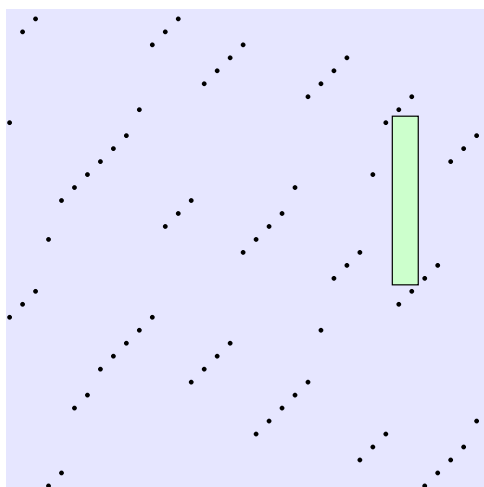

507. (29, 16, 32, 28)

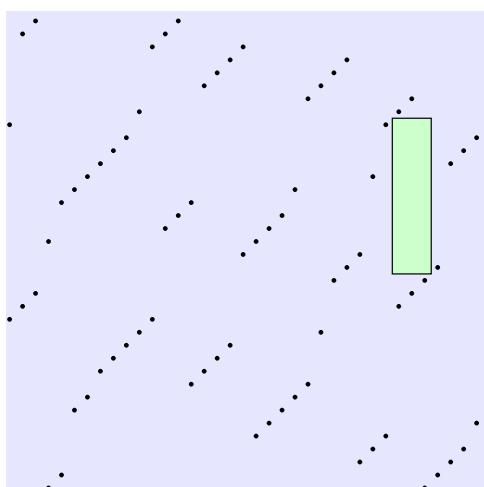

508. (29, 17, 33, 28)

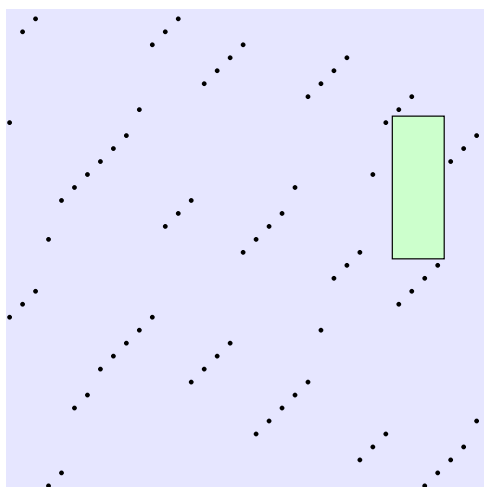

509. (29, 25, 34, 28)

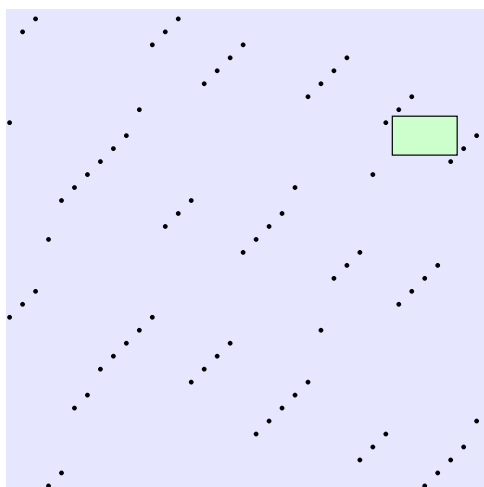

510. (29, 26, 35, 28)

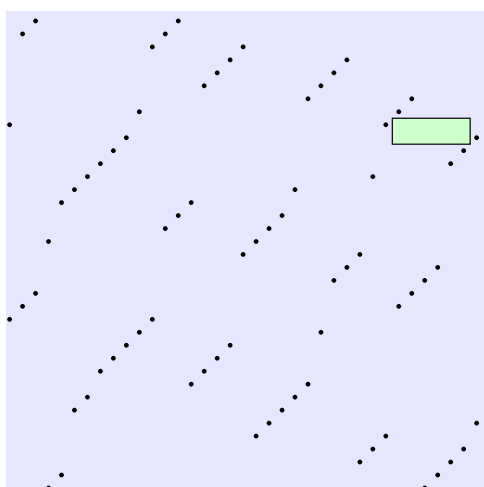

511. (29, 27, 36, 28)

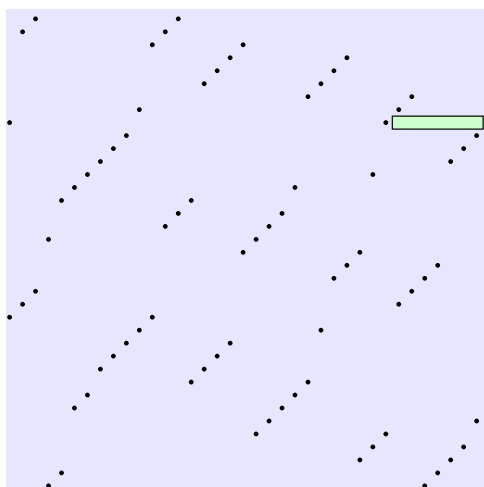

512. (29, 29, 30, 13)

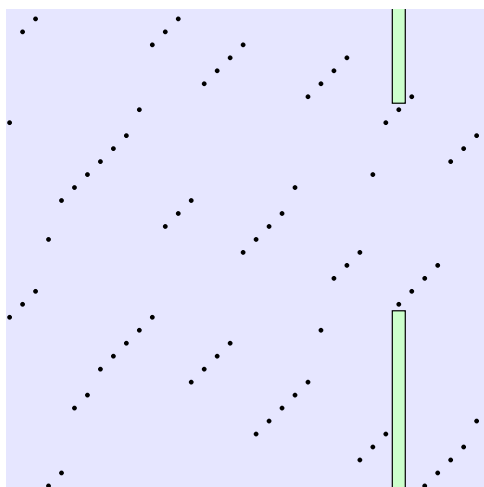

513. (29, 30, 31, 13)

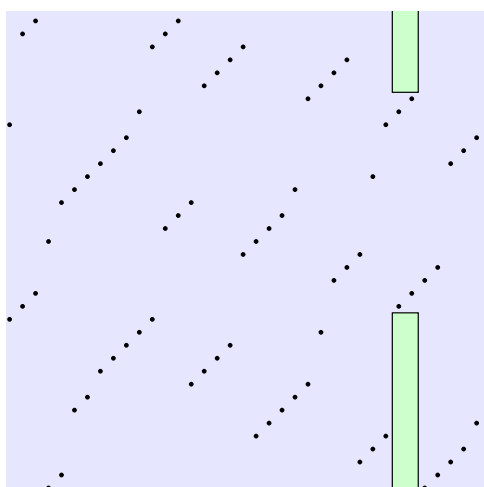

514. (30, 0, 32, 14)

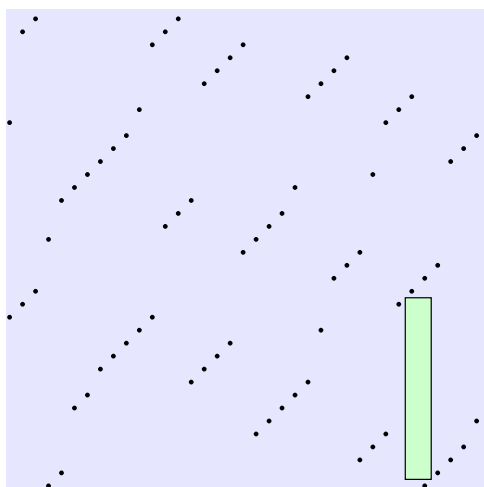

515. (30, 1, 33, 14)

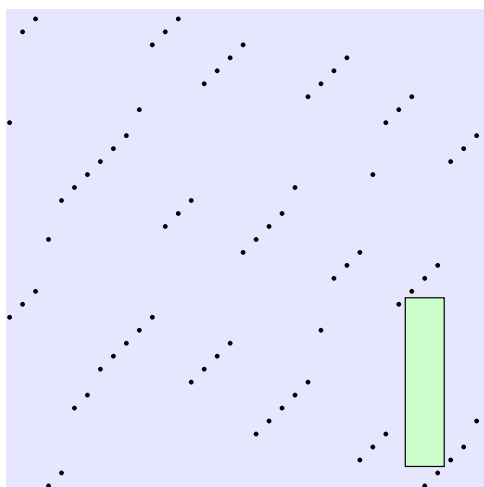

516. (30, 2, 34, 14)

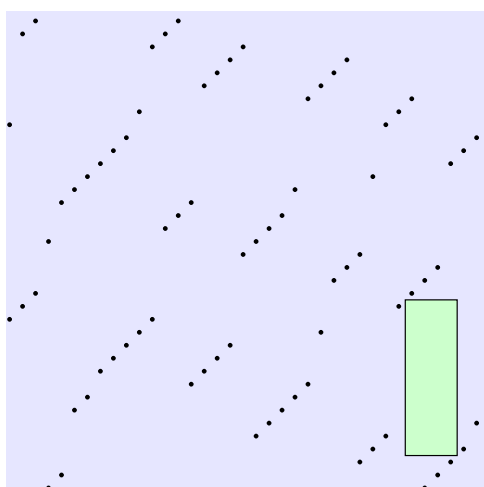

517.  $(30, 3, 35, 14)$

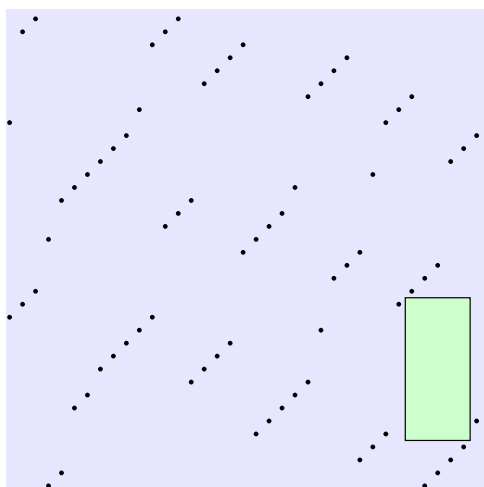

518.  $(30, 5, 36, 14)$

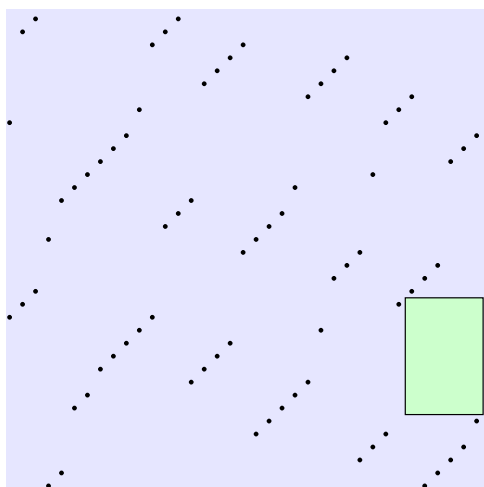

519.  $(30, 13, 0, 14)$

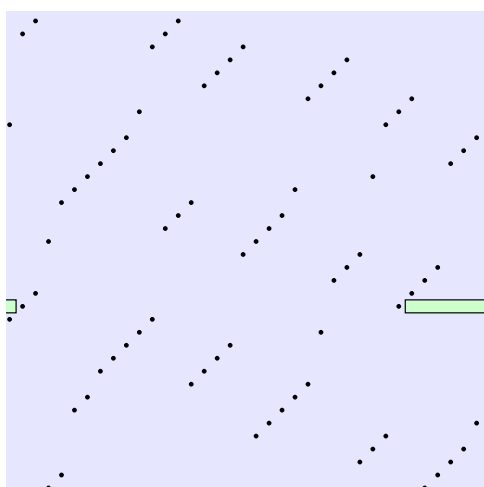

520. (30, 15, 31, 29)

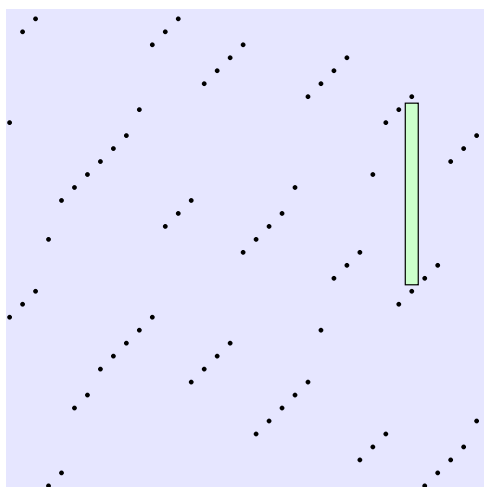

521. (30, 16, 32, 29)

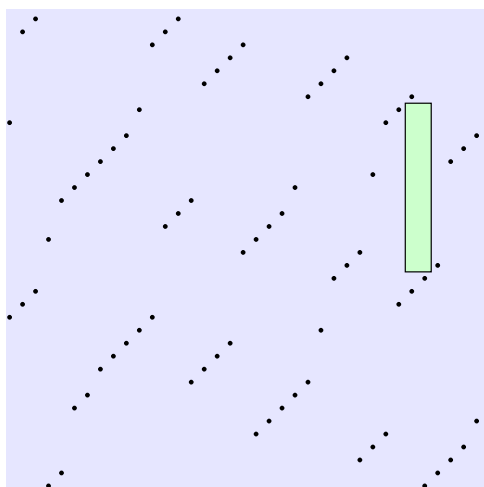

522. (30, 17, 33, 29)

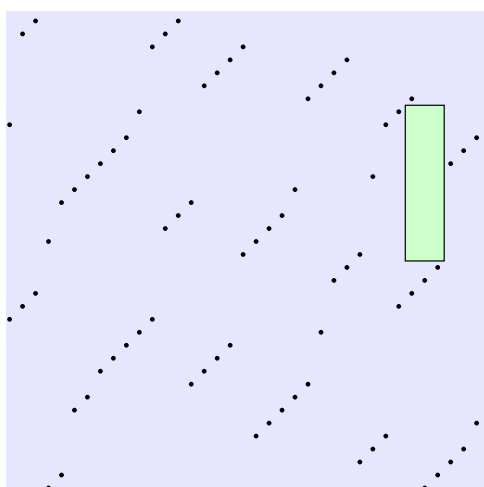

523. (30, 25, 34, 29)

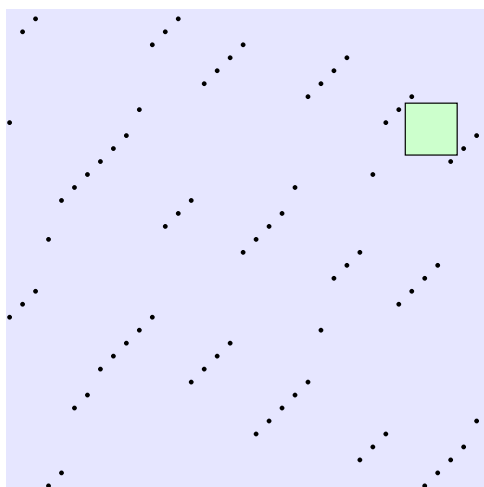

524. (30, 26, 35, 29)

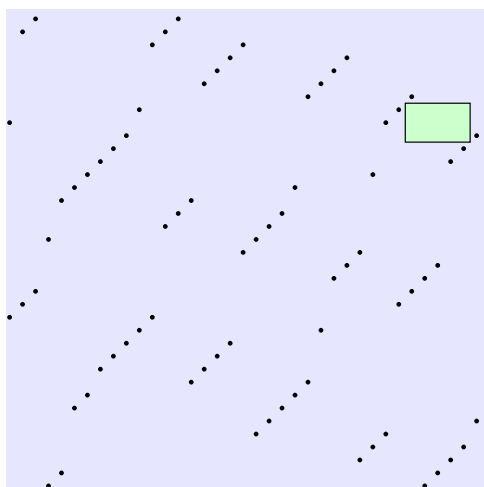

525. (30, 27, 36, 29)

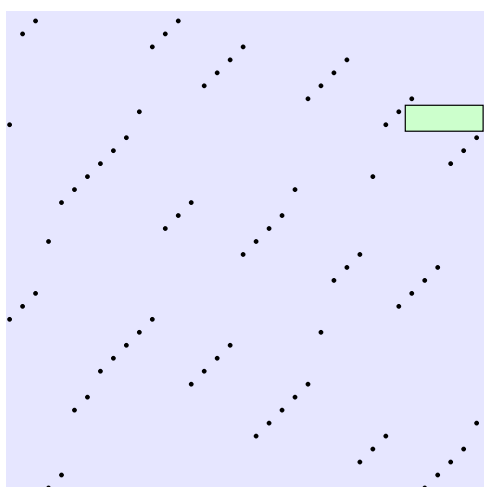

526. (30, 28, 9, 29)

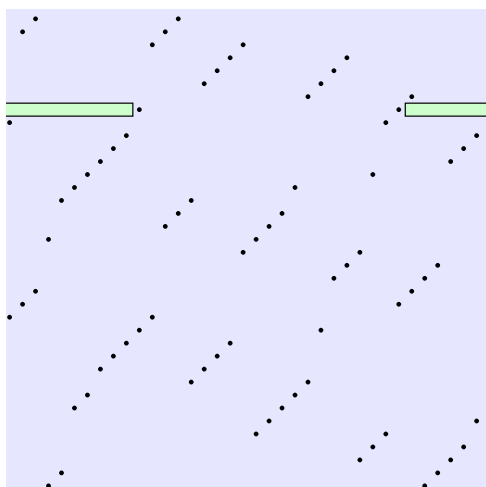

527. (30, 30, 31, 14)

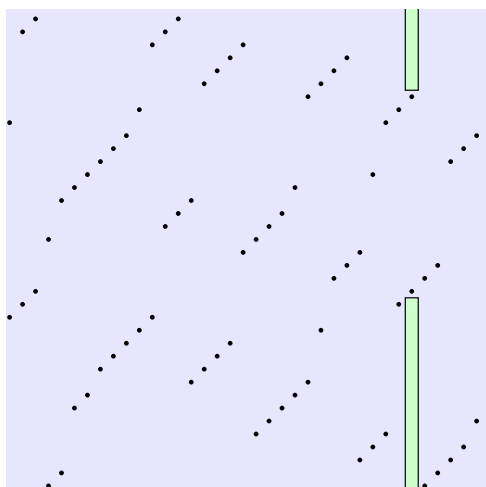

528. (31, 0, 32, 15)

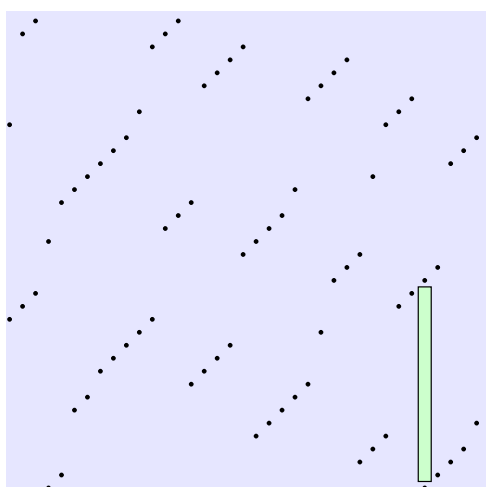



529. (31, 1, 33, 15)

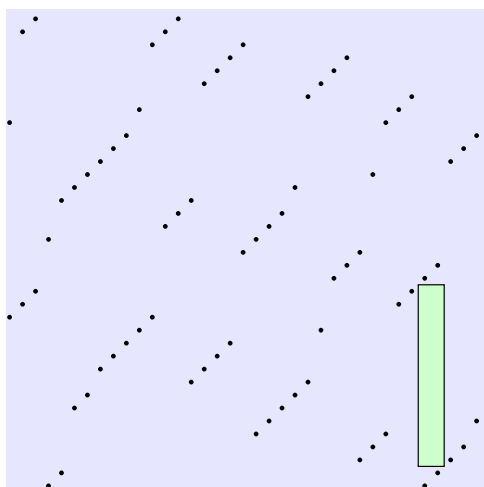

530. (31, 2, 34, 15)

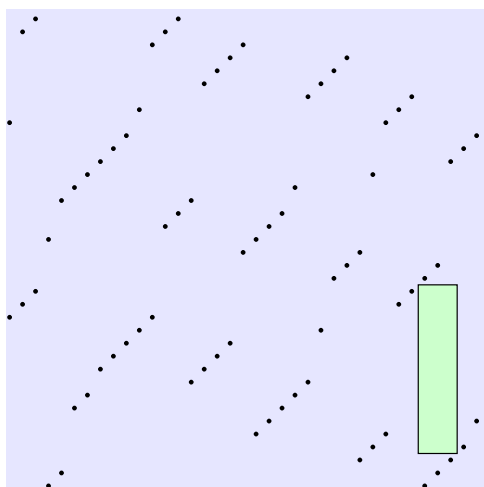

531. (31, 3, 35, 15)

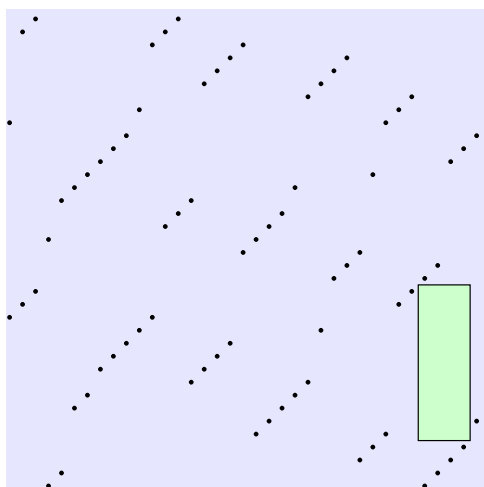

532. (31, 5, 36, 15)

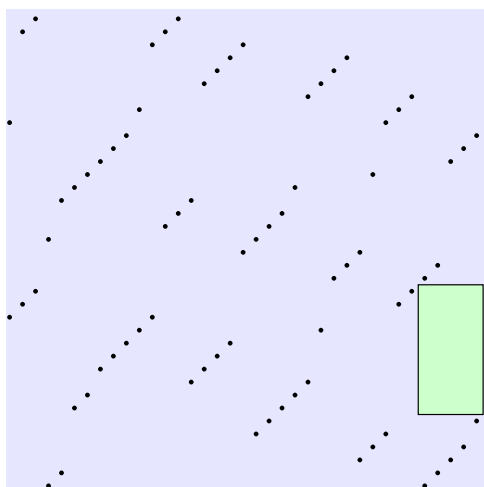

533. (31, 13, 0, 15)

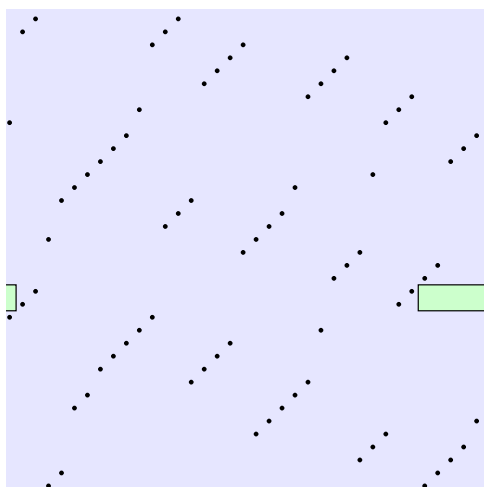

534. (31, 14, 1, 15)

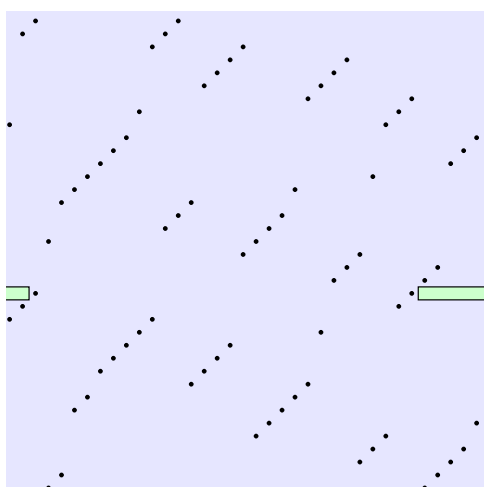

535. (31, 16, 32, 36)

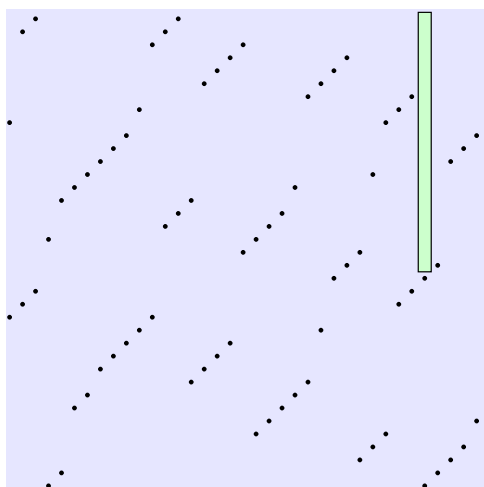

536. (31, 17, 33, 36)

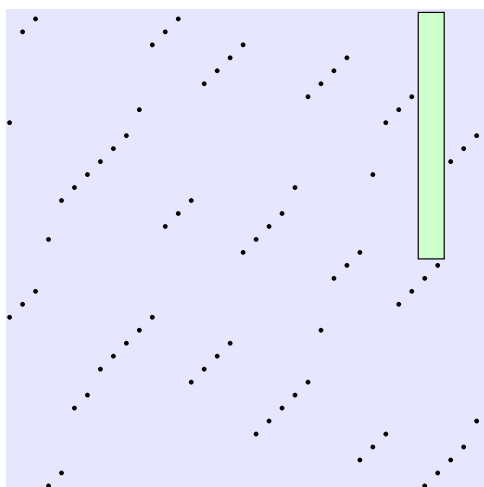

537. (31, 25, 34, 36)

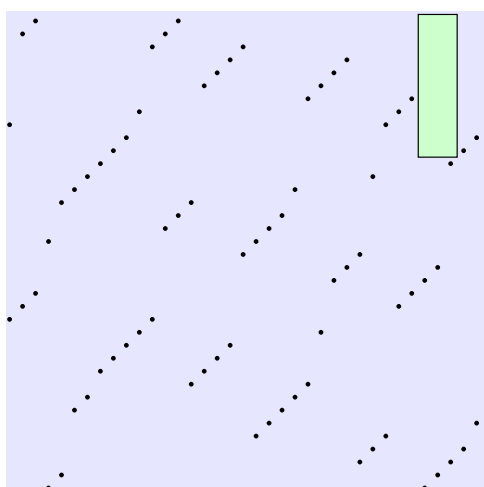

538. (31, 26, 35, 36)

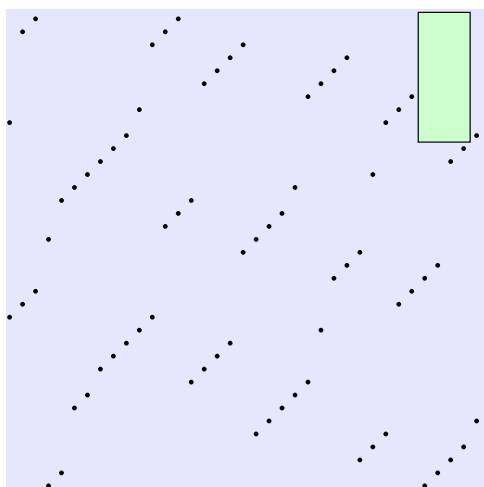

539. (31, 27, 36, 36)

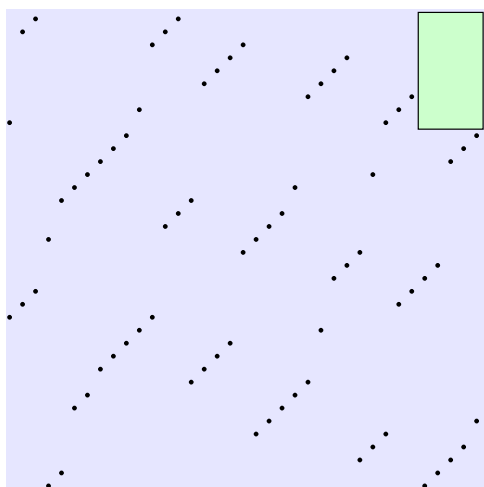

540. (31, 28, 0, 36)

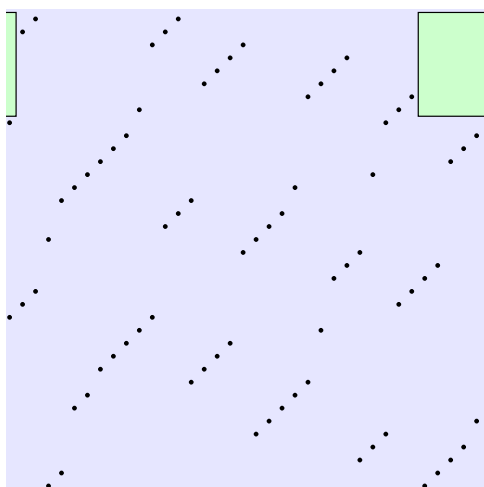

541. (31, 28, 9, 34)

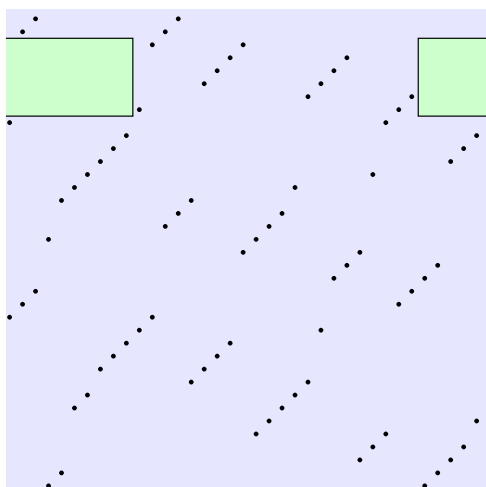

542. (31, 29, 10, 34)

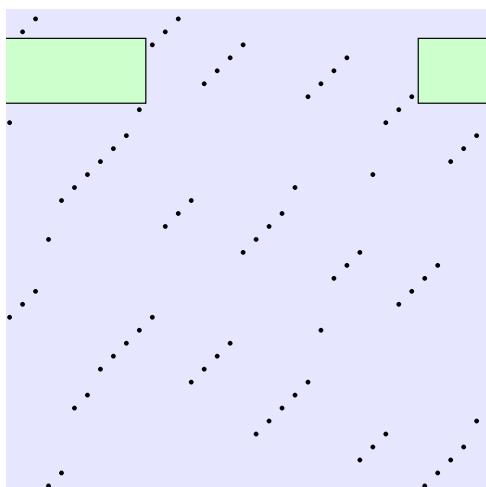

543. (31, 29, 14, 33)

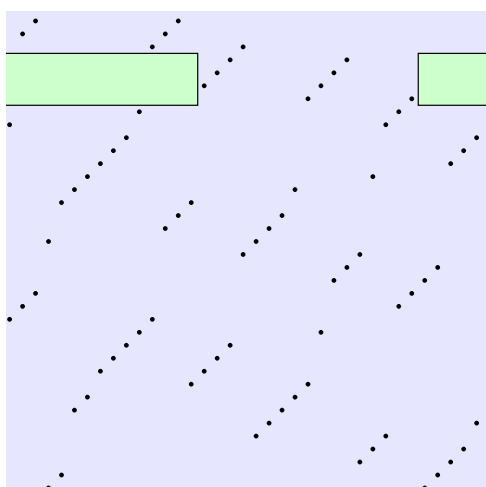

544. (31, 29, 22, 30)

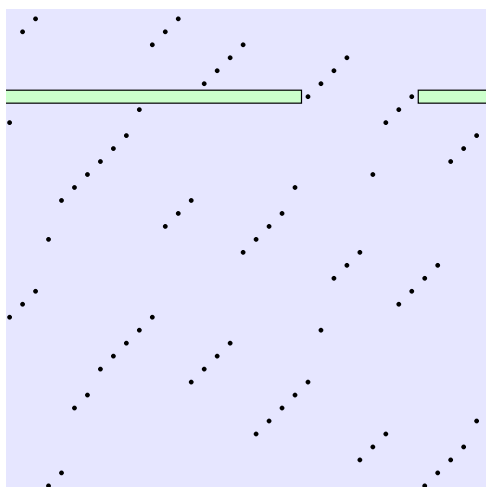

545. (32, 1, 33, 16)

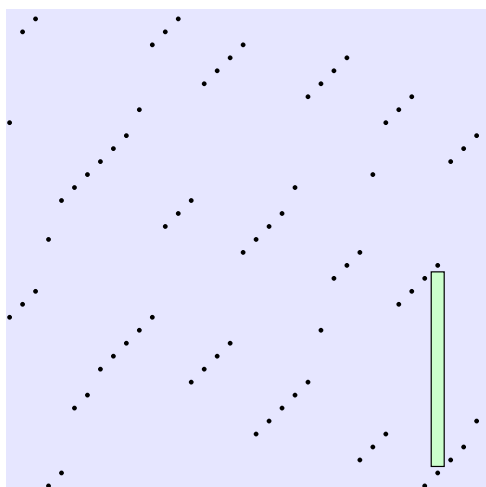

546. (32, 2, 34, 16)

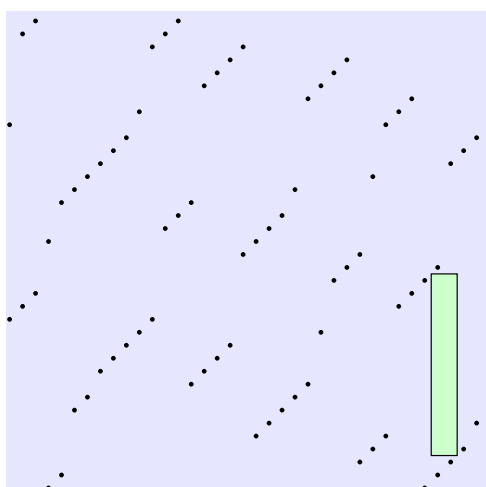

547. (32, 3, 35, 16)

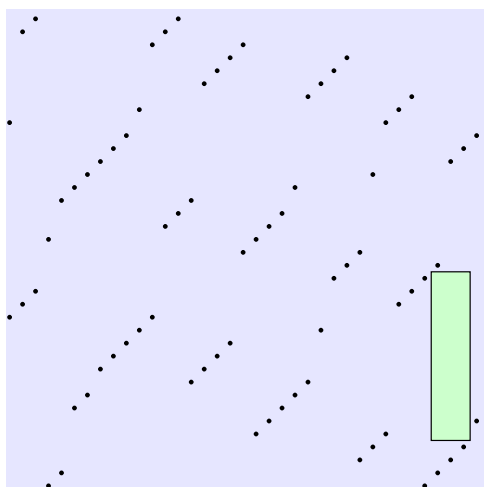

548. (32, 5, 36, 16)

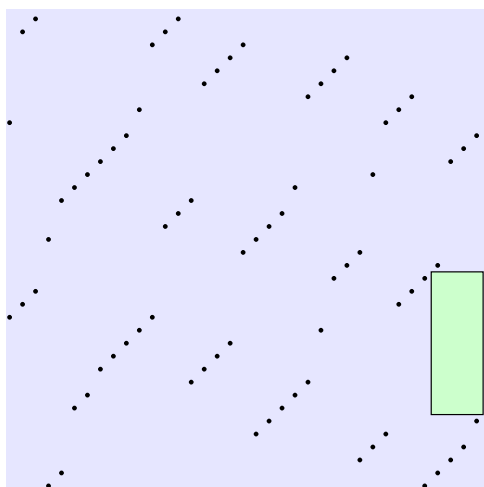

549. (32, 13, 0, 16)

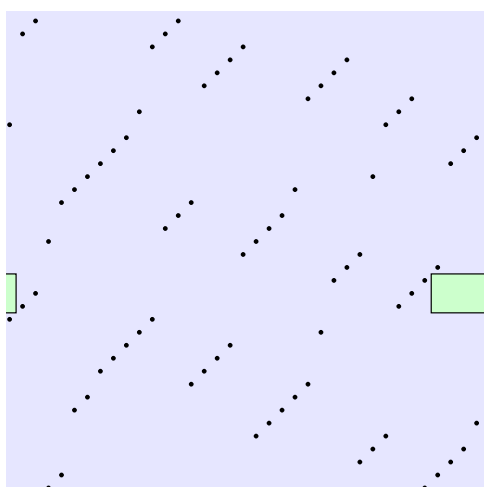

550. (32, 14, 1, 16)

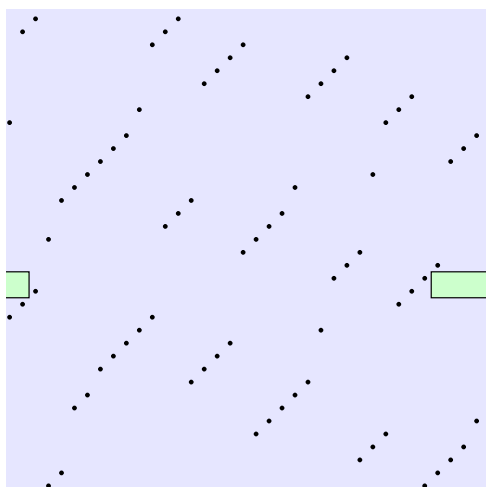

551. (32, 15, 24, 16)

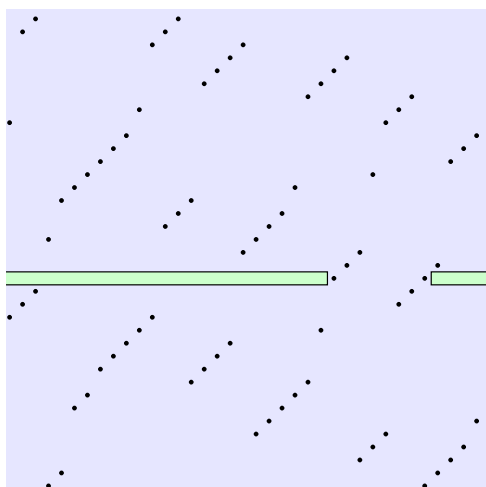

552. (32, 17, 33, 0)

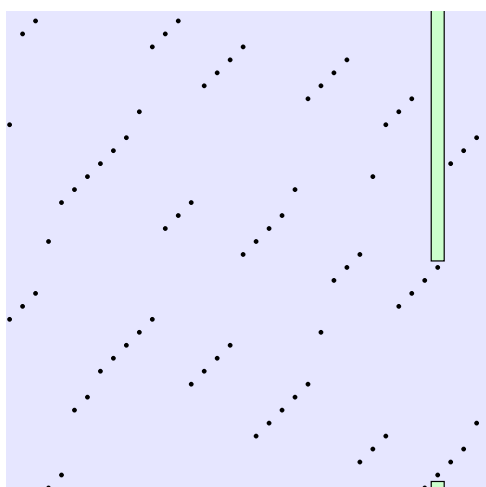



553. (32, 25, 34, 0)

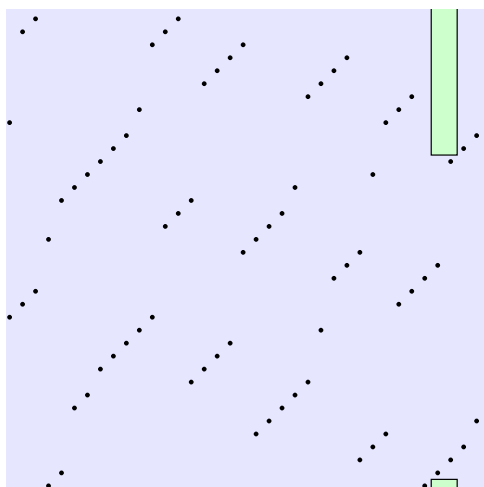

554. (32, 26, 35, 0)

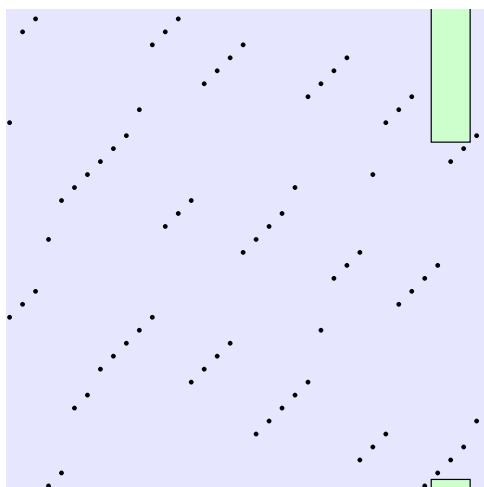

555. (32, 27, 36, 0)

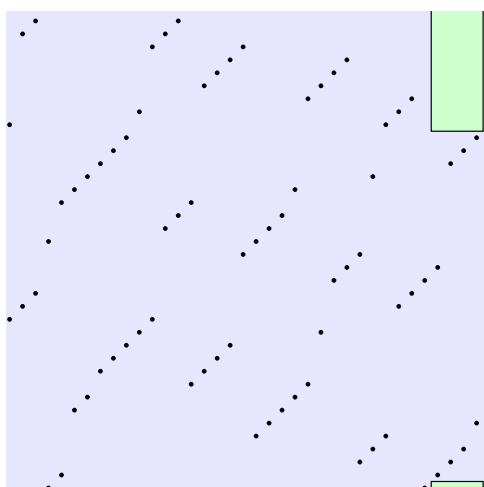

556.  $(32, 28, 0, 0)$

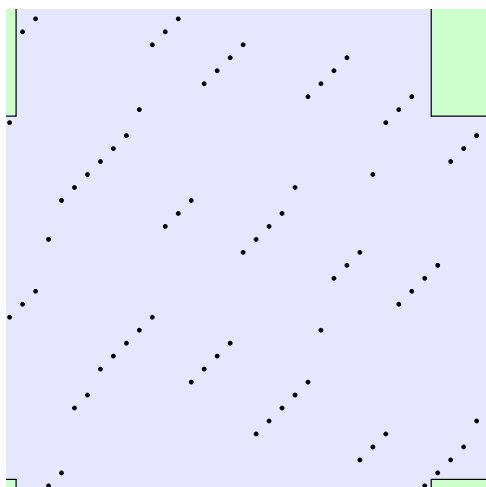

557.  $(32, 35, 1, 0)$

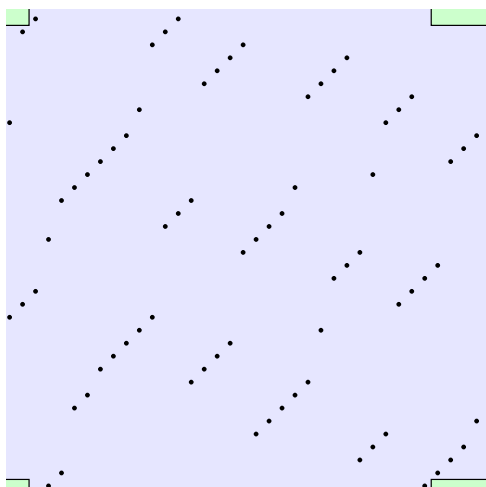

558.  $(32, 36, 2, 0)$

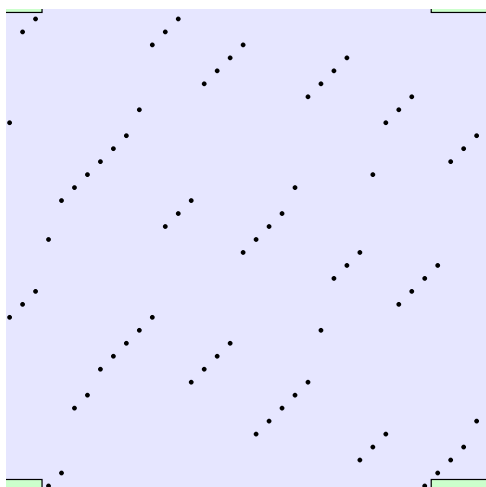

559.  $(33, 0, 3, 1)$

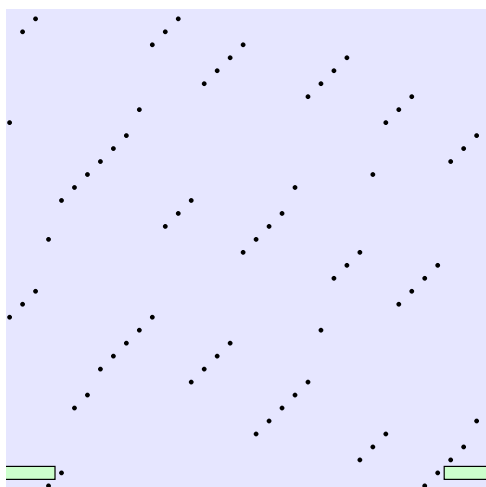

560.  $(33, 2, 34, 24)$

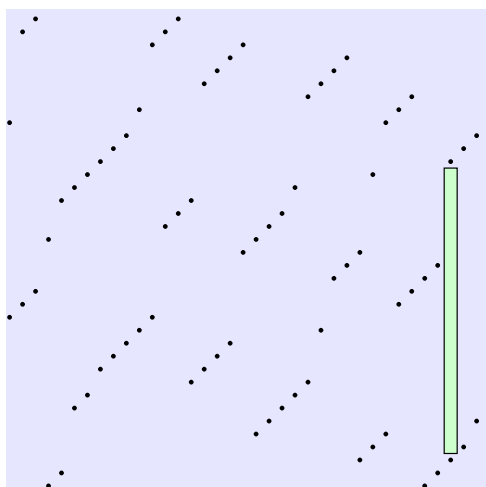

561.  $(33, 3, 35, 24)$

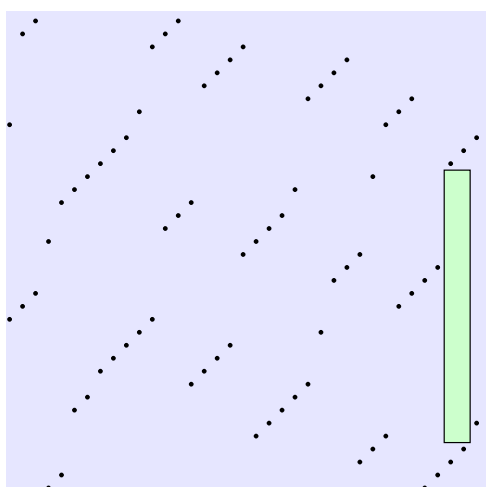

562.  $(33, 5, 36, 24)$

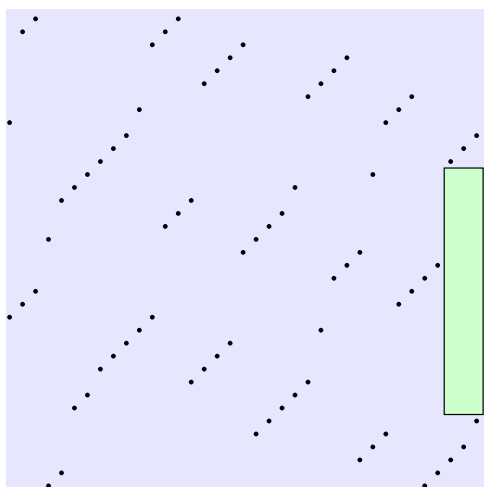

563.  $(33, 13, 0, 24)$

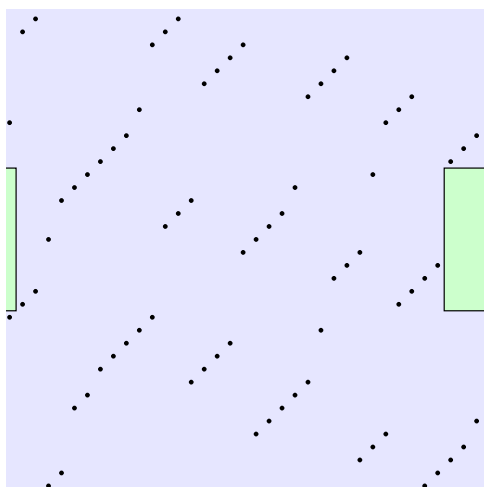

564.  $(33, 14, 1, 24)$

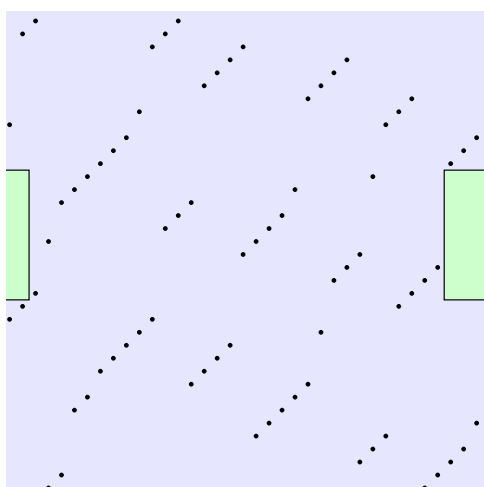

565. (33, 15, 2, 24)

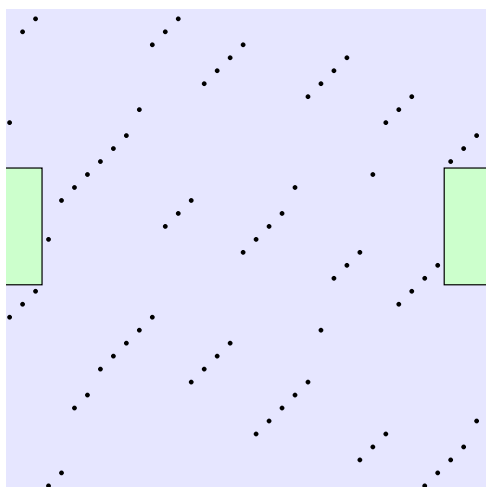

566. (33, 15, 17, 18)

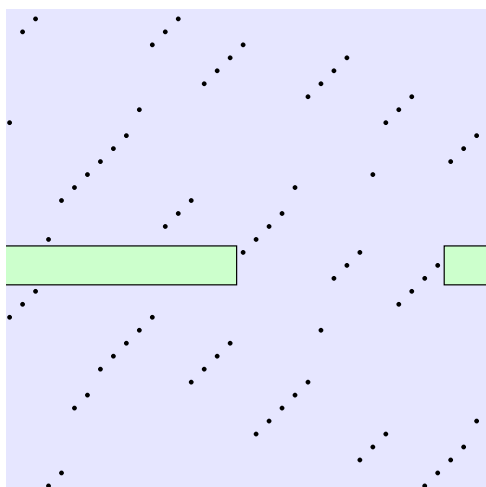

567. (33, 15, 24, 17)

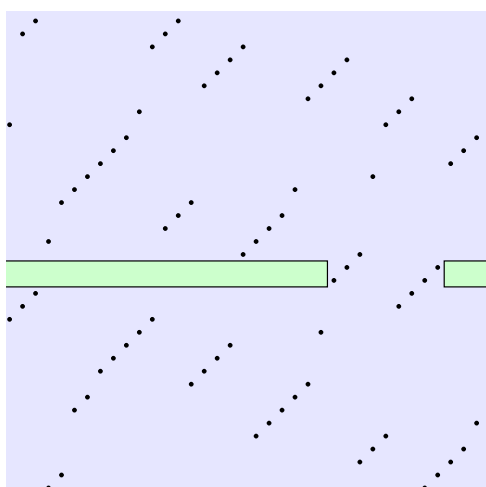

568. (33, 16, 25, 17)

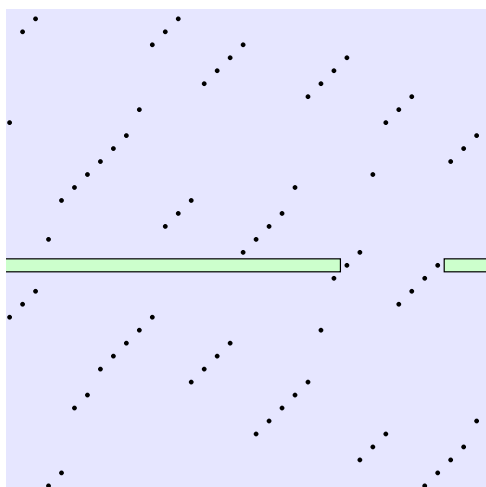

569. (33, 25, 34, 1)

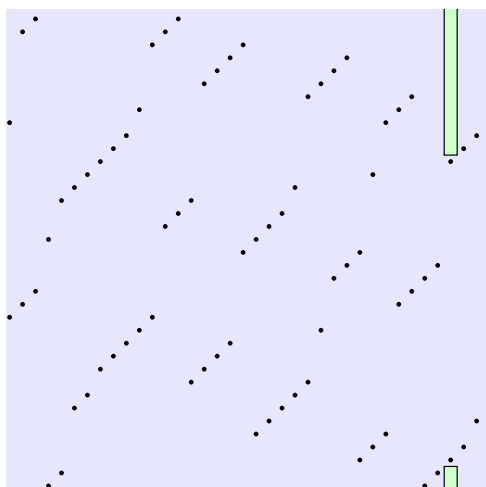

570. (33, 26, 35, 1)

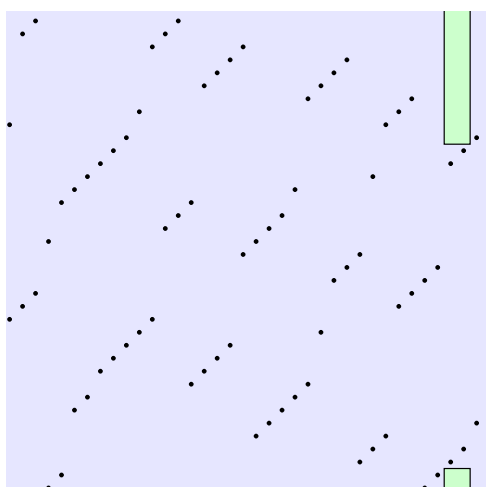

571.  $(33, 27, 36, 1)$

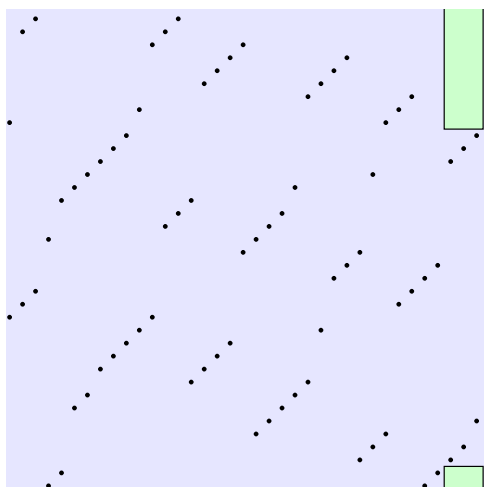

572.  $(33, 28, 0, 1)$

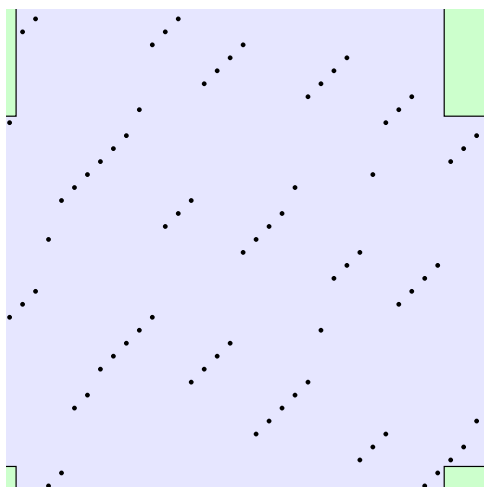

573.  $(33, 35, 1, 1)$

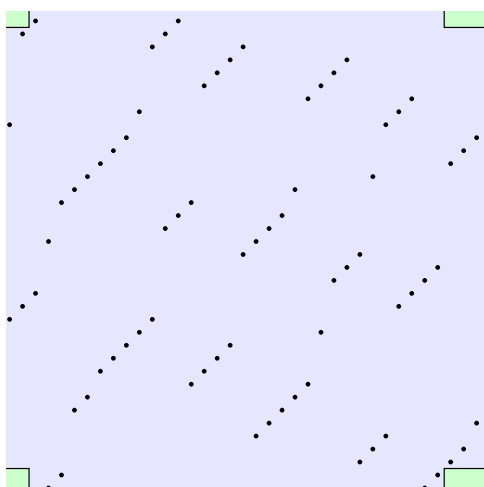

574.  $(33, 36, 2, 1)$

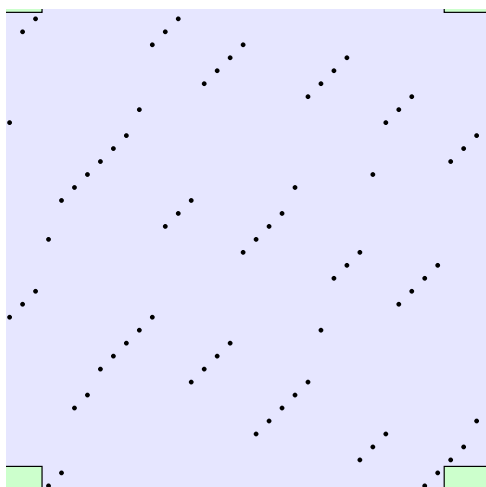

575.  $(34, 0, 3, 2)$

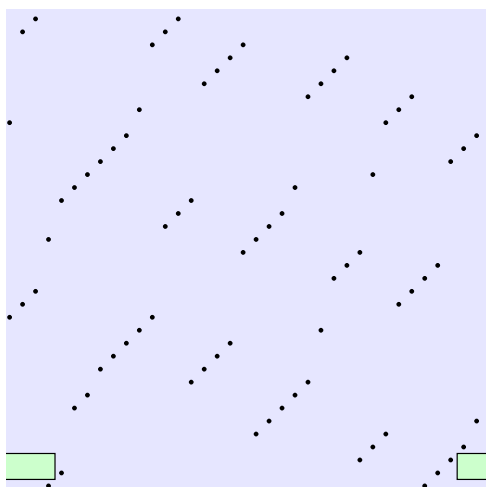

576.  $(34, 1, 26, 2)$

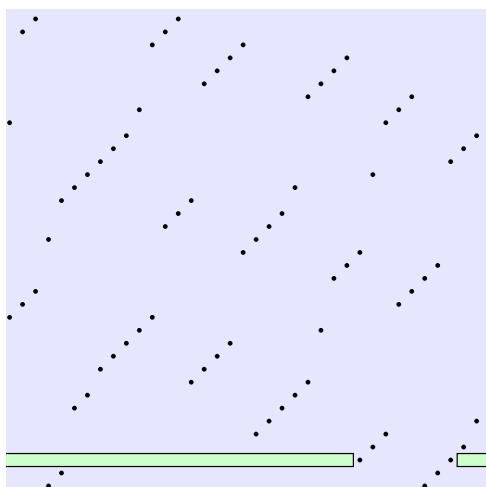



577. (34, 3, 35, 25)

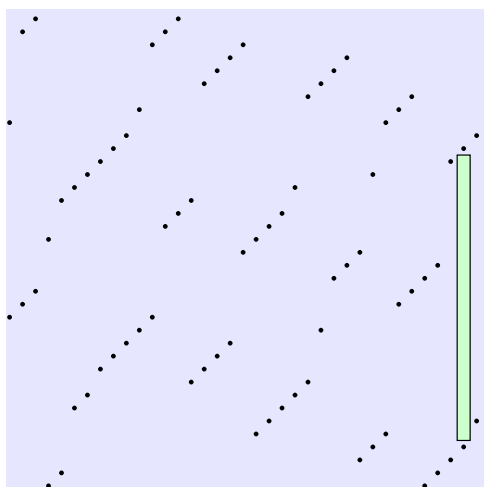

578. (34, 5, 36, 25)

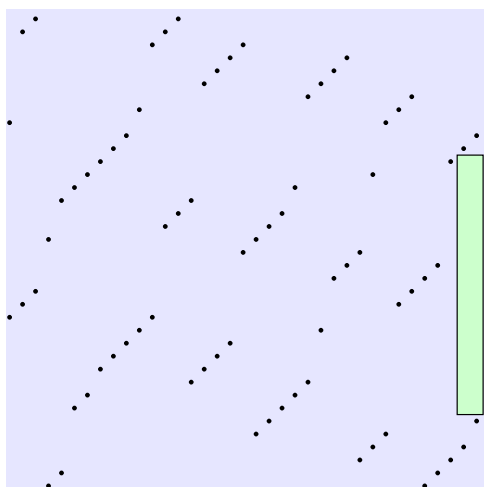

579. (34, 13, 0, 25)

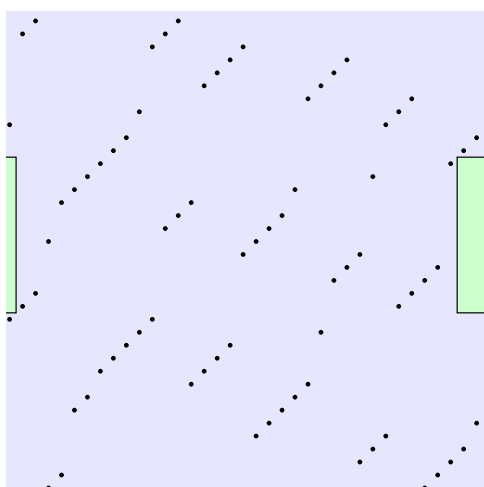

580. (34, 14, 1, 25)

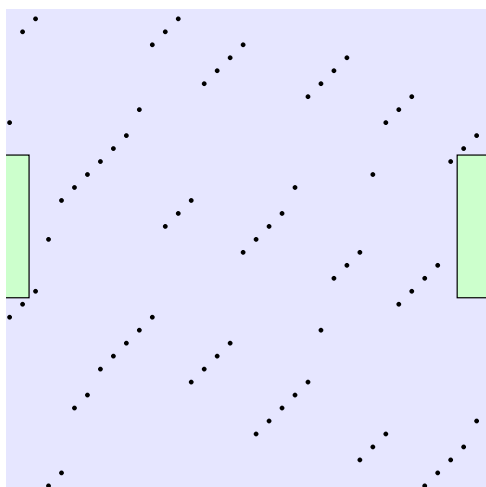

581. (34, 15, 2, 25)

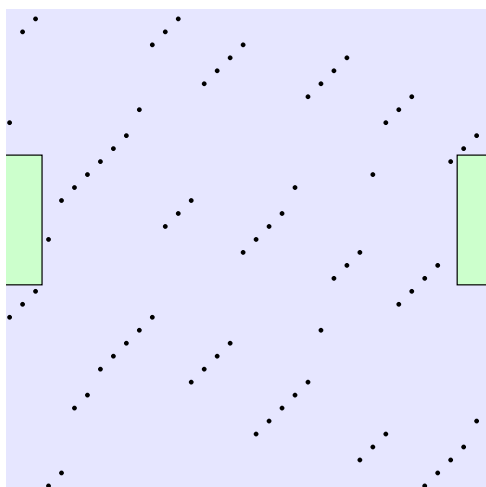

582. (34, 19, 3, 25)

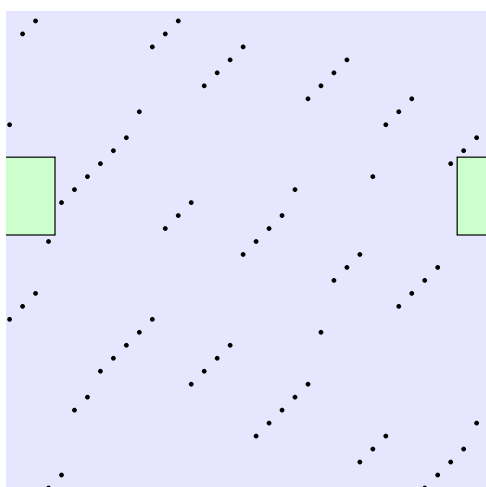

583. (34, 22, 4, 25)

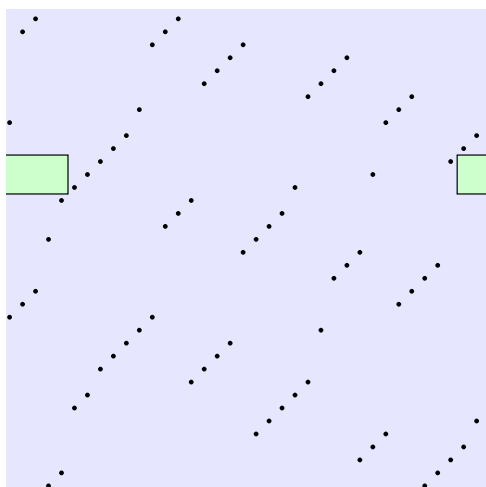

584. (34, 23, 5, 25)

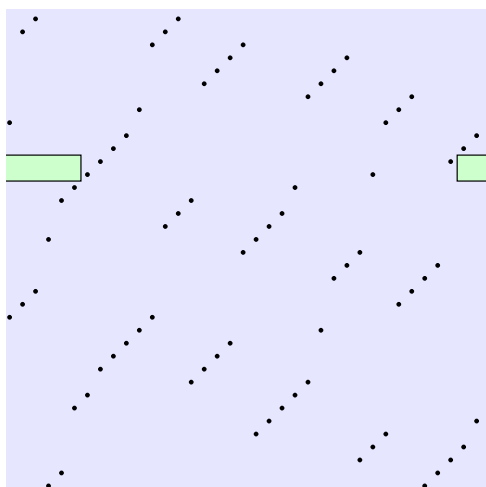

585. (34, 24, 6, 25)

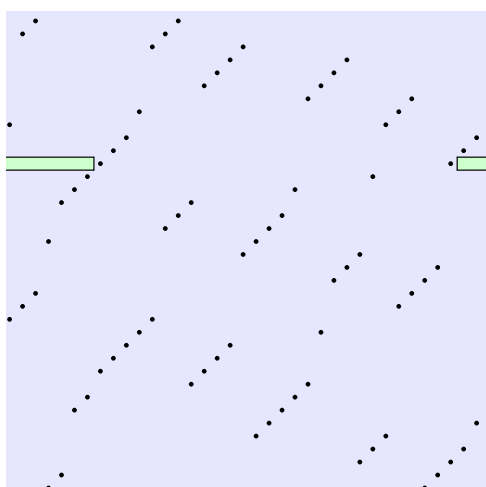

586. (34, 26, 35, 2)

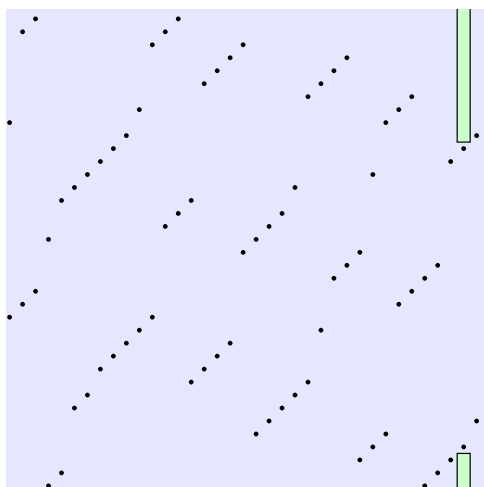

587. (34, 27, 36, 2)

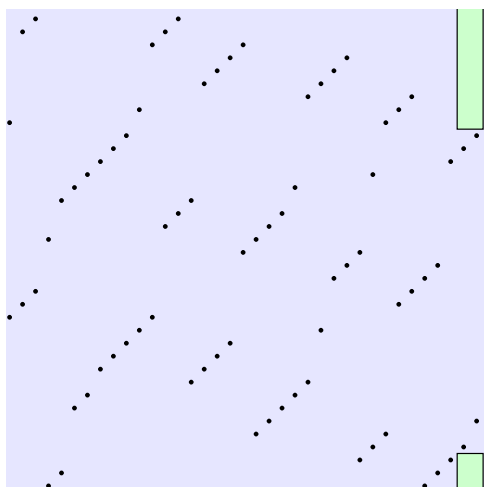

588. (34, 28, 0, 2)

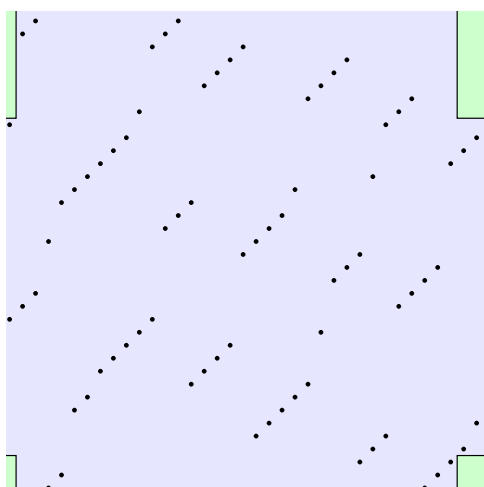

589. (34, 35, 1, 2)

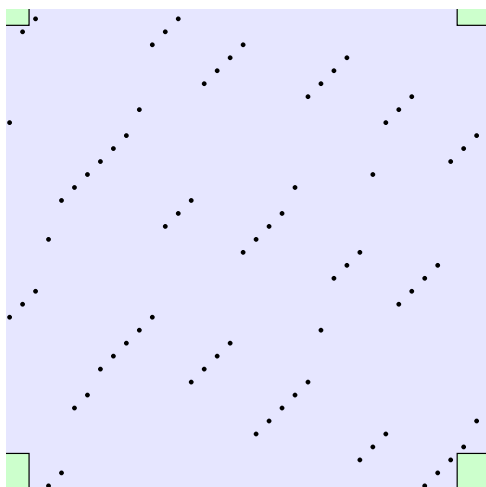

590. (34, 36, 2, 2)

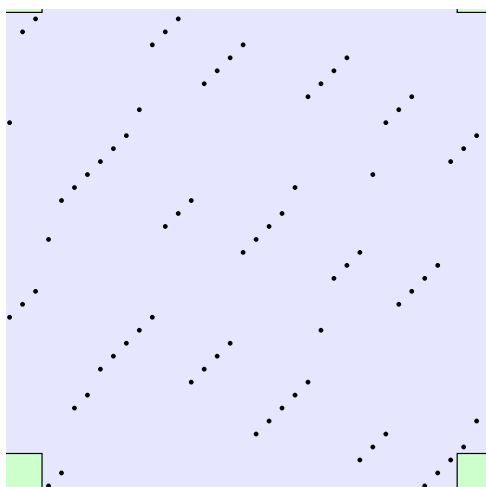

591. (35, 0, 3, 4)

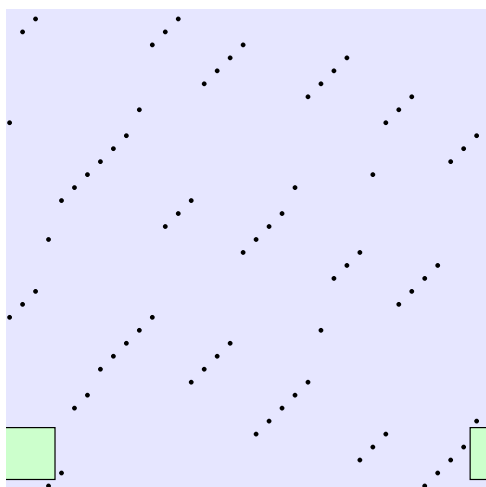

592. (35, 1, 18, 4)

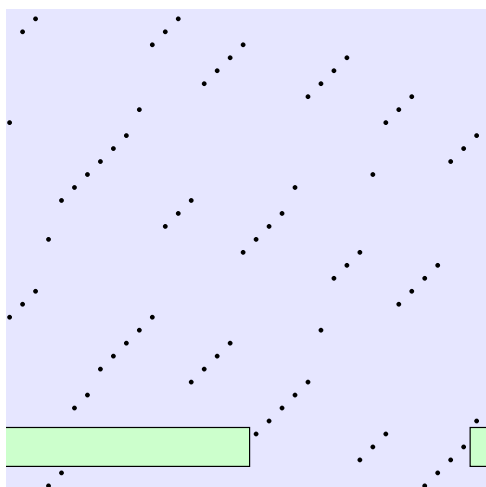

593. (35, 1, 26, 3)

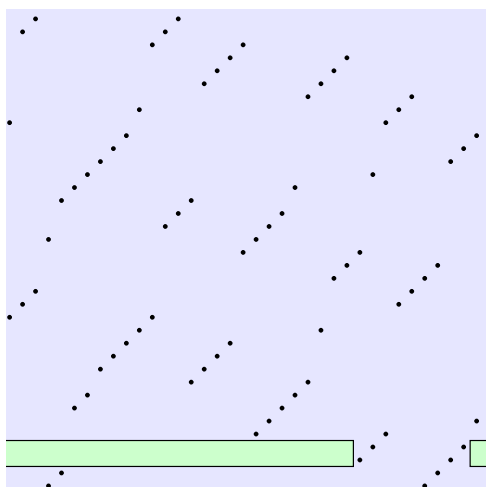

594. (35, 2, 27, 3)

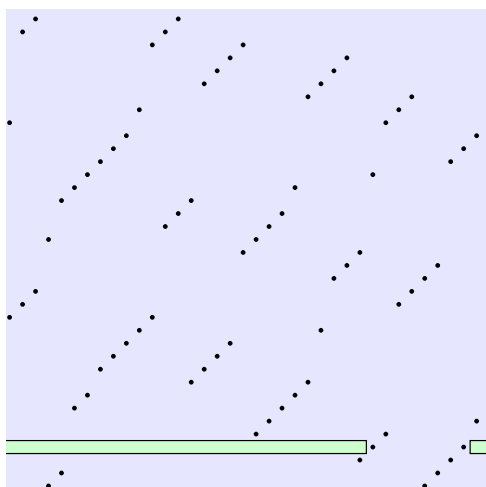

595. (35, 5, 36, 26)

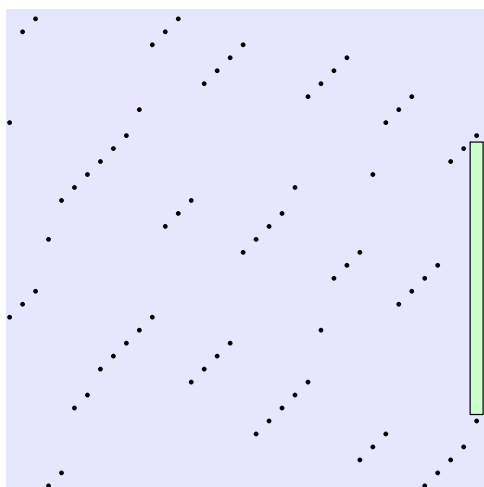

596. (35, 13, 0, 26)

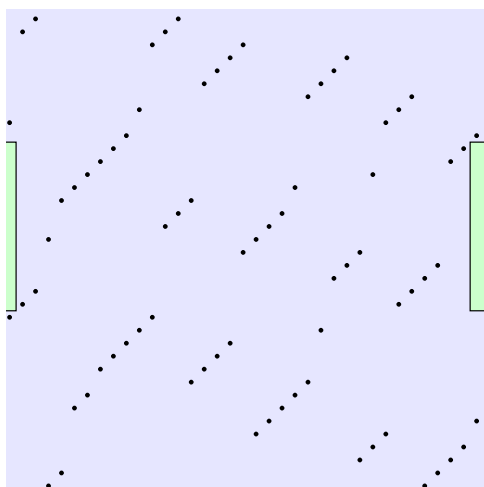

597. (35, 14, 1, 26)

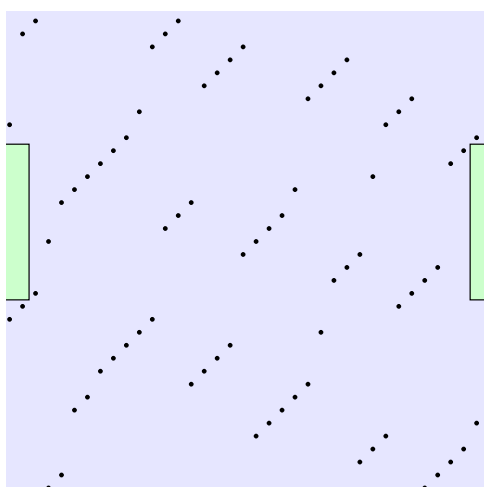

598. (35, 15, 2, 26)

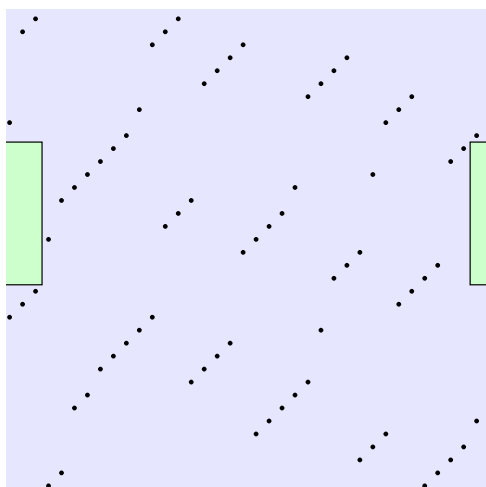

599. (35, 19, 3, 26)

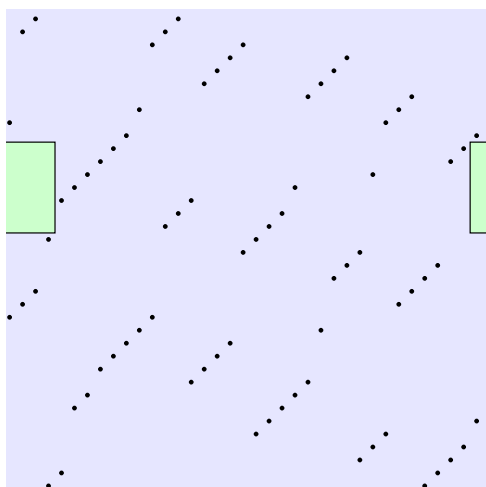

600. (35, 22, 4, 26)

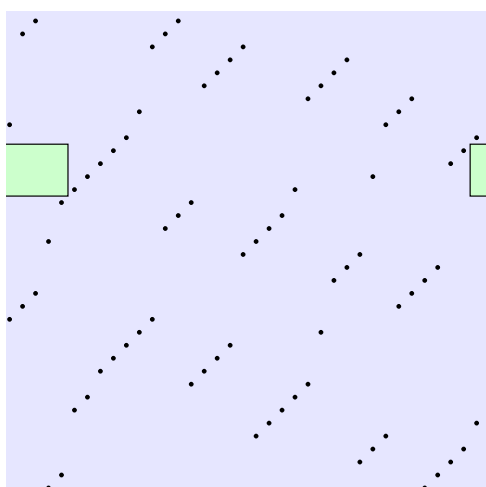



601. (35, 23, 5, 26)

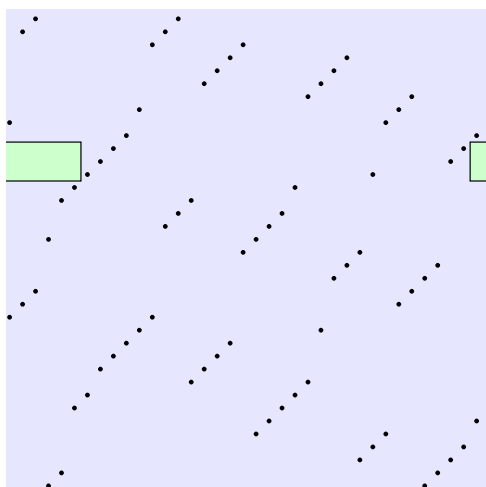

602. (35, 24, 6, 26)

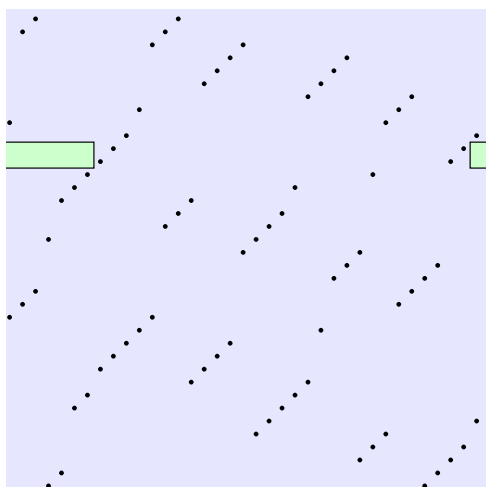

603. (35, 25, 7, 26)

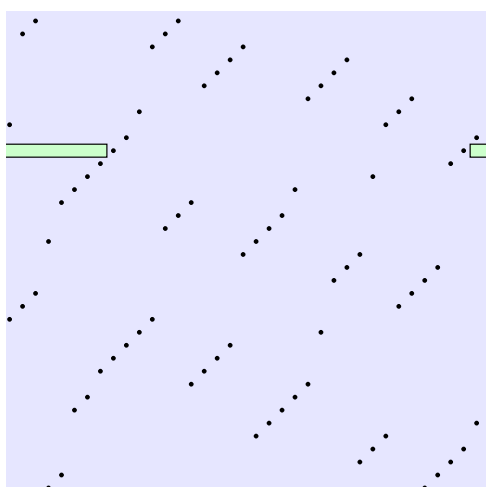

604. (35, 27, 36, 4)

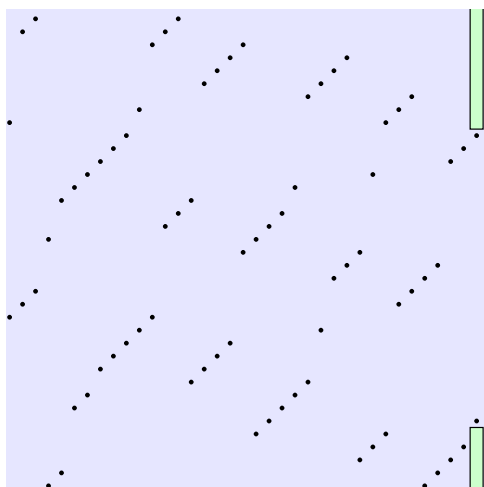

605. (35, 28, 0, 4)

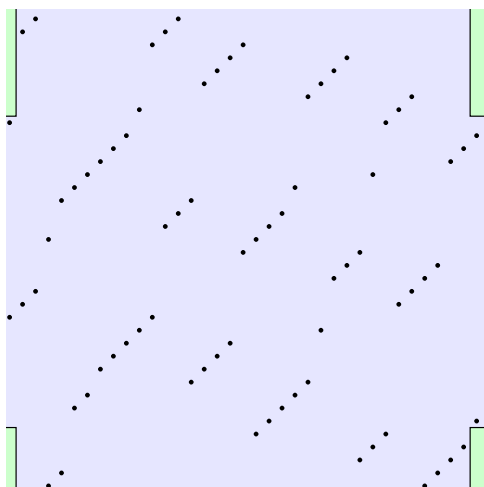

606. (35, 35, 1, 4)

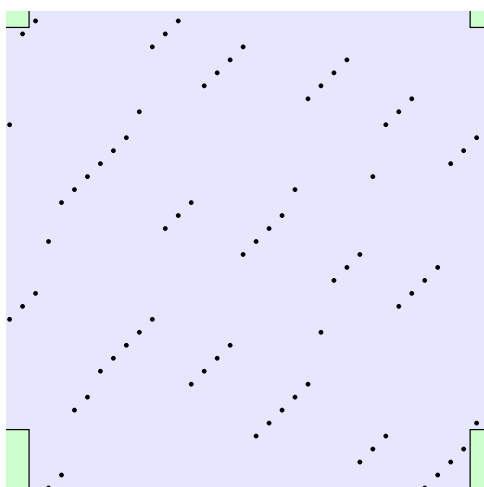

607. (35, 36, 2, 4)

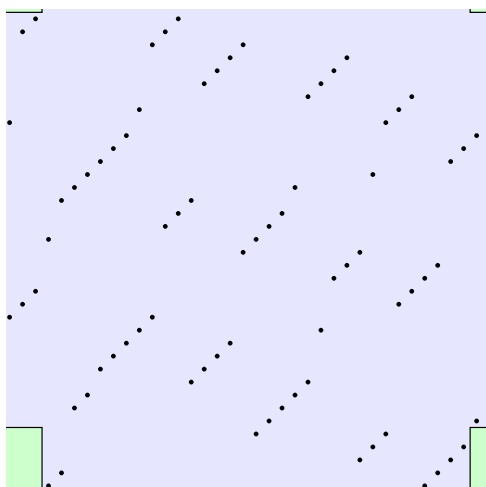

608. (36, 0, 3, 12)

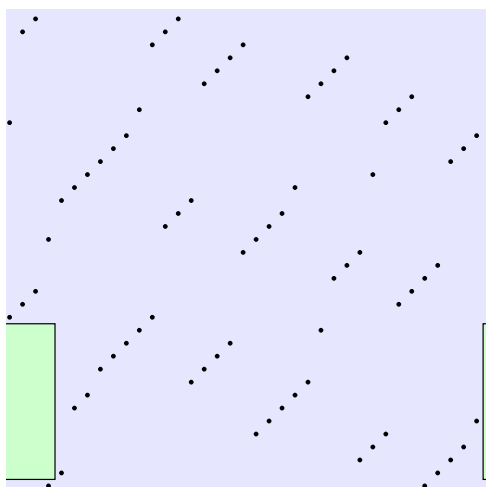

609. (36, 1, 4, 12)

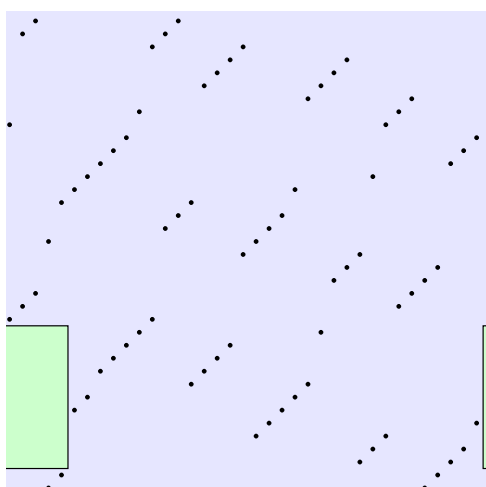

610.  $(36, 1, 18, 5)$

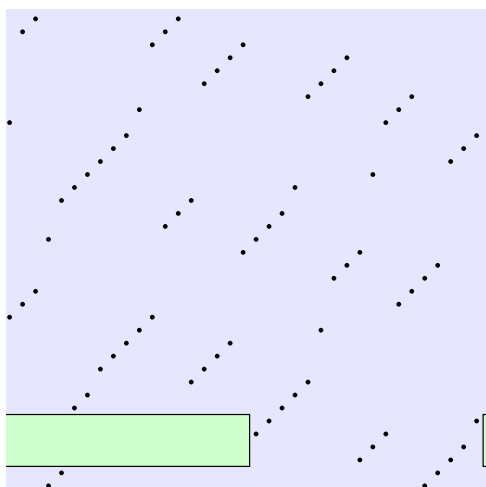

611.  $(36, 4, 19, 5)$

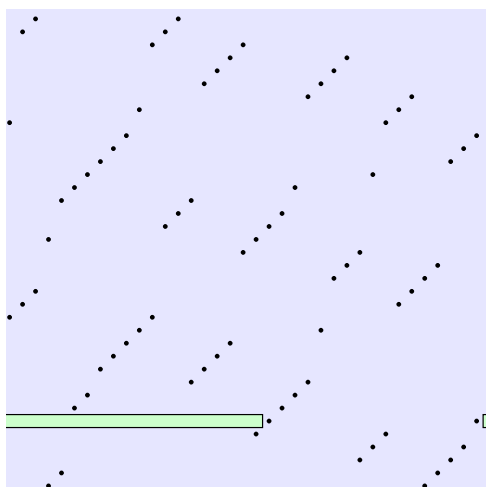

612.  $(36, 13, 0, 27)$

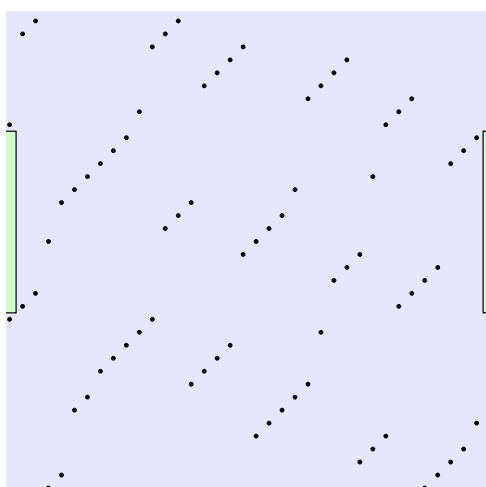

613. (36, 14, 1, 27)

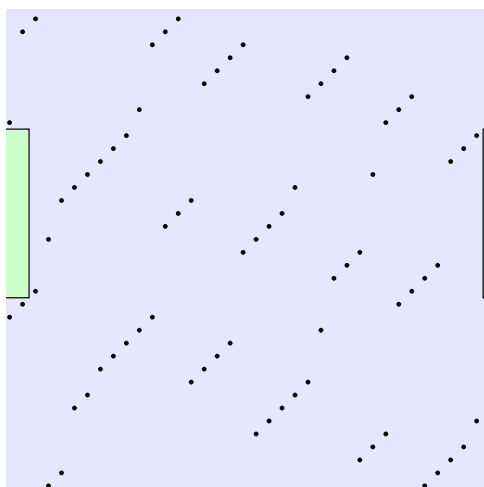

614. (36, 15, 2, 27)

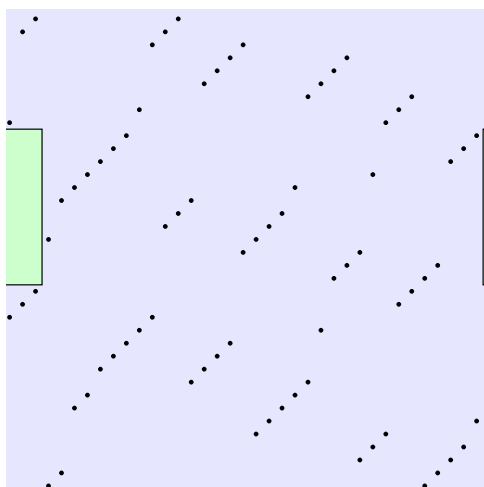

615. (36, 19, 3, 27)

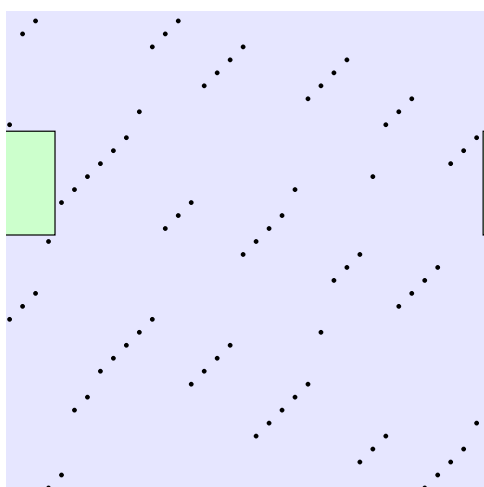

616. (36, 22, 4, 27)

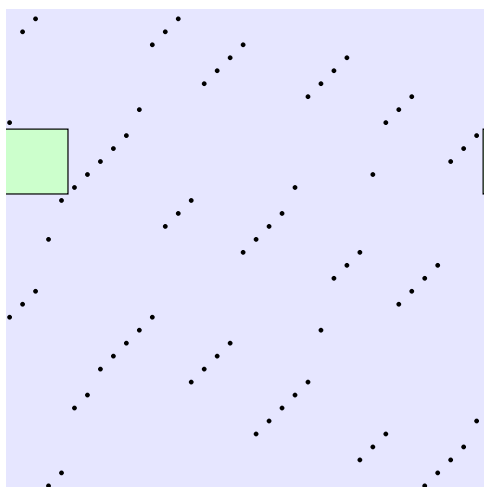

617. (36, 23, 5, 27)

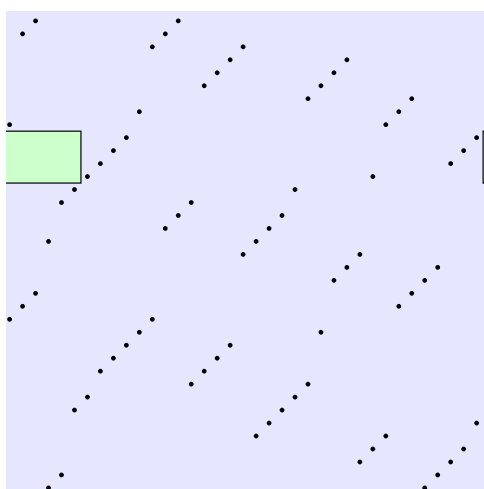

618. (36, 24, 6, 27)

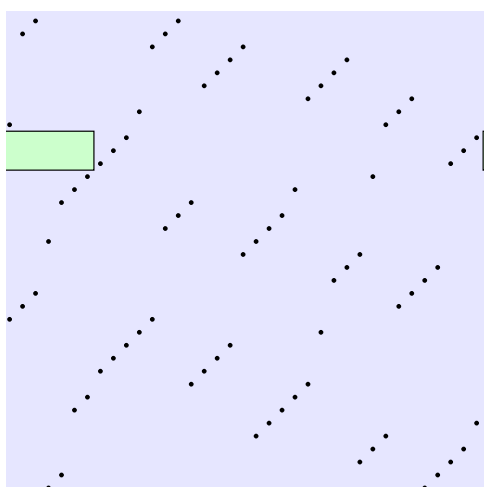

619. (36, 25, 7, 27)

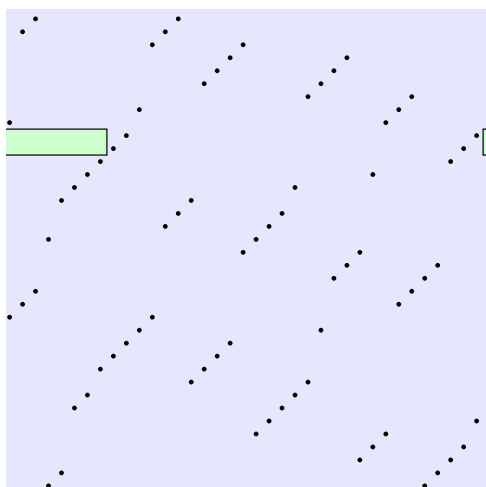

620. (36, 26, 8, 27)

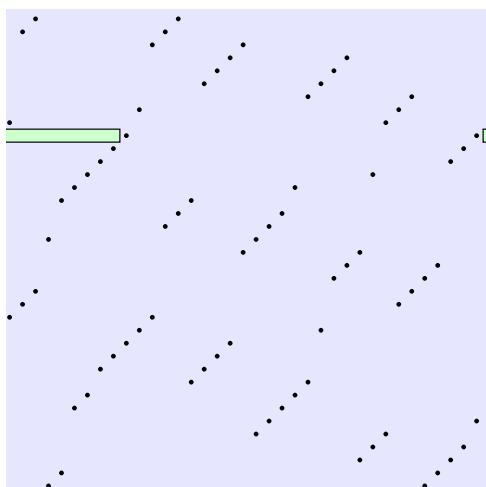

621. (36, 28, 0, 12)

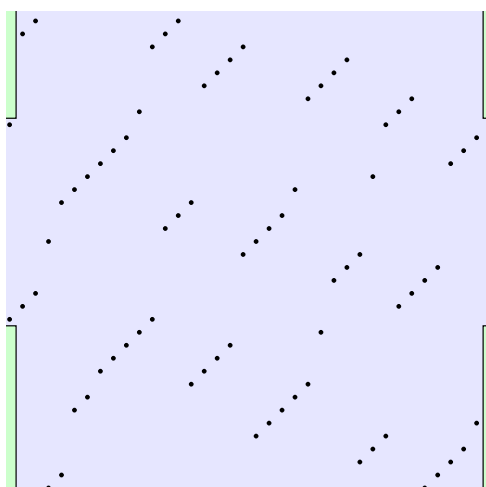

622.  $(36, 35, 1, 12)$

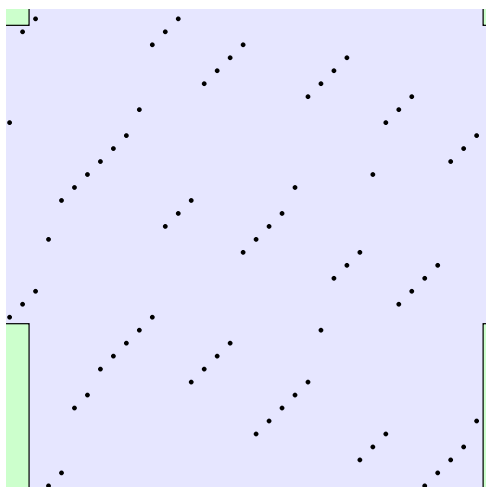

623.  $(36, 36, 2, 12)$

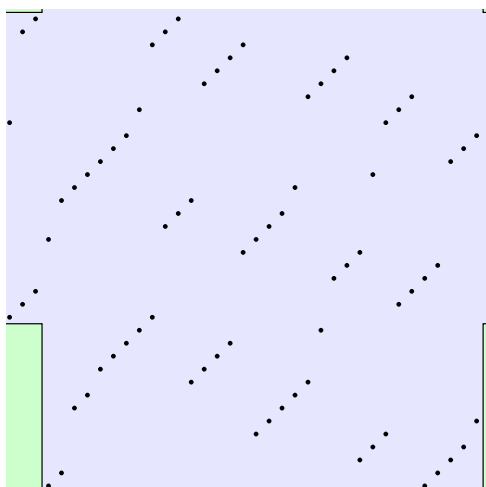

Supplement: Supplementary file 2 [file max-types.pdf]
